# Supplementary material for: Separating signal from combinatorial jets in a high background environment
Source: arXiv:2301.09148 source file (2023-07-31)
Supplement: Supplementary file 1 [file appendix.tex]

\clearpage
\subsection{Area vs. Jet Width}
\begin{figure*}
    \centering
    \includegraphics[width=\linewidth]{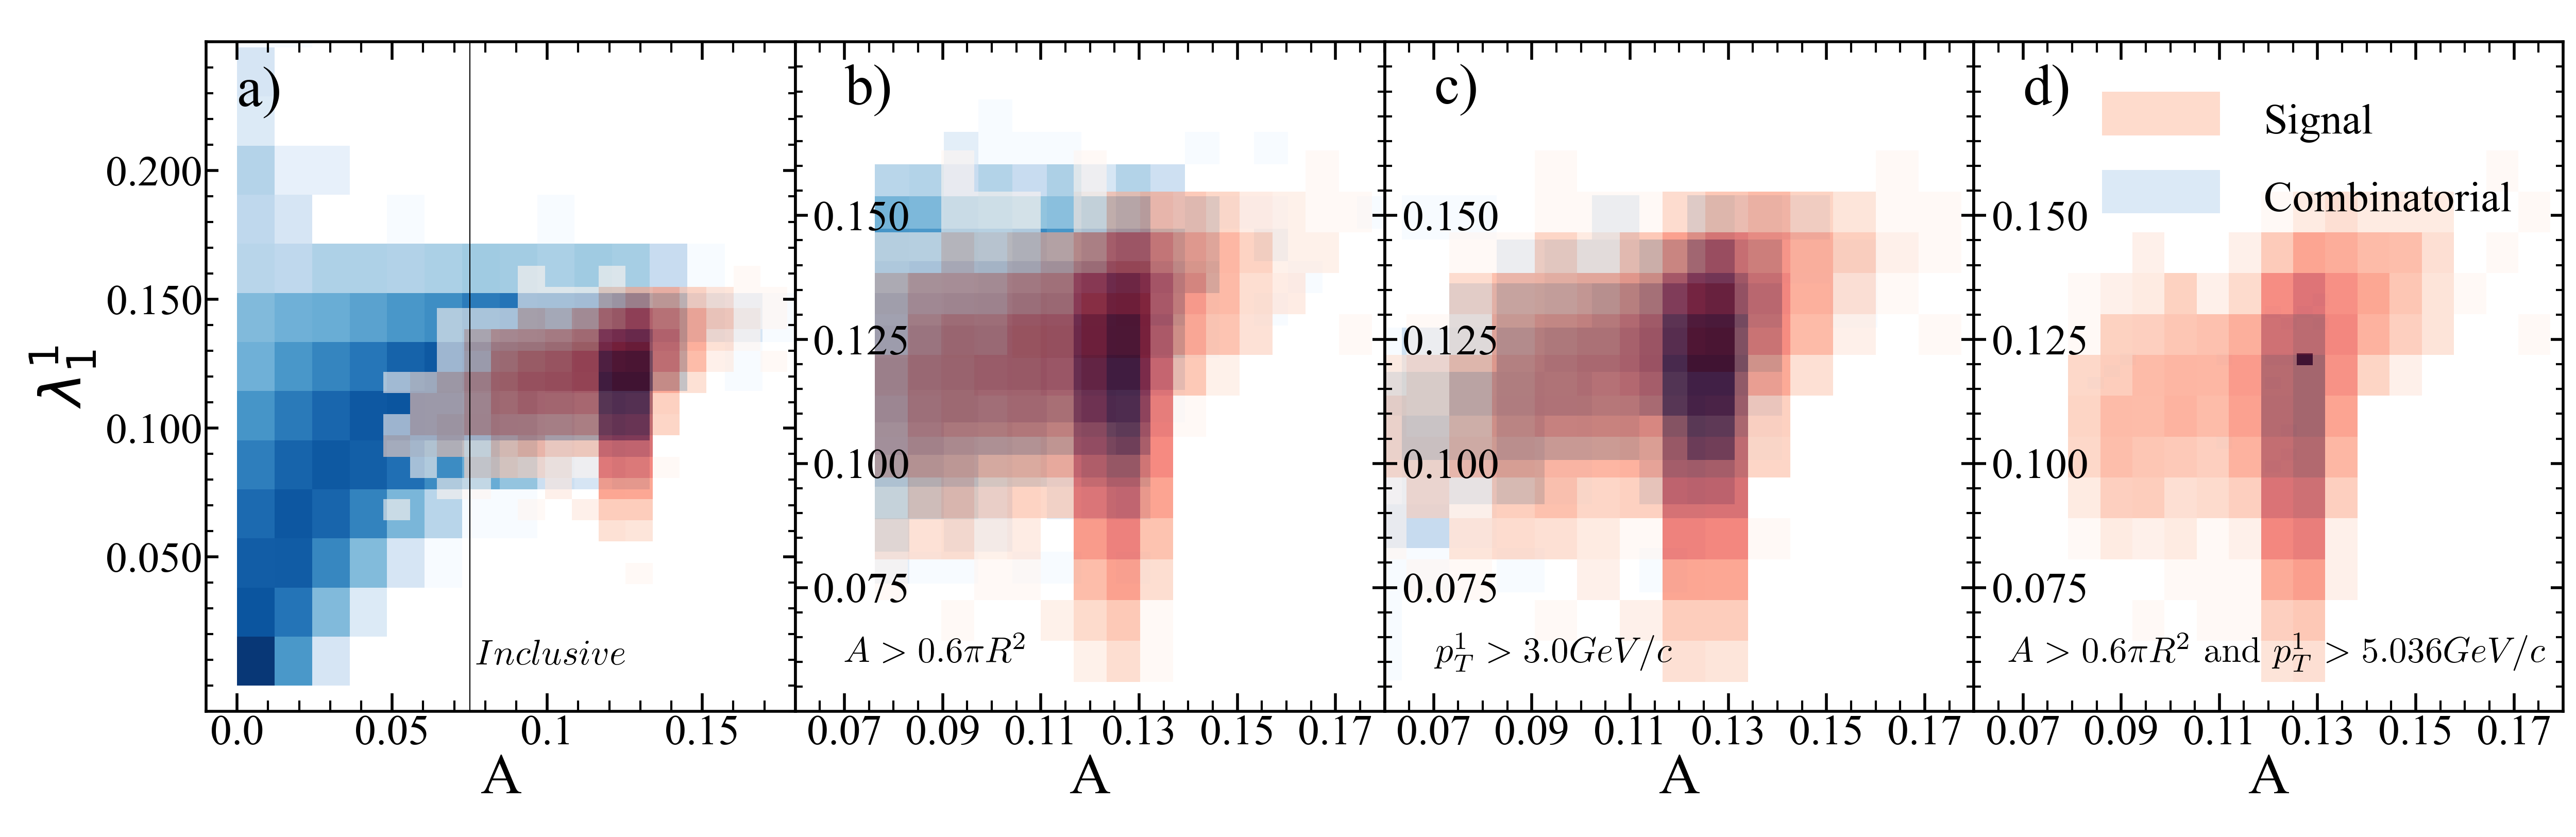}
    \caption{R=0.2 \ptH=10 \GeV}
    \label{fig:blob_02_10}
\end{figure*}

\begin{figure*}
    \centering
    \includegraphics[width=\linewidth]{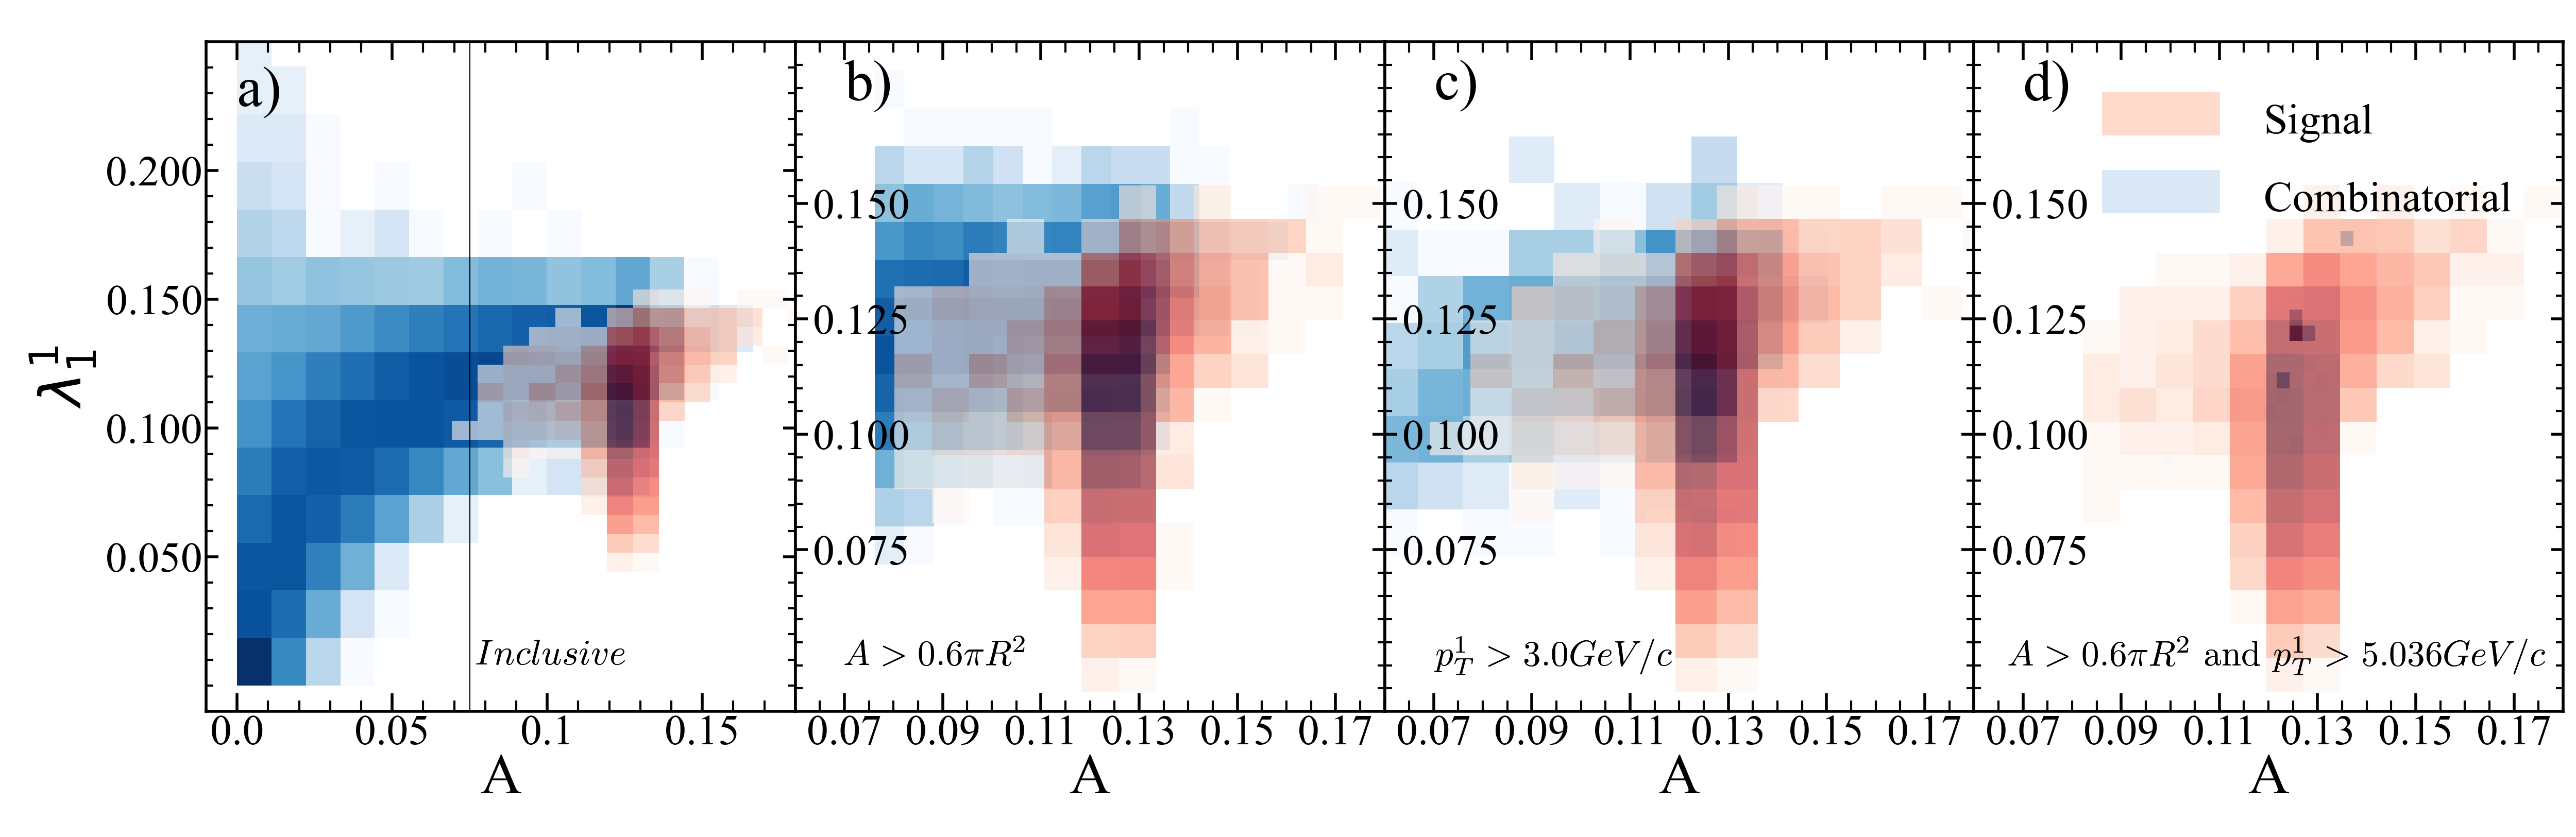}
    \caption{R=0.2 \ptH=20 \GeV}
    \label{fig:blob_02_20}
\end{figure*}

\begin{figure*}
    \centering
    \includegraphics[width=\linewidth]{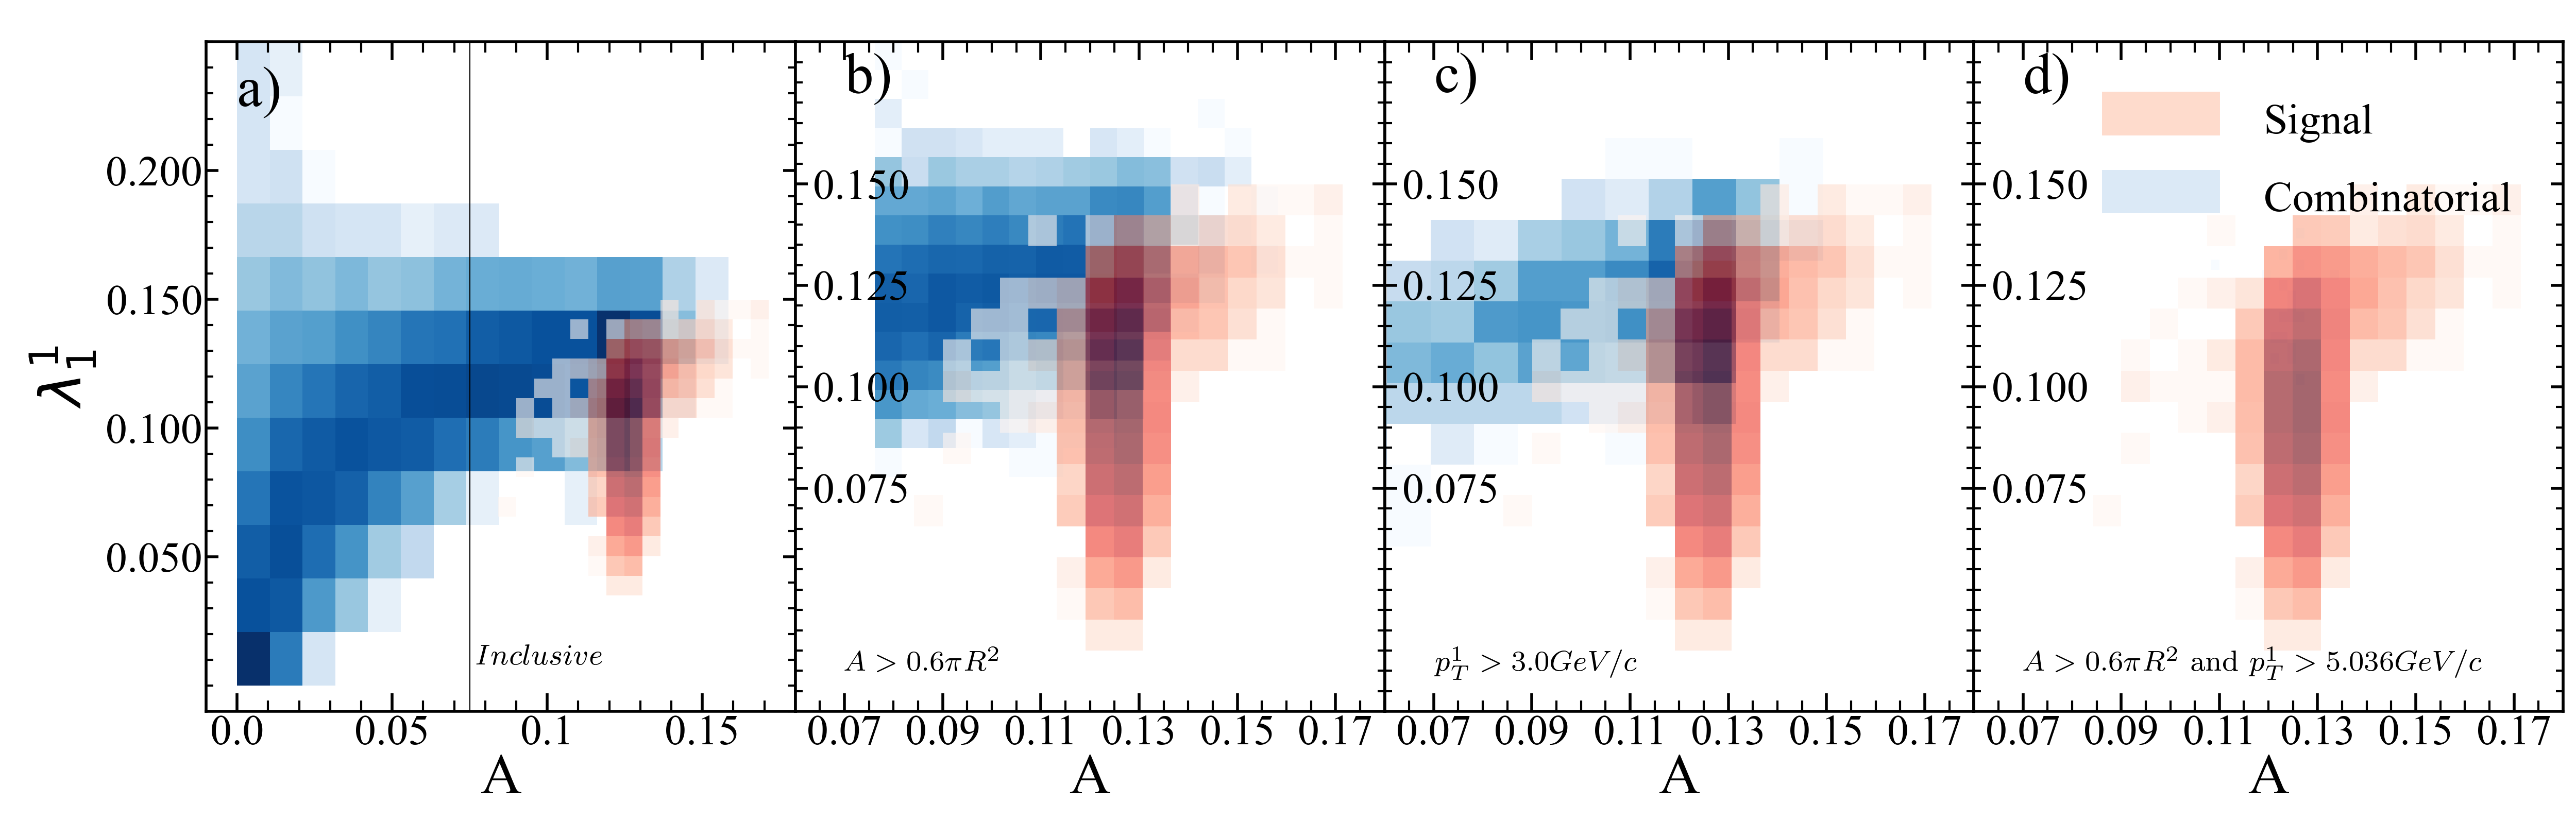}
    \caption{R=0.2 \ptH=30 \GeV}
    \label{fig:blob_02_30}
\end{figure*}

\begin{figure*}
    \centering
    \includegraphics[width=\linewidth]{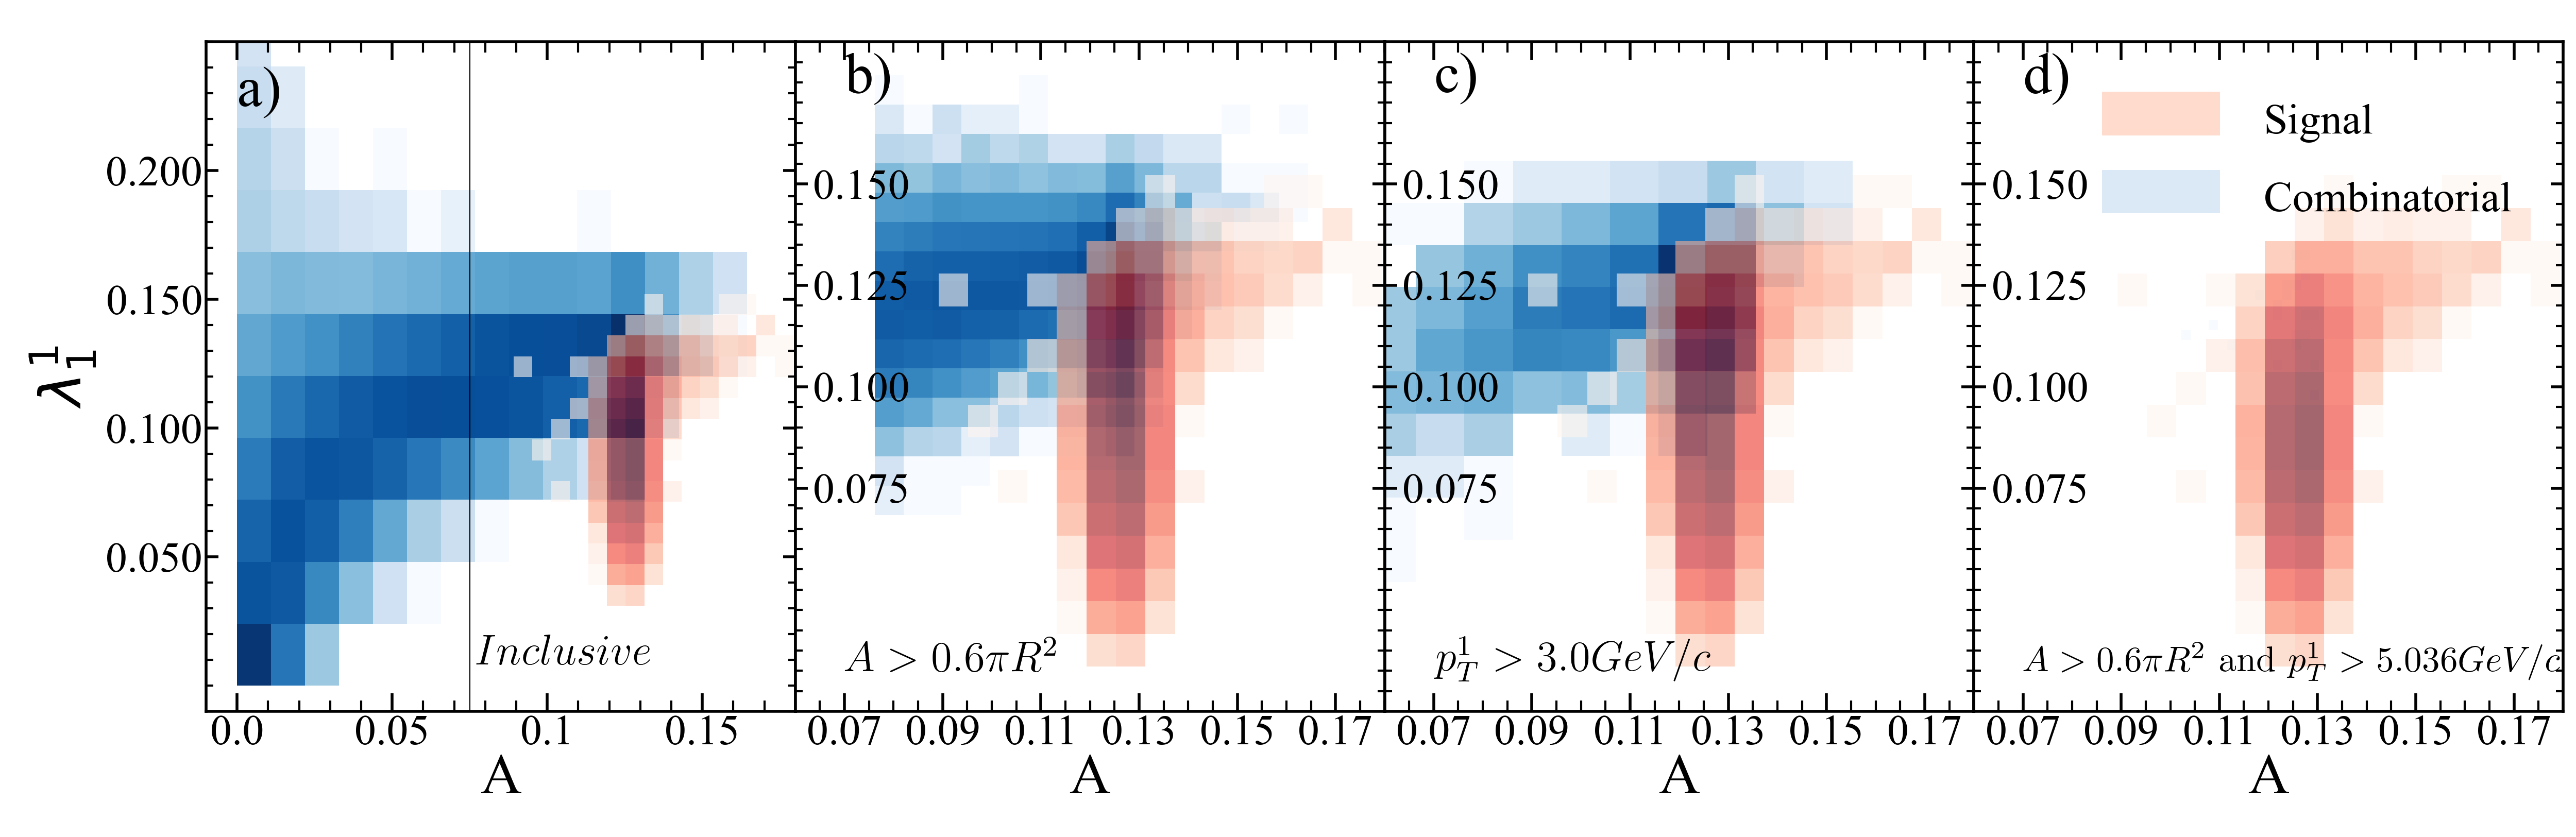}
    \caption{R=0.2 \ptH=40 \GeV}
    \label{fig:blob_02_40}
\end{figure*}

\begin{figure*}
    \centering
    \includegraphics[width=\linewidth]{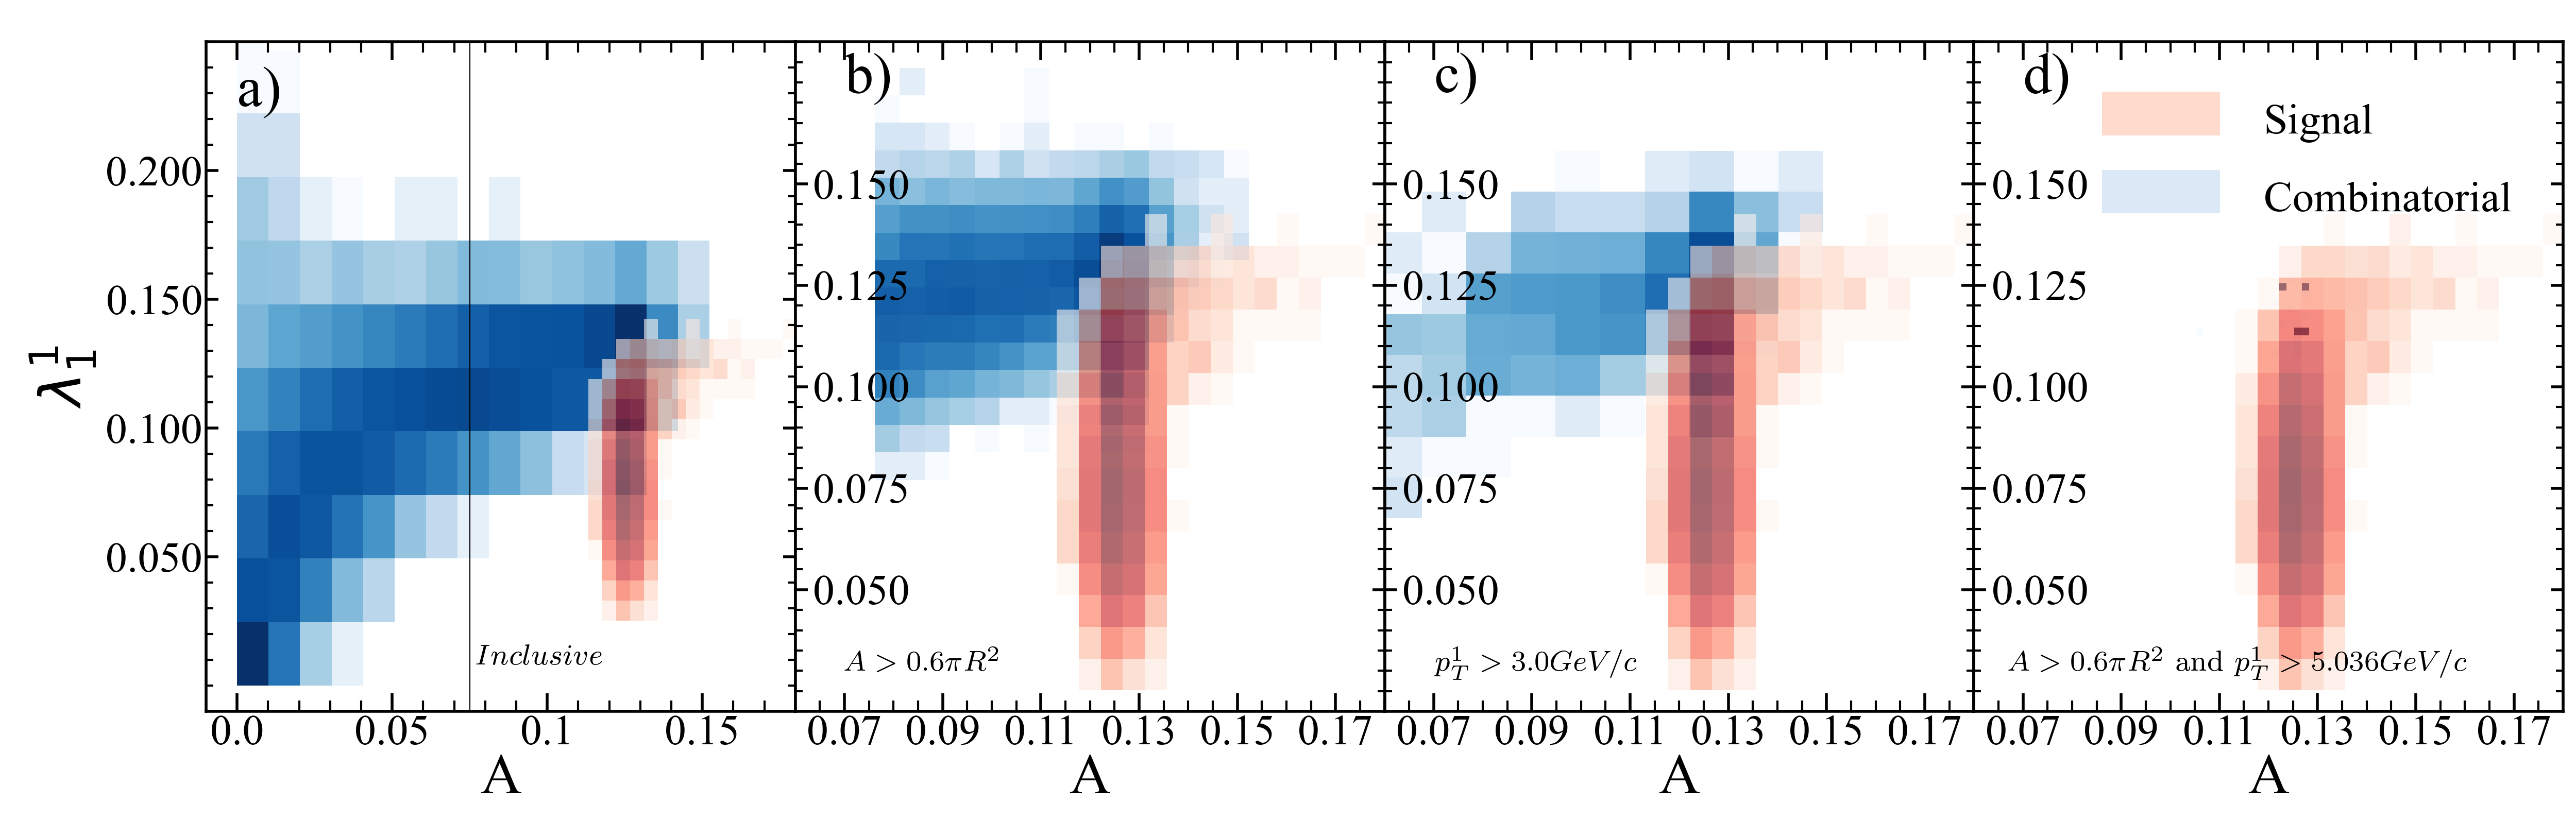}
    \caption{R=0.2 \ptH=60 \GeV}
    \label{fig:blob_02_60}
\end{figure*}

\begin{figure*}
    \centering
    \includegraphics[width=\linewidth]{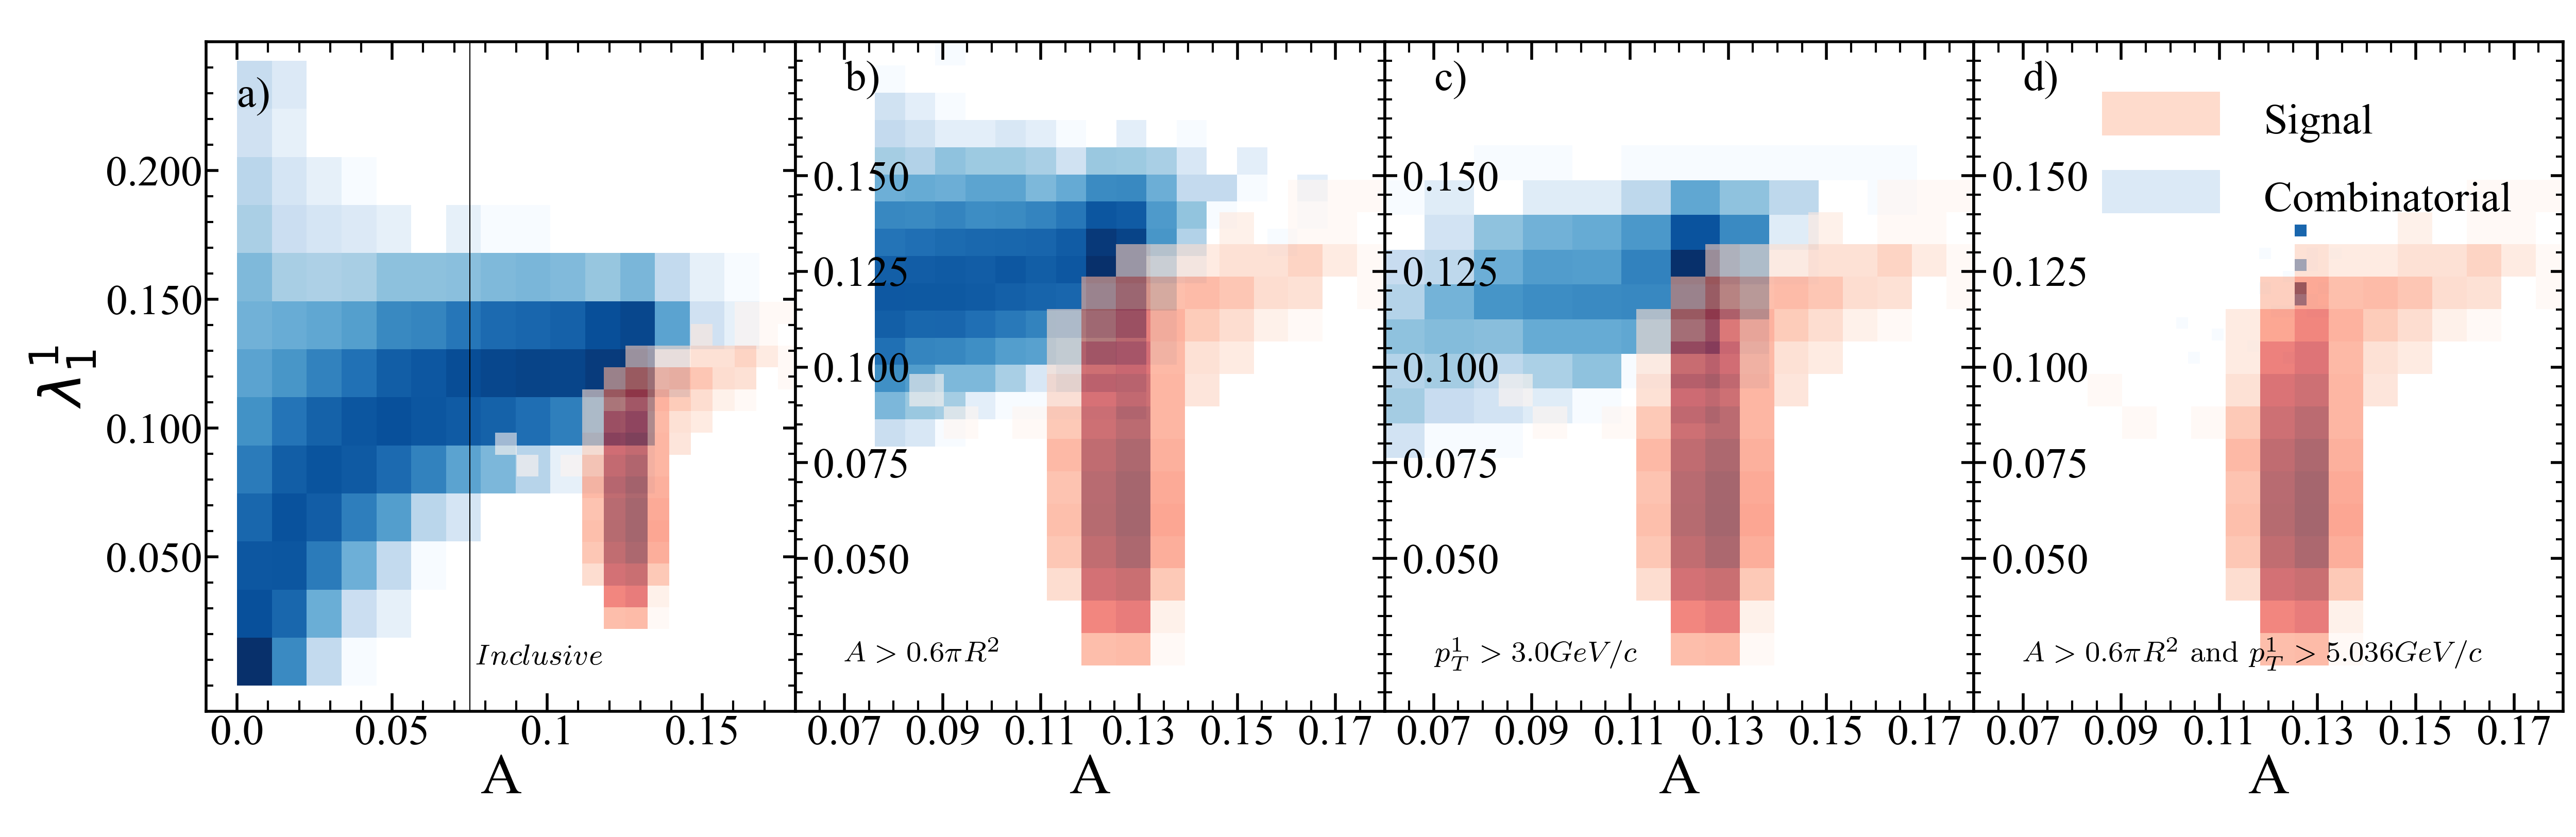}
    \caption{R=0.2 \ptH=80 \GeV}
    \label{fig:blob_02_80}
\end{figure*}

\begin{figure*}
    \centering
    \includegraphics[width=\linewidth]{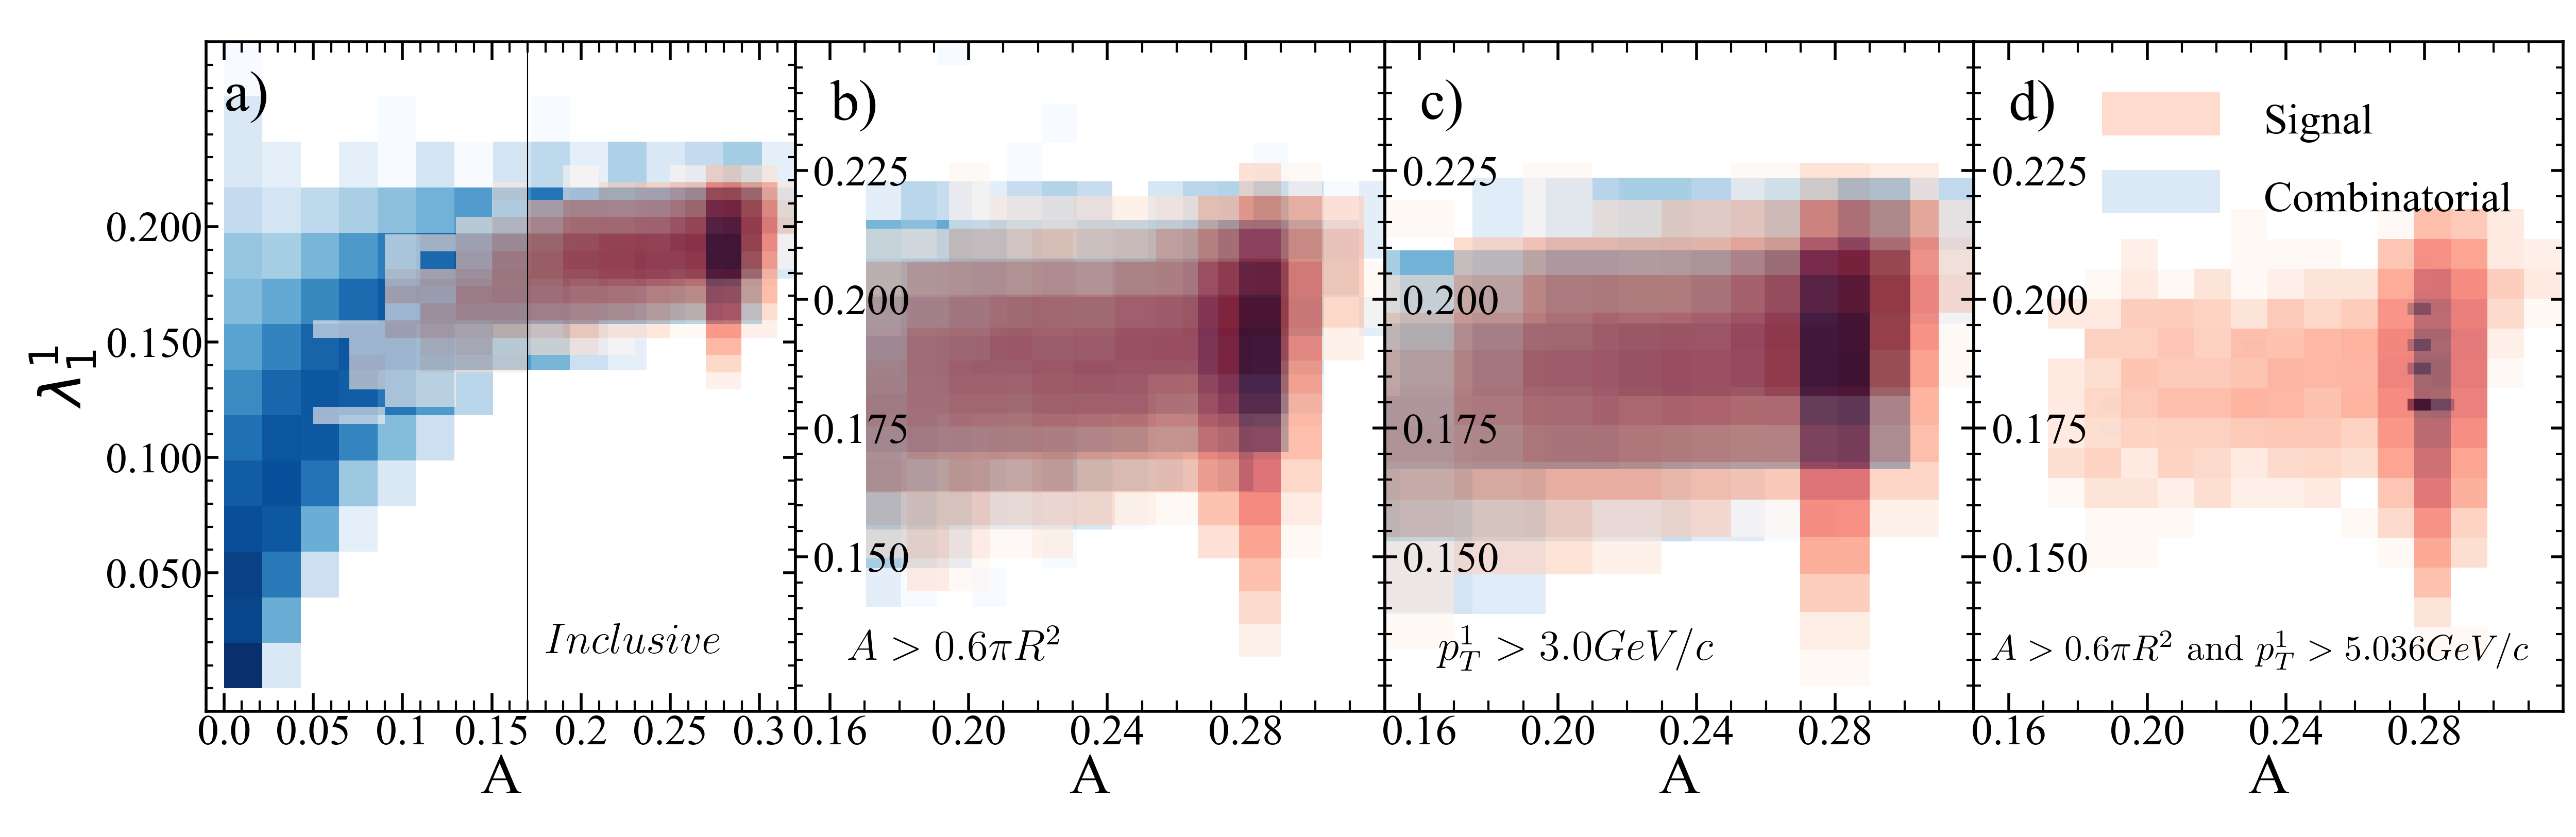}
    \caption{R=0.3 \ptH=10 \GeV}
    \label{fig:blob_03_10}
\end{figure*}

\begin{figure*}
    \centering
    \includegraphics[width=\linewidth]{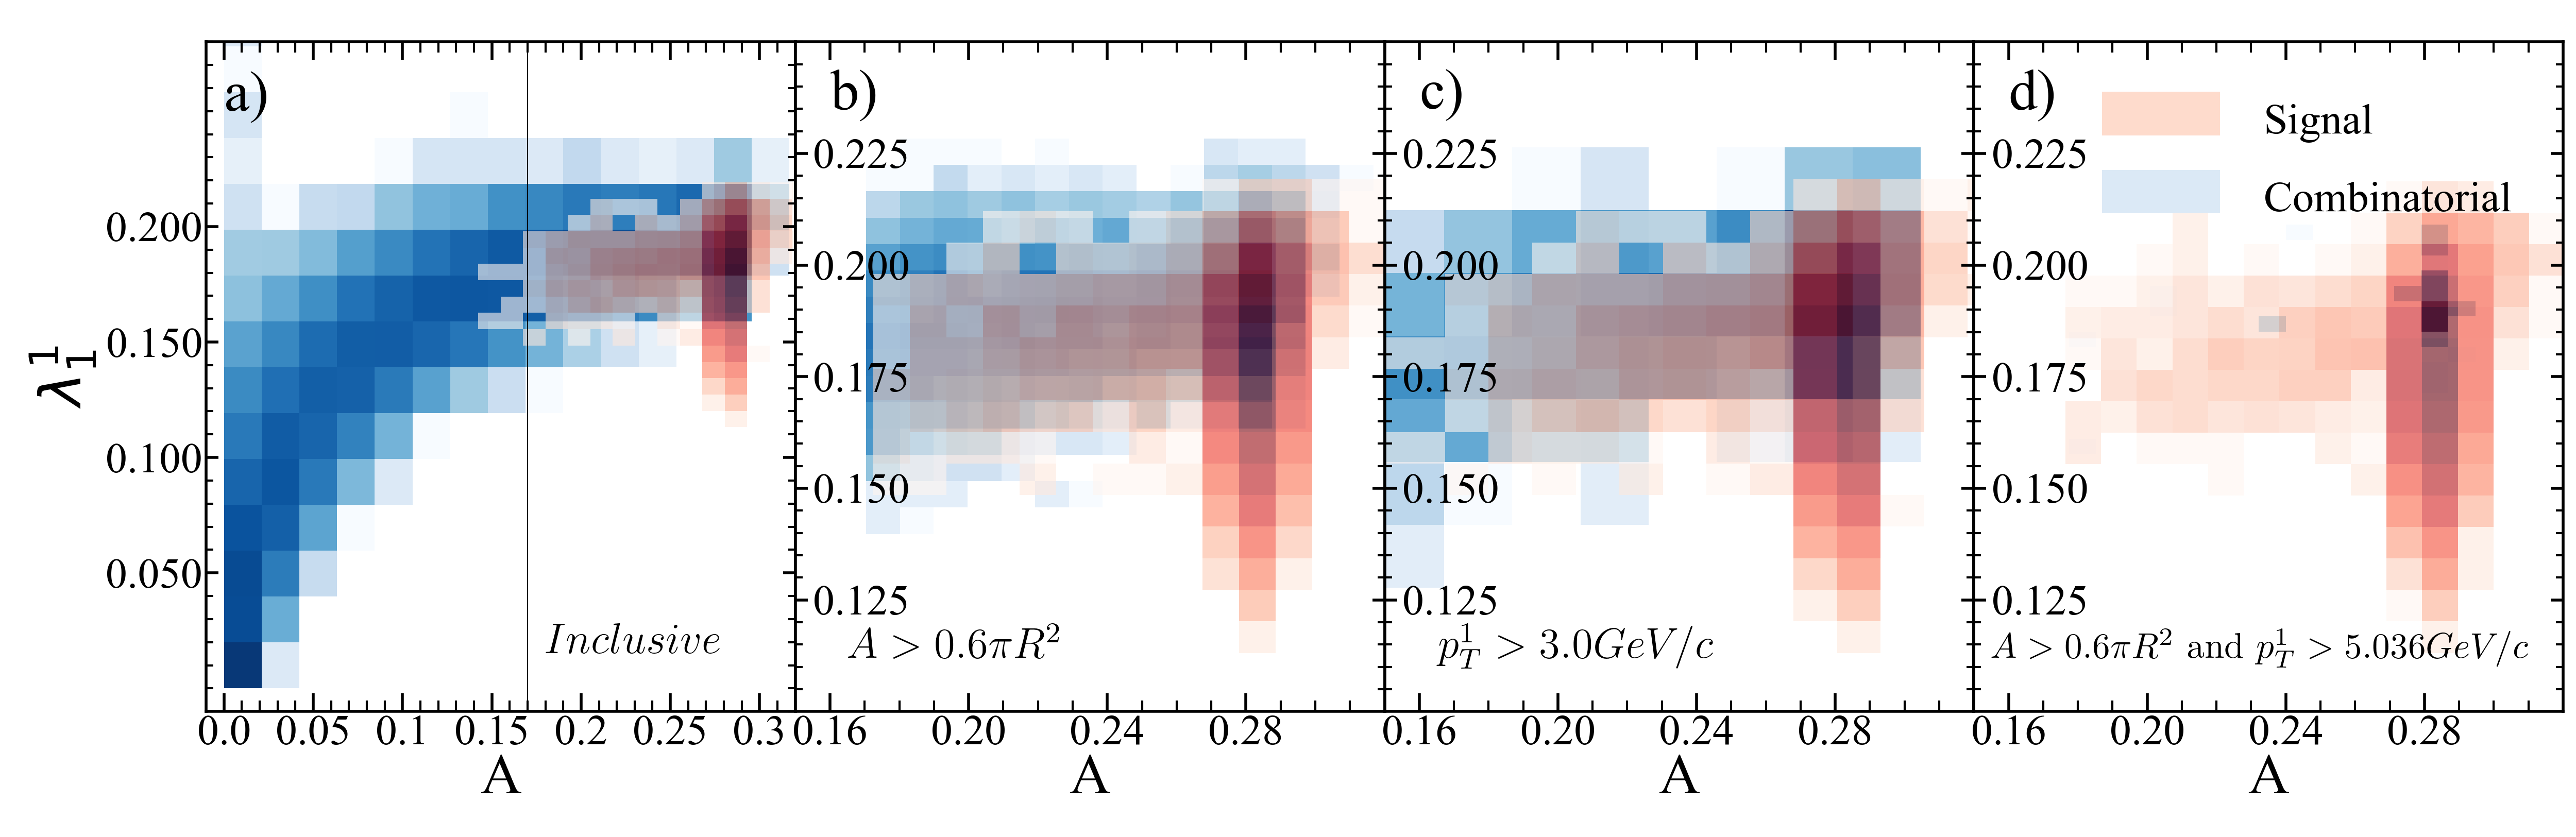}
    \caption{R=0.3 \ptH=20 \GeV}
    \label{fig:blob_03_20}
\end{figure*}

\begin{figure*}
    \centering
    \includegraphics[width=\linewidth]{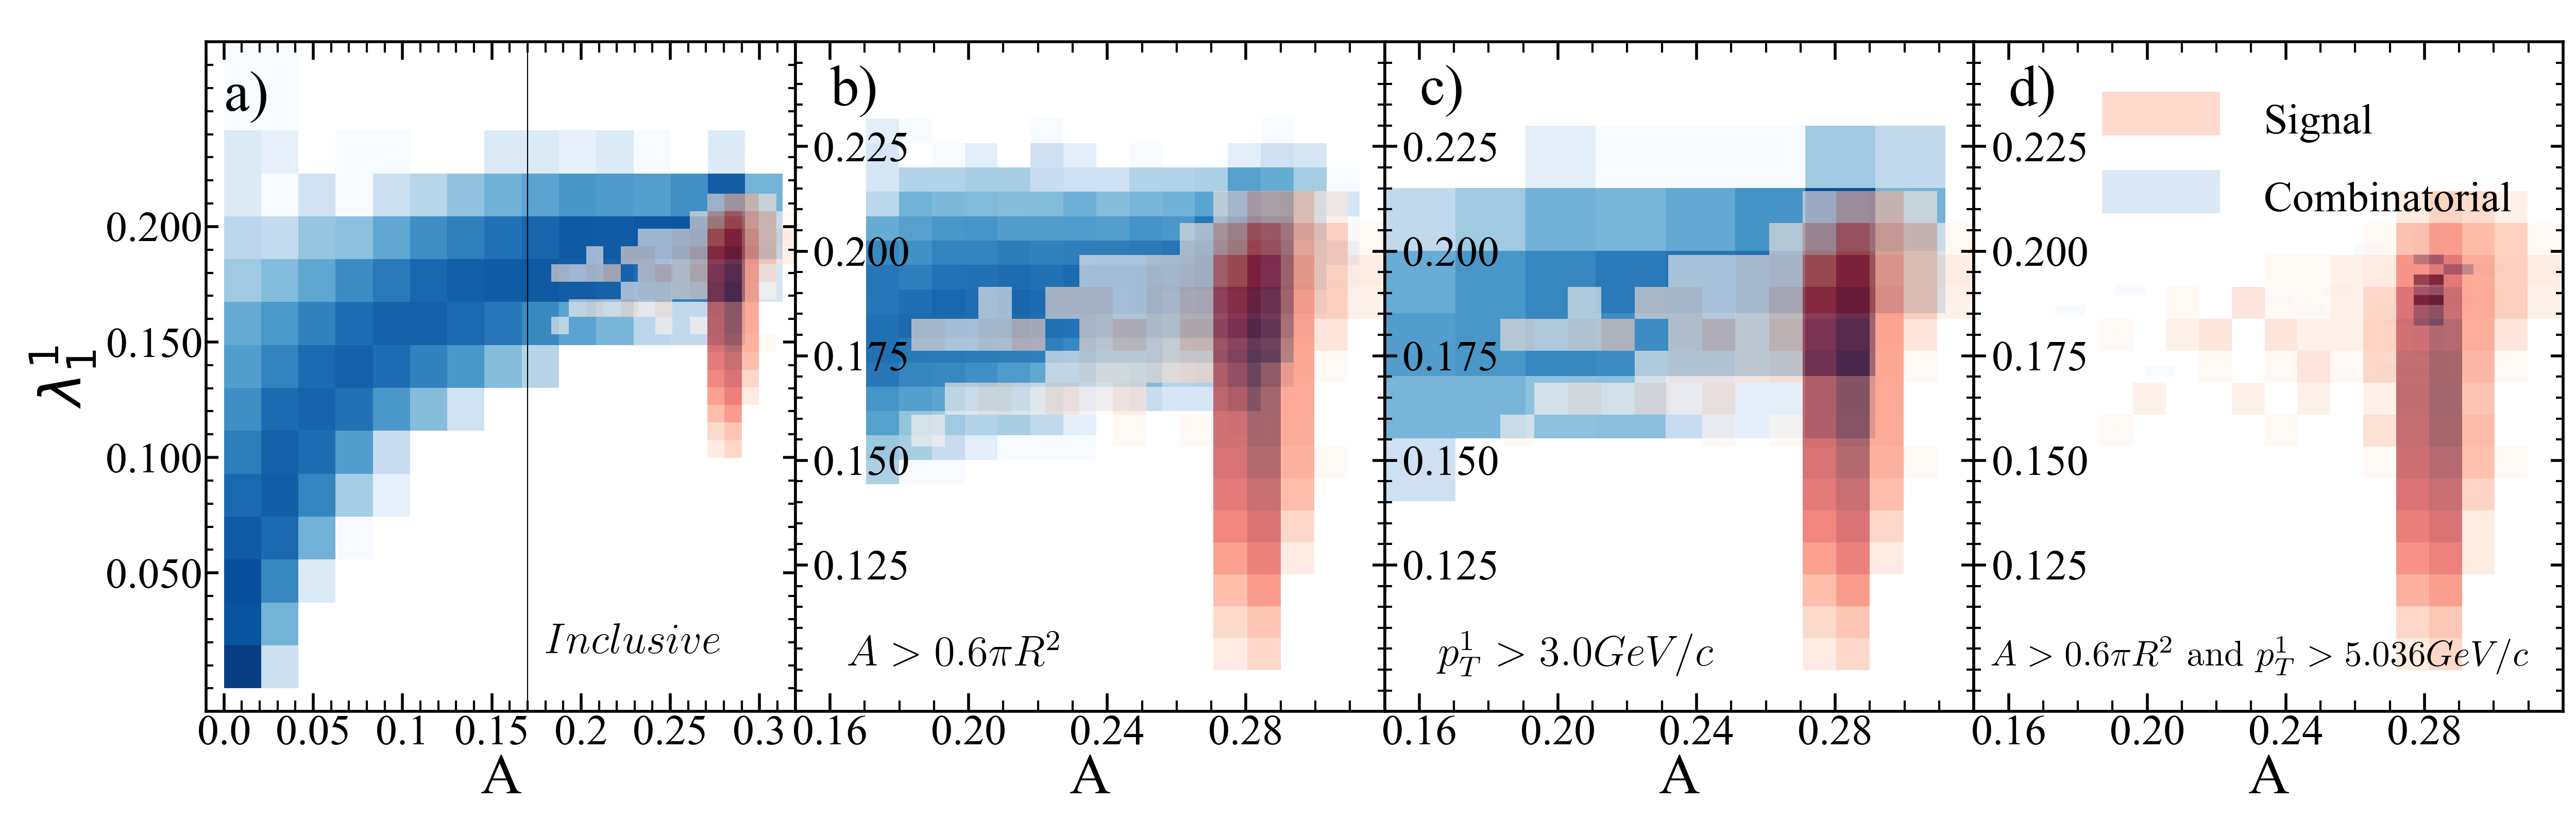}
    \caption{R=0.3 \ptH=30 \GeV}
    \label{fig:blob_03_30}
\end{figure*}

\begin{figure*}
    \centering
    \includegraphics[width=\linewidth]{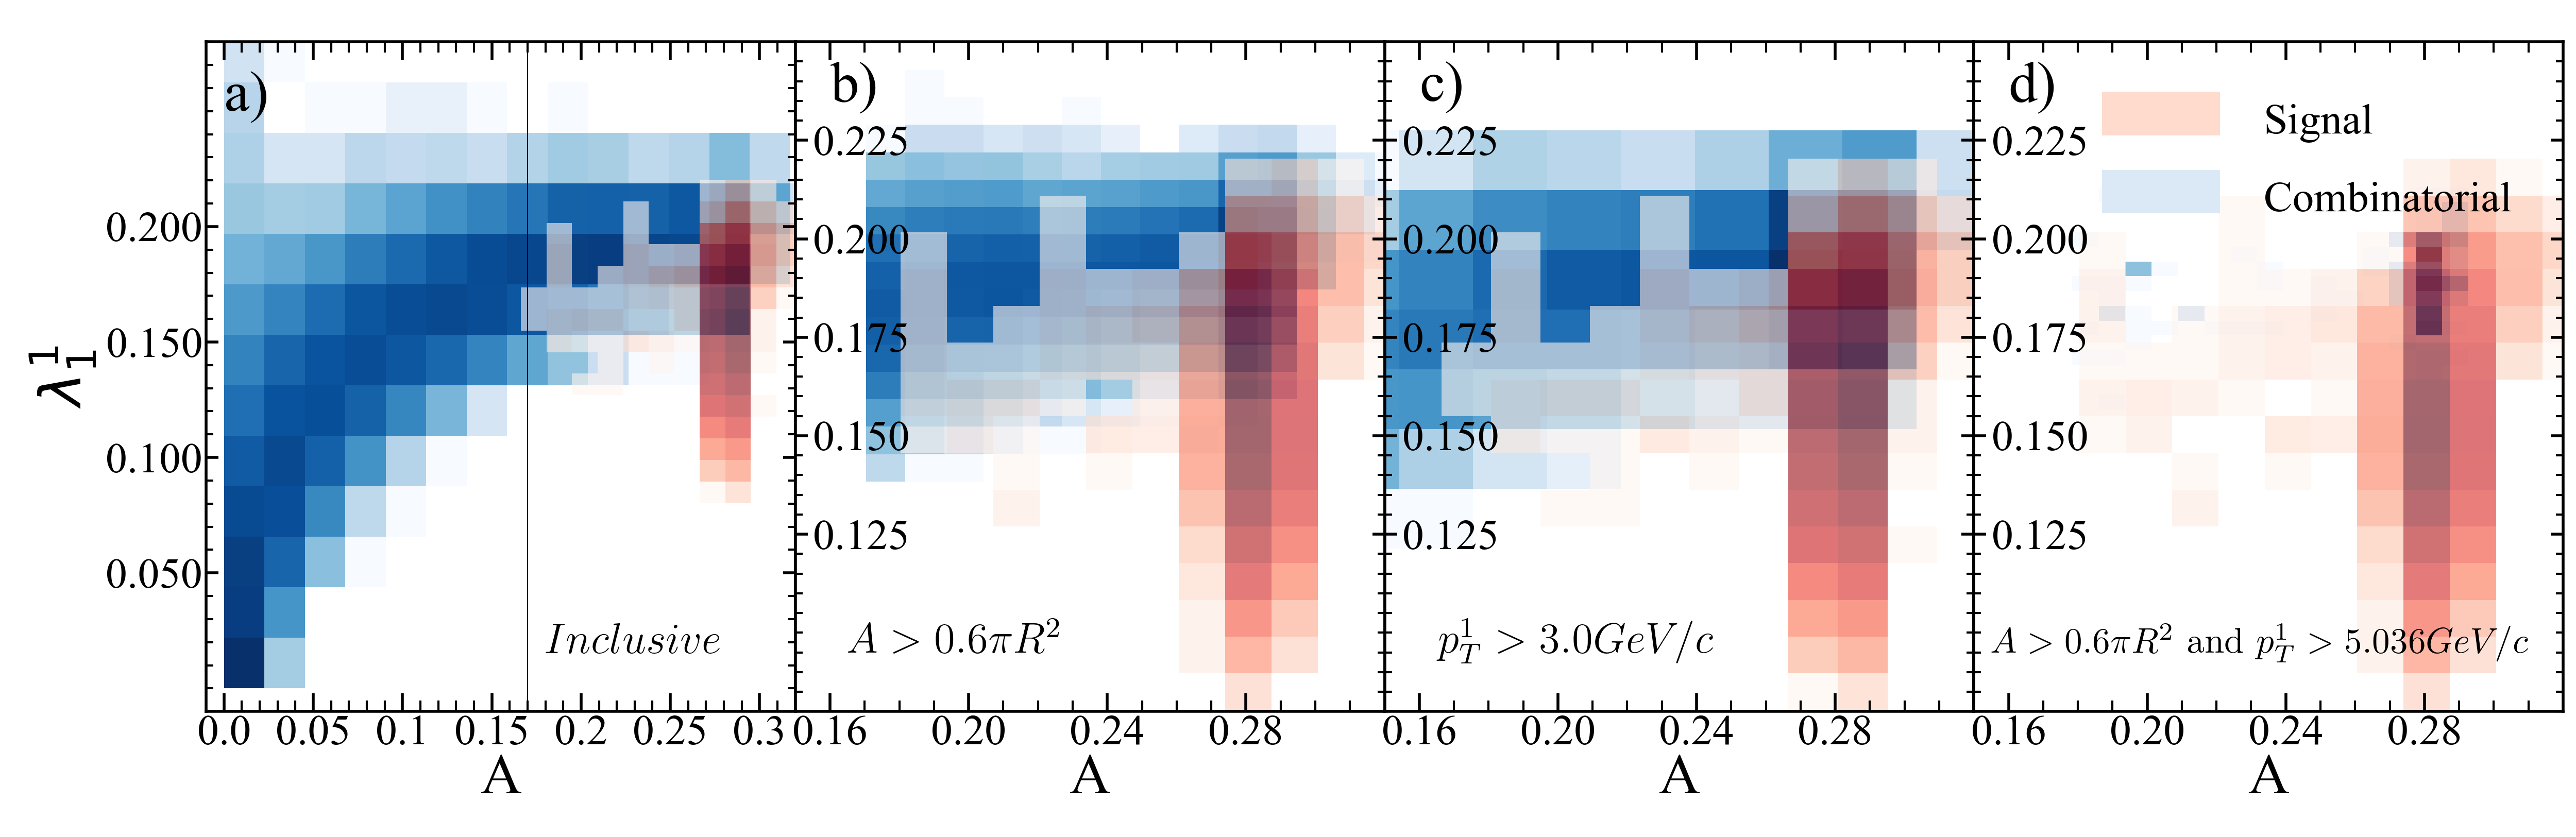}
    \caption{R=0.3 \ptH=40 \GeV}
    \label{fig:blob_03_40}
\end{figure*}

\begin{figure*}
    \centering
    \includegraphics[width=\linewidth]{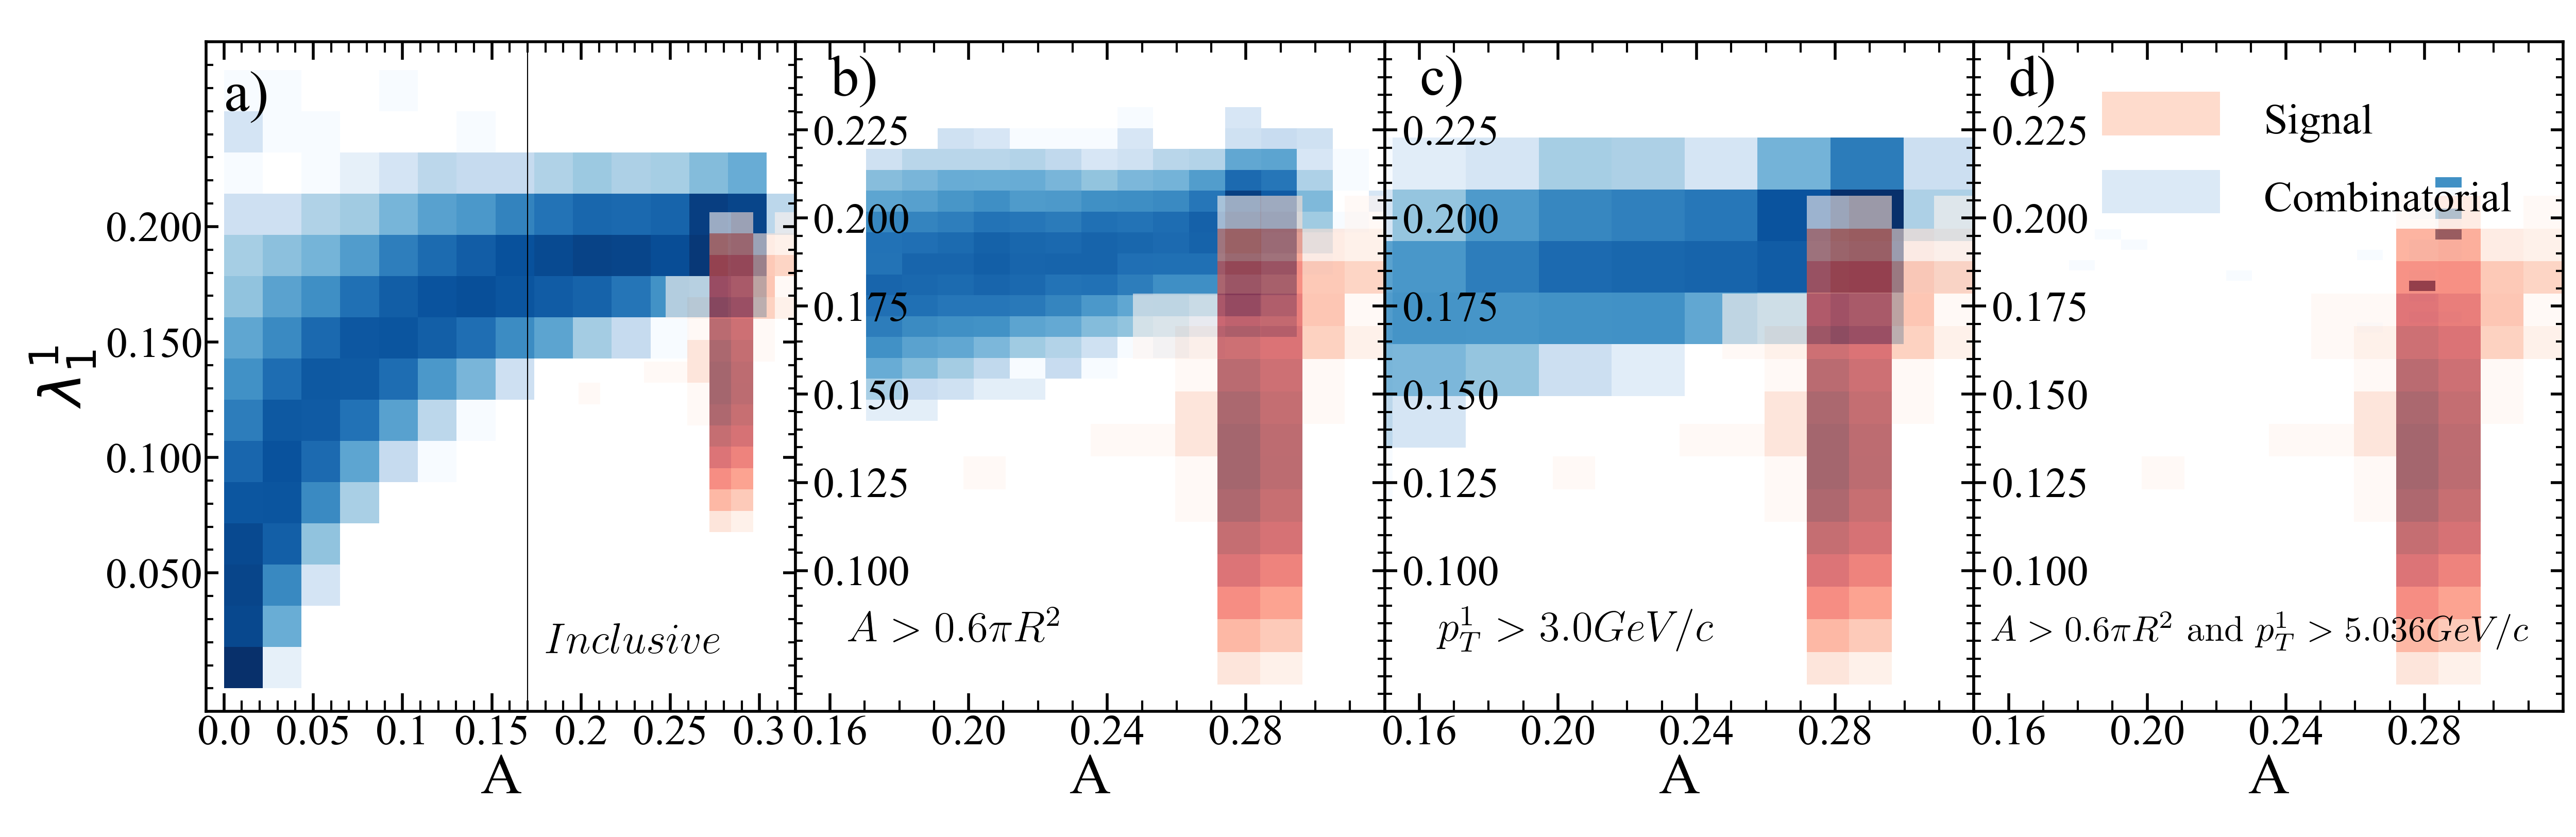}
    \caption{R=0.3 \ptH=60 \GeV}
    \label{fig:blob_03_60}
\end{figure*}

\begin{figure*}
    \centering
    \includegraphics[width=\linewidth]{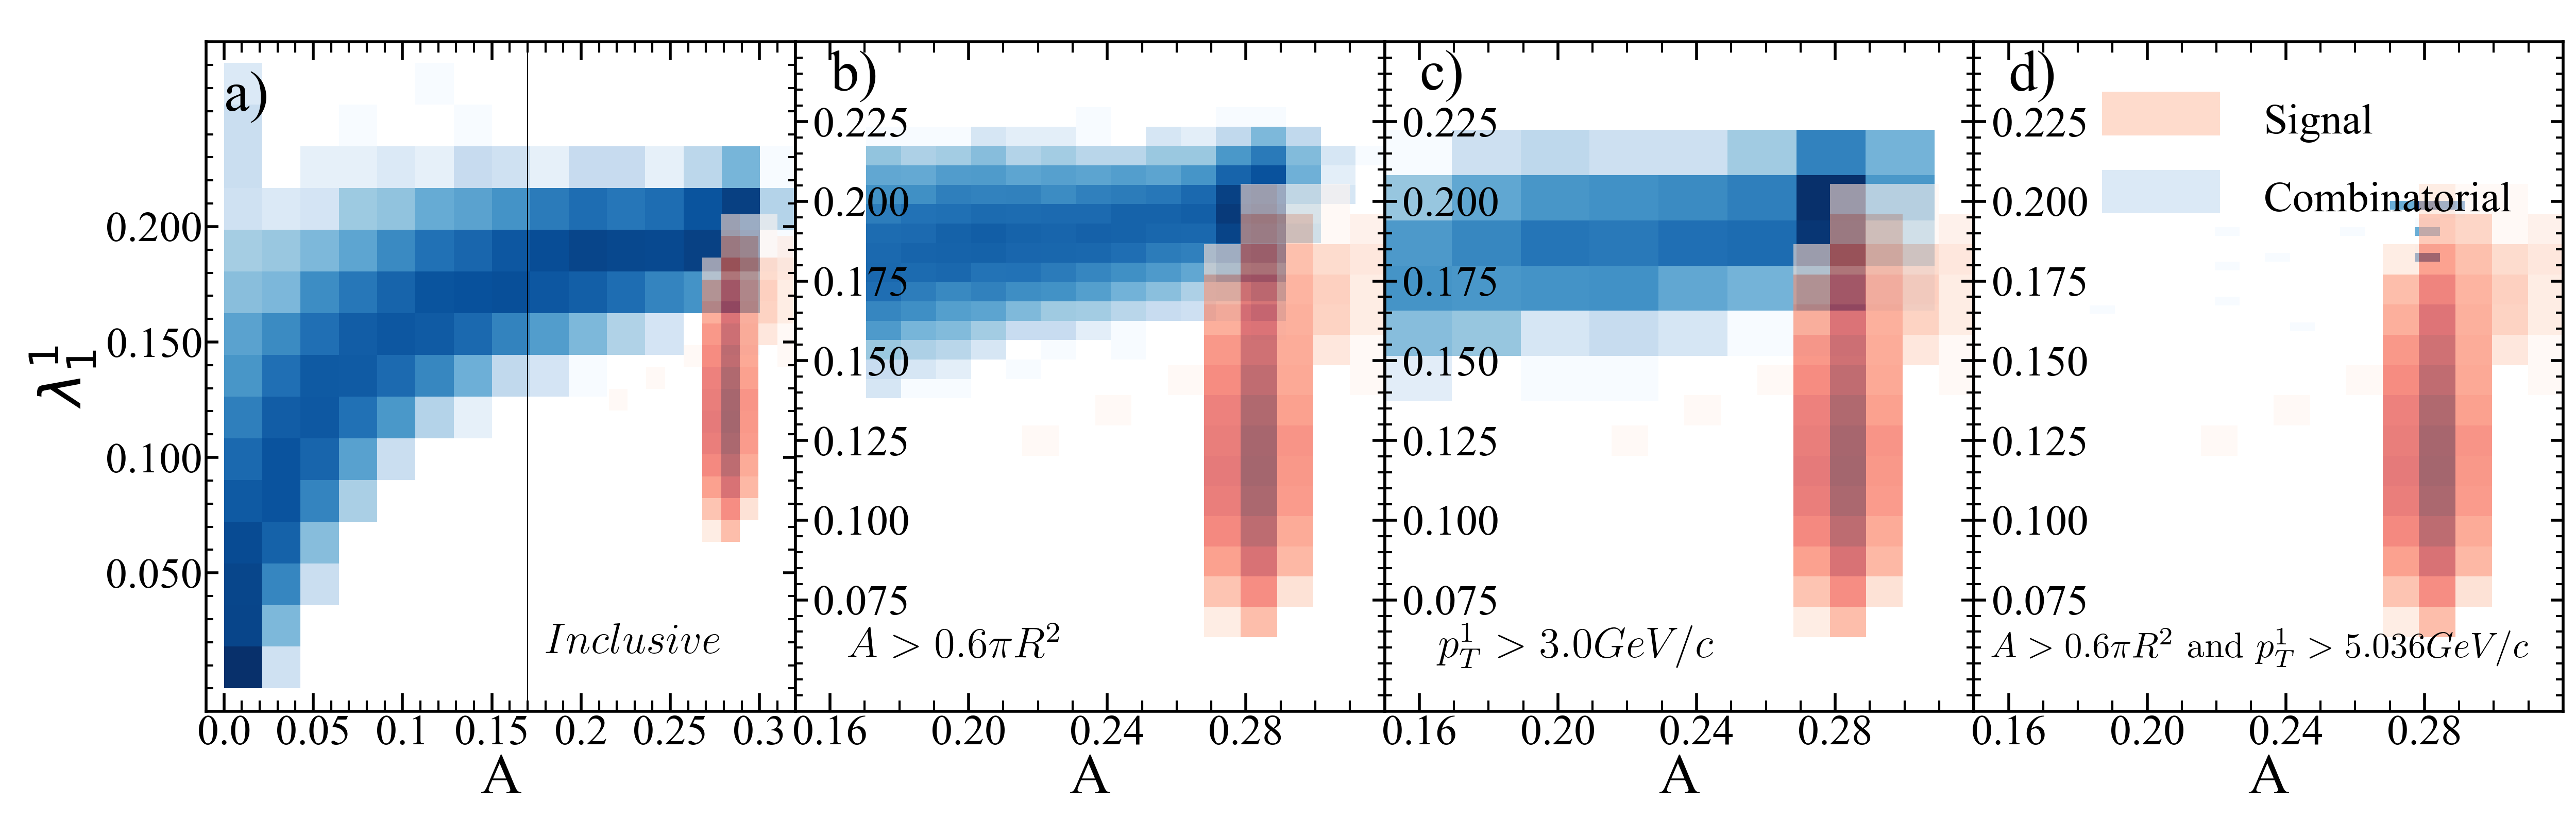}
    \caption{R=0.3 \ptH=80 \GeV}
    \label{fig:blob_03_80}
\end{figure*}

\begin{figure*}
    \centering
    \includegraphics[width=\linewidth]{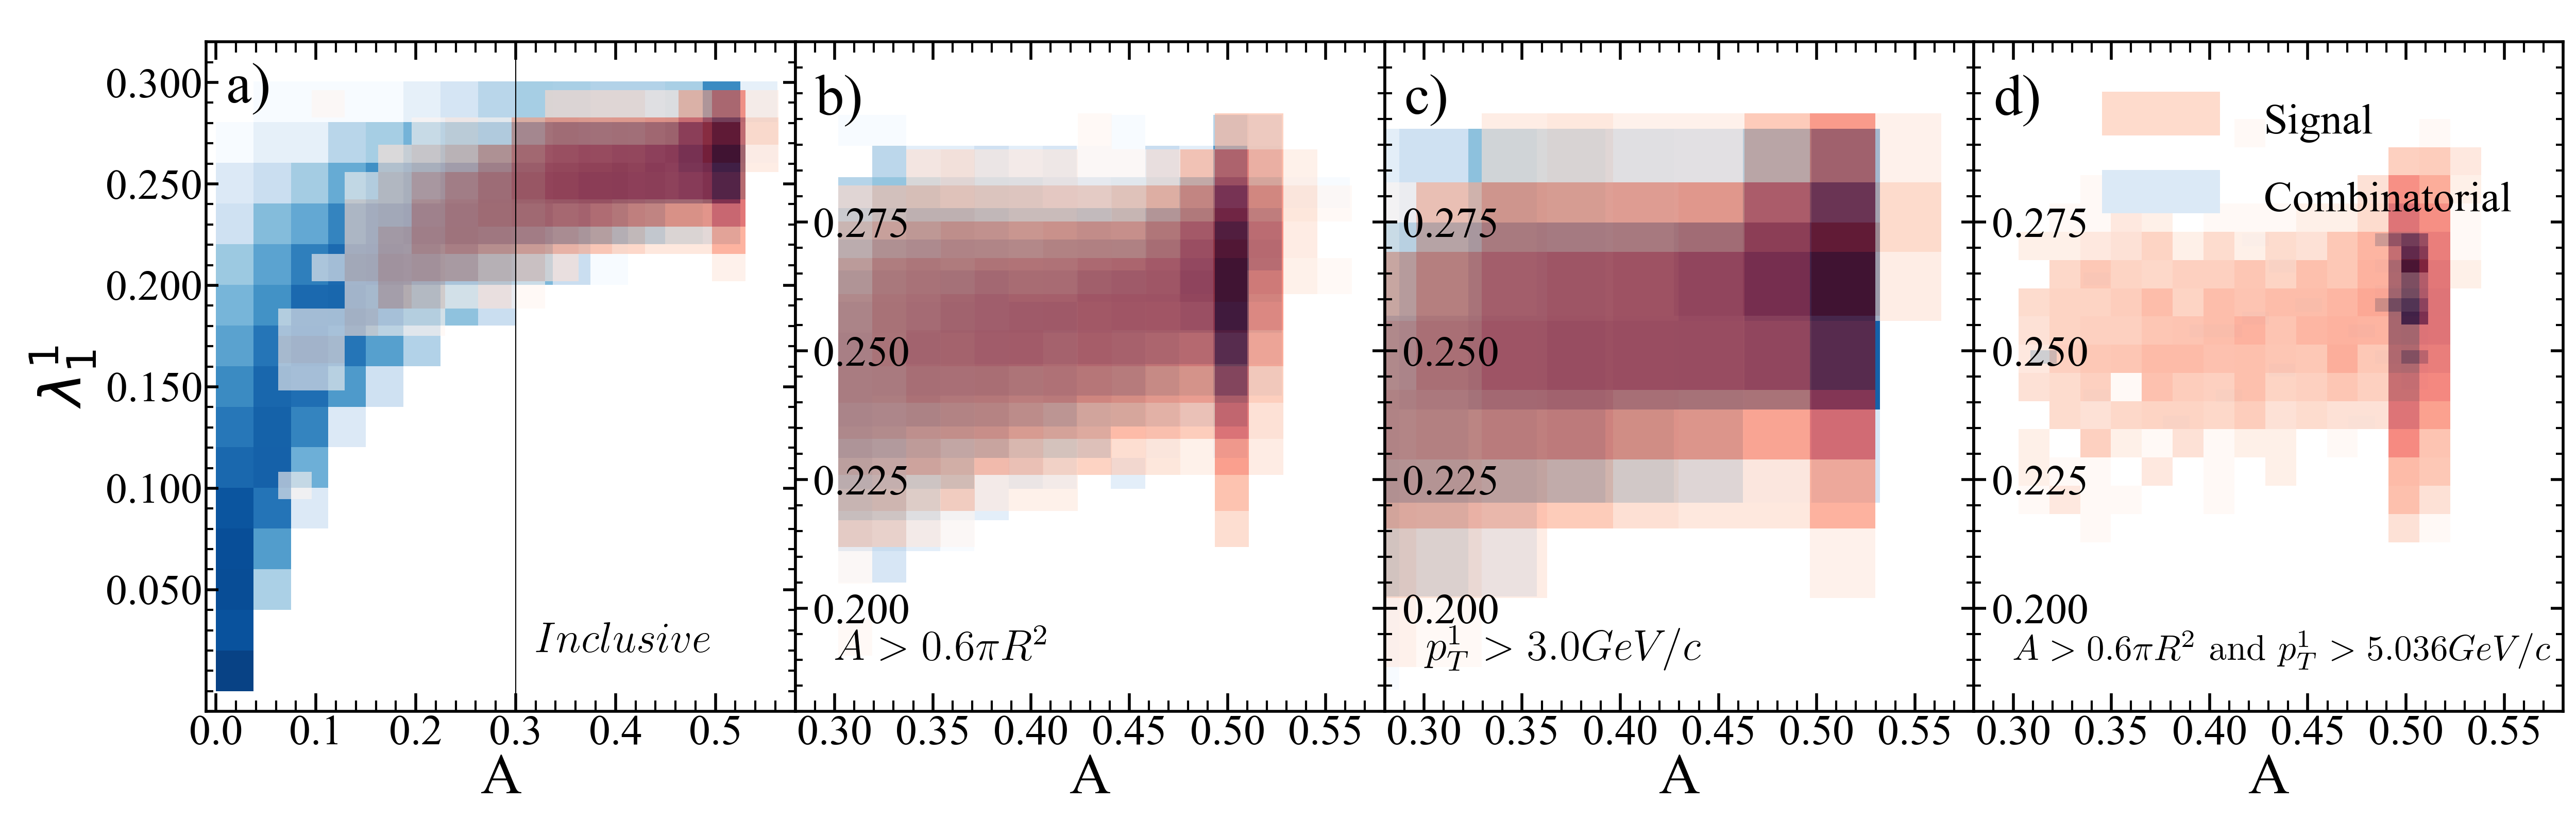}
    \caption{R=0.4 \ptH=10 \GeV}
    \label{fig:blob_04_10}
\end{figure*}

\begin{figure*}
    \centering
    \includegraphics[width=\linewidth]{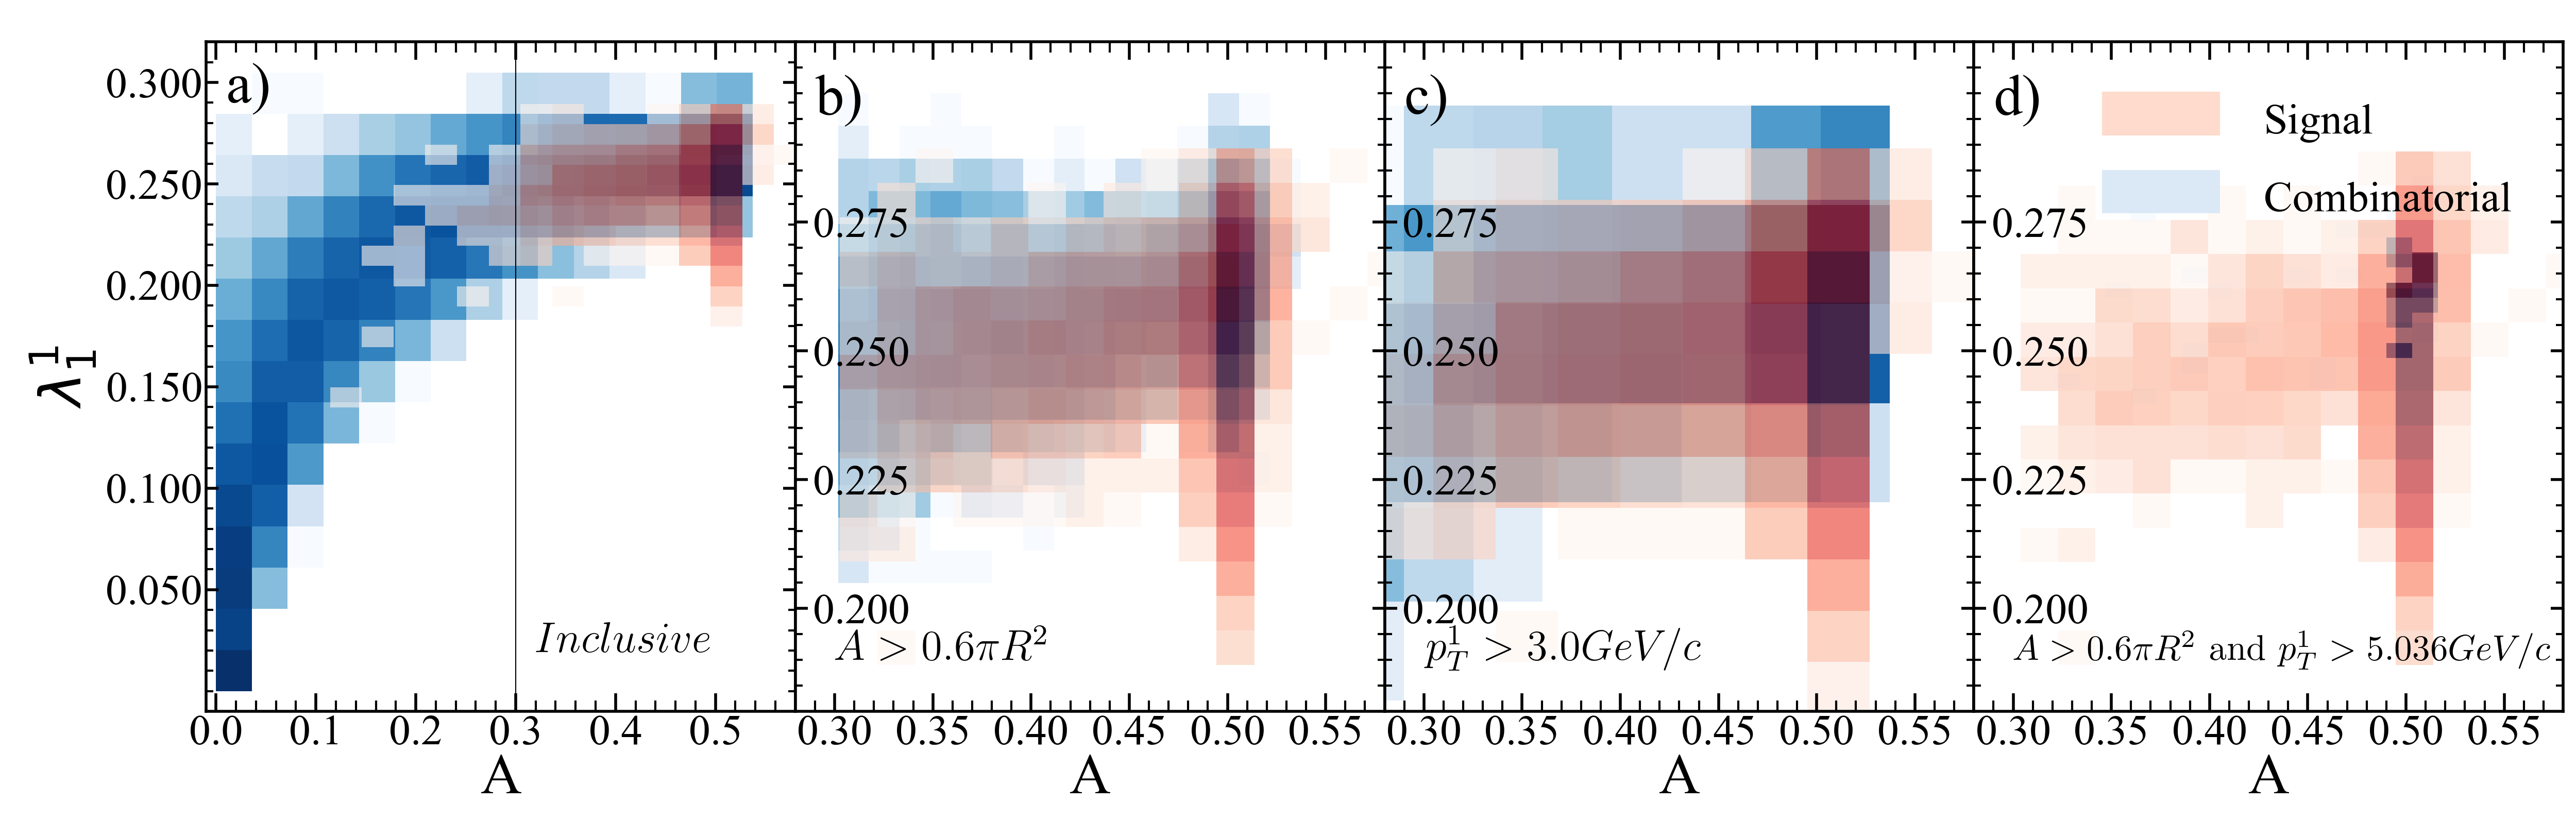}
    \caption{R=0.4 \ptH=20 \GeV}
    \label{fig:blob_04_20}
\end{figure*}

\begin{figure*}
    \centering
    \includegraphics[width=\linewidth]{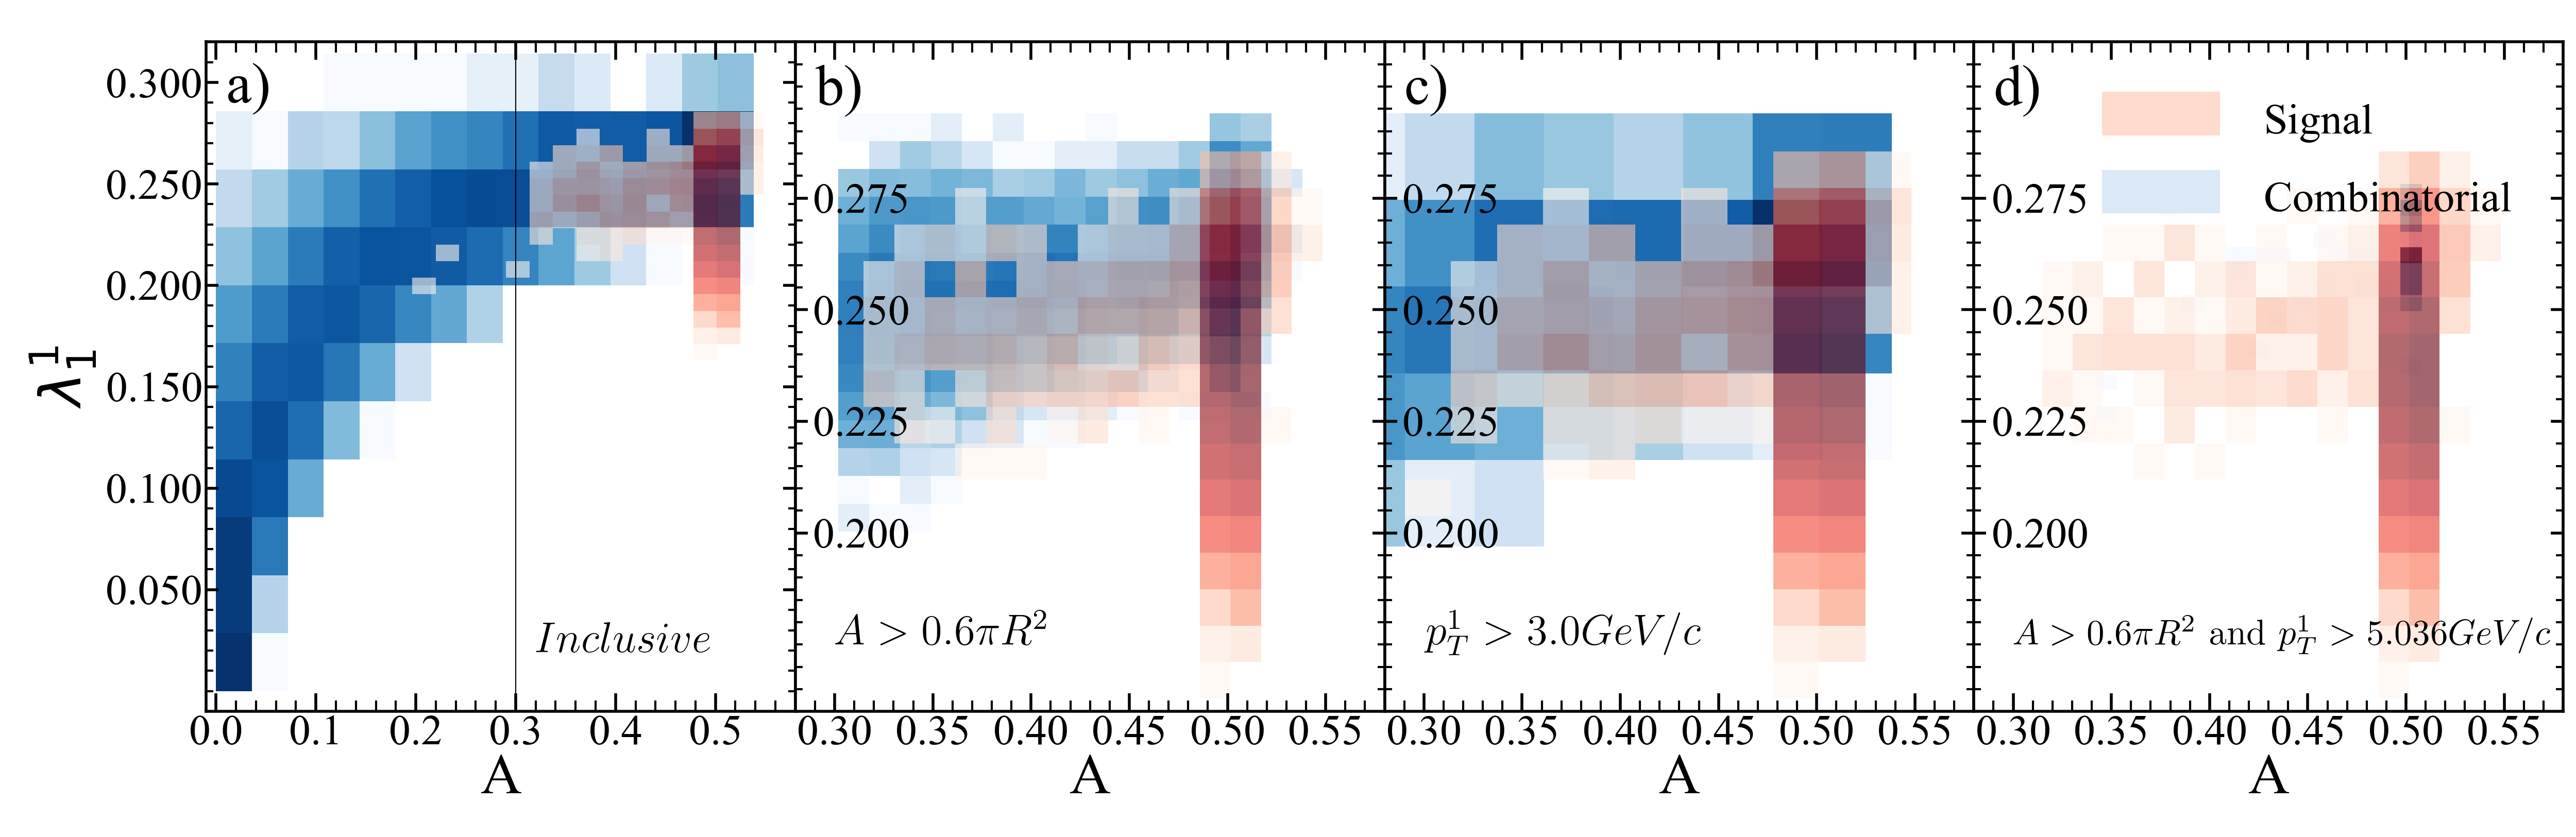}
    \caption{R=0.4 \ptH=30 \GeV}
    \label{fig:blob_04_30}
\end{figure*}

\begin{figure*}
    \centering
    \includegraphics[width=\linewidth]{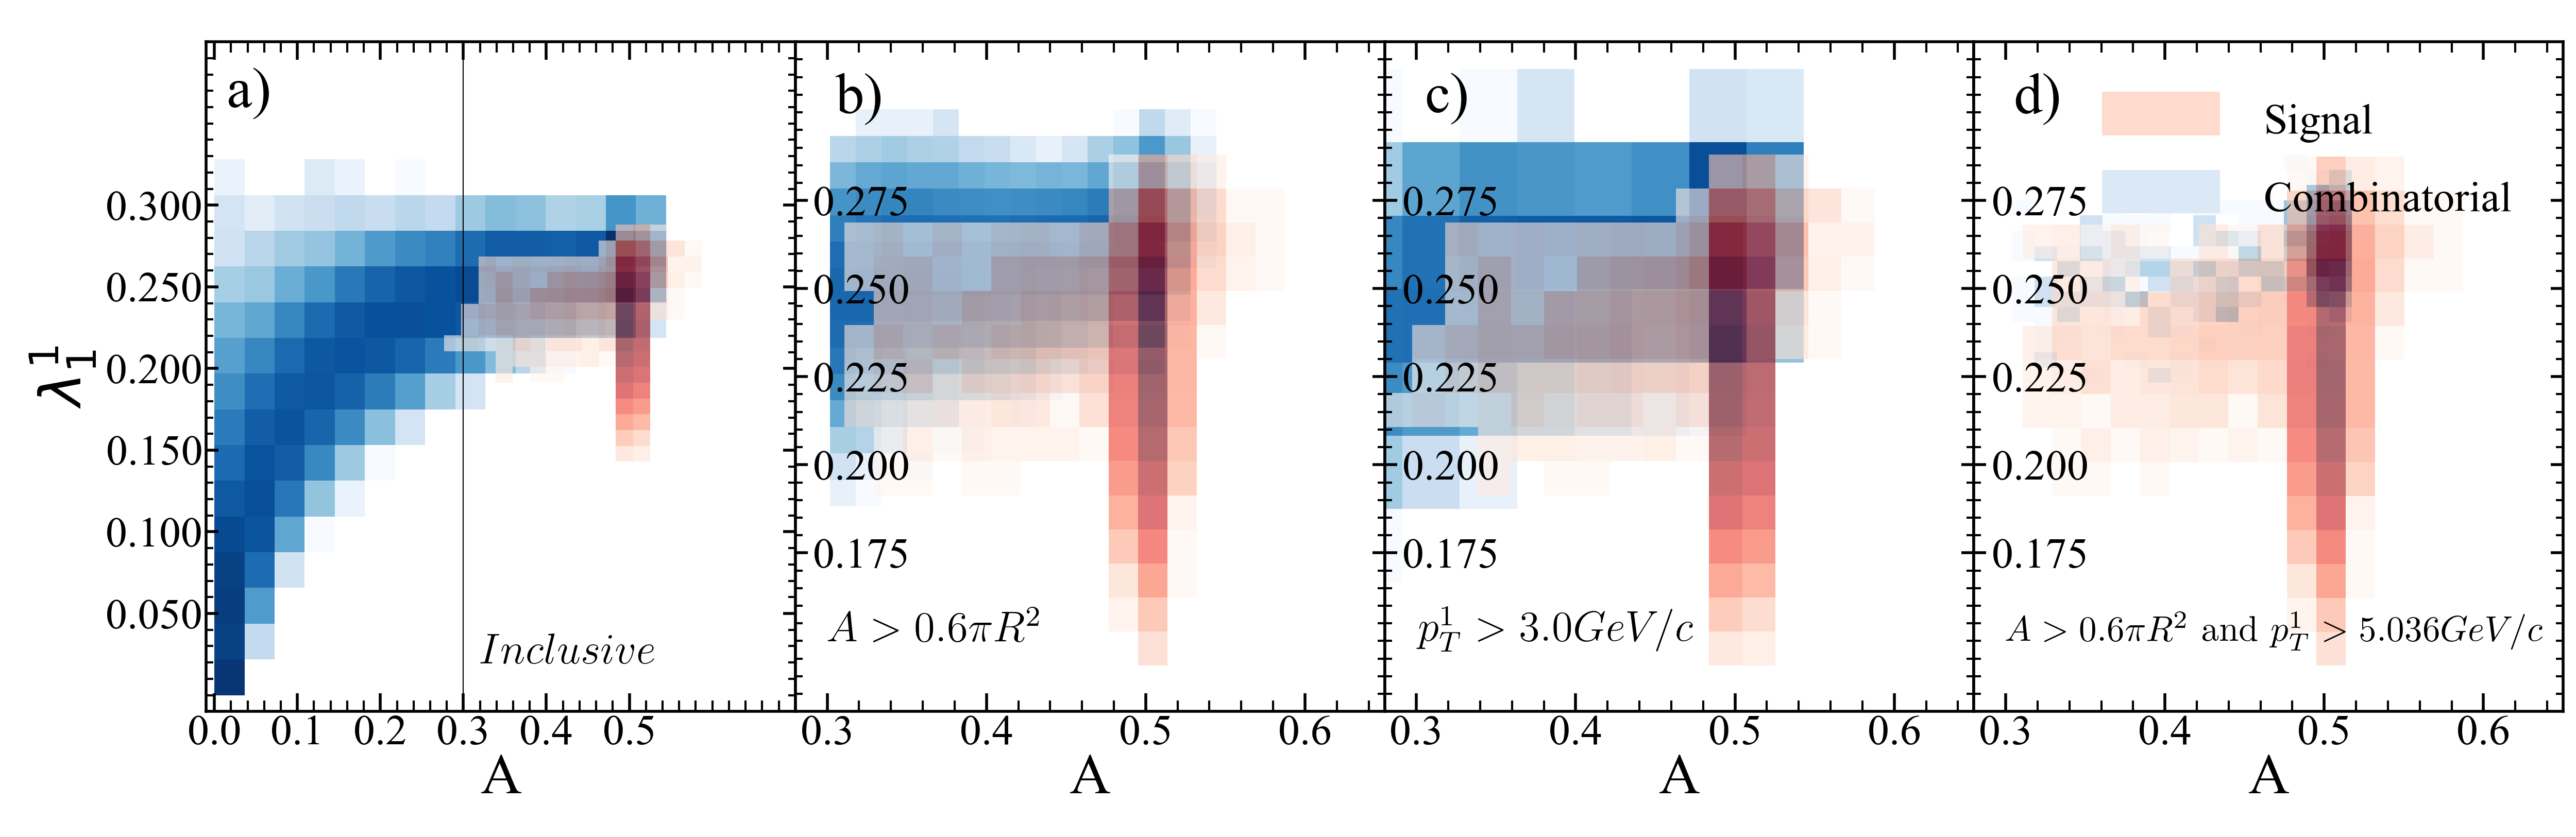}
    \caption{R=0.4 \ptH=40 \GeV}
    \label{fig:blob_04_40}
\end{figure*}

\begin{figure*}
    \centering
    \includegraphics[width=\linewidth]{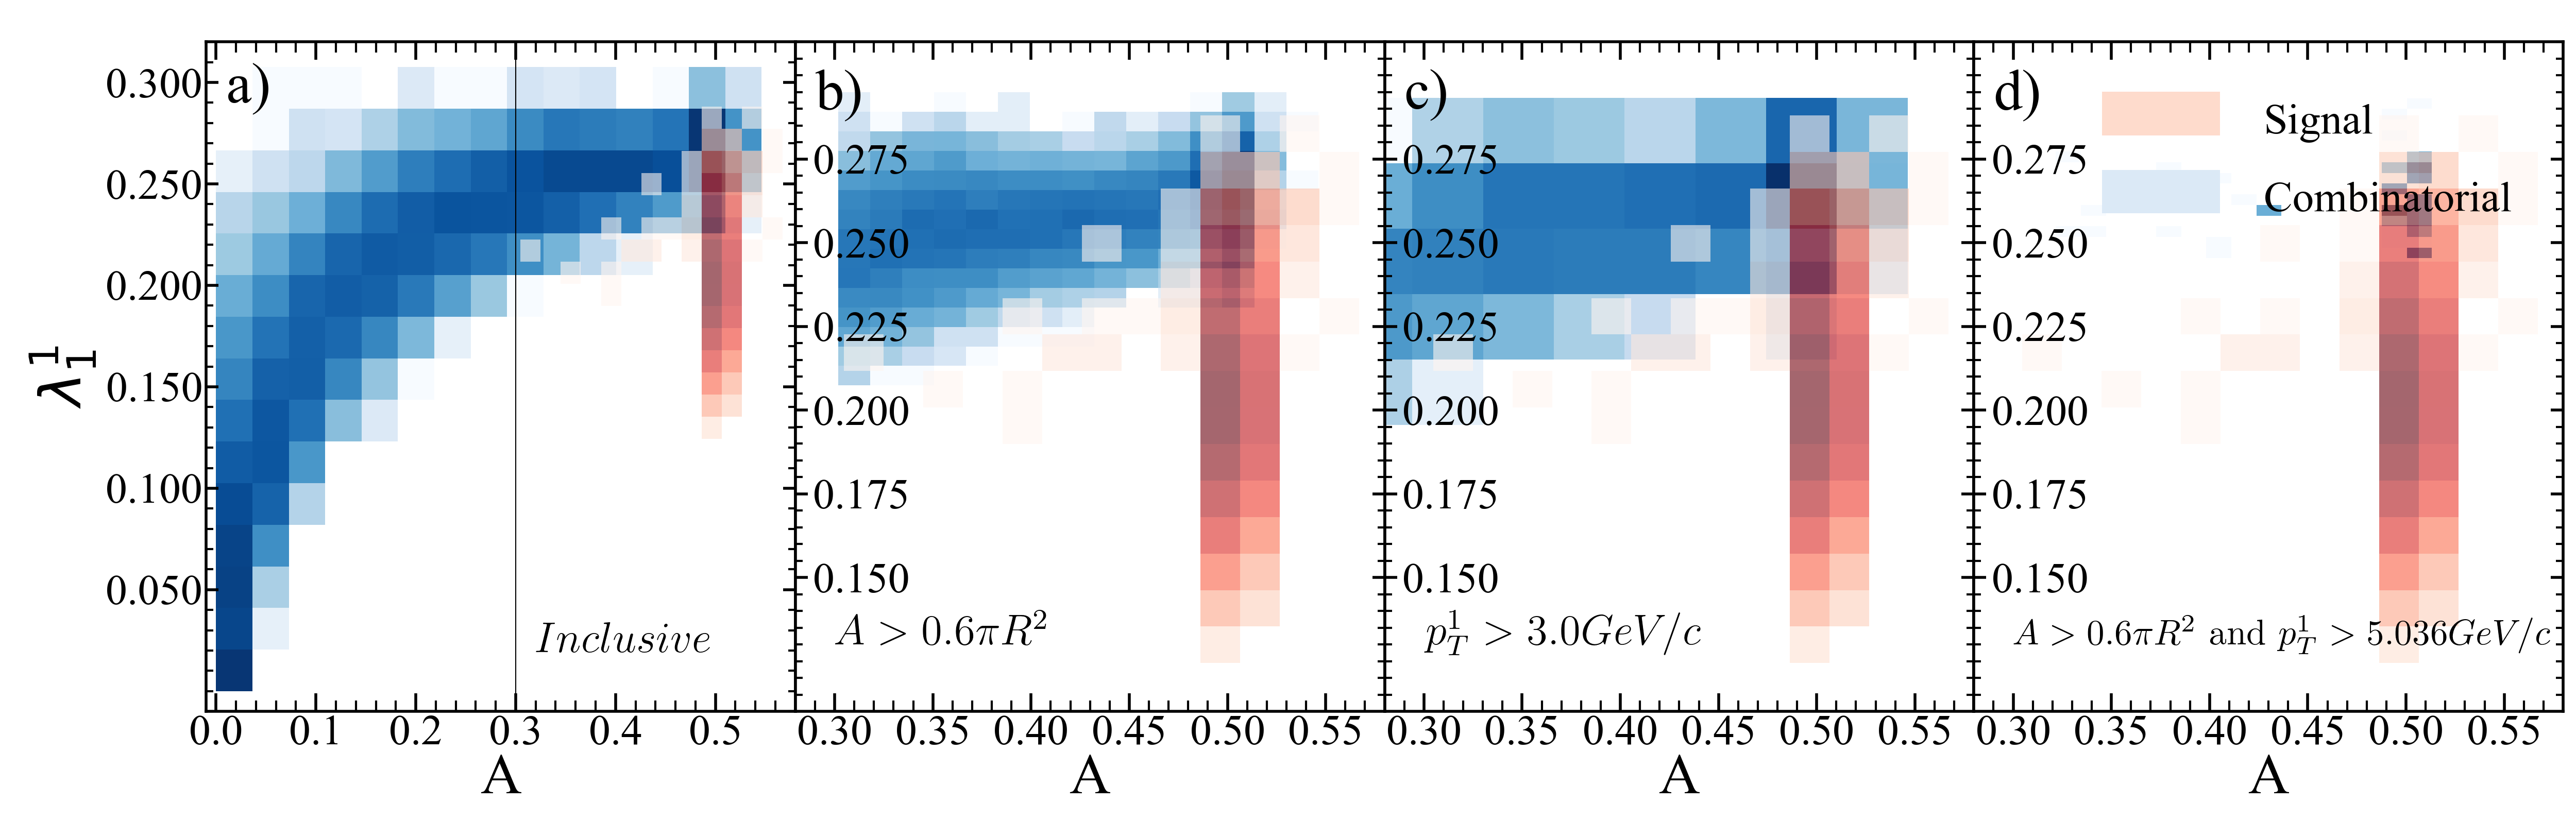}
    \caption{R=0.4 \ptH=60 \GeV}
    \label{fig:blob_04_60}
\end{figure*}

\begin{figure*}
    \centering
    \includegraphics[width=\linewidth]{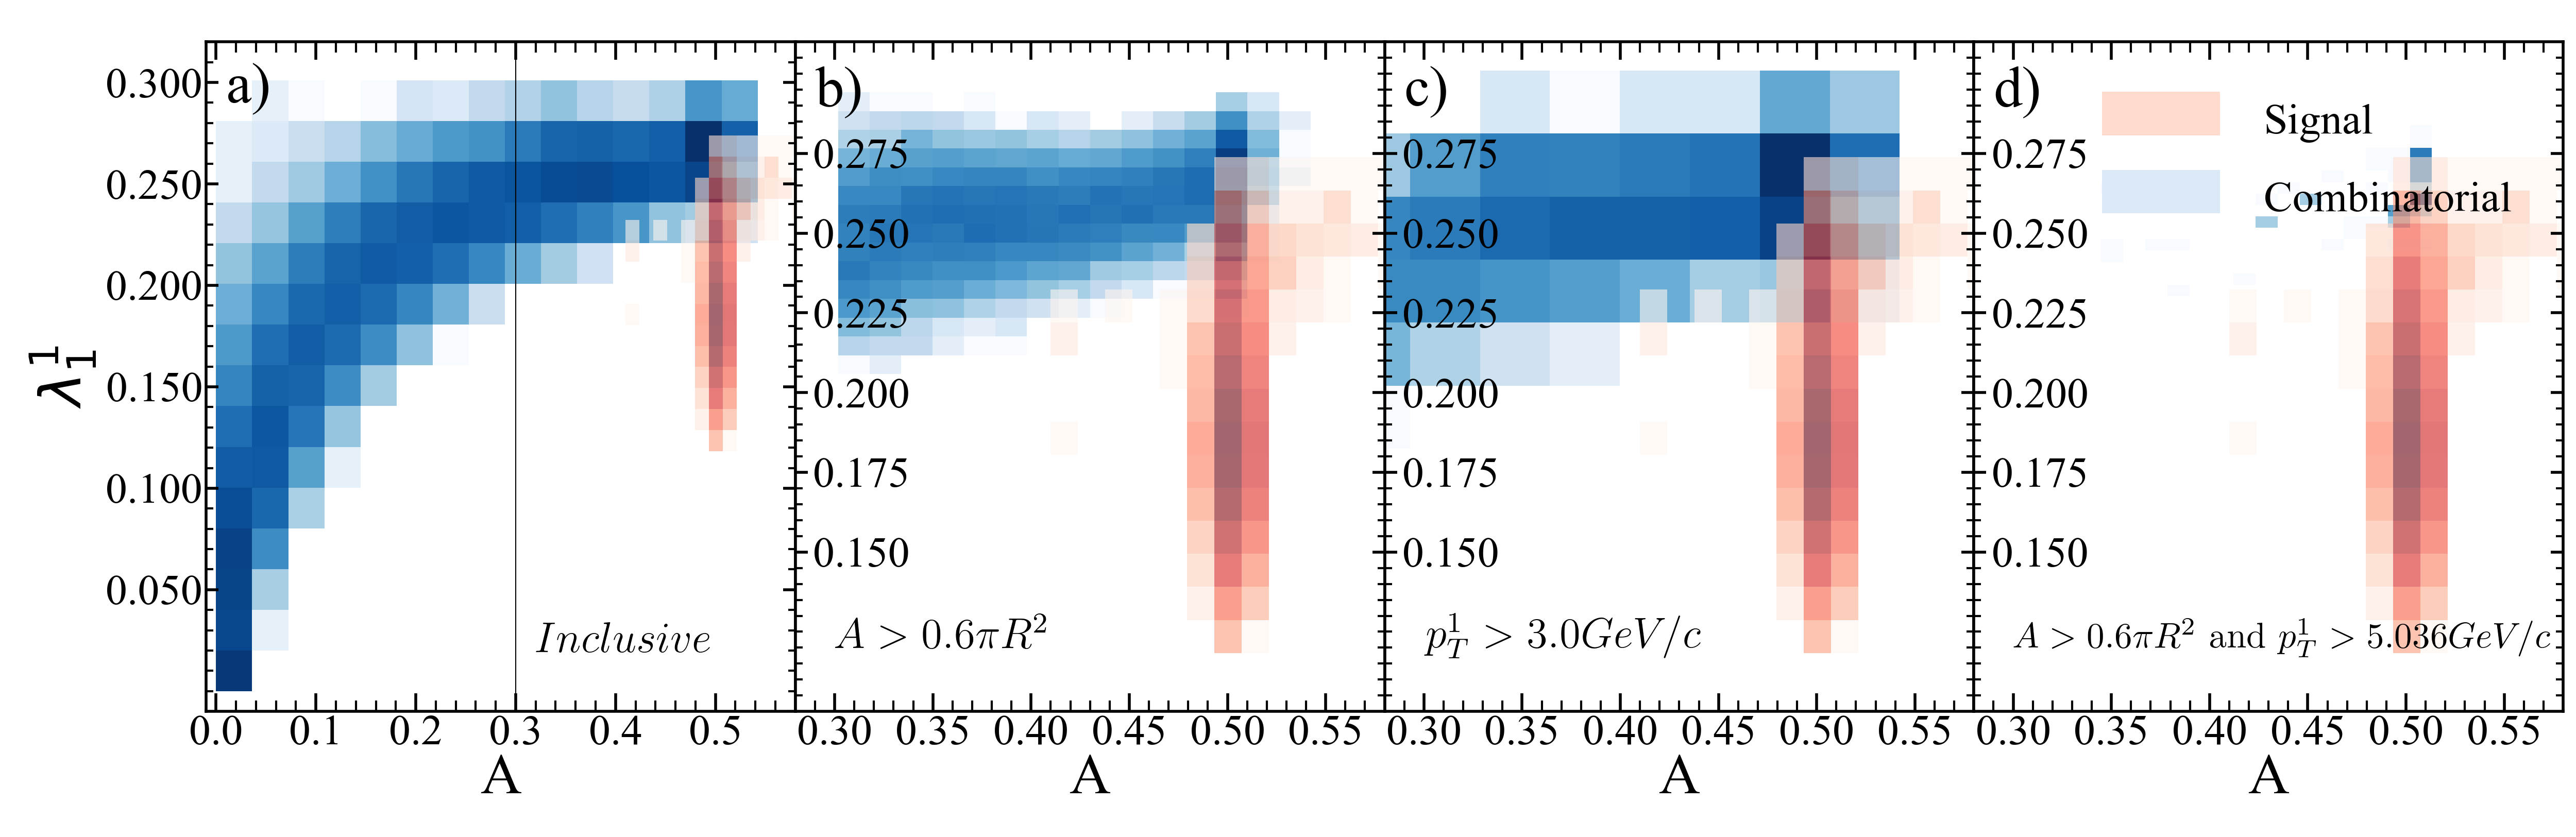}
    \caption{R=0.4 \ptH=80 \GeV}
    \label{fig:blob_04_80}
\end{figure*}

\begin{figure*}
    \centering
    \includegraphics[width=\linewidth]{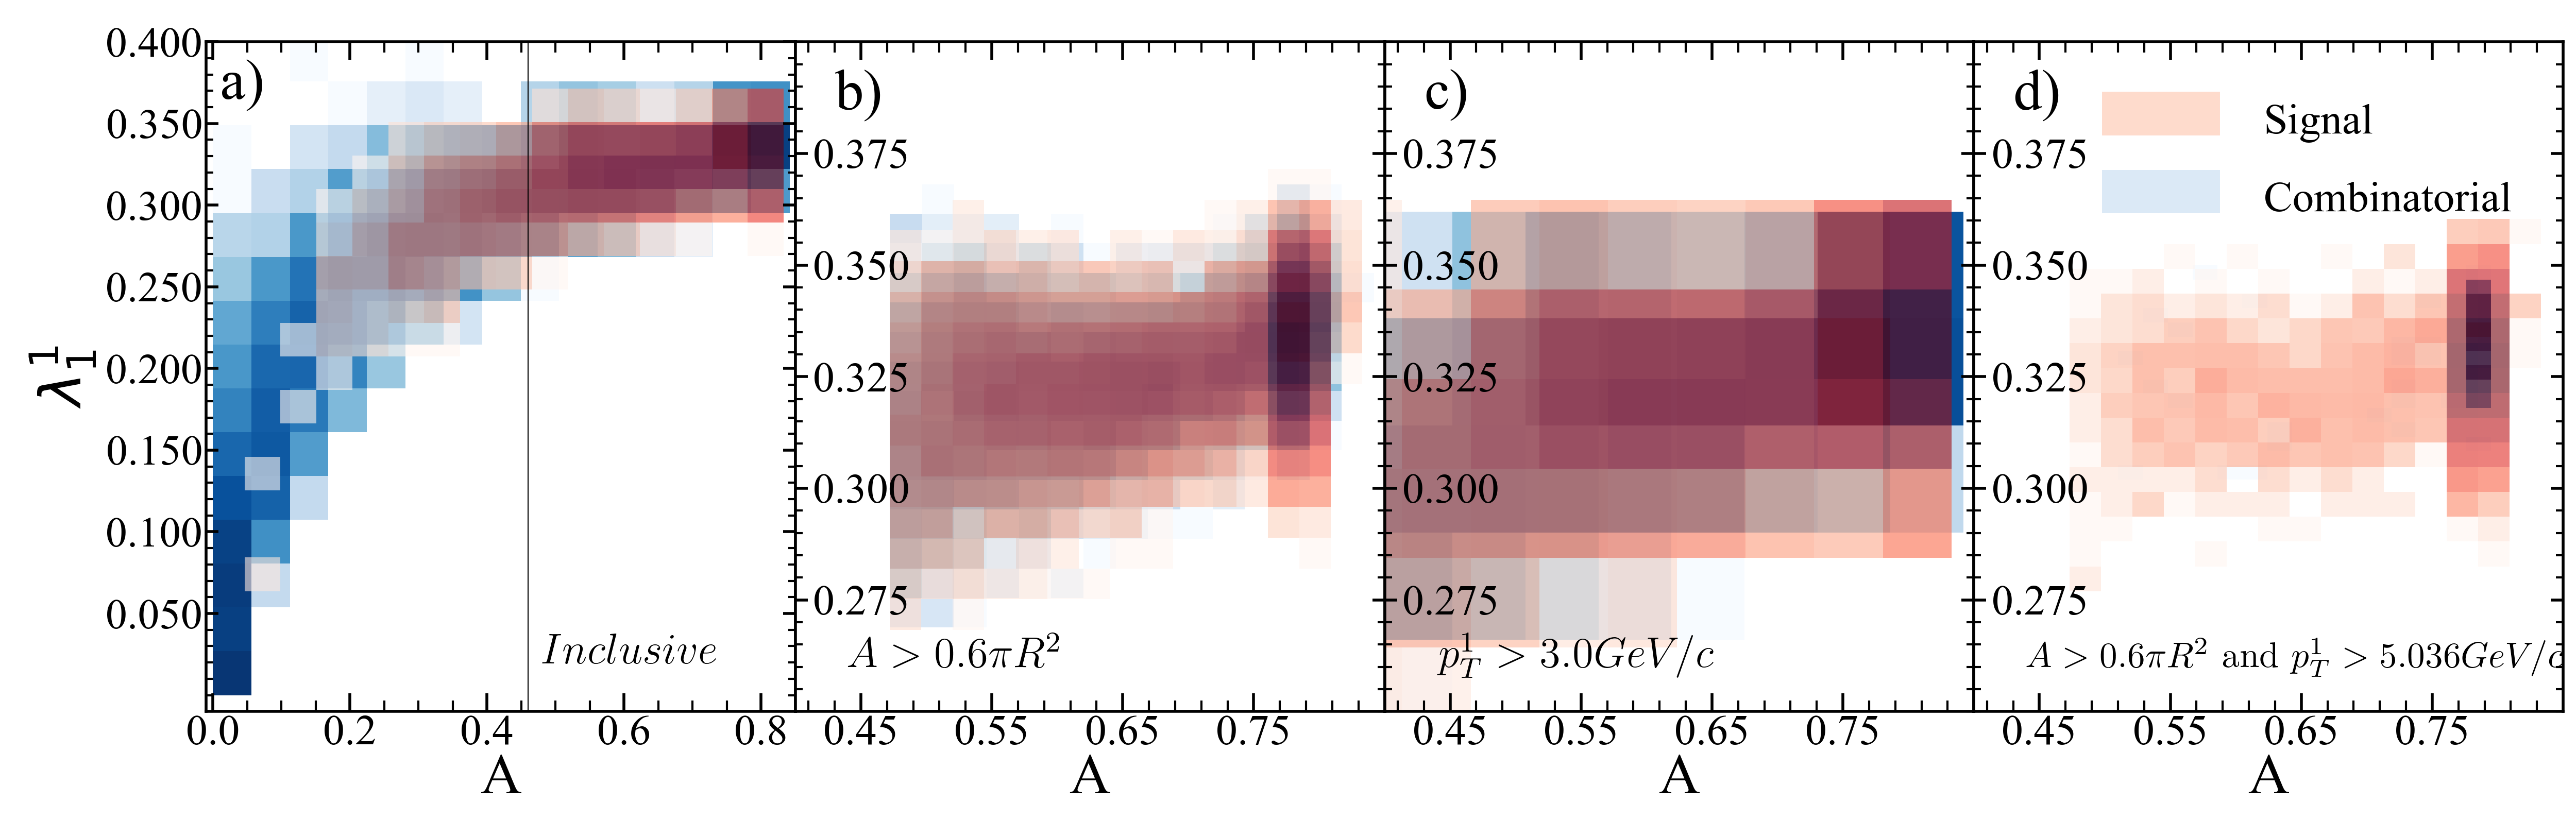}
    \caption{R=0.5 \ptH=10 \GeV}
    \label{fig:blob_05_10}
\end{figure*}

\begin{figure*}
    \centering
    \includegraphics[width=\linewidth]{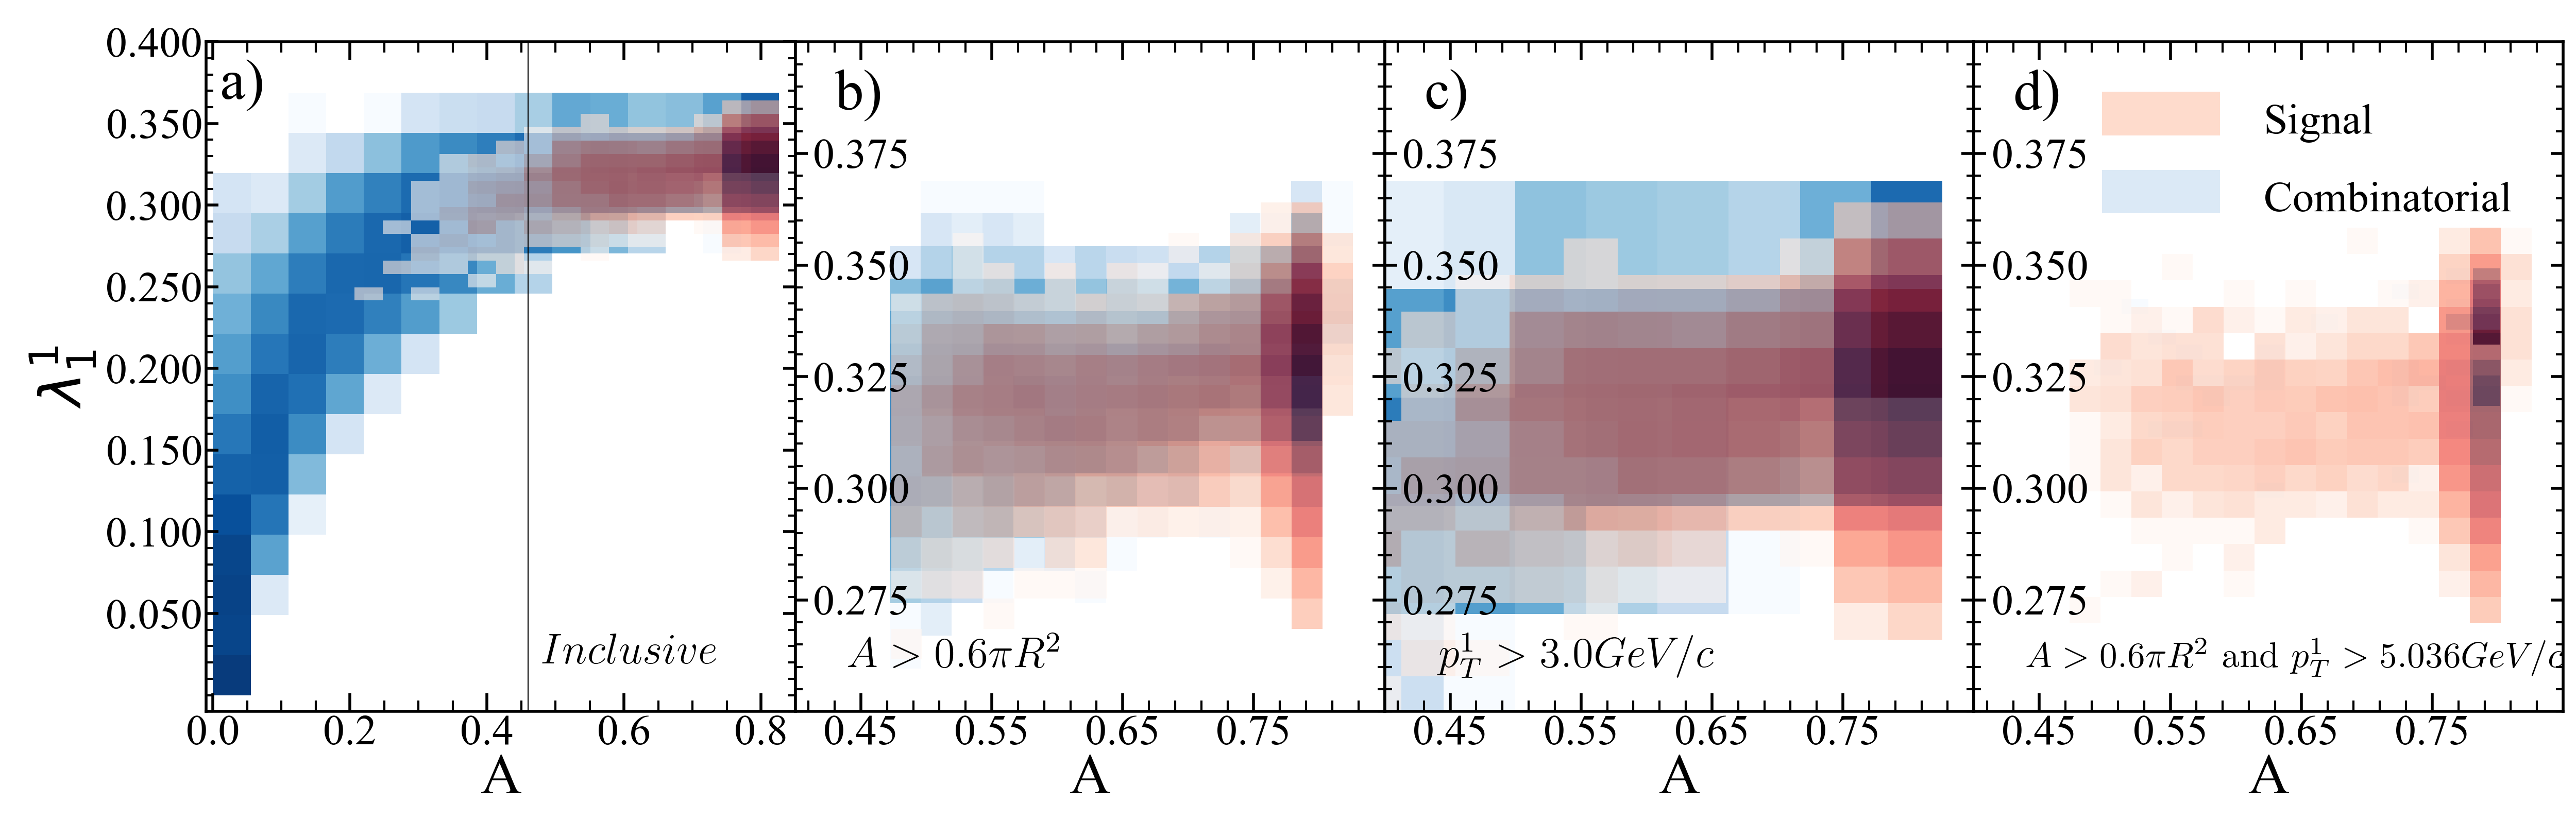}
    \caption{R=0.5 \ptH=20 \GeV}
    \label{fig:blob_05_20}
\end{figure*}

\begin{figure*}
    \centering
    \includegraphics[width=\linewidth]{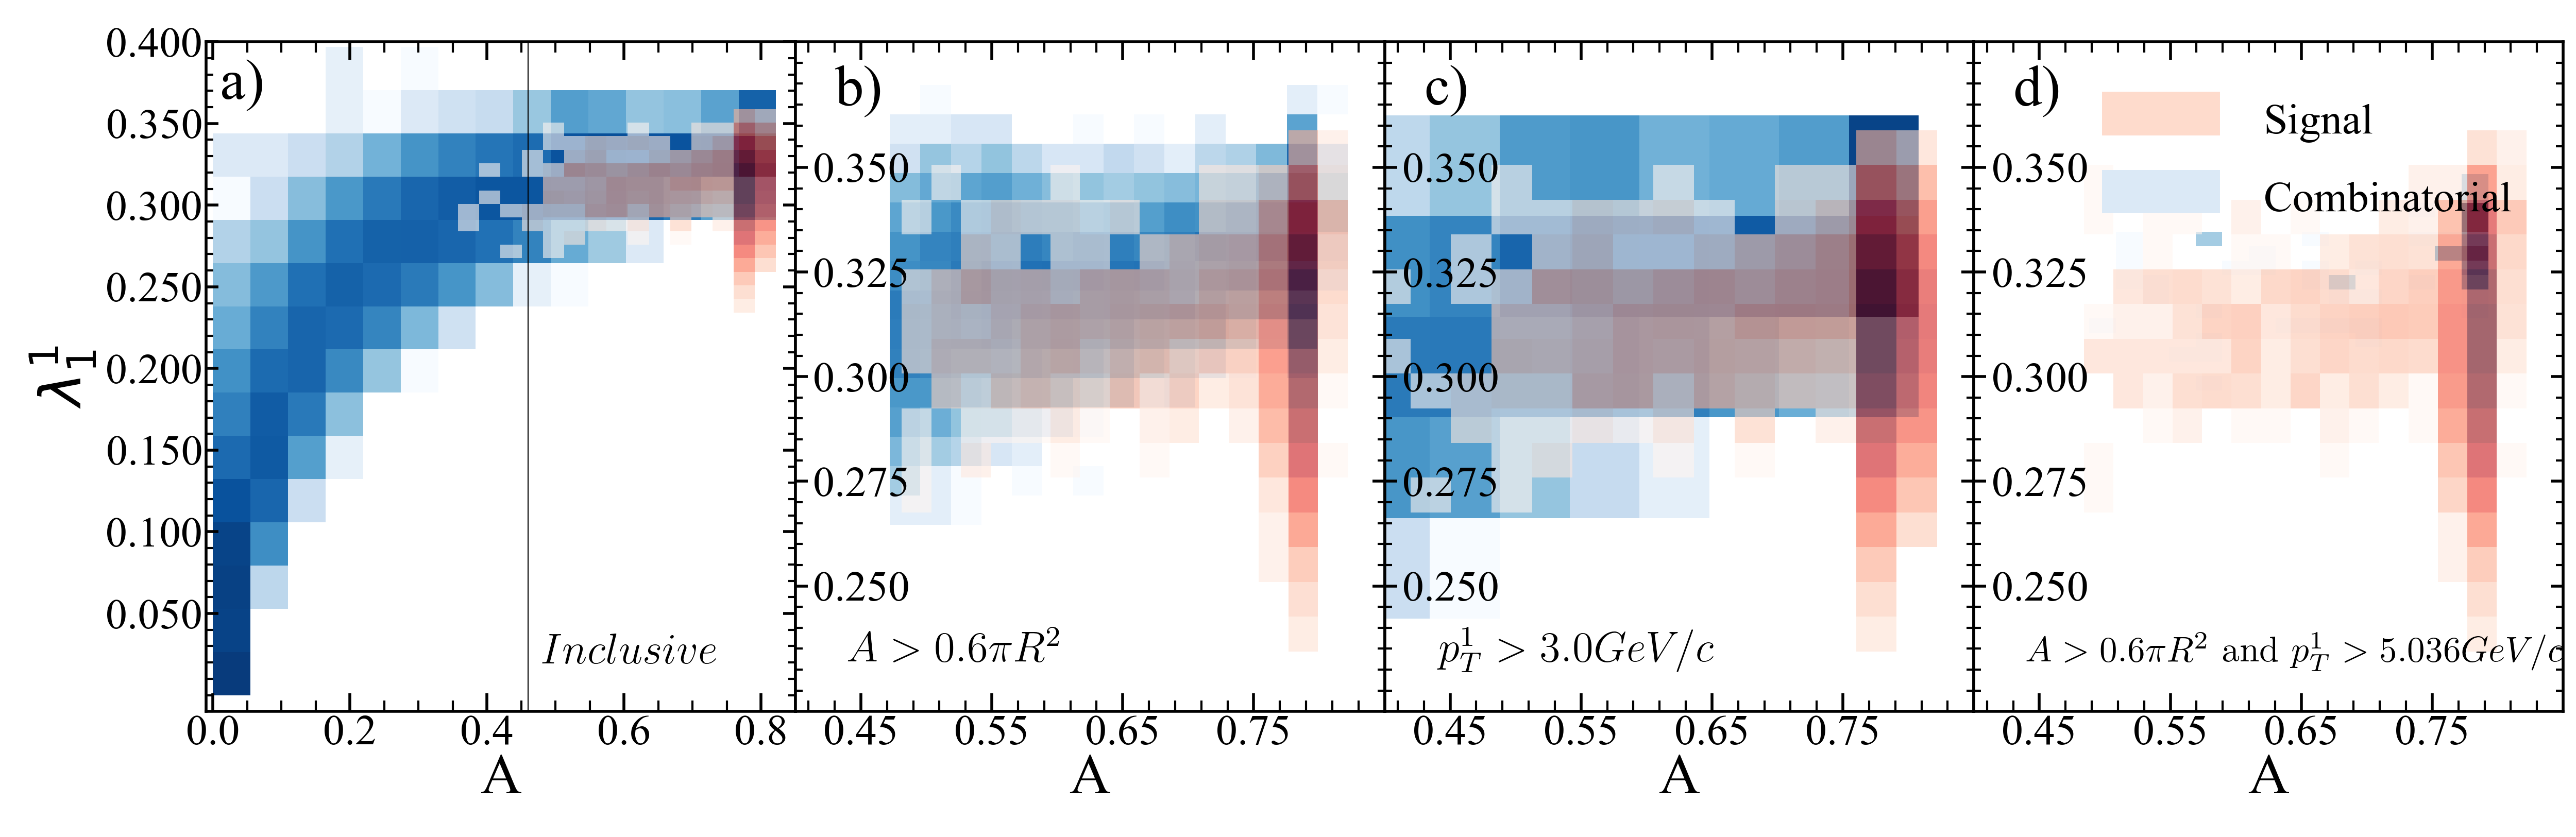}
    \caption{R=0.5 \ptH=30 \GeV}
    \label{fig:blob_05_30}
\end{figure*}

\begin{figure*}
    \centering
    \includegraphics[width=\linewidth]{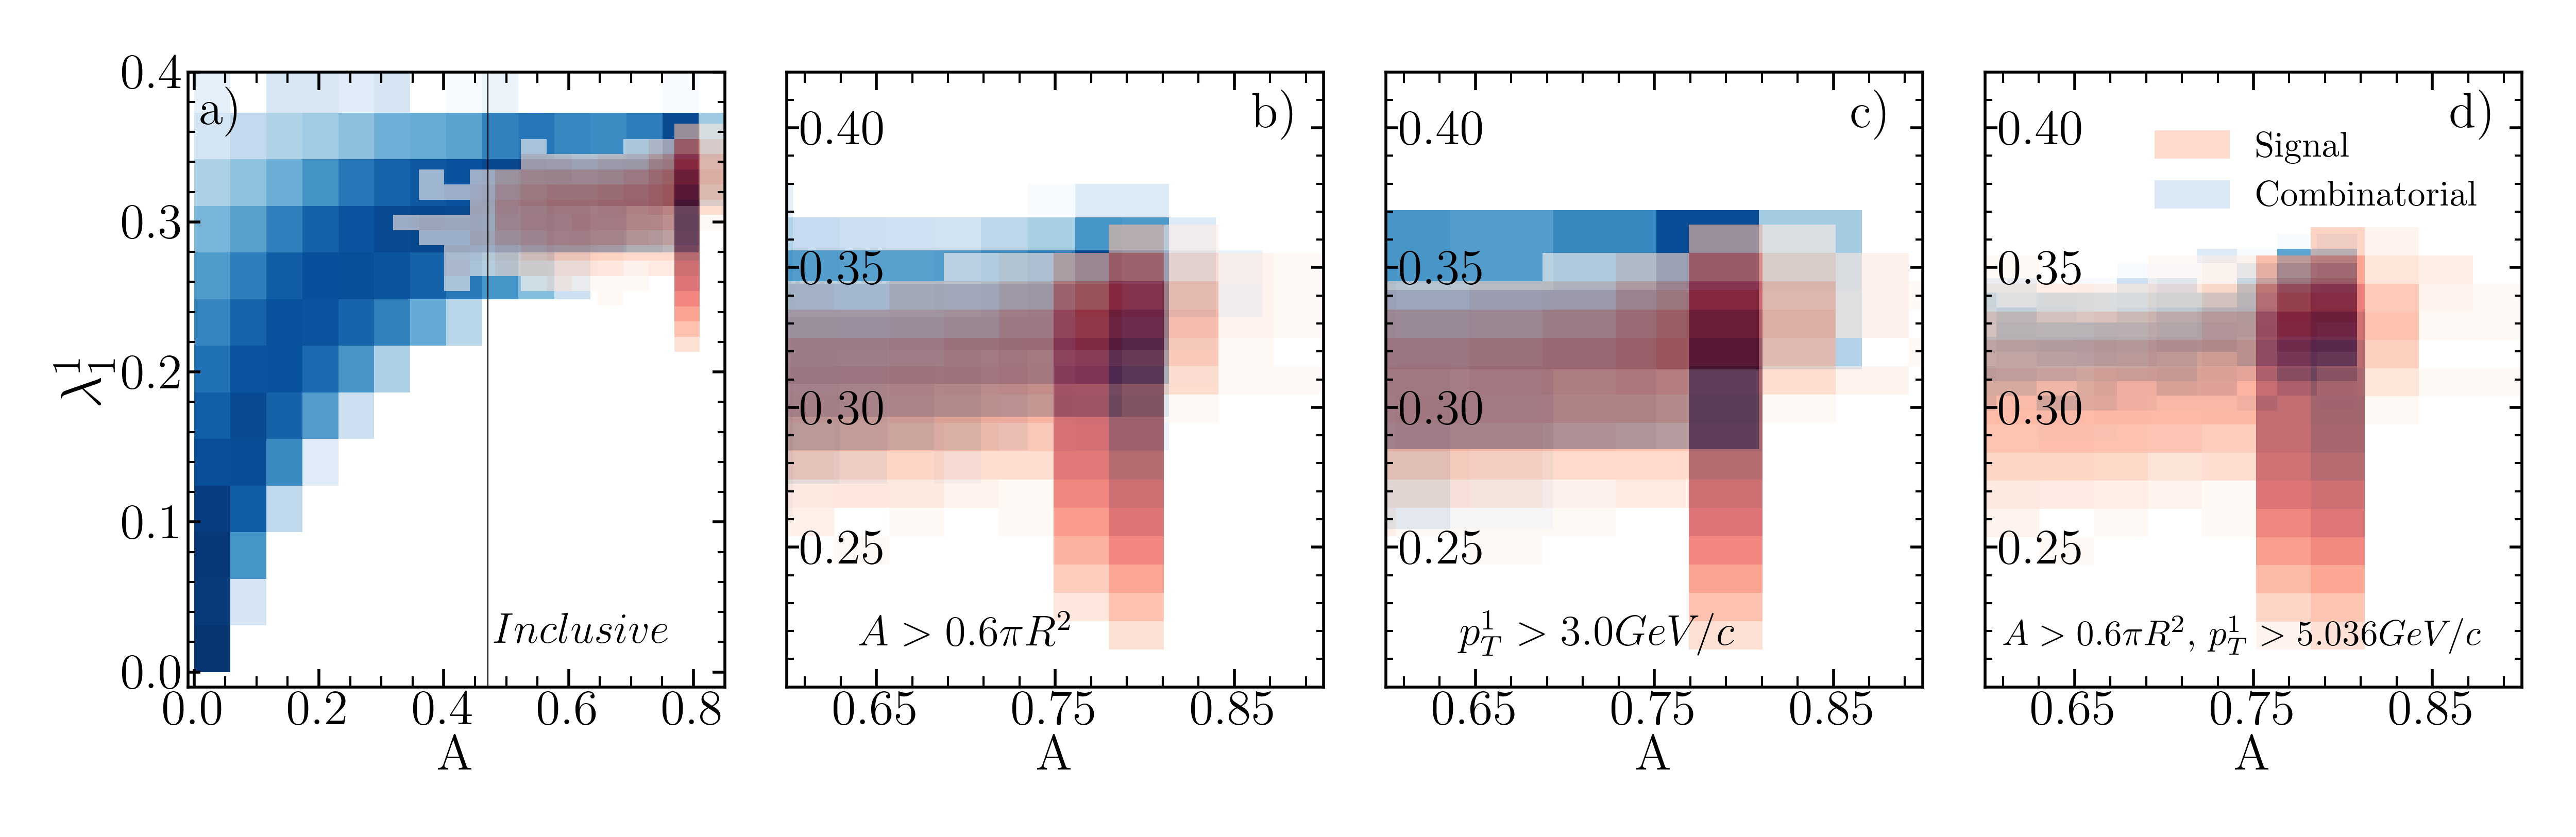}
    \caption{R=0.5 \ptH=40 \GeV}
    \label{fig:blob_05_40}
\end{figure*}

\begin{figure*}
    \centering
    \includegraphics[width=\linewidth]{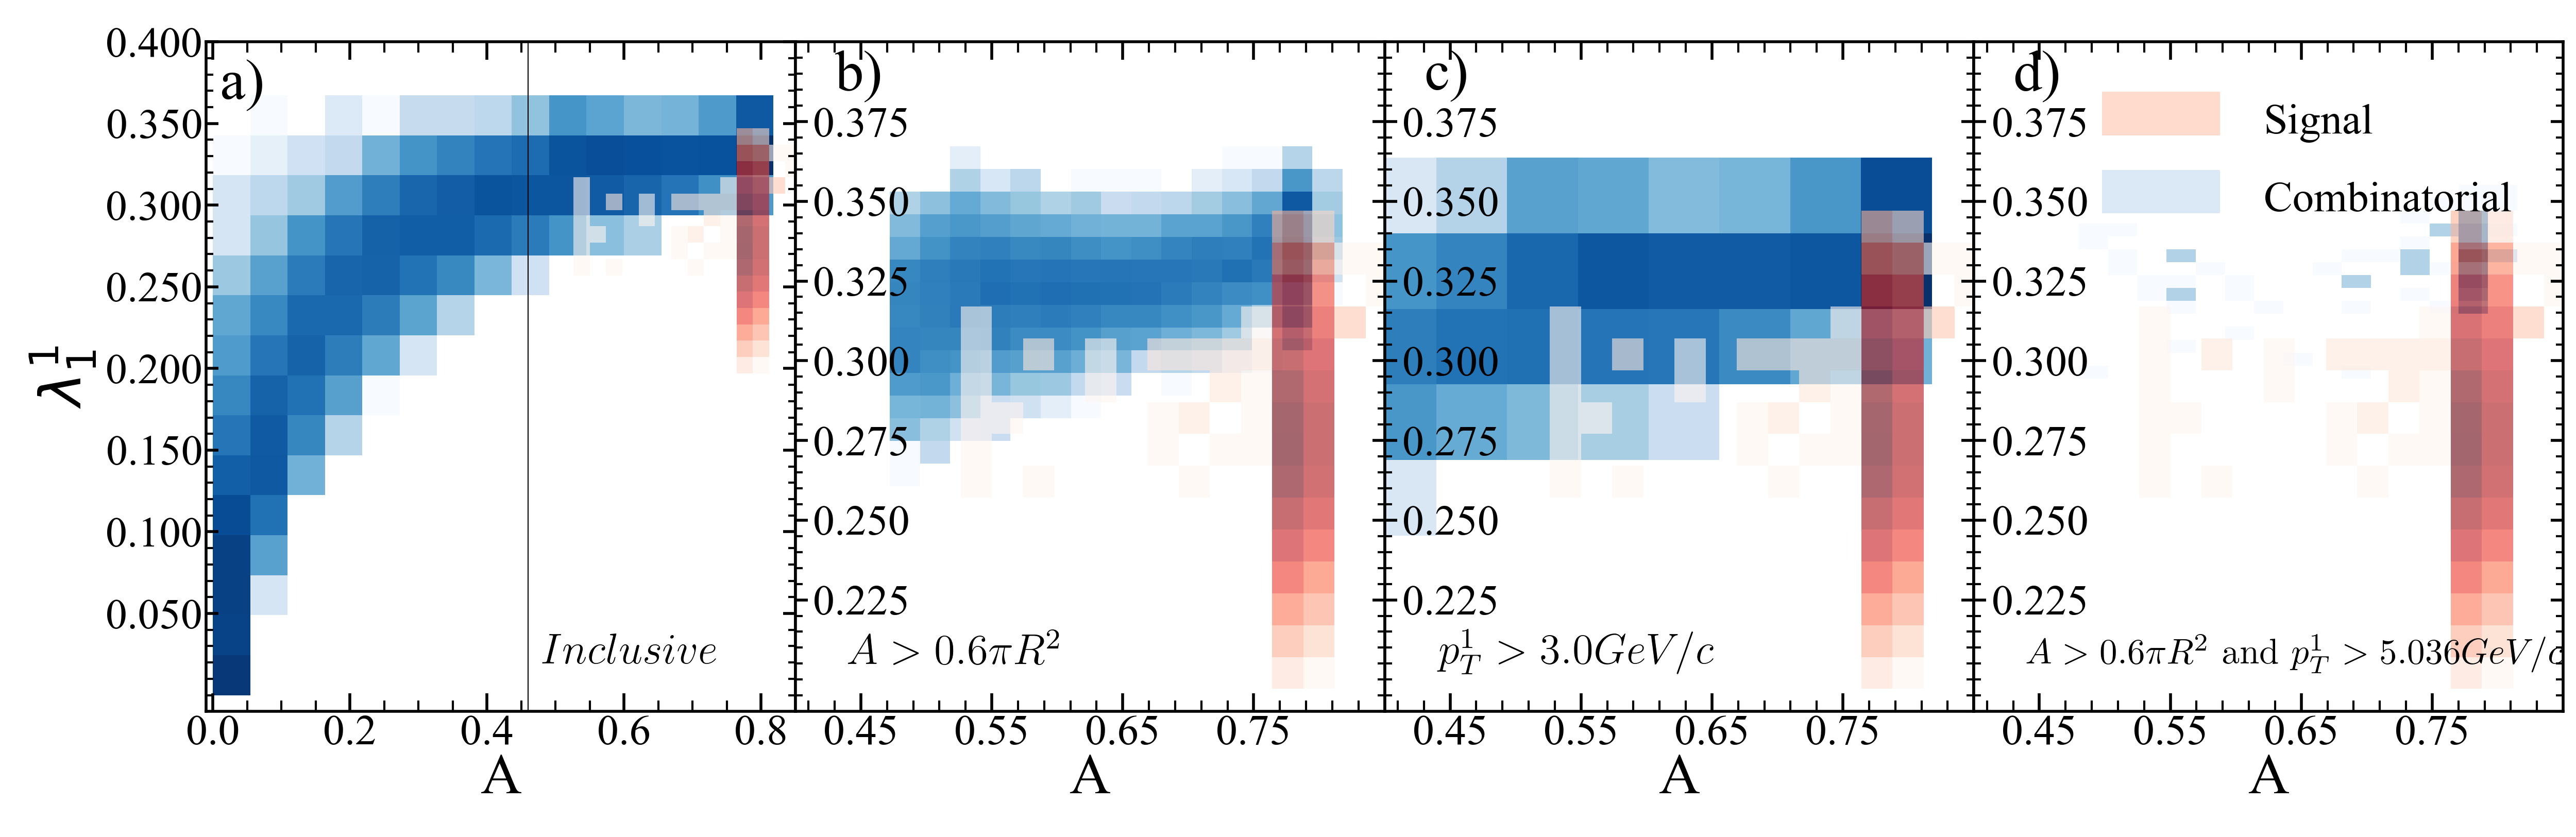}
    \caption{R=0.5 \ptH=60 \GeV}
    \label{fig:blob_05_60}
\end{figure*}

\begin{figure*}
    \centering
    \includegraphics[width=\linewidth]{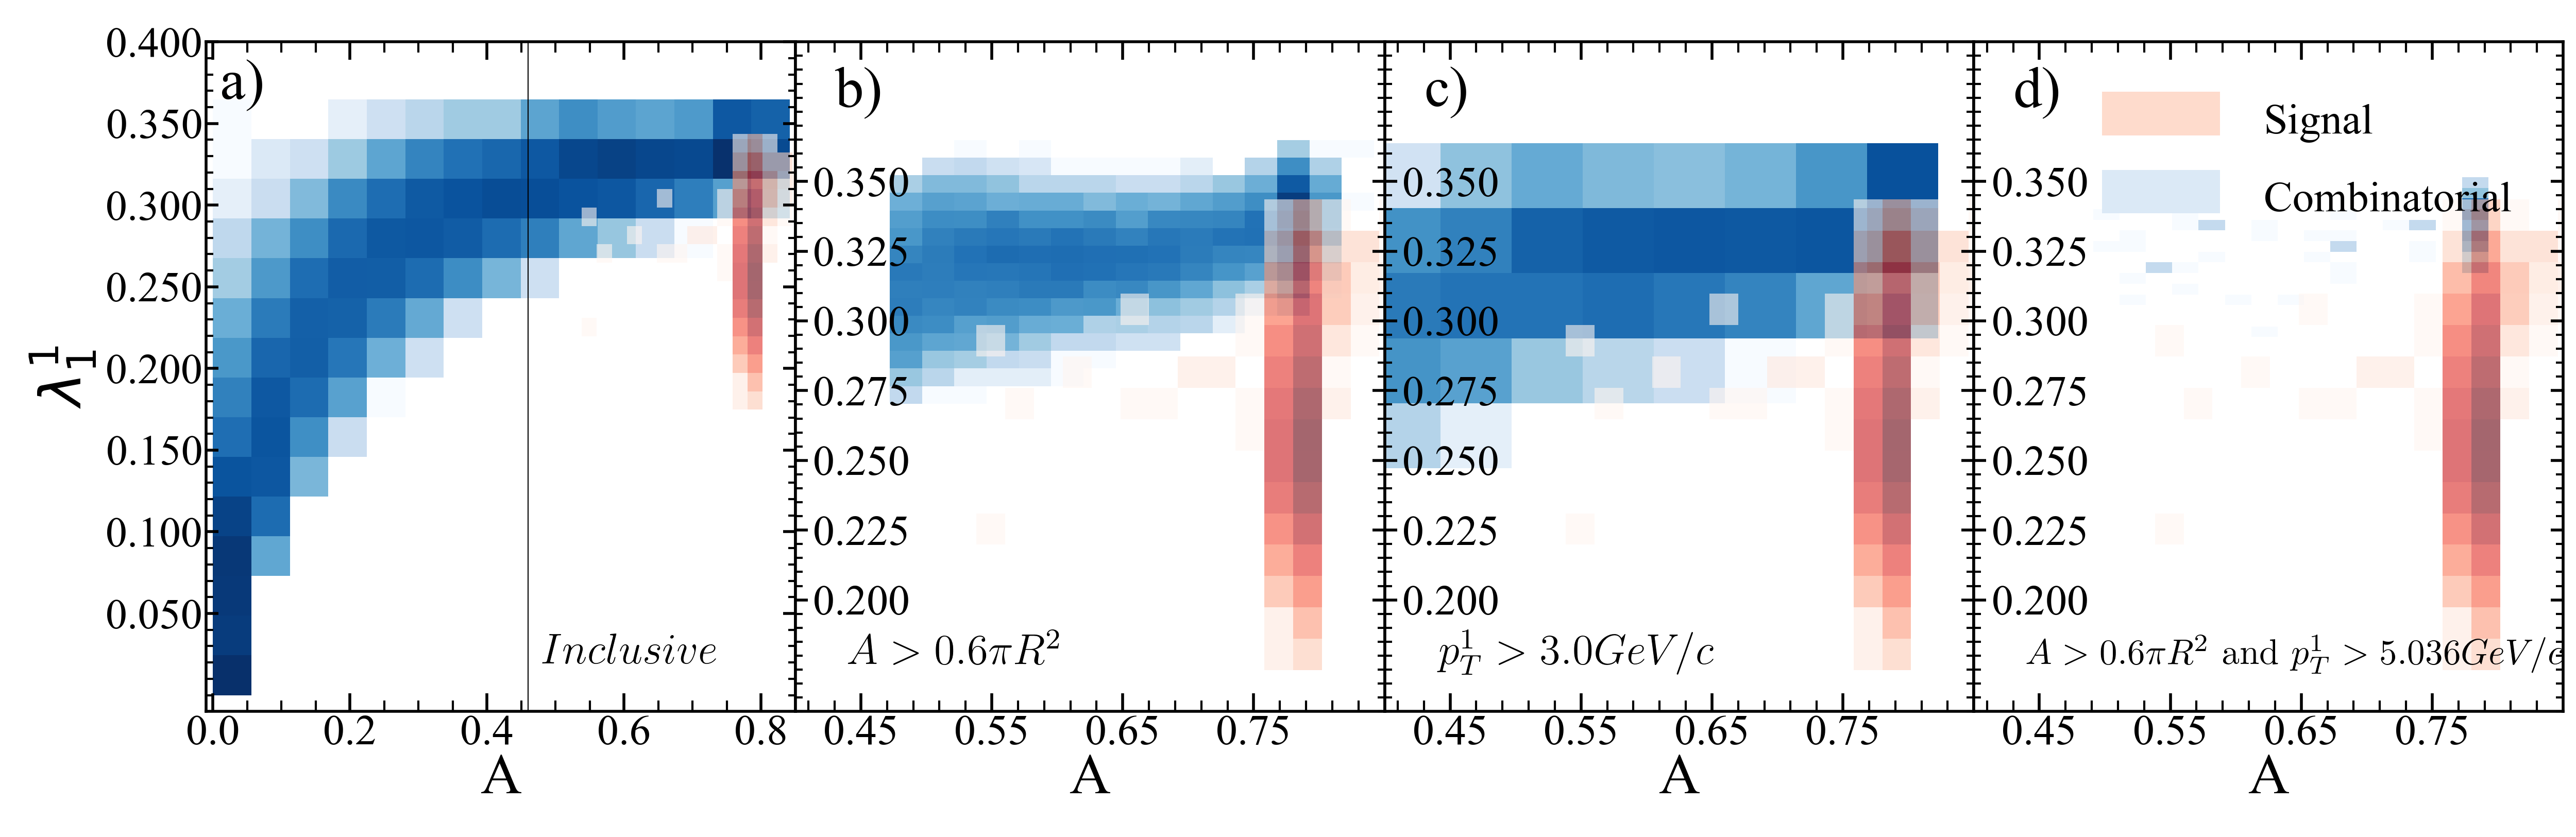}
    \caption{R=0.5 \ptH=80 \GeV}
    \label{fig:blob_05_80}
\end{figure*}

\begin{figure*}
    \centering
    \includegraphics[width=\linewidth]{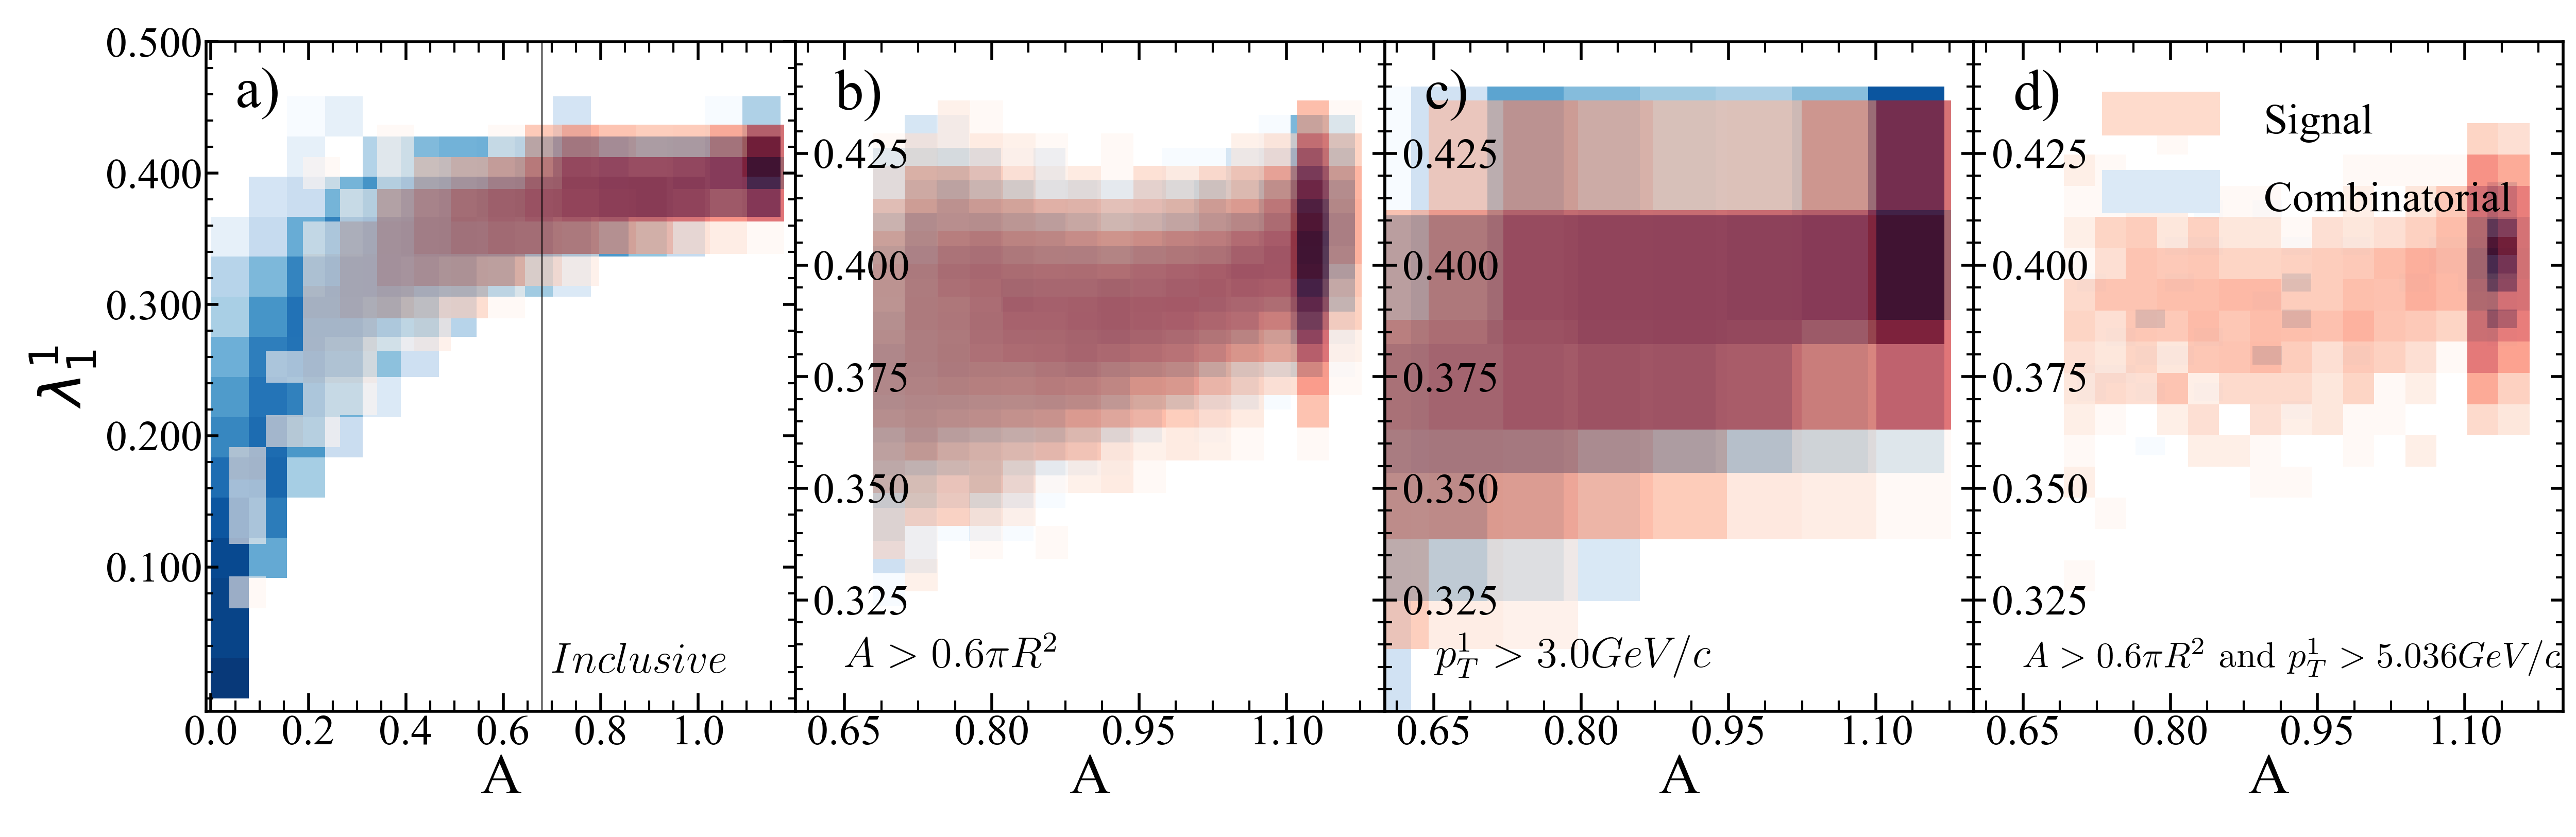}
    \caption{R=0.6 \ptH=10 \GeV}
    \label{fig:blob_06_10}
\end{figure*}

\begin{figure*}
    \centering
    \includegraphics[width=\linewidth]{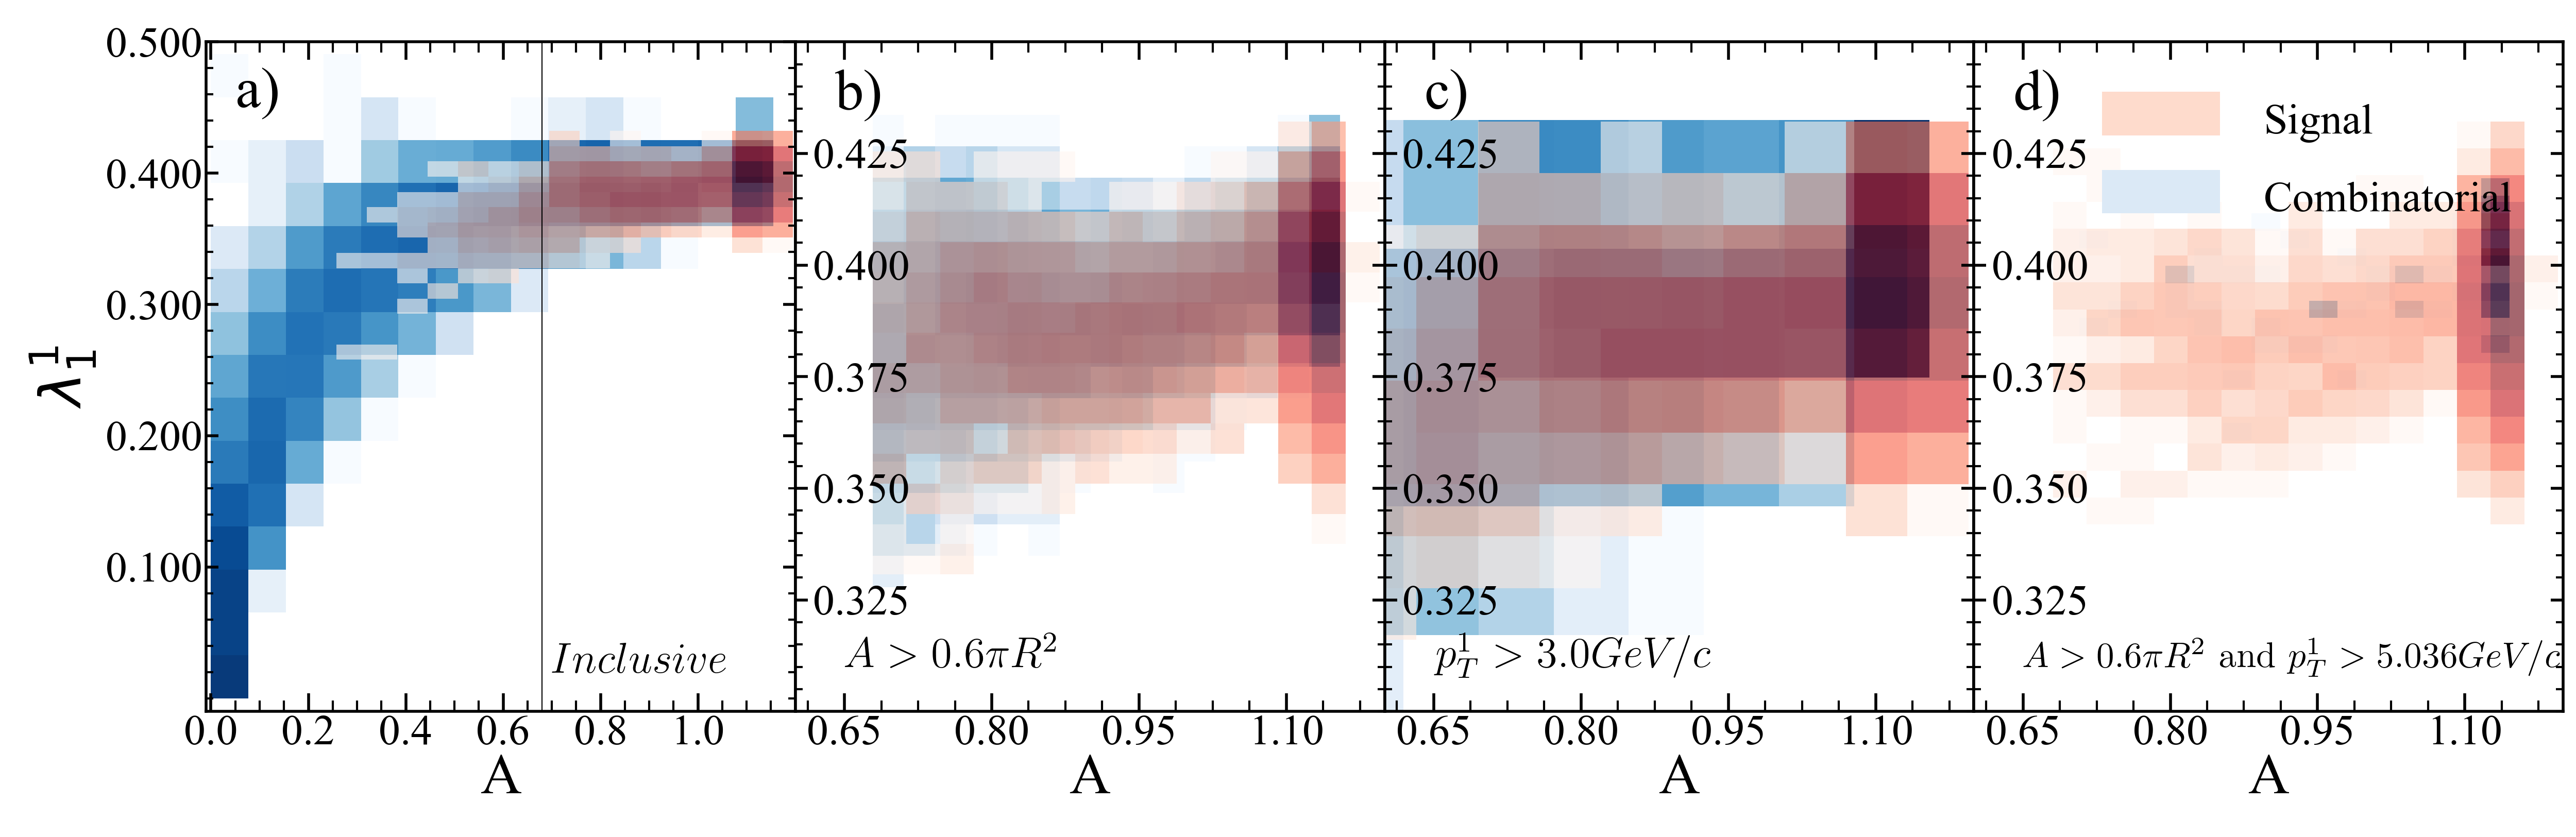}
    \caption{R=0.6 \ptH=20 \GeV}
    \label{fig:blob_06_20}
\end{figure*}

\begin{figure*}
    \centering
    \includegraphics[width=\linewidth]{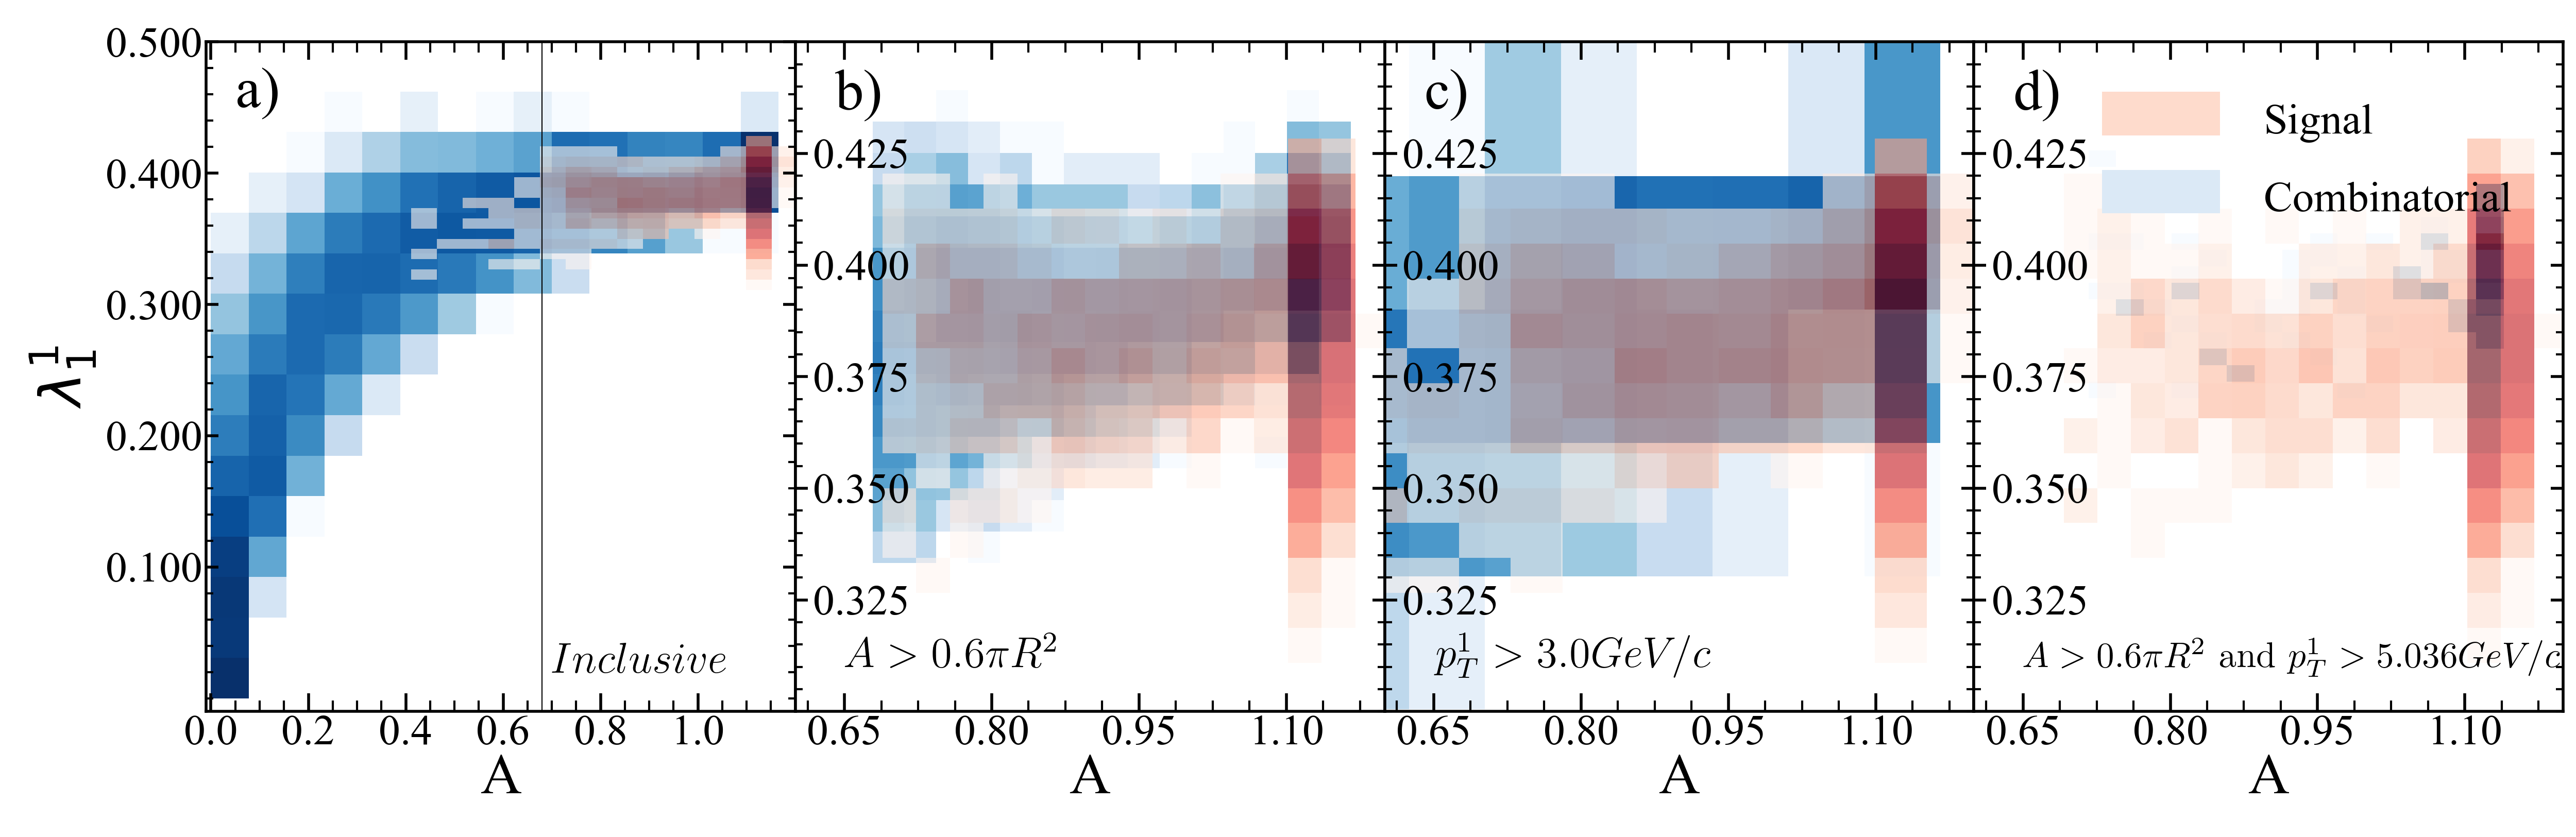}
    \caption{R=0.6 \ptH=30 \GeV}
    \label{fig:blob_06_30}
\end{figure*}

\begin{figure*}
    \centering
    \includegraphics[width=\linewidth]{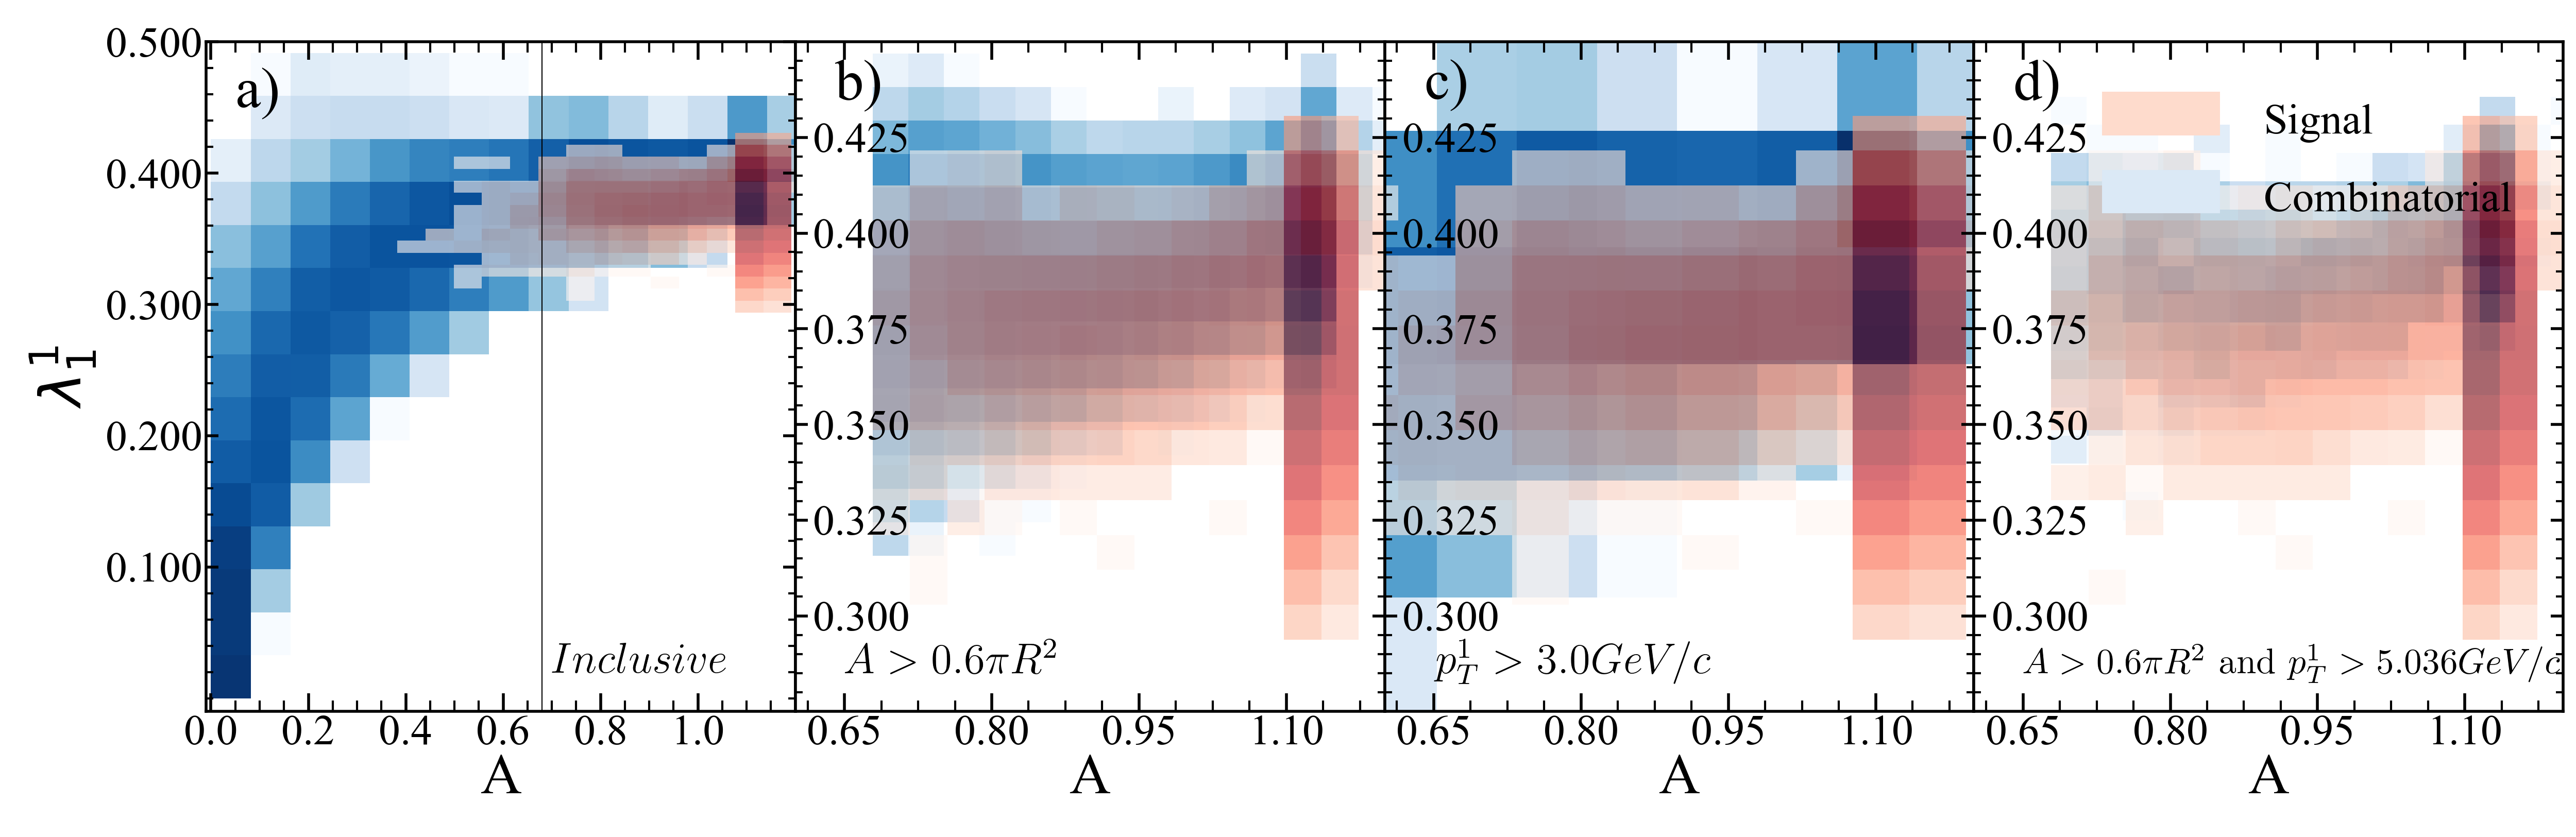}
    \caption{R=0.6 \ptH=40 \GeV}
    \label{fig:blob_06_40}
\end{figure*}

\begin{figure*}
    \centering
    \includegraphics[width=\linewidth]{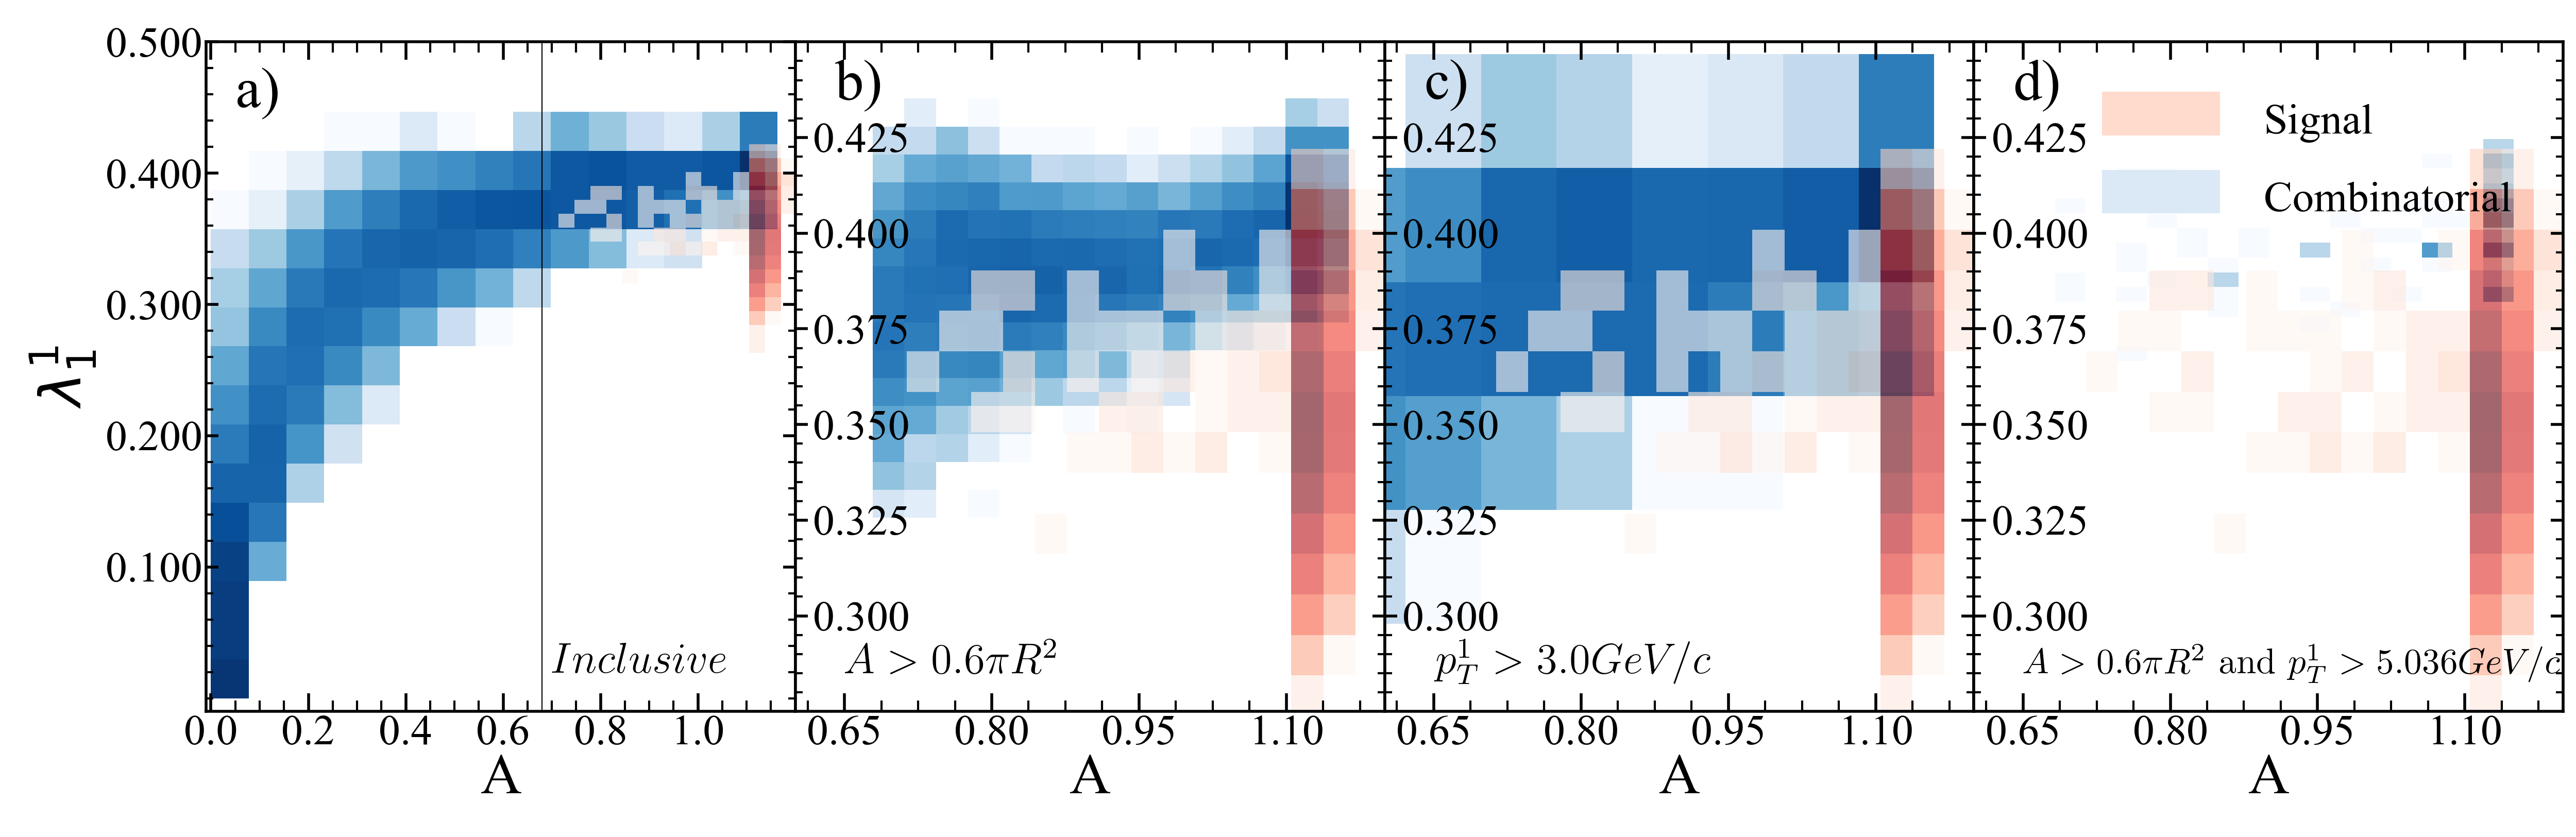}
    \caption{R=0.6 \ptH=60 \GeV}
    \label{fig:blob_06_60}
\end{figure*}

\begin{figure*}
    \centering
    \includegraphics[width=\linewidth]{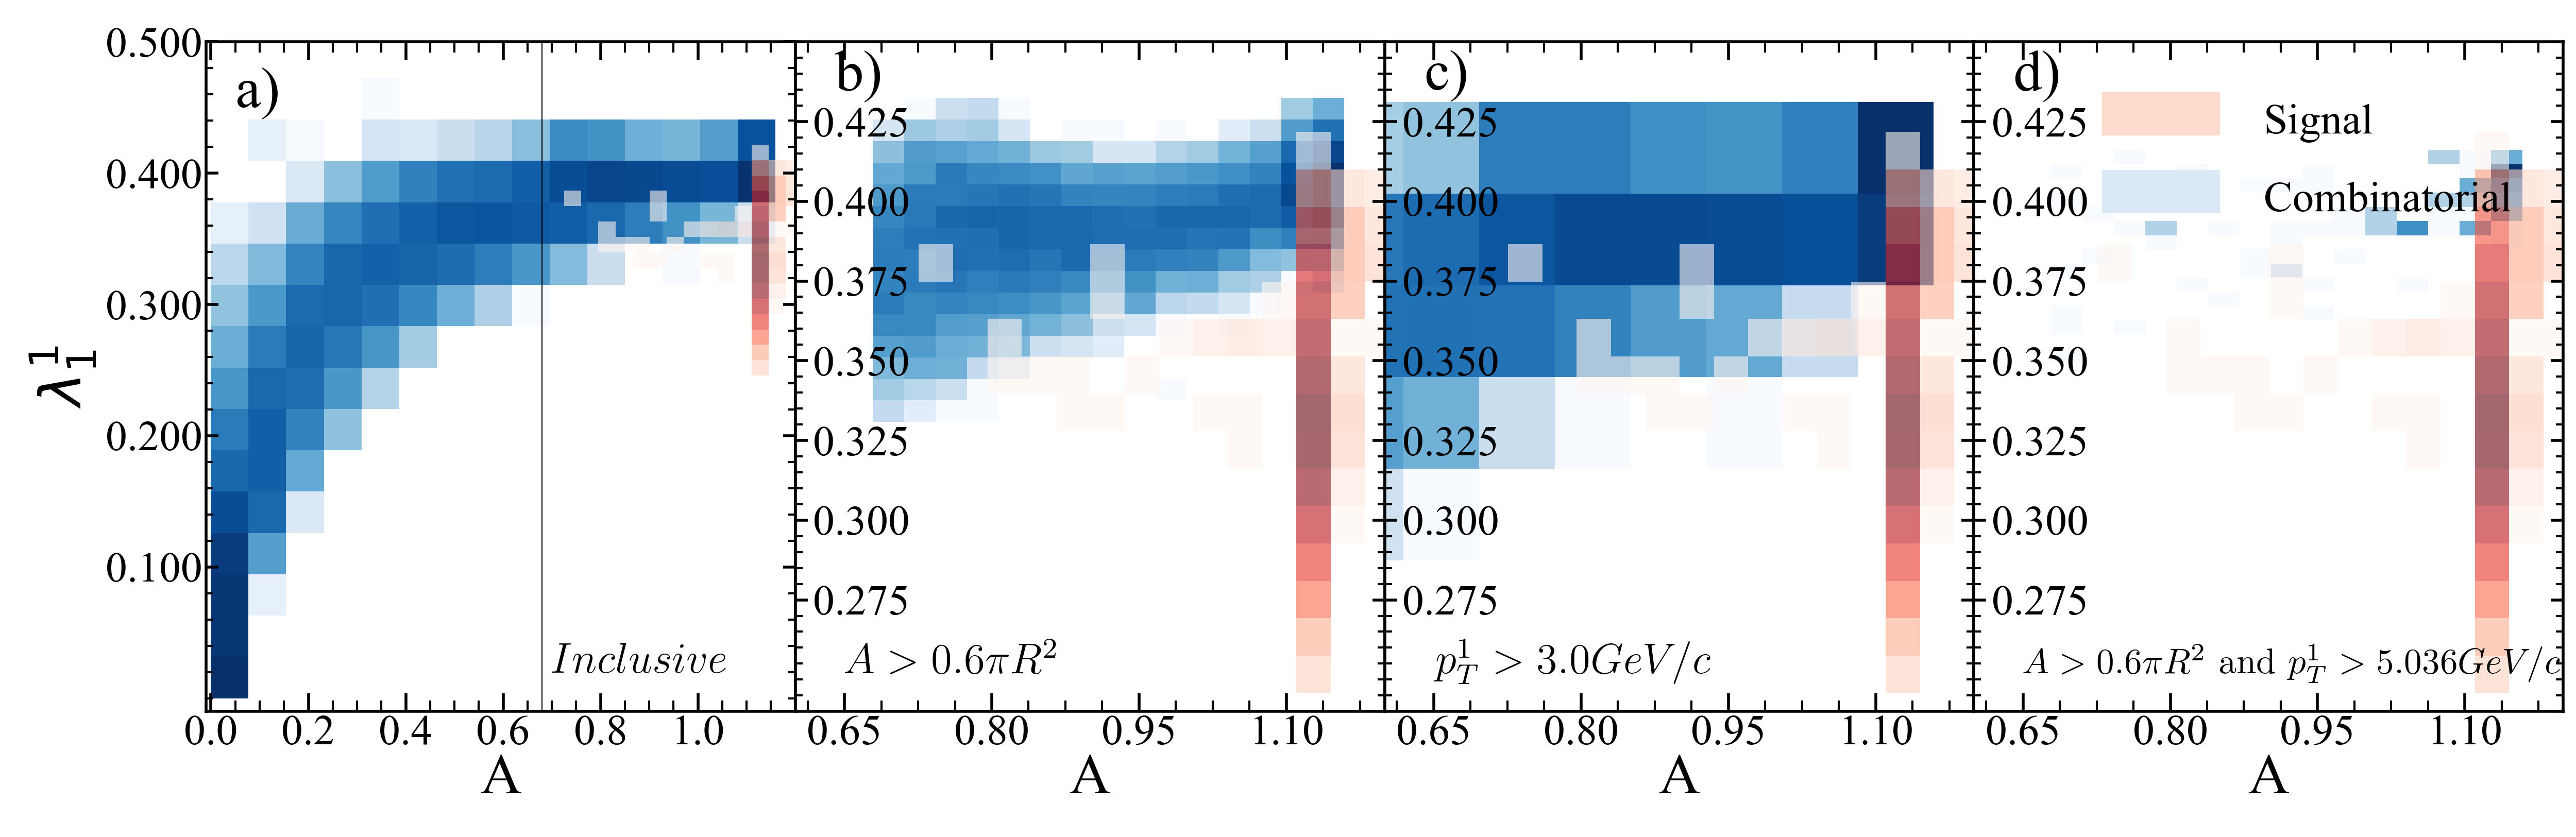}
    \caption{R=0.6 \ptH=80 \GeV}
    \label{fig:blob_06_80}
\end{figure*}
\clearpage
\subsection{Leading hadron momentum, jet width, and mean constituent momentum after applying the area selection.}

\begin{figure*}
    \centering
    \includegraphics[width=\linewidth]{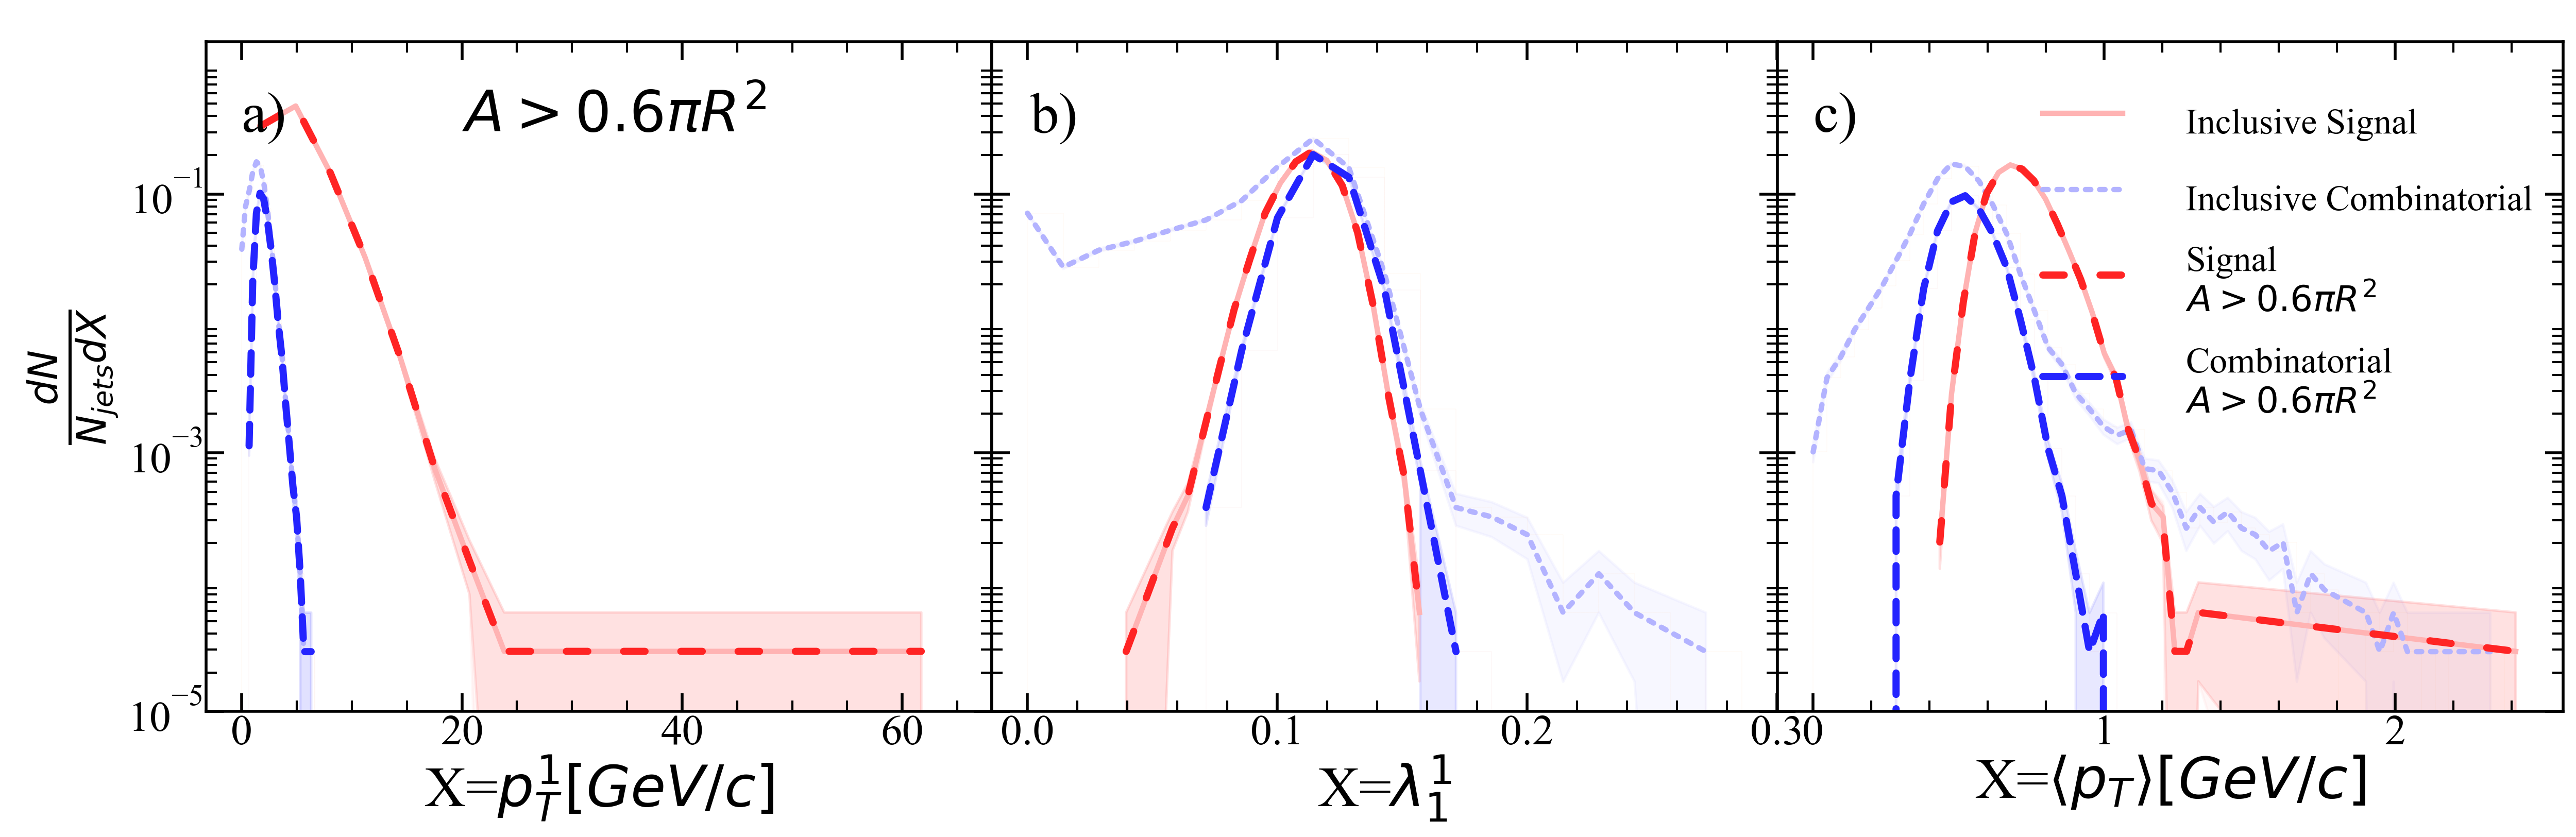}
    \caption{R=0.2 \ptH=10 \GeV}
    \label{fig:area_02_10}
\end{figure*}

\begin{figure*}
    \centering
    \includegraphics[width=\linewidth]{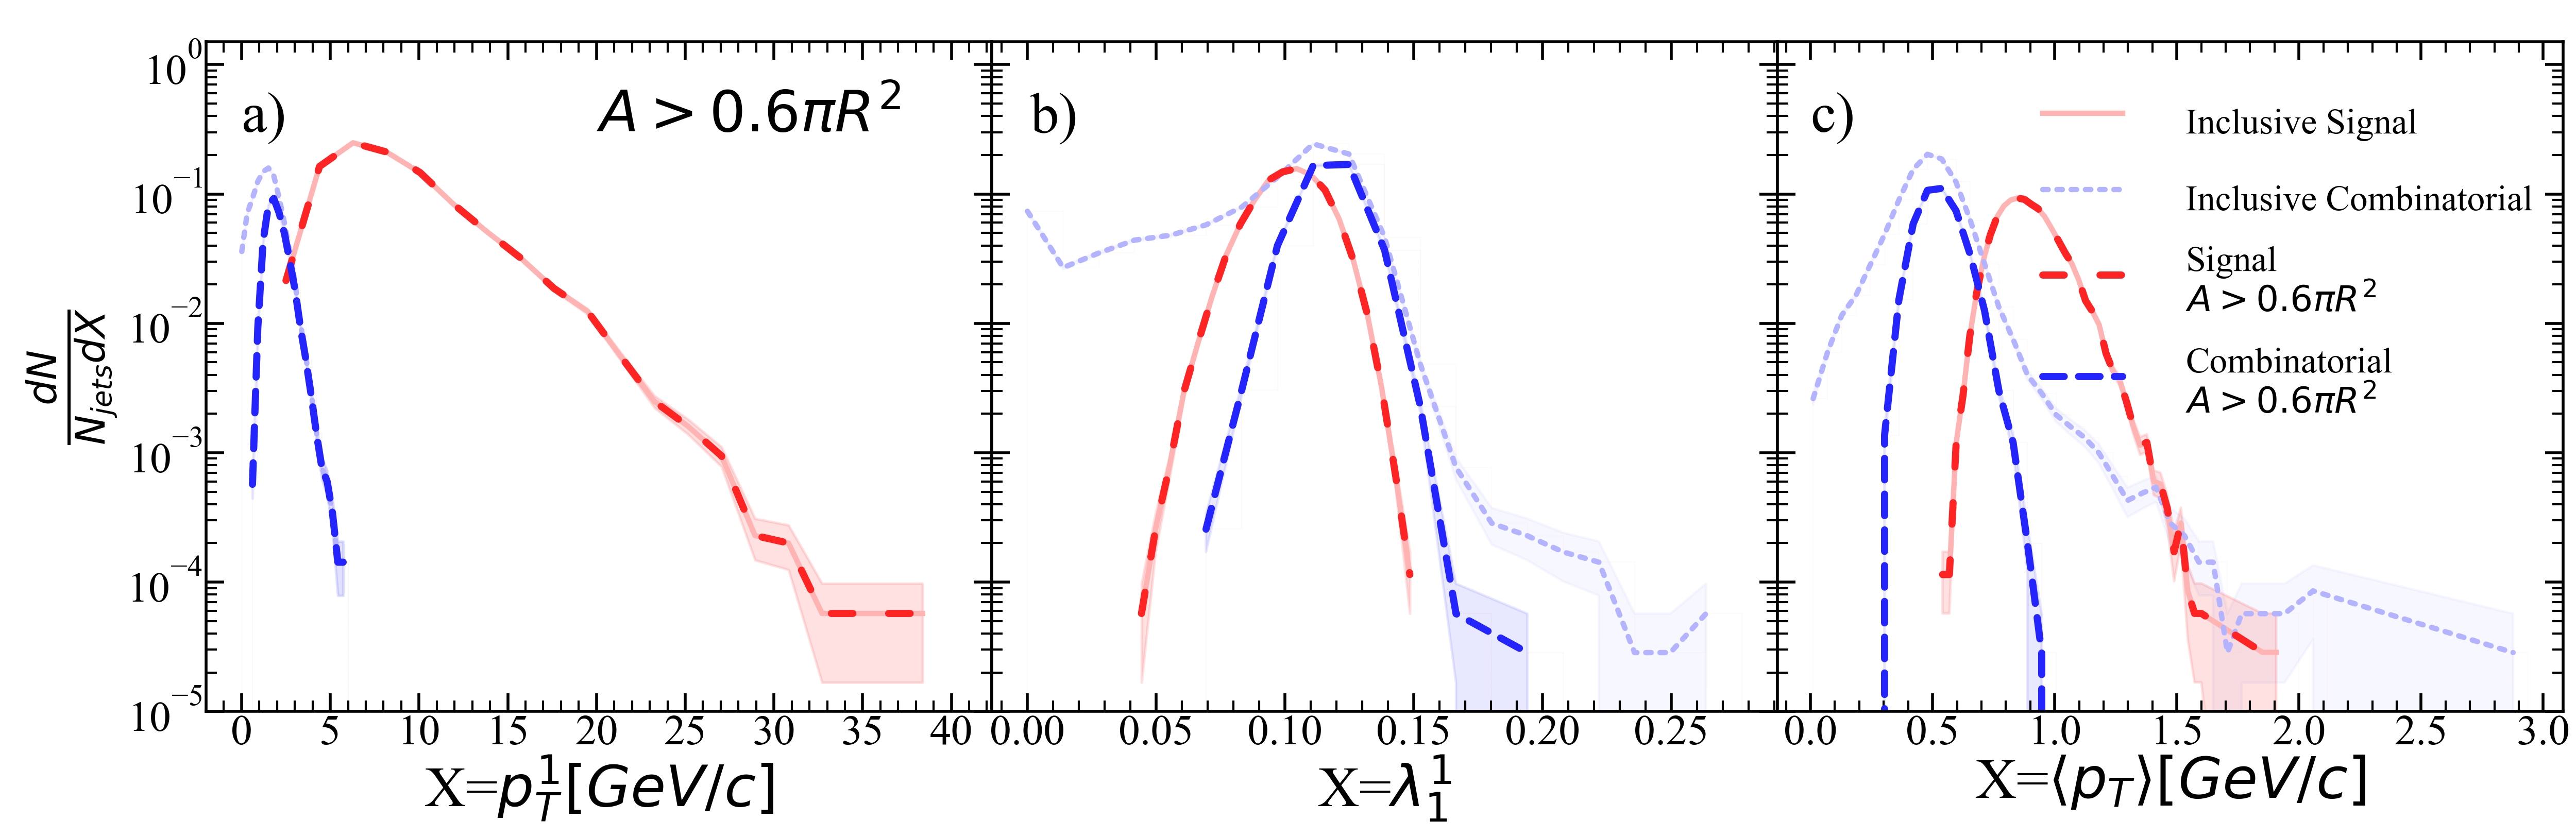}
    \caption{R=0.2 \ptH=20 \GeV}
    \label{fig:area_02_20}
\end{figure*}

\begin{figure*}
    \centering
    \includegraphics[width=\linewidth]{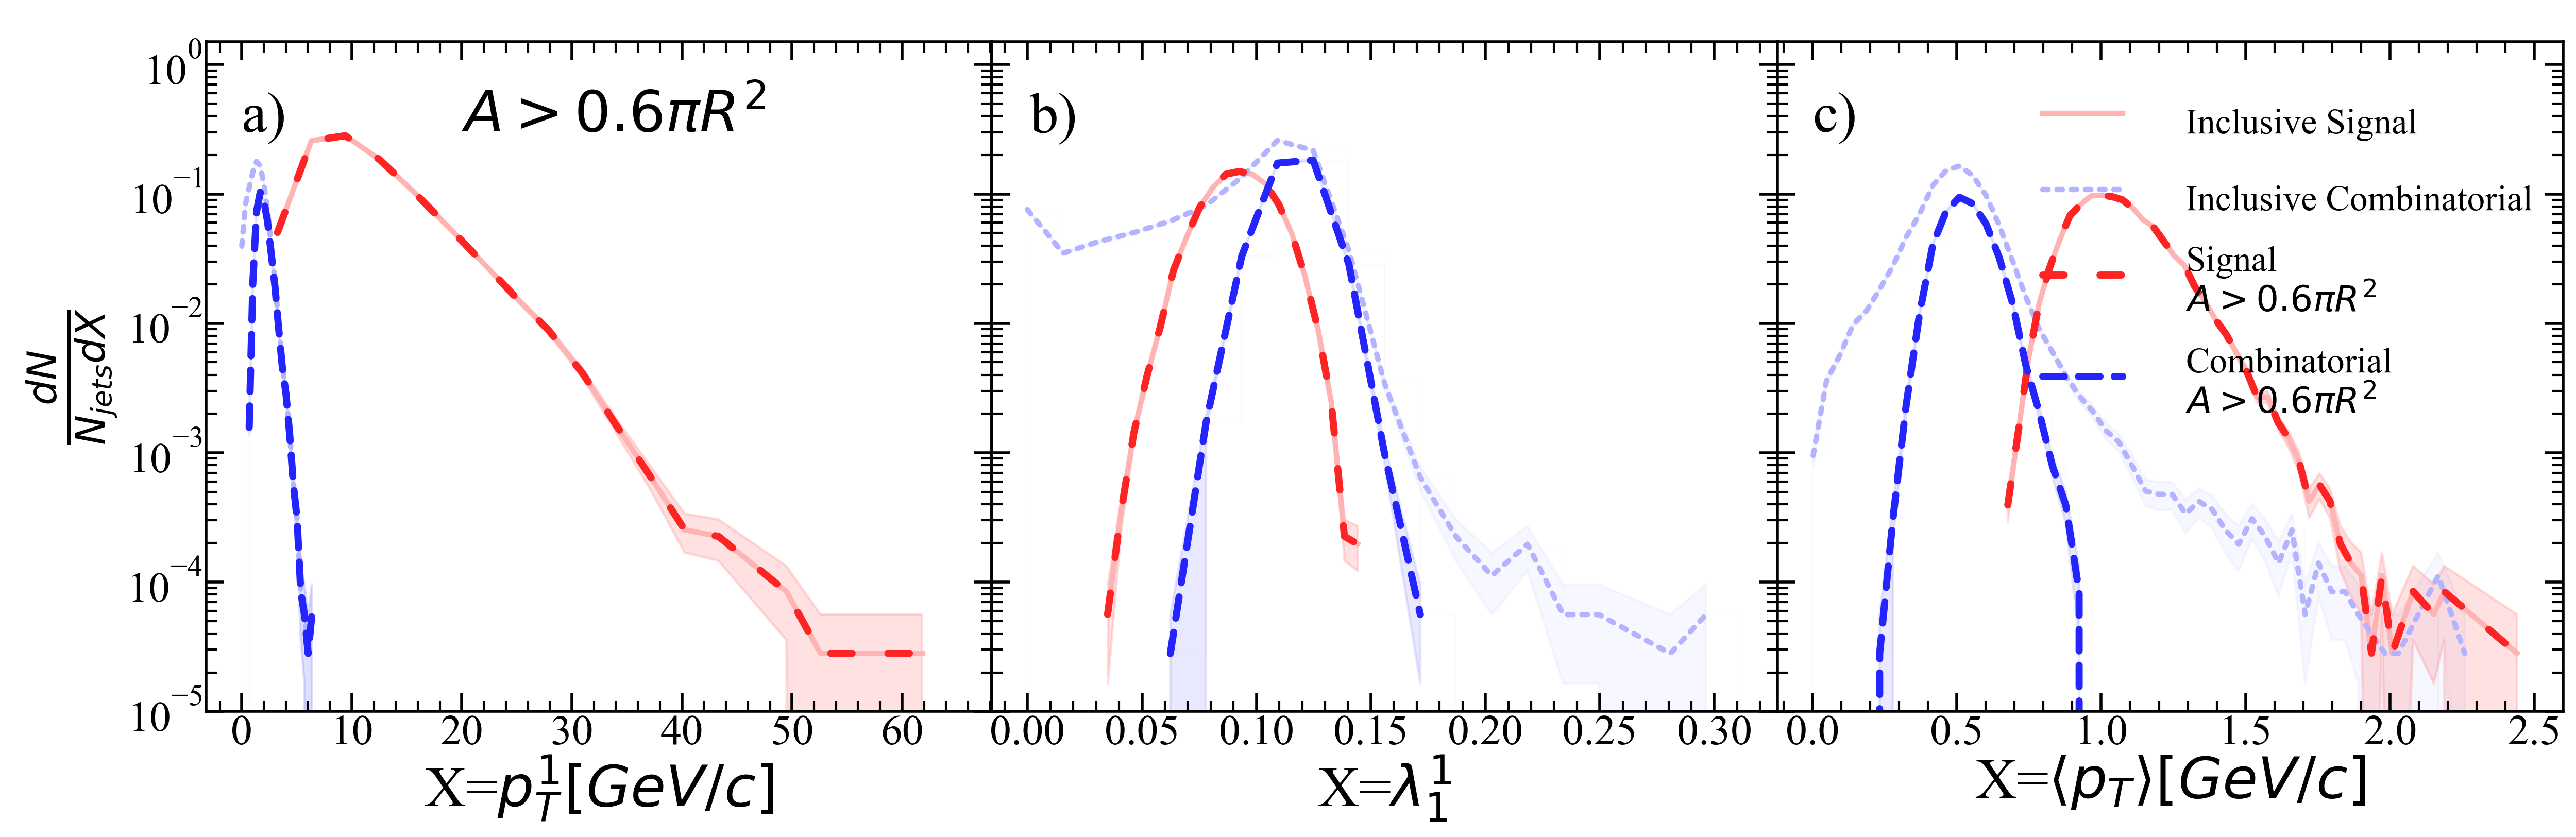}
    \caption{R=0.2 \ptH=30 \GeV}
    \label{fig:area_02_30}
\end{figure*}

\begin{figure*}
    \centering
    \includegraphics[width=\linewidth]{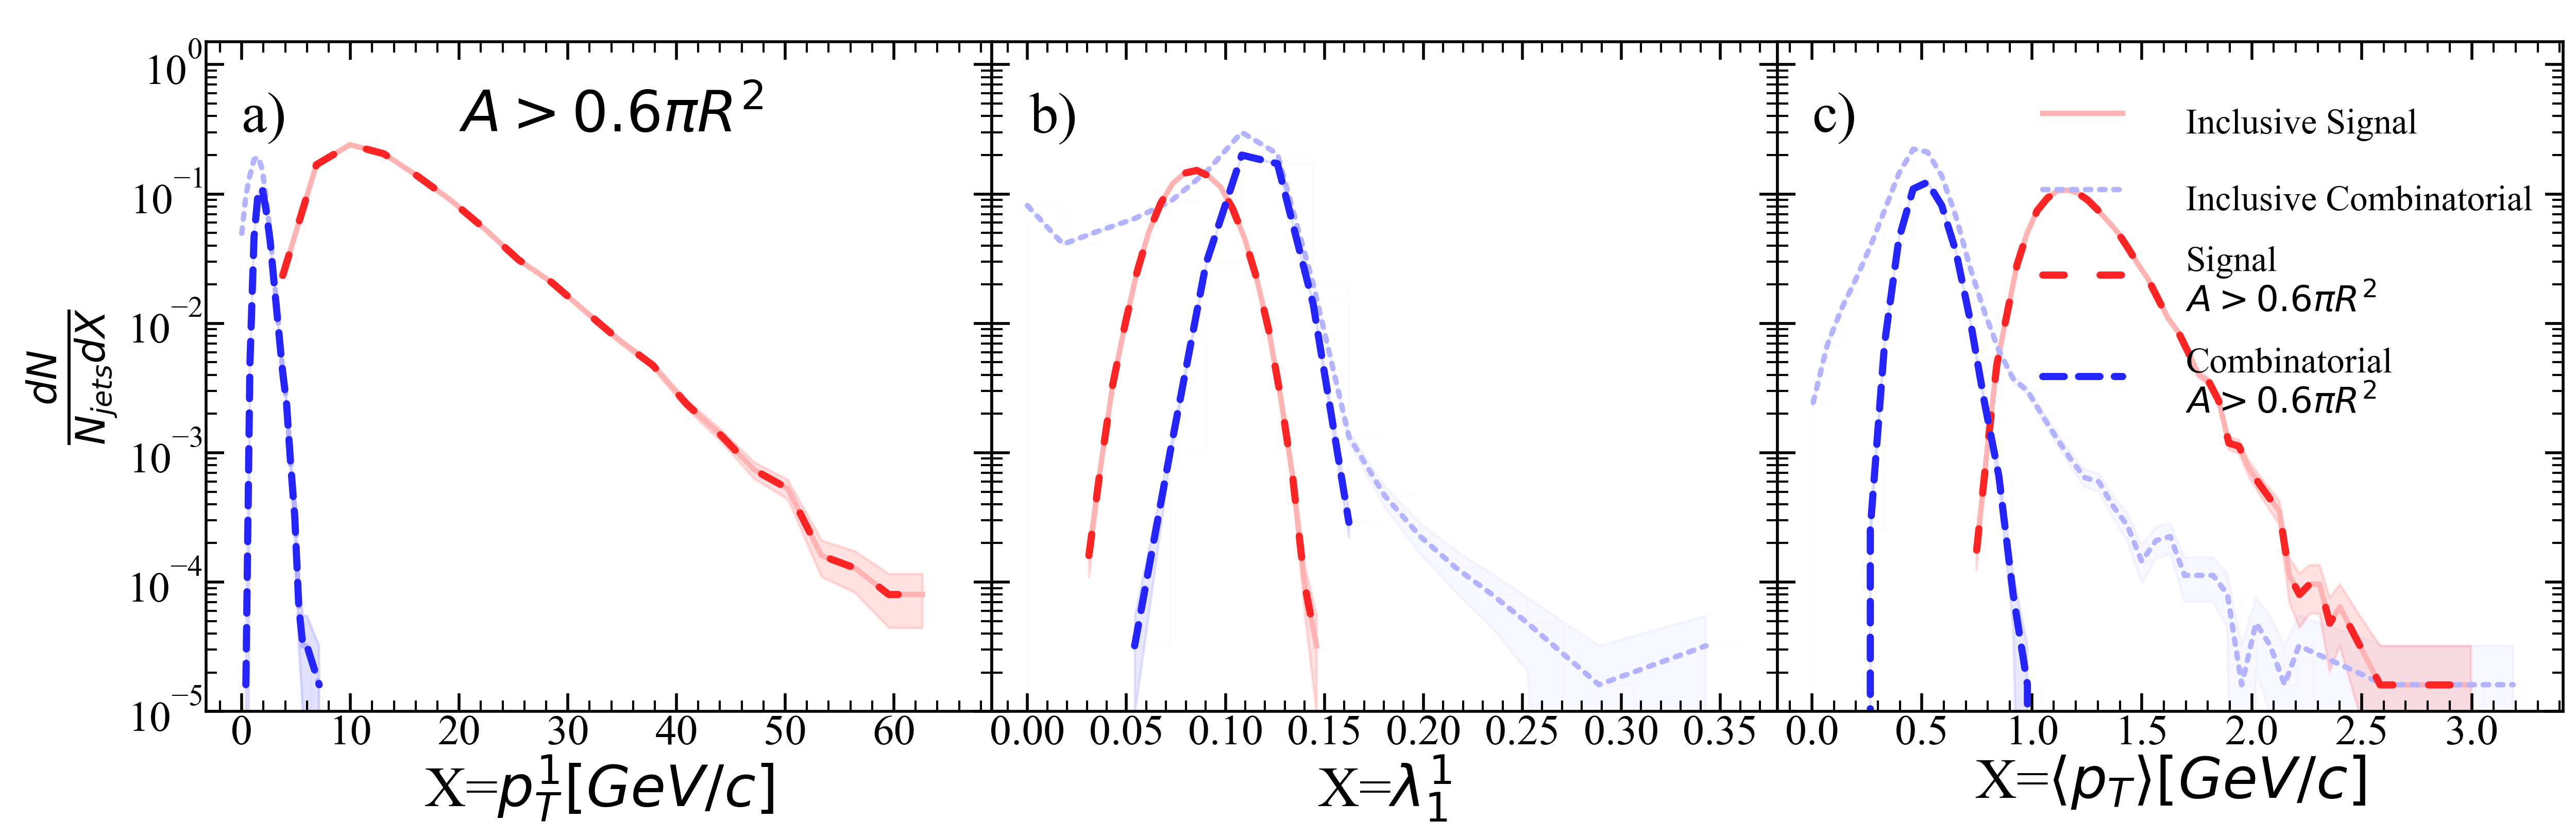}
    \caption{R=0.2 \ptH=40 \GeV}
    \label{fig:area_02_40}
\end{figure*}

\begin{figure*}
    \centering
    \includegraphics[width=\linewidth]{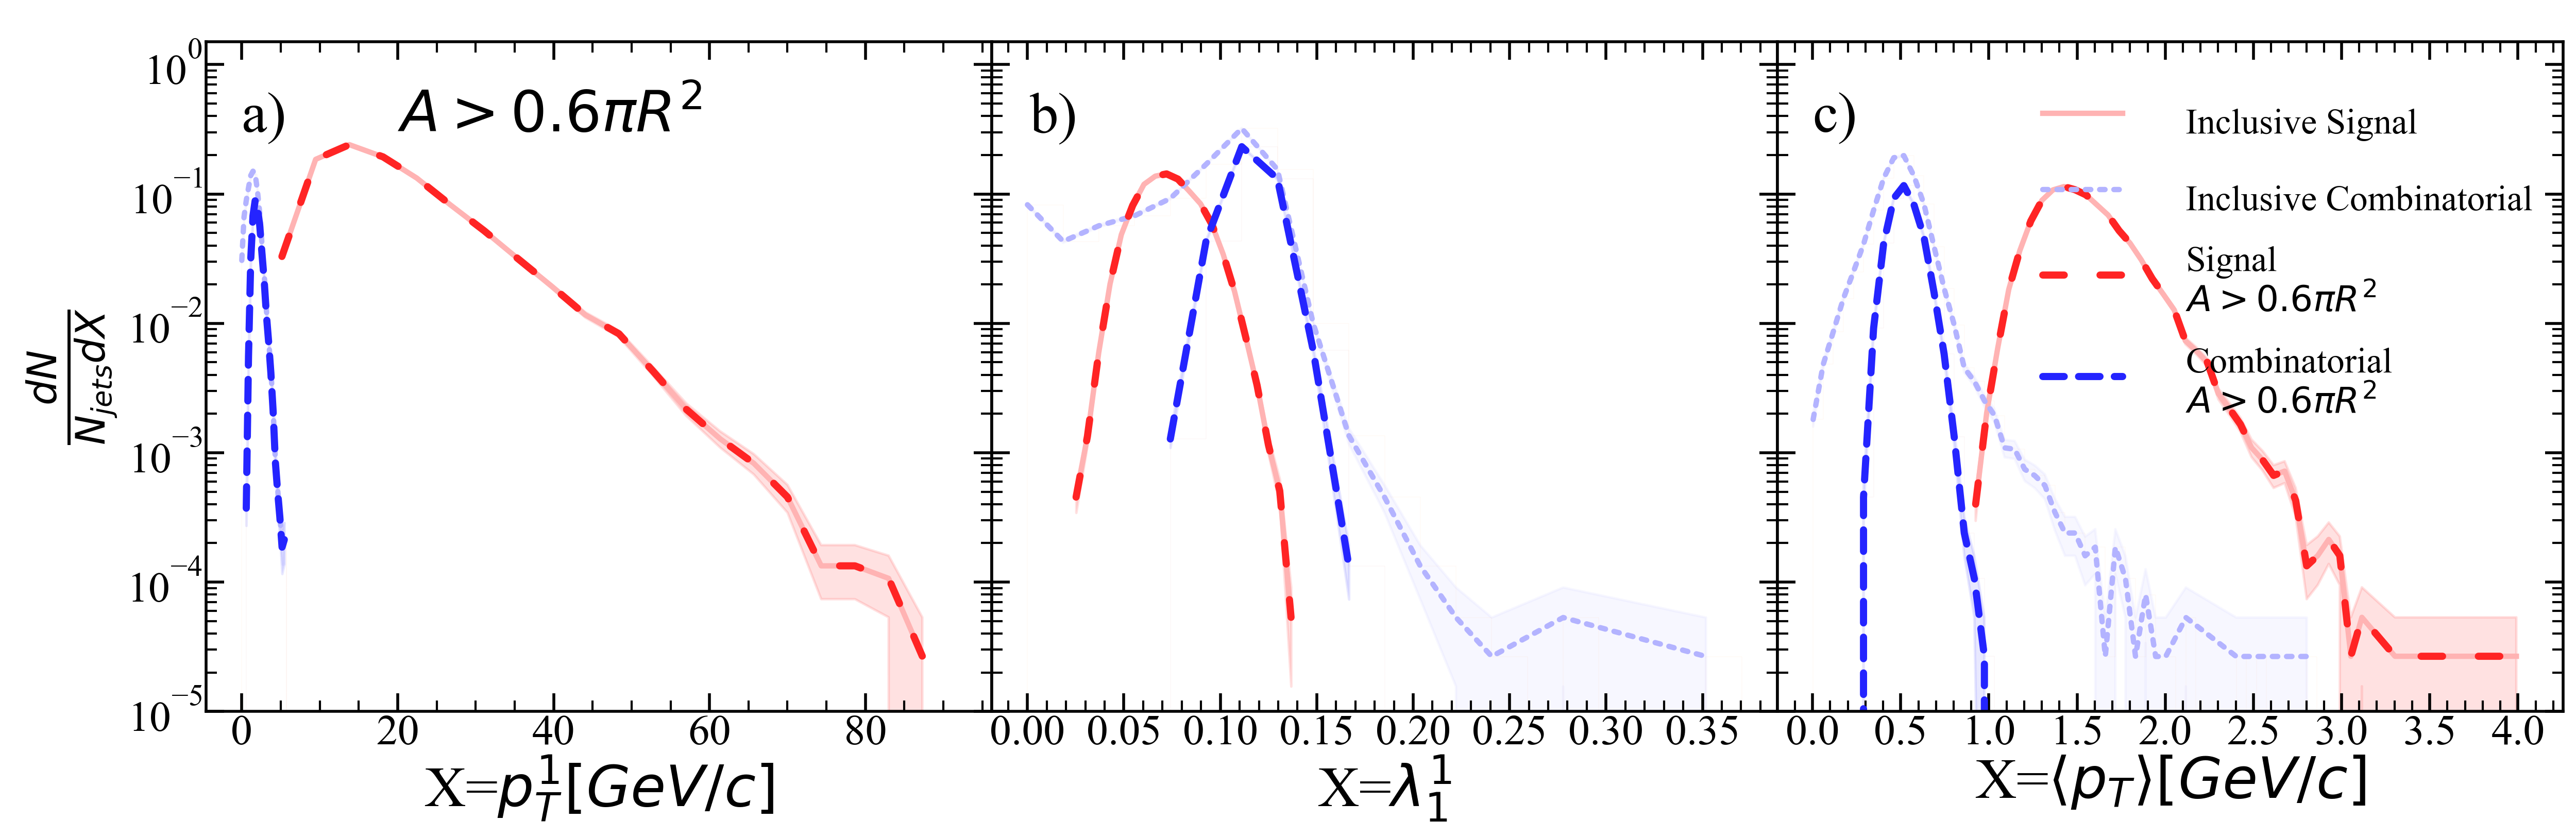}
    \caption{R=0.2 \ptH=60 \GeV}
    \label{fig:area_02_60}
\end{figure*}

\begin{figure*}
    \centering
    \includegraphics[width=\linewidth]{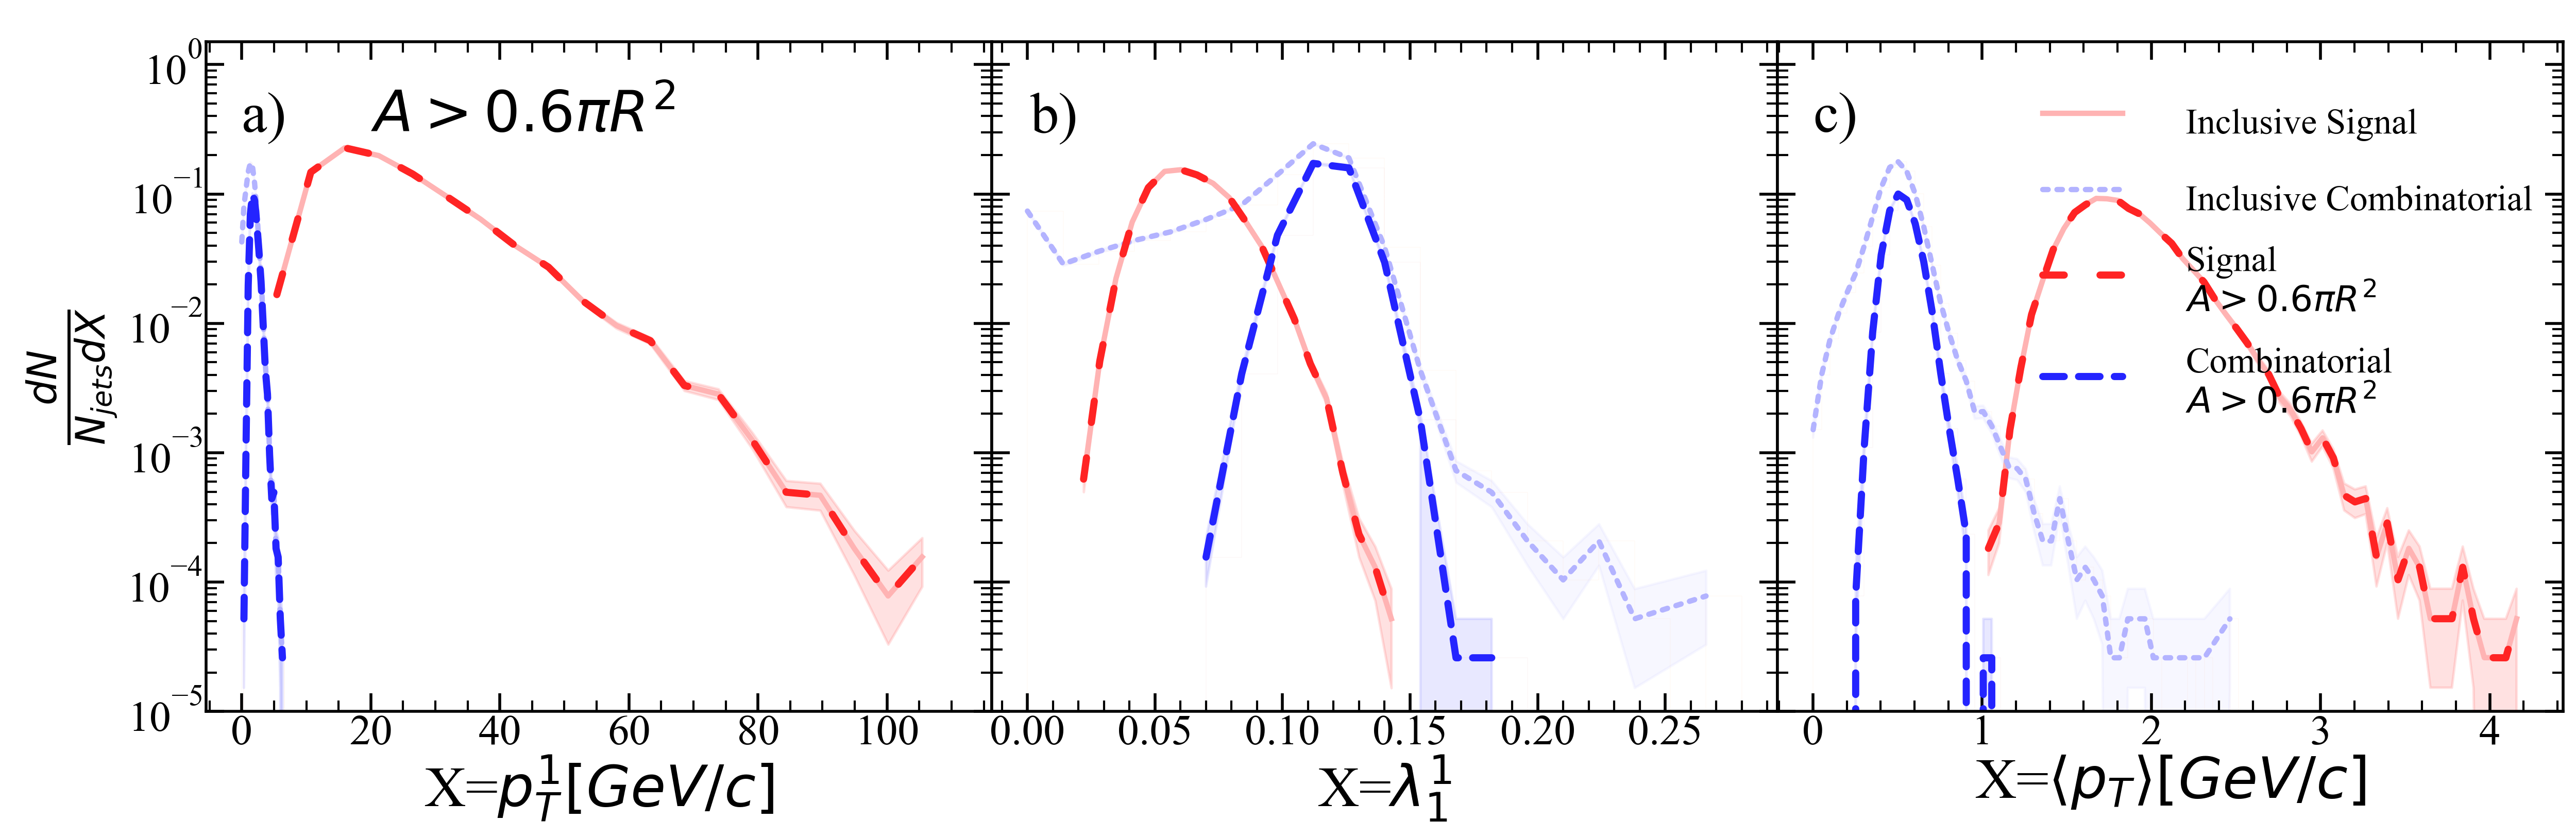}
    \caption{R=0.2 \ptH=80 \GeV}
    \label{fig:area_02_80}
\end{figure*}

\begin{figure*}
    \centering
    \includegraphics[width=\linewidth]{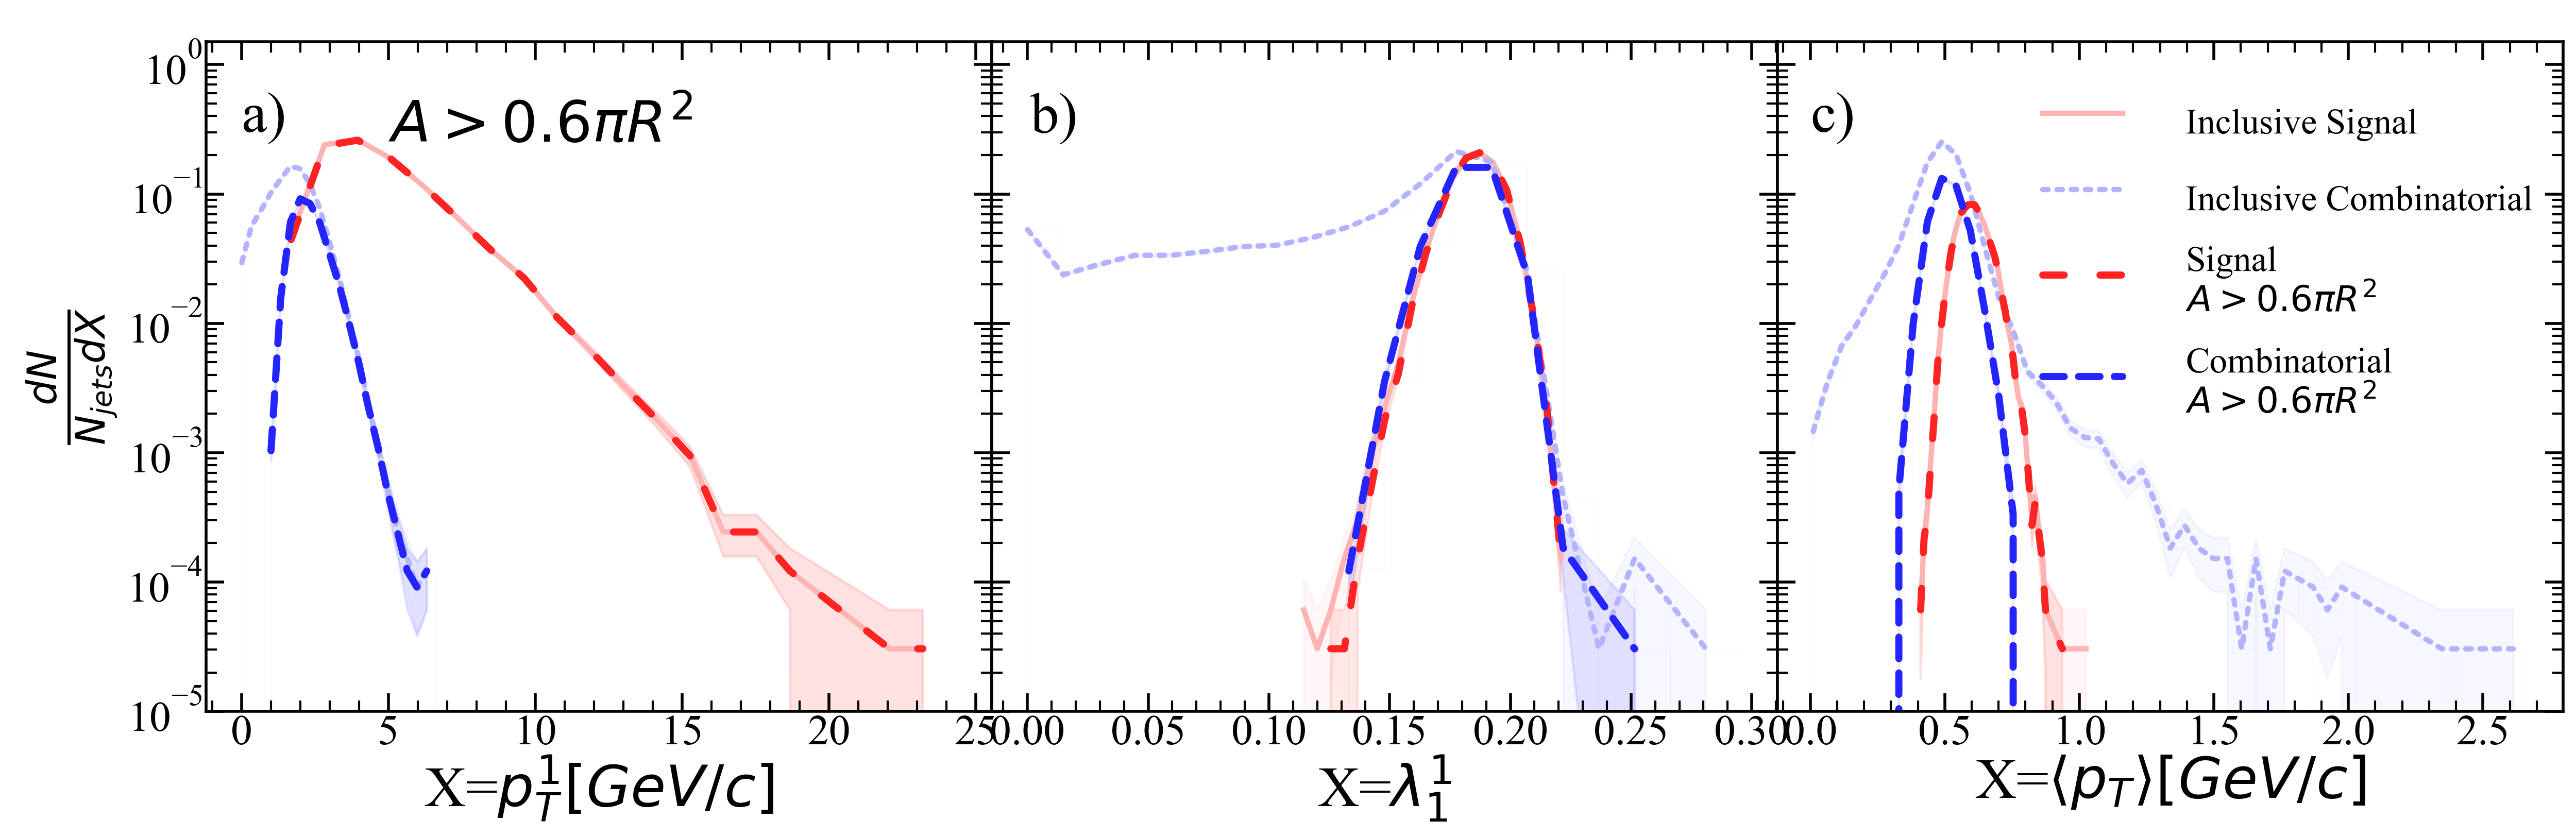}
    \caption{R=0.3 \ptH=10 \GeV}
    \label{fig:area_03_10}
\end{figure*}

\begin{figure*}
    \centering
    \includegraphics[width=\linewidth]{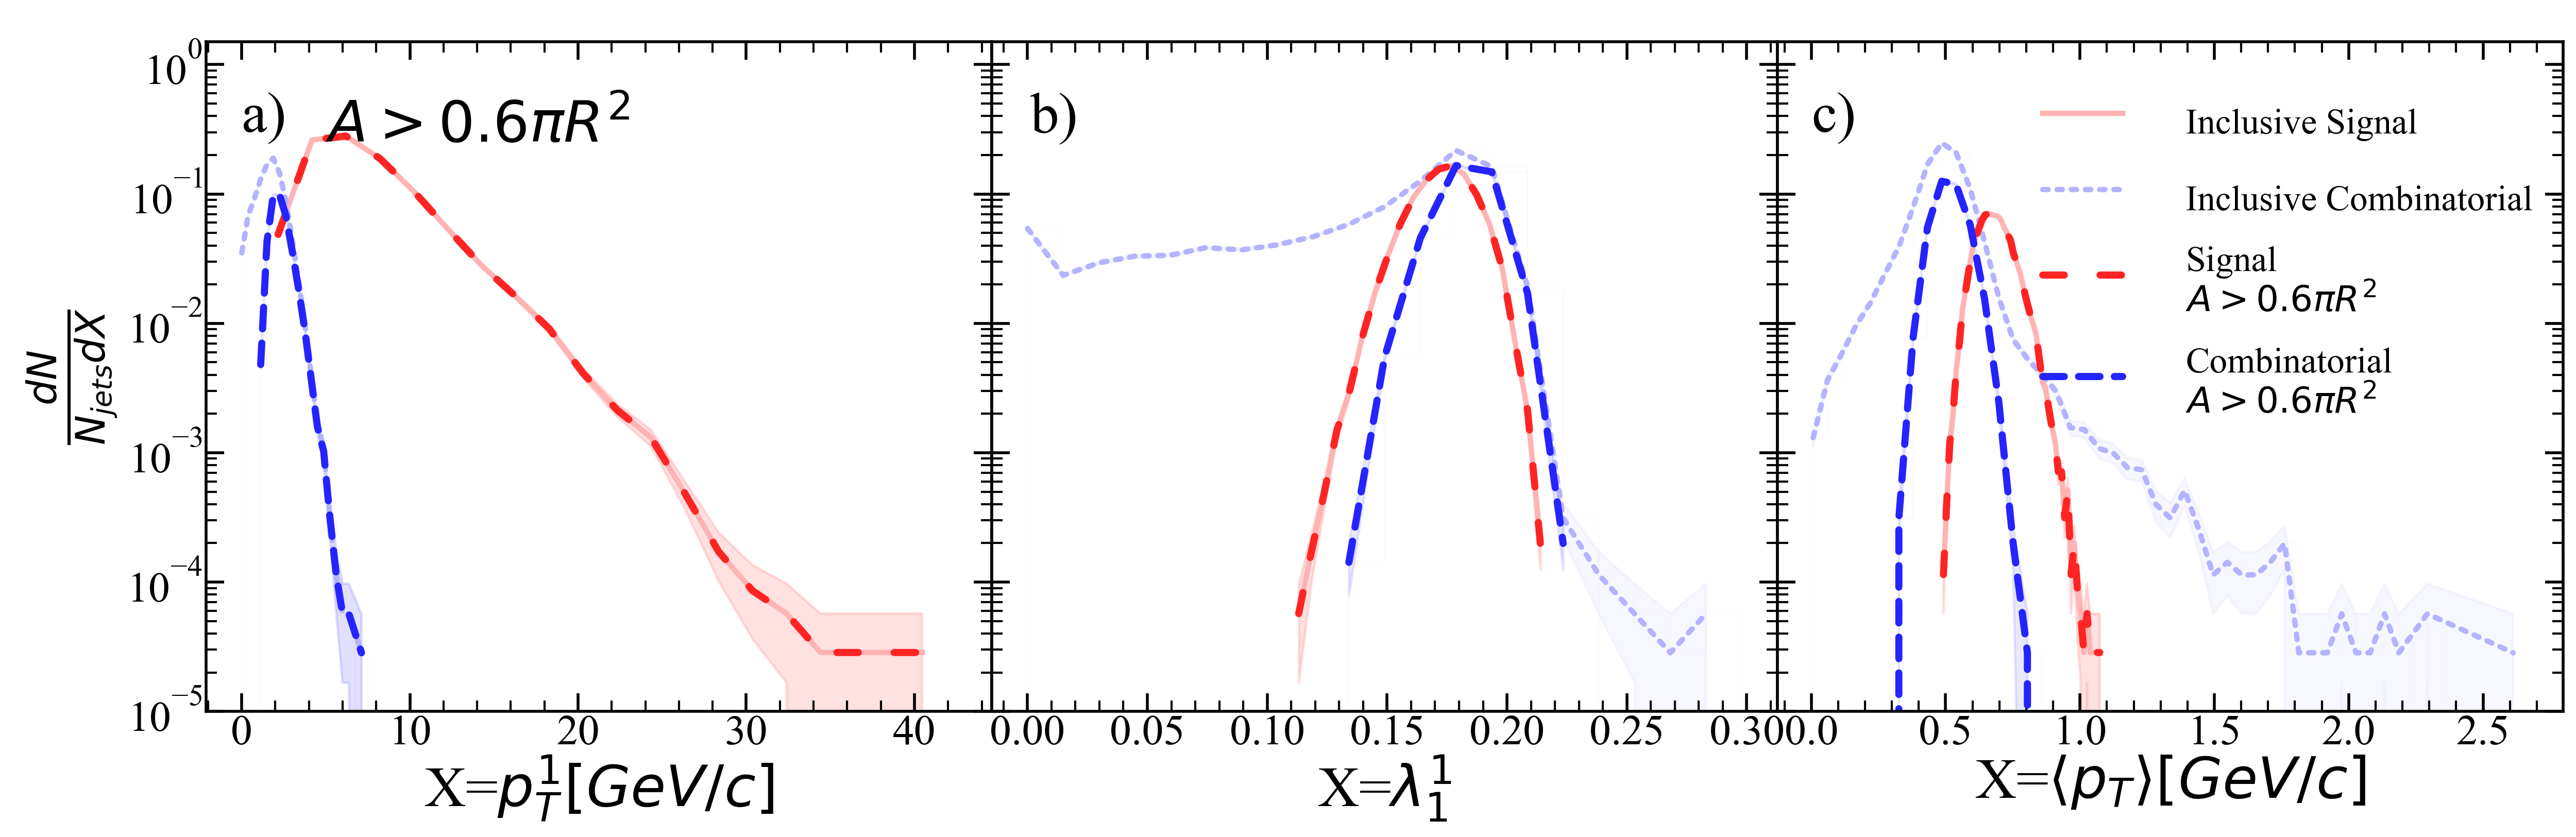}
    \caption{R=0.3 \ptH=20 \GeV}
    \label{fig:area_03_20}
\end{figure*}

\begin{figure*}
    \centering
    \includegraphics[width=\linewidth]{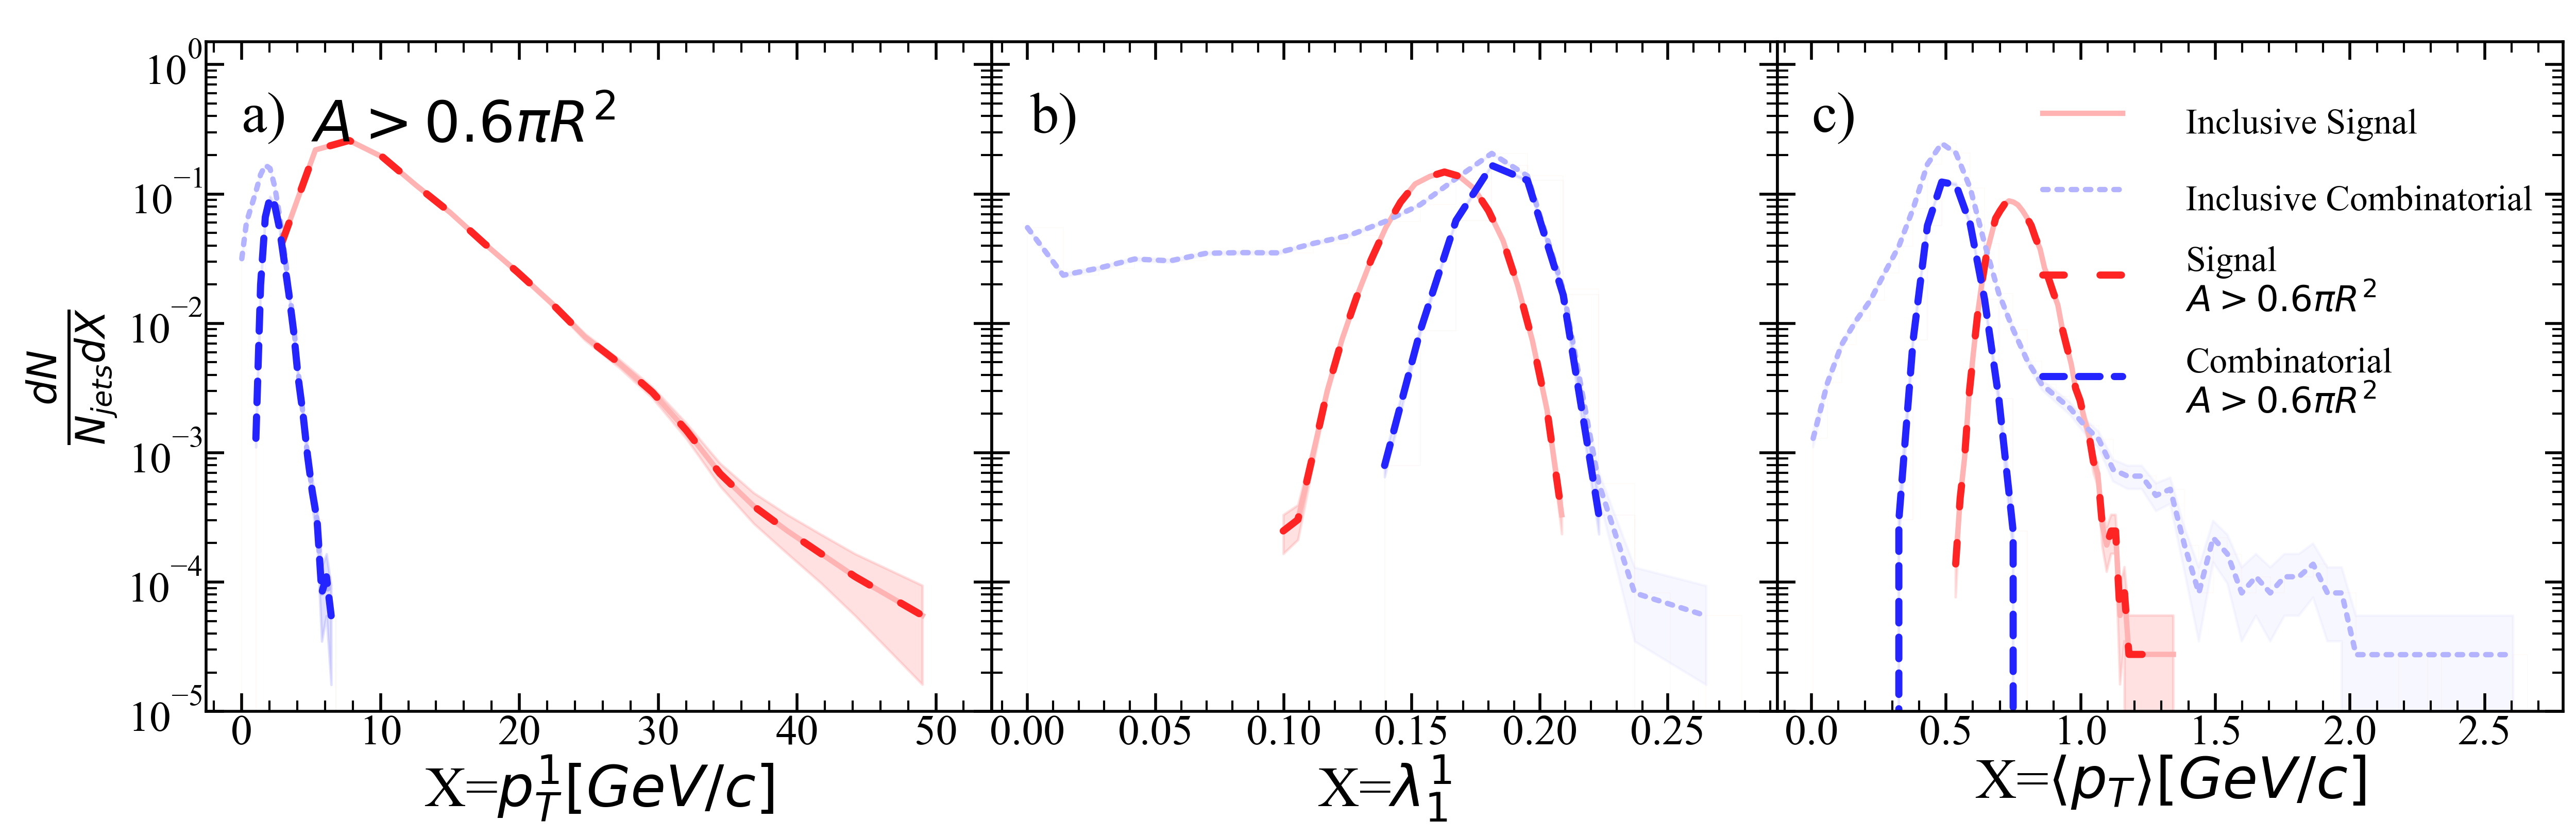}
    \caption{R=0.3 \ptH=30 \GeV}
    \label{fig:area_03_30}
\end{figure*}

\begin{figure*}
    \centering
    \includegraphics[width=\linewidth]{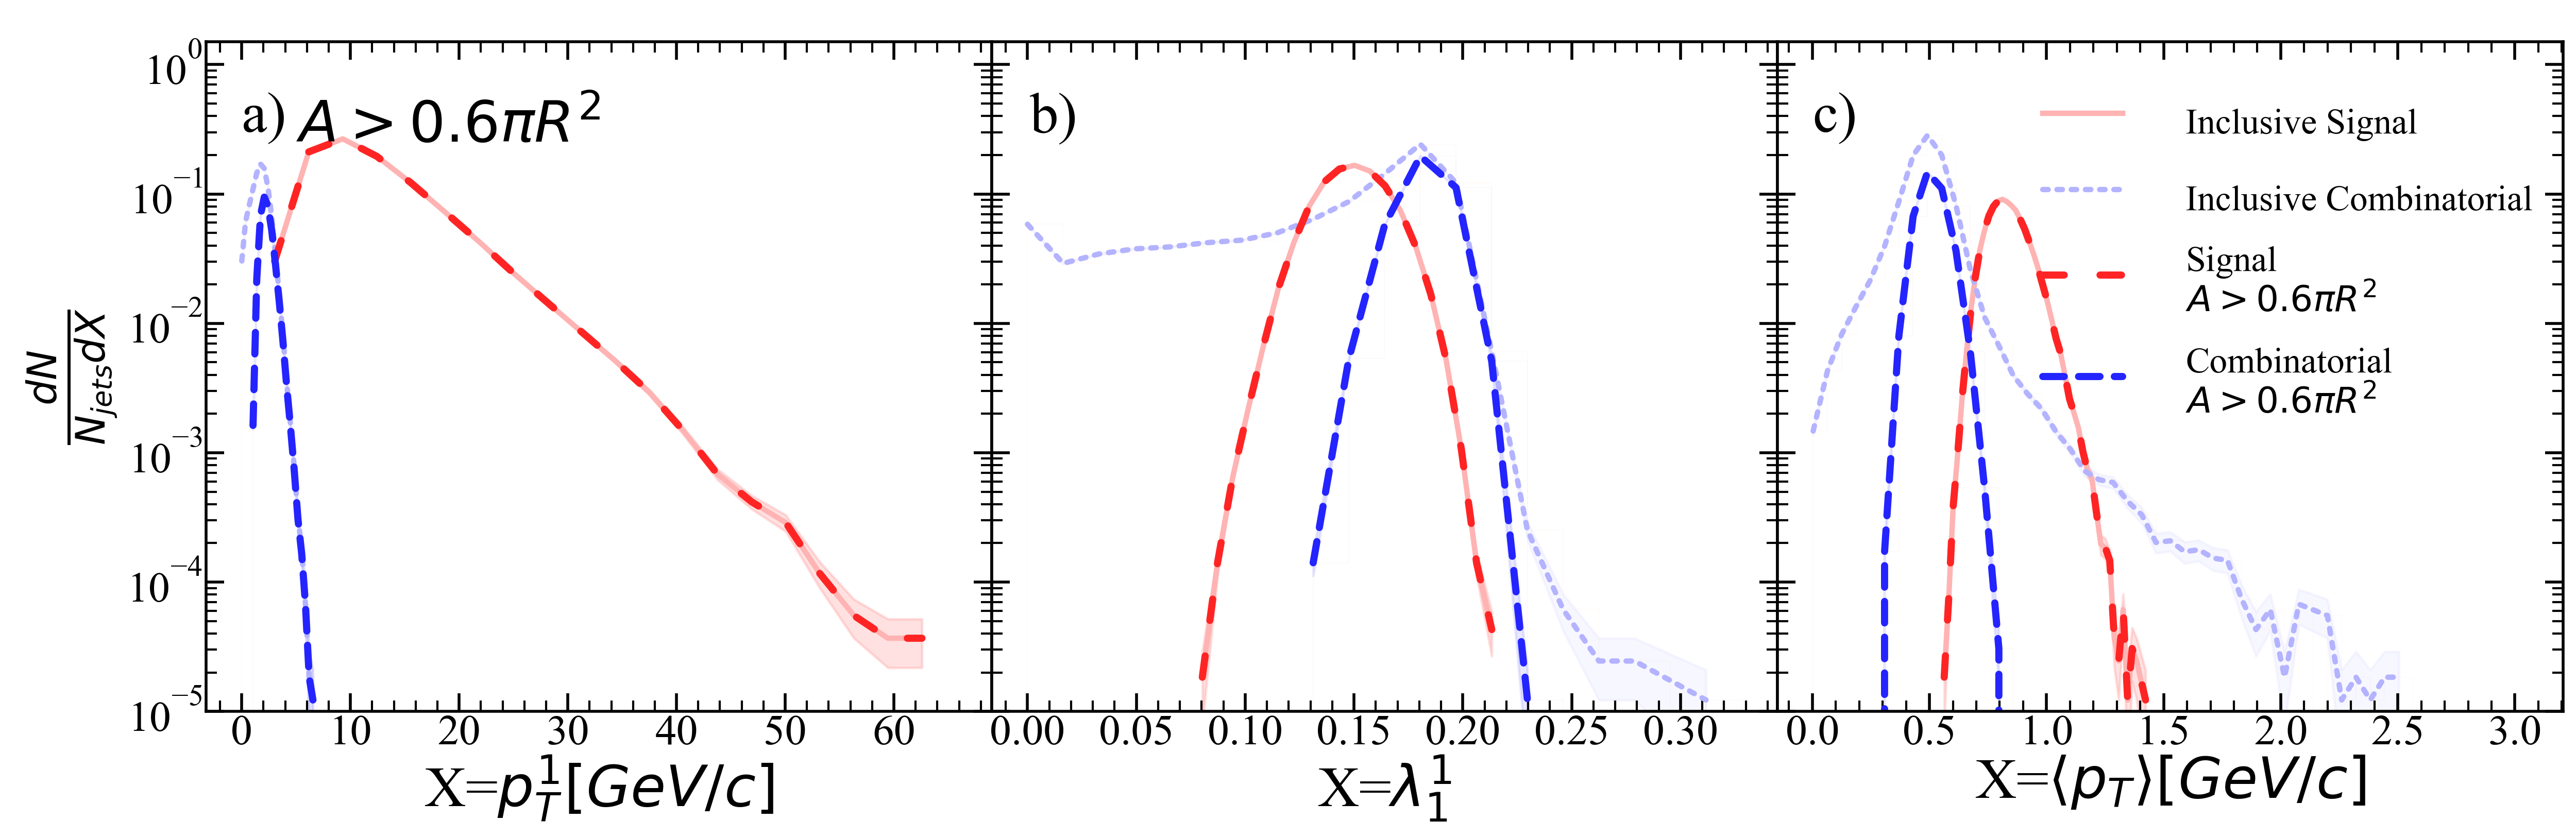}
    \caption{R=0.3 \ptH=40 \GeV}
    \label{fig:area_03_40}
\end{figure*}

\begin{figure*}
    \centering
    \includegraphics[width=\linewidth]{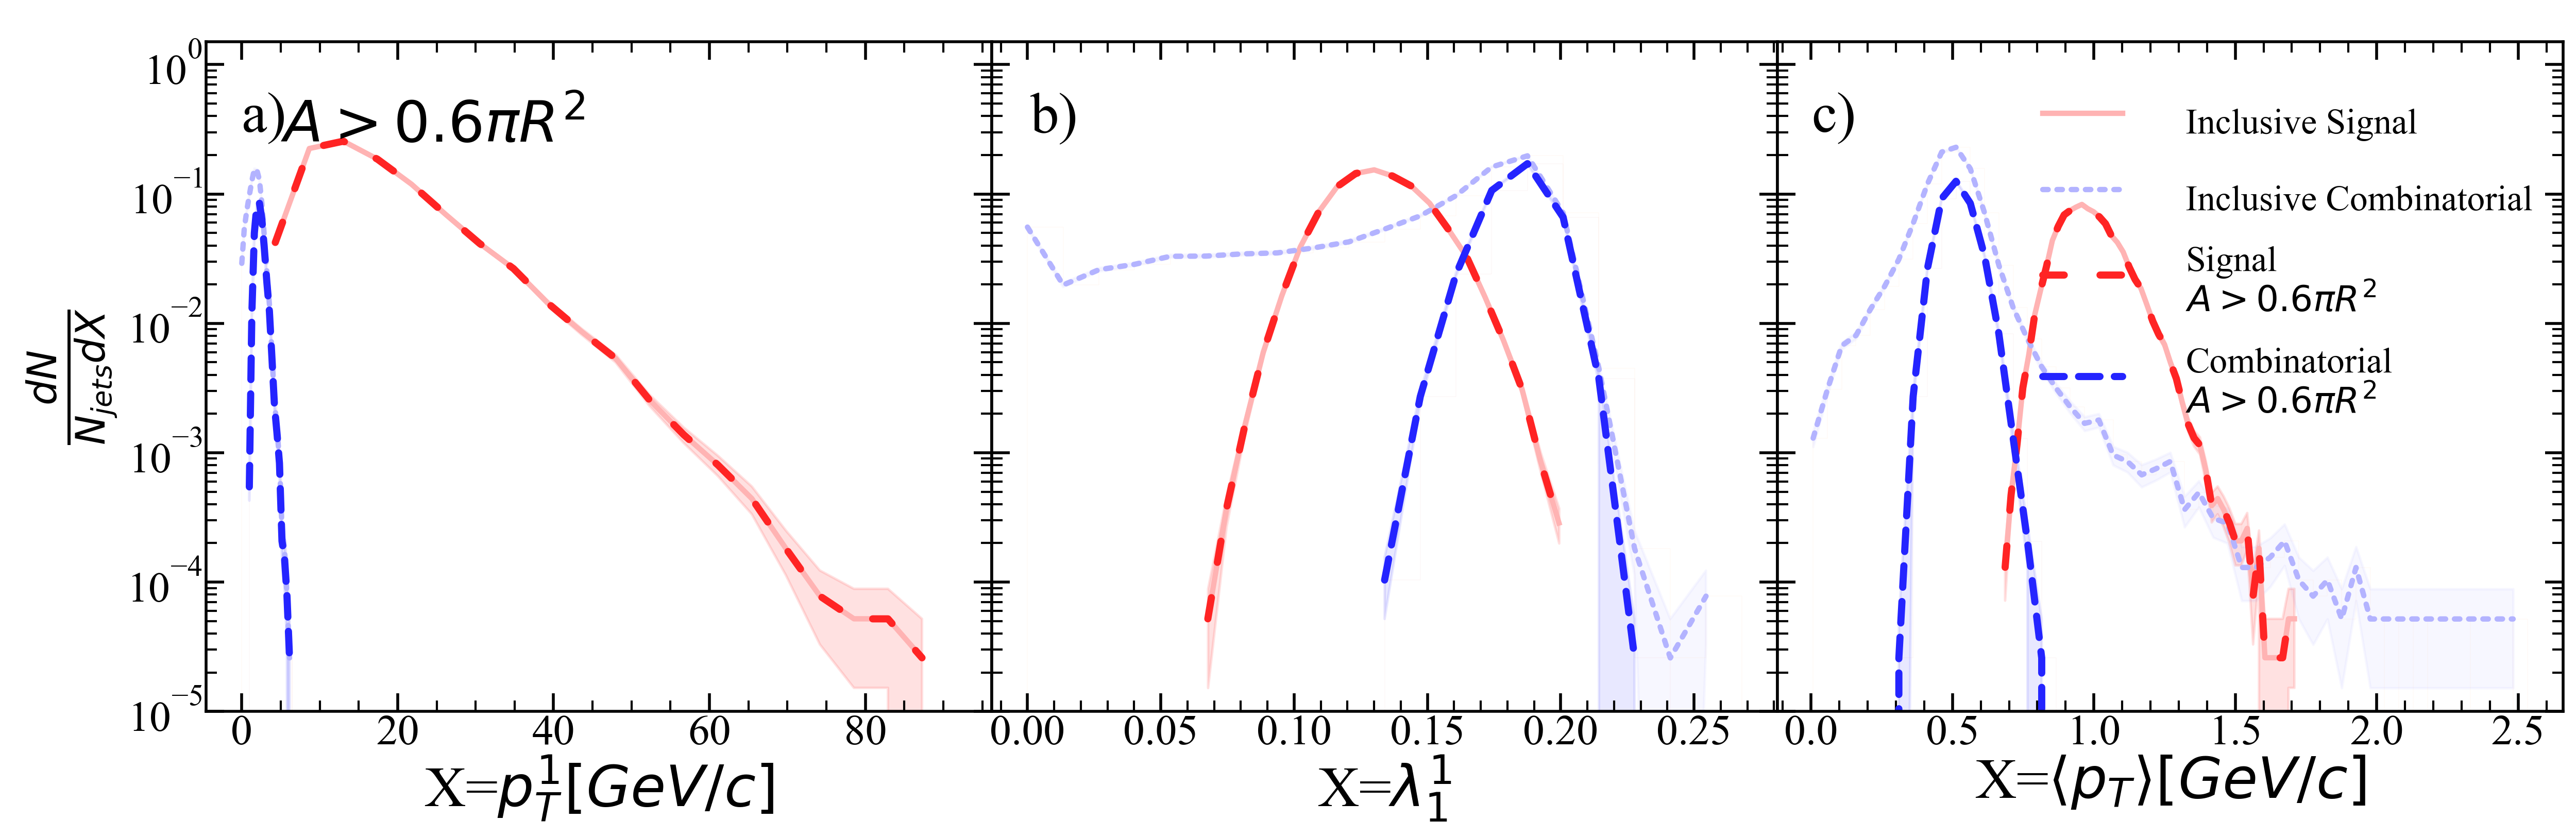}
    \caption{R=0.3 \ptH=60 \GeV}
    \label{fig:area_03_60}
\end{figure*}

\begin{figure*}
    \centering
    \includegraphics[width=\linewidth]{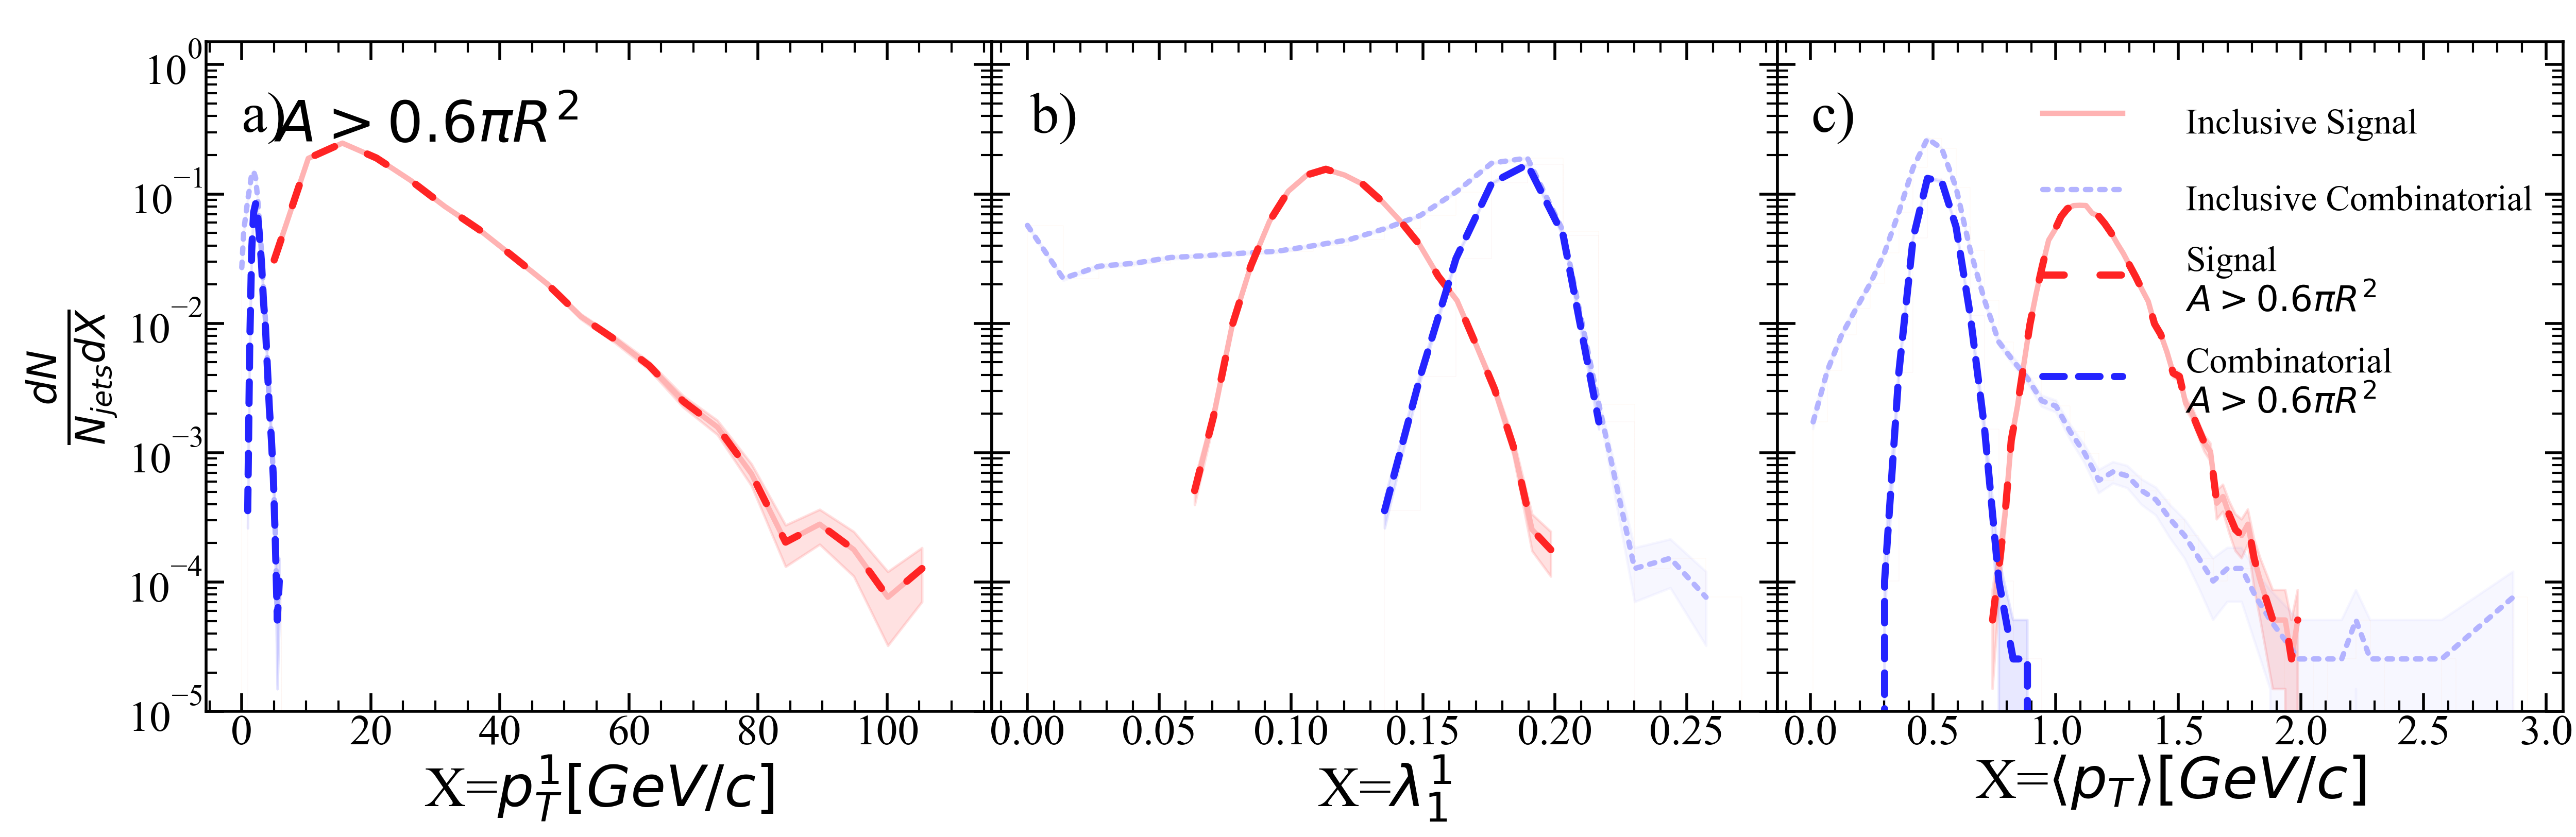}
    \caption{R=0.3 \ptH=80 \GeV}
    \label{fig:area_03_80}
\end{figure*}

\begin{figure*}
    \centering
    \includegraphics[width=\linewidth]{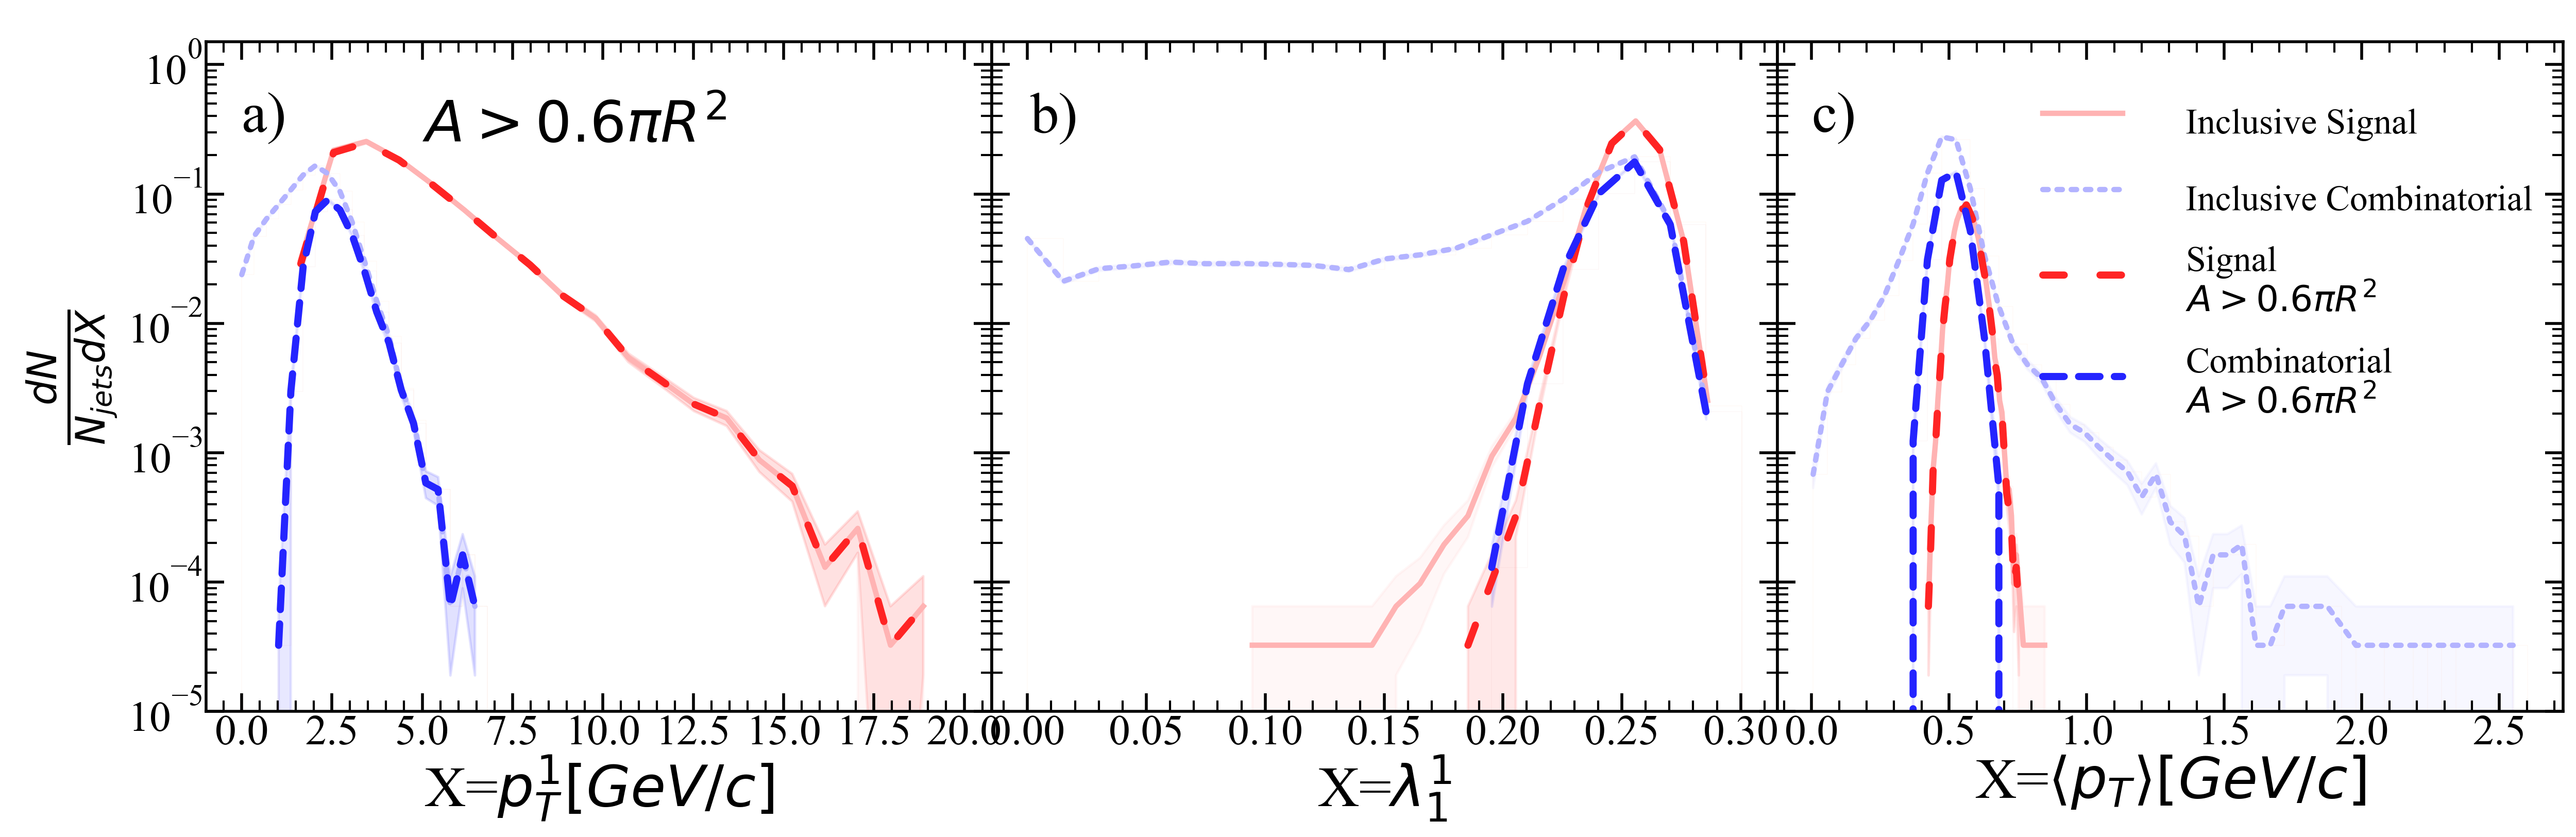}
    \caption{R=0.4 \ptH=10 \GeV}
    \label{fig:area_04_10}
\end{figure*}

\begin{figure*}
    \centering
    \includegraphics[width=\linewidth]{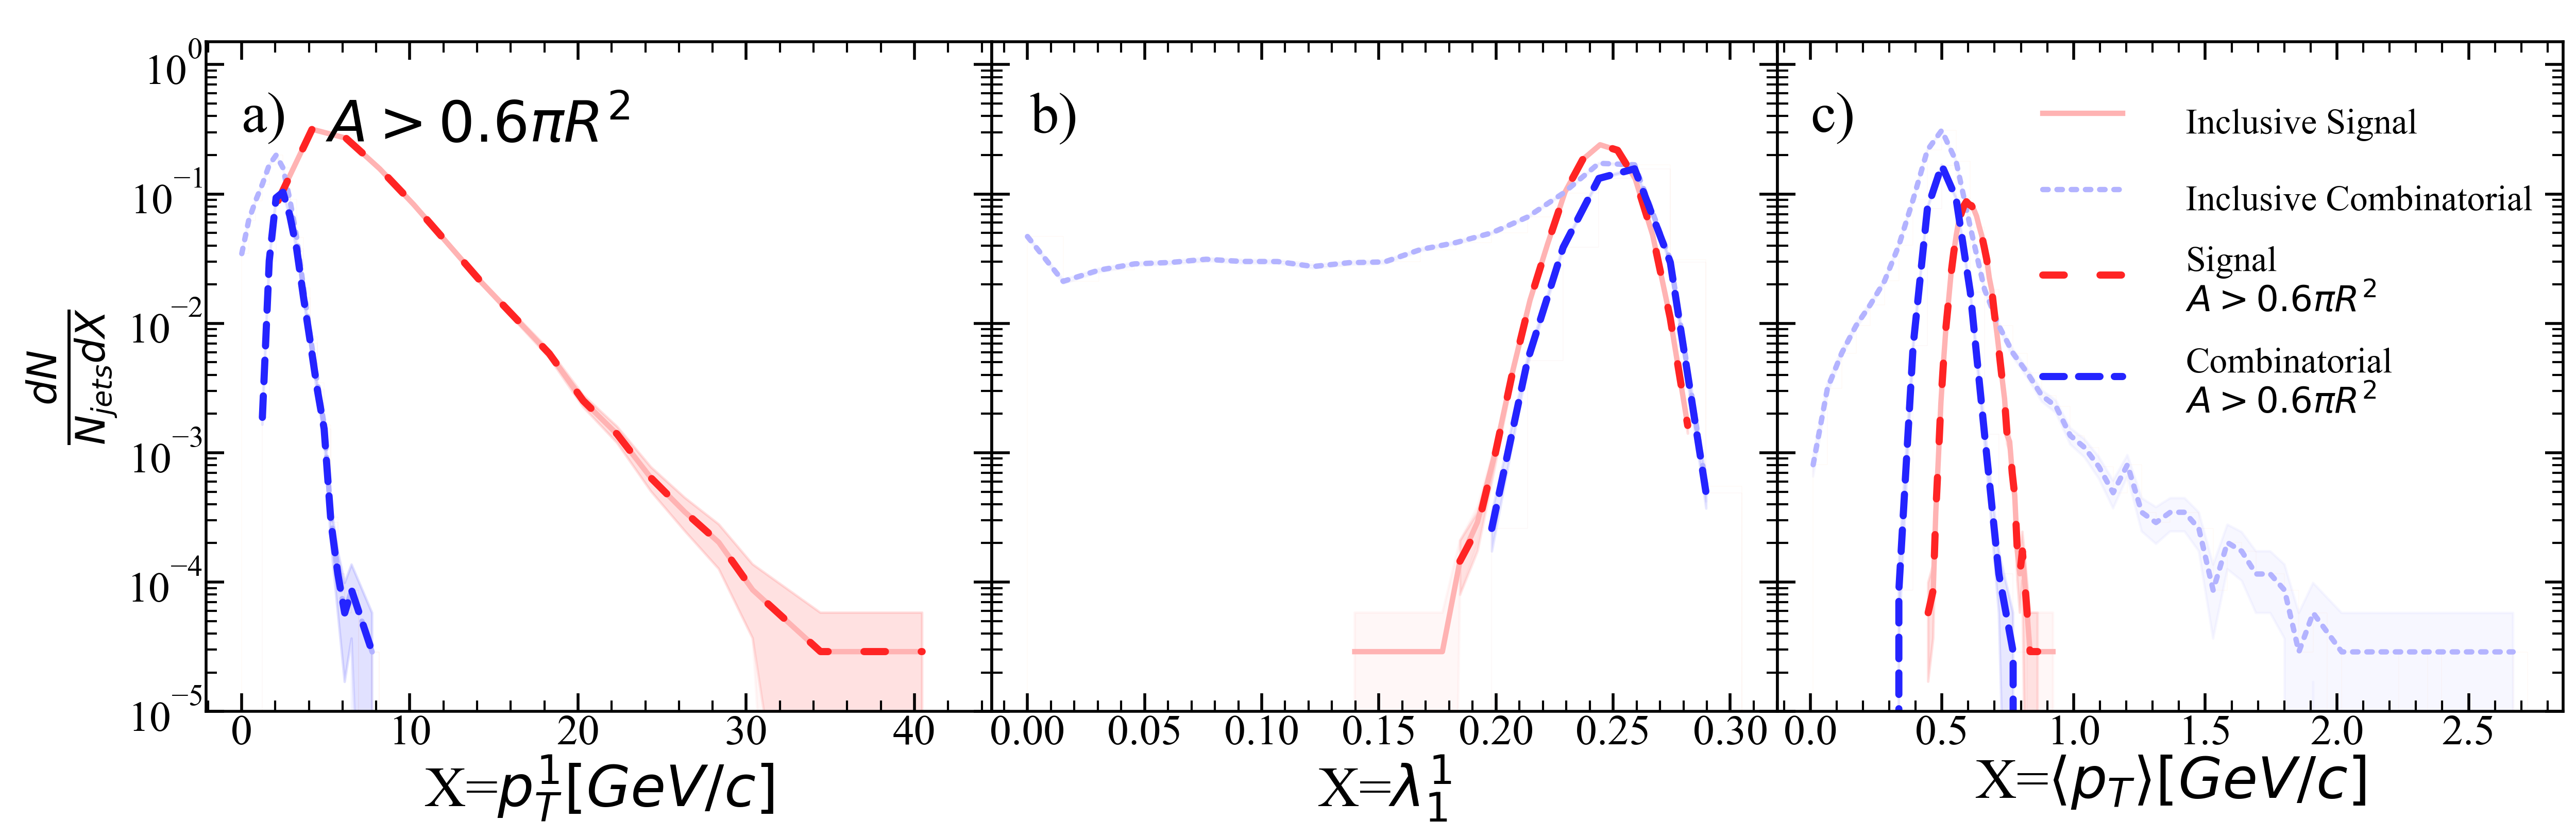}
    \caption{R=0.4 \ptH=20 \GeV}
    \label{fig:area_04_20}
\end{figure*}

\begin{figure*}
    \centering
    \includegraphics[width=\linewidth]{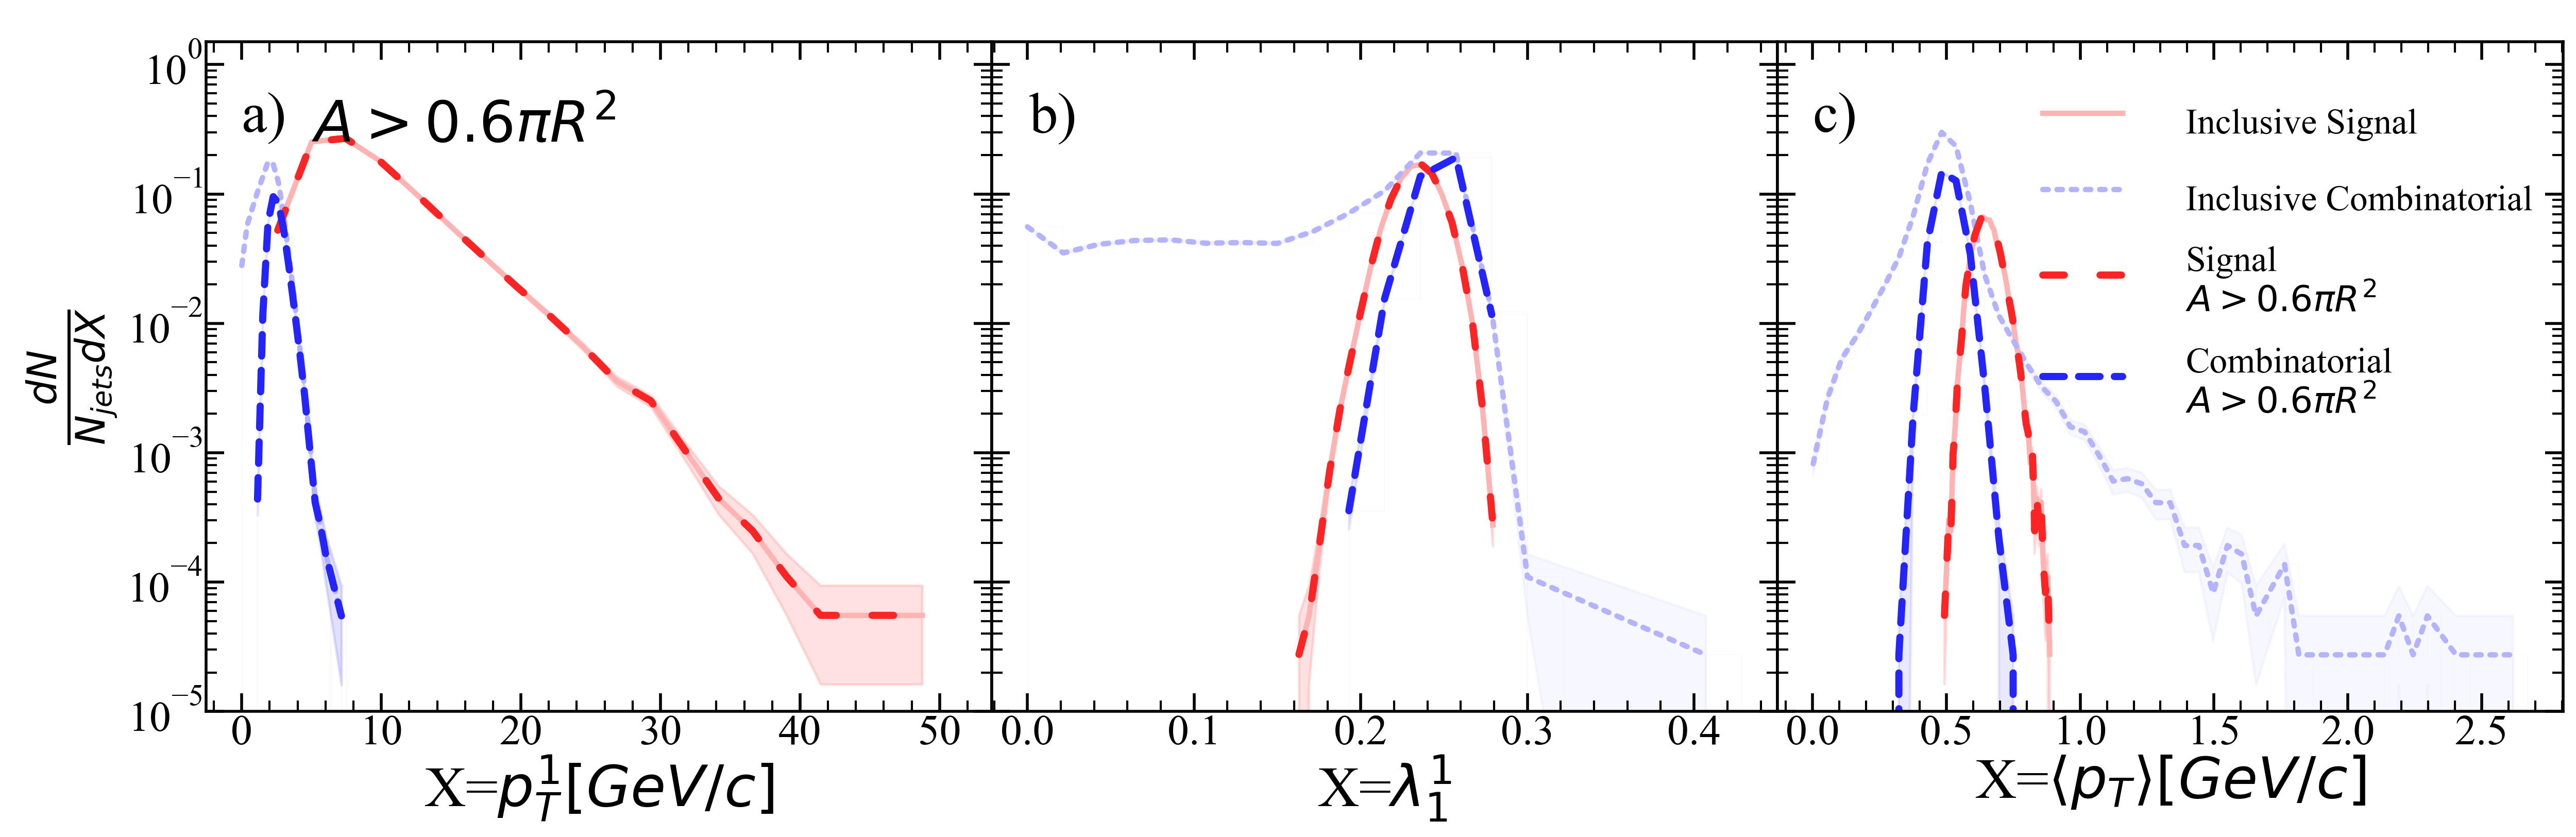}
    \caption{R=0.4 \ptH=30 \GeV}
    \label{fig:area_04_30}
\end{figure*}

\begin{figure*}
    \centering
    \includegraphics[width=\linewidth]{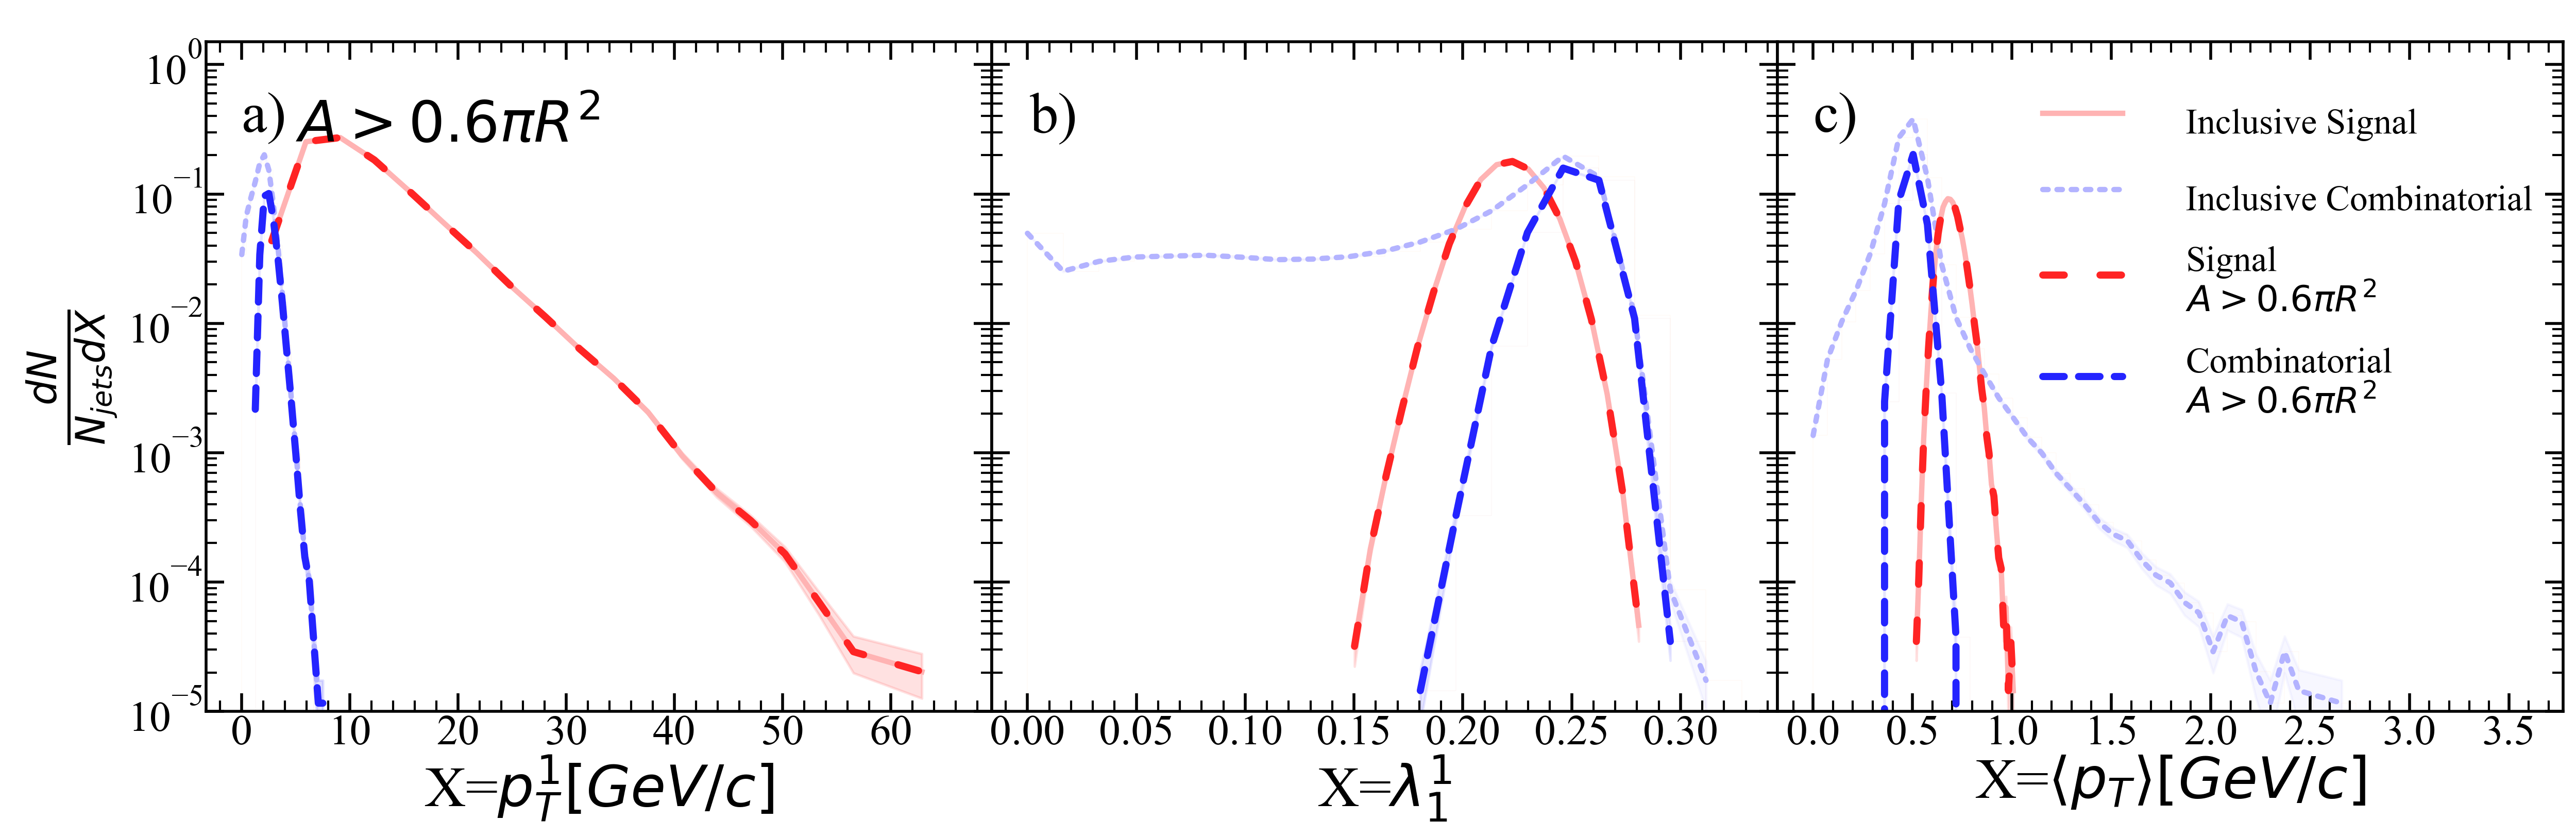}
    \caption{R=0.4 \ptH=40 \GeV}
    \label{fig:area_04_40}
\end{figure*}

\begin{figure*}
    \centering
    \includegraphics[width=\linewidth]{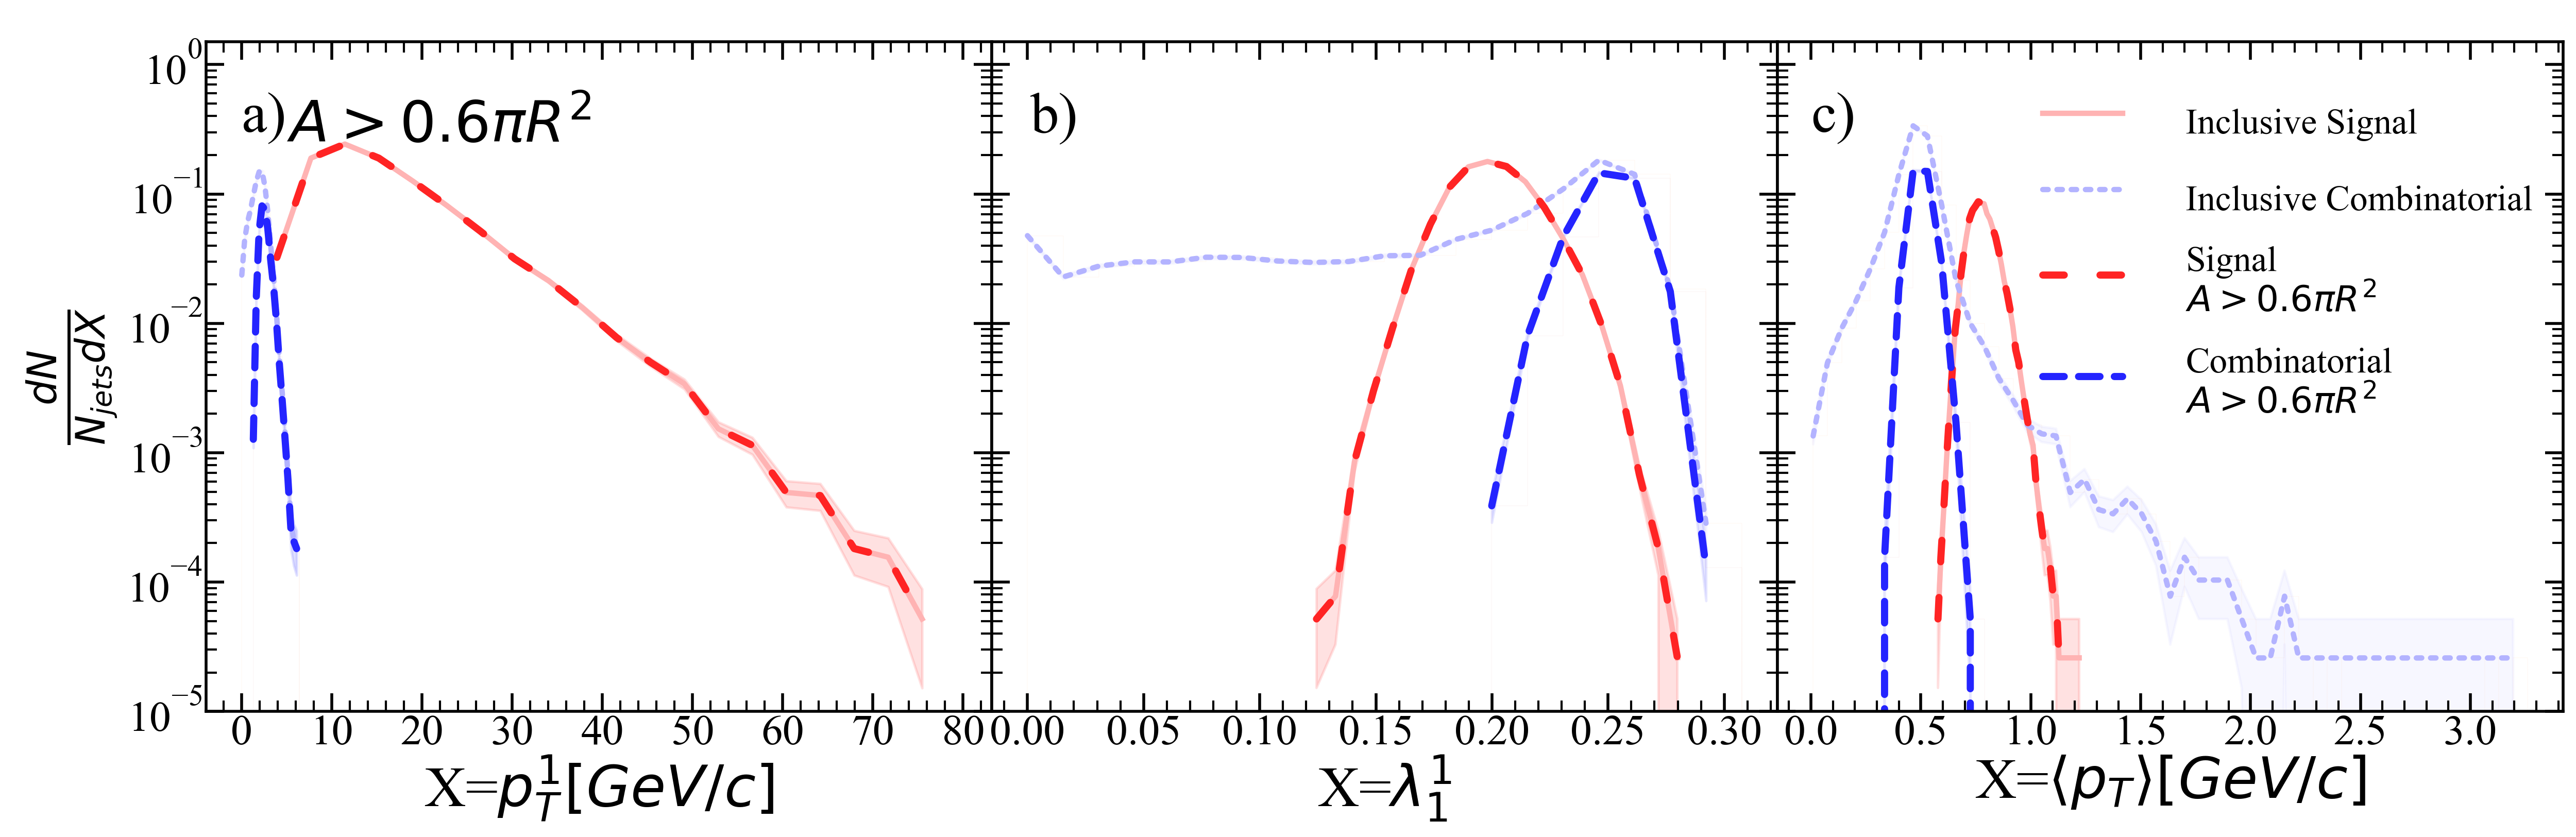}
    \caption{R=0.4 \ptH=60 \GeV}
    \label{fig:area_04_60}
\end{figure*}

\begin{figure*}
    \centering
    \includegraphics[width=\linewidth]{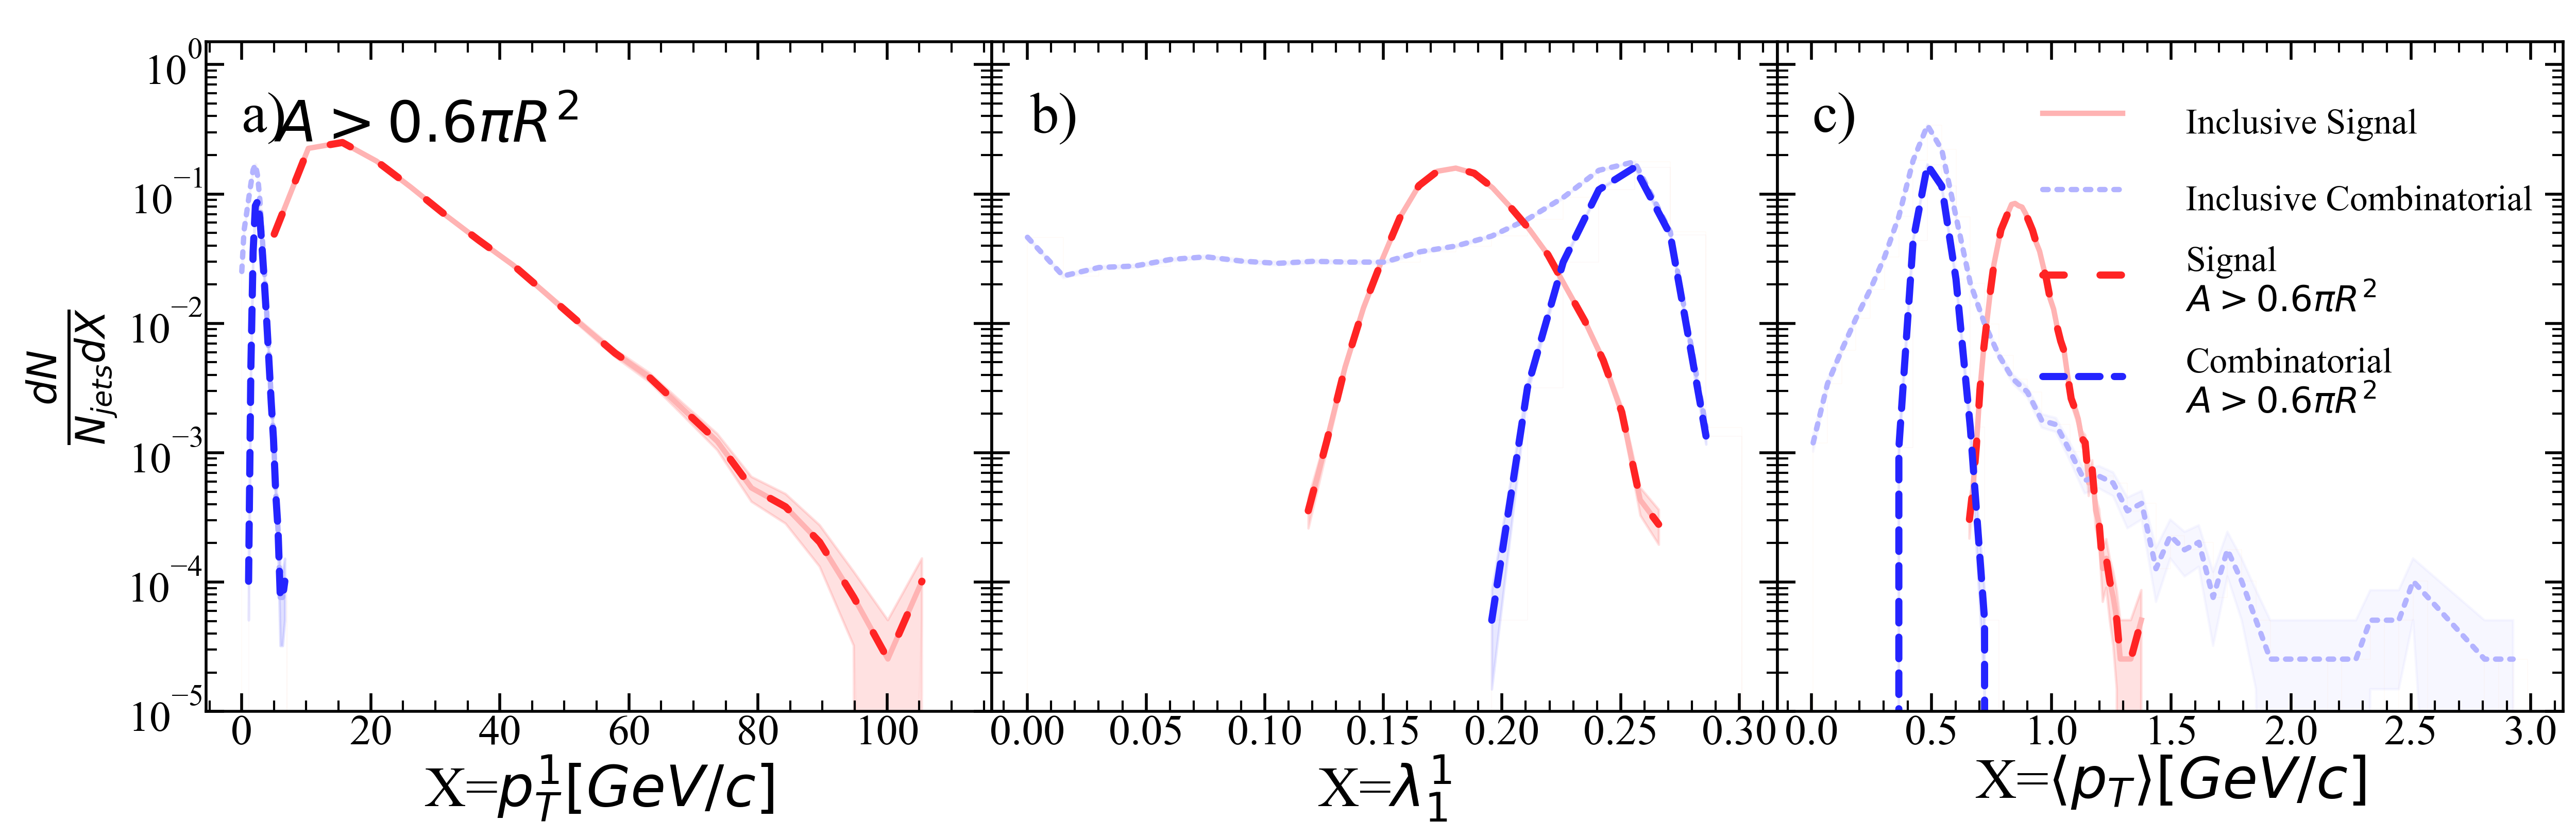}
    \caption{R=0.4 \ptH=80 \GeV}
    \label{fig:area_04_80}
\end{figure*}

\begin{figure*}
    \centering
    \includegraphics[width=\linewidth]{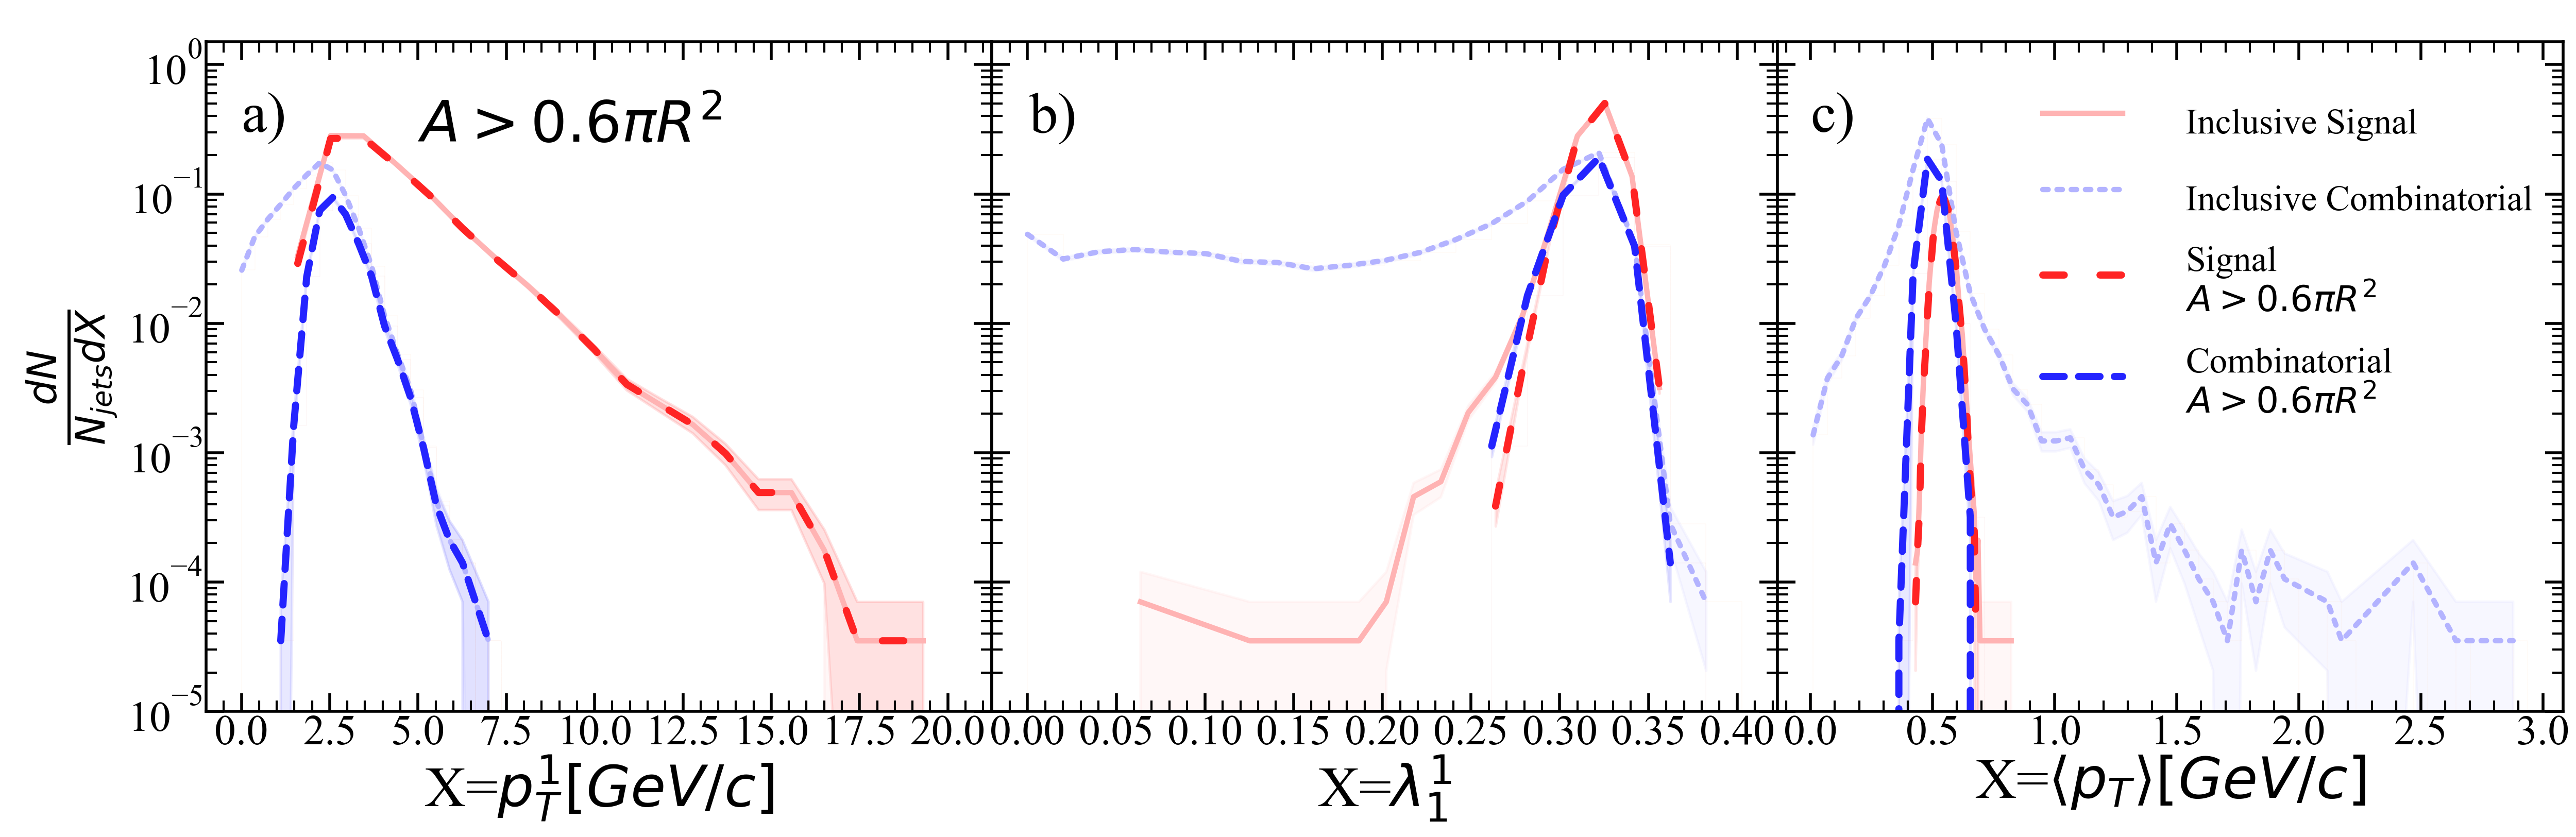}
    \caption{R=0.5 \ptH=10 \GeV}
    \label{fig:area_05_10}
\end{figure*}

\begin{figure*}
    \centering
    \includegraphics[width=\linewidth]{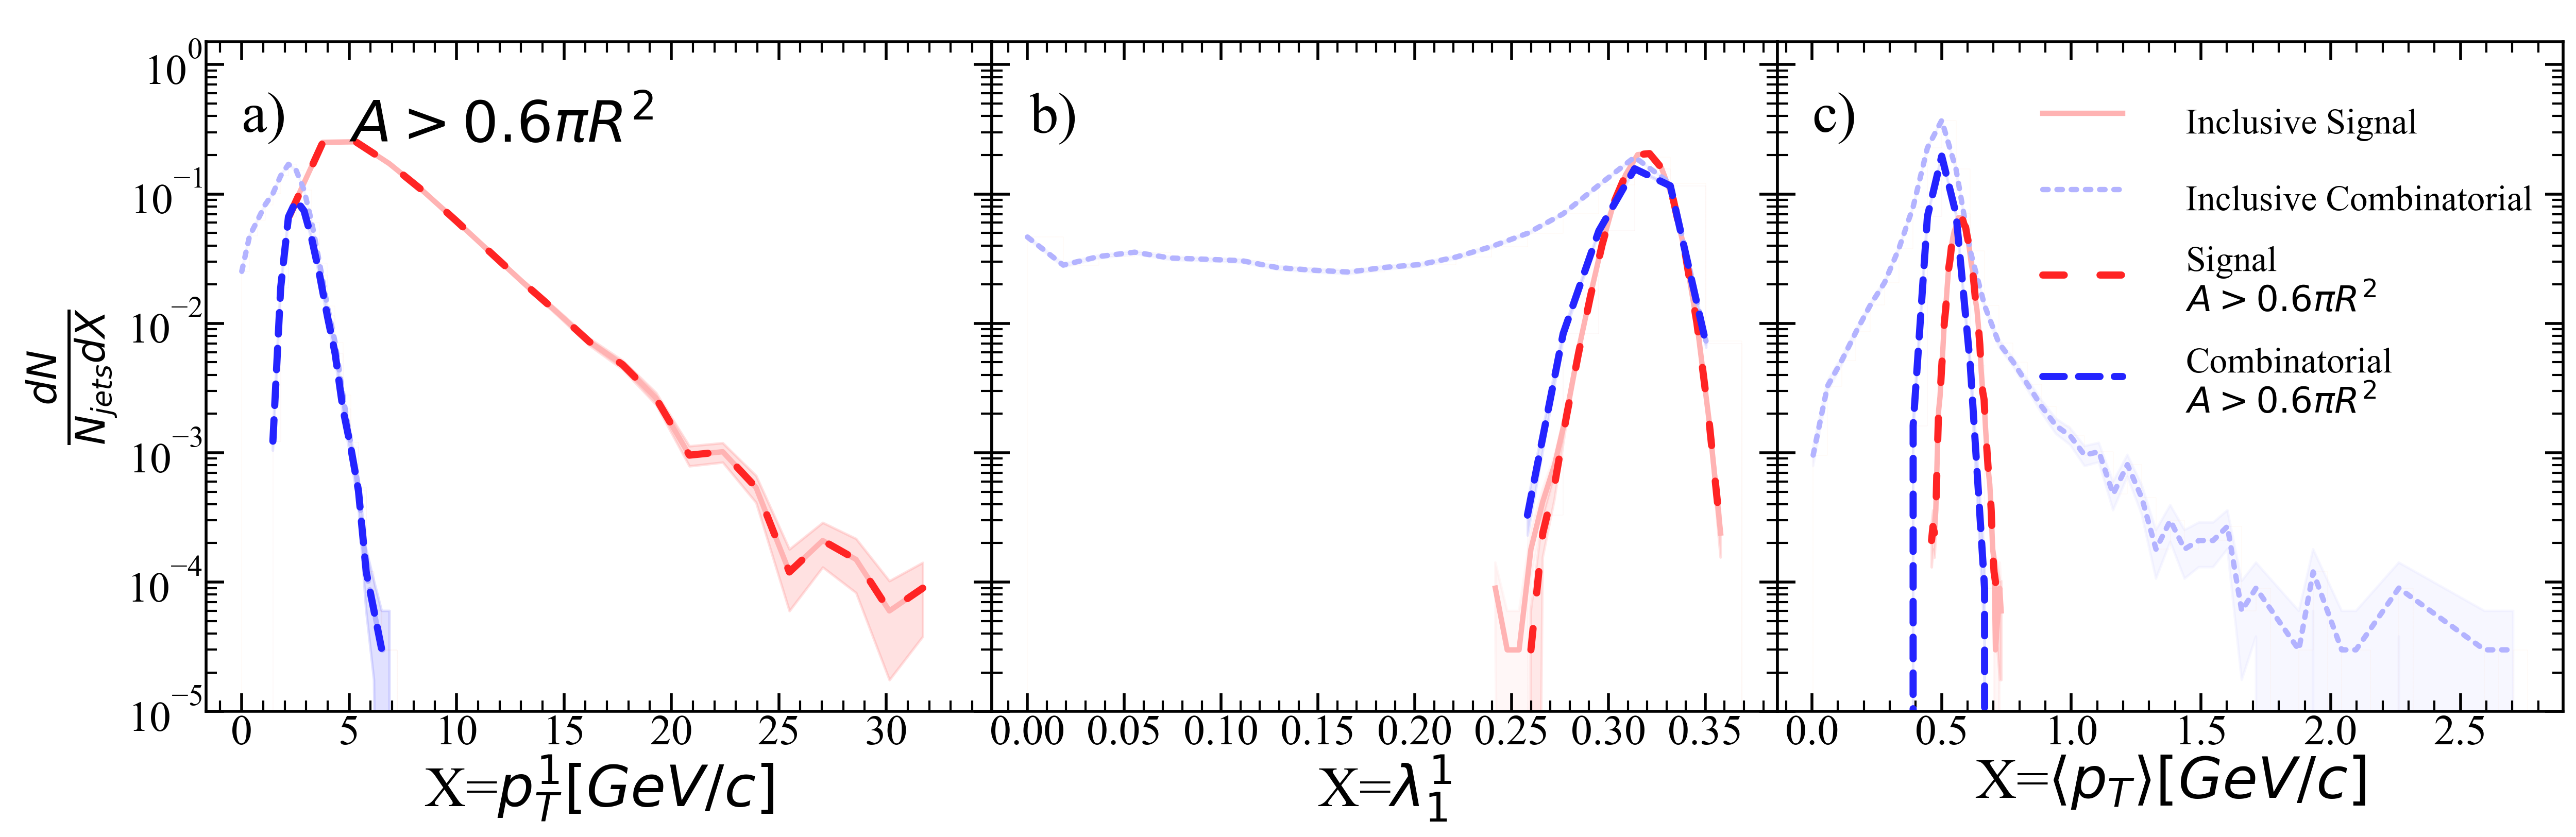}
    \caption{R=0.5 \ptH=20 \GeV}
    \label{fig:area_05_20}
\end{figure*}

\begin{figure*}
    \centering
    \includegraphics[width=\linewidth]{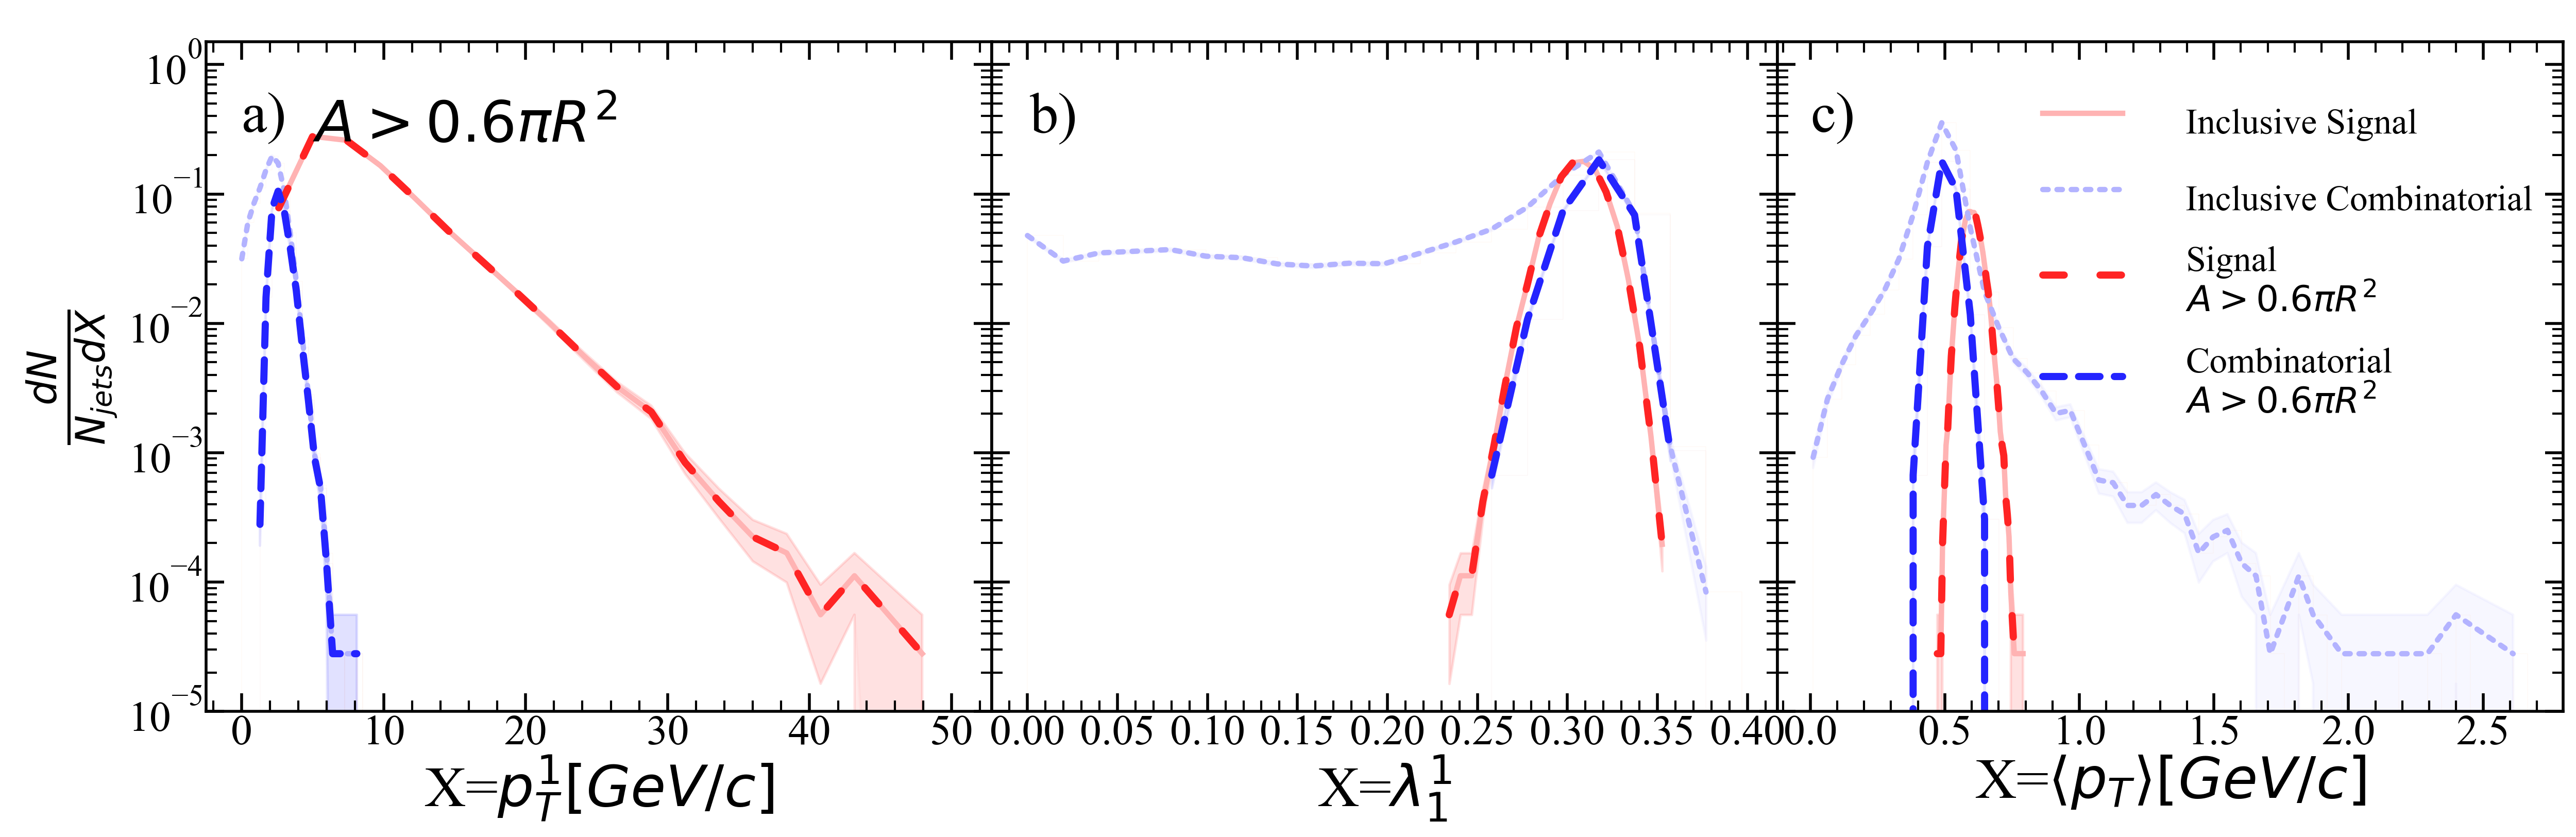}
    \caption{R=0.5 \ptH=30 \GeV}
    \label{fig:area_05_30}
\end{figure*}

\begin{figure*}
    \centering
    \includegraphics[width=\linewidth]{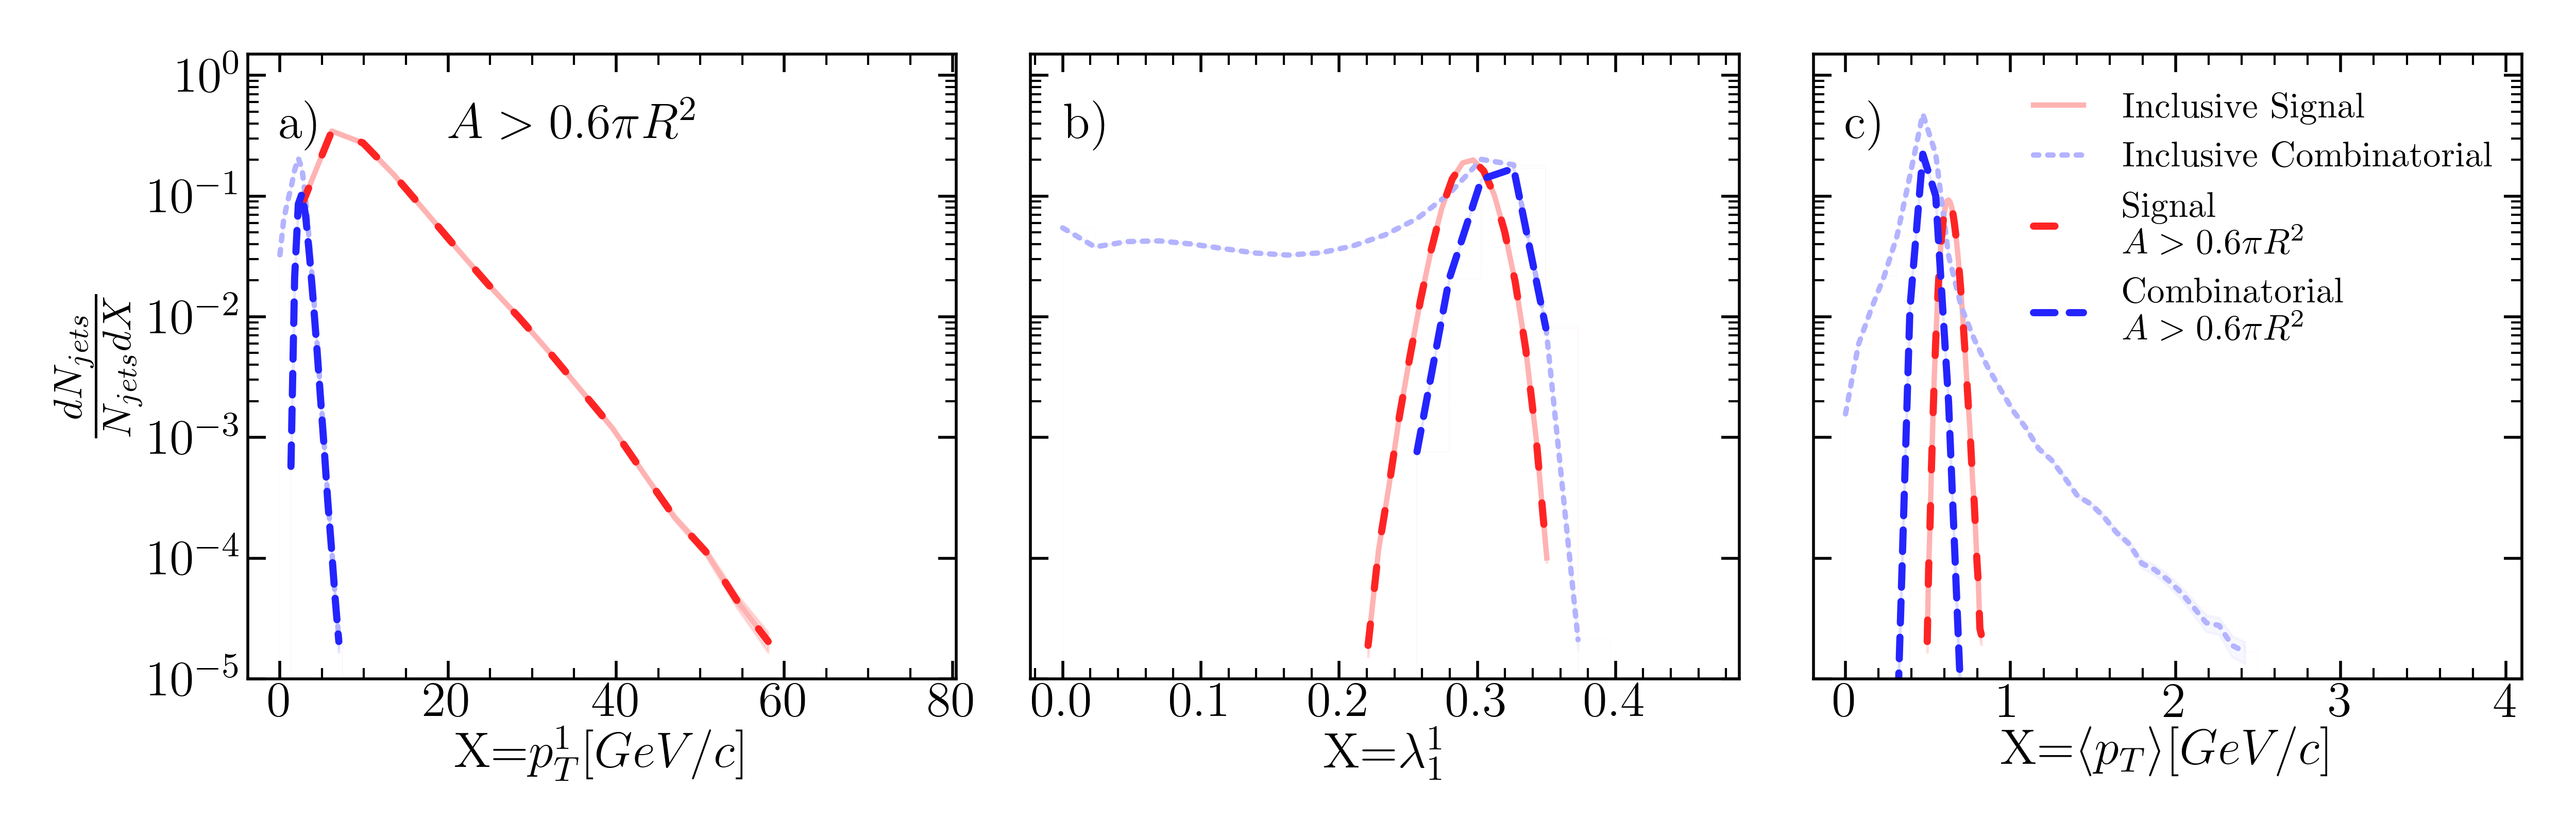}
    \caption{R=0.5 \ptH=40 \GeV}
    \label{fig:area_05_40}
\end{figure*}

\begin{figure*}
    \centering
    \includegraphics[width=\linewidth]{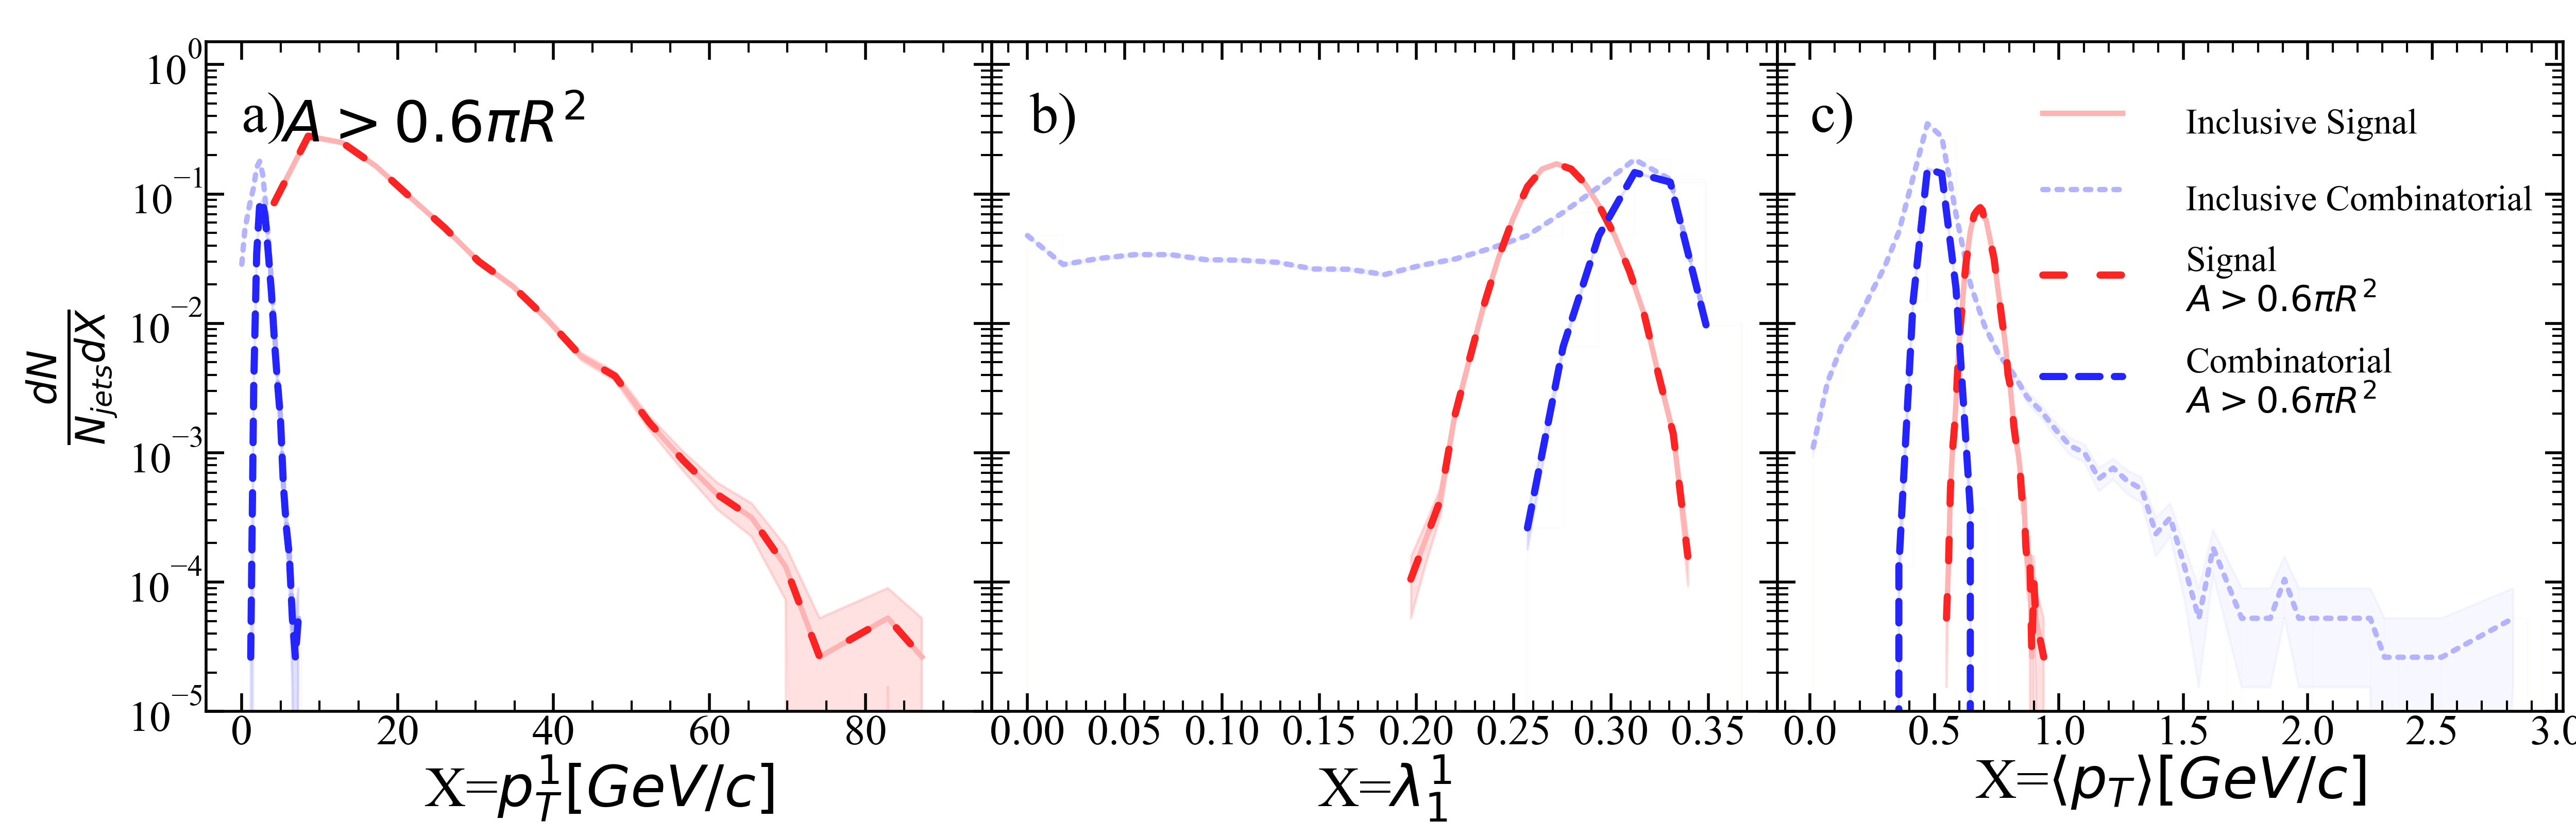}
    \caption{R=0.5 \ptH=60 \GeV}
    \label{fig:area_05_60}
\end{figure*}

\begin{figure*}
    \centering
    \includegraphics[width=\linewidth]{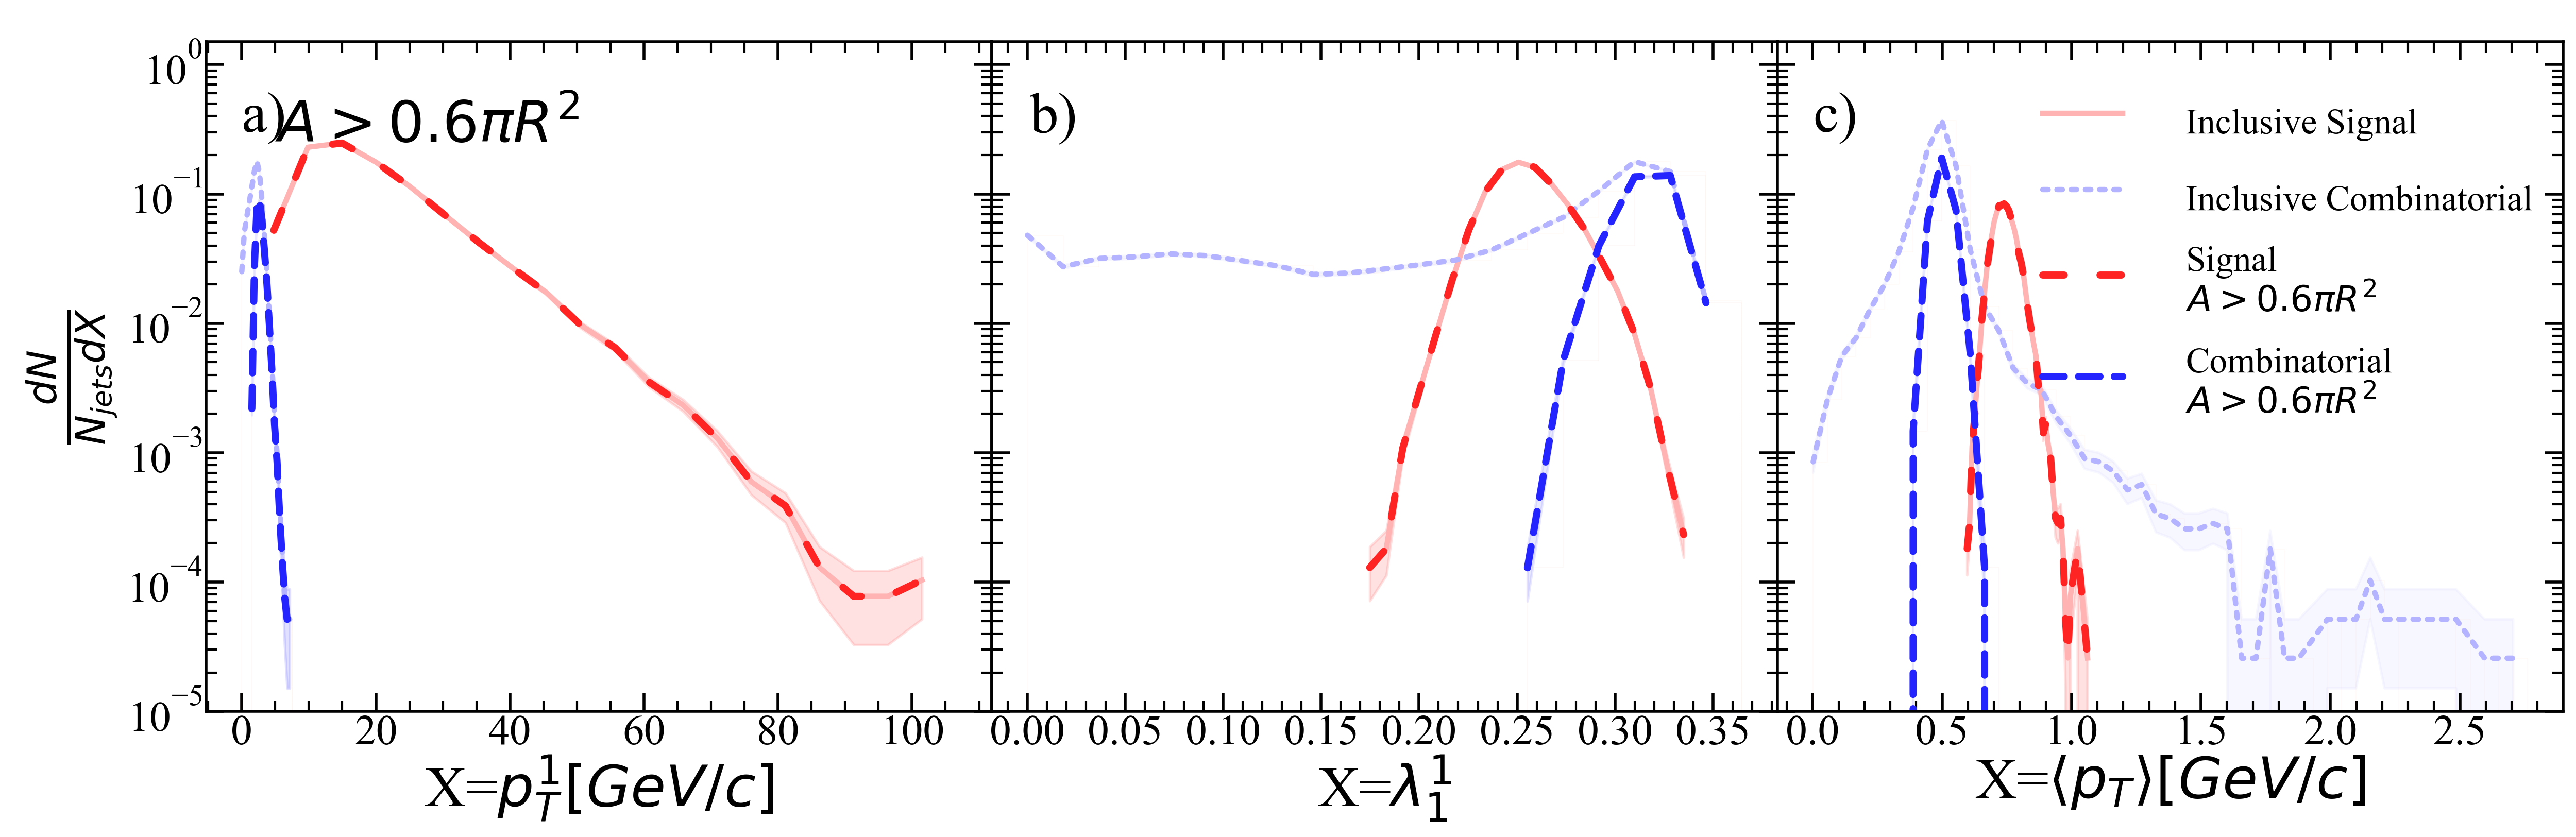}
    \caption{R=0.5 \ptH=80 \GeV}
    \label{fig:area_05_80}
\end{figure*}

\begin{figure*}
    \centering
    \includegraphics[width=\linewidth]{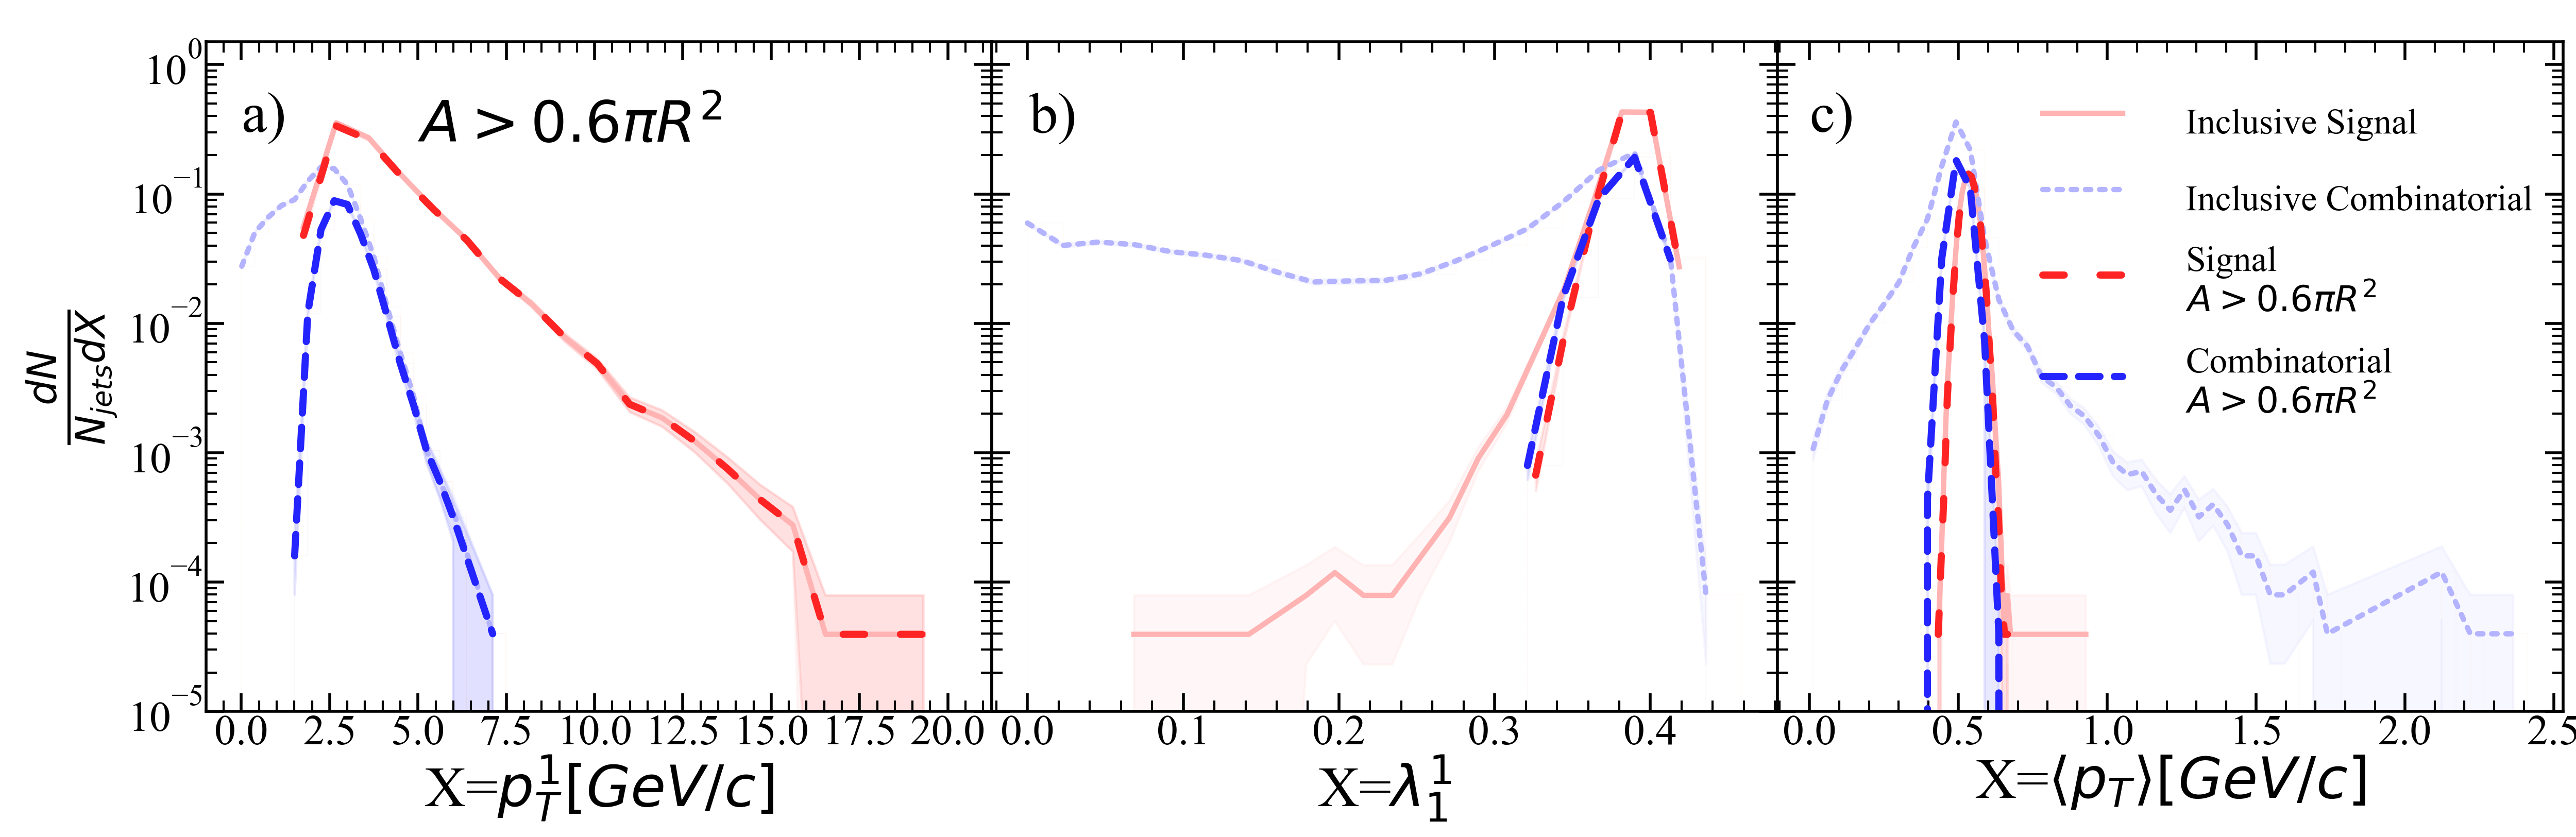}
    \caption{R=0.6 \ptH=10 \GeV}
    \label{fig:area_06_10}
\end{figure*}

\begin{figure*}
    \centering
    \includegraphics[width=\linewidth]{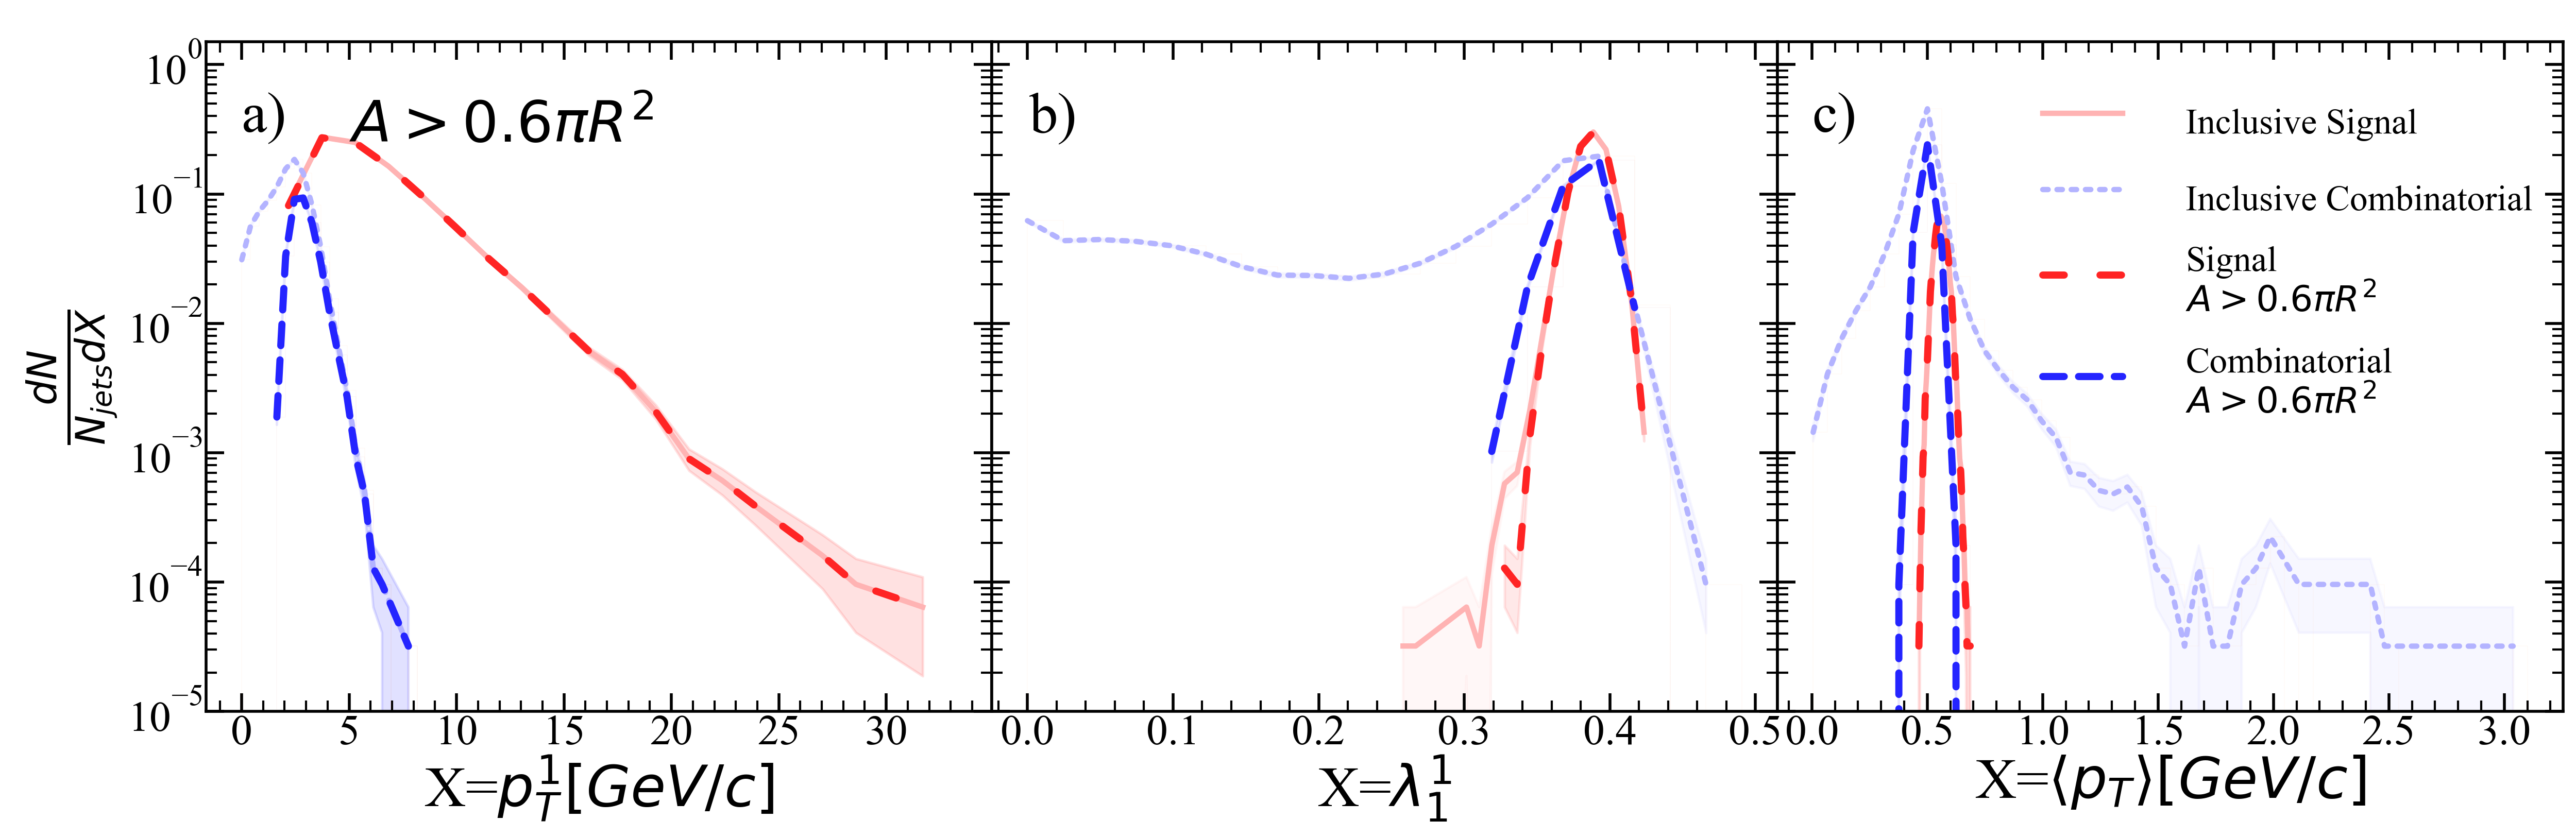}
    \caption{R=0.6 \ptH=20 \GeV}
    \label{fig:area_06_20}
\end{figure*}

\begin{figure*}
    \centering
    \includegraphics[width=\linewidth]{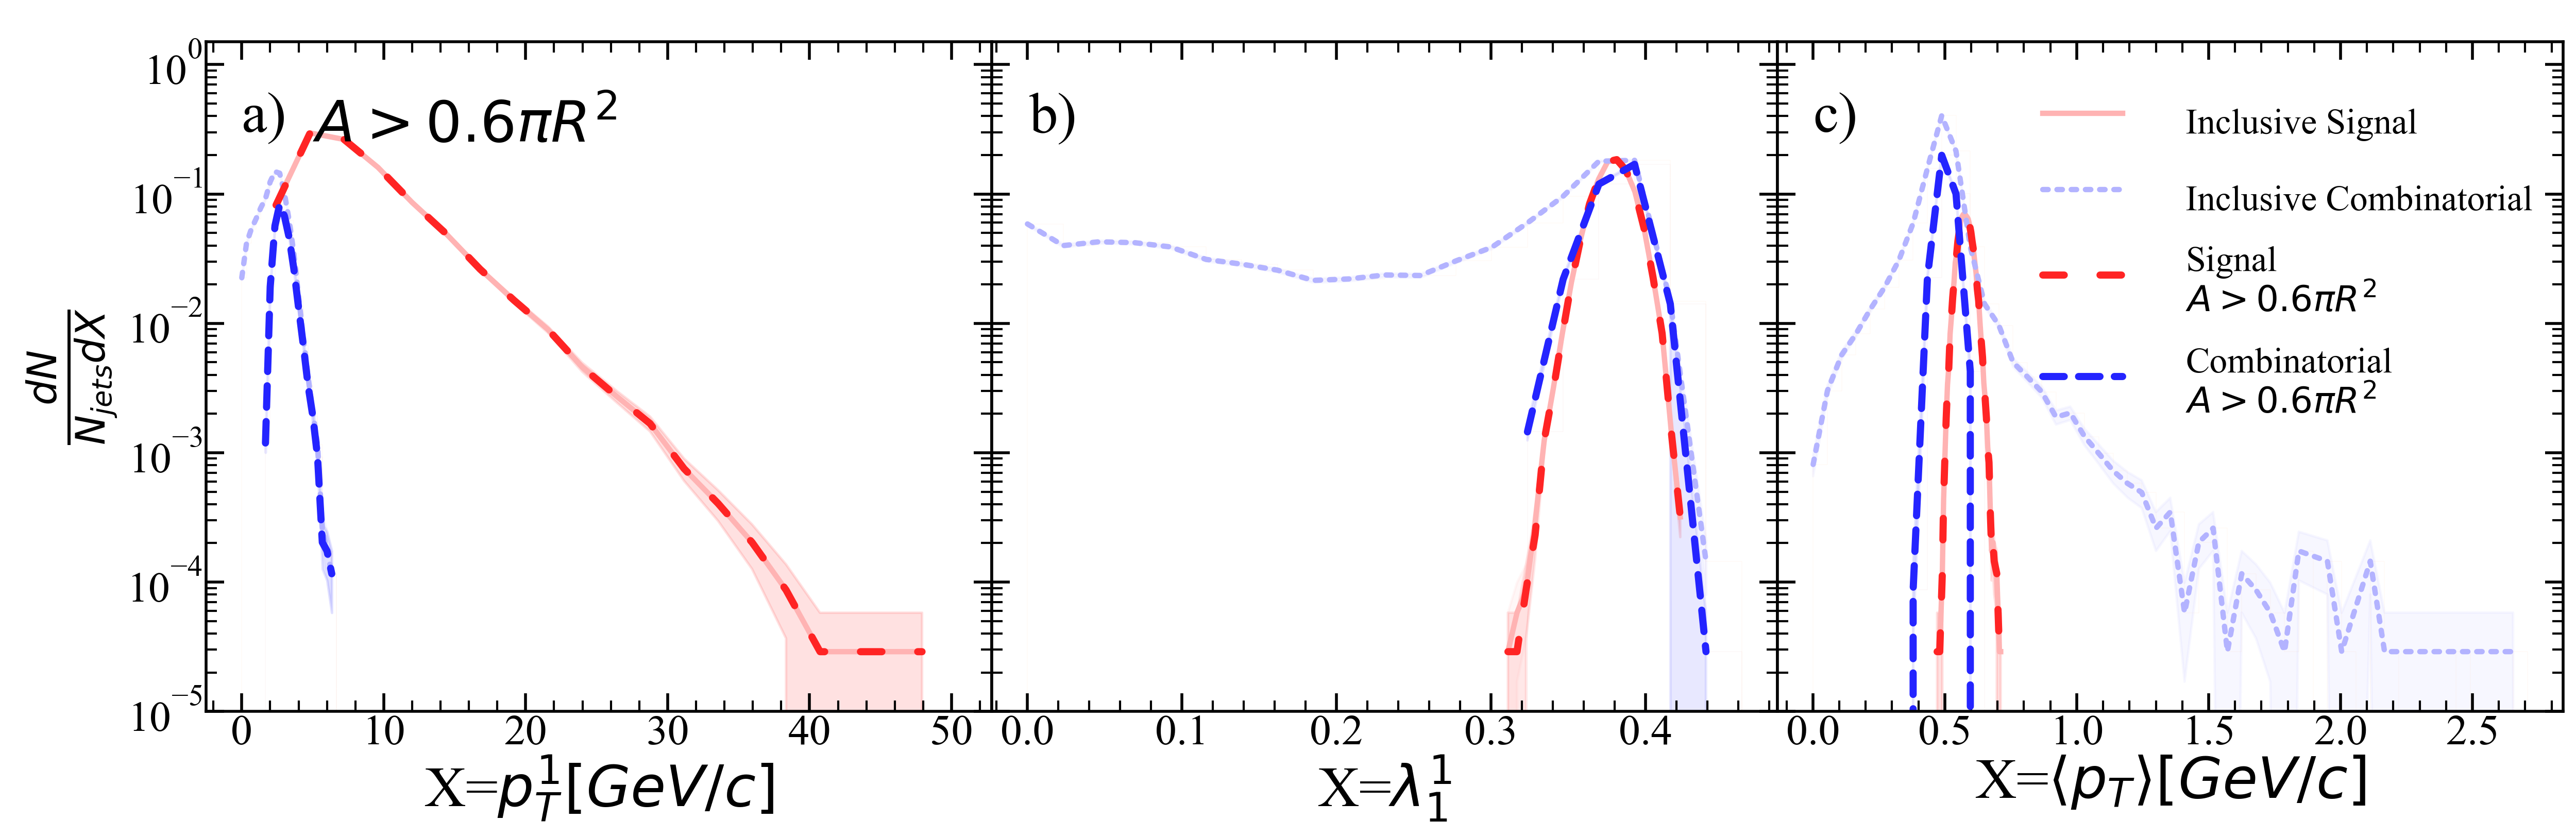}
    \caption{R=0.6 \ptH=30 \GeV}
    \label{fig:area_06_30}
\end{figure*}

\begin{figure*}
    \centering
    \includegraphics[width=\linewidth]{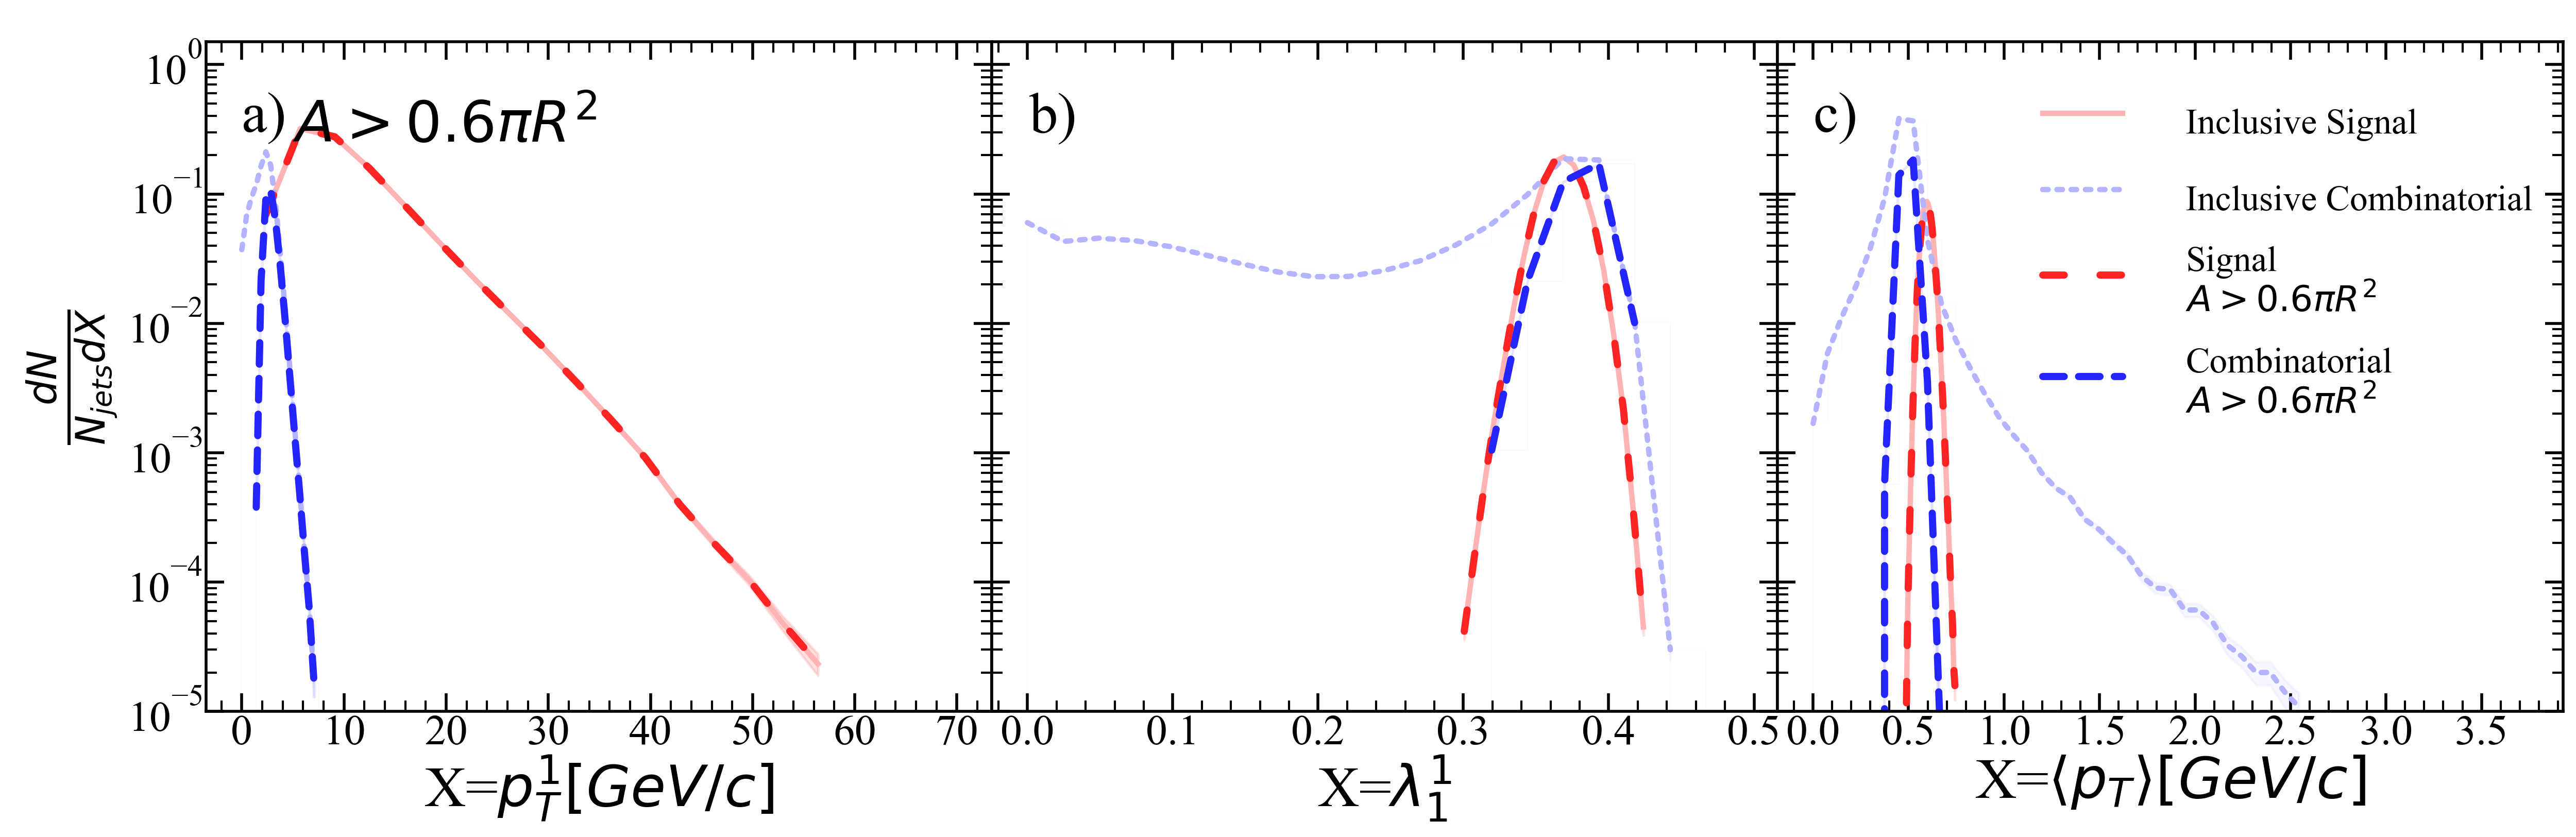}
    \caption{R=0.6 \ptH=40 \GeV}
    \label{fig:area_06_40}
\end{figure*}

\begin{figure*}
    \centering
    \includegraphics[width=\linewidth]{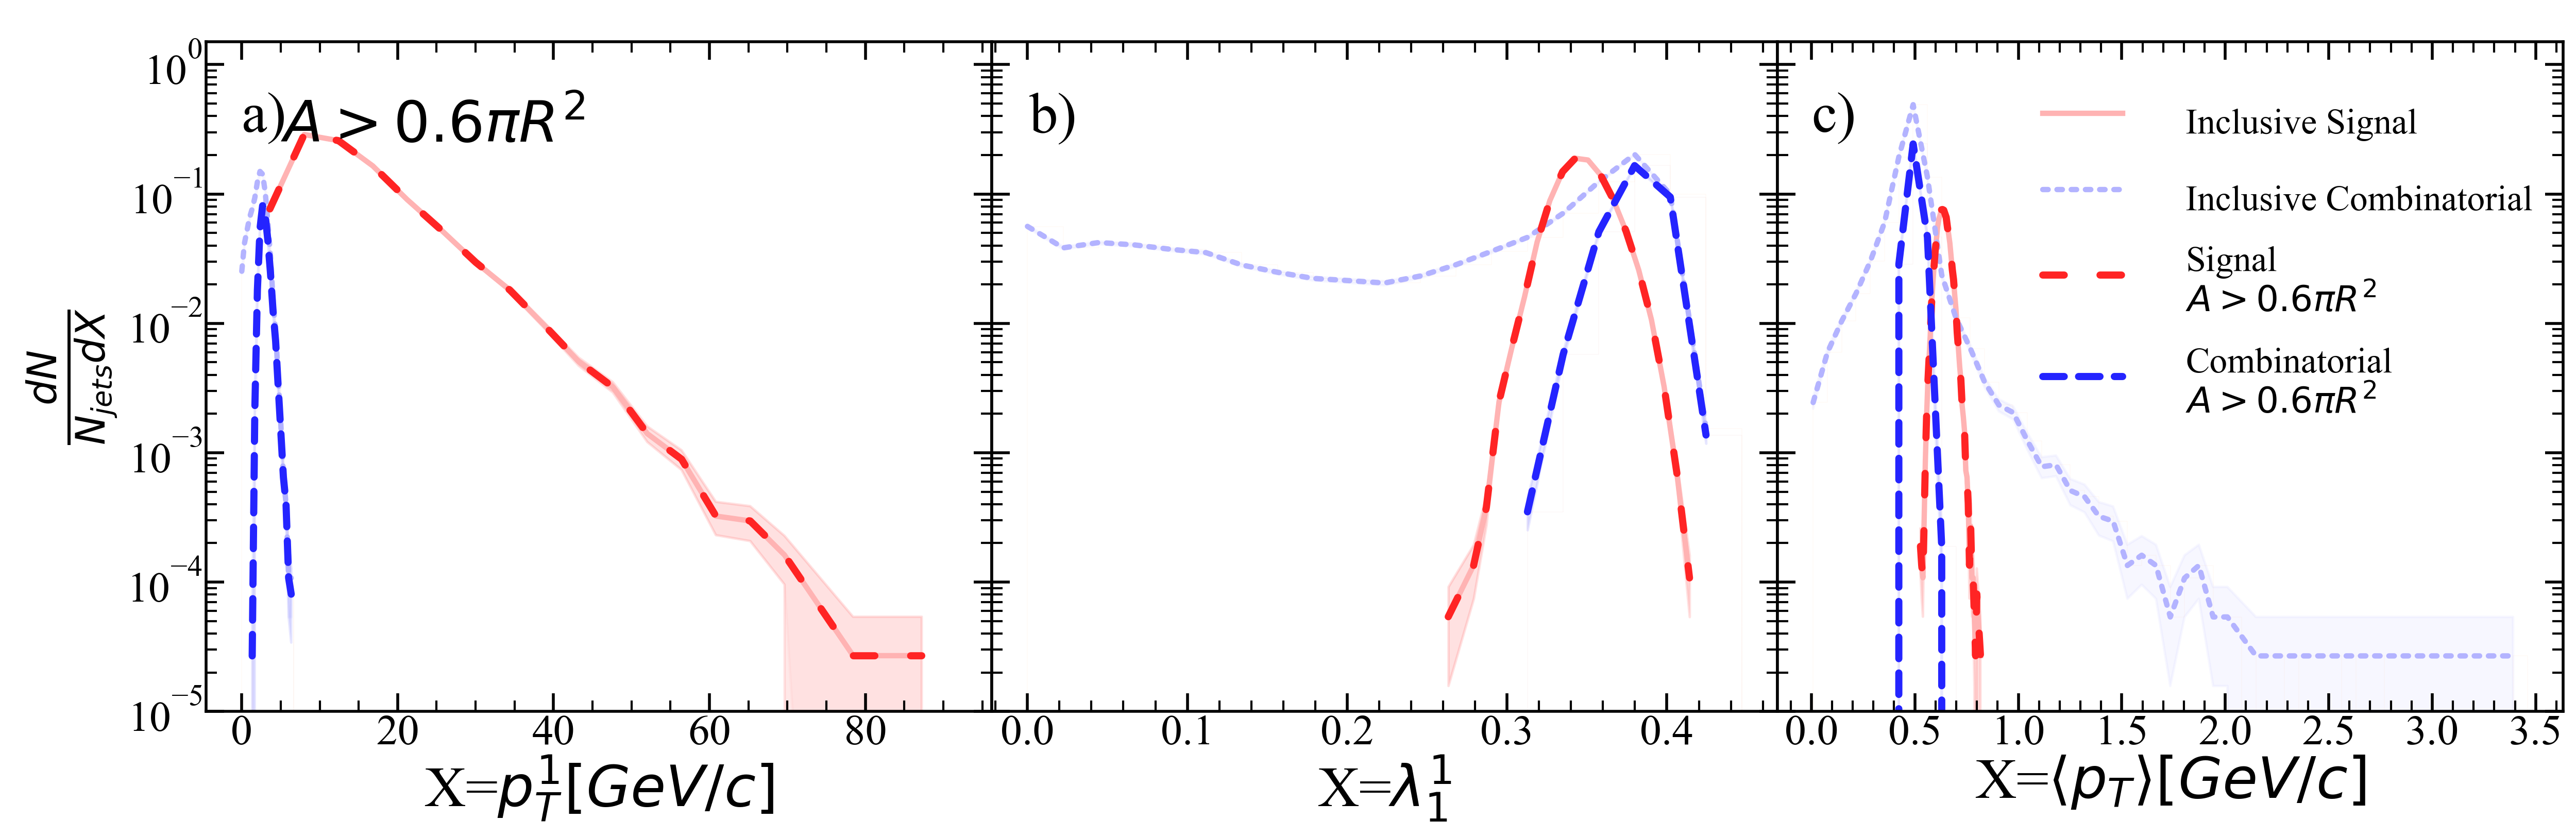}
    \caption{R=0.6 \ptH=60 \GeV}
    \label{fig:area_06_60}
\end{figure*}

\begin{figure*}
    \centering
    \includegraphics[width=\linewidth]{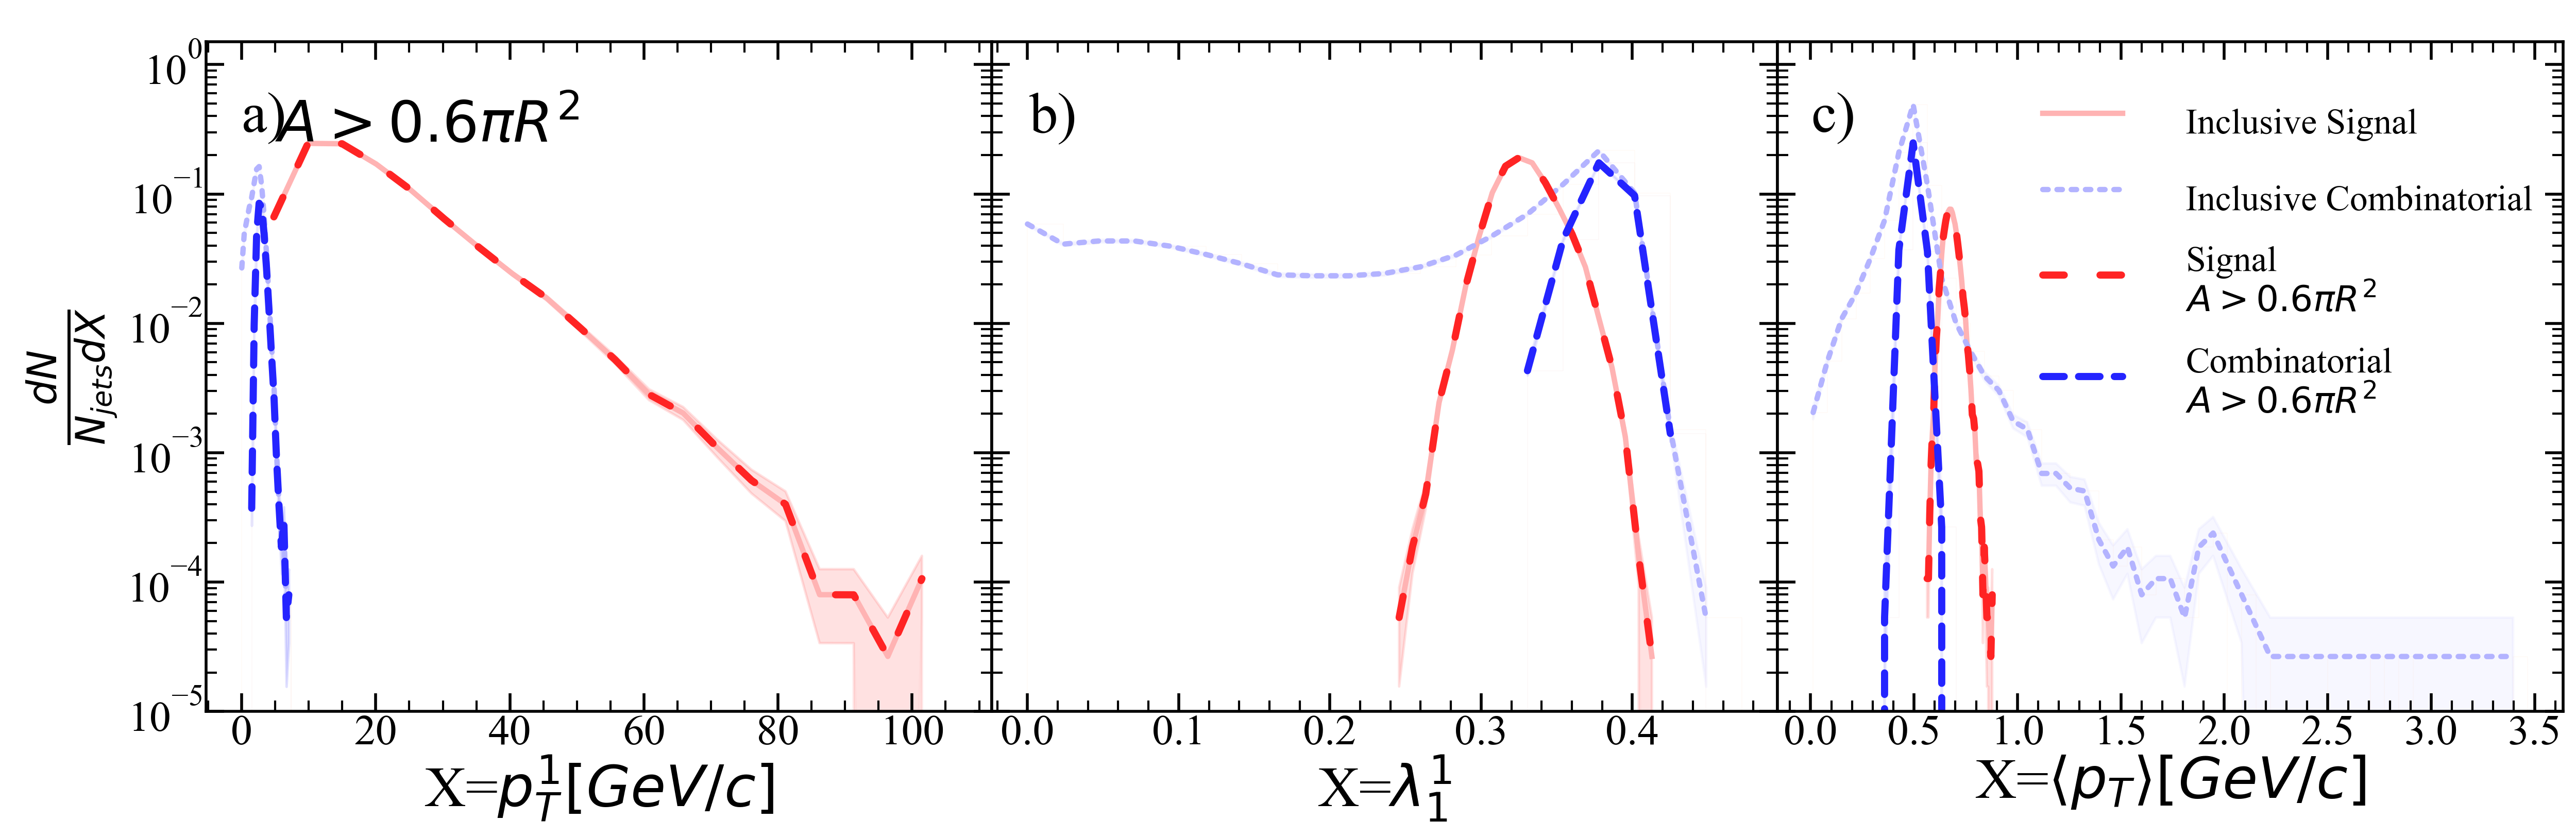}
    \caption{R=0.6 \ptH=80 \GeV}
    \label{fig:area_06_80}
\end{figure*}
\clearpage
\subsection{Area, jet width, and mean constituent momentum after applying the area selection and the tighter leading hadron momentum selection suggested by the machine learning algorithm.}

\begin{figure*}
    \centering
    \includegraphics[width=\linewidth]{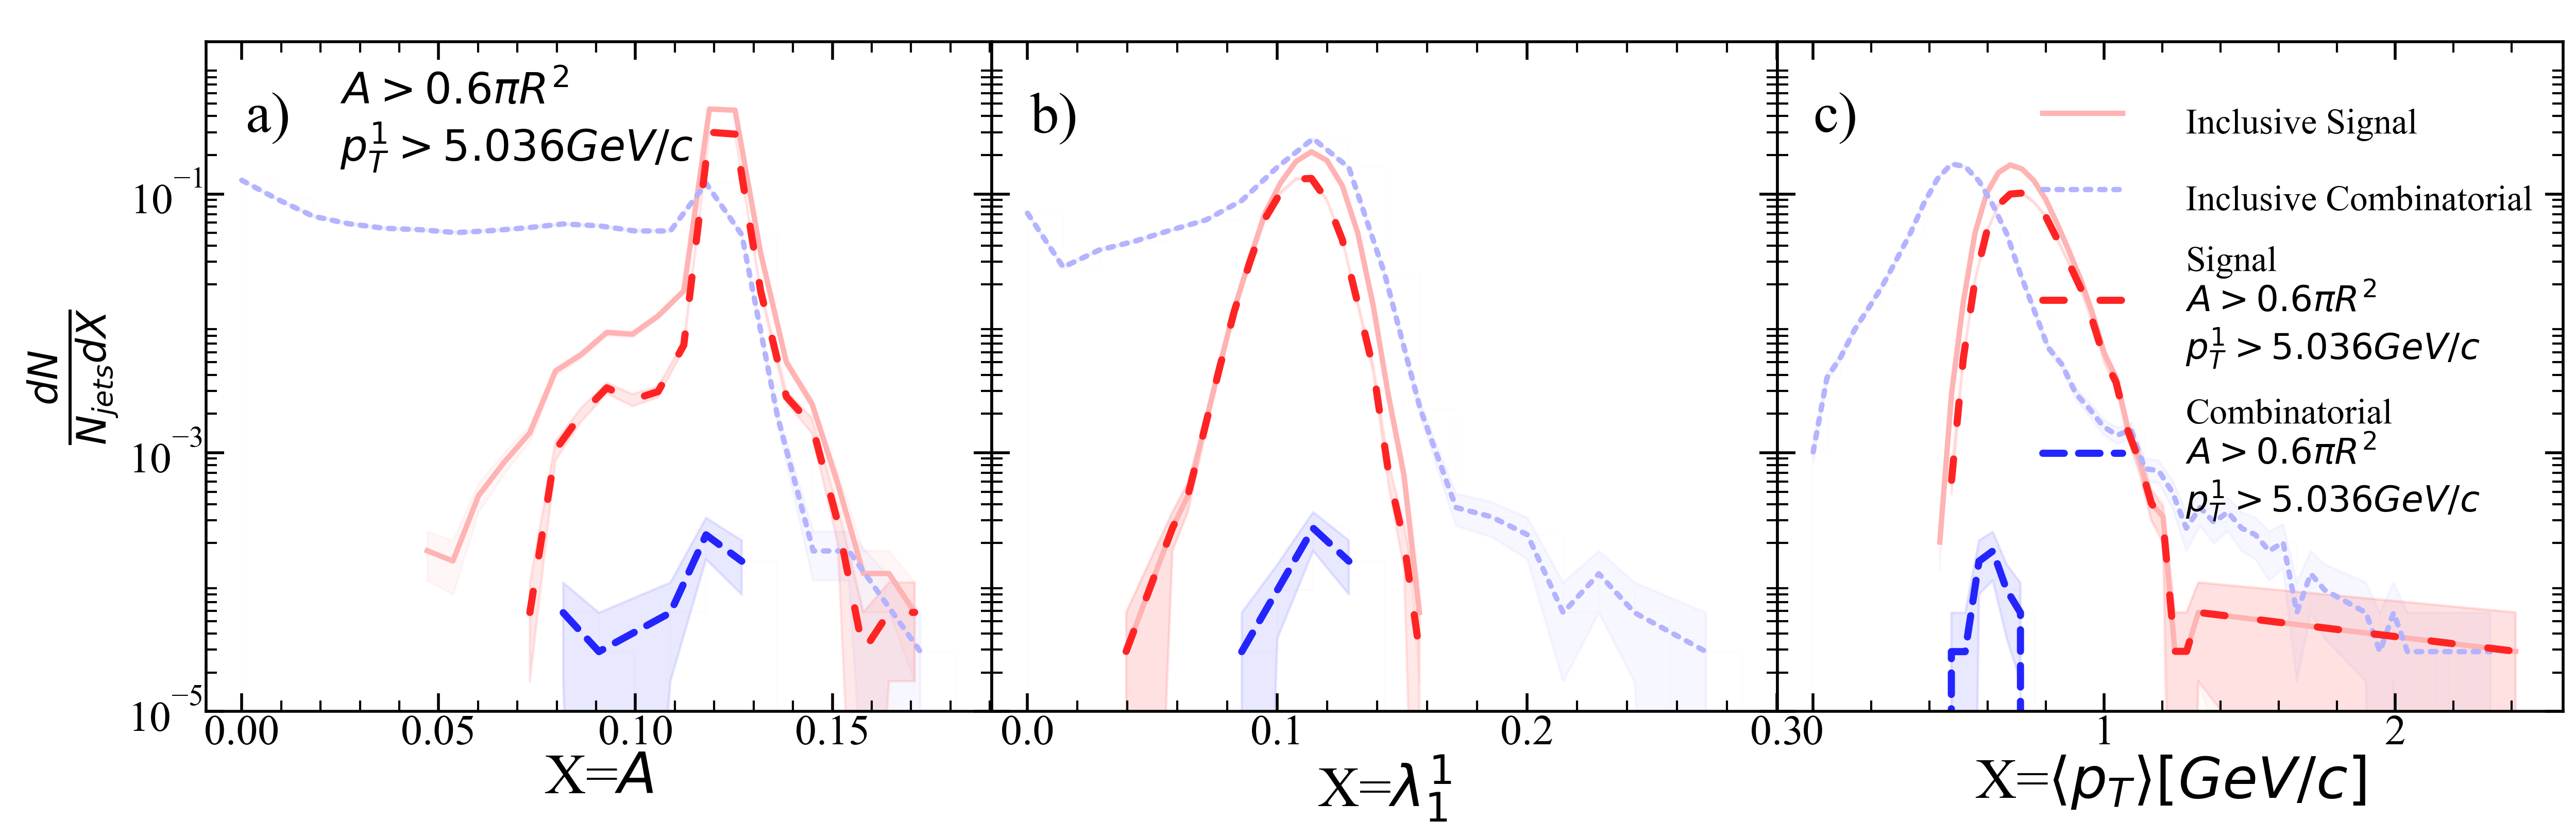}
    \caption{R=0.2 \ptH=10 \GeV}
    \label{fig:ml_02_10}
\end{figure*}

\begin{figure*}
    \centering
    \includegraphics[width=\linewidth]{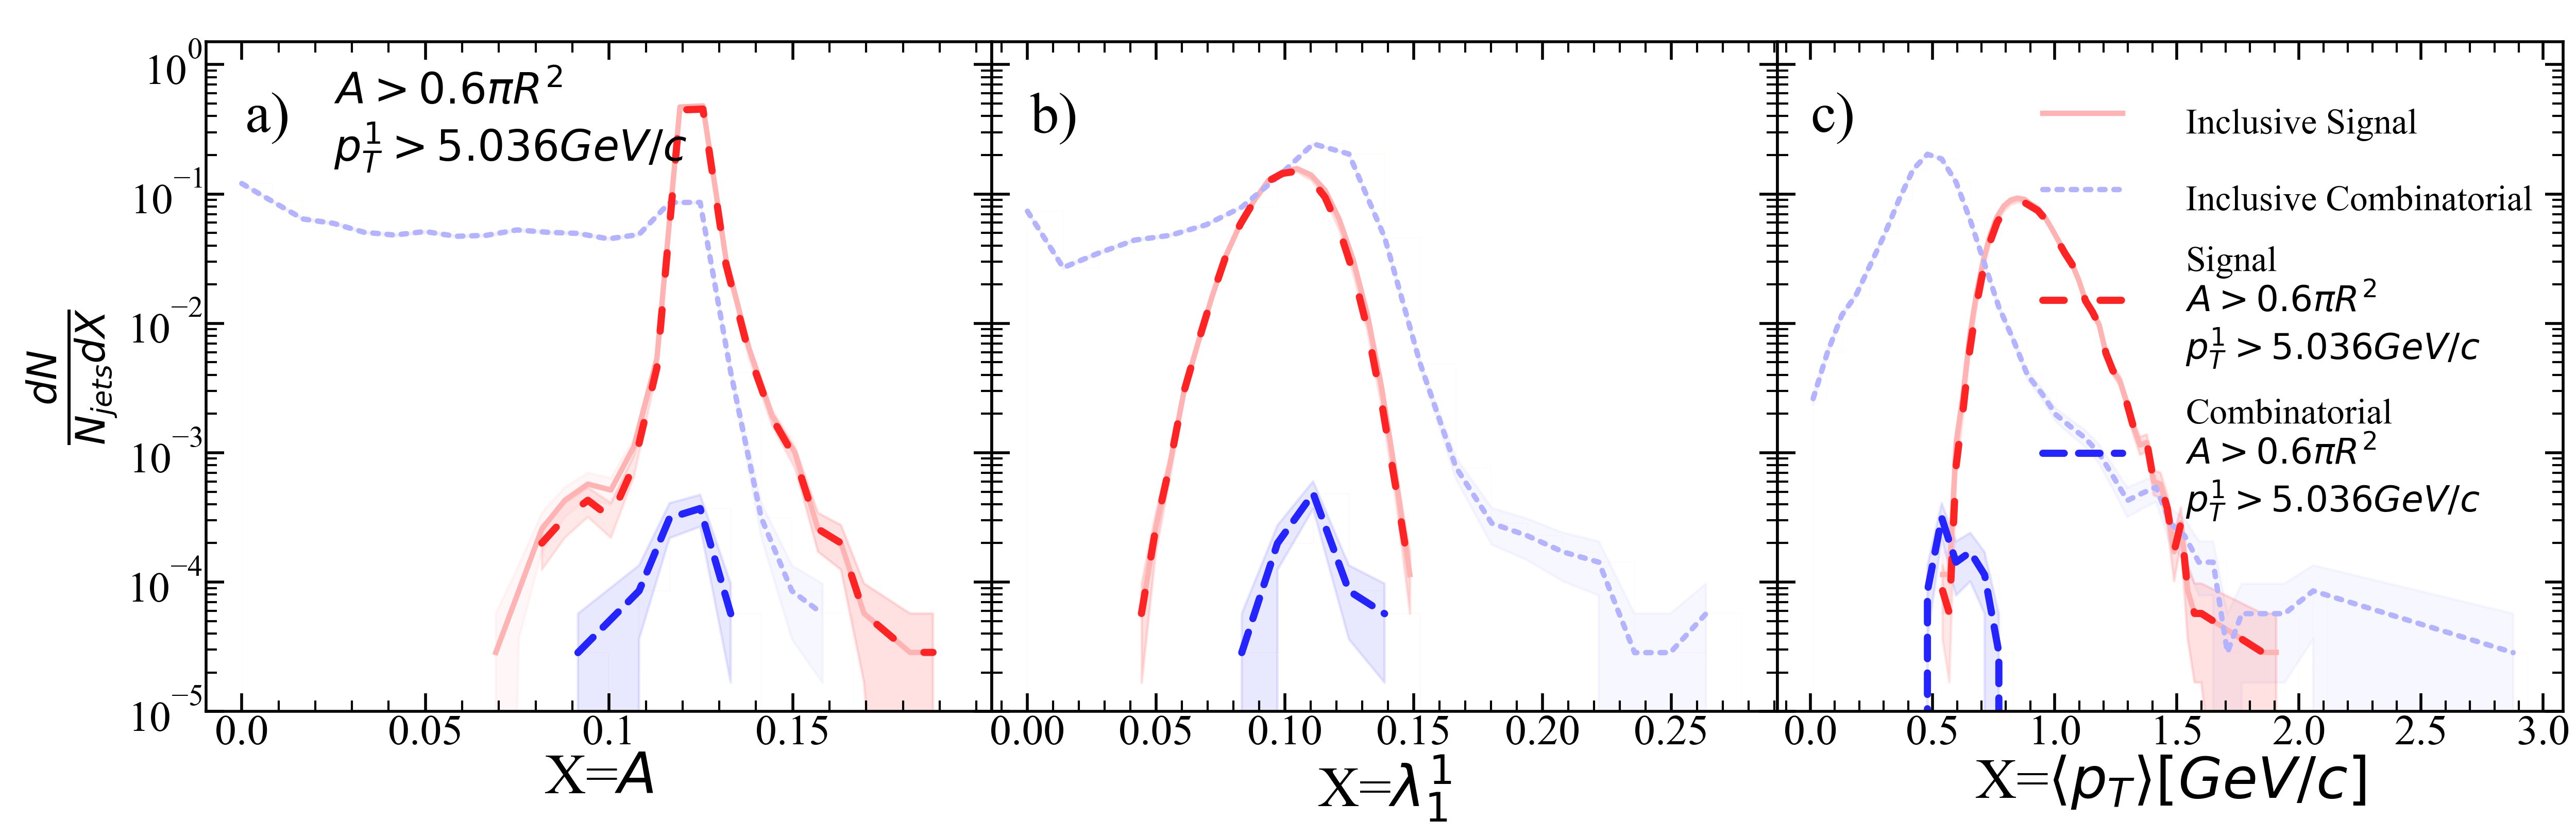}
    \caption{R=0.2 \ptH=20 \GeV}
    \label{fig:ml_02_20}
\end{figure*}

\begin{figure*}
    \centering
    \includegraphics[width=\linewidth]{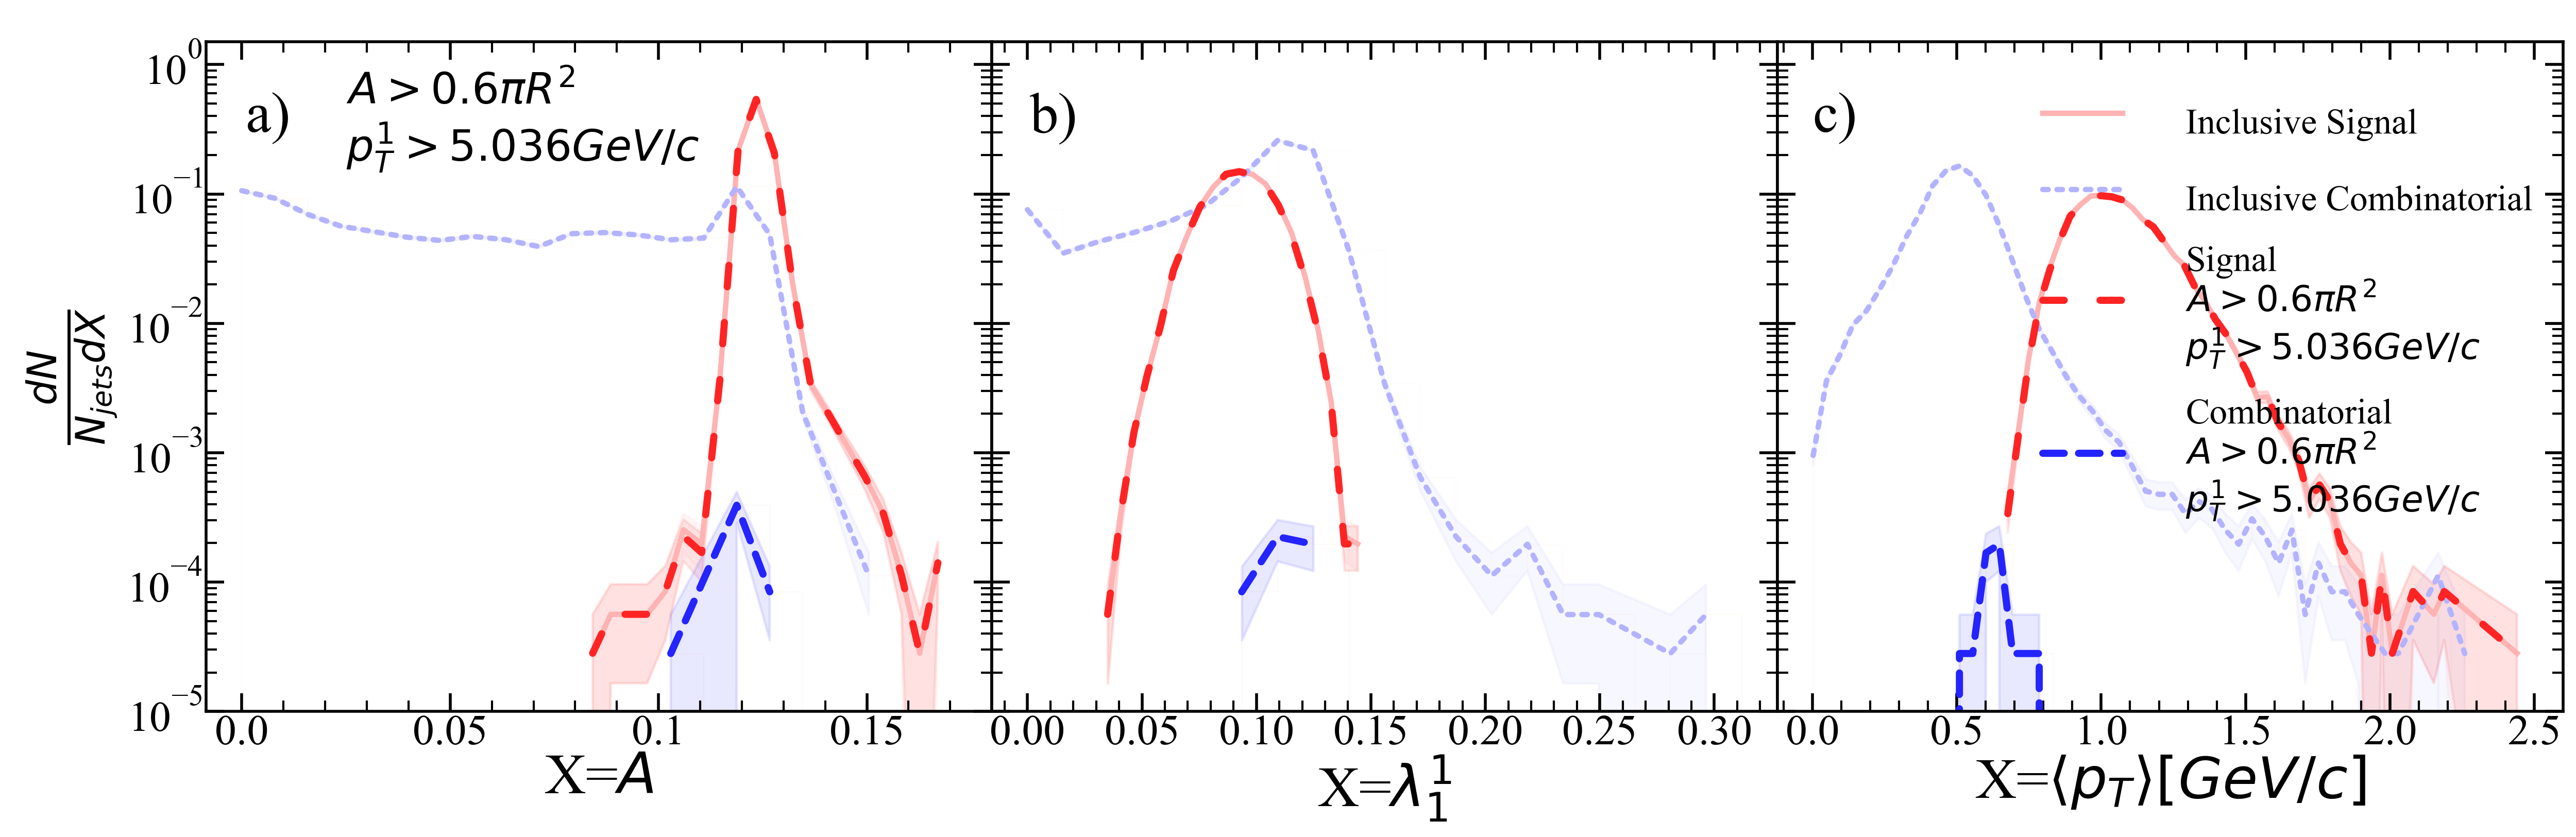}
    \caption{R=0.2 \ptH=30 \GeV}
    \label{fig:ml_02_30}
\end{figure*}

\begin{figure*}
    \centering
    \includegraphics[width=\linewidth]{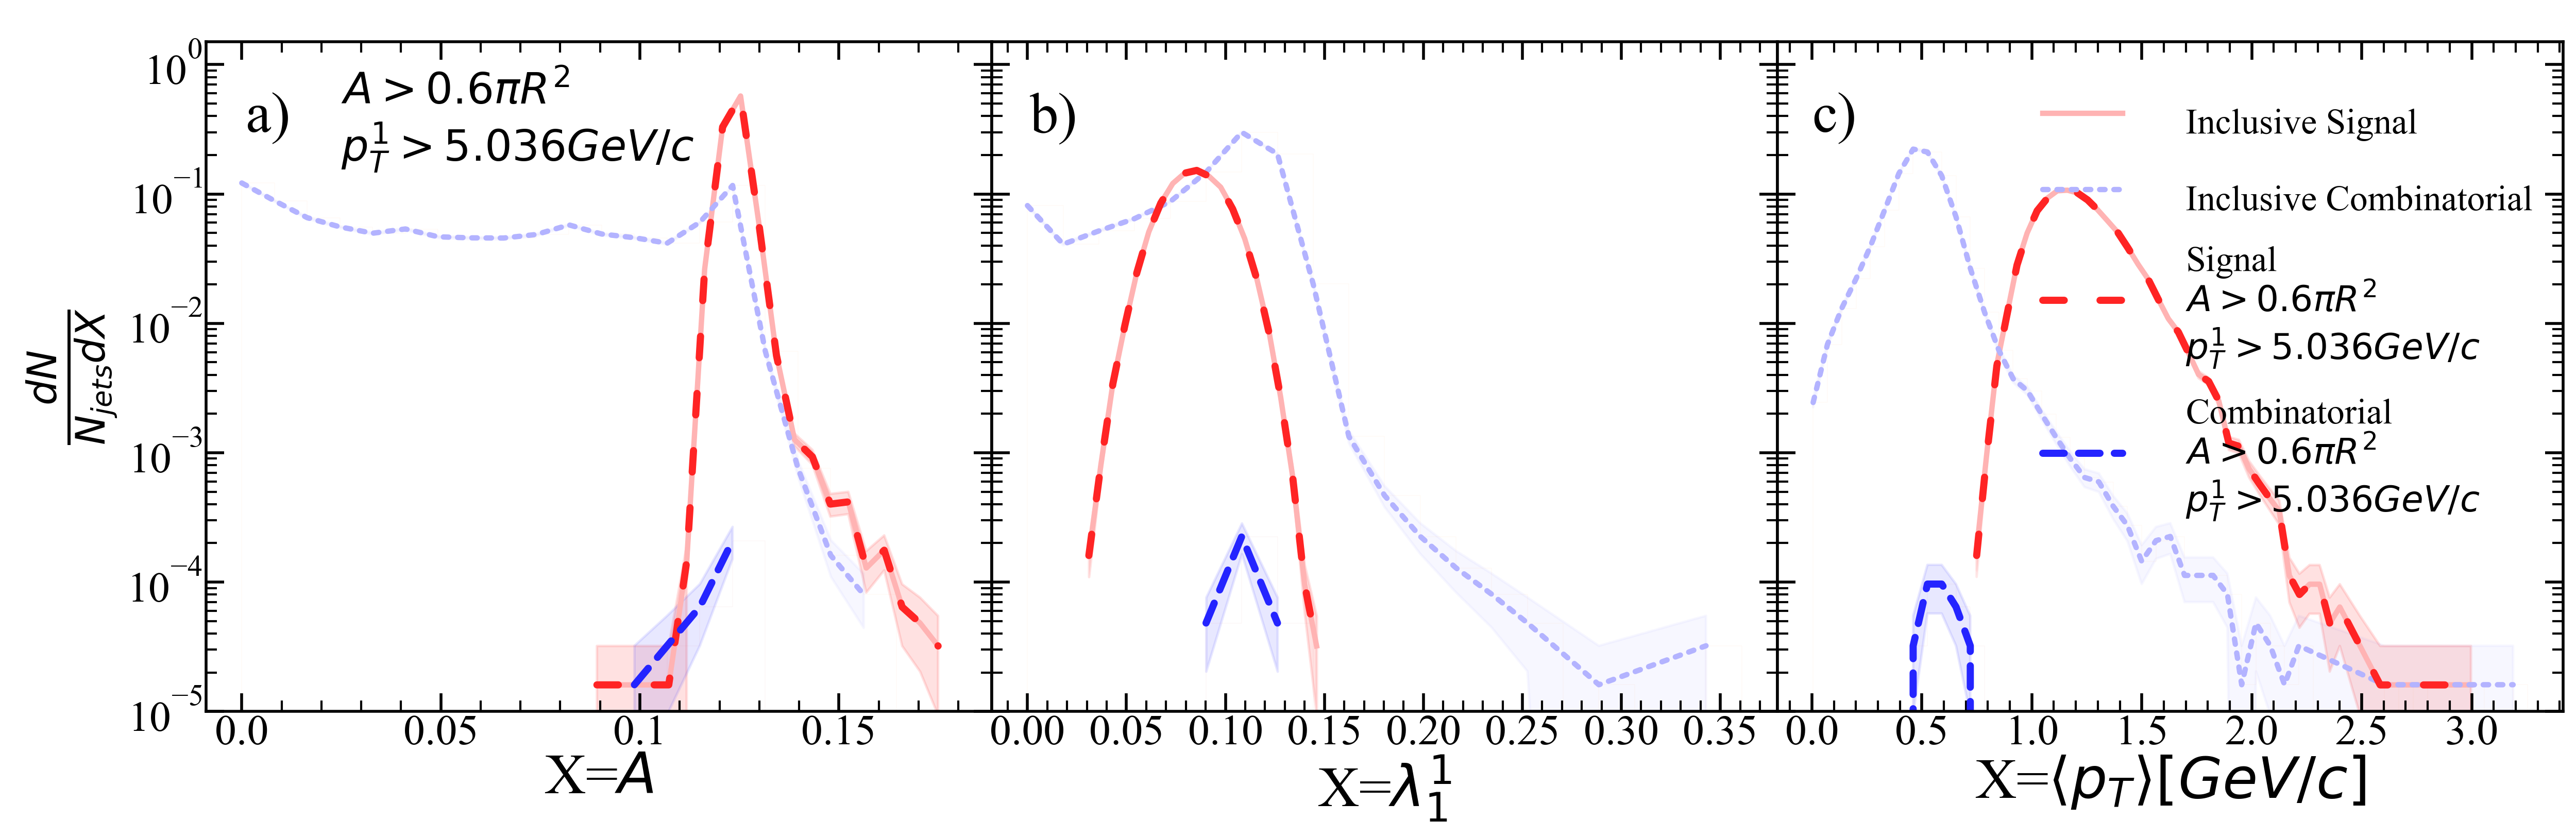}
    \caption{R=0.2 \ptH=40 \GeV}
    \label{fig:ml_02_40}
\end{figure*}

\begin{figure*}
    \centering
    \includegraphics[width=\linewidth]{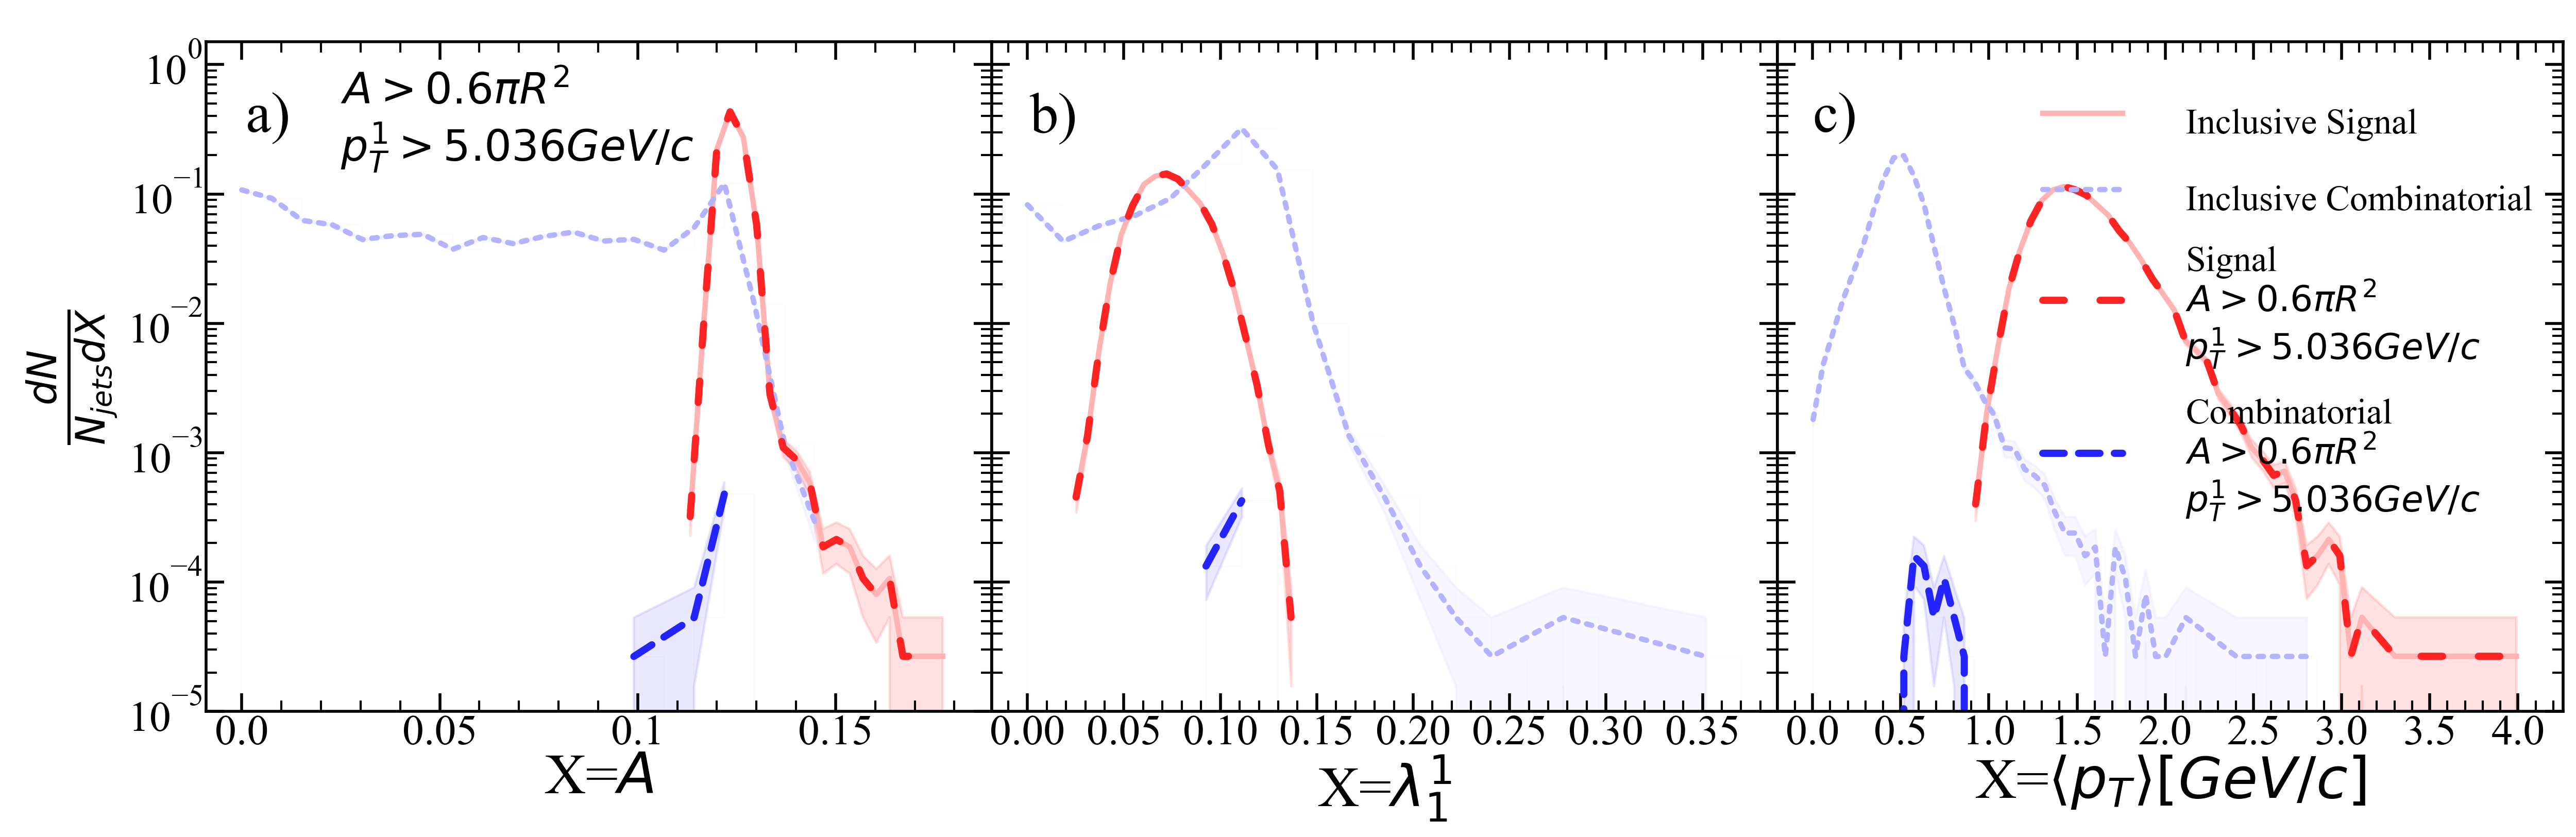}
    \caption{R=0.2 \ptH=60 \GeV}
    \label{fig:ml_02_60}
\end{figure*}

\begin{figure*}
    \centering
    \includegraphics[width=\linewidth]{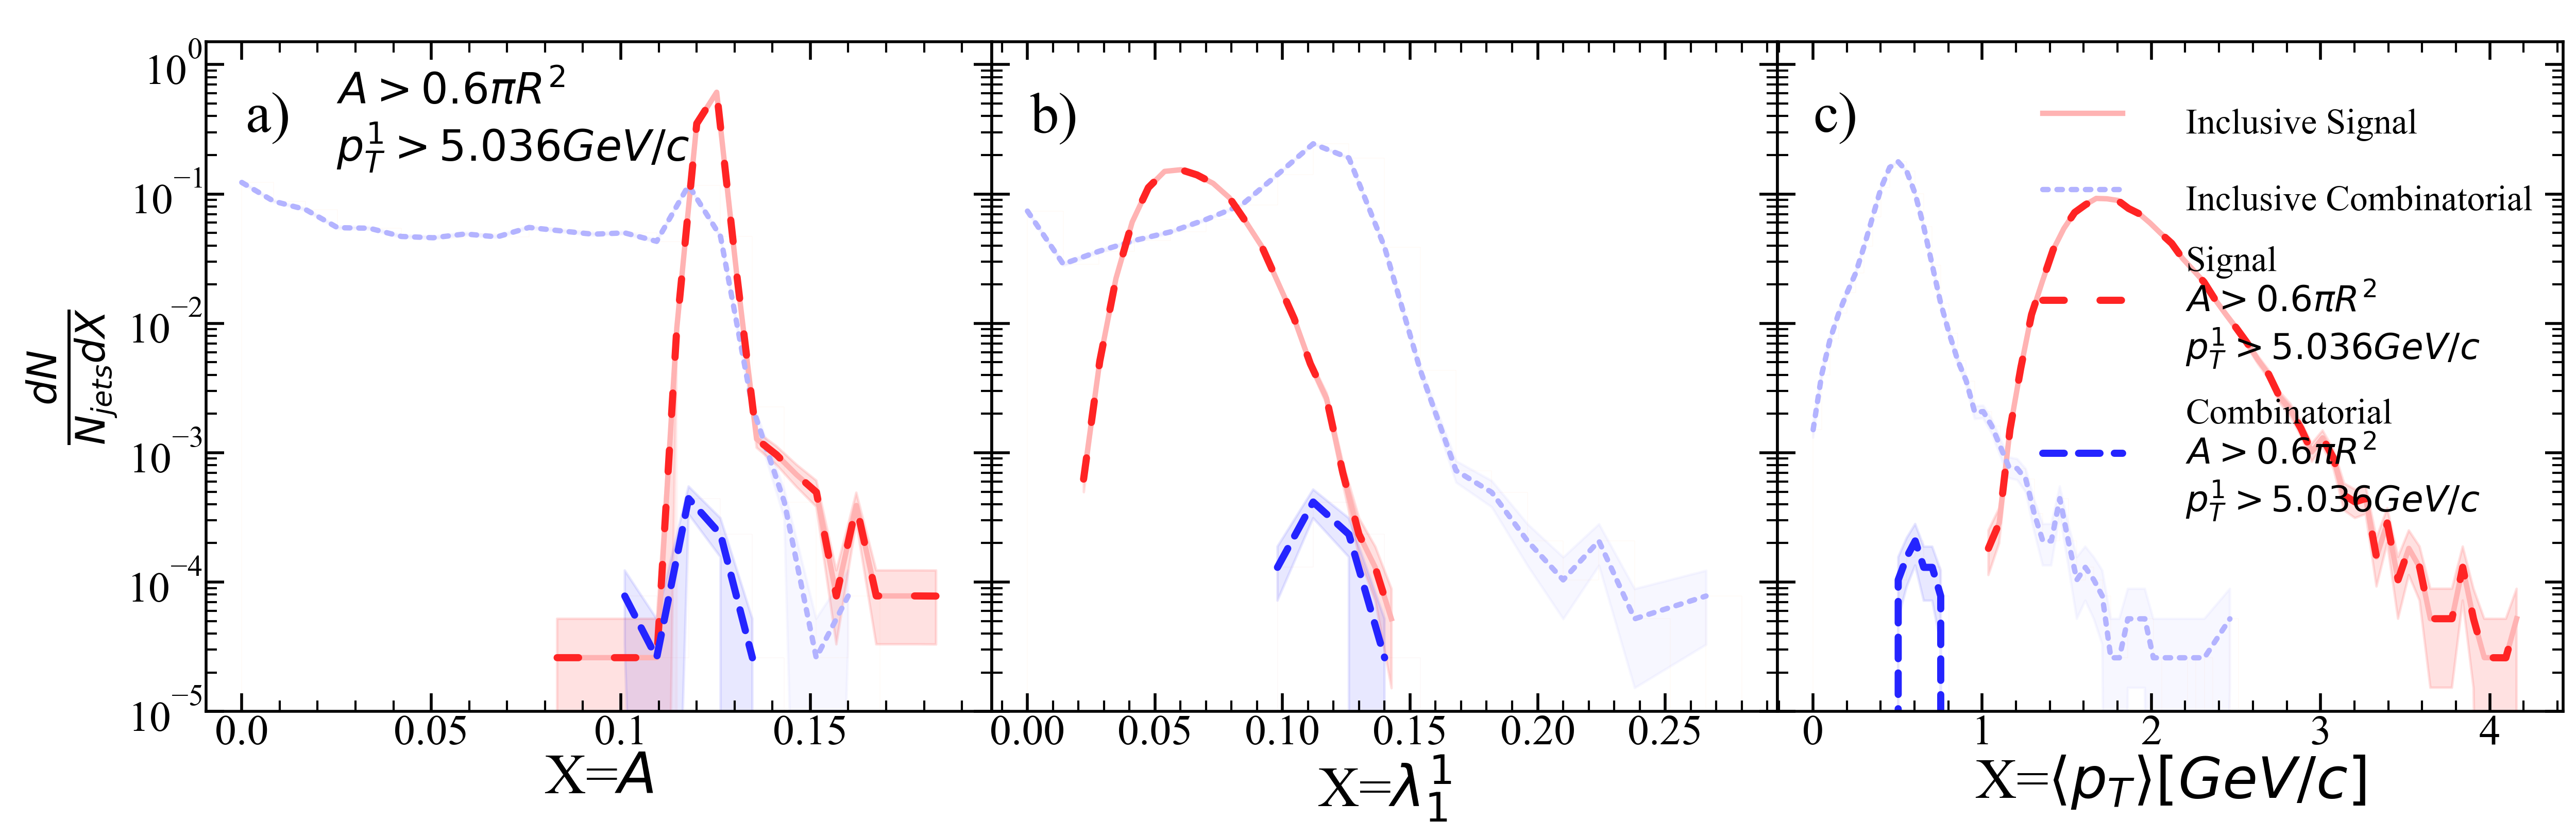}
    \caption{R=0.2 \ptH=80 \GeV}
    \label{fig:ml_02_80}
\end{figure*}

\begin{figure*}
    \centering
    \includegraphics[width=\linewidth]{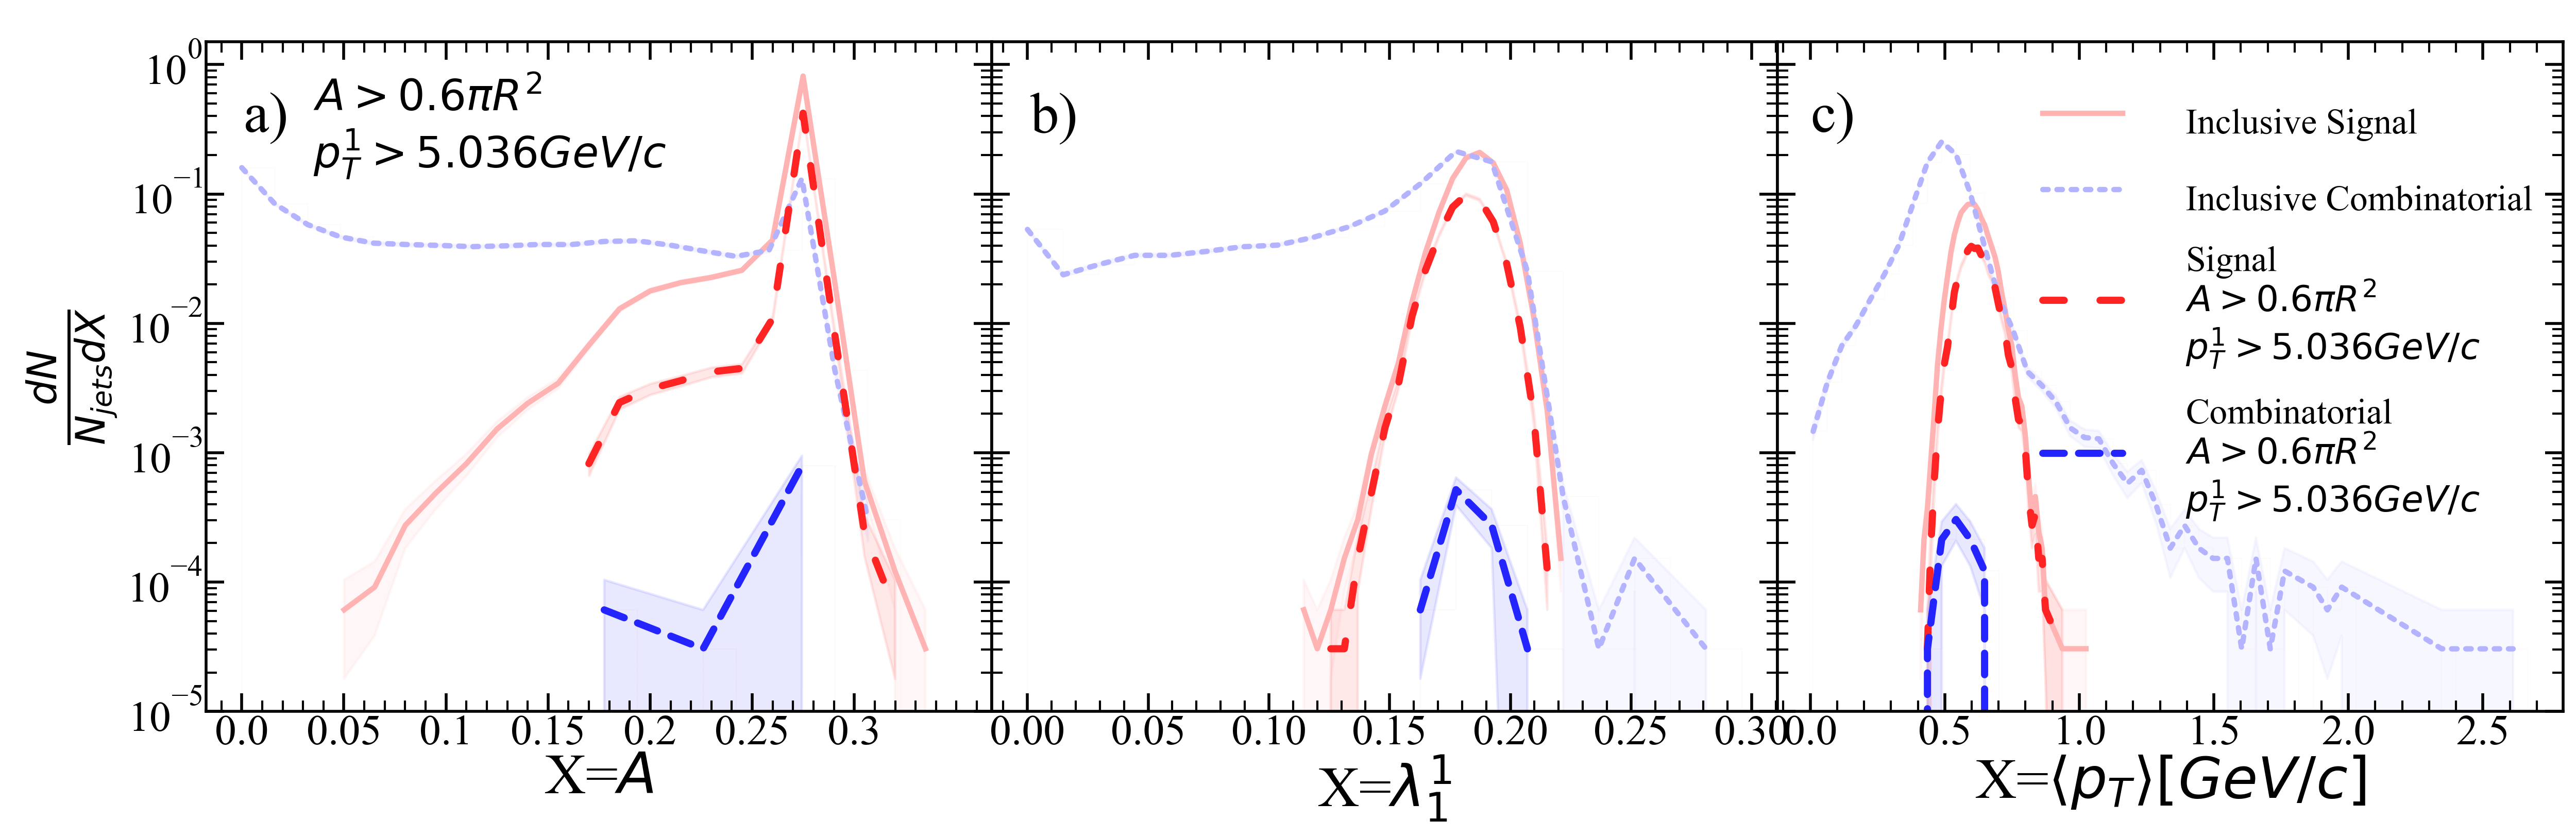}
    \caption{R=0.3 \ptH=10 \GeV}
    \label{fig:ml_03_10}
\end{figure*}

\begin{figure*}
    \centering
    \includegraphics[width=\linewidth]{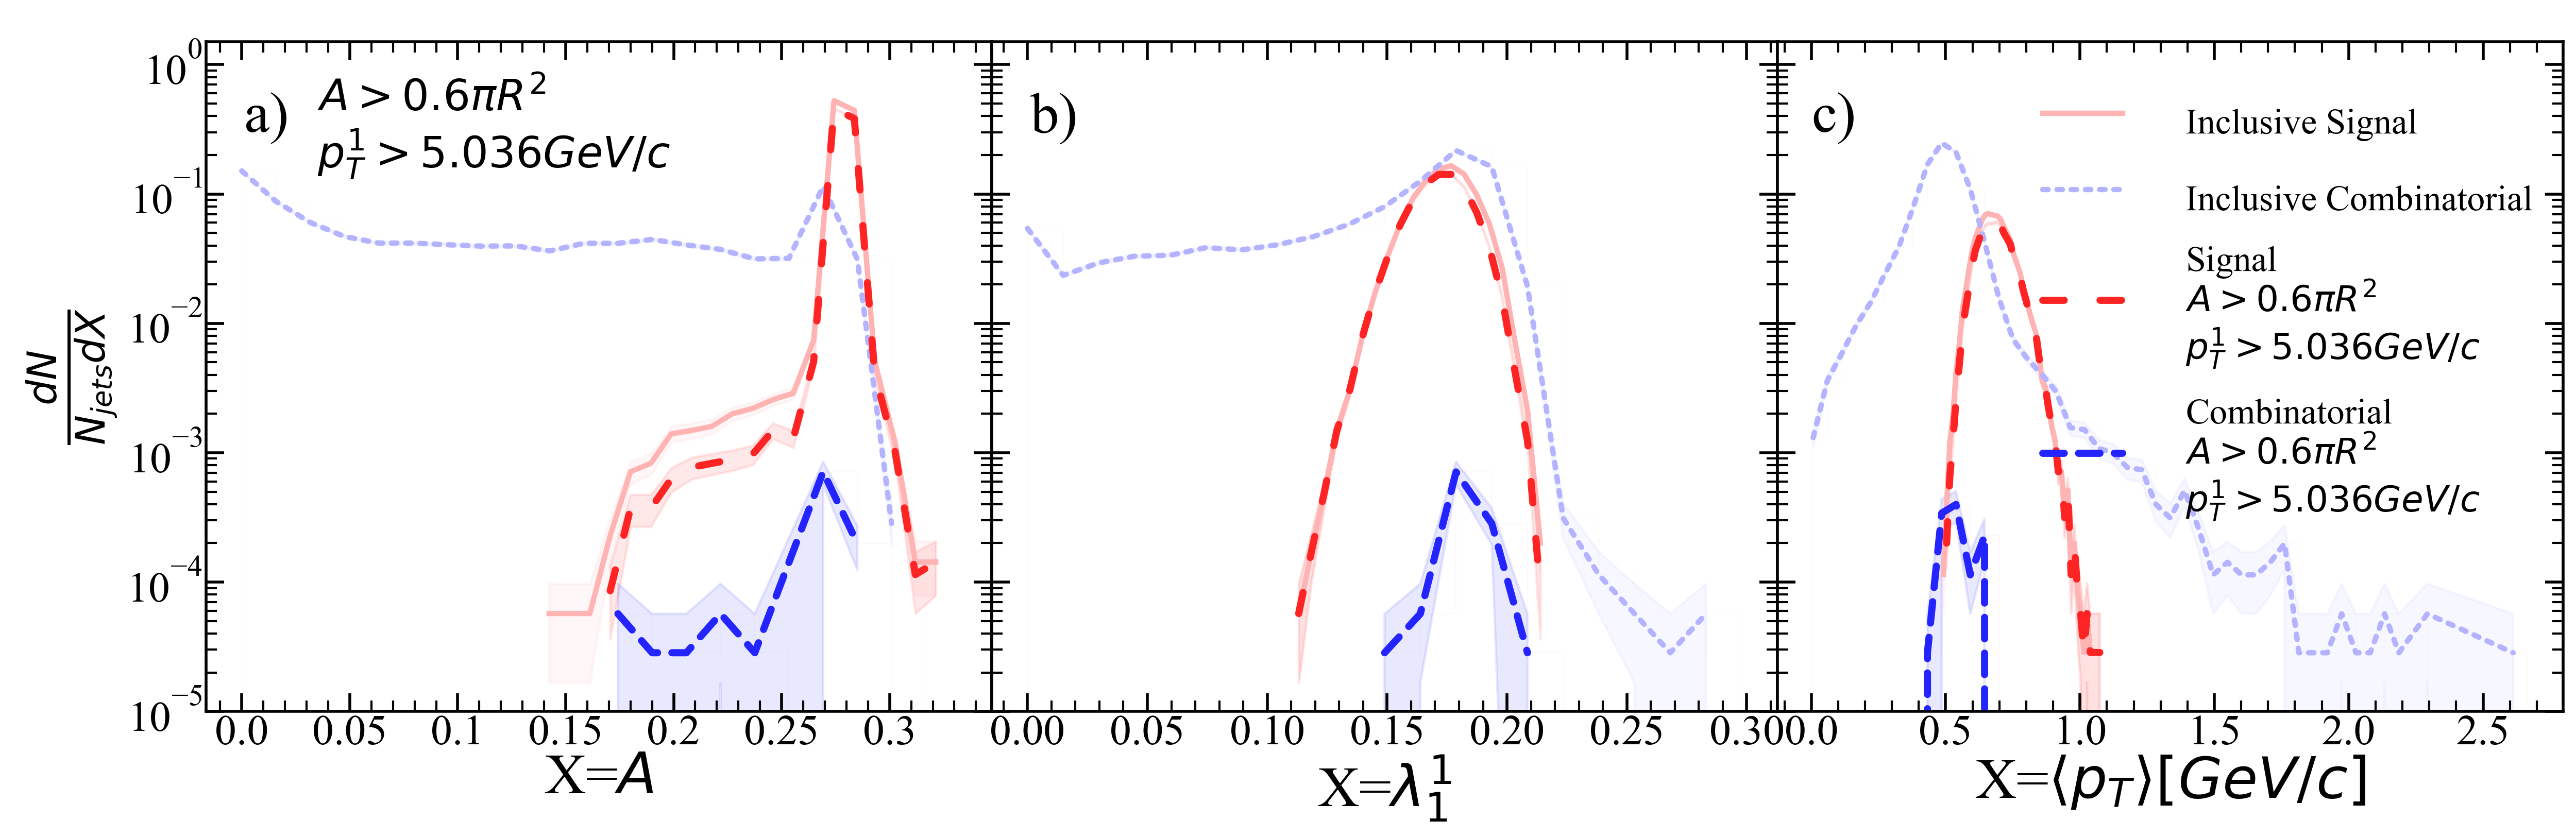}
    \caption{R=0.3 \ptH=20 \GeV}
    \label{fig:ml_03_20}
\end{figure*}

\begin{figure*}
    \centering
    \includegraphics[width=\linewidth]{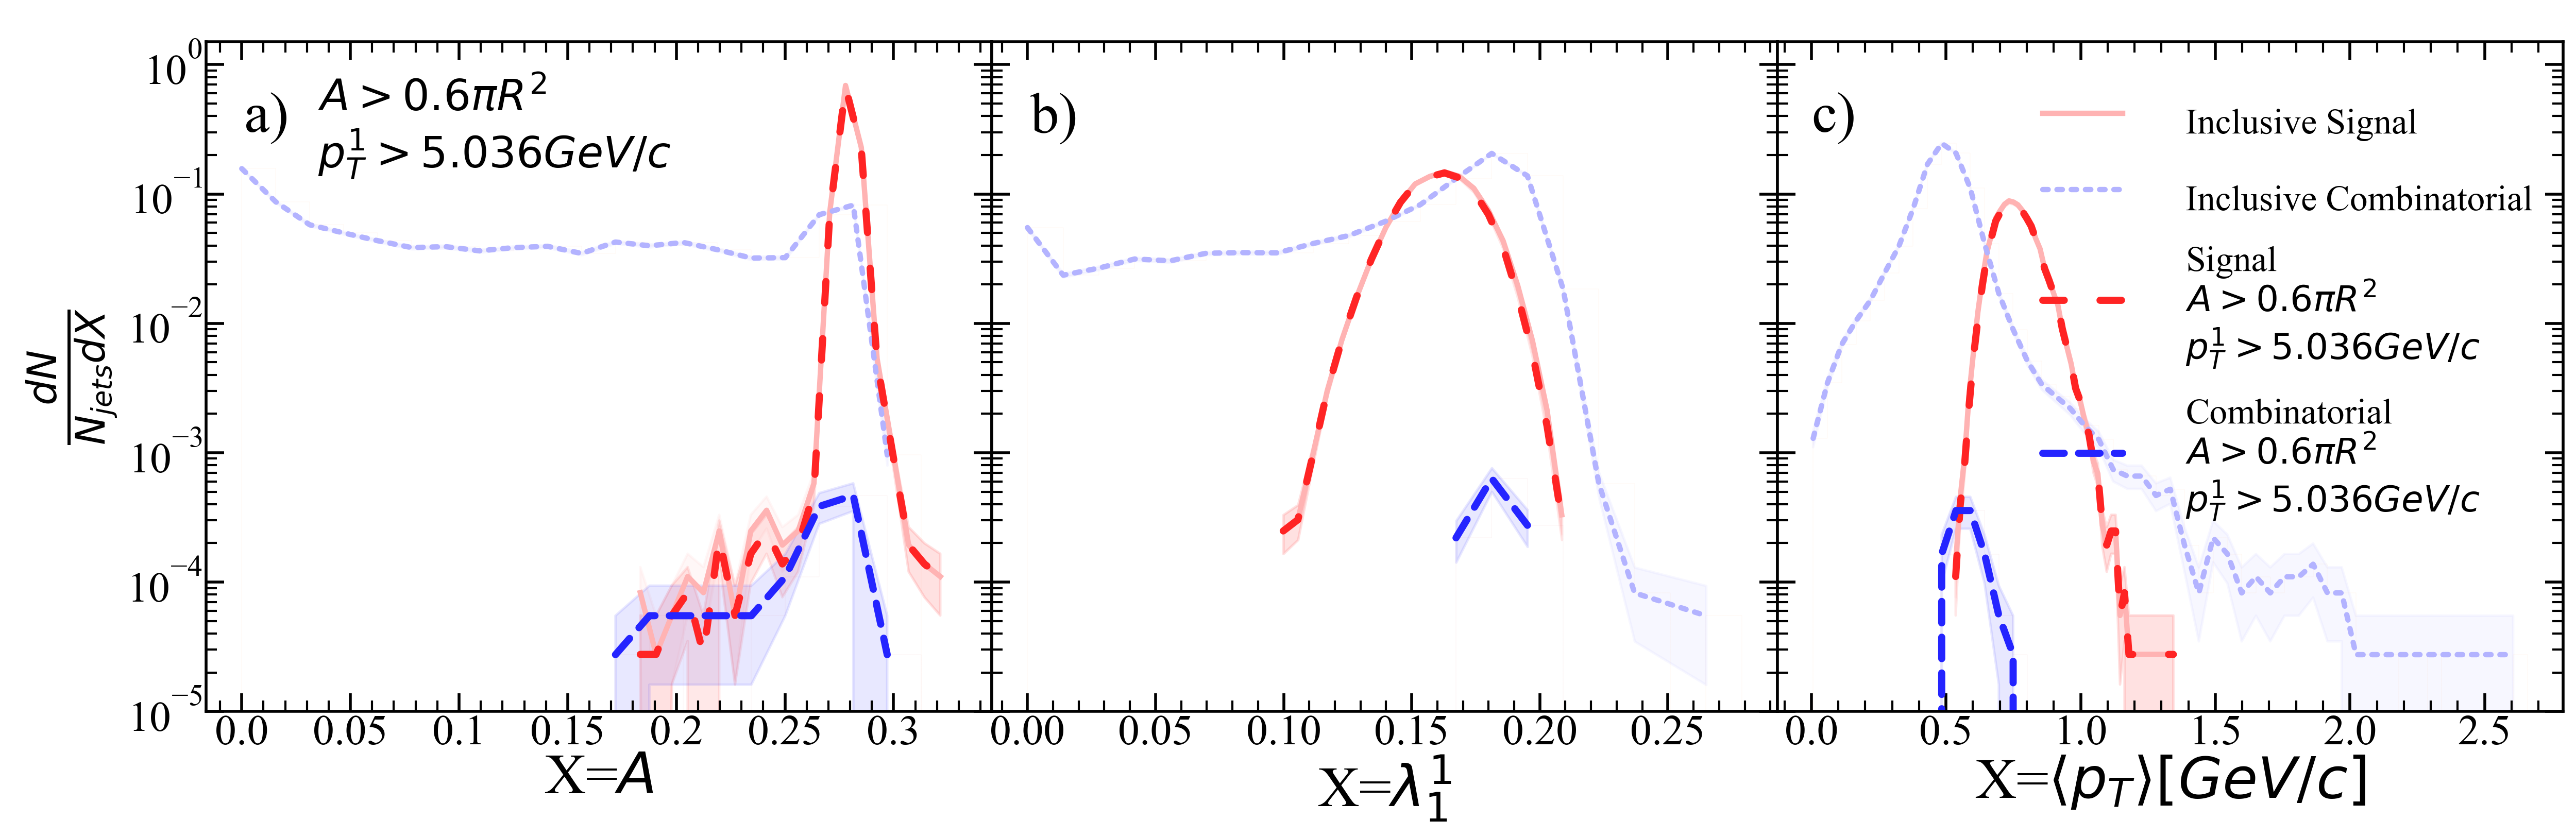}
    \caption{R=0.3 \ptH=30 \GeV}
    \label{fig:ml_03_30}
\end{figure*}

\begin{figure*}
    \centering
    \includegraphics[width=\linewidth]{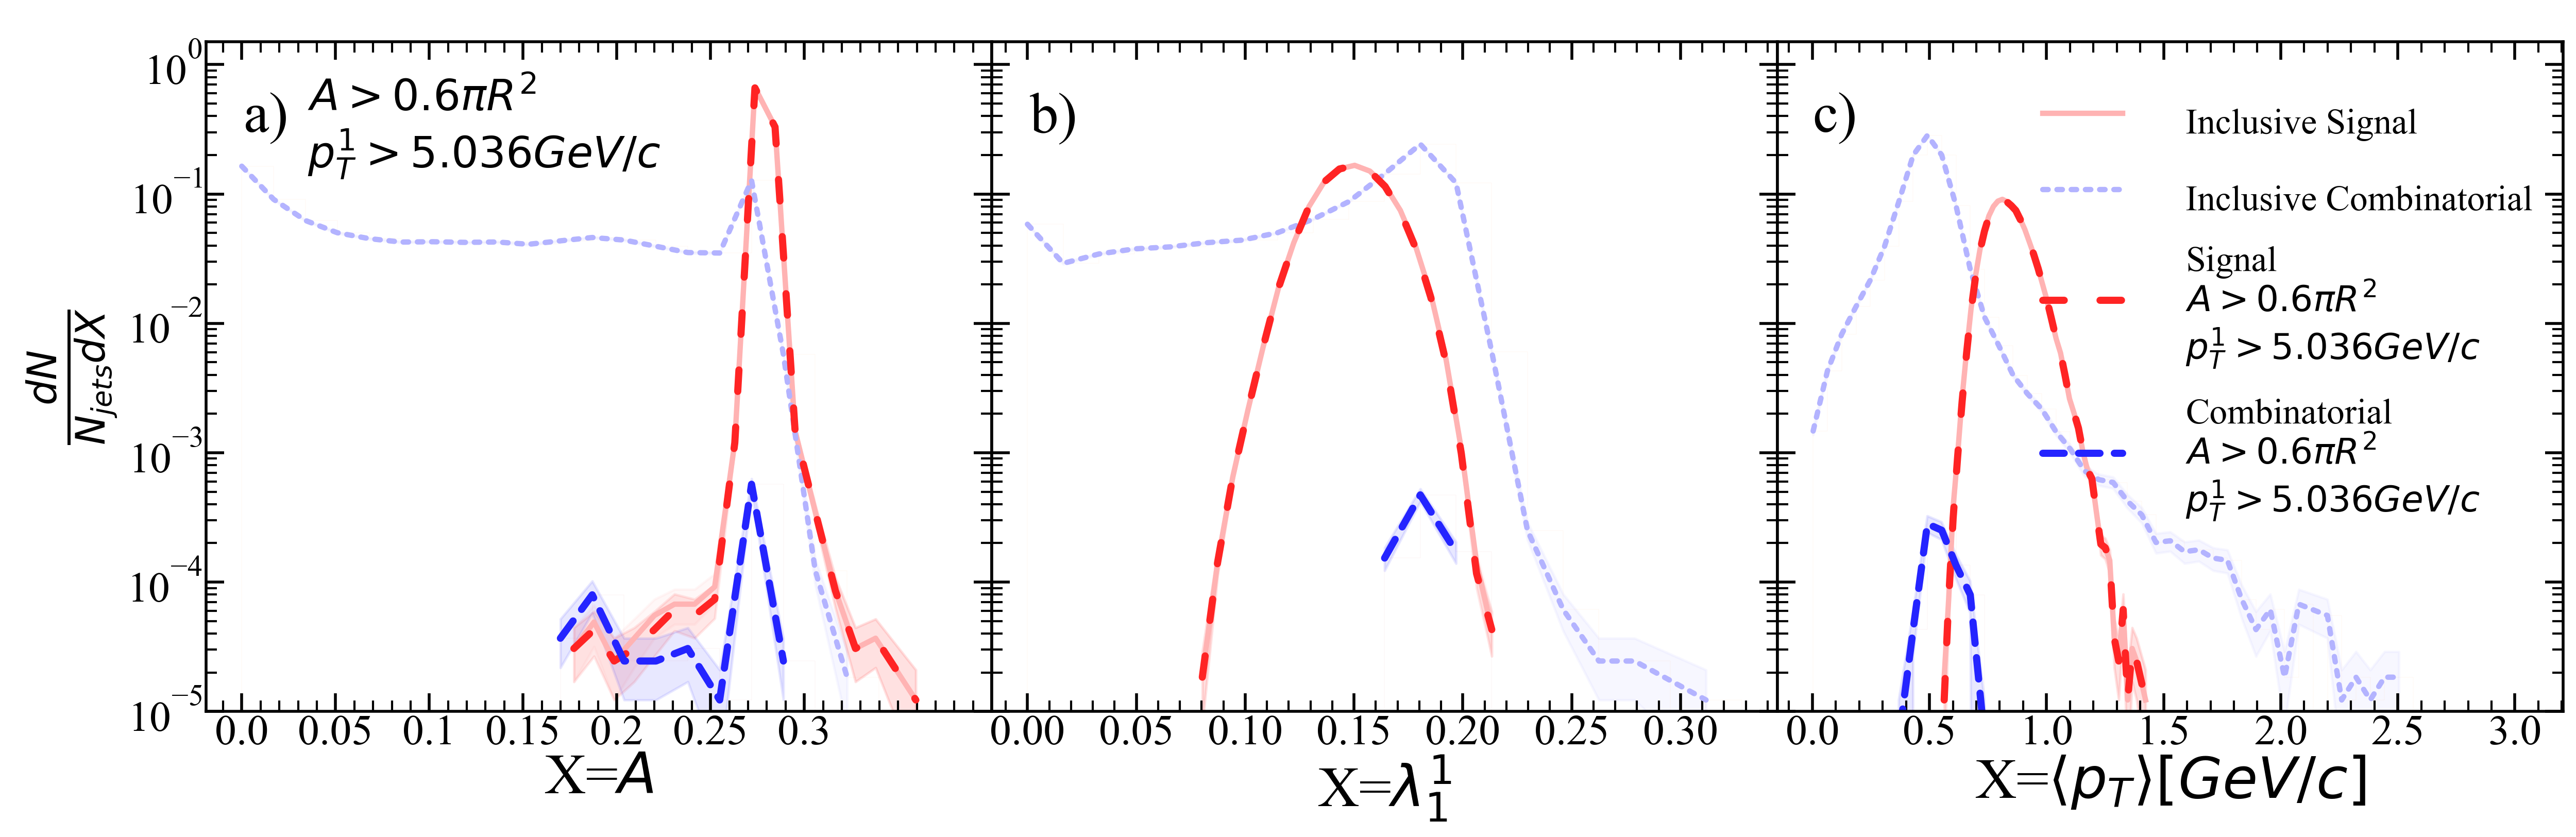}
    \caption{R=0.3 \ptH=40 \GeV}
    \label{fig:ml_03_40}
\end{figure*}

\begin{figure*}
    \centering
    \includegraphics[width=\linewidth]{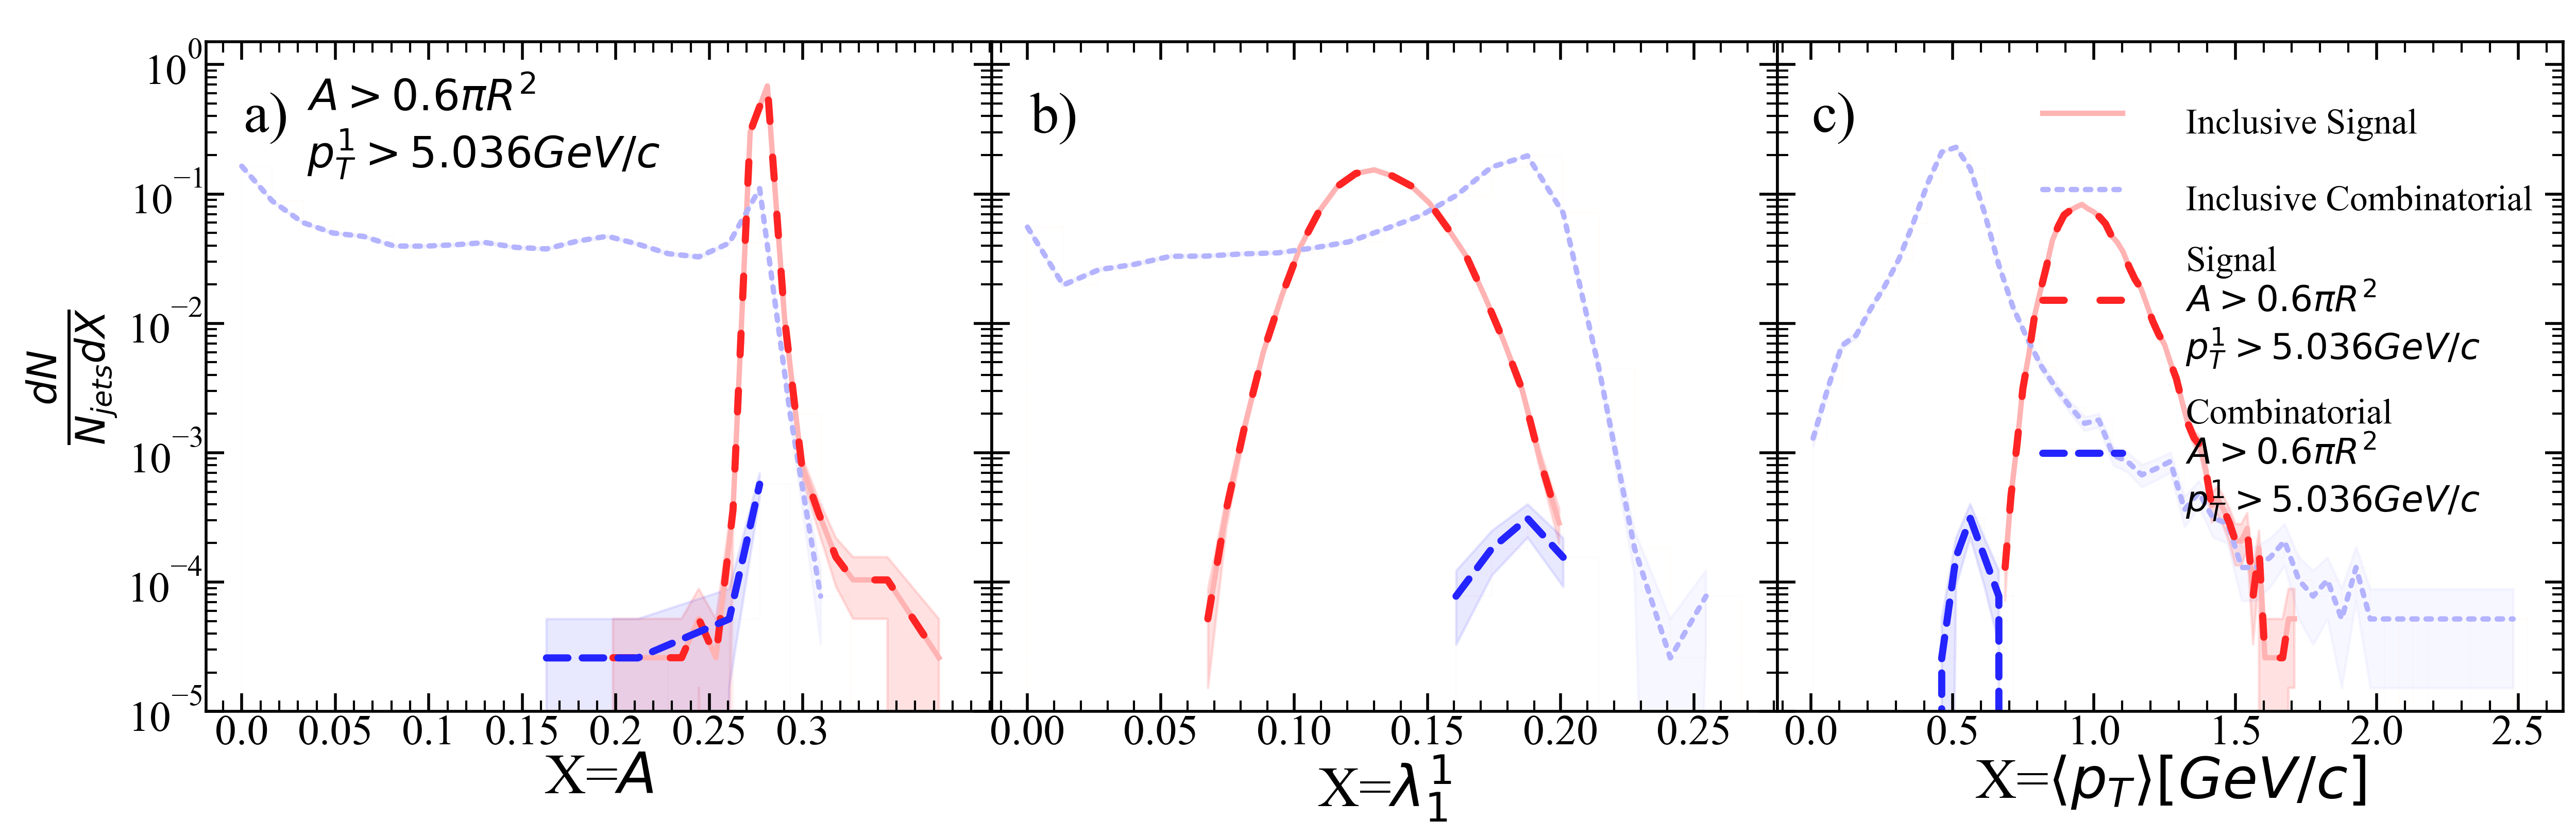}
    \caption{R=0.3 \ptH=60 \GeV}
    \label{fig:ml_03_60}
\end{figure*}

\begin{figure*}
    \centering
    \includegraphics[width=\linewidth]{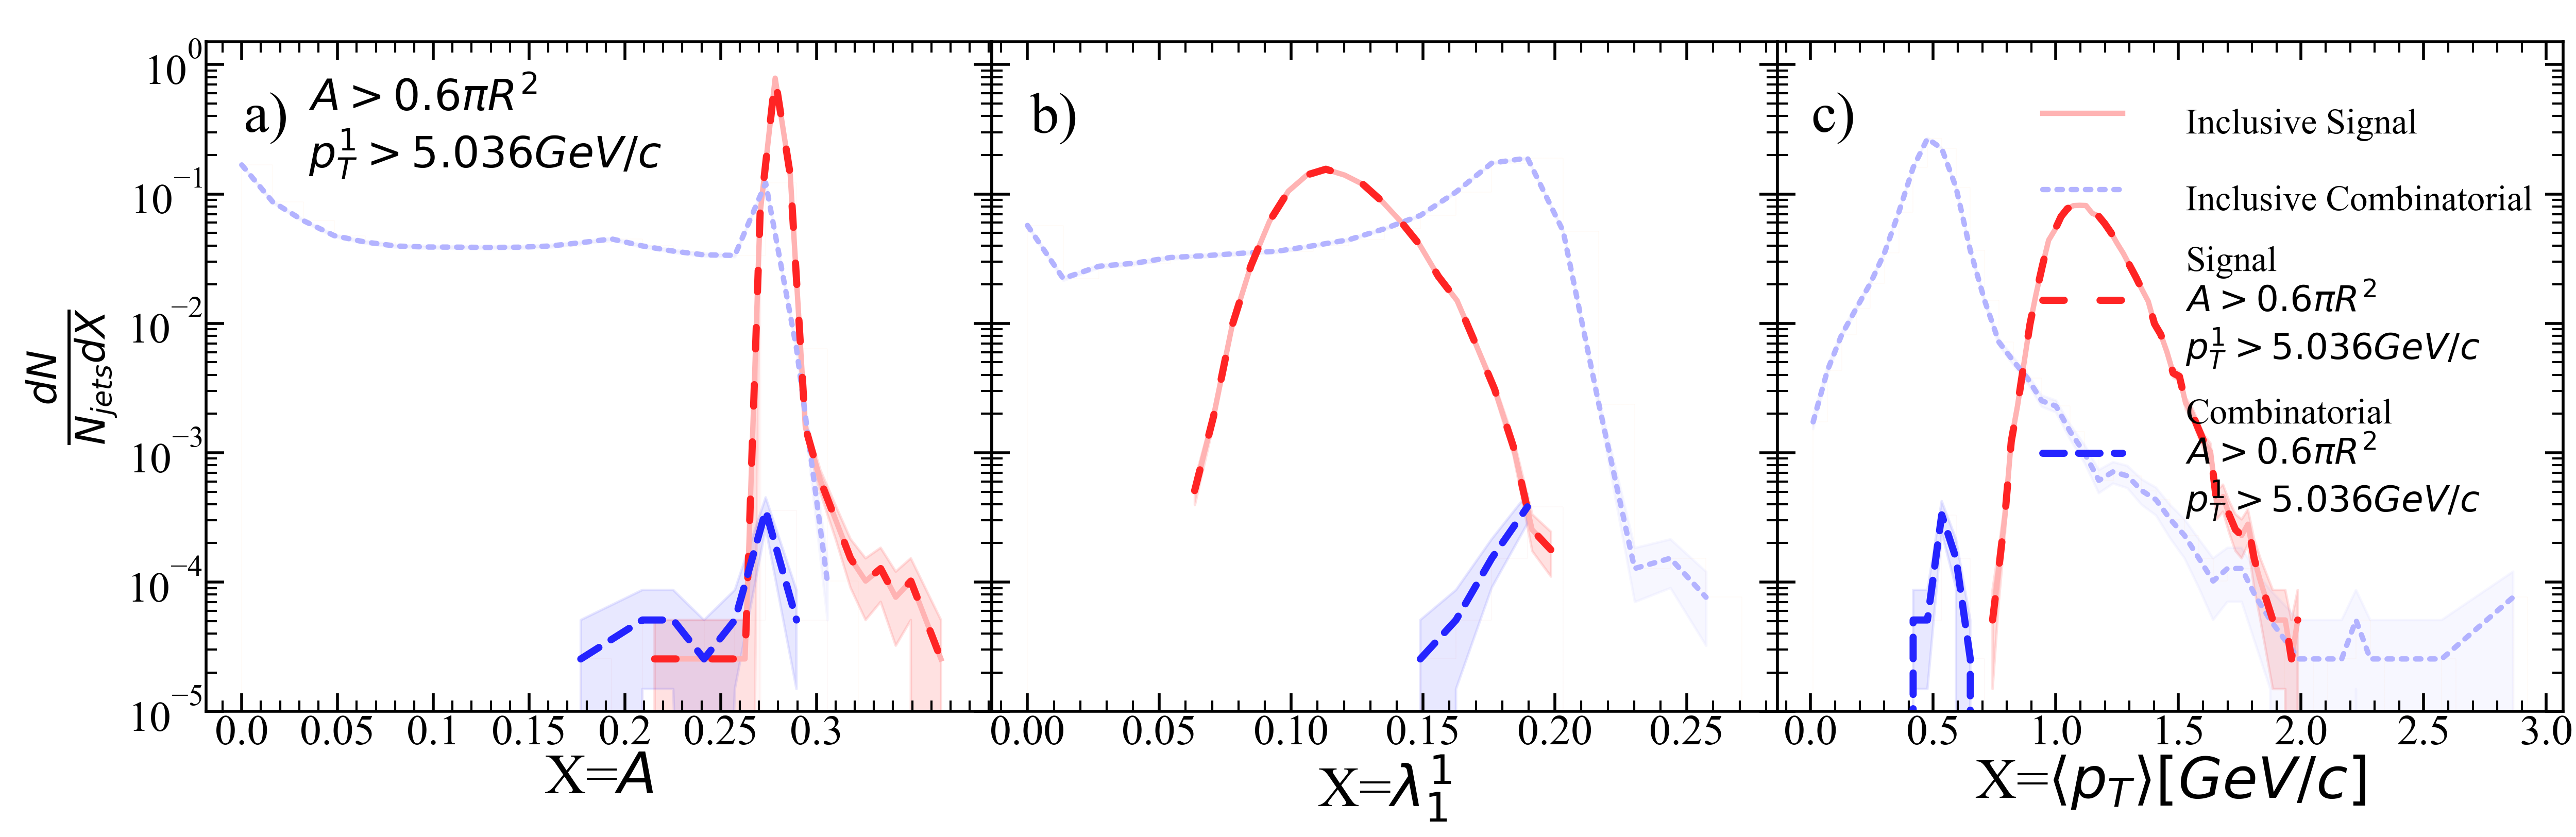}
    \caption{R=0.3 \ptH=80 \GeV}
    \label{fig:ml_03_80}
\end{figure*}

\begin{figure*}
    \centering
    \includegraphics[width=\linewidth]{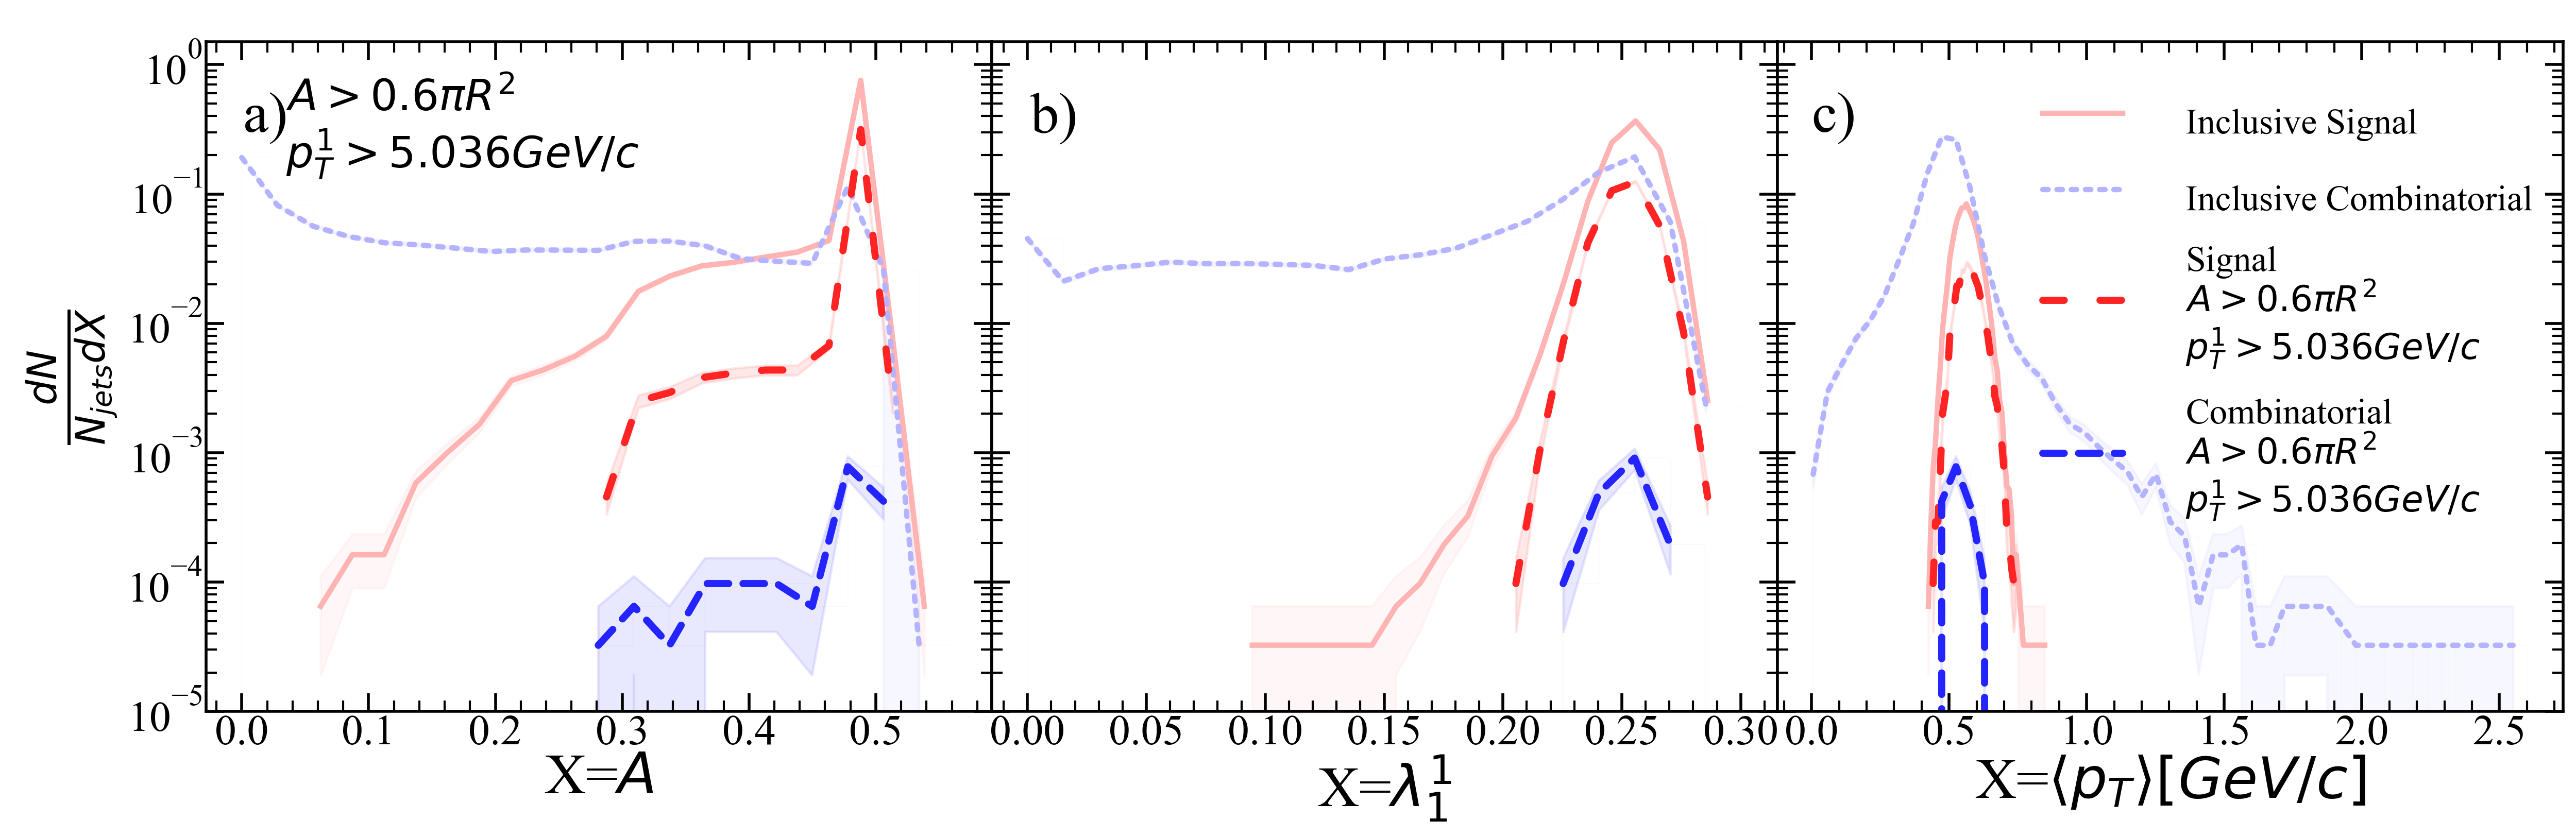}
    \caption{R=0.4 \ptH=10 \GeV}
    \label{fig:ml_04_10}
\end{figure*}

\begin{figure*}
    \centering
    \includegraphics[width=\linewidth]{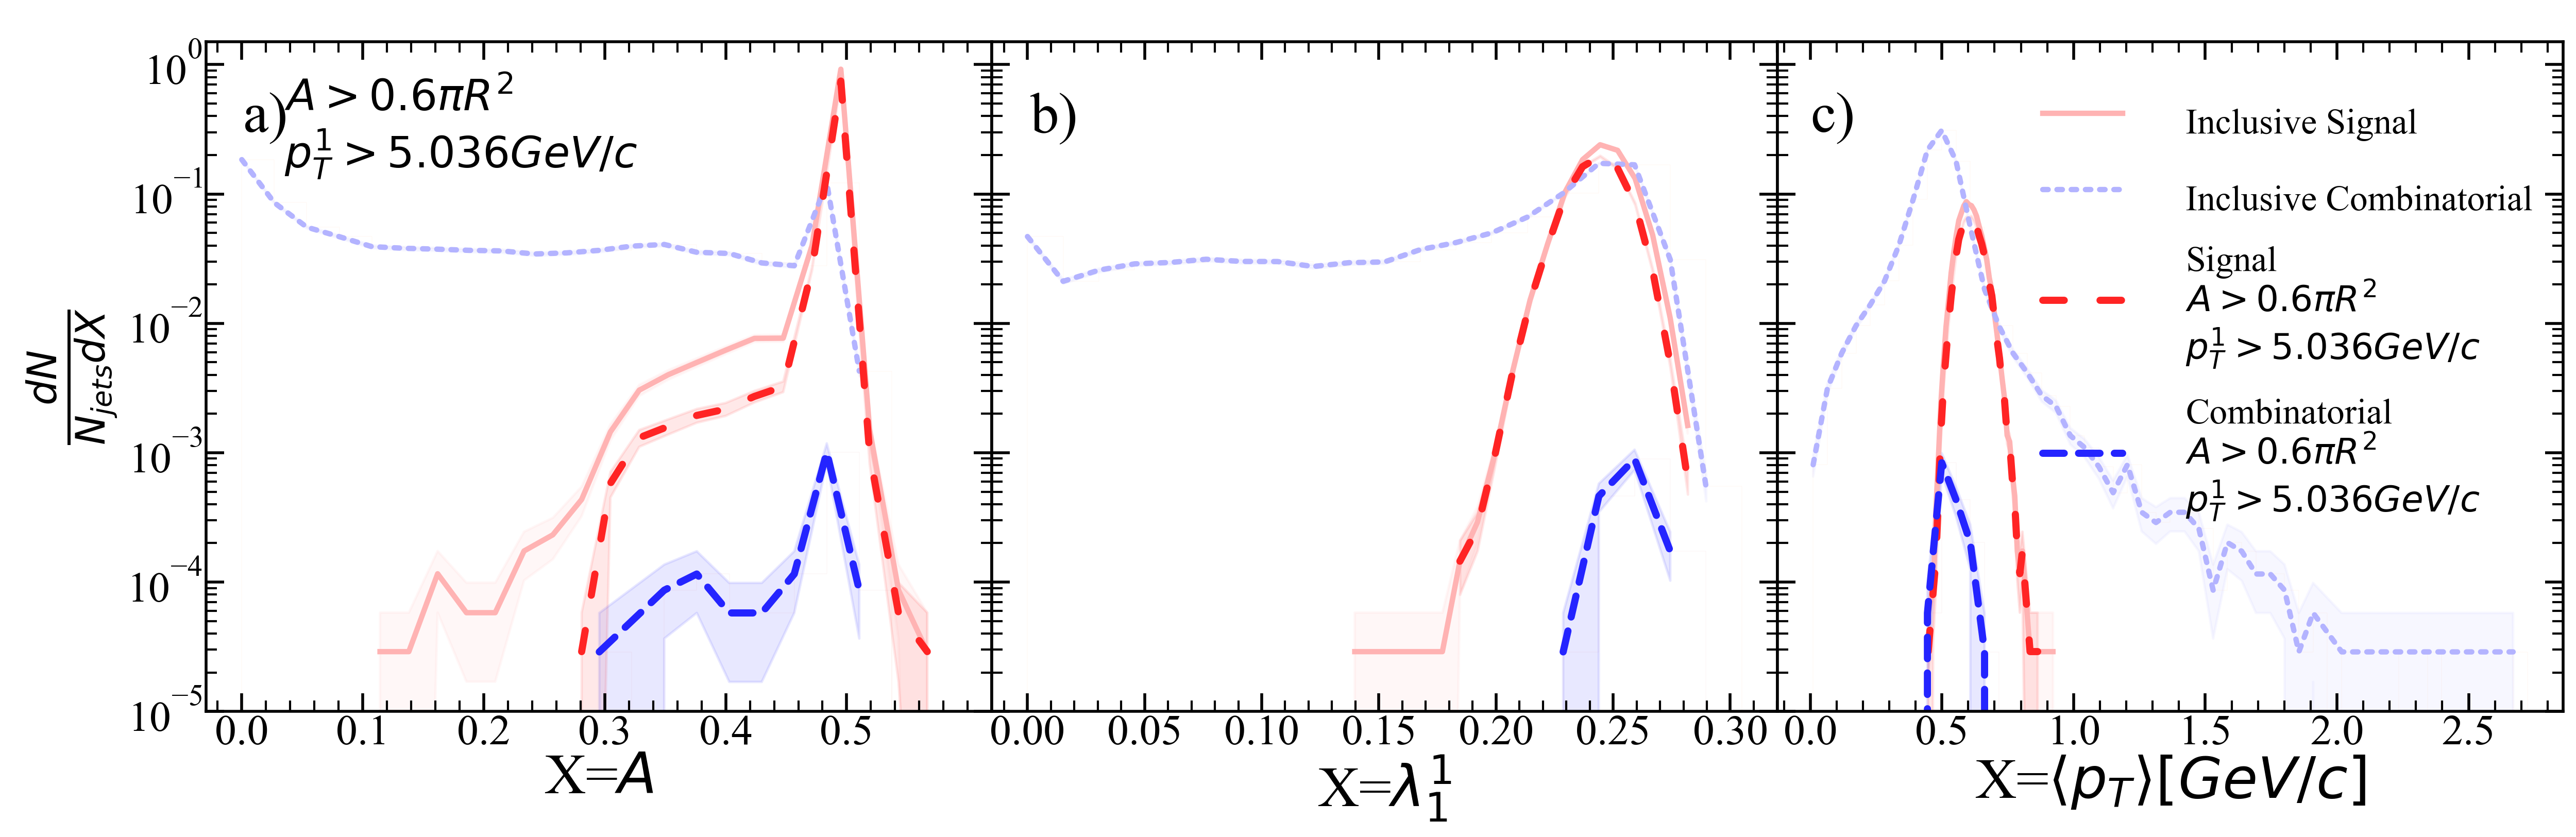}
    \caption{R=0.4 \ptH=20 \GeV}
    \label{fig:ml_04_20}
\end{figure*}

\begin{figure*}
    \centering
    \includegraphics[width=\linewidth]{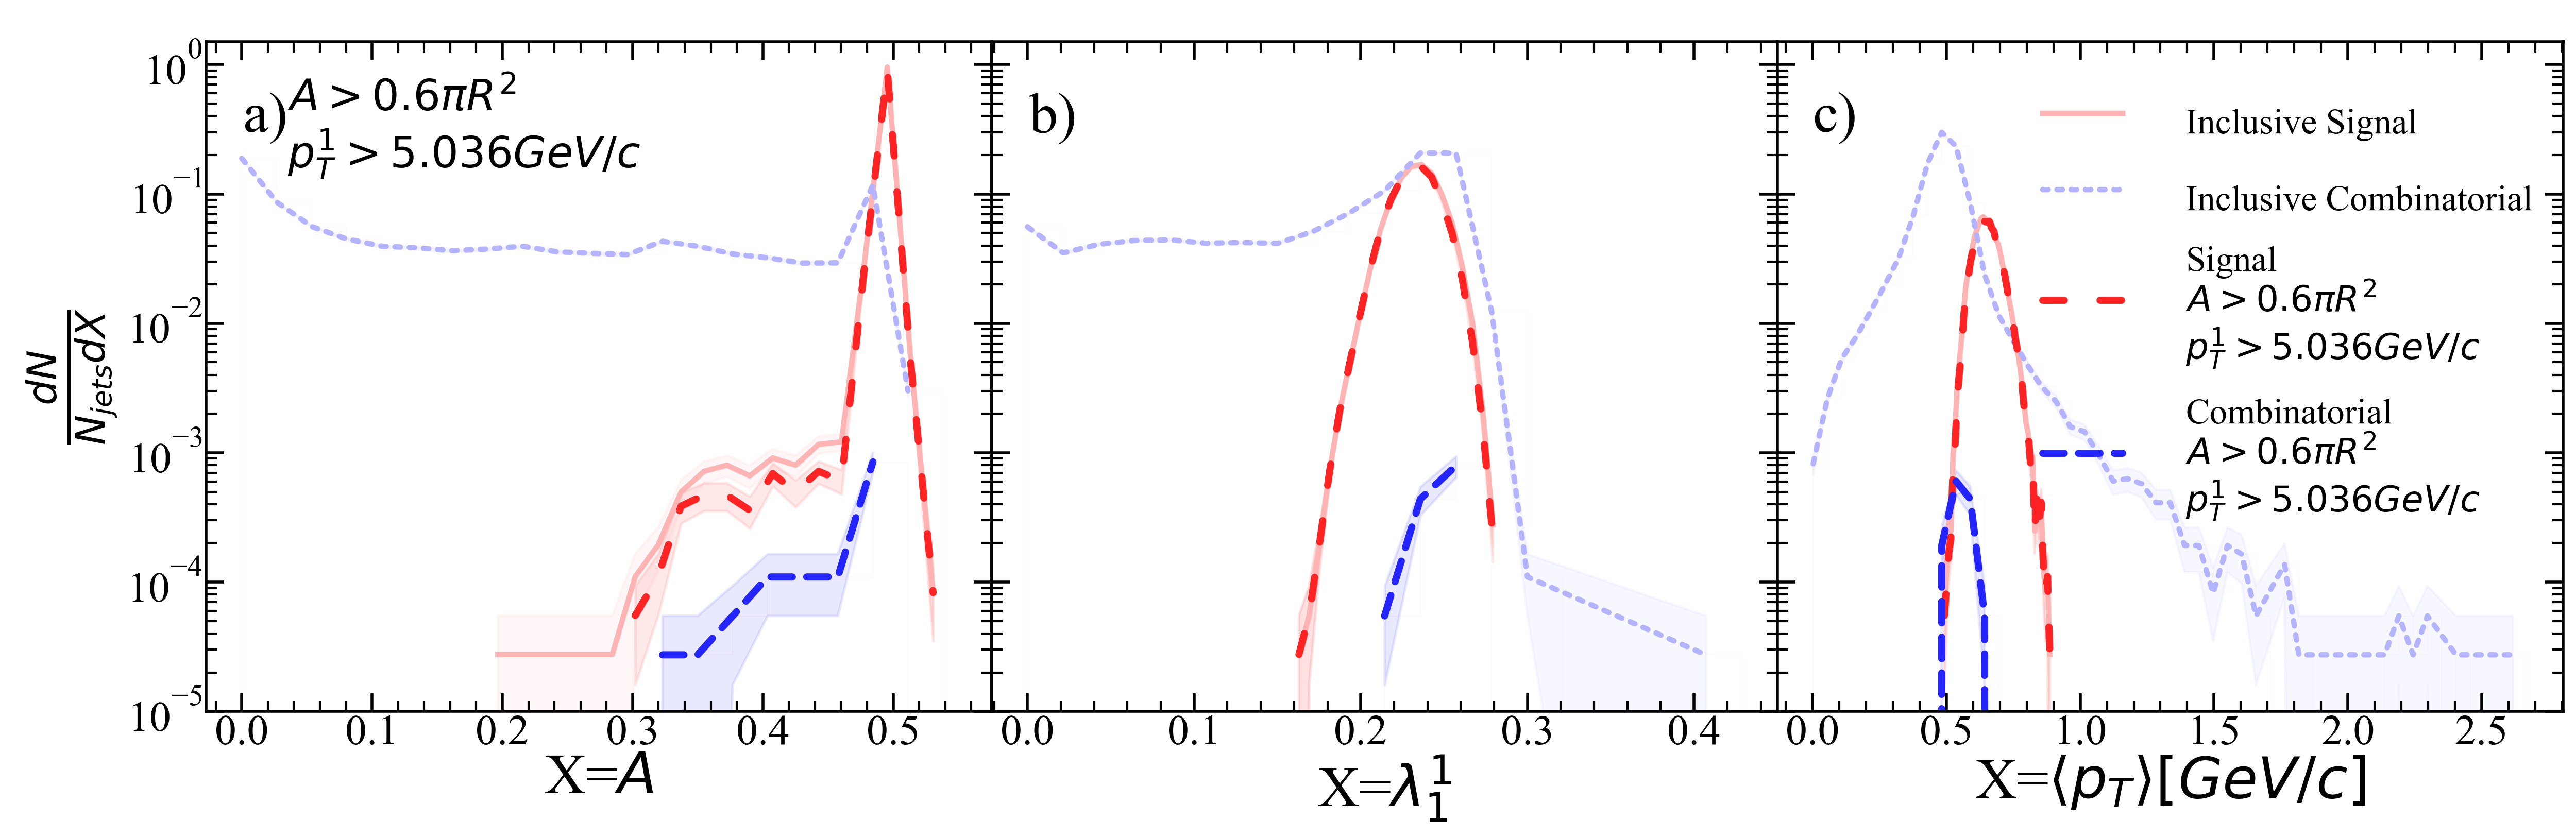}
    \caption{R=0.4 \ptH=30 \GeV}
    \label{fig:ml_04_30}
\end{figure*}

\begin{figure*}
    \centering
    \includegraphics[width=\linewidth]{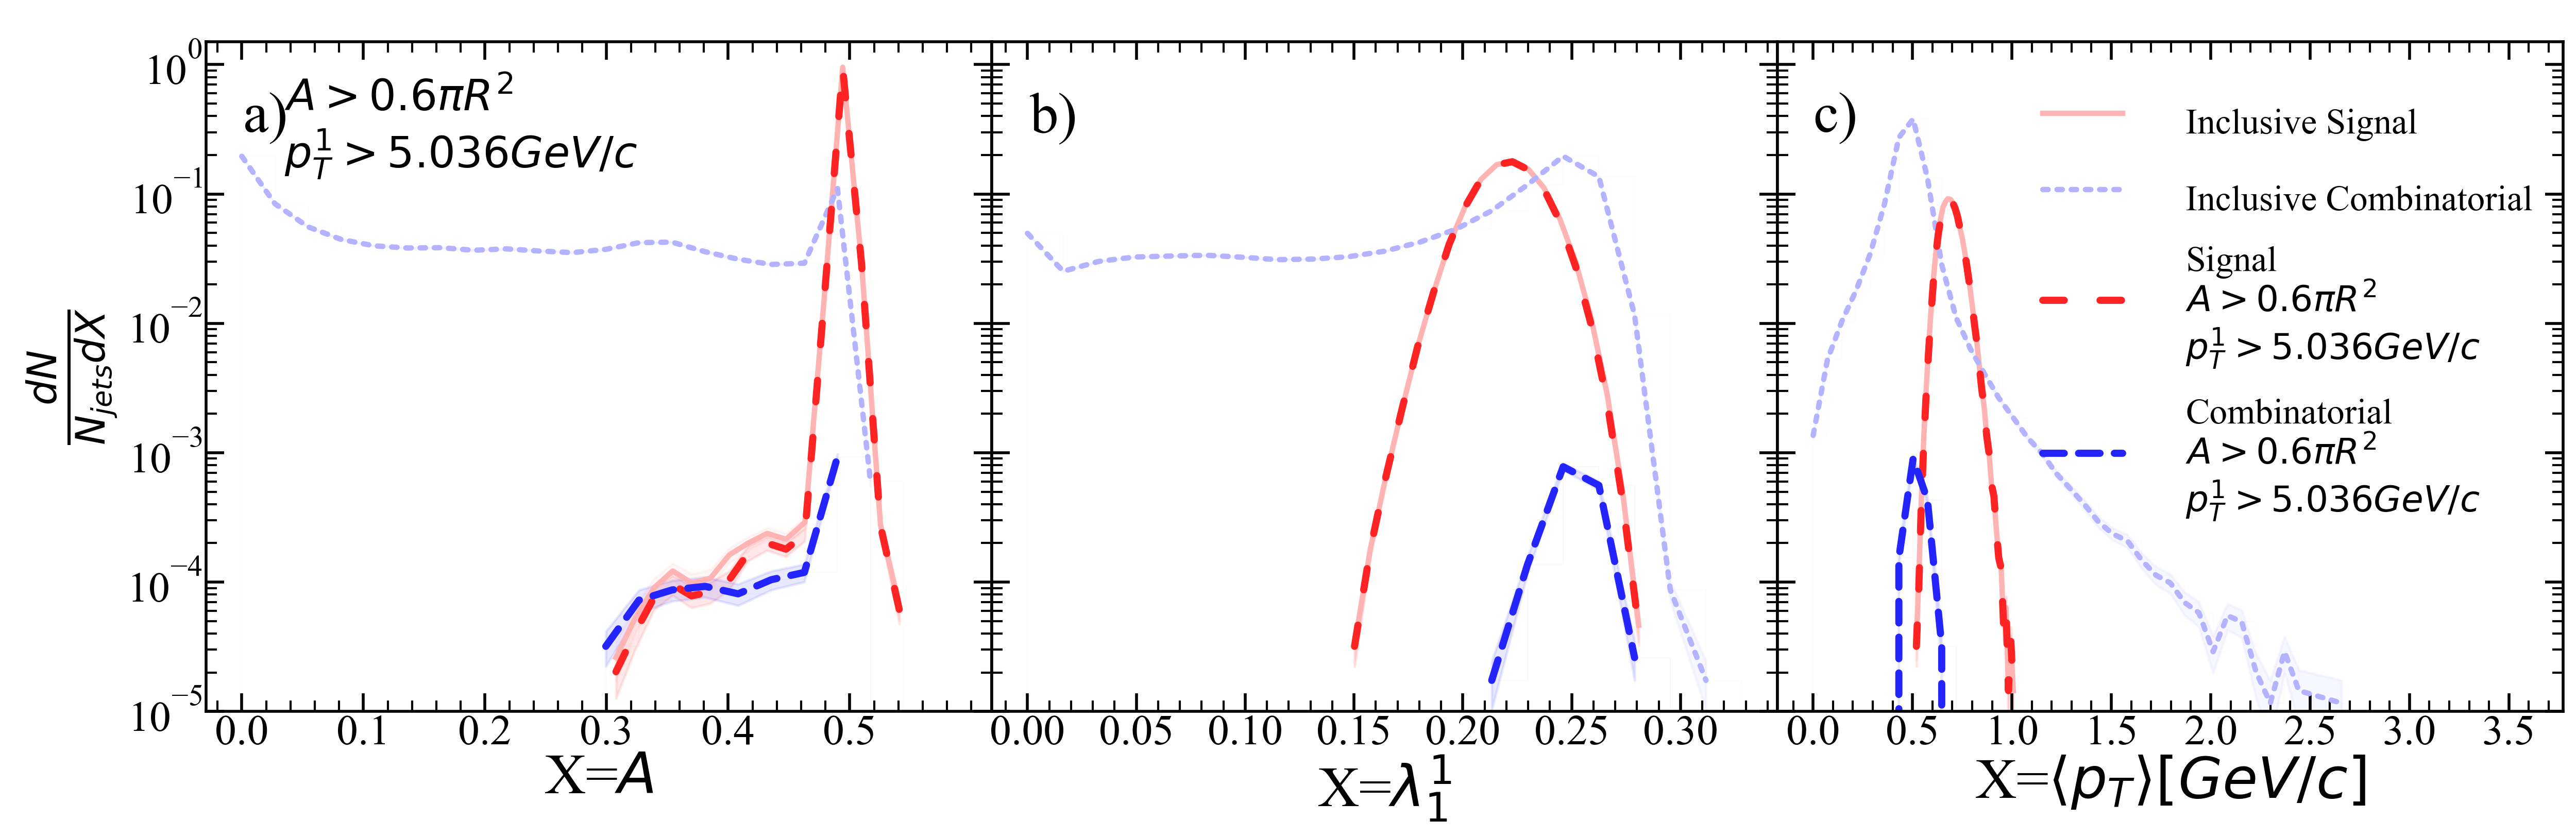}
    \caption{R=0.4 \ptH=40 \GeV}
    \label{fig:ml_04_40}
\end{figure*}

\begin{figure*}
    \centering
    \includegraphics[width=\linewidth]{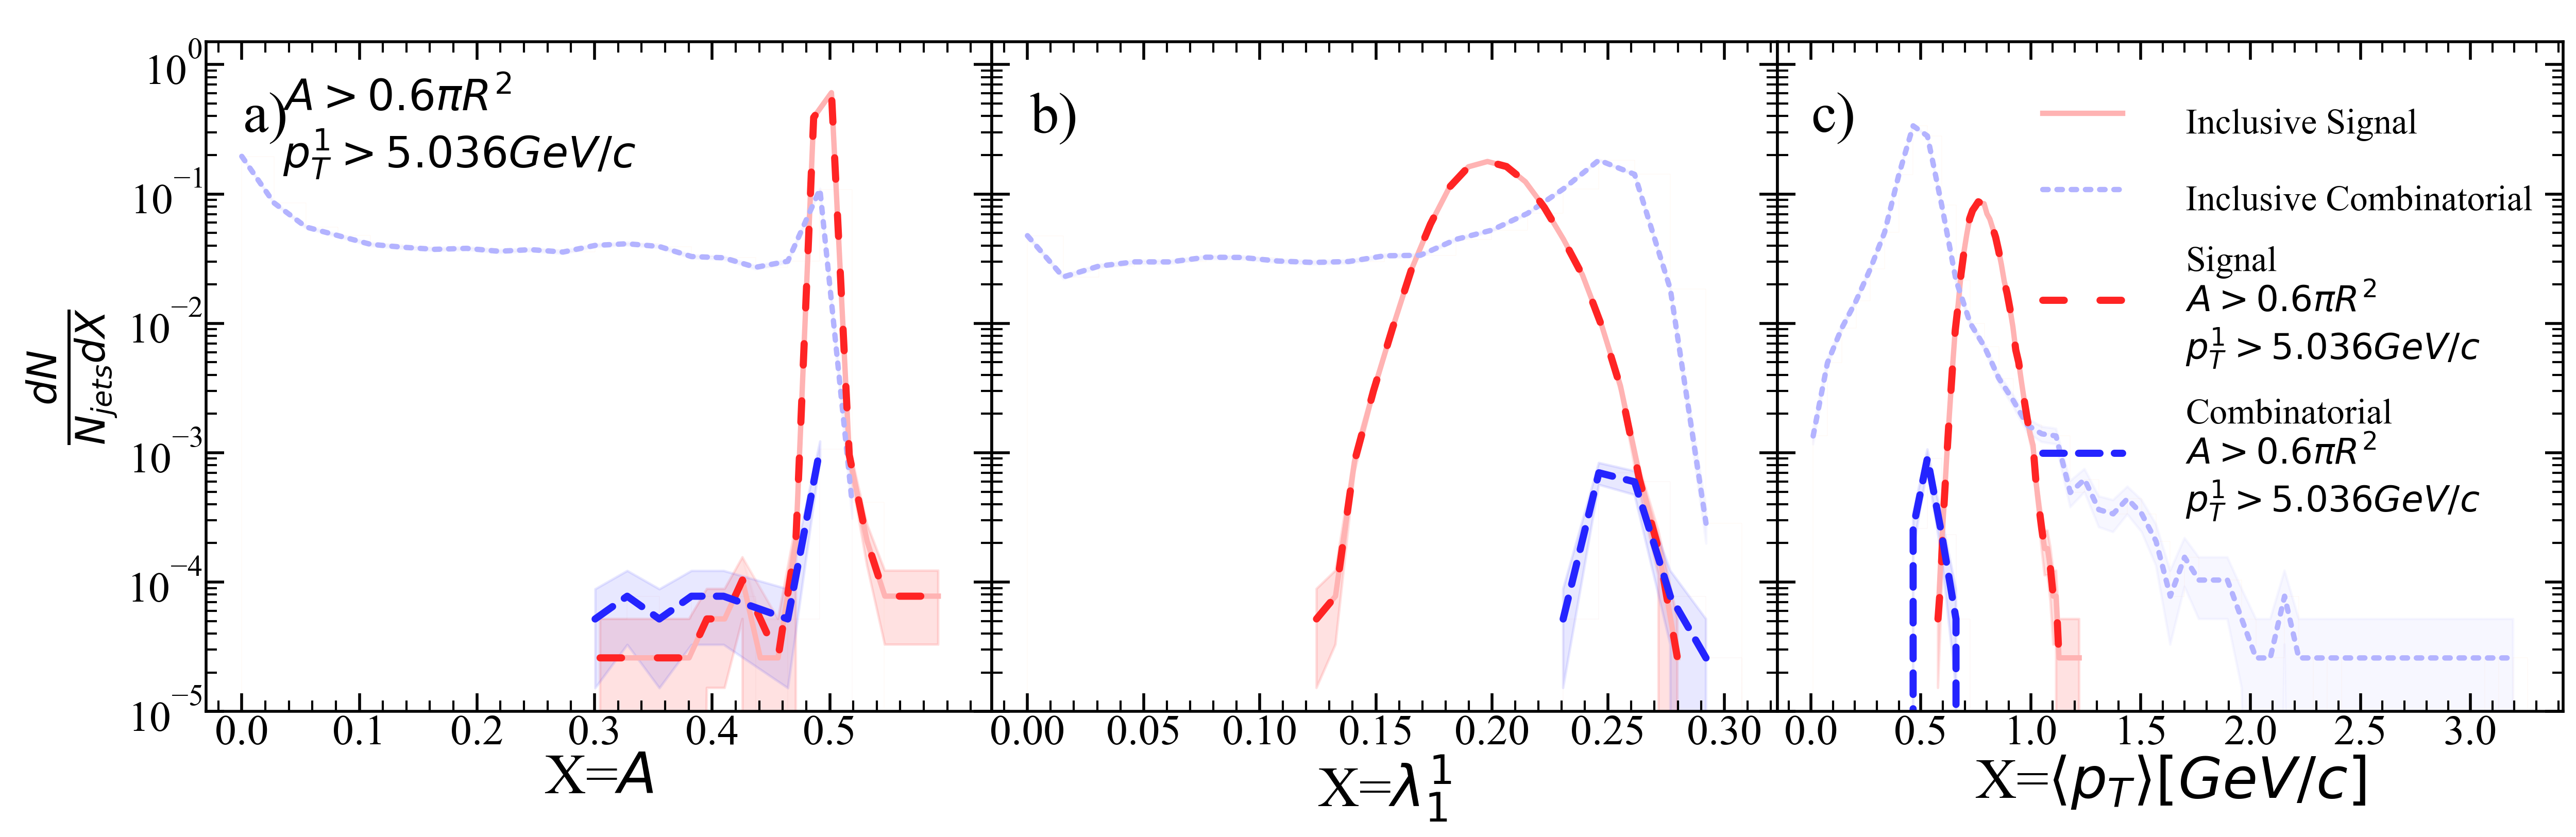}
    \caption{R=0.4 \ptH=60 \GeV}
    \label{fig:ml_04_60}
\end{figure*}

\begin{figure*}
    \centering
    \includegraphics[width=\linewidth]{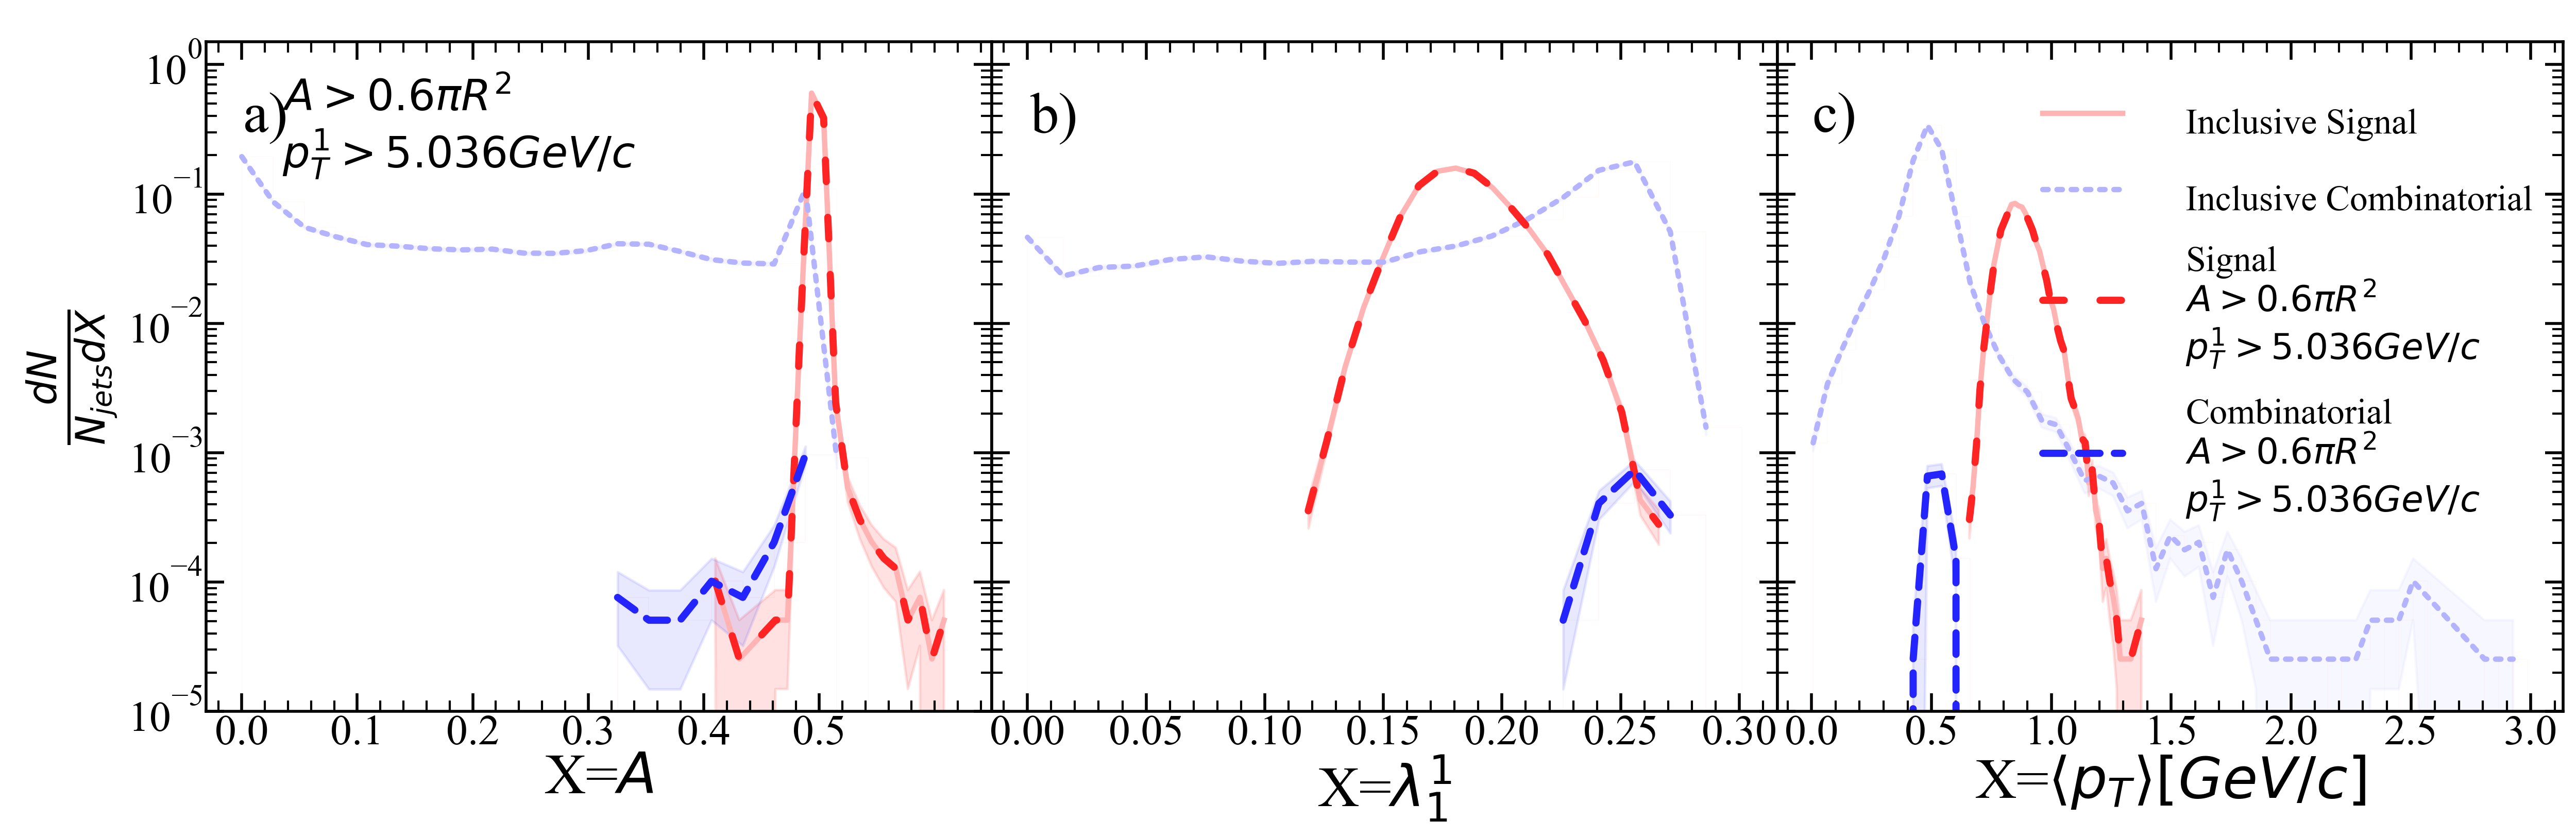}
    \caption{R=0.4 \ptH=80 \GeV}
    \label{fig:ml_04_80}
\end{figure*}

\begin{figure*}
    \centering
    \includegraphics[width=\linewidth]{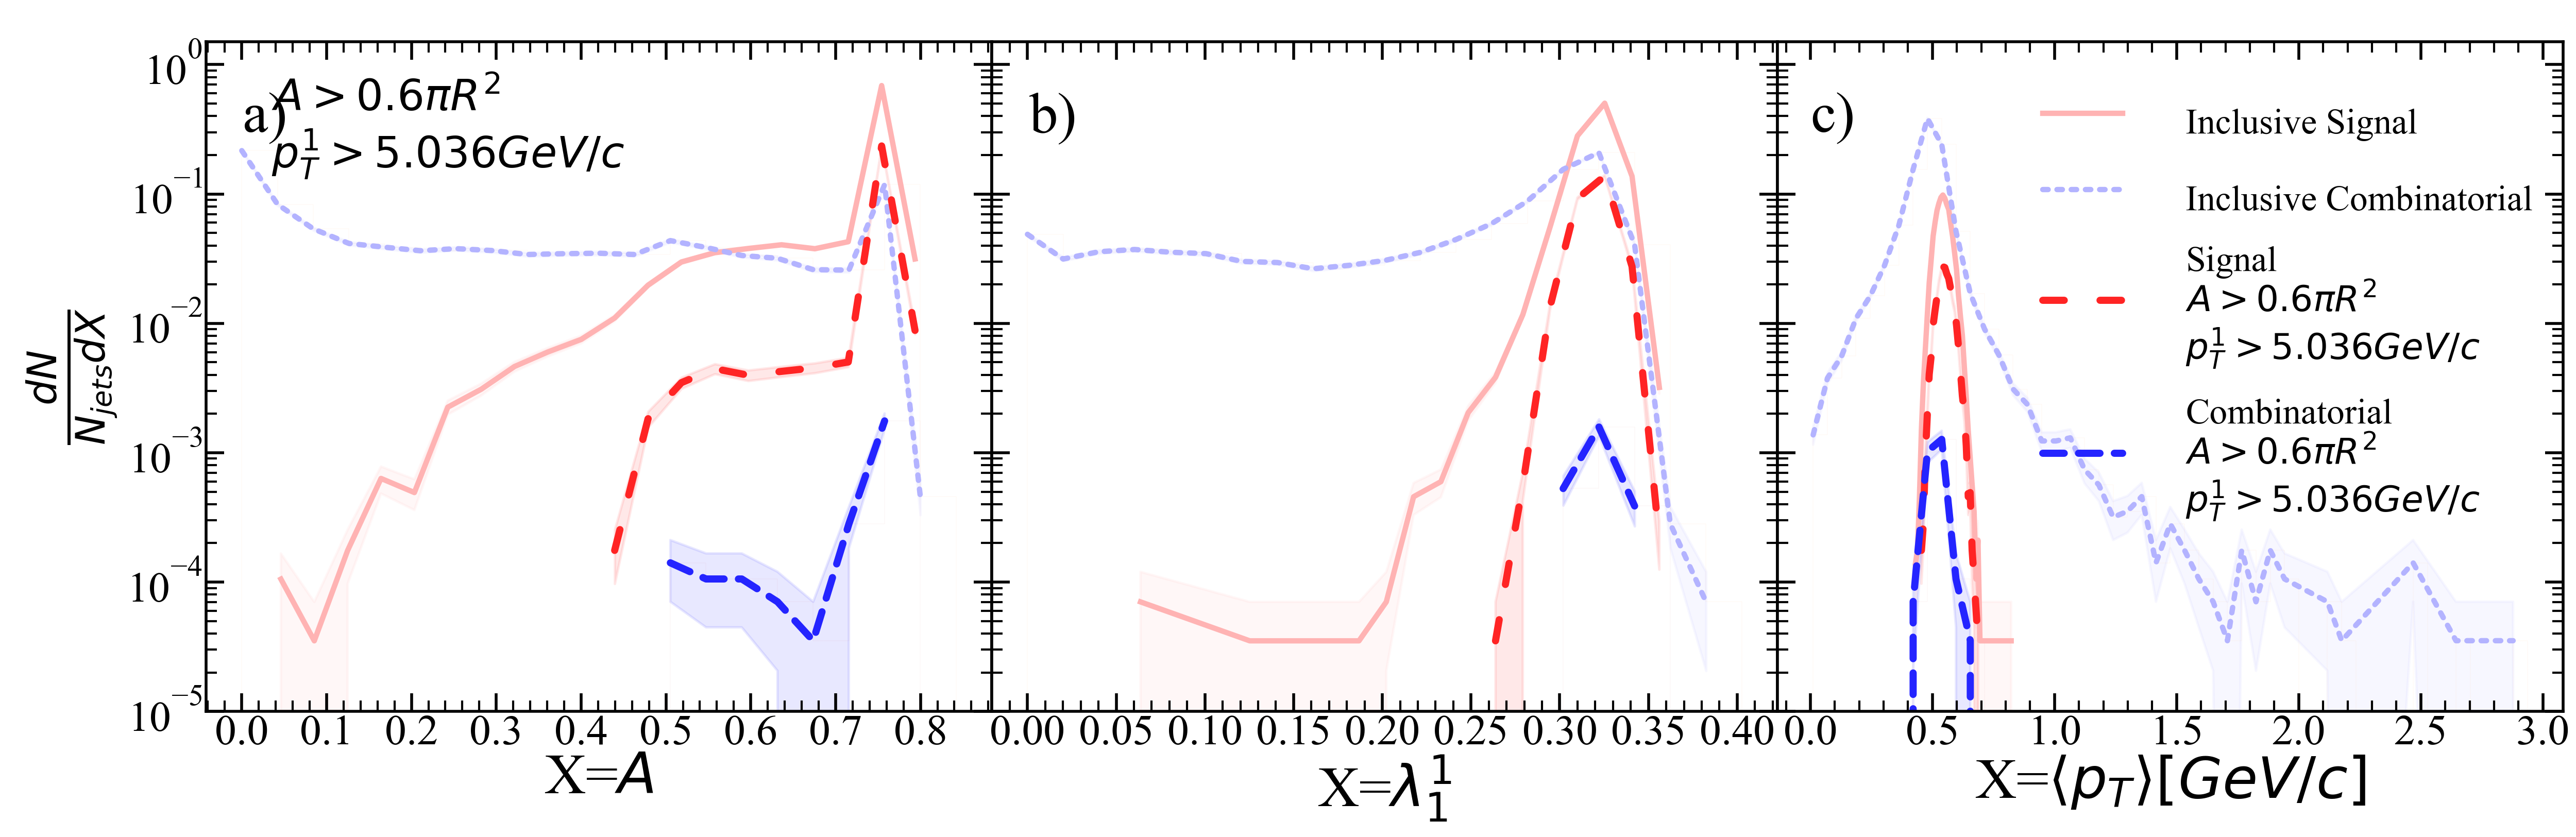}
    \caption{R=0.5 \ptH=10 \GeV}
    \label{fig:ml_05_10}
\end{figure*}

\begin{figure*}
    \centering
    \includegraphics[width=\linewidth]{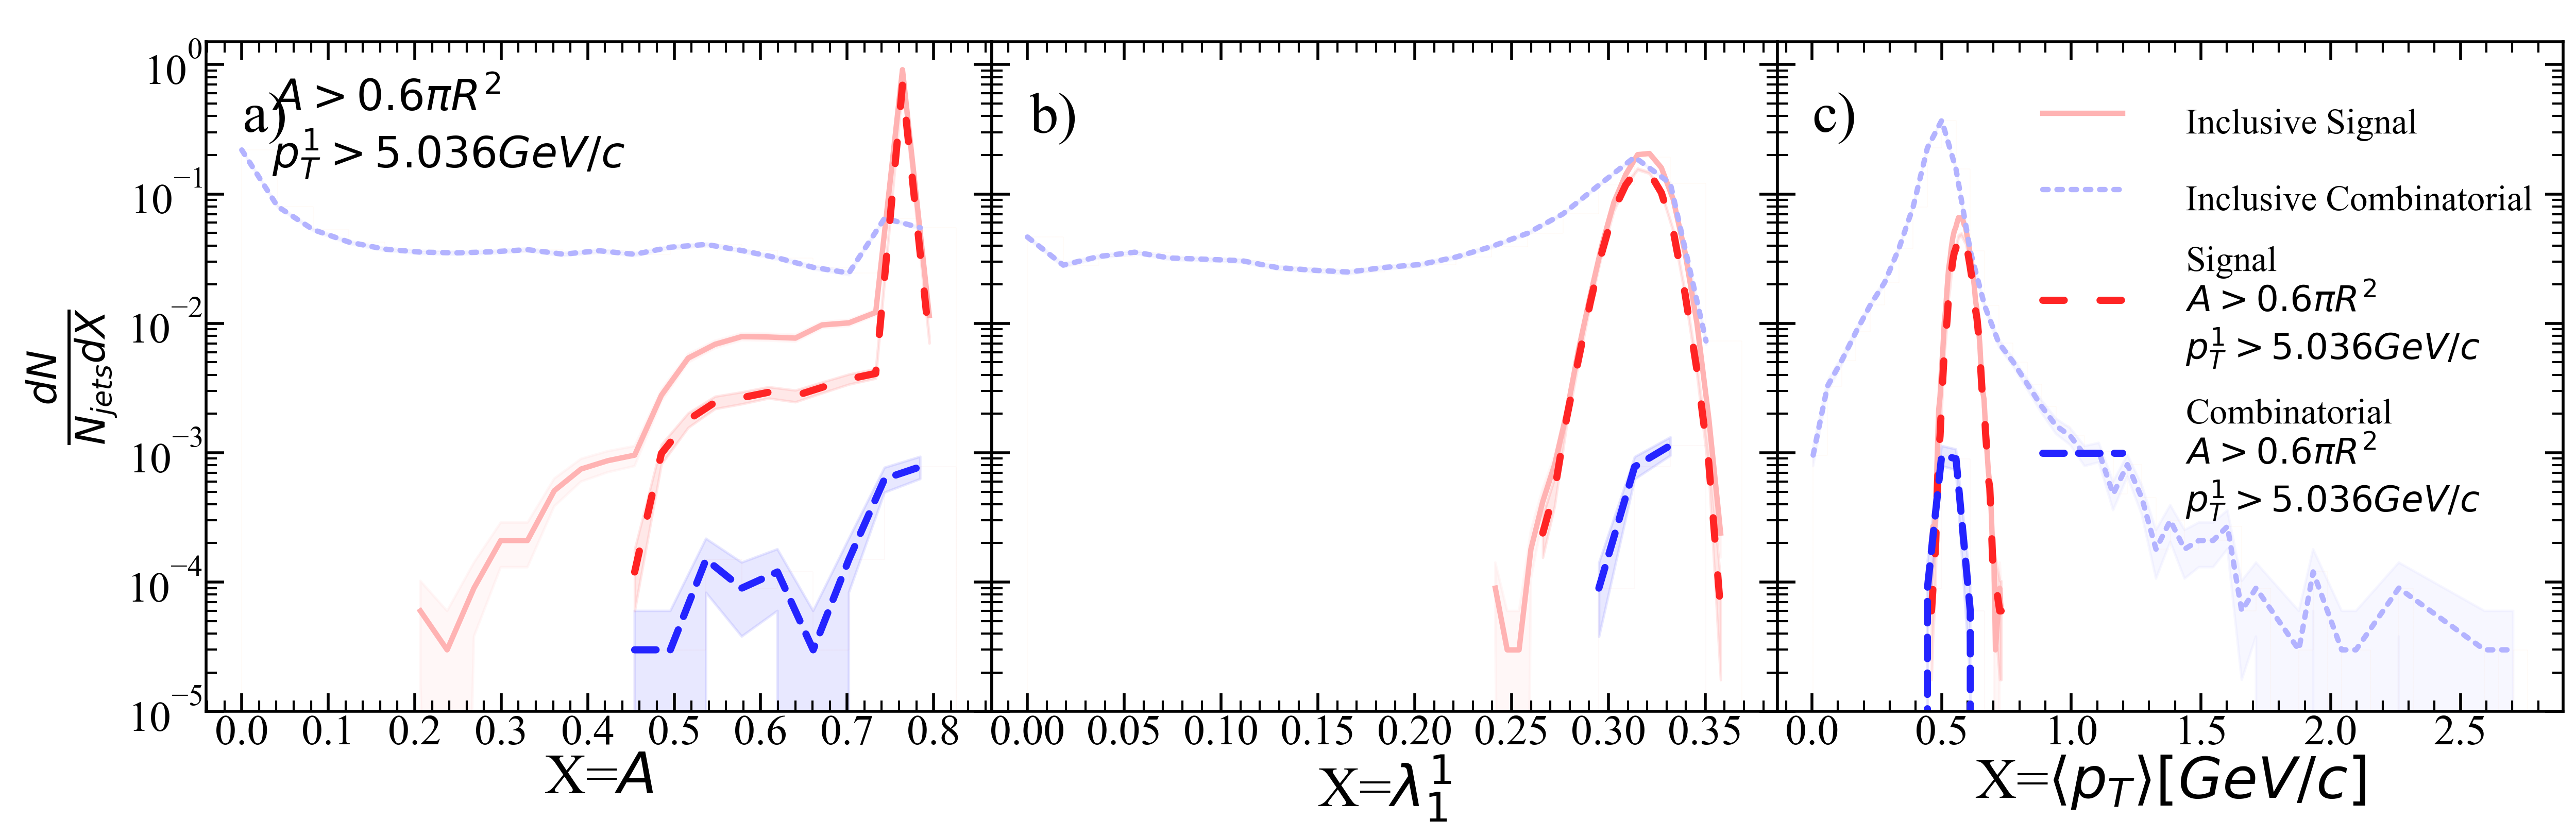}
    \caption{R=0.5 \ptH=20 \GeV}
    \label{fig:ml_05_20}
\end{figure*}

\begin{figure*}
    \centering
    \includegraphics[width=\linewidth]{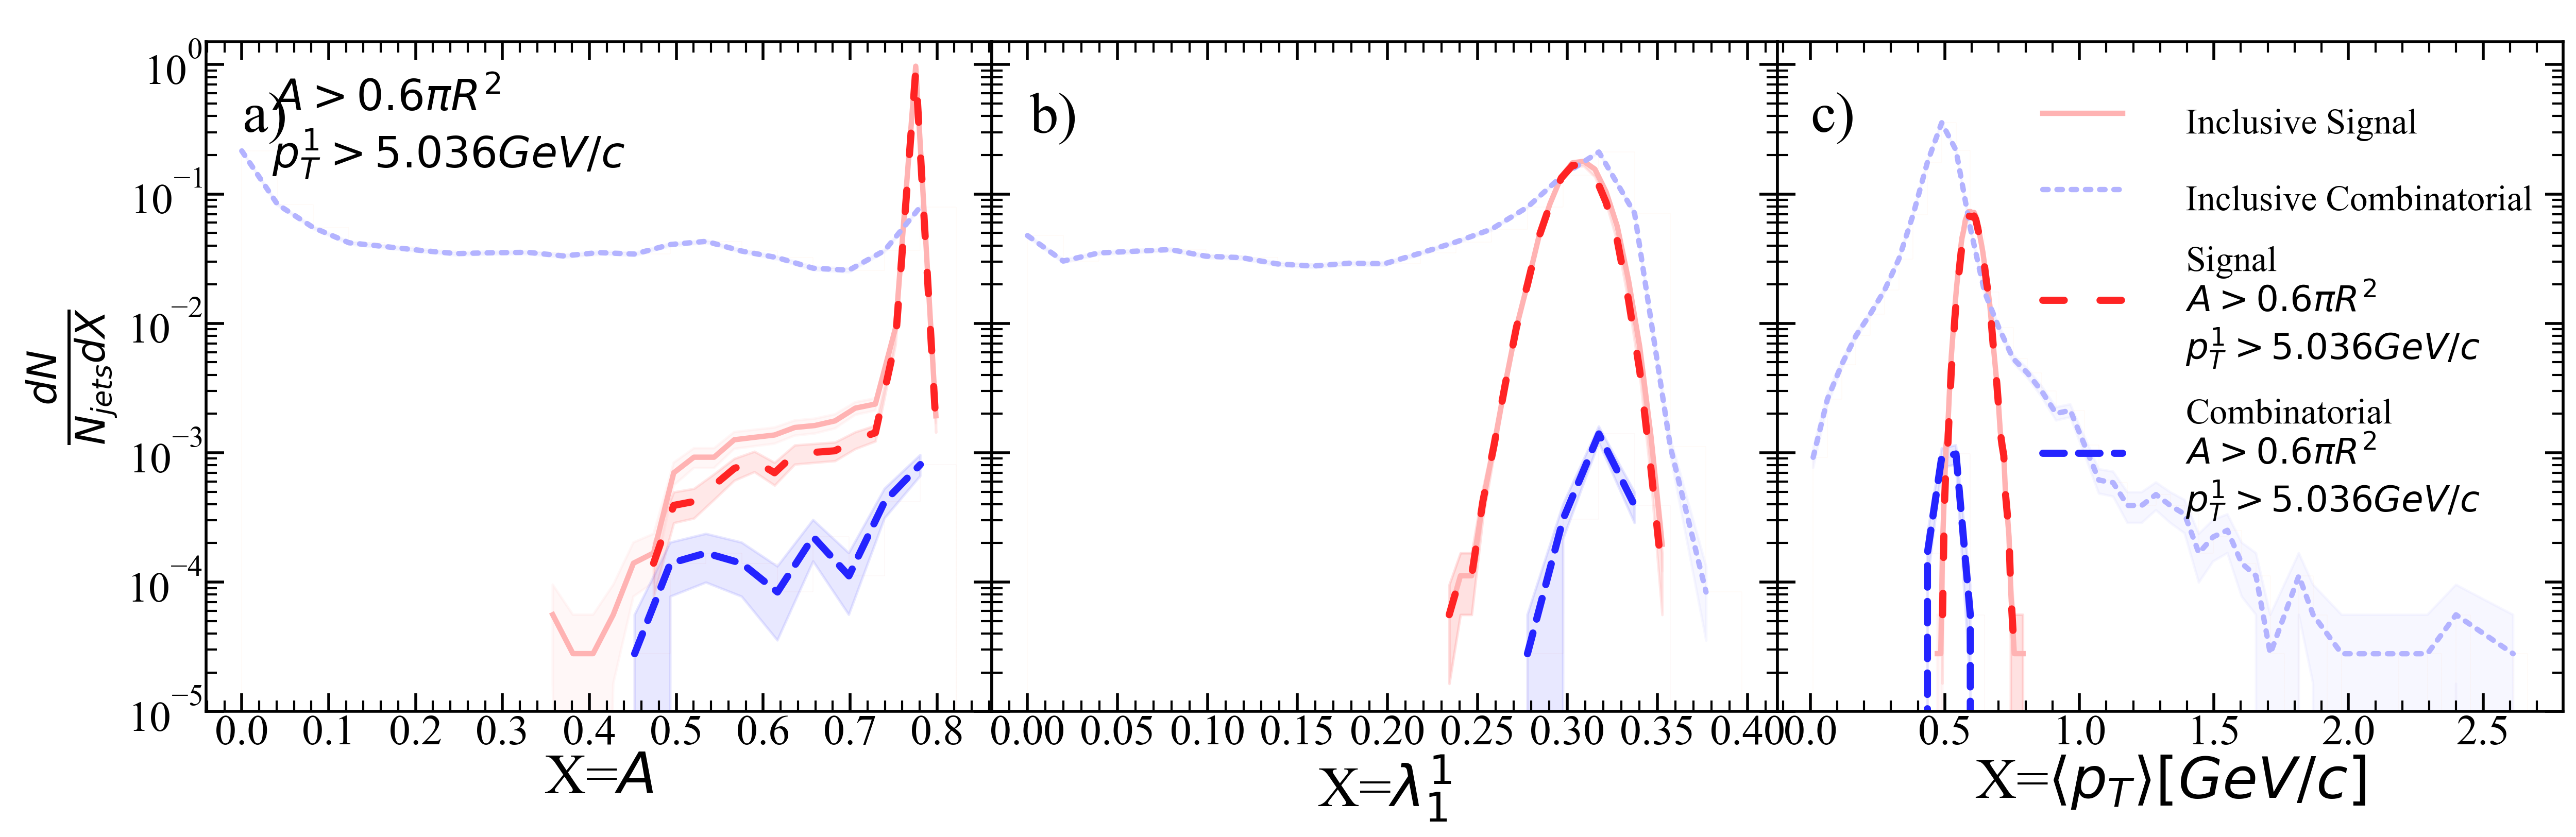}
    \caption{R=0.5 \ptH=30 \GeV}
    \label{fig:ml_05_30}
\end{figure*}

\begin{figure*}
    \centering
    \includegraphics[width=\linewidth]{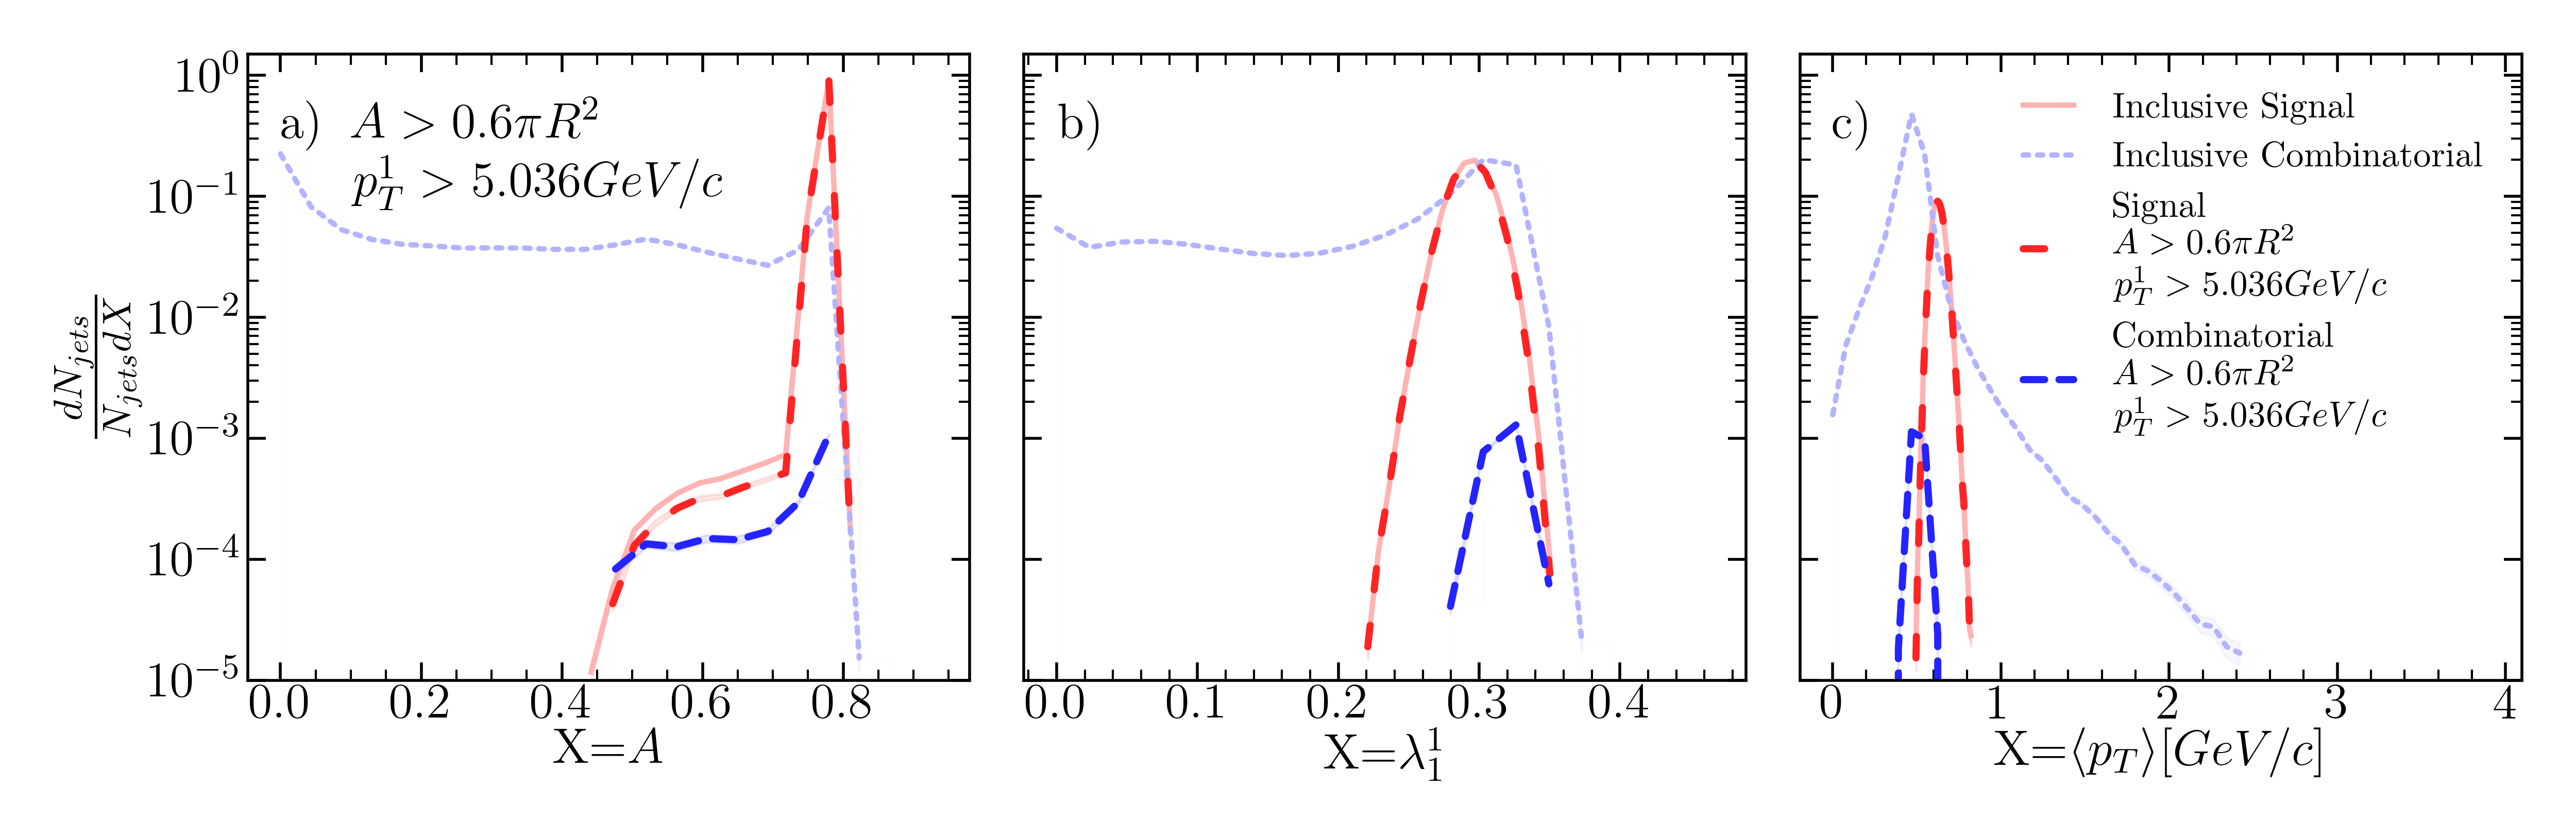}
    \caption{R=0.5 \ptH=40 \GeV}
    \label{fig:ml_05_40}
\end{figure*}

\begin{figure*}
    \centering
    \includegraphics[width=\linewidth]{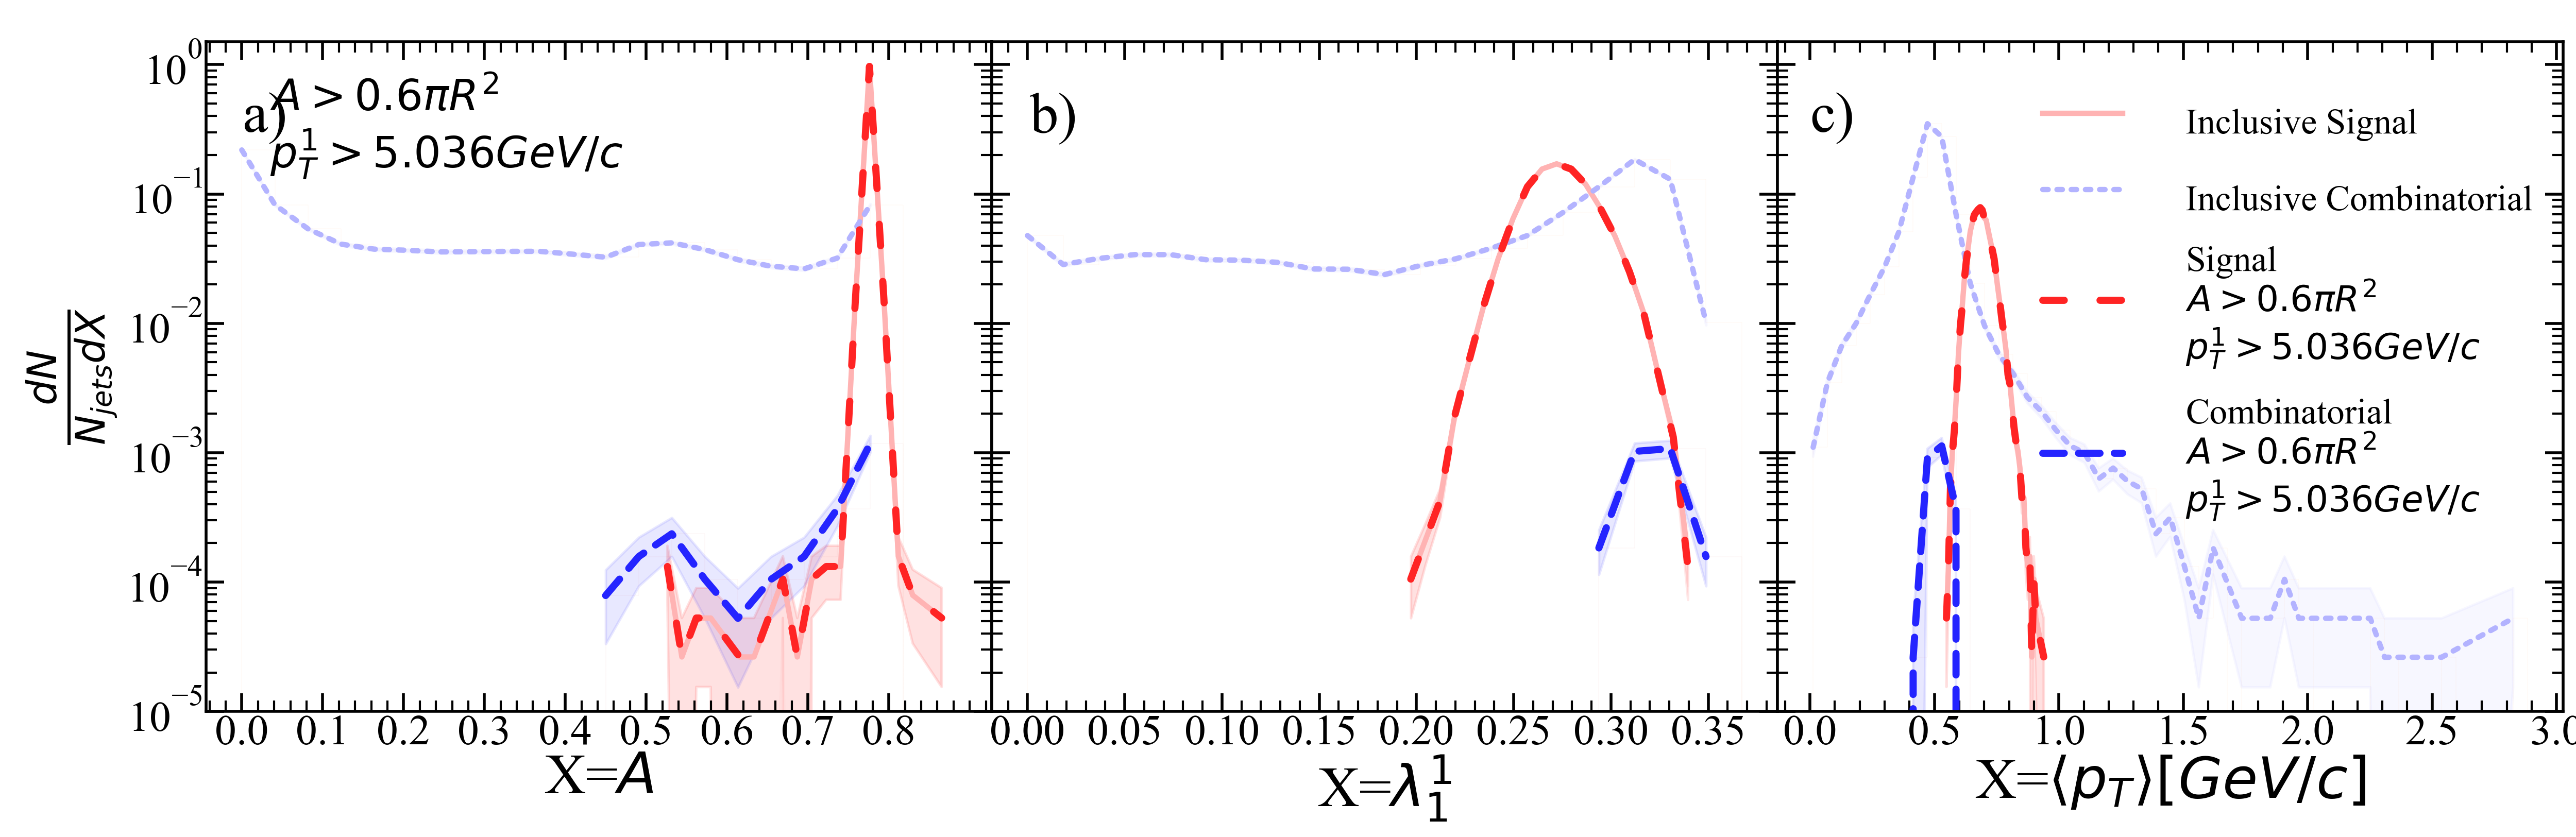}
    \caption{R=0.5 \ptH=60 \GeV}
    \label{fig:ml_05_60}
\end{figure*}

\begin{figure*}
    \centering
    \includegraphics[width=\linewidth]{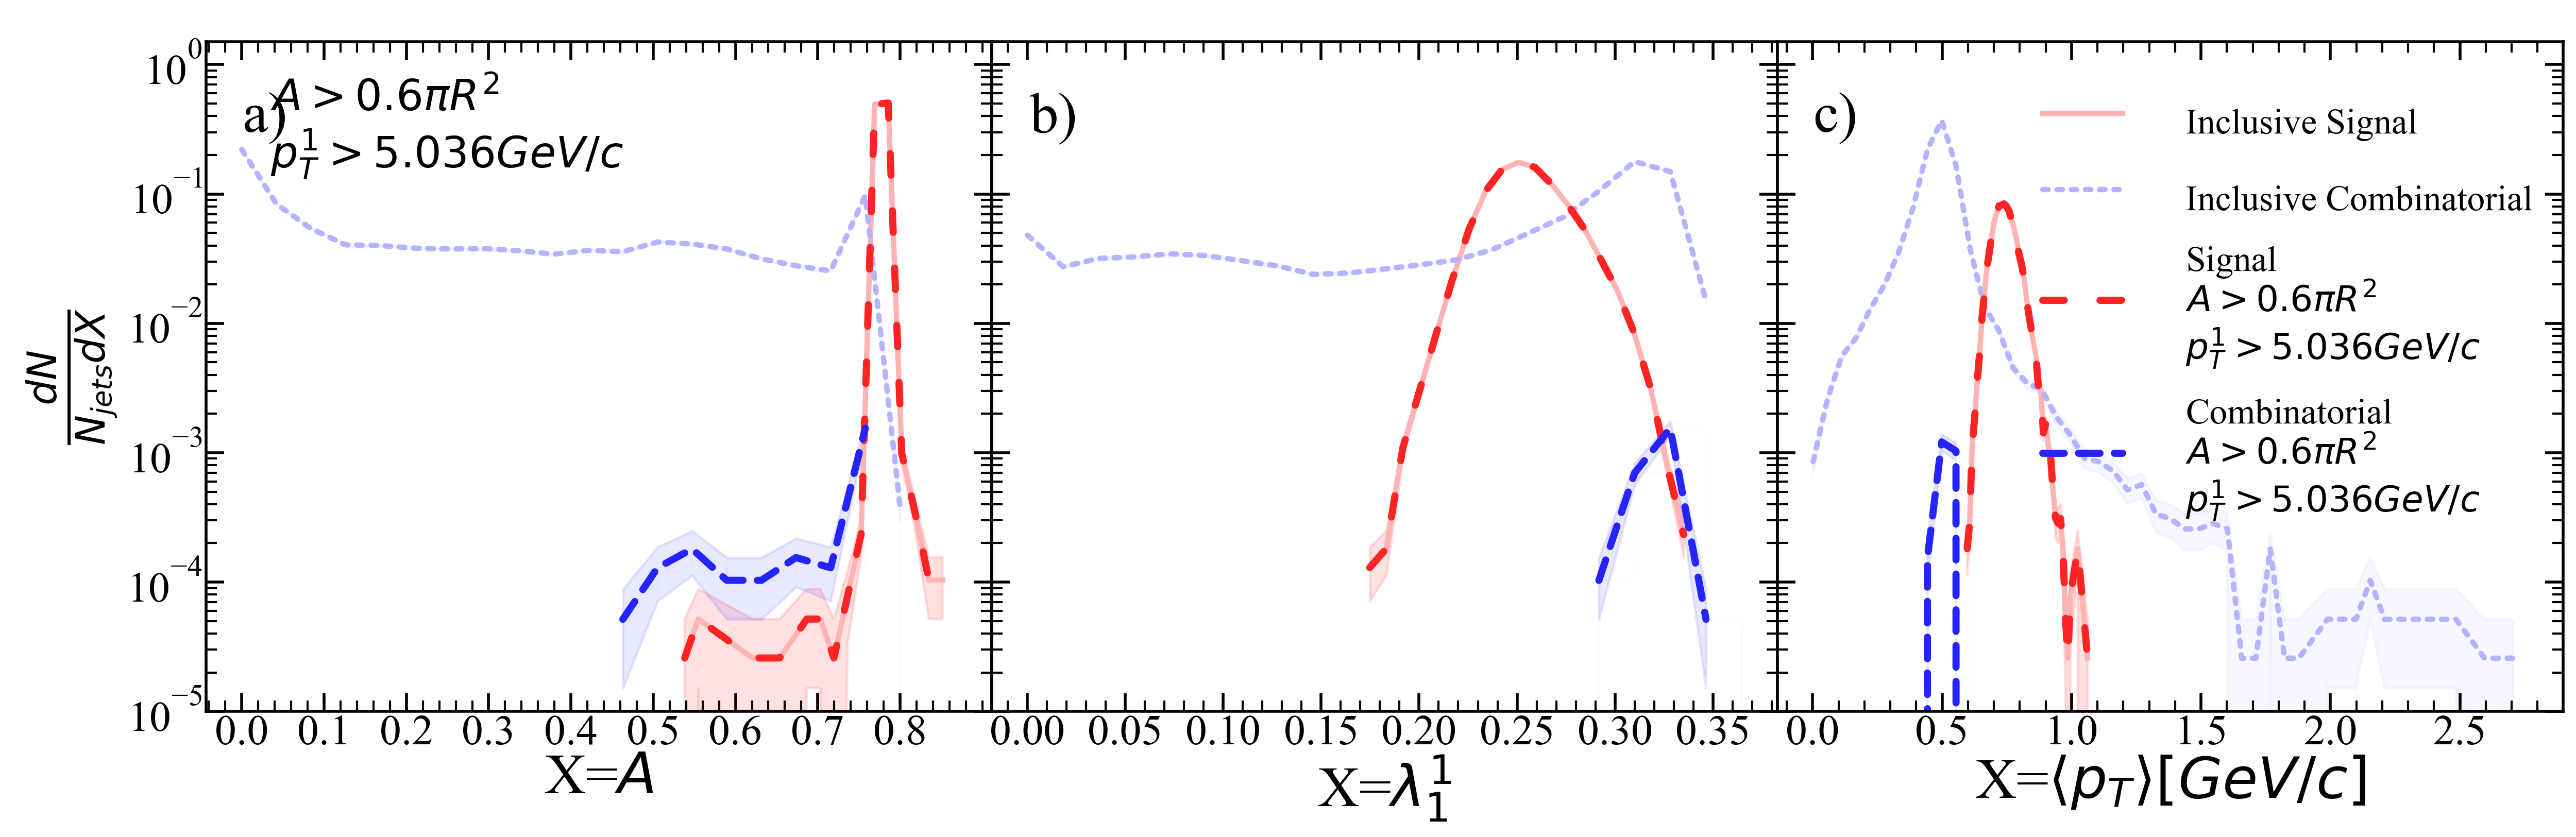}
    \caption{R=0.5 \ptH=80 \GeV}
    \label{fig:ml_05_80}
\end{figure*}

\begin{figure*}
    \centering
    \includegraphics[width=\linewidth]{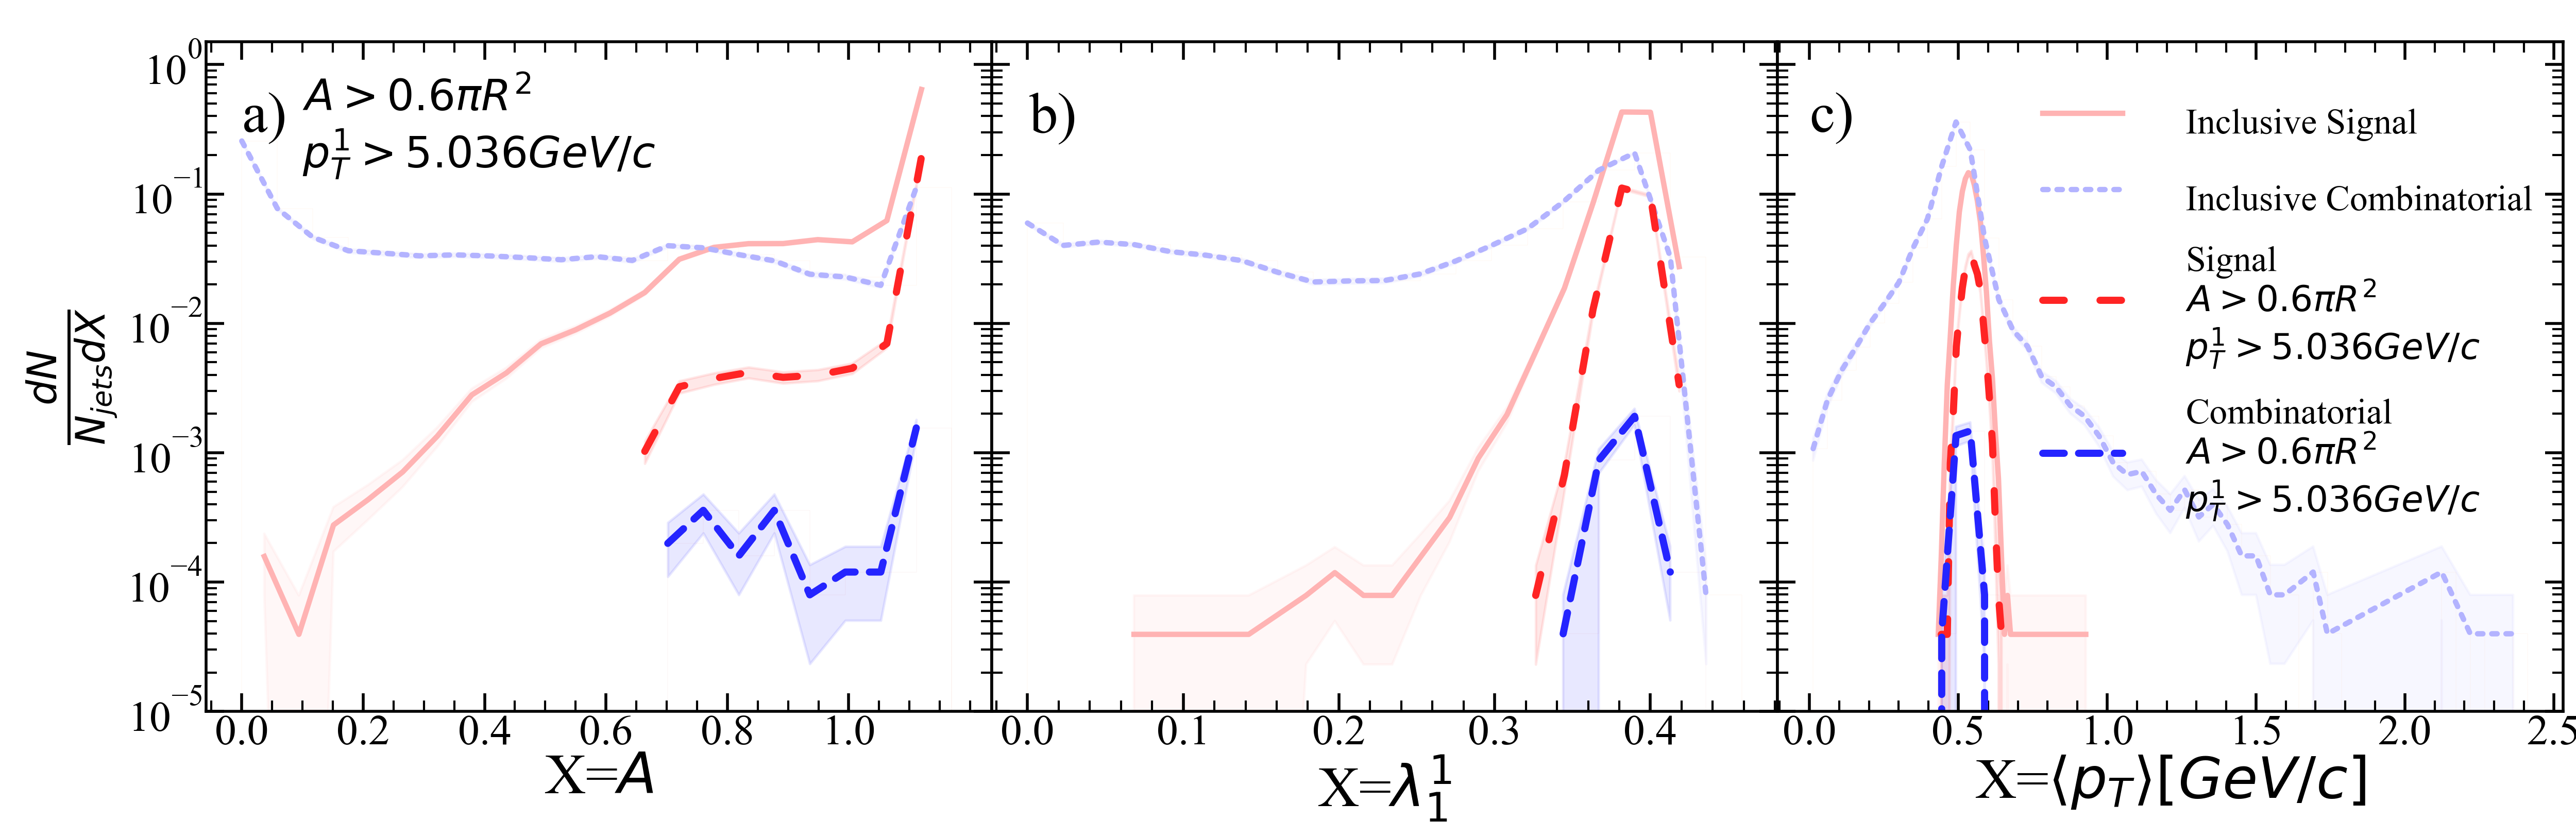}
    \caption{R=0.6 \ptH=10 \GeV}
    \label{fig:ml_06_10}
\end{figure*}

\begin{figure*}
    \centering
    \includegraphics[width=\linewidth]{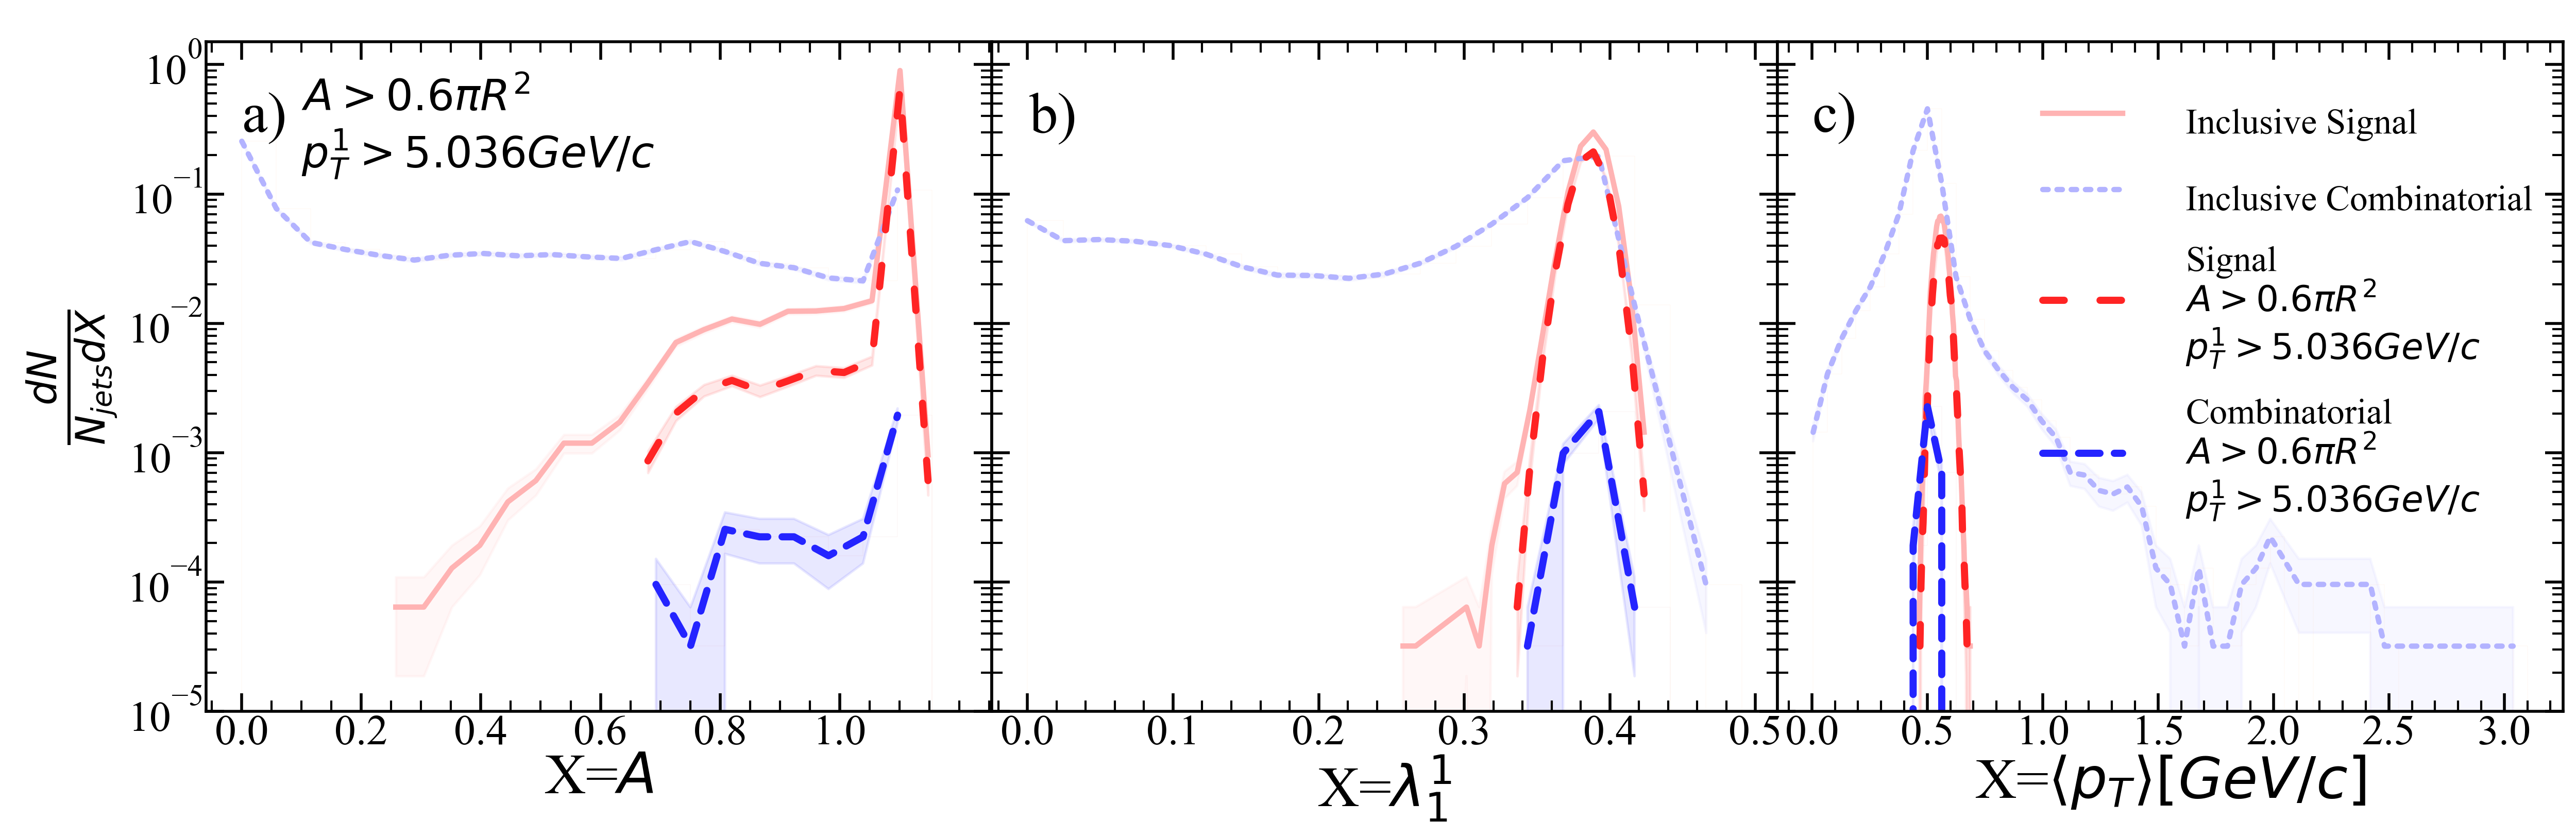}
    \caption{R=0.6 \ptH=20 \GeV}
    \label{fig:ml_06_20}
\end{figure*}

\begin{figure*}
    \centering
    \includegraphics[width=\linewidth]{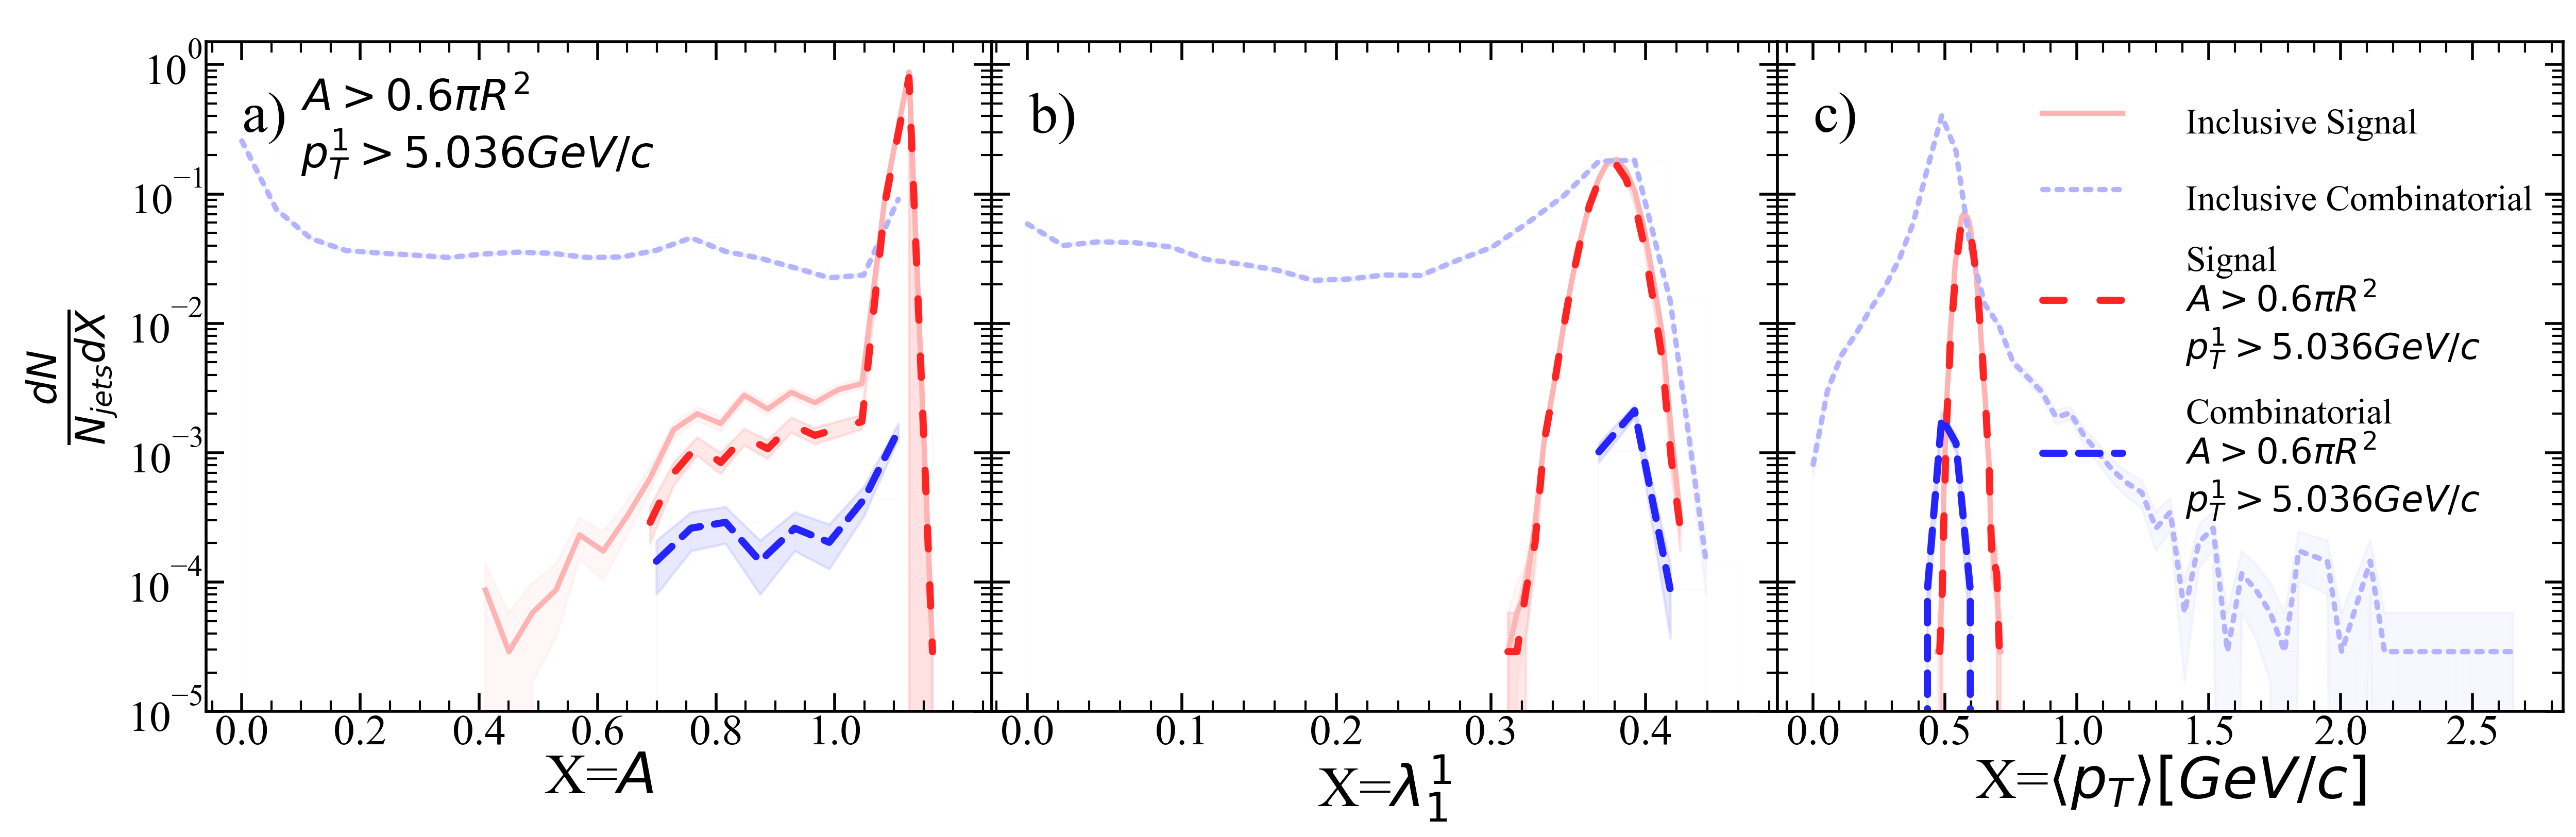}
    \caption{R=0.6 \ptH=30 \GeV}
    \label{fig:ml_06_30}
\end{figure*}

\begin{figure*}
    \centering
    \includegraphics[width=\linewidth]{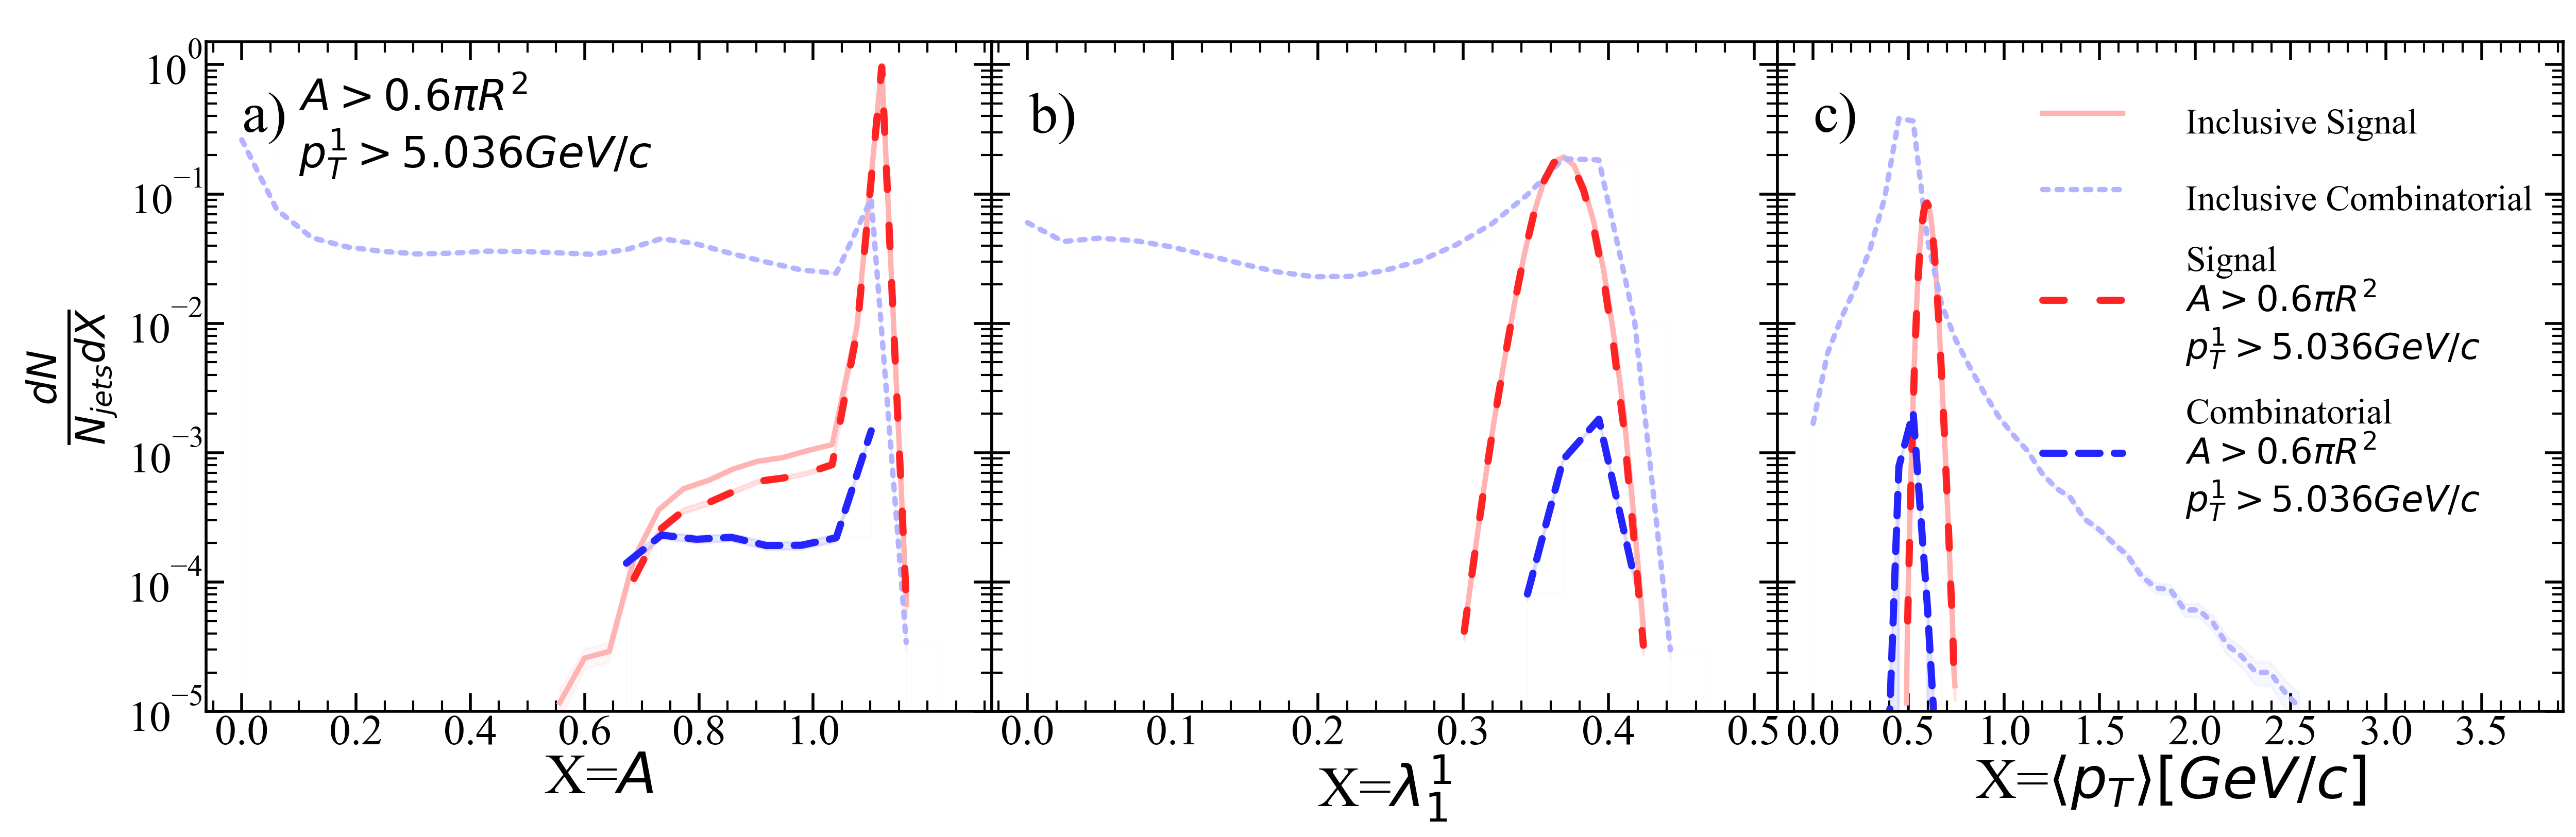}
    \caption{R=0.6 \ptH=40 \GeV}
    \label{fig:ml_06_40}
\end{figure*}

\begin{figure*}
    \centering
    \includegraphics[width=\linewidth]{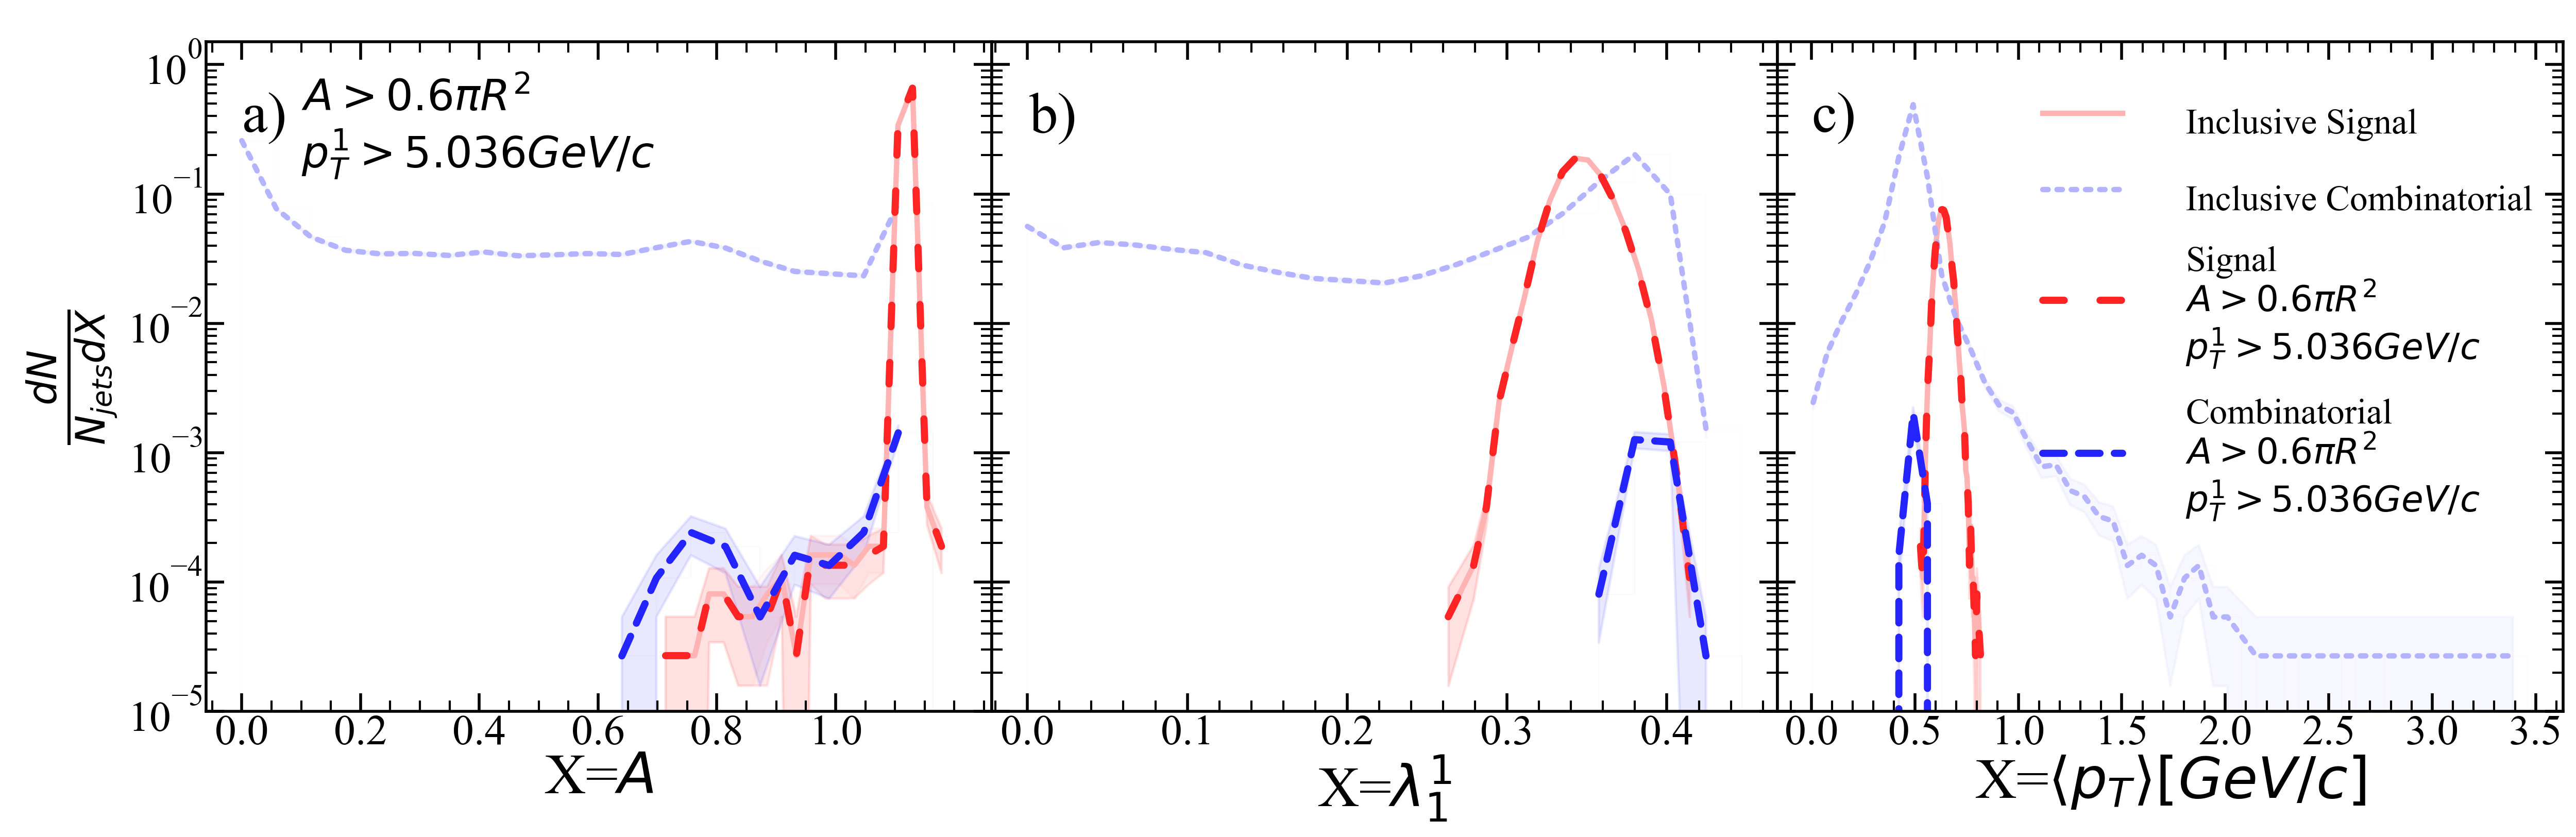}
    \caption{R=0.6 \ptH=60 \GeV}
    \label{fig:ml_06_60}
\end{figure*}

\begin{figure*}
    \centering
    \includegraphics[width=\linewidth]{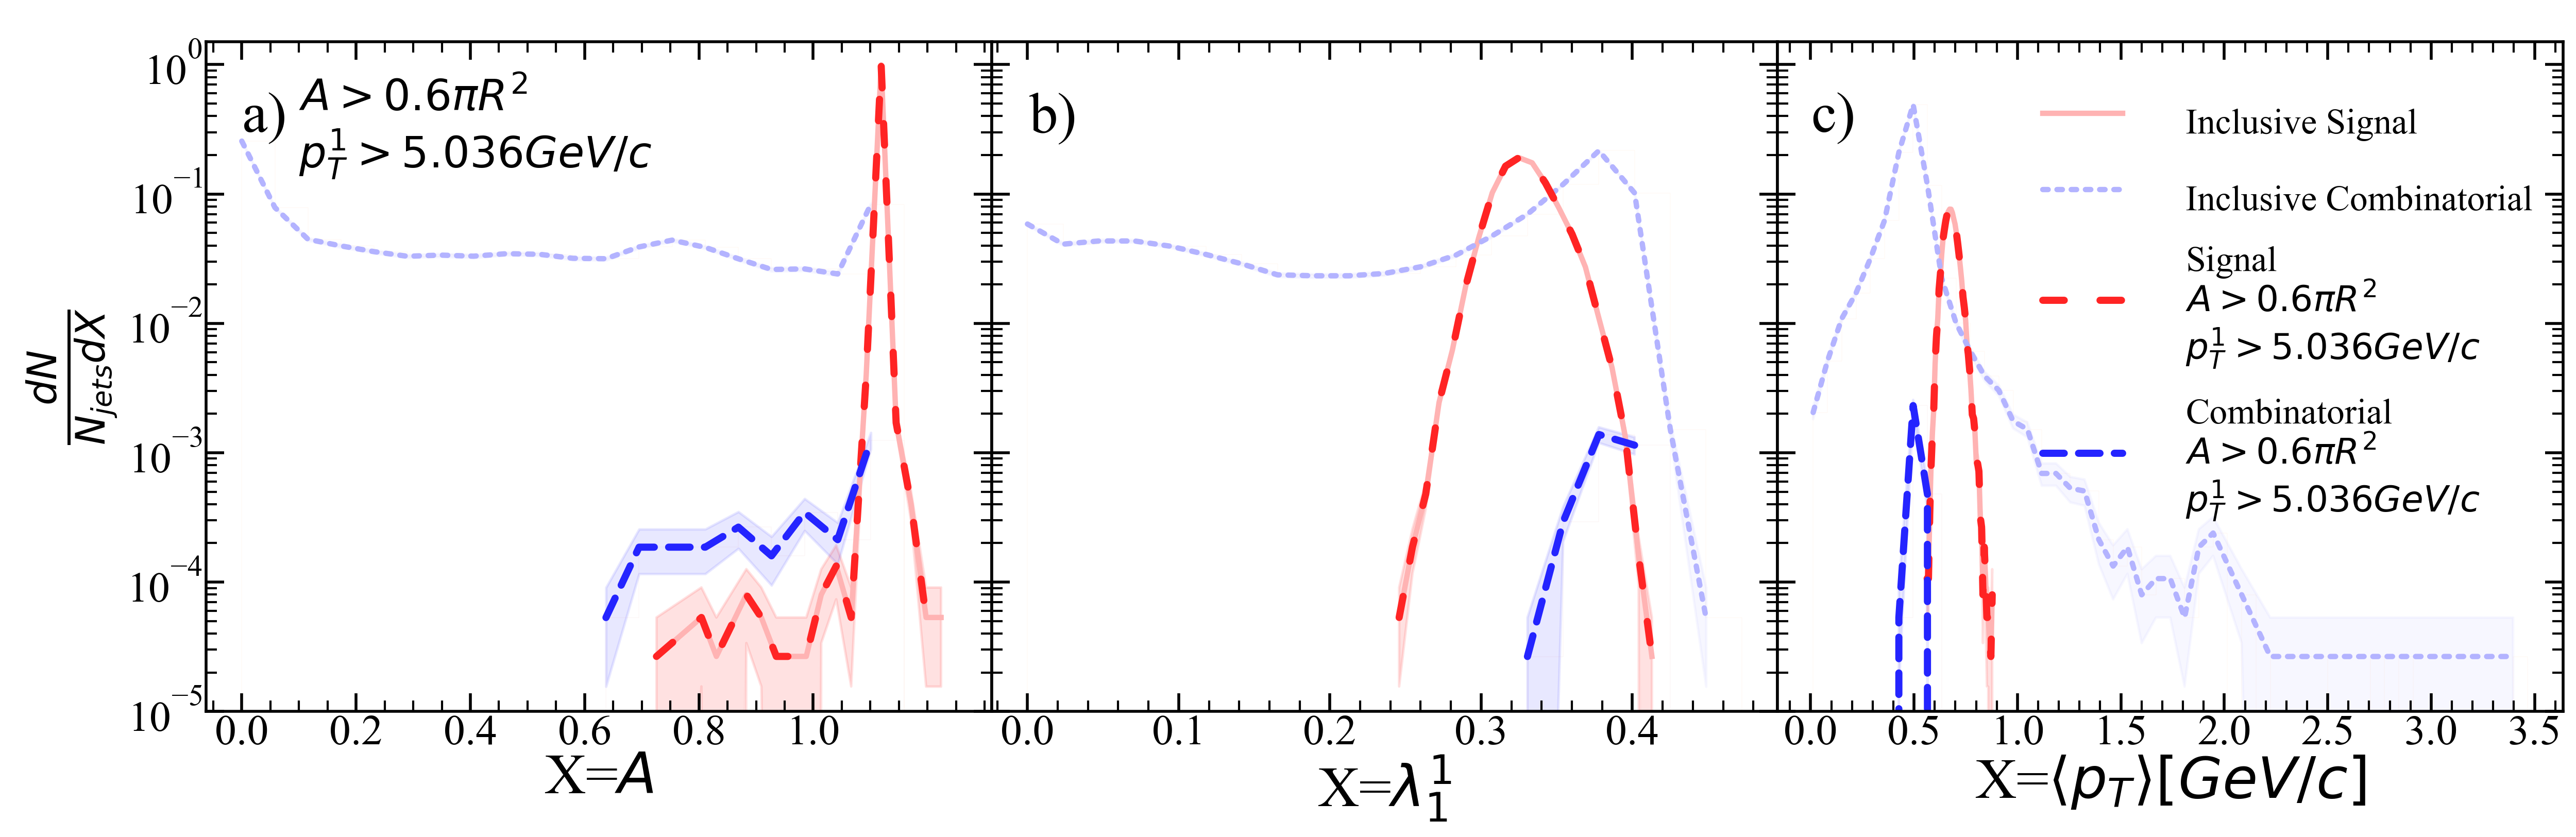}
    \caption{R=0.6 \ptH=80 \GeV}
    \label{fig:ml_06_80}
\end{figure*}
\clearpage
\subsection{Area, jet width, and mean constituent momentum after applying the looser leading hadron momentum selection.}

\begin{figure*}
    \centering
    \includegraphics[width=\linewidth]{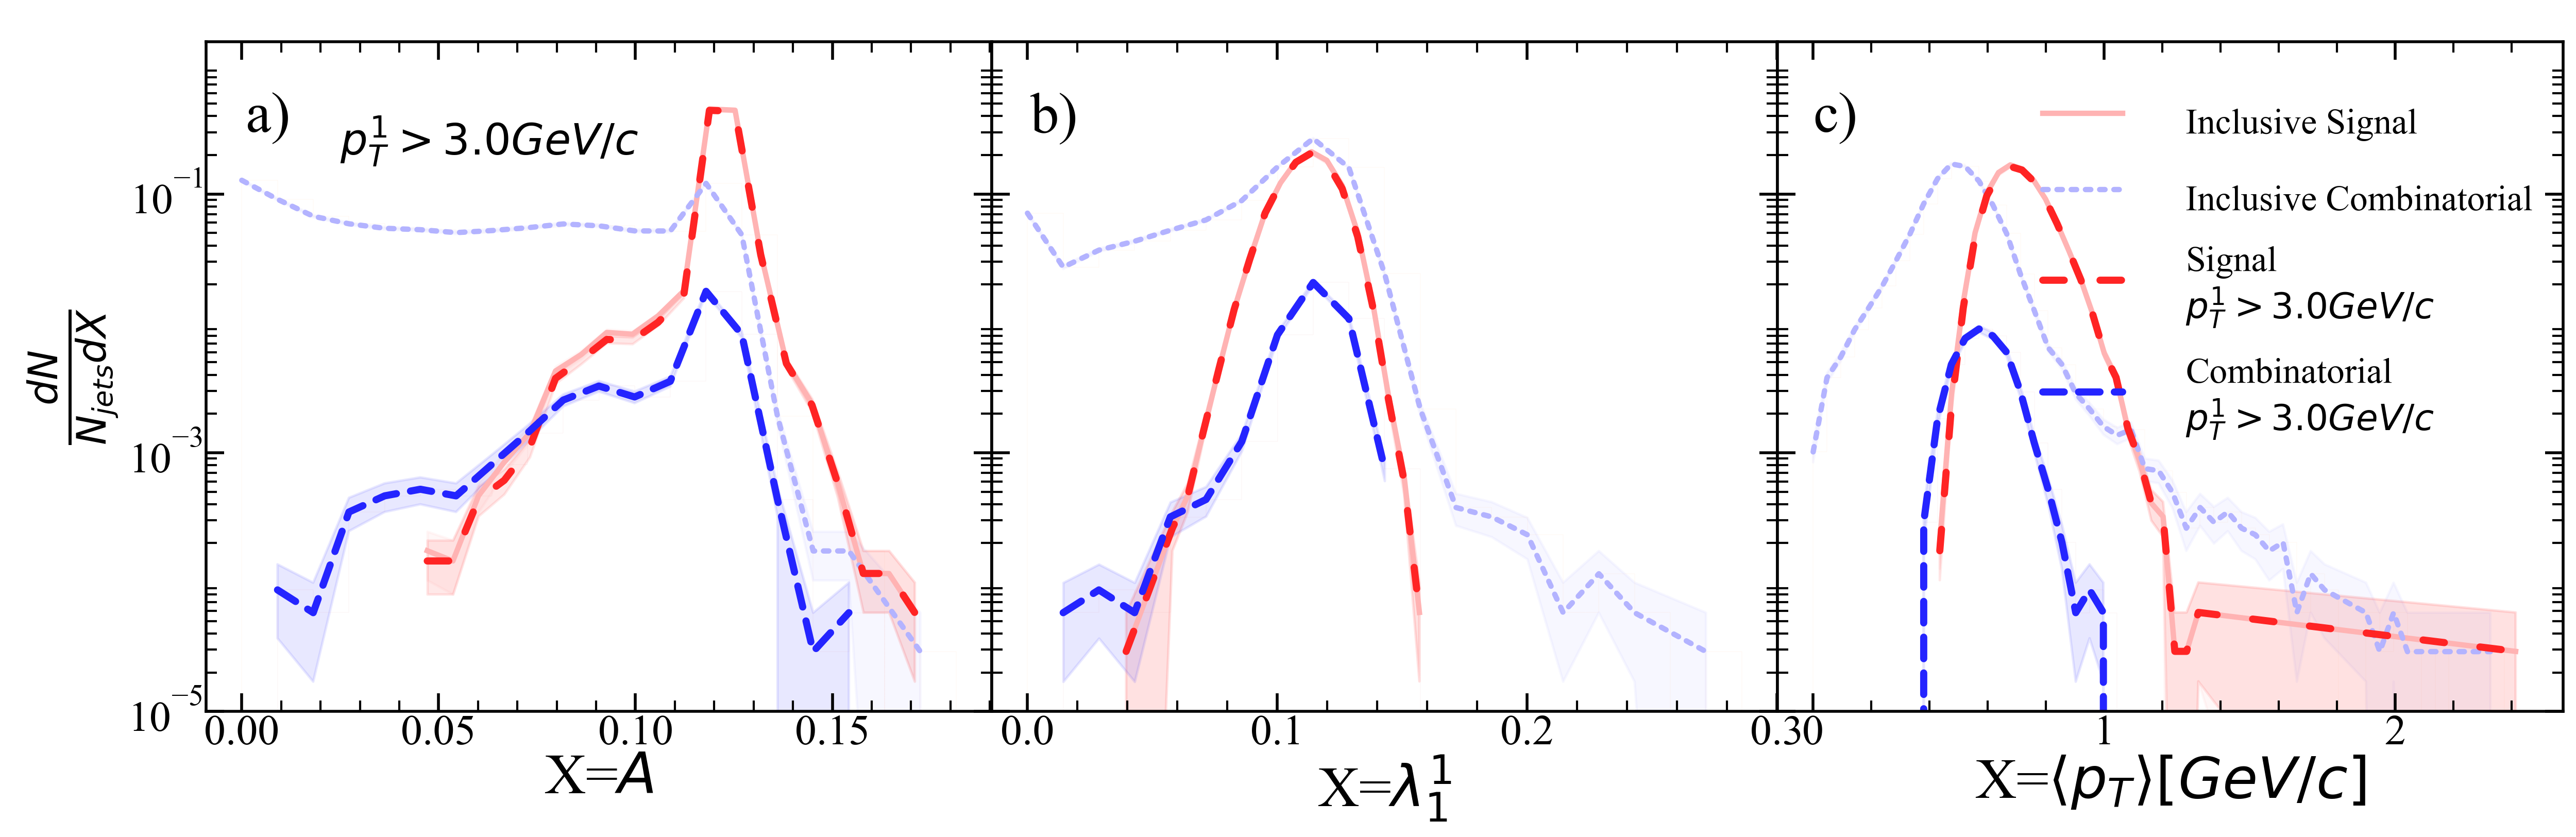}
    \caption{R=0.2 \ptH=10 \GeV}
    \label{fig:pT1_02_10}
\end{figure*}

\begin{figure*}
    \centering
    \includegraphics[width=\linewidth]{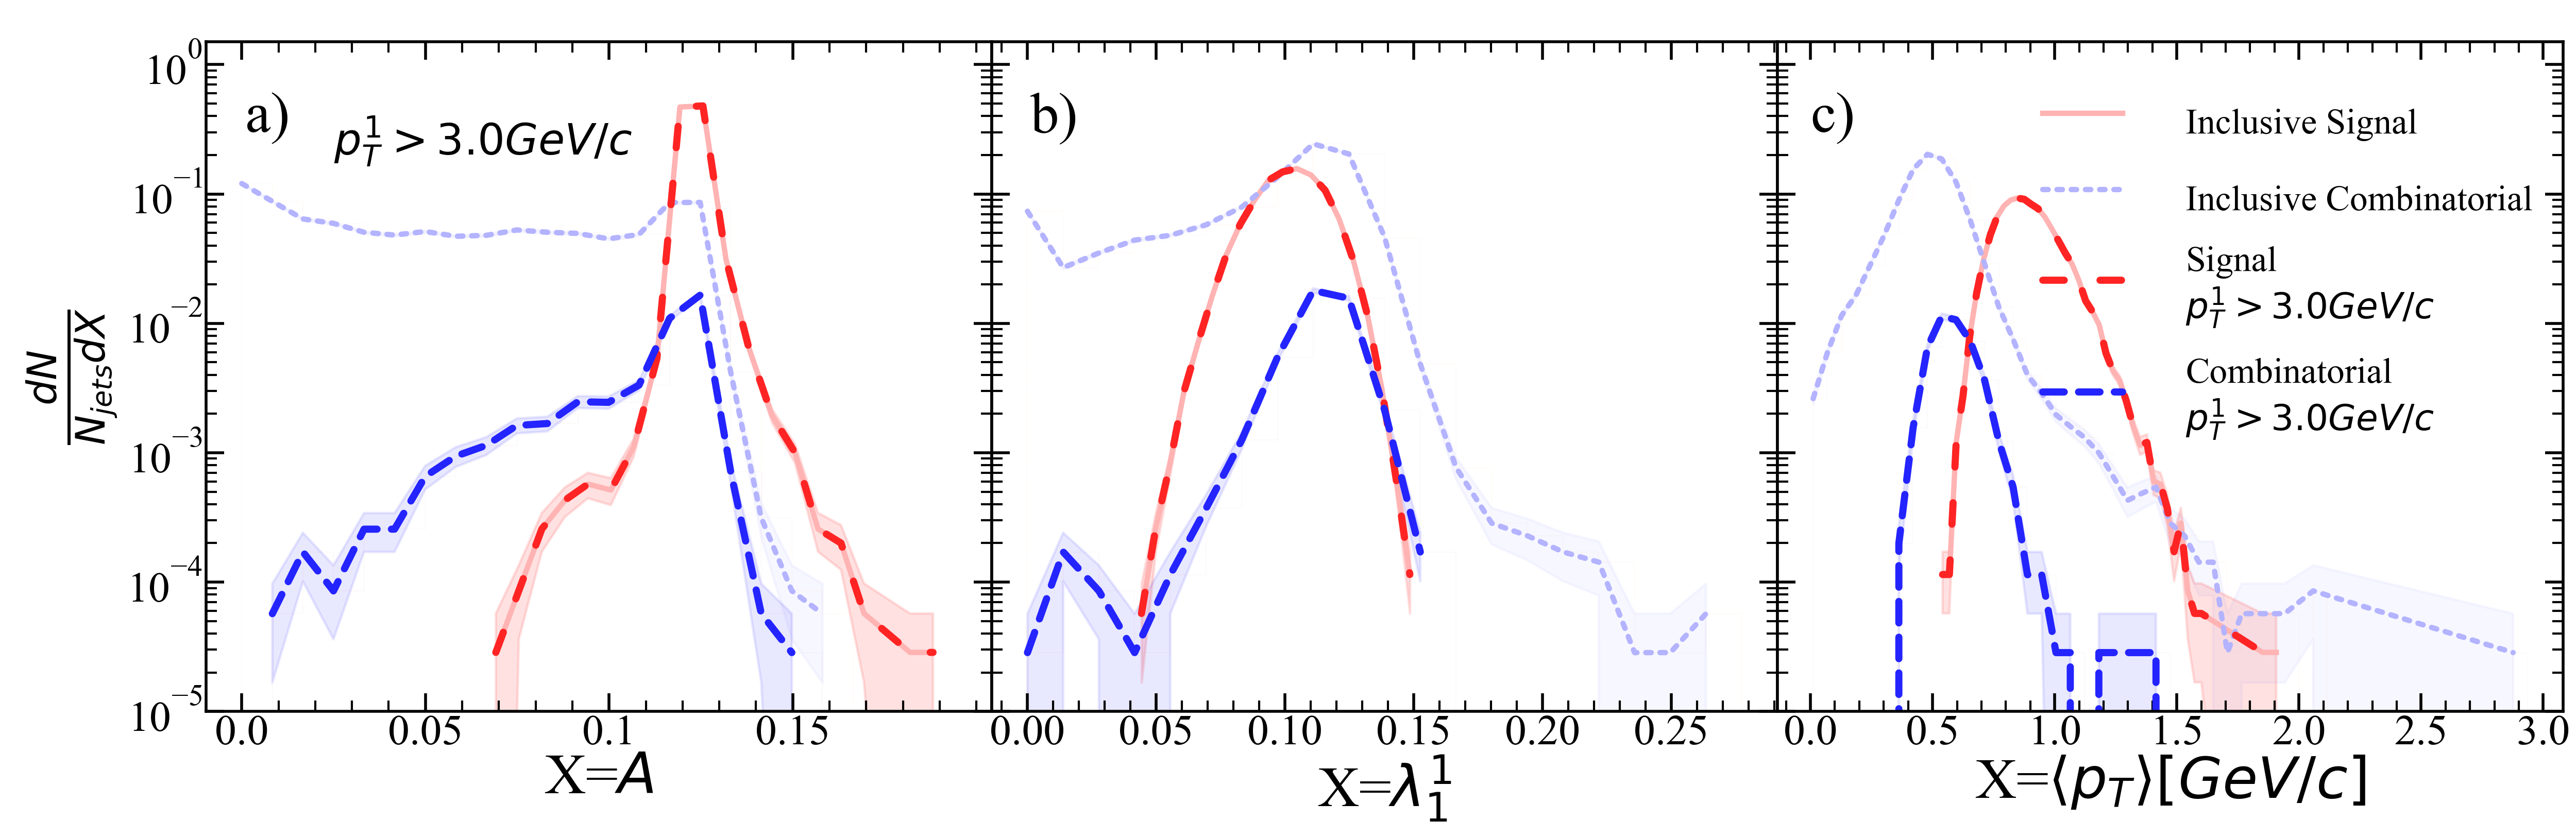}
    \caption{R=0.2 \ptH=20 \GeV}
    \label{fig:pT1_02_20}
\end{figure*}

\begin{figure*}
    \centering
    \includegraphics[width=\linewidth]{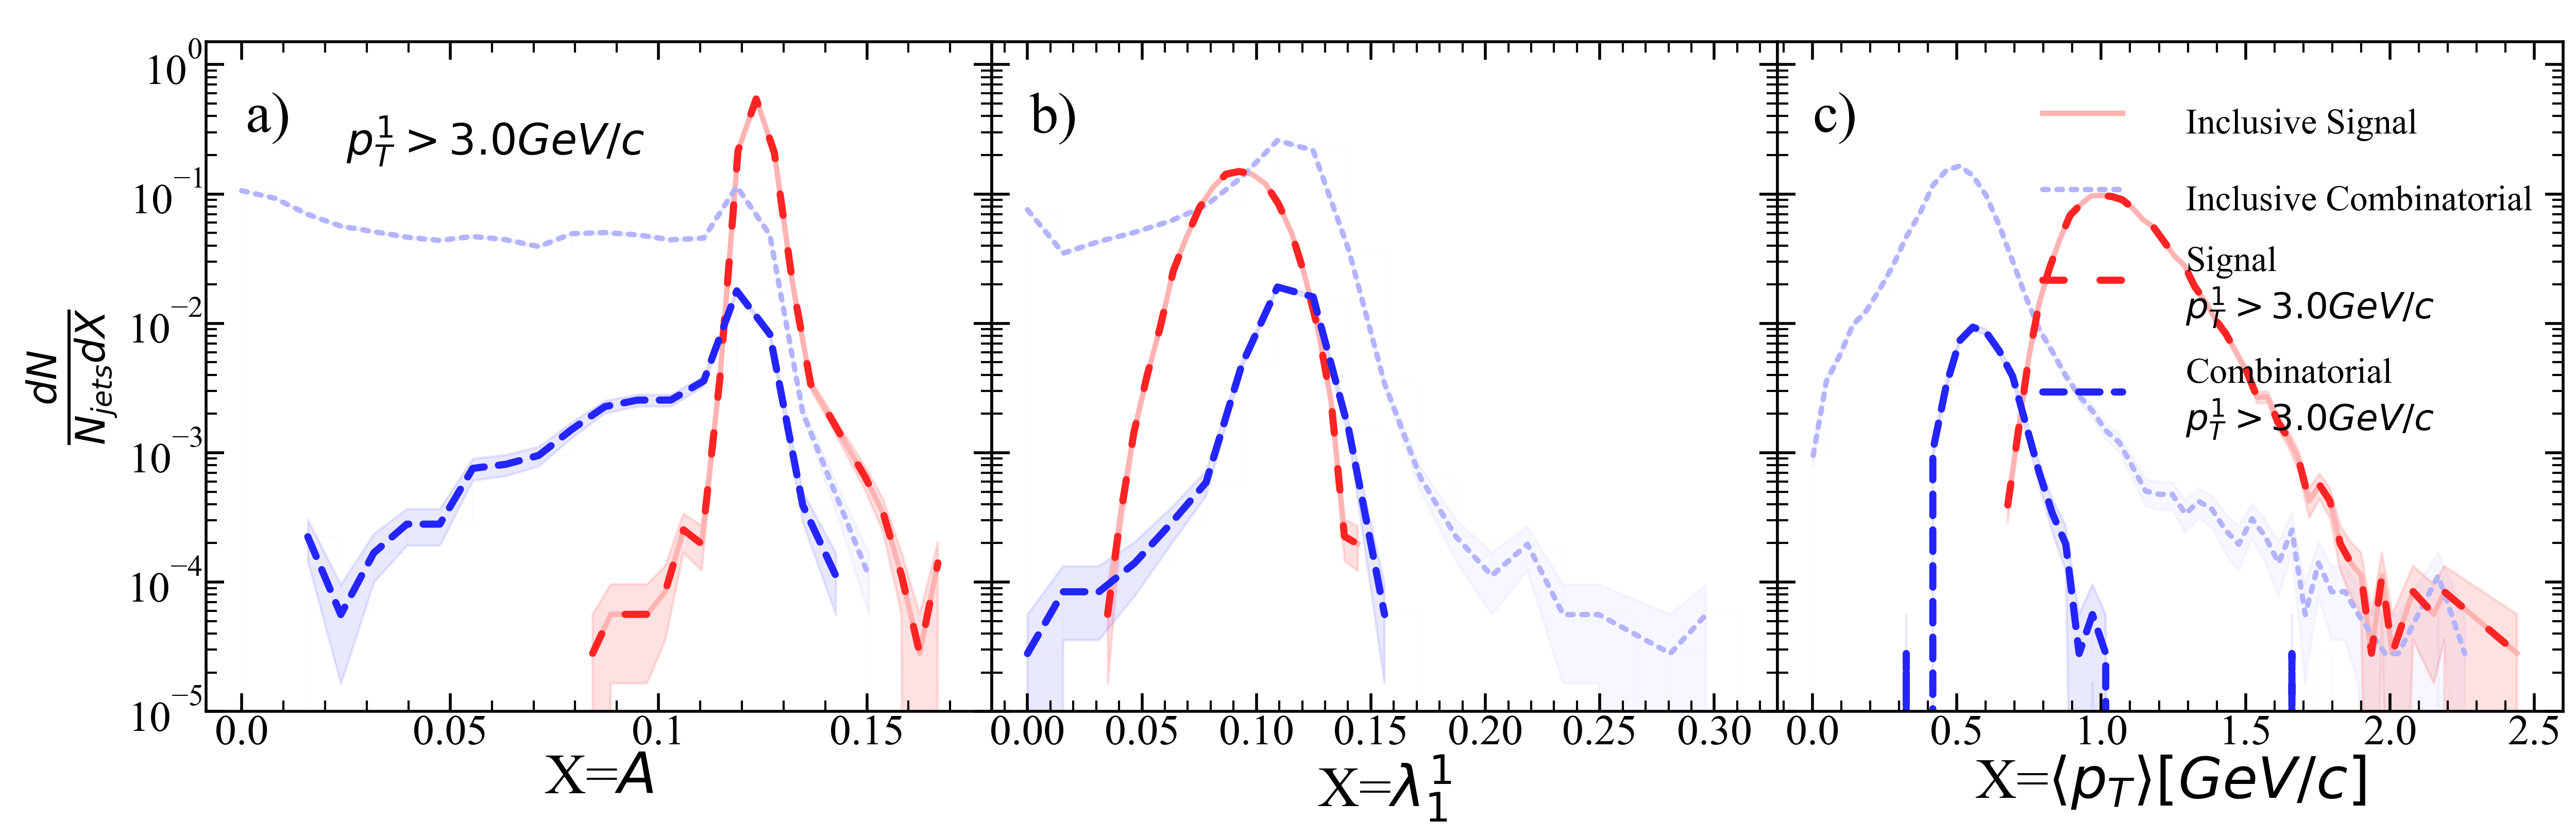}
    \caption{R=0.2 \ptH=30 \GeV}
    \label{fig:pT1_02_30}
\end{figure*}

\begin{figure*}
    \centering
    \includegraphics[width=\linewidth]{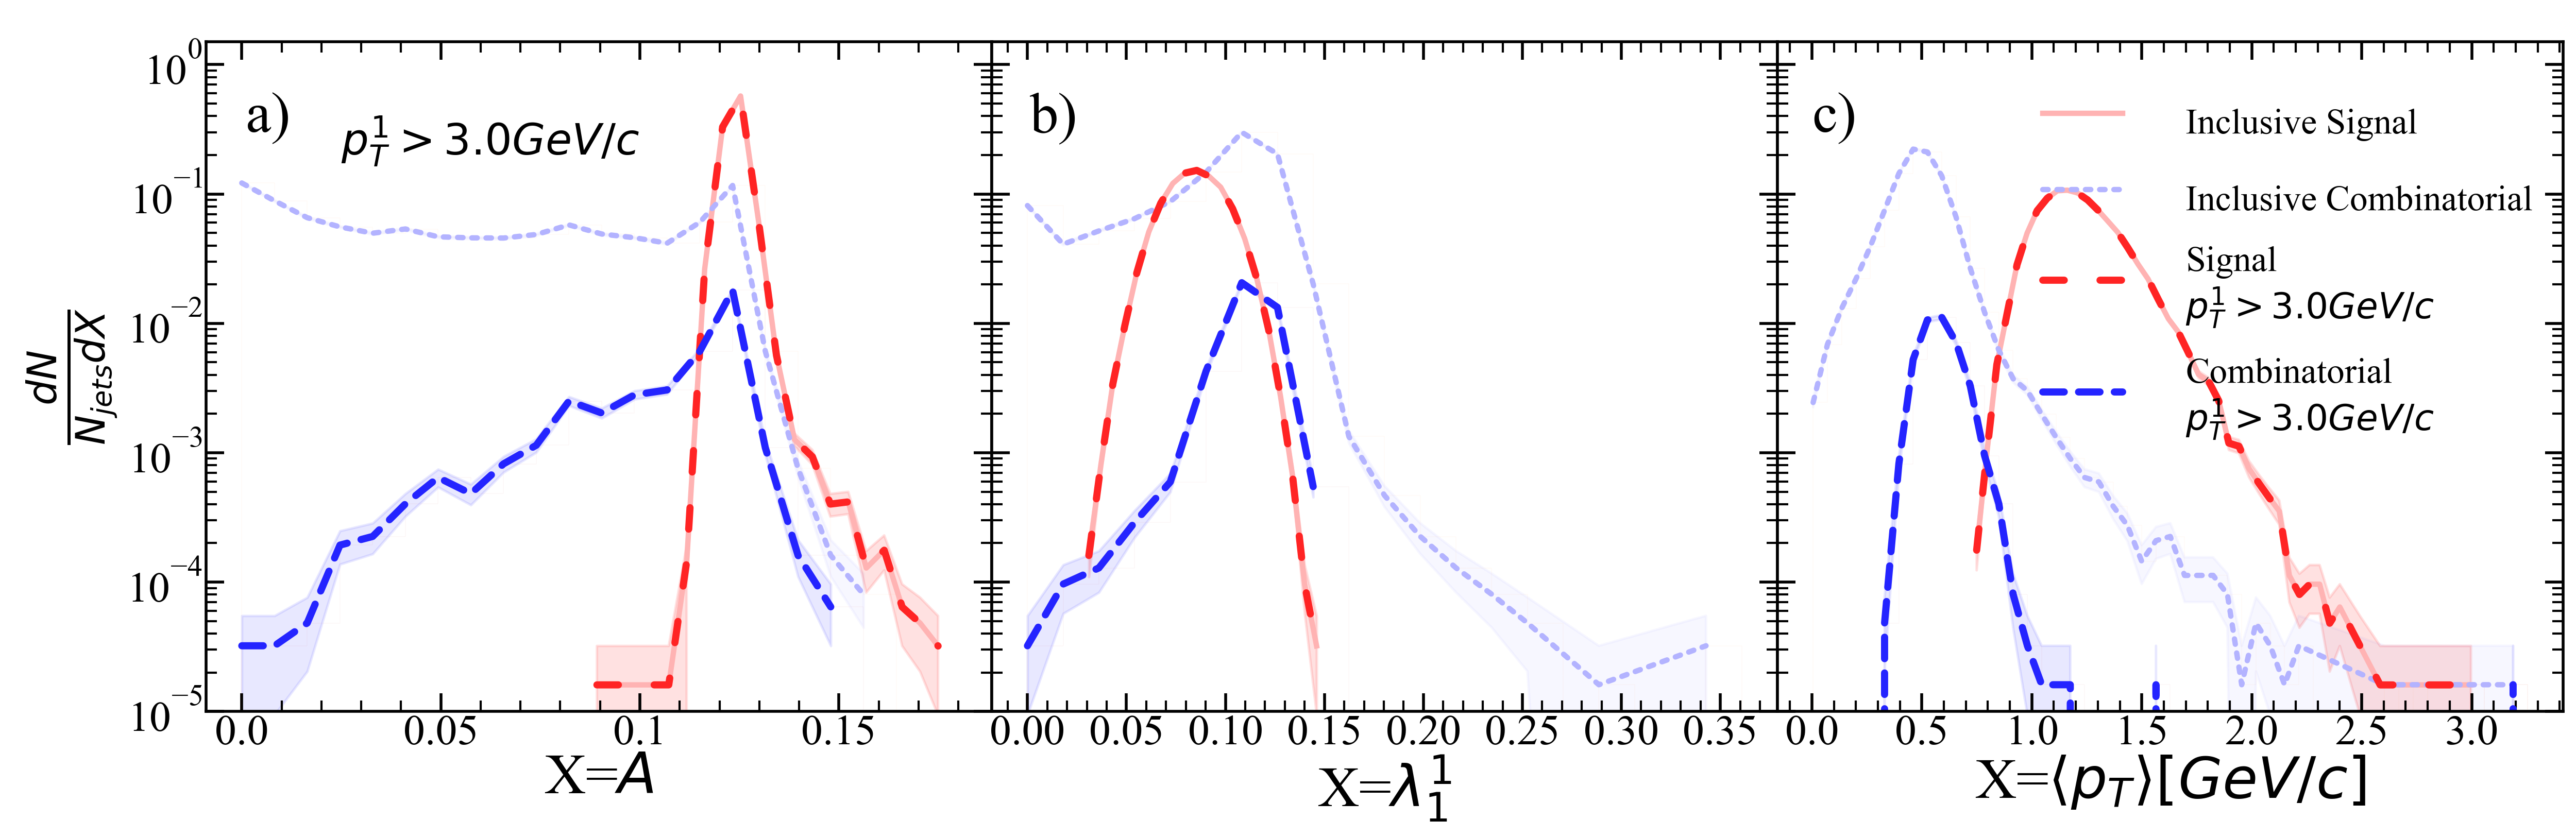}
    \caption{R=0.2 \ptH=40 \GeV}
    \label{fig:pT1_02_40}
\end{figure*}

\begin{figure*}
    \centering
    \includegraphics[width=\linewidth]{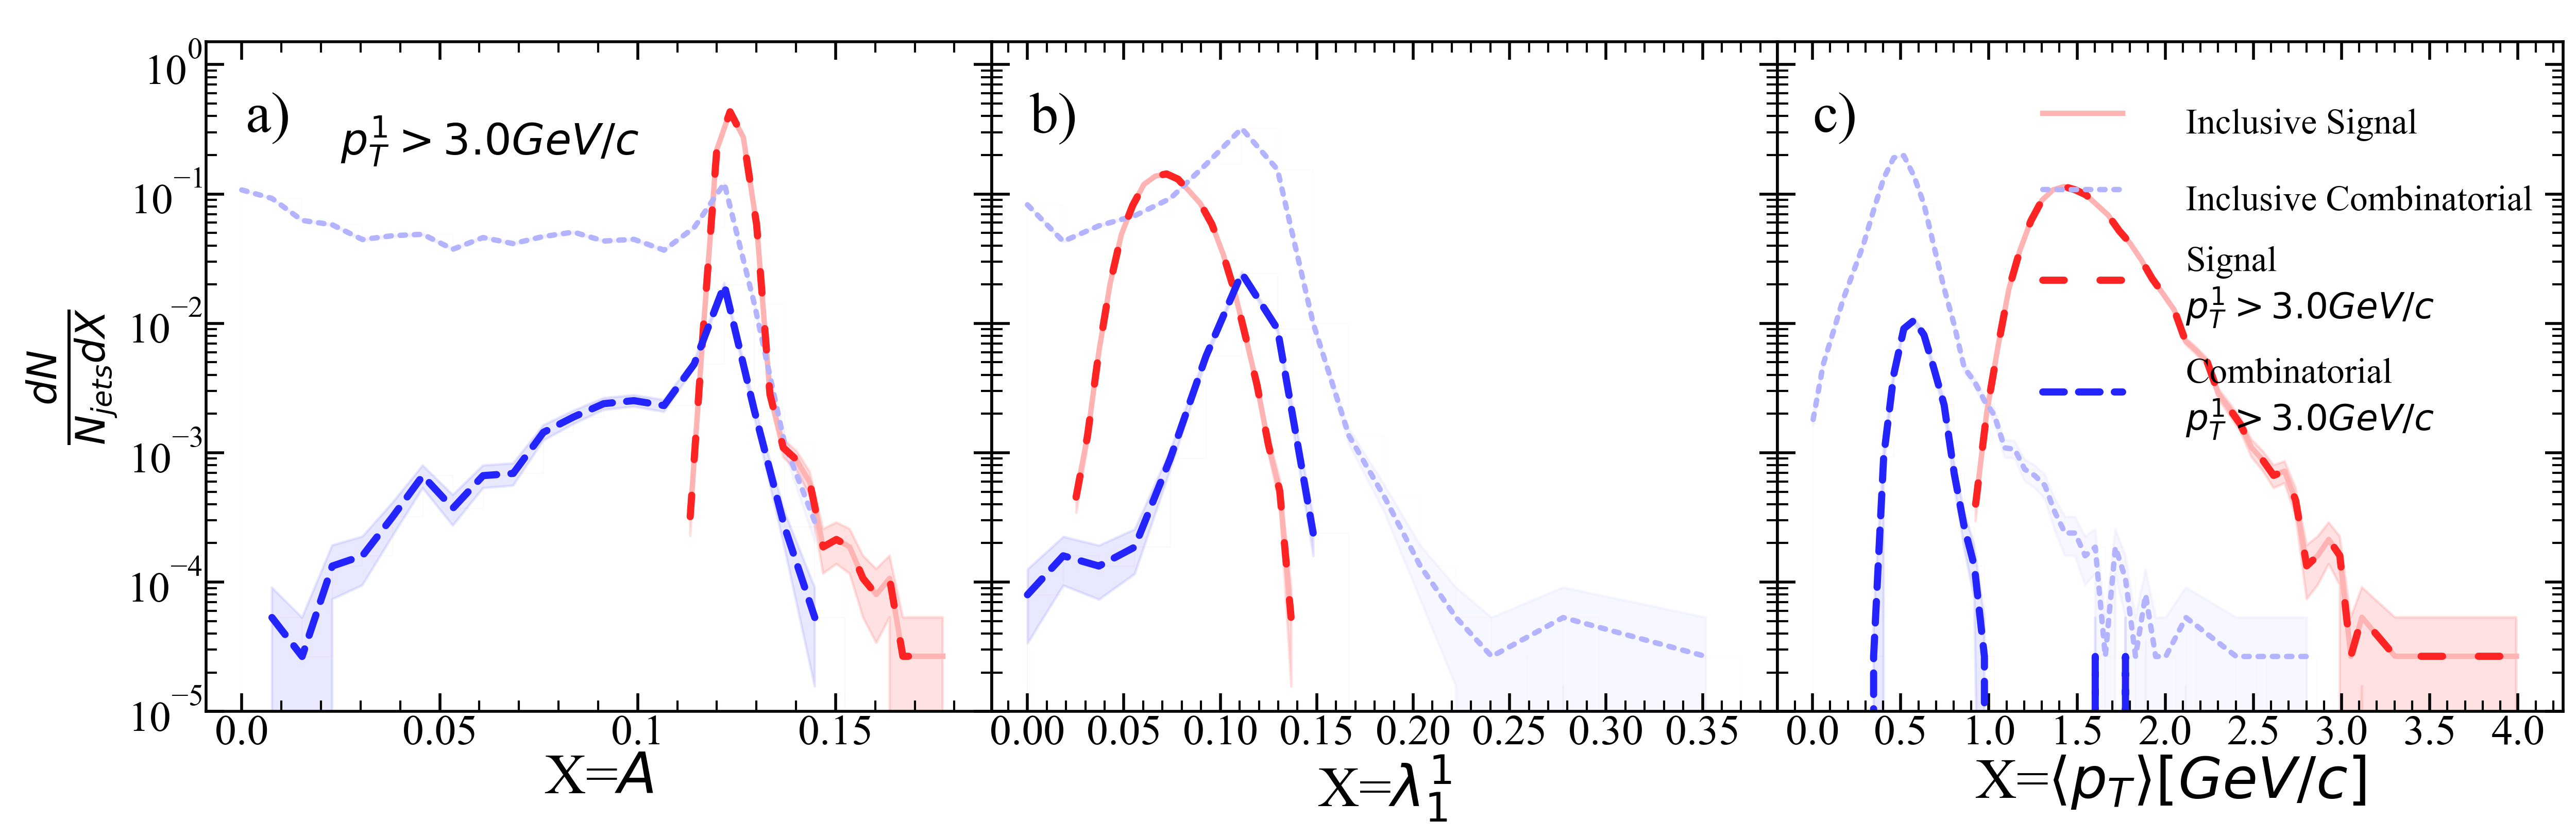}
    \caption{R=0.2 \ptH=60 \GeV}
    \label{fig:pT1_02_60}
\end{figure*}

\begin{figure*}
    \centering
    \includegraphics[width=\linewidth]{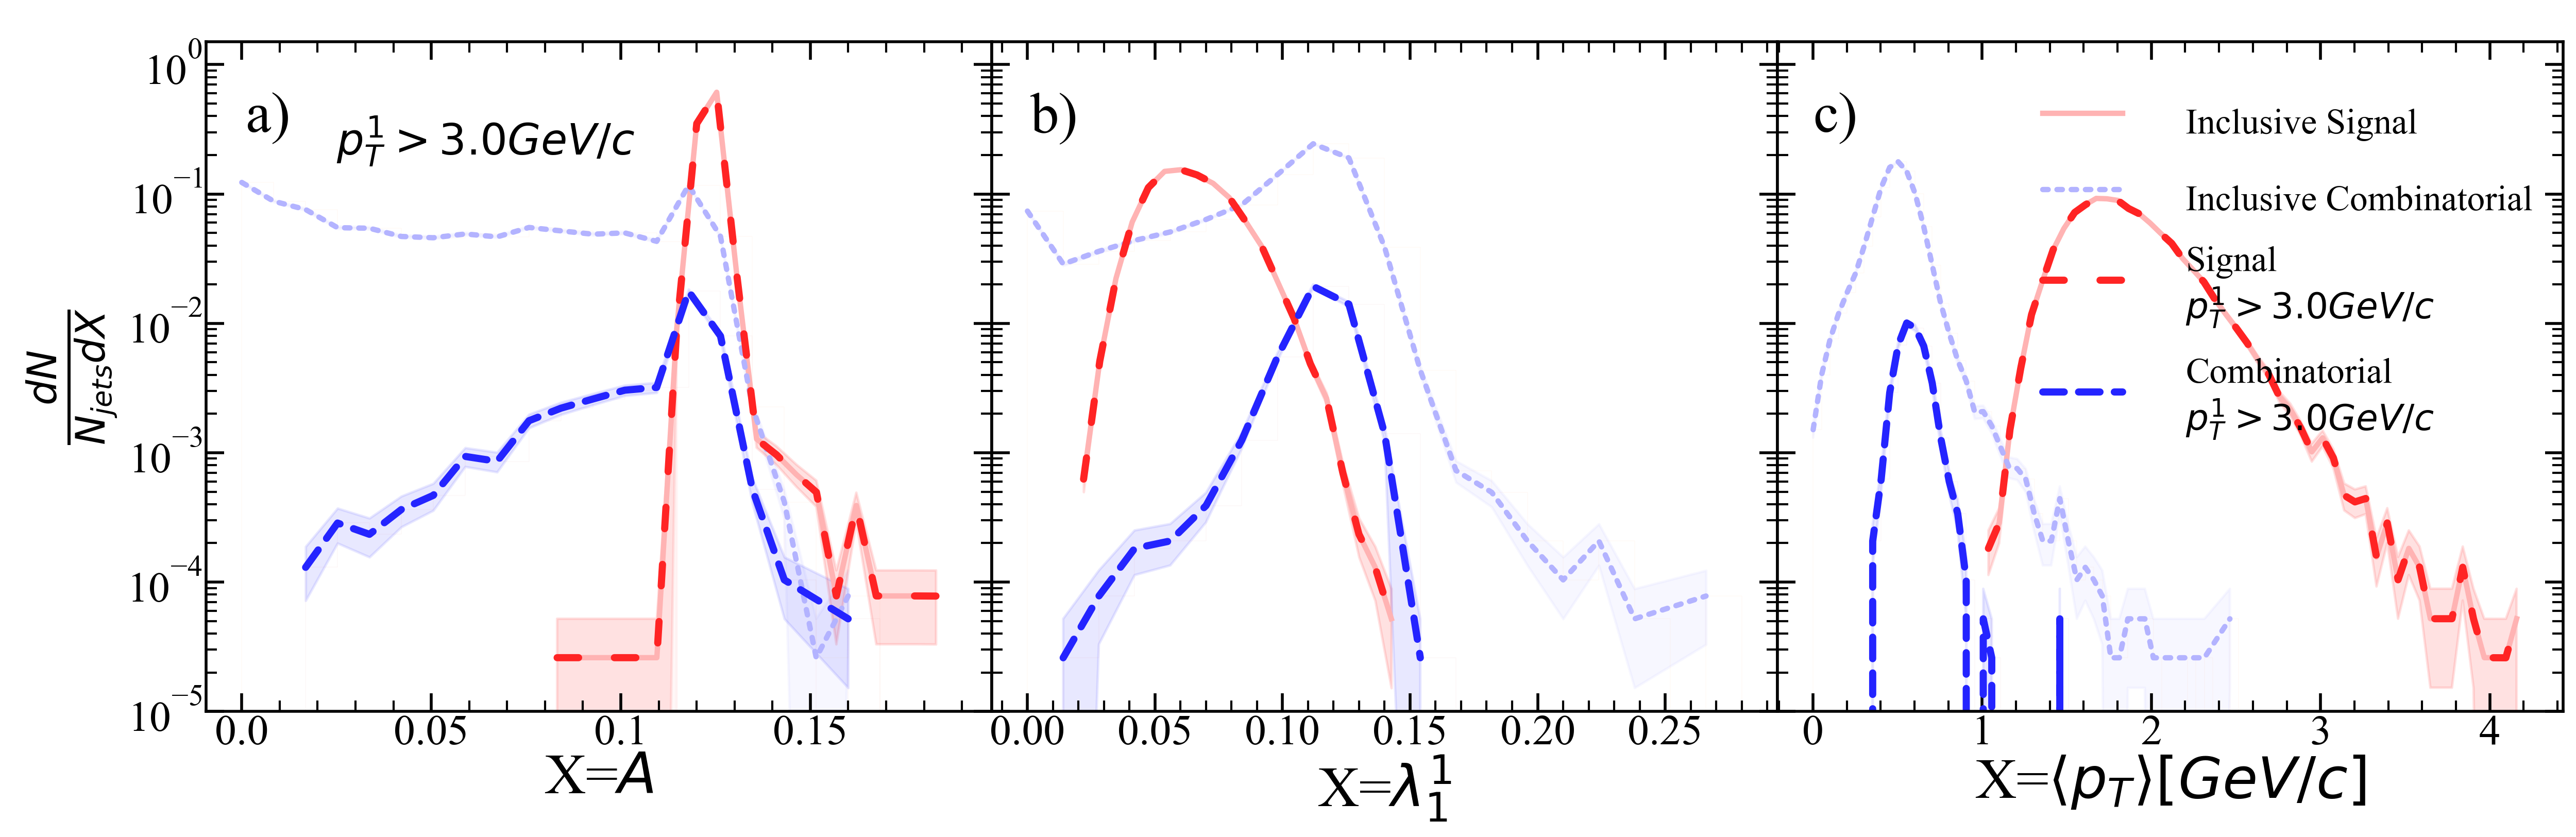}
    \caption{R=0.2 \ptH=80 \GeV}
    \label{fig:pT1_02_80}
\end{figure*}

\begin{figure*}
    \centering
    \includegraphics[width=\linewidth]{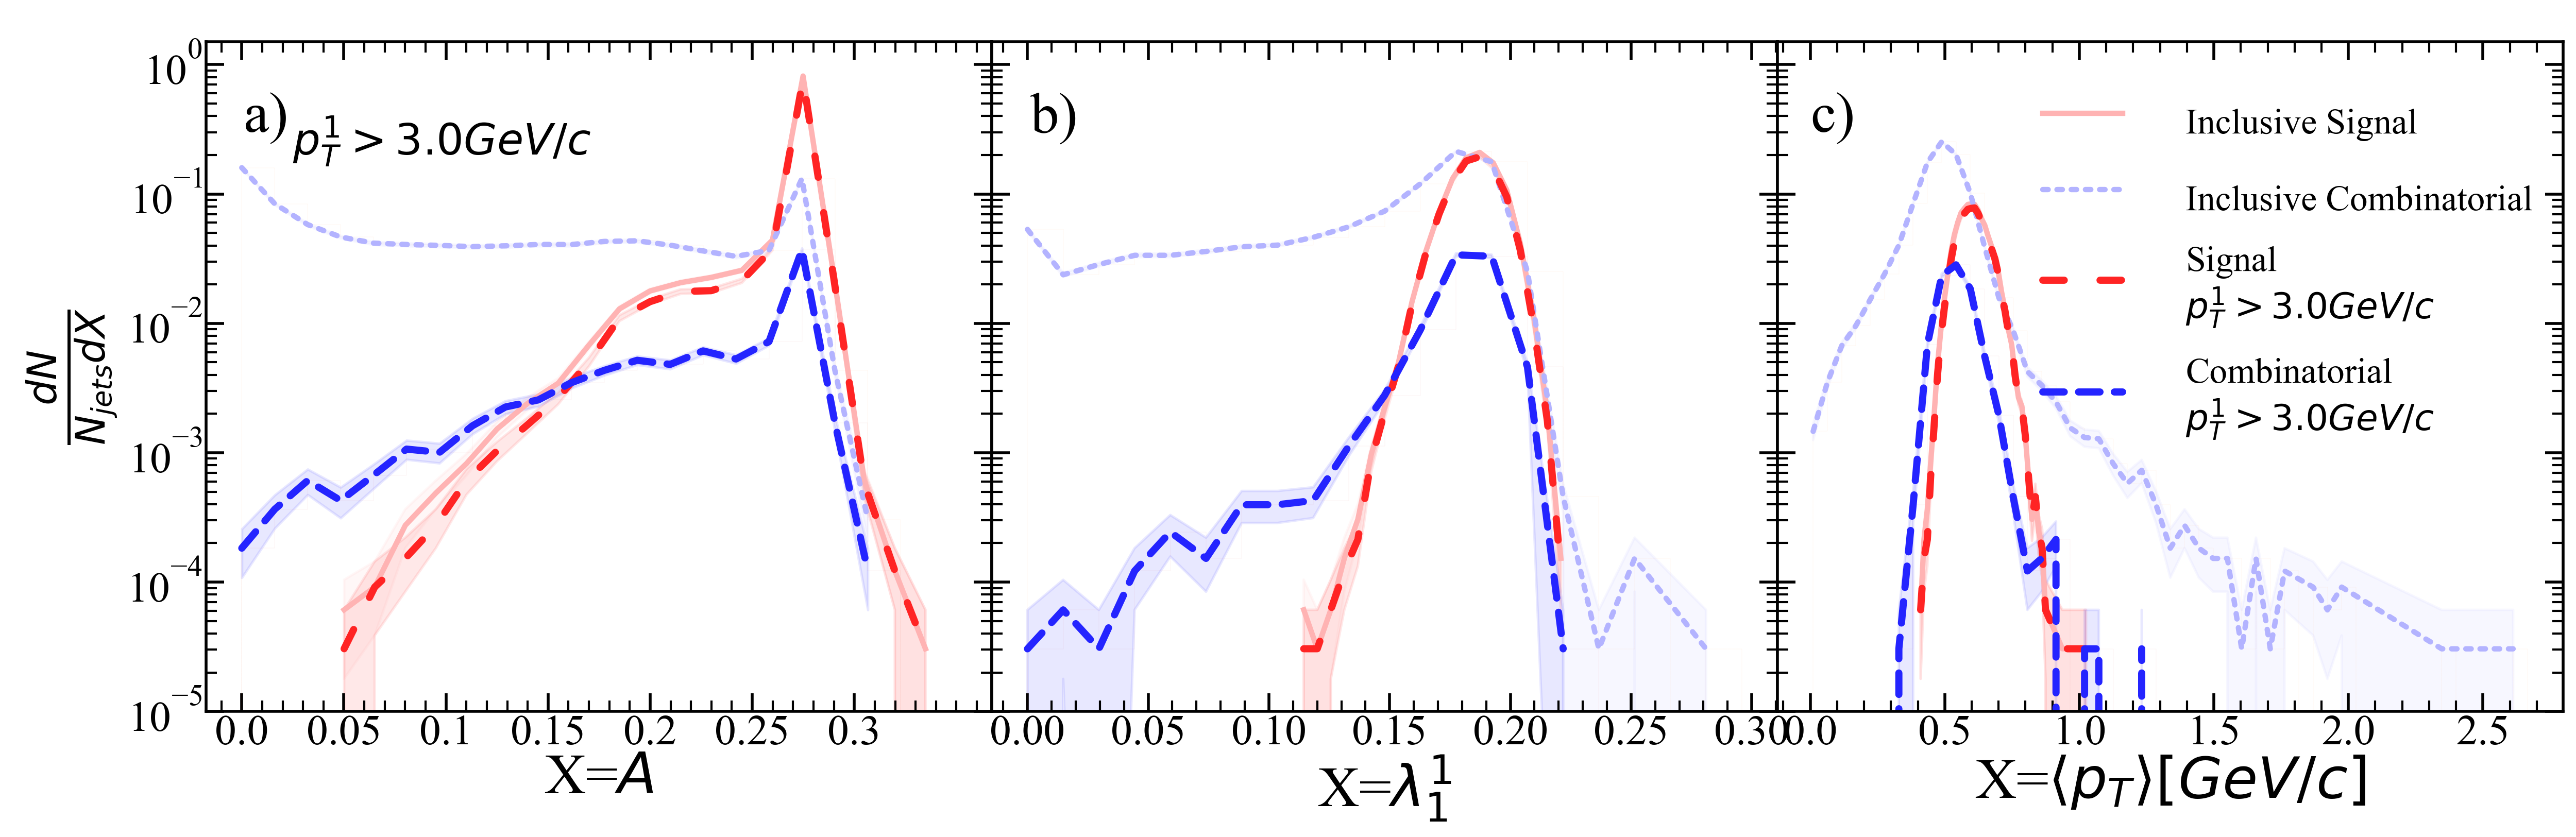}
    \caption{R=0.3 \ptH=10 \GeV}
    \label{fig:pT1_03_10}
\end{figure*}

\begin{figure*}
    \centering
    \includegraphics[width=\linewidth]{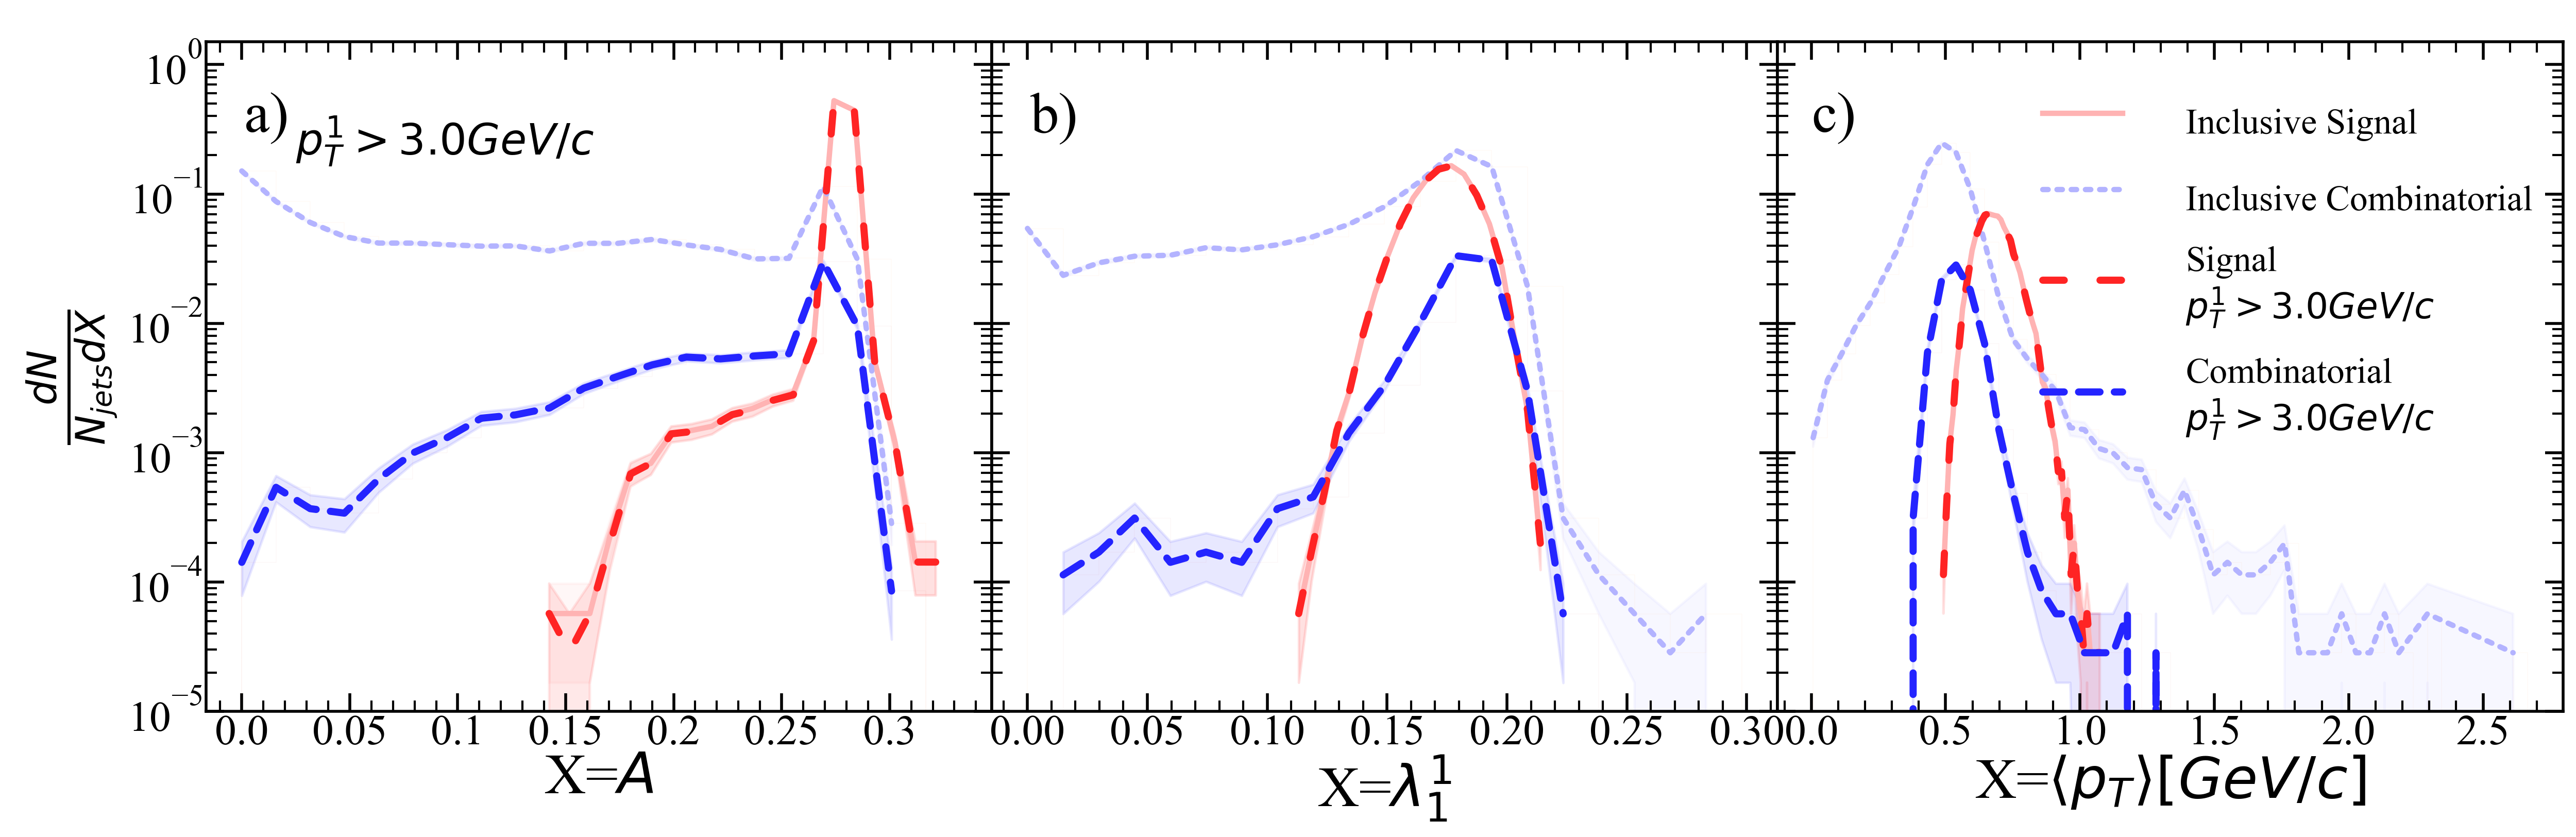}
    \caption{R=0.3 \ptH=20 \GeV}
    \label{fig:pT1_03_20}
\end{figure*}

\begin{figure*}
    \centering
    \includegraphics[width=\linewidth]{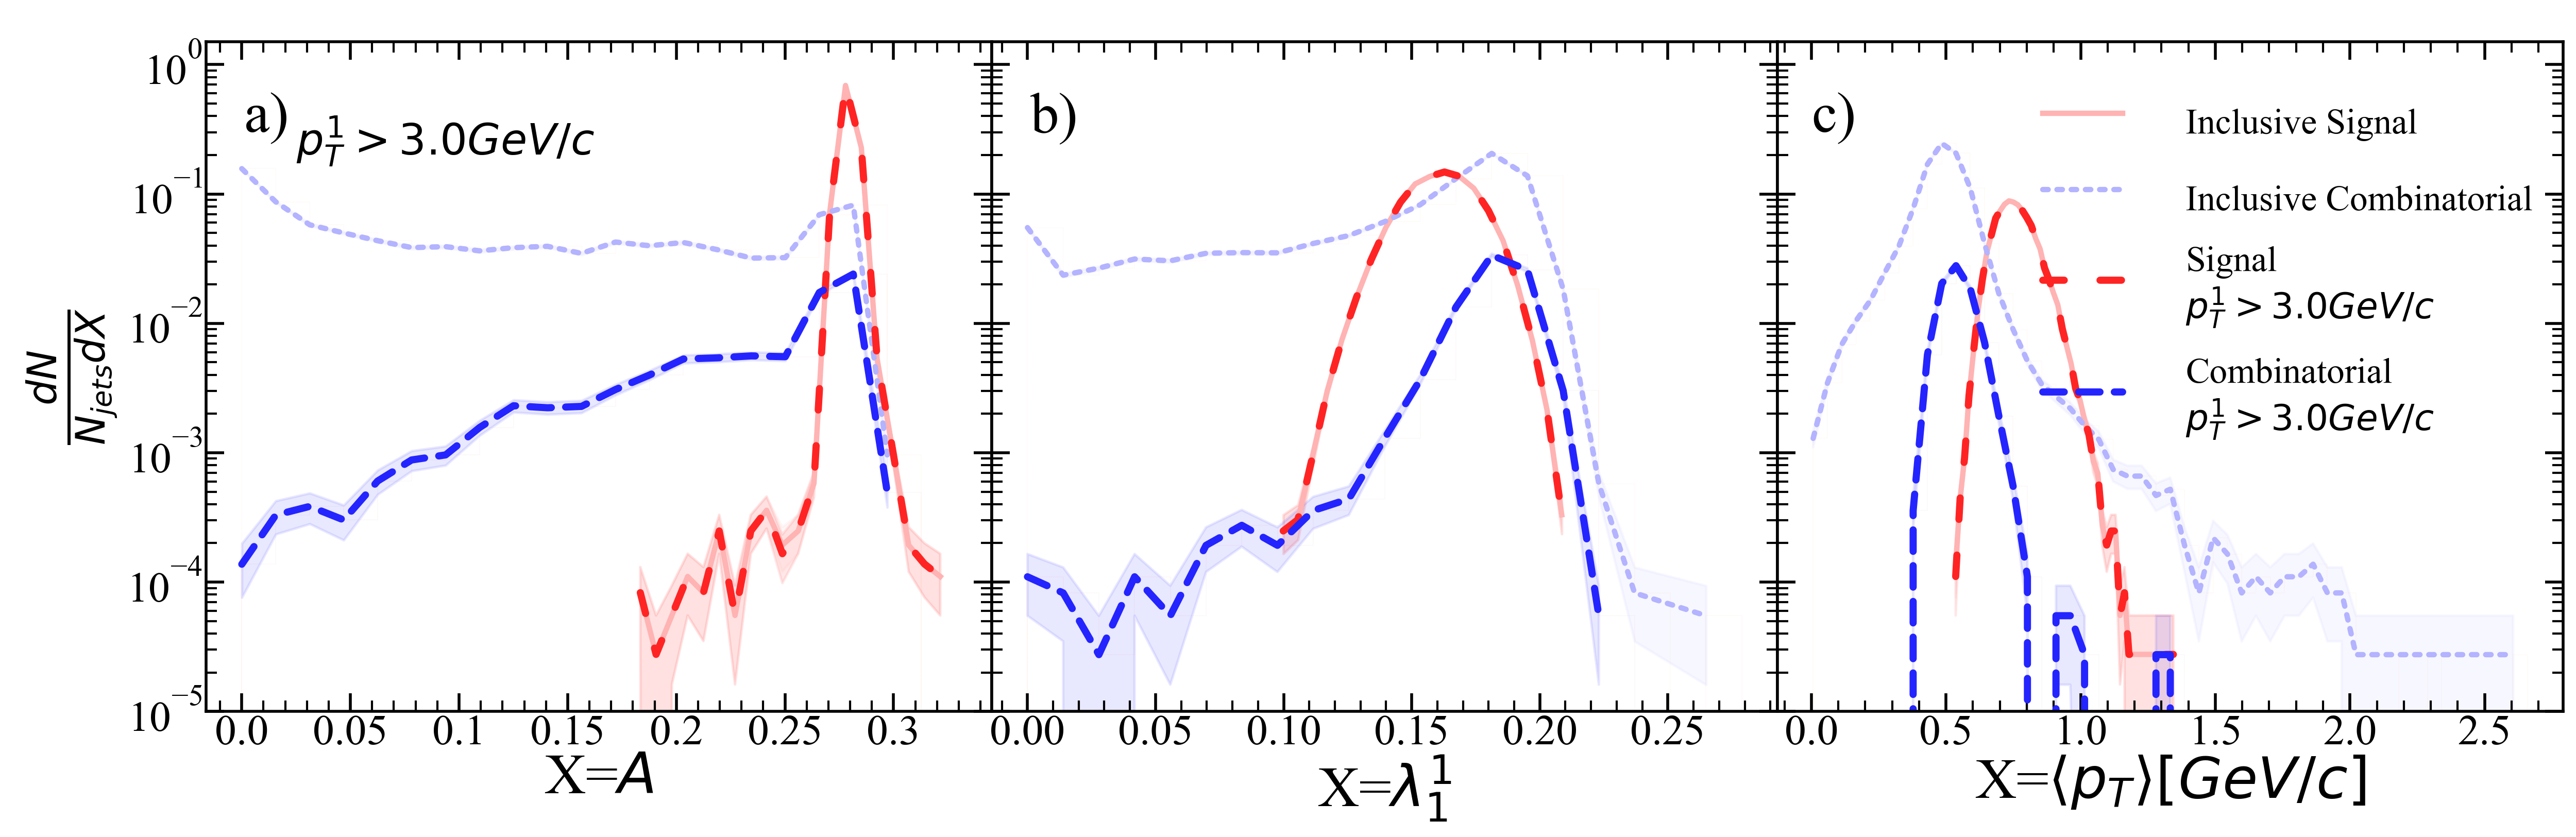}
    \caption{R=0.3 \ptH=30 \GeV}
    \label{fig:pT1_03_30}
\end{figure*}

\begin{figure*}
    \centering
    \includegraphics[width=\linewidth]{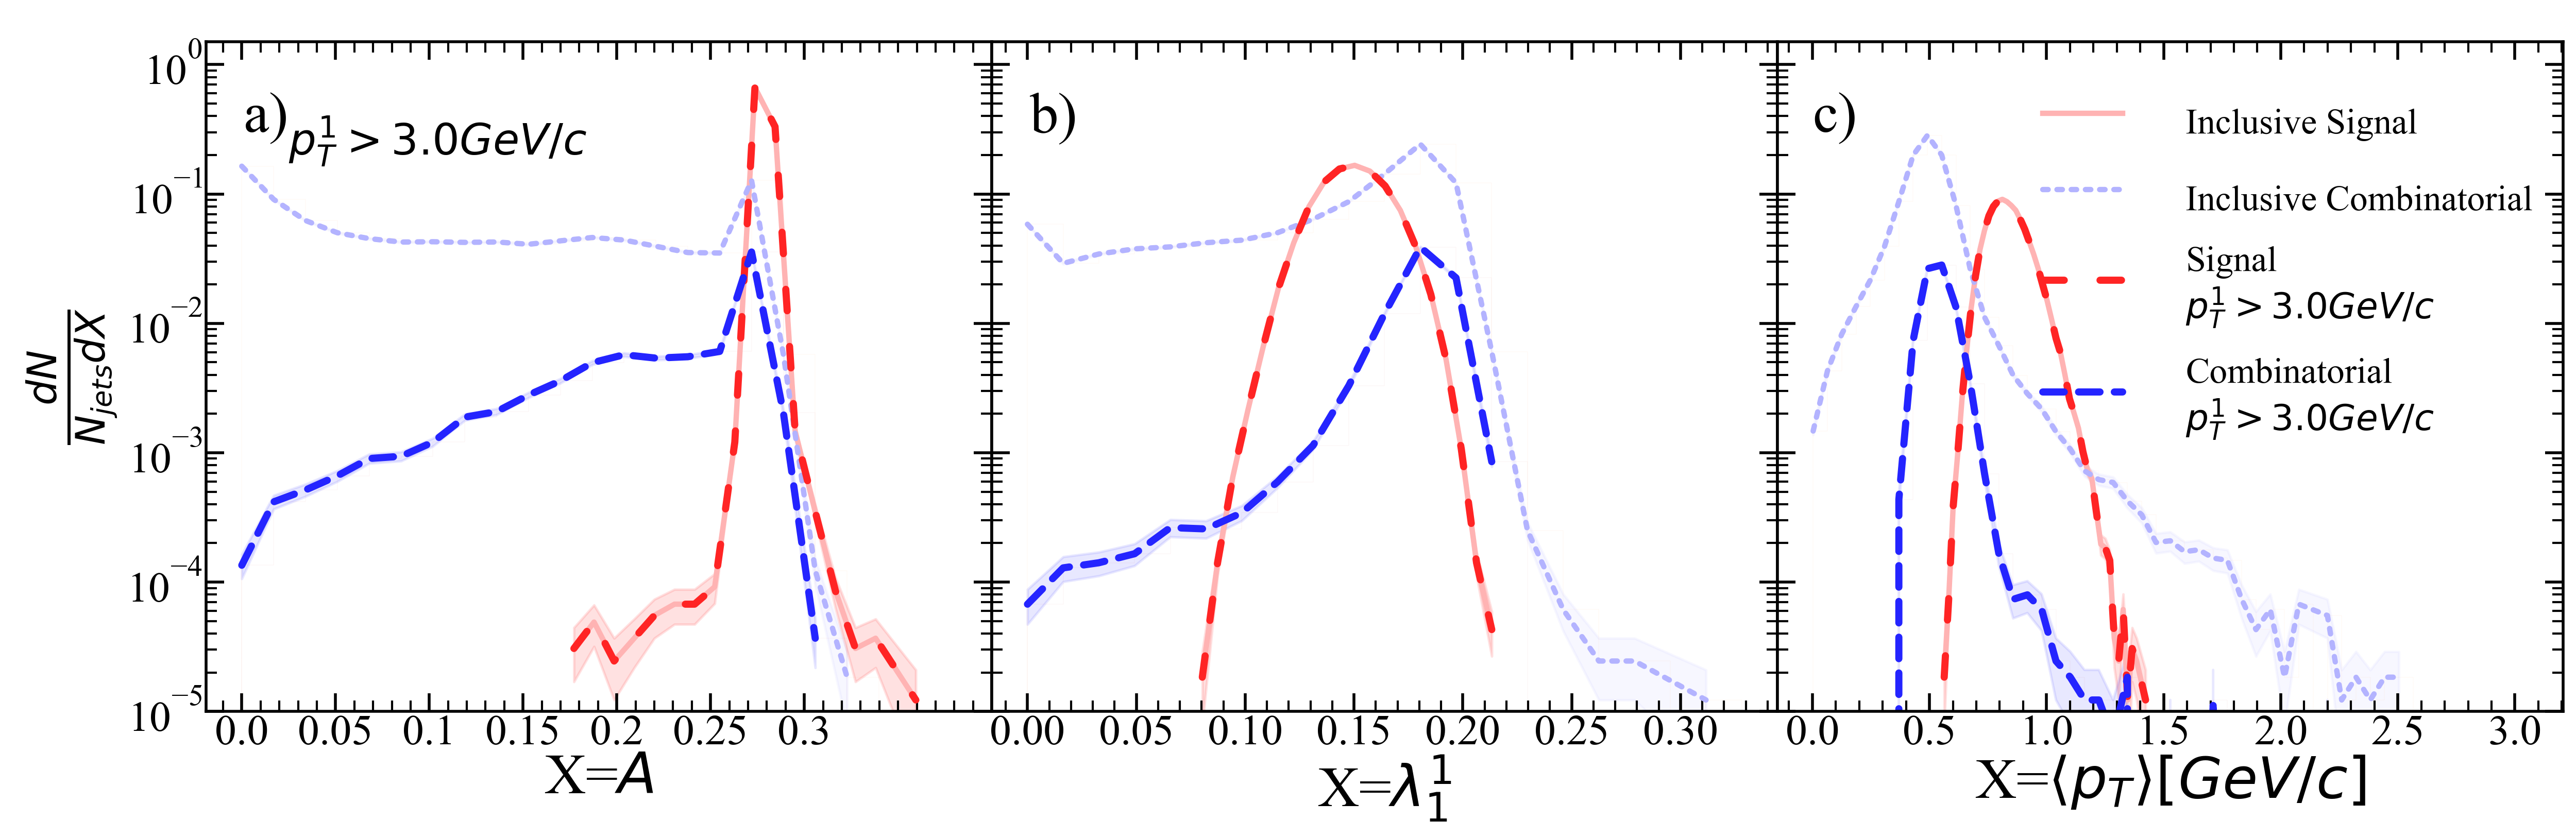}
    \caption{R=0.3 \ptH=40 \GeV}
    \label{fig:pT1_03_40}
\end{figure*}

\begin{figure*}
    \centering
    \includegraphics[width=\linewidth]{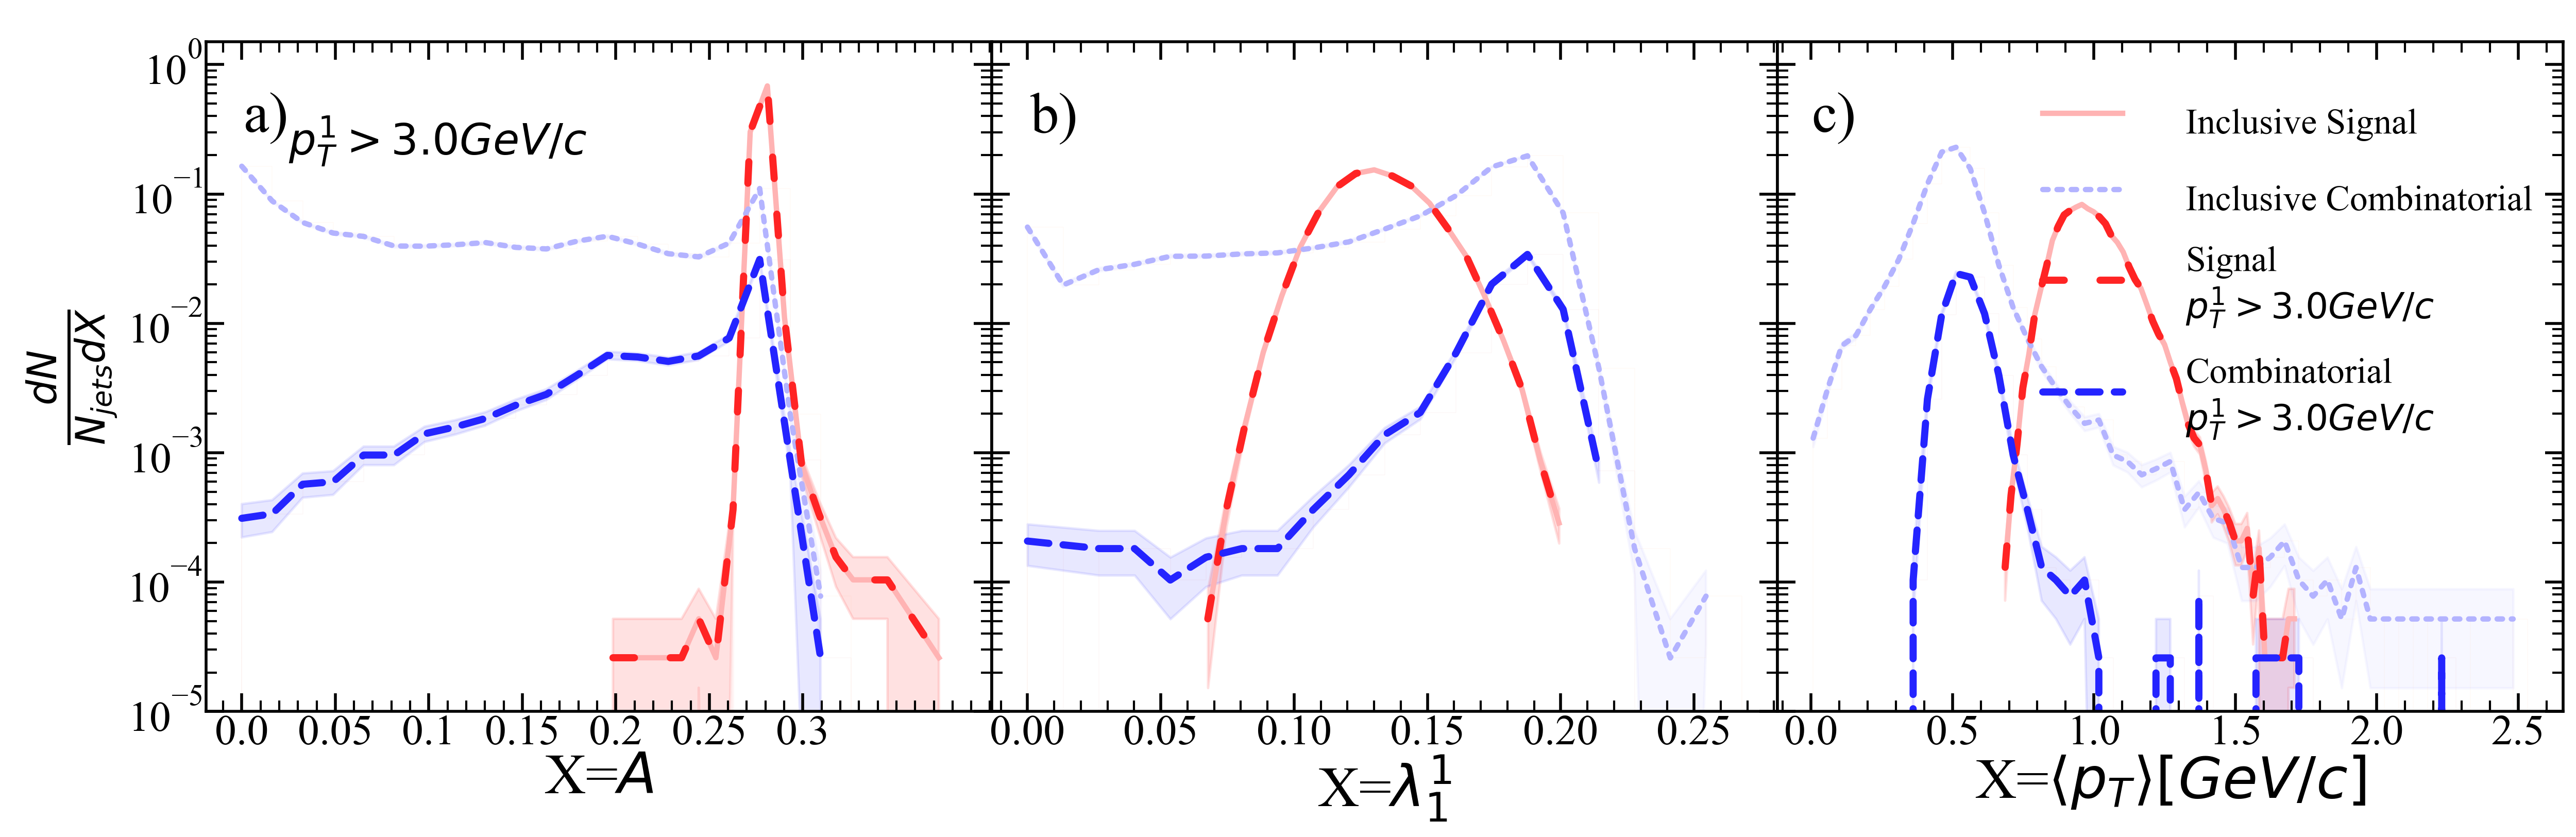}
    \caption{R=0.3 \ptH=60 \GeV}
    \label{fig:pT1_03_60}
\end{figure*}

\begin{figure*}
    \centering
    \includegraphics[width=\linewidth]{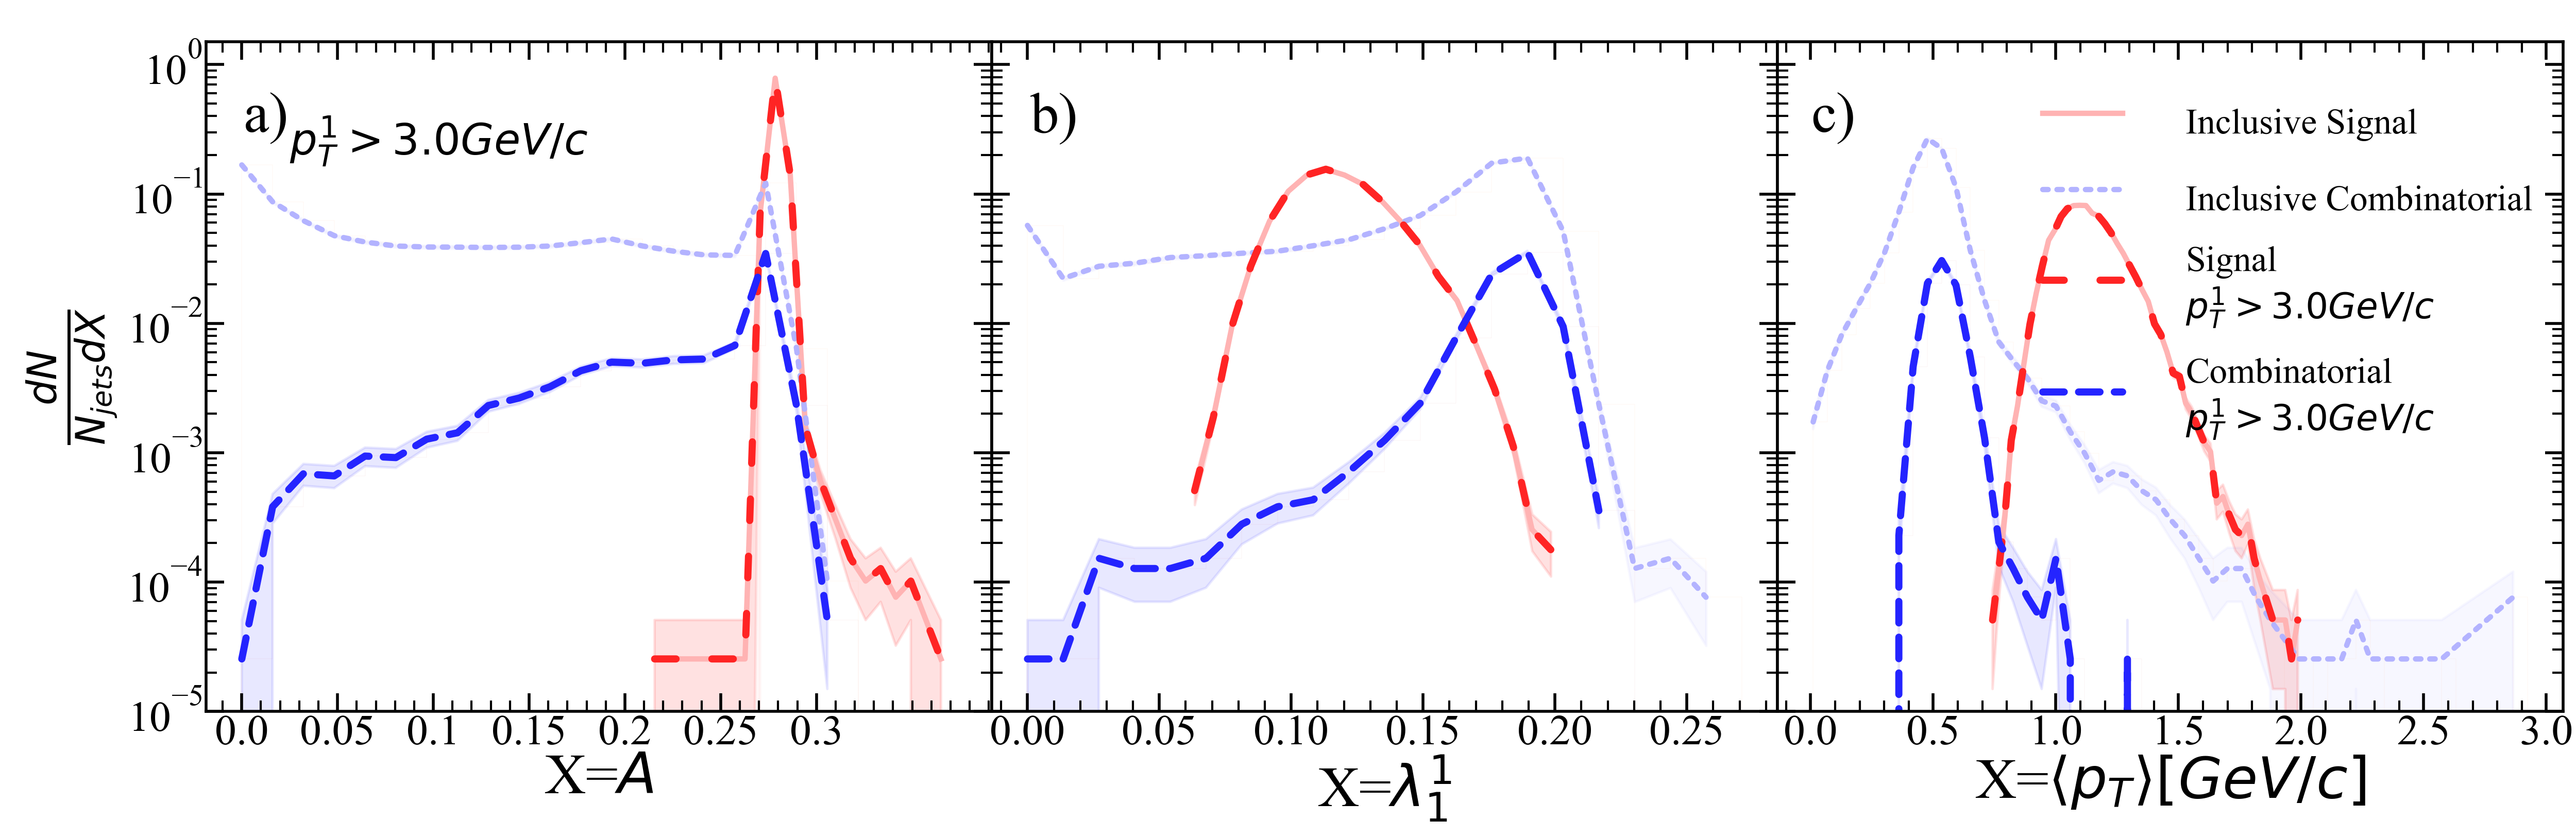}
    \caption{R=0.3 \ptH=80 \GeV}
    \label{fig:pT1_03_80}
\end{figure*}

\begin{figure*}
    \centering
    \includegraphics[width=\linewidth]{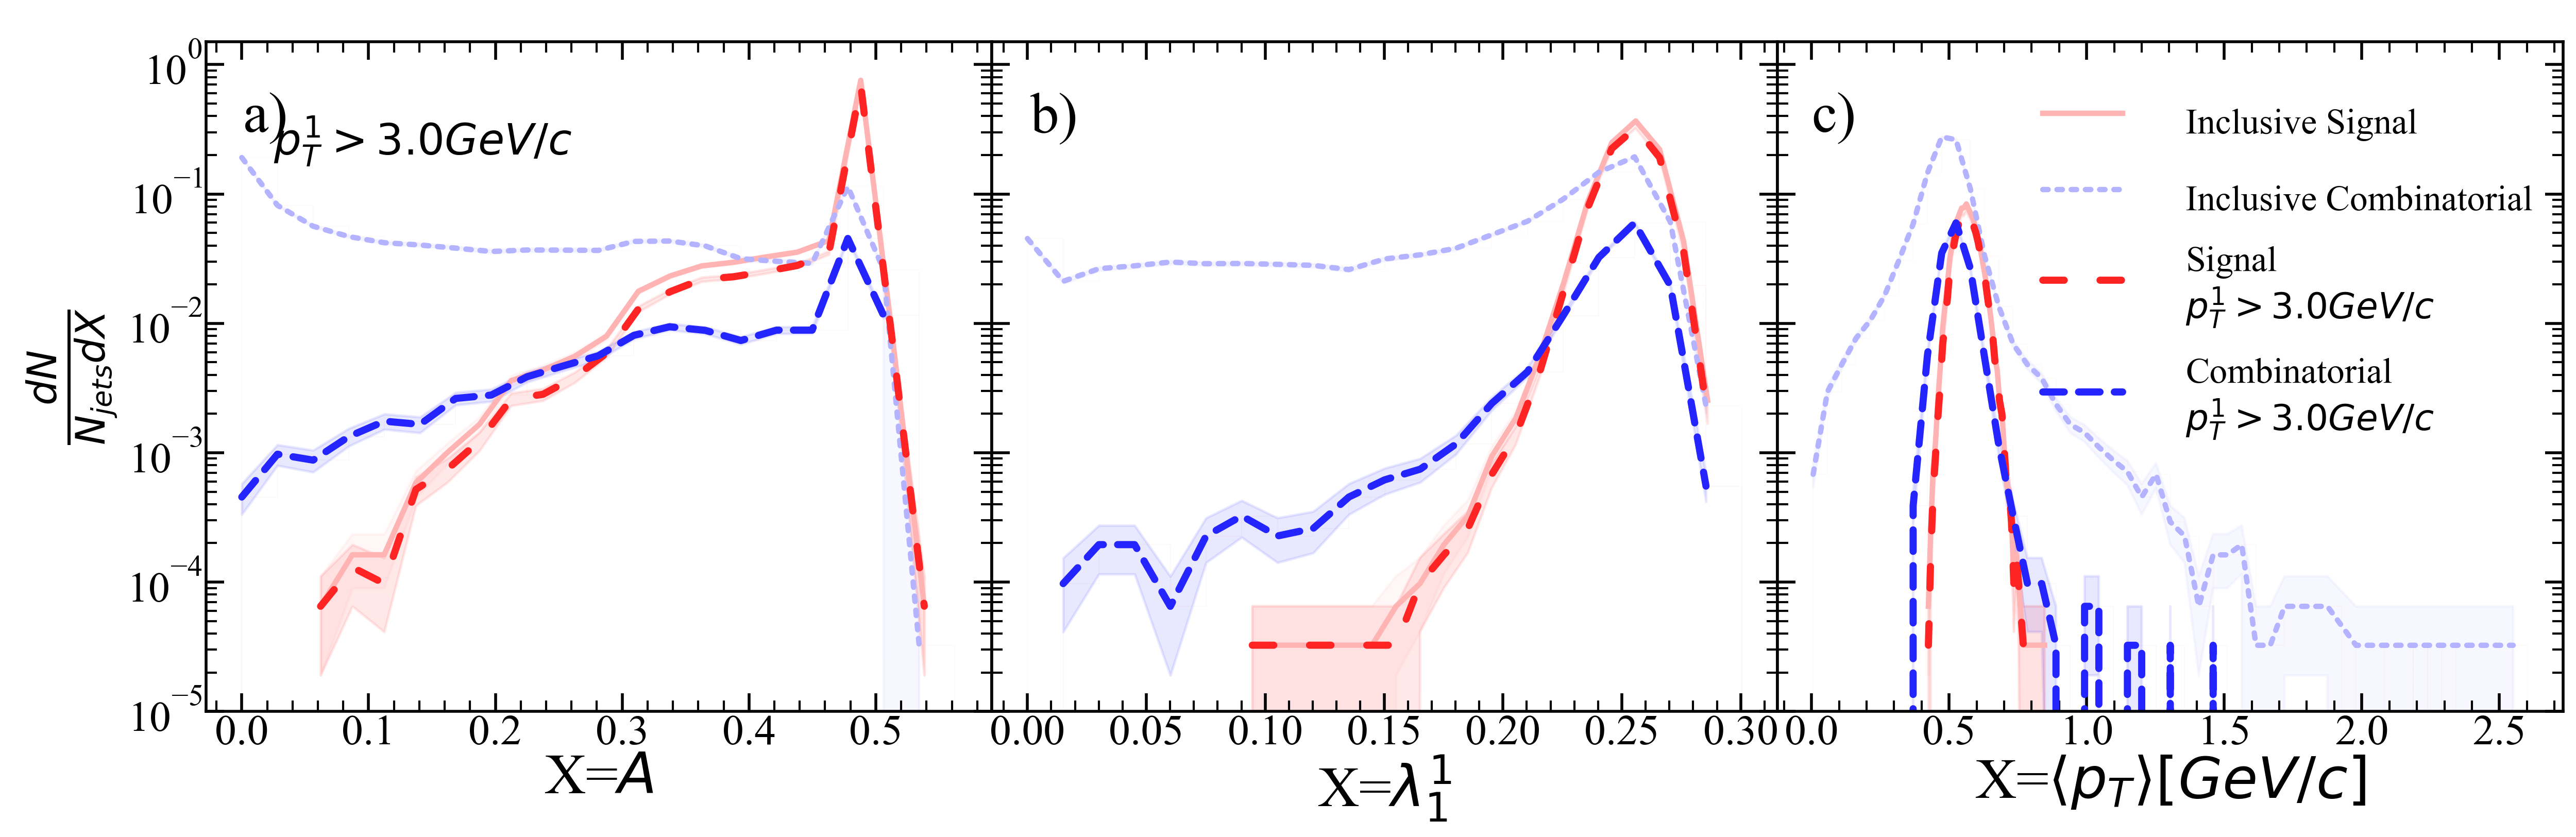}
    \caption{R=0.4 \ptH=10 \GeV}
    \label{fig:pT1_04_10}
\end{figure*}

\begin{figure*}
    \centering
    \includegraphics[width=\linewidth]{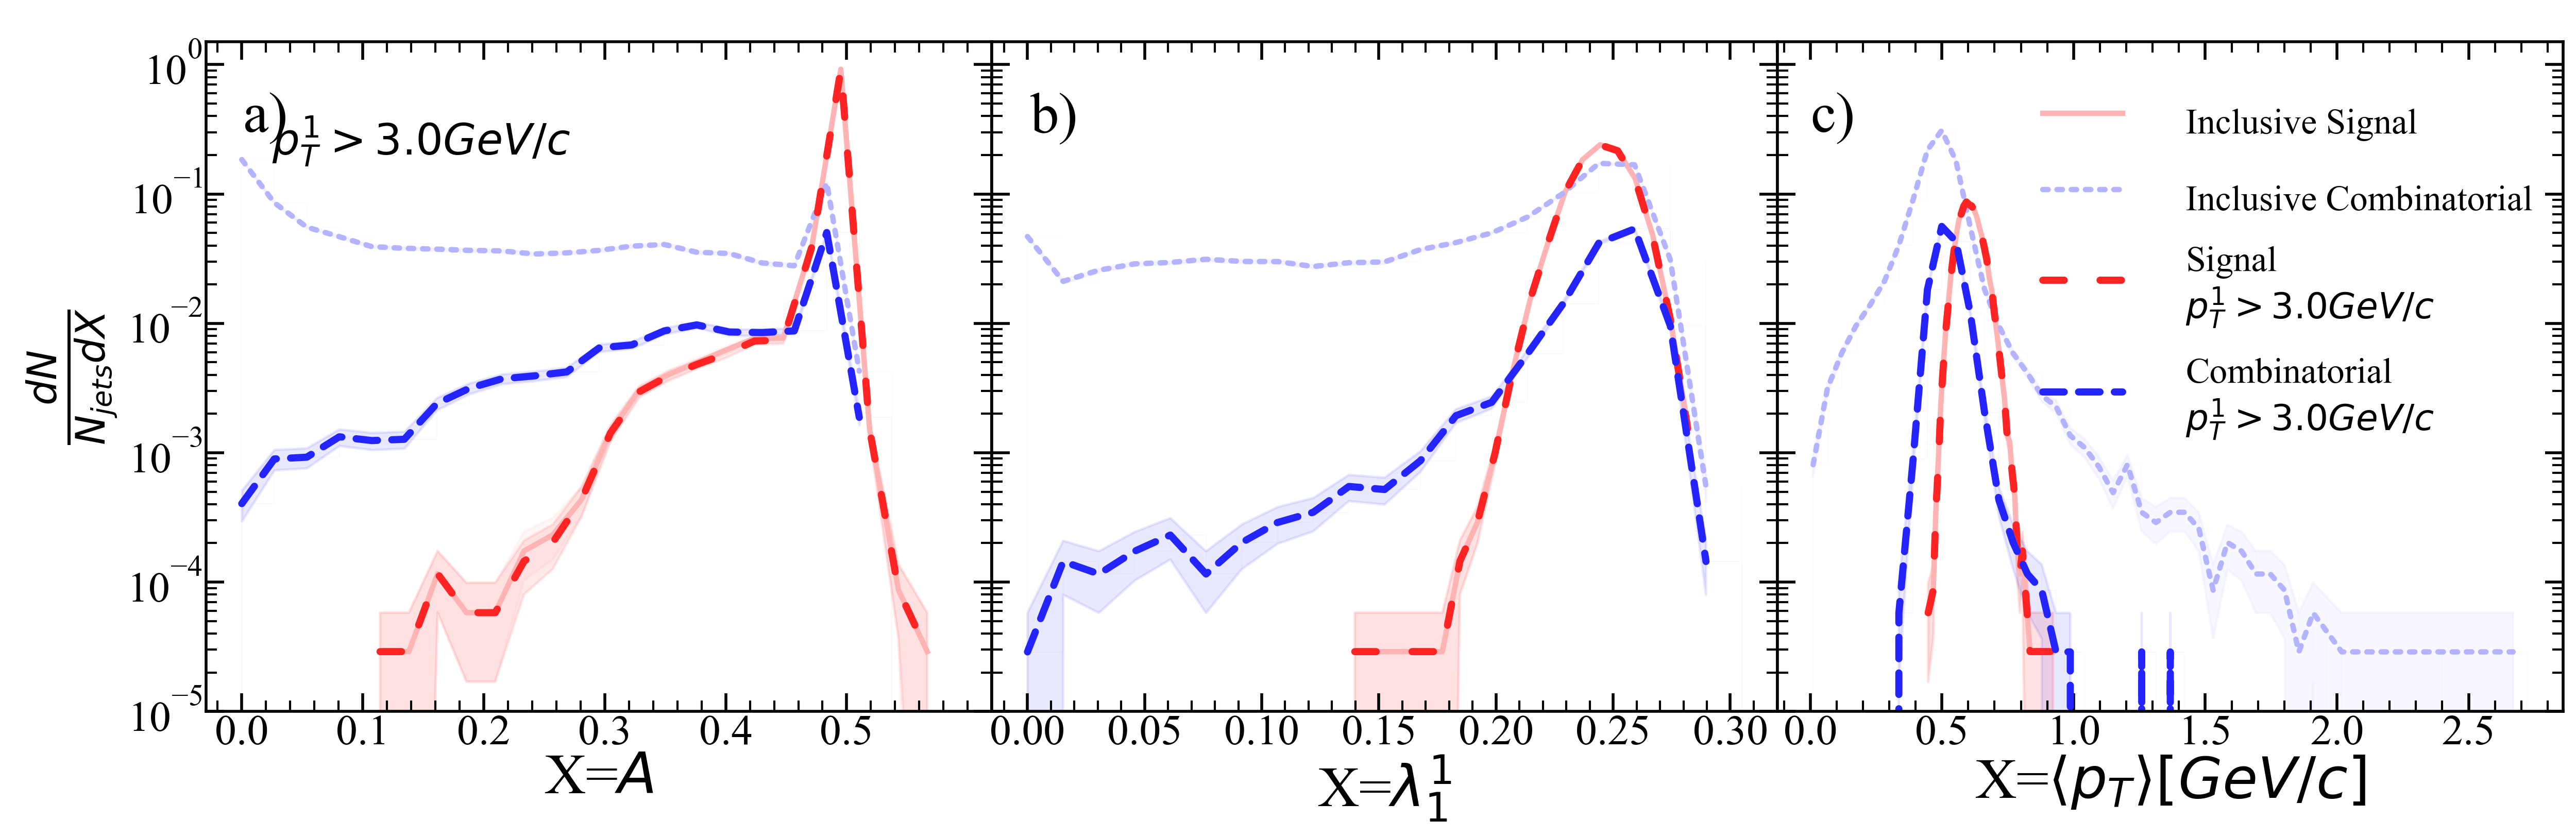}
    \caption{R=0.4 \ptH=20 \GeV}
    \label{fig:pT1_04_20}
\end{figure*}

\begin{figure*}
    \centering
    \includegraphics[width=\linewidth]{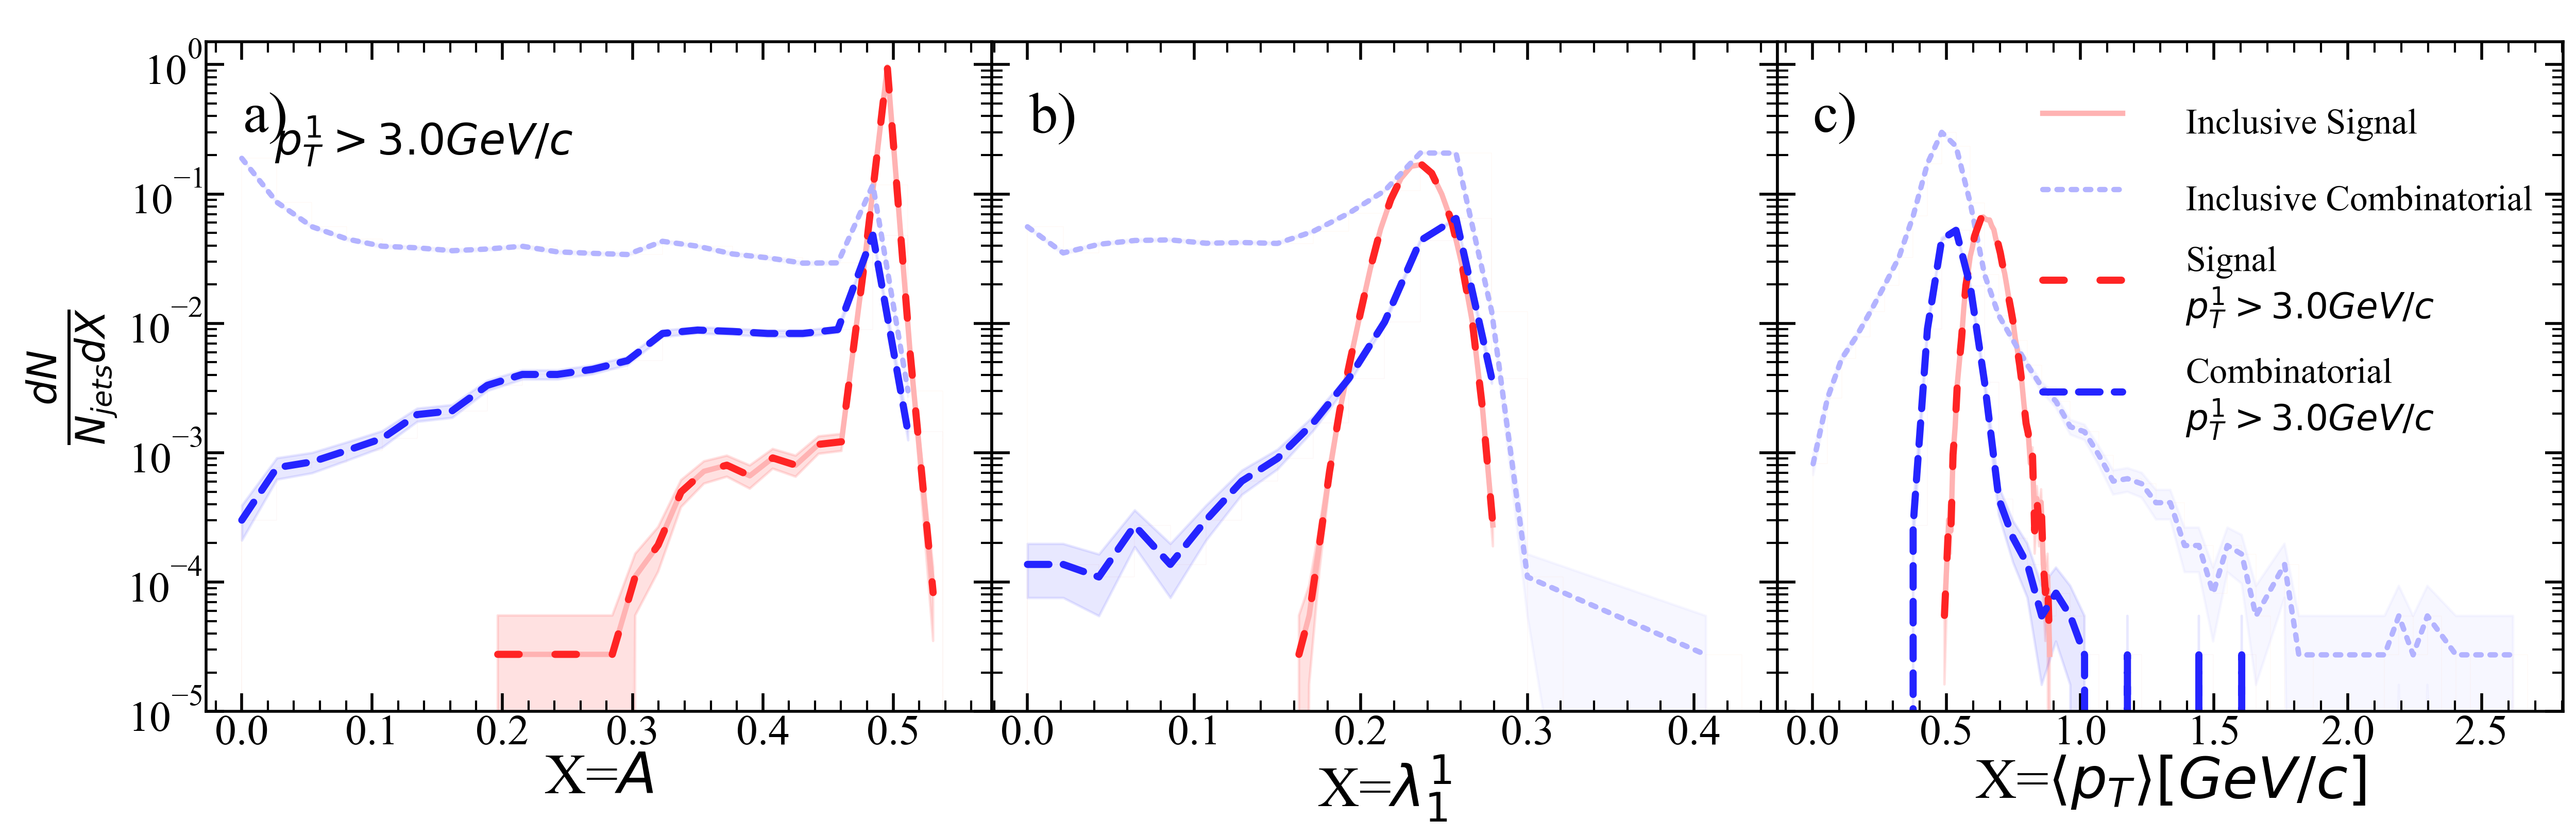}
    \caption{R=0.4 \ptH=30 \GeV}
    \label{fig:pT1_04_30}
\end{figure*}

\begin{figure*}
    \centering
    \includegraphics[width=\linewidth]{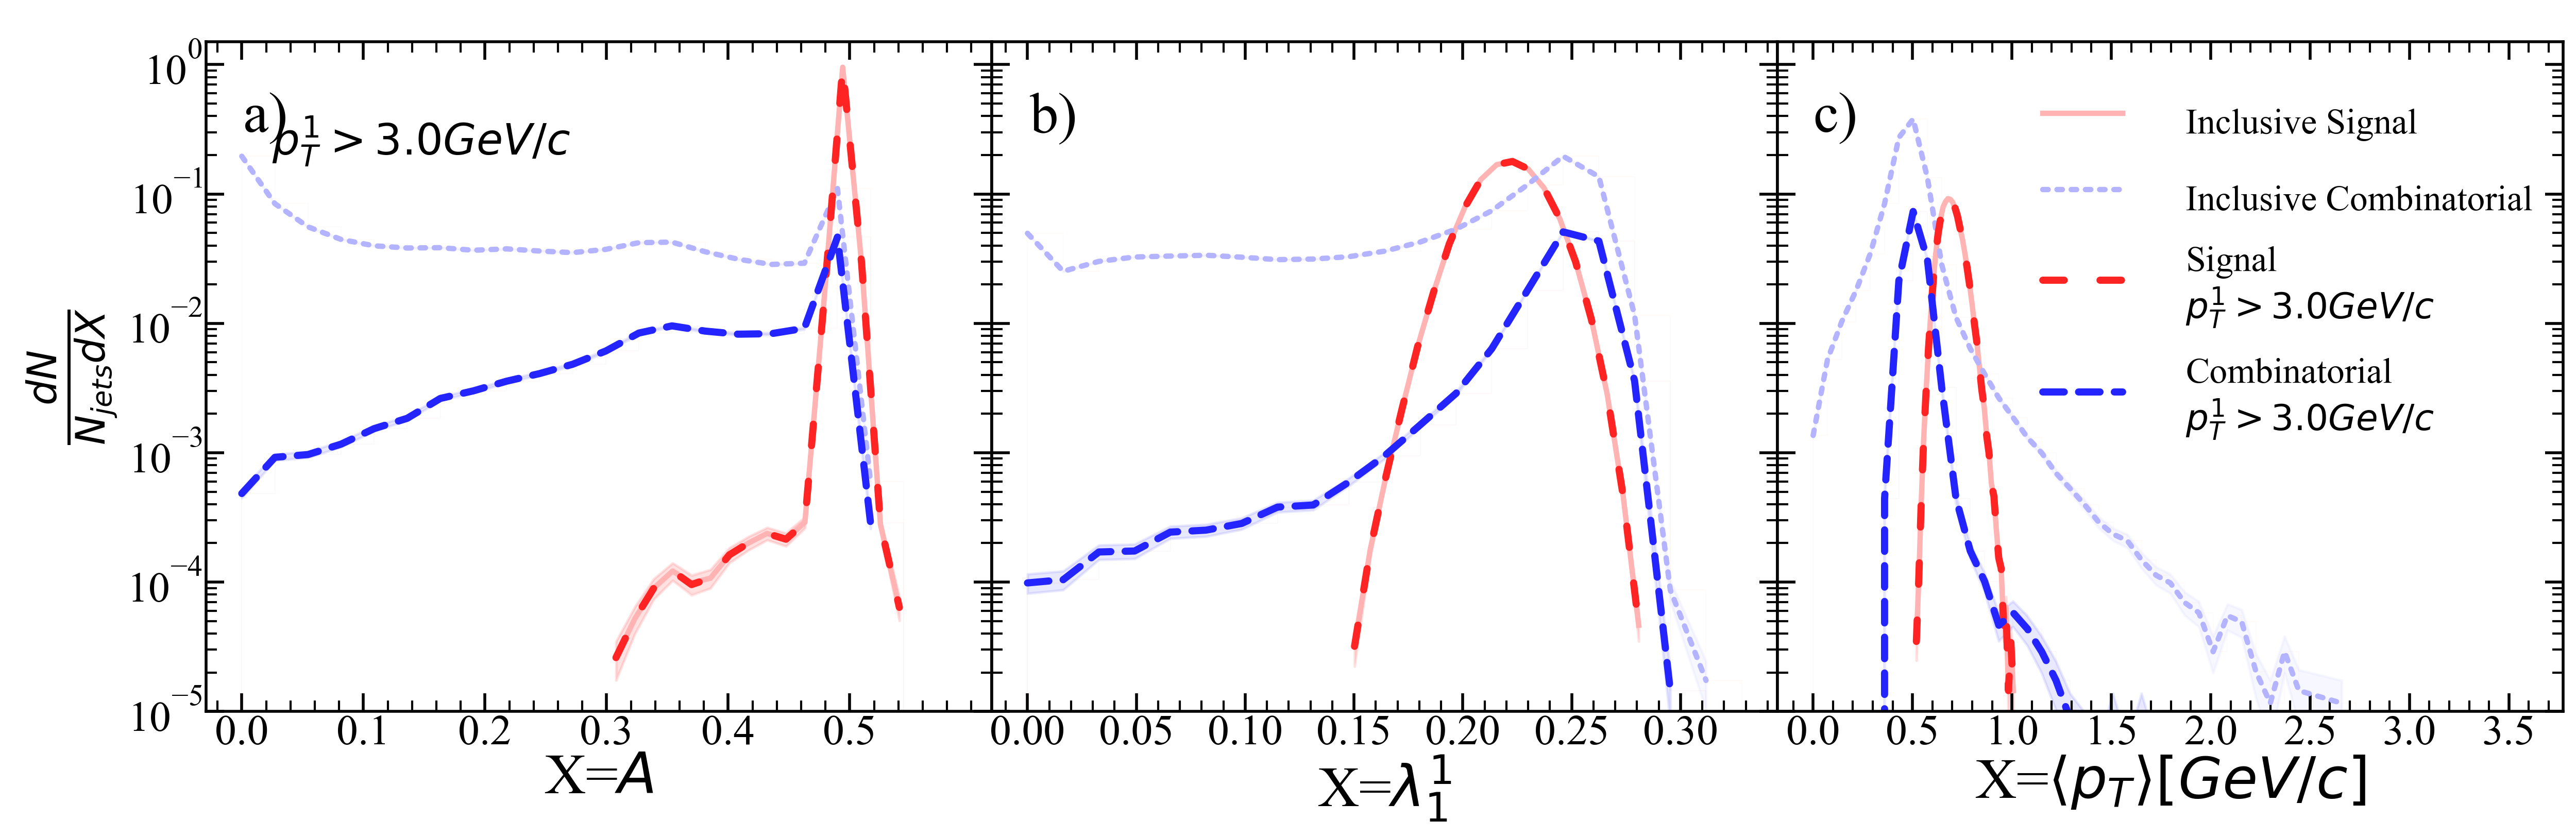}
    \caption{R=0.4 \ptH=40 \GeV}
    \label{fig:pT1_04_40}
\end{figure*}

\begin{figure*}
    \centering
    \includegraphics[width=\linewidth]{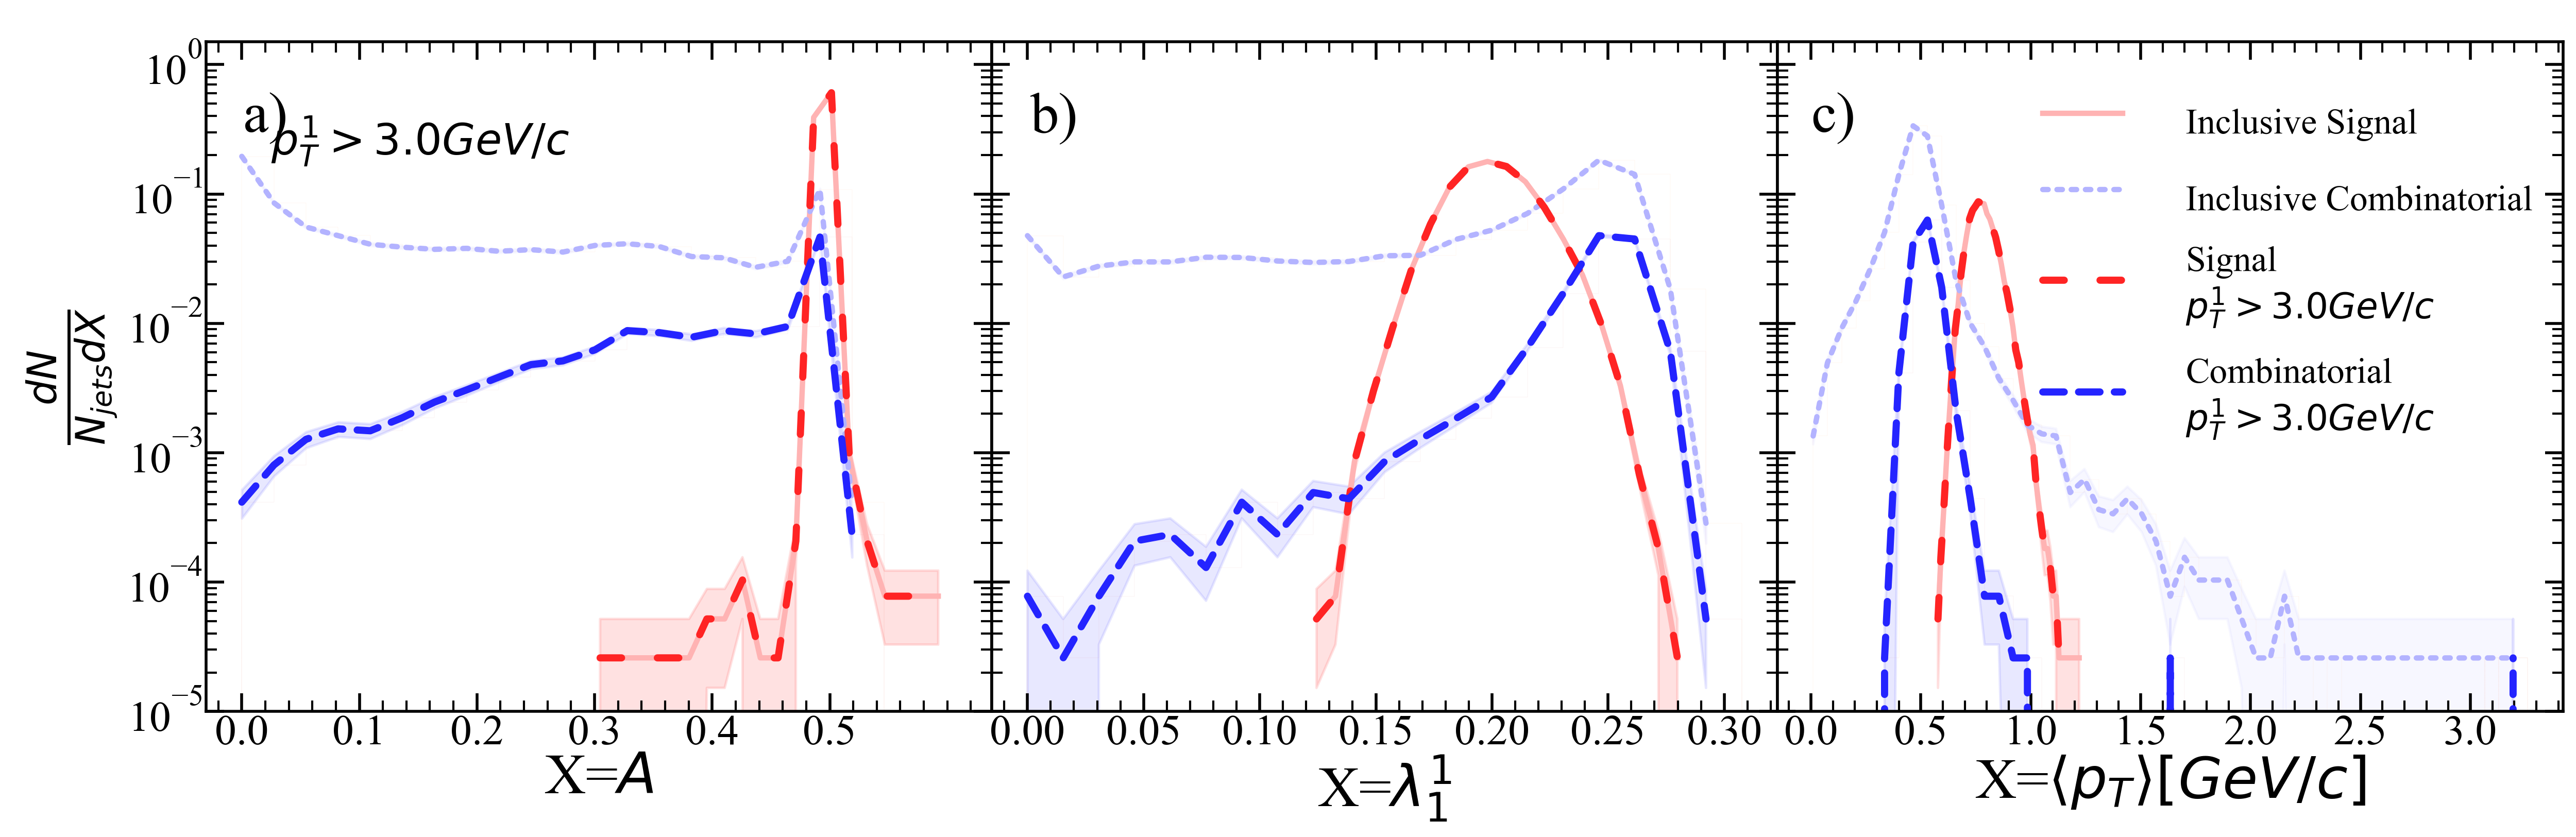}
    \caption{R=0.4 \ptH=60 \GeV}
    \label{fig:pT1_04_60}
\end{figure*}

\begin{figure*}
    \centering
    \includegraphics[width=\linewidth]{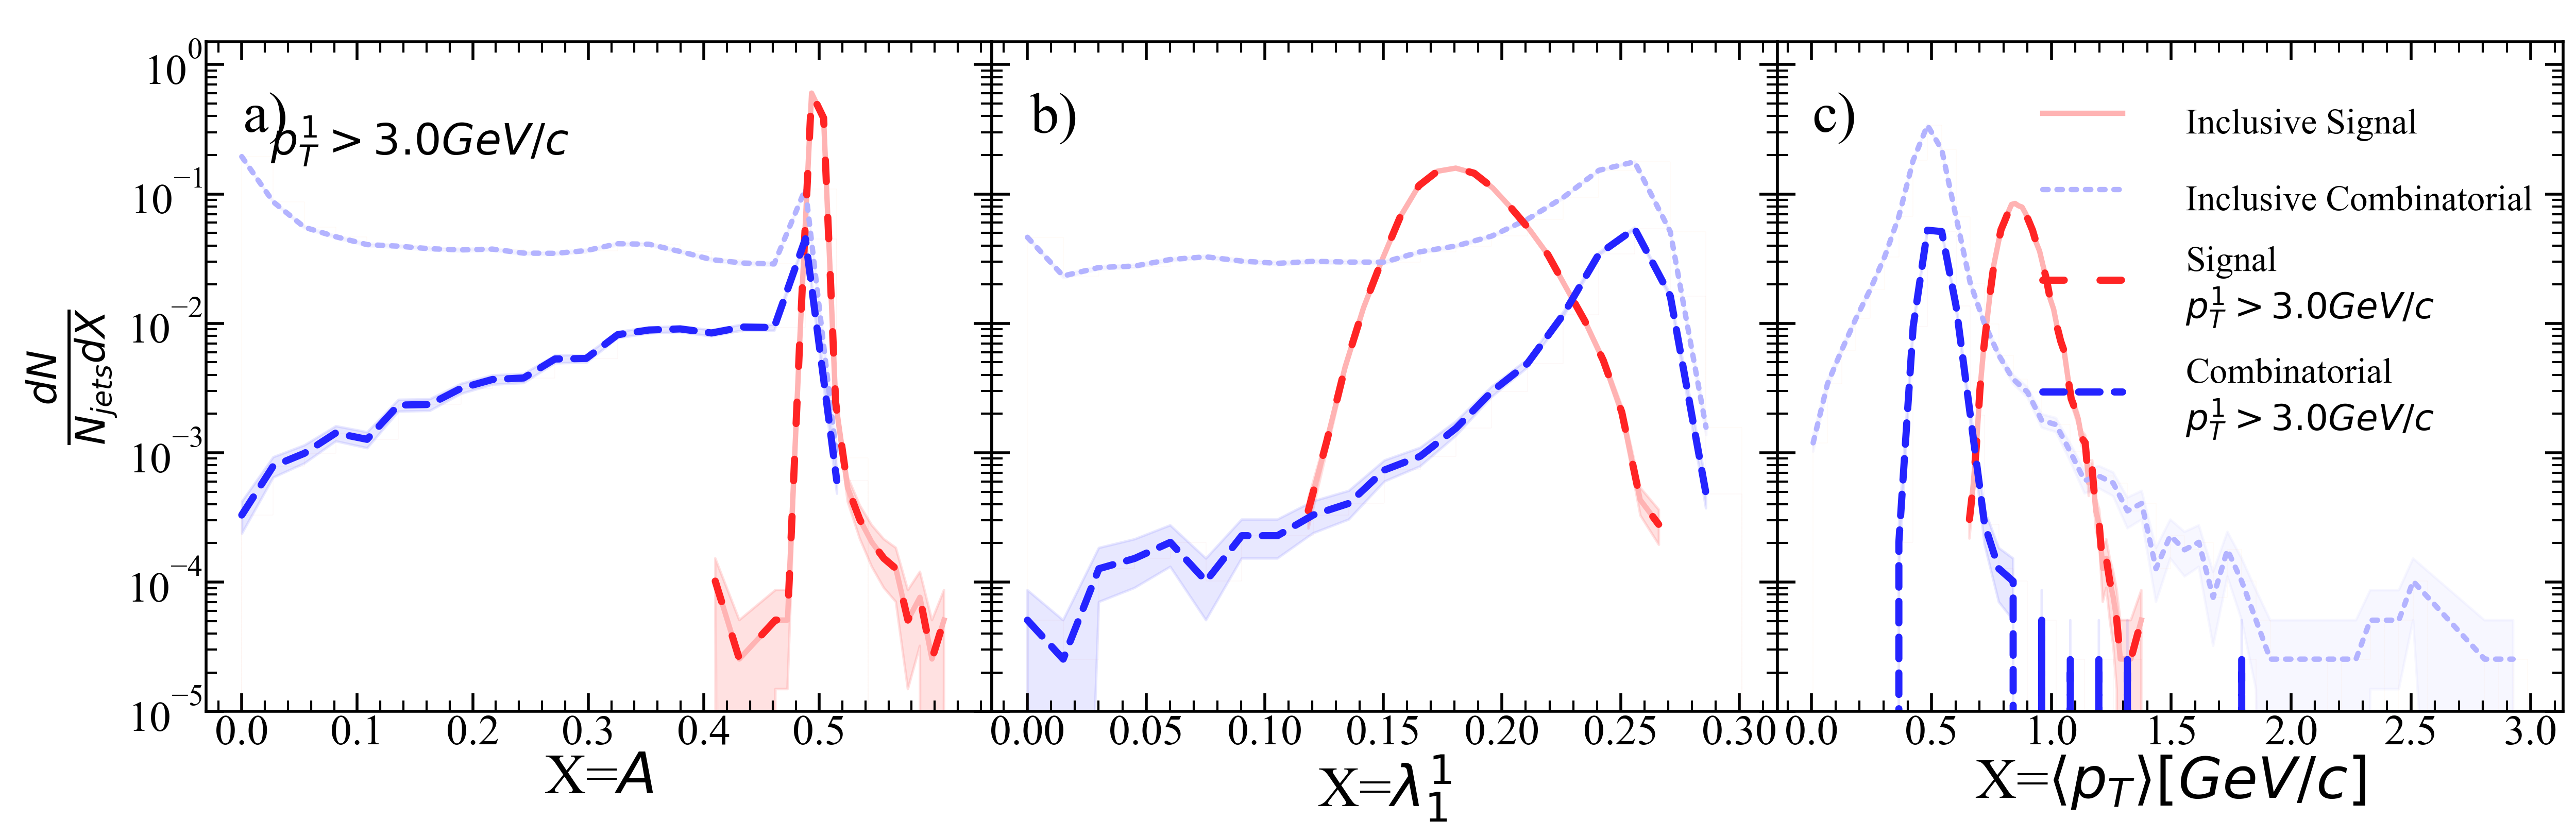}
    \caption{R=0.4 \ptH=80 \GeV}
    \label{fig:pT1_04_80}
\end{figure*}

\begin{figure*}
    \centering
    \includegraphics[width=\linewidth]{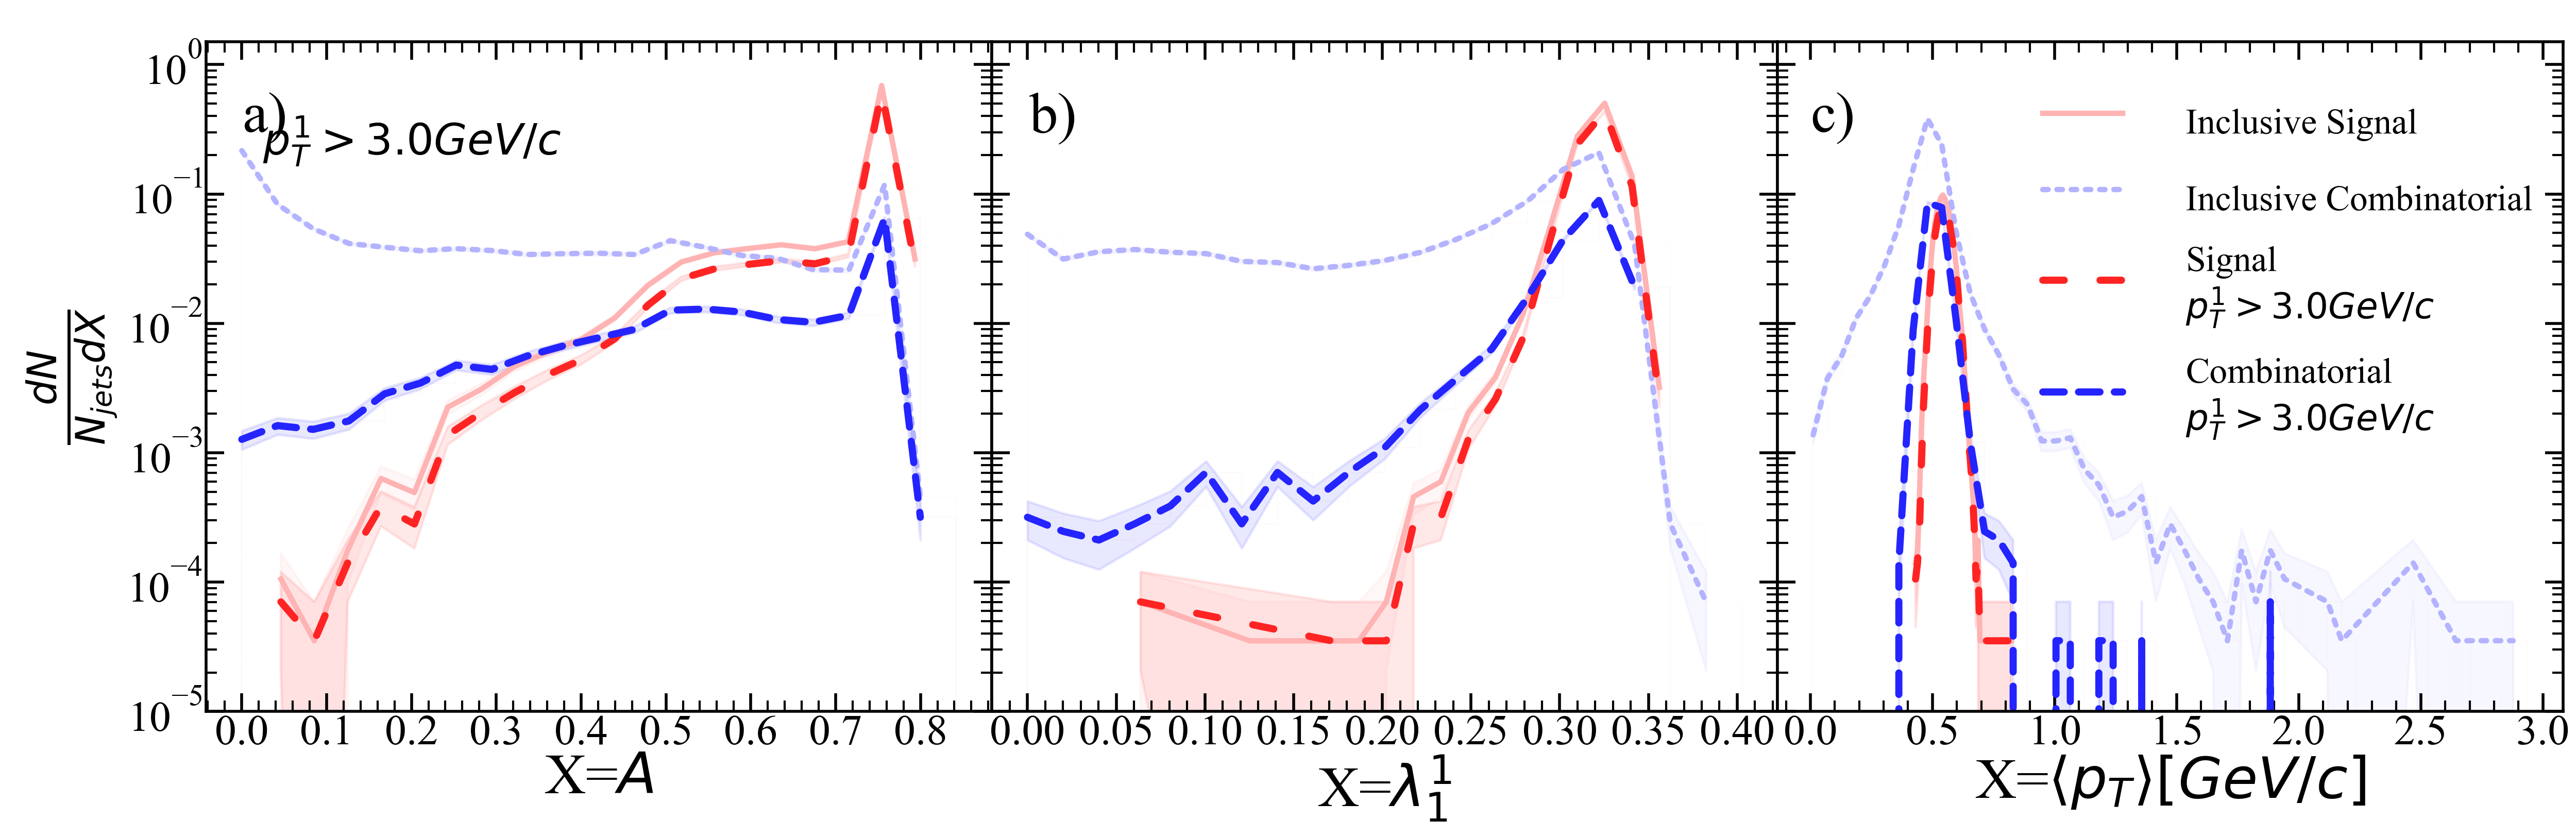}
    \caption{R=0.5 \ptH=10 \GeV}
    \label{fig:pT1_05_10}
\end{figure*}

\begin{figure*}
    \centering
    \includegraphics[width=\linewidth]{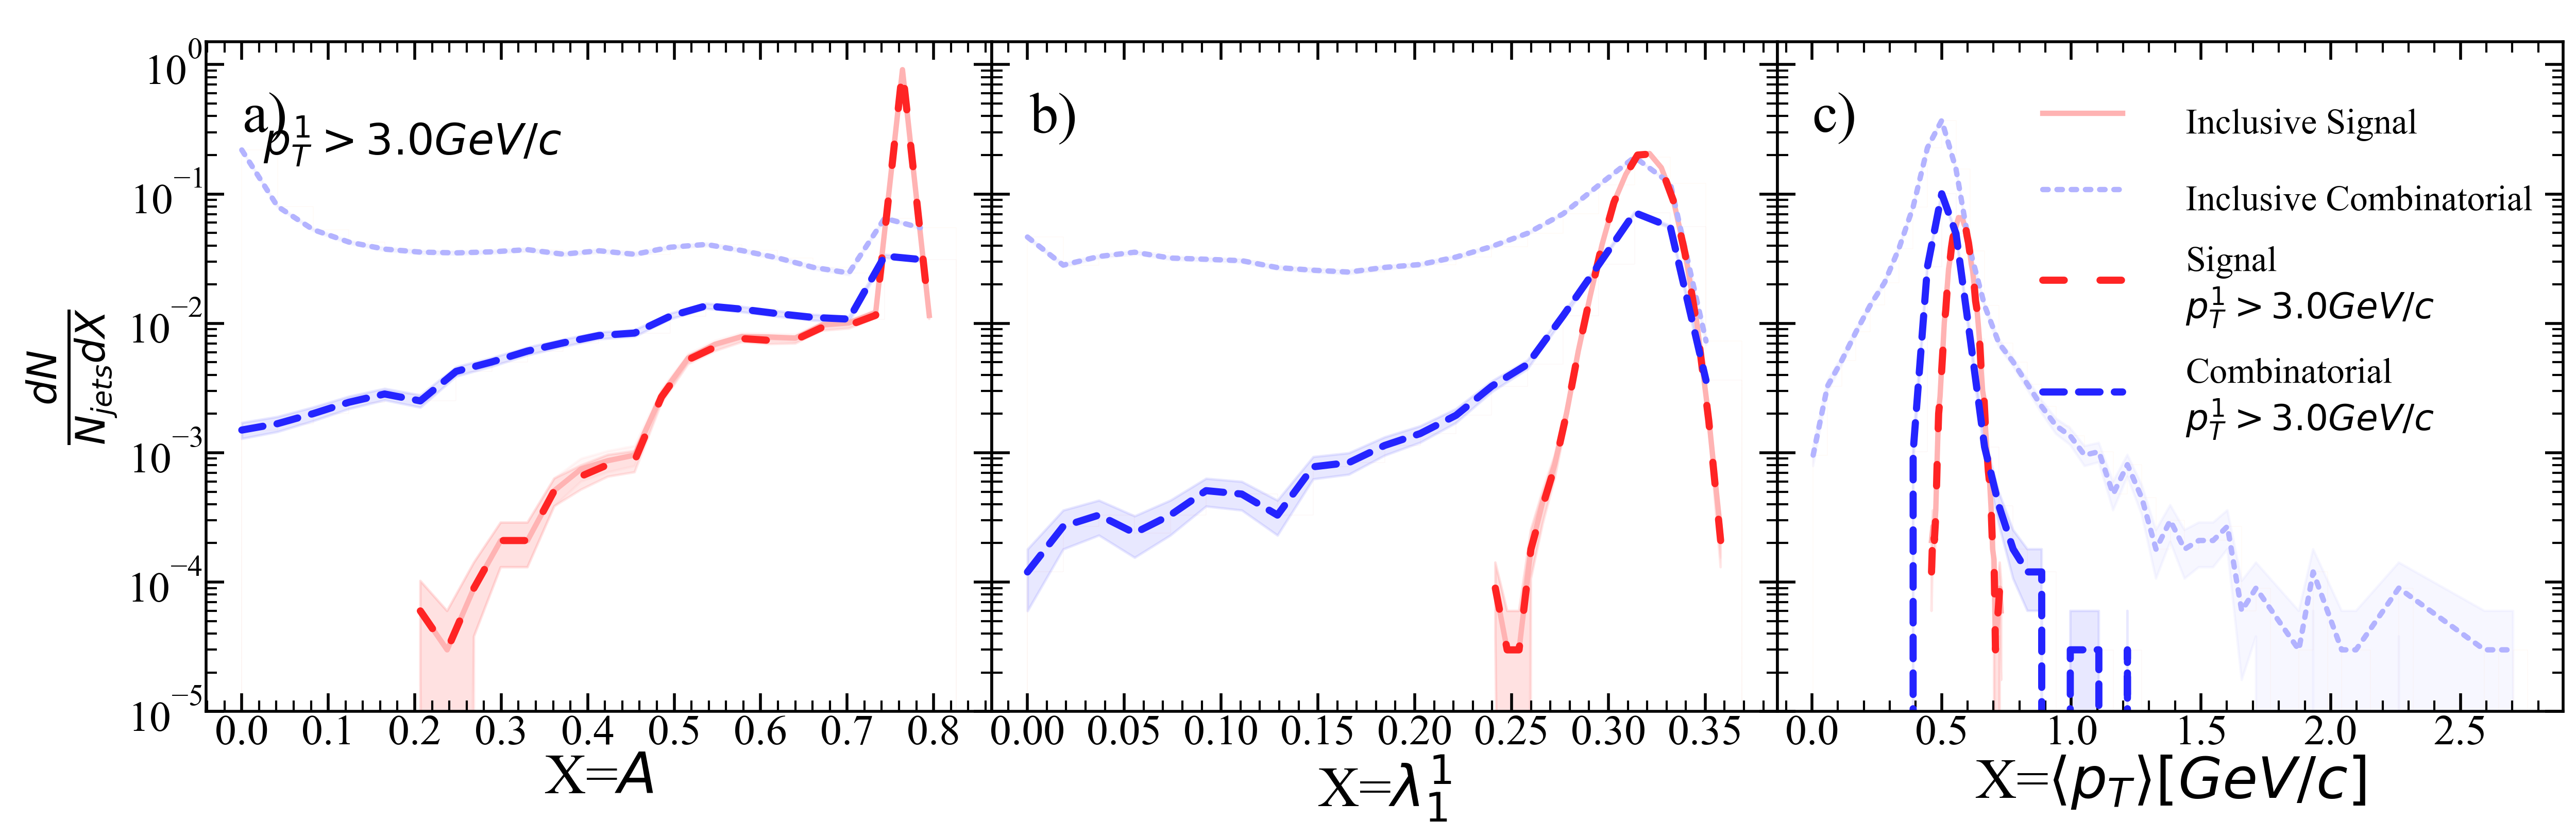}
    \caption{R=0.5 \ptH=20 \GeV}
    \label{fig:pT1_05_20}
\end{figure*}

\begin{figure*}
    \centering
    \includegraphics[width=\linewidth]{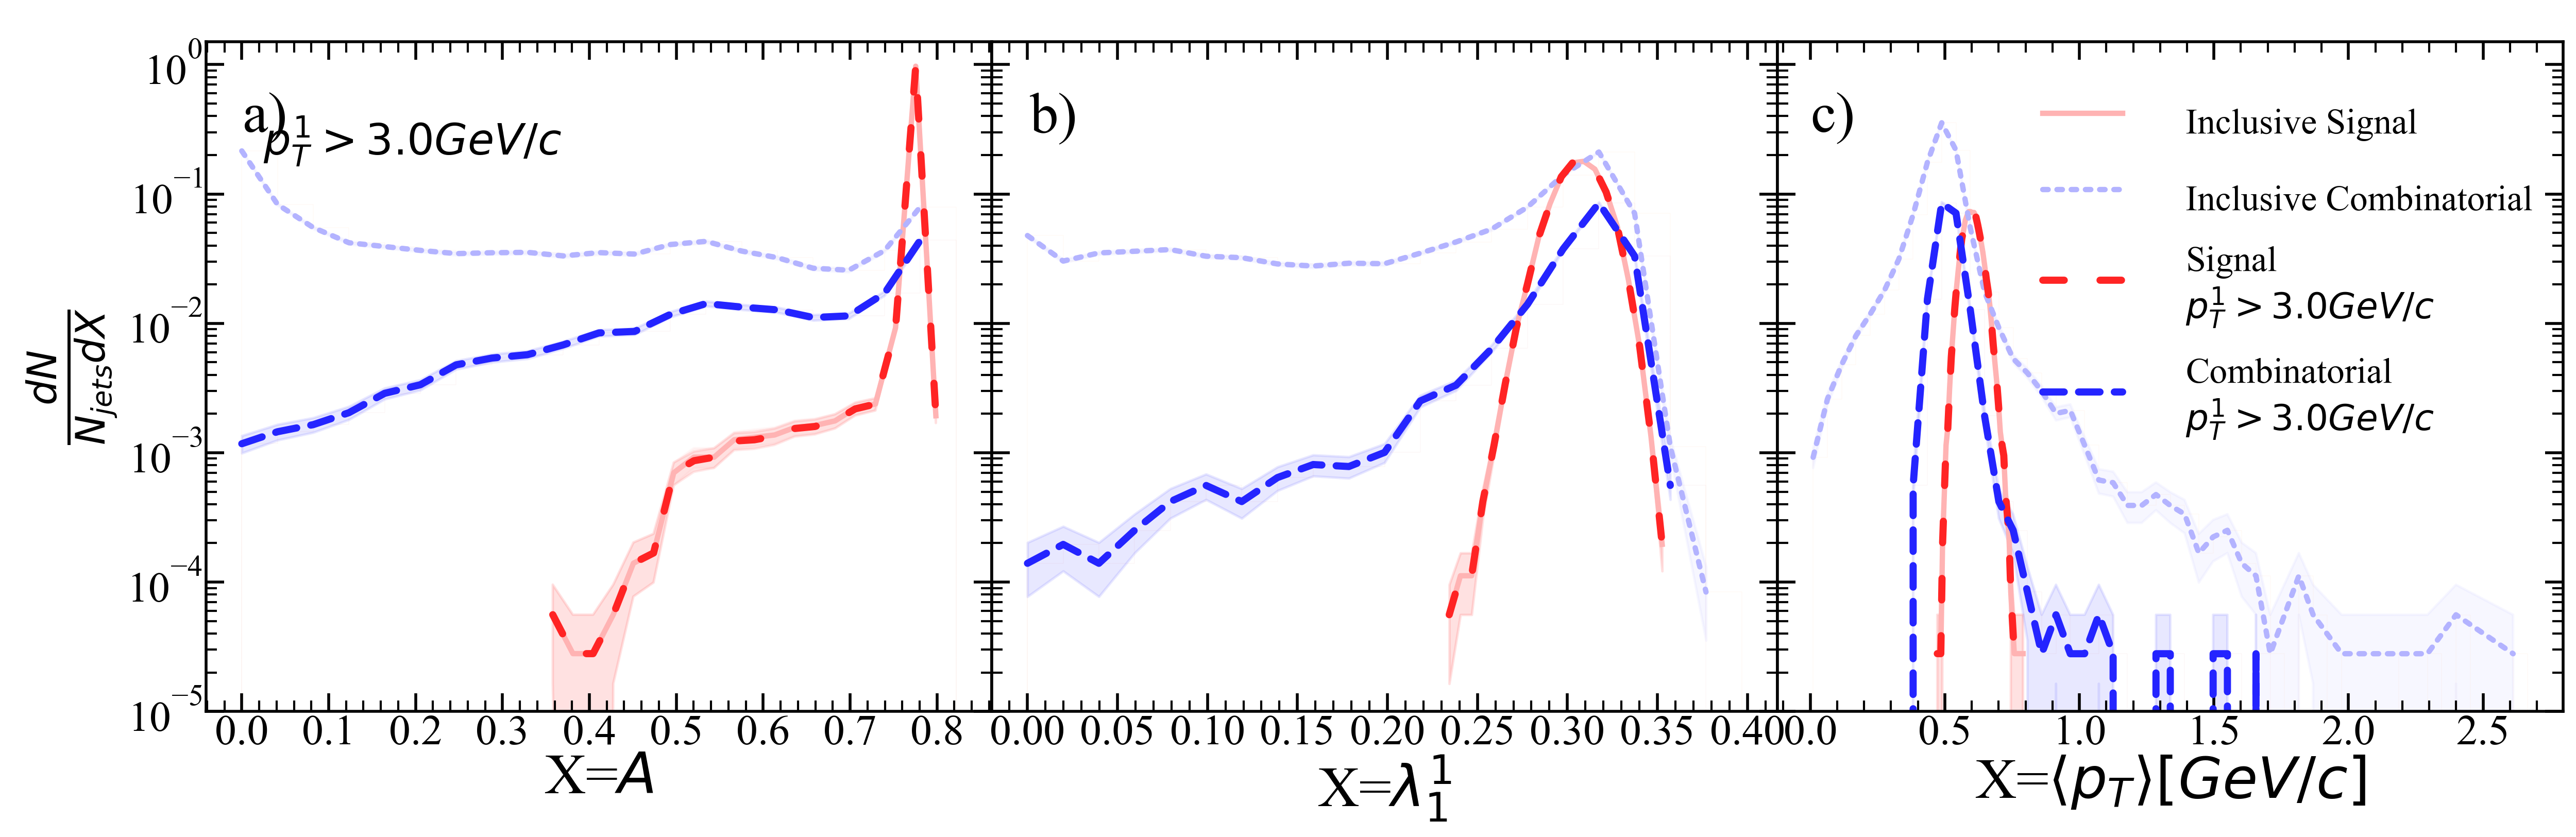}
    \caption{R=0.5 \ptH=30 \GeV}
    \label{fig:pT1_05_30}
\end{figure*}

\begin{figure*}
    \centering
    \includegraphics[width=\linewidth]{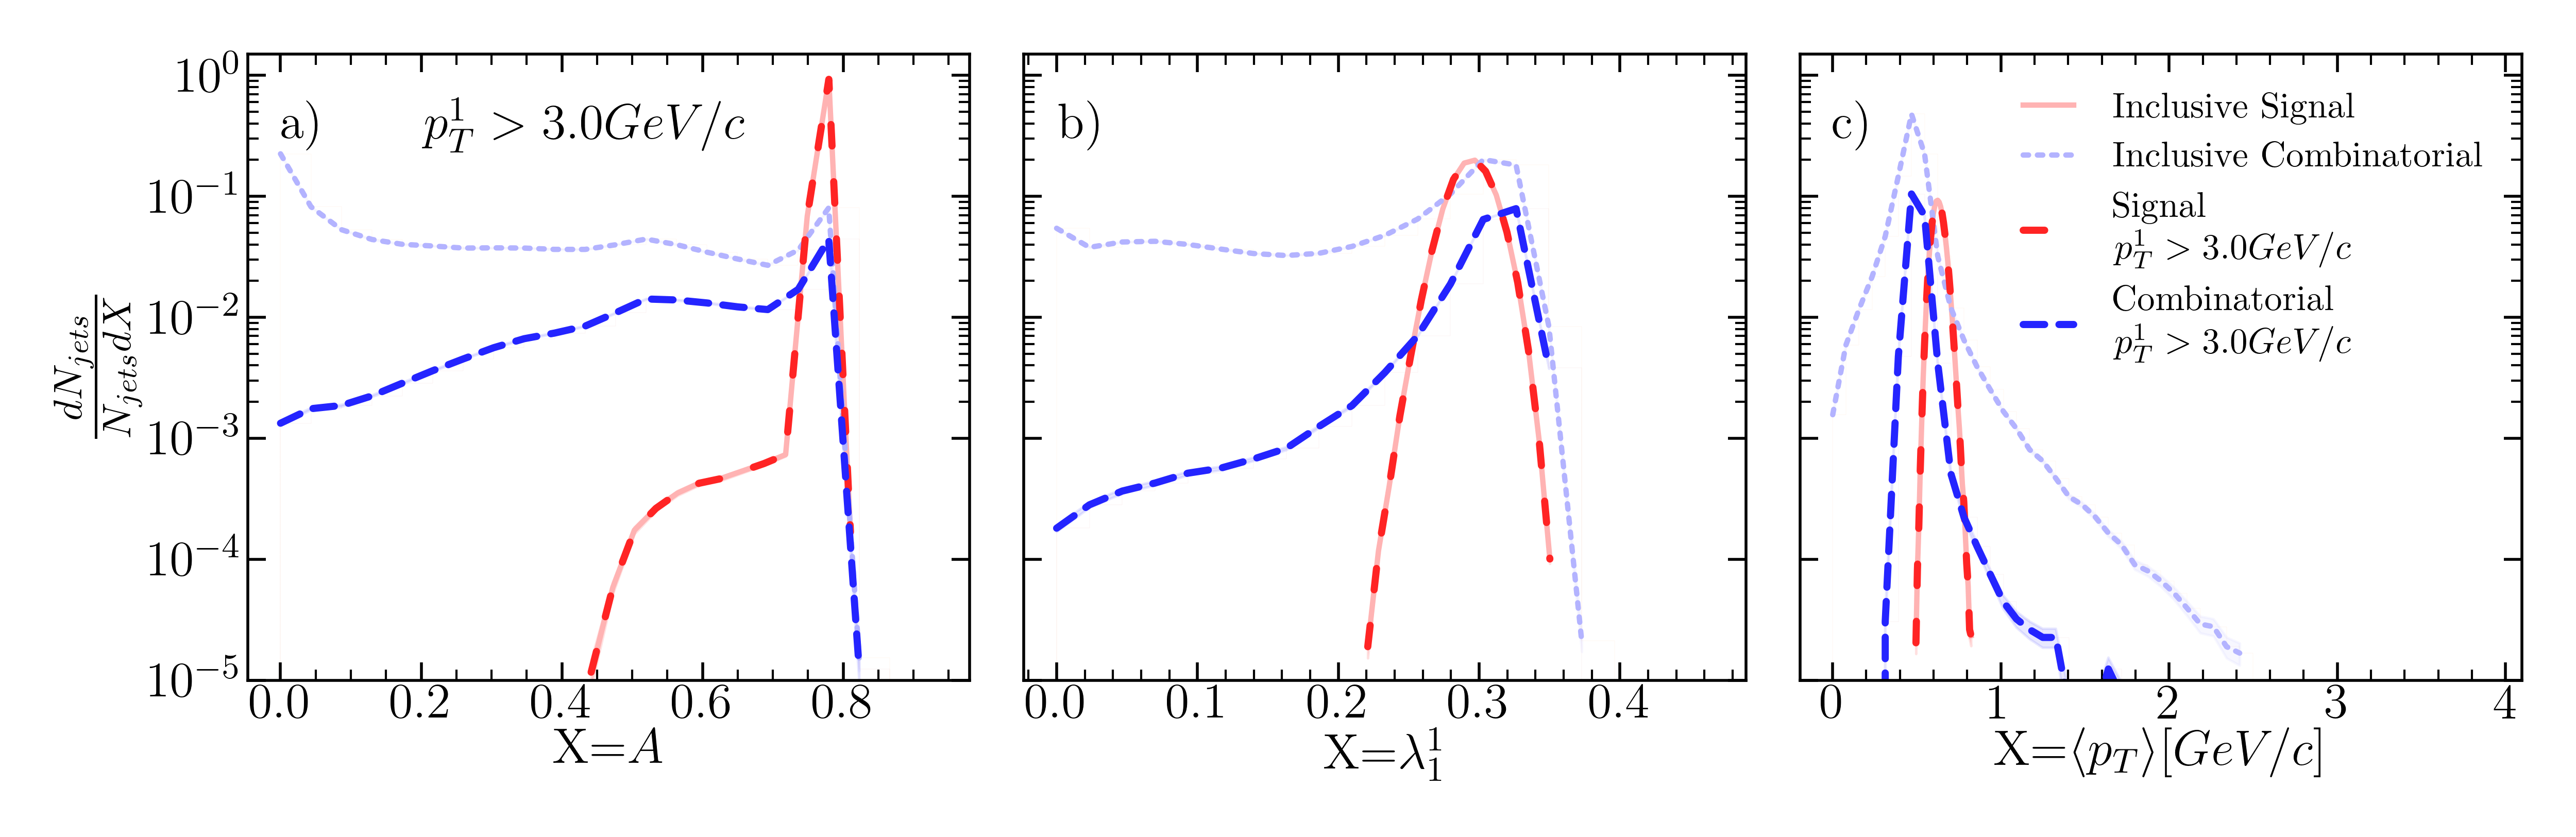}
    \caption{R=0.5 \ptH=40 \GeV}
    \label{fig:pT1_05_40}
\end{figure*}

\begin{figure*}
    \centering
    \includegraphics[width=\linewidth]{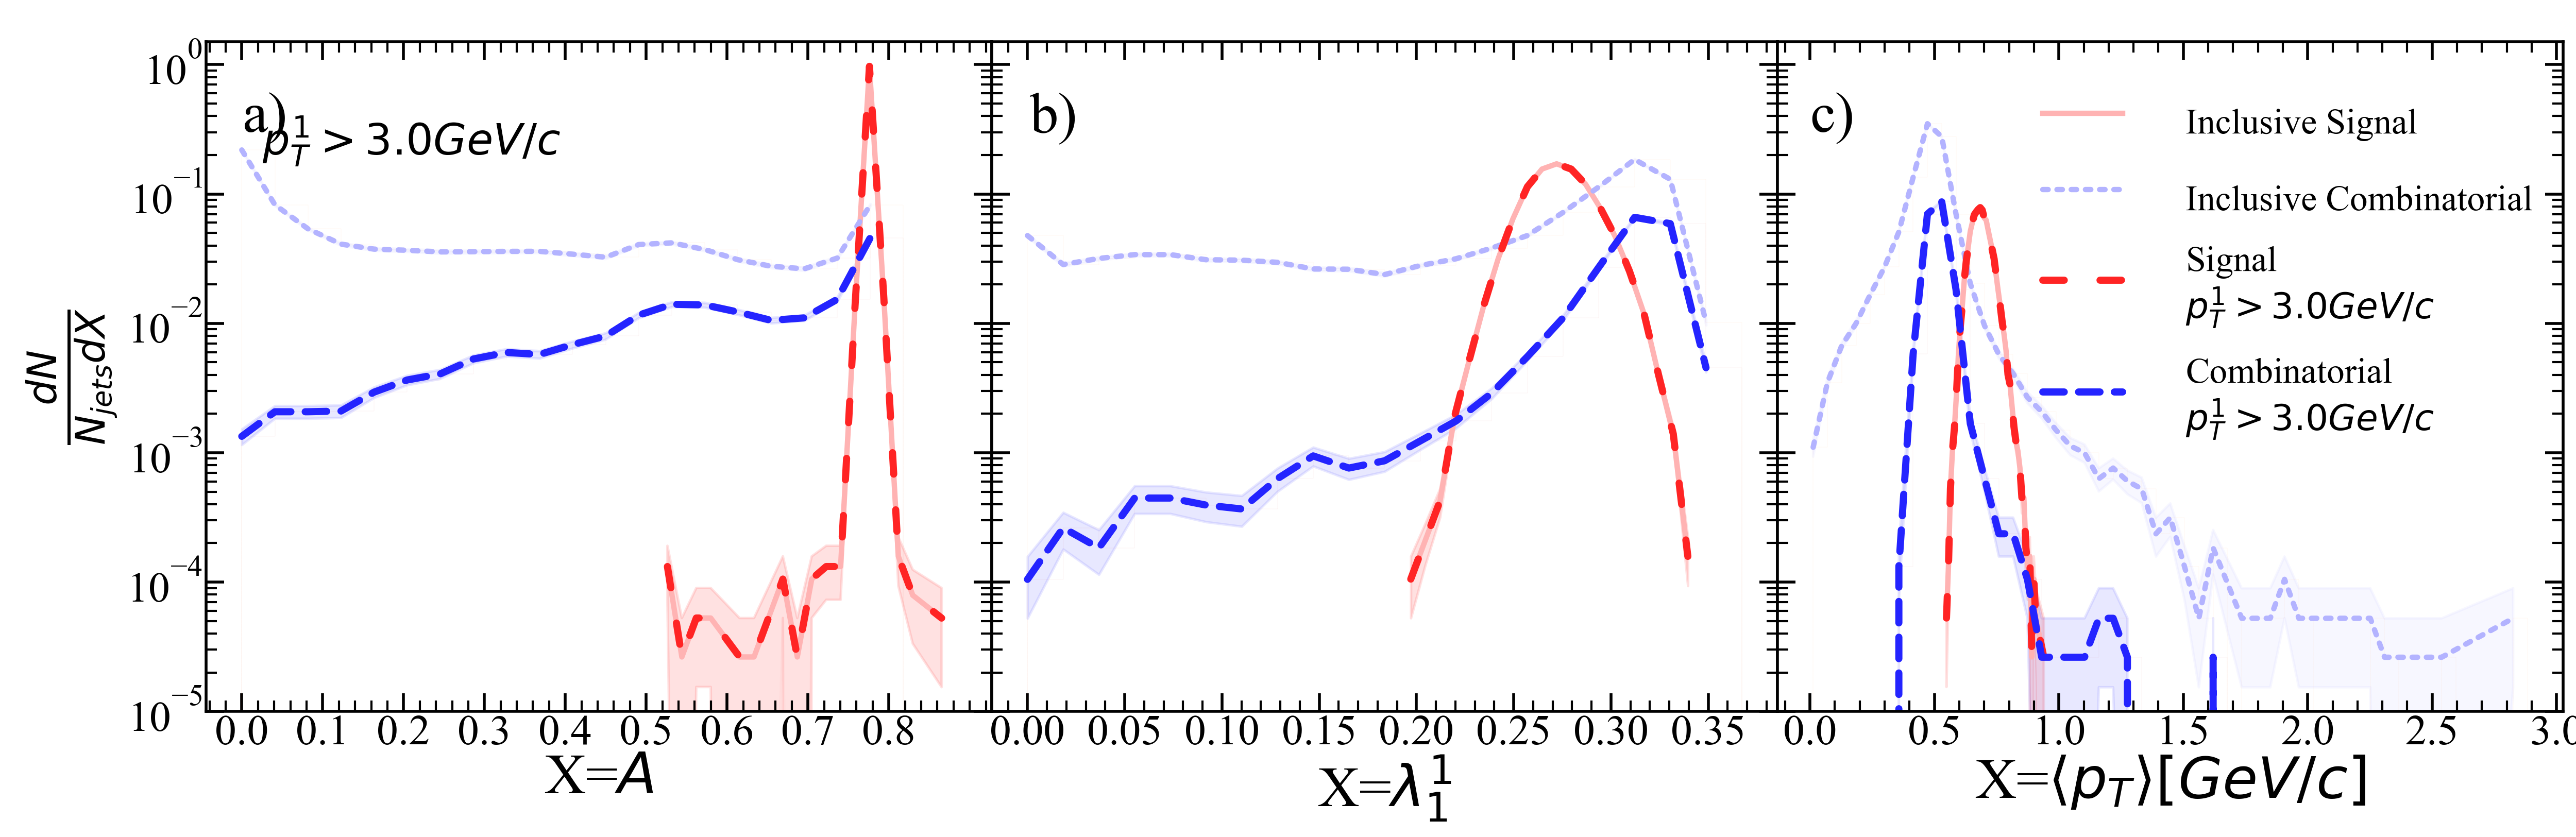}
    \caption{R=0.5 \ptH=60 \GeV}
    \label{fig:pT1_05_60}
\end{figure*}

\begin{figure*}
    \centering
    \includegraphics[width=\linewidth]{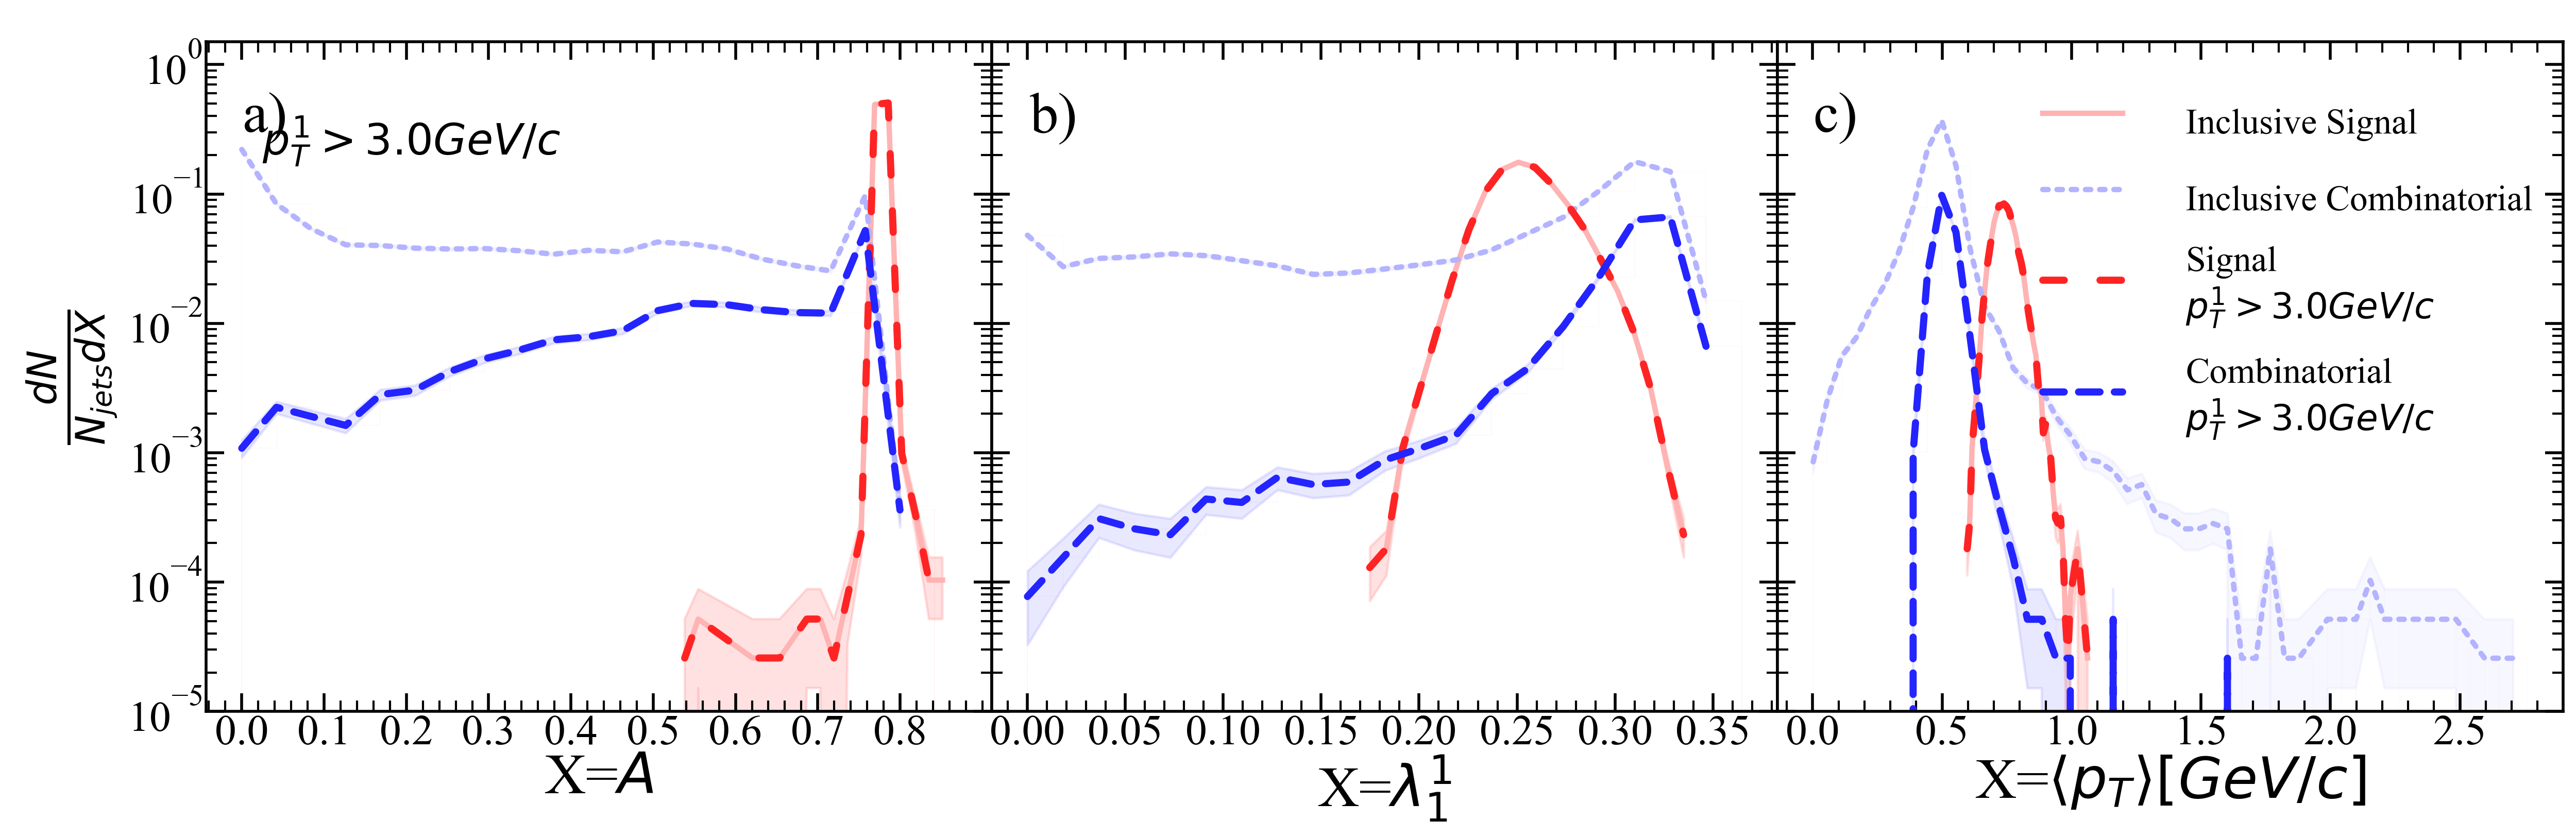}
    \caption{R=0.5 \ptH=80 \GeV}
    \label{fig:pT1_05_80}
\end{figure*}

\begin{figure*}
    \centering
    \includegraphics[width=\linewidth]{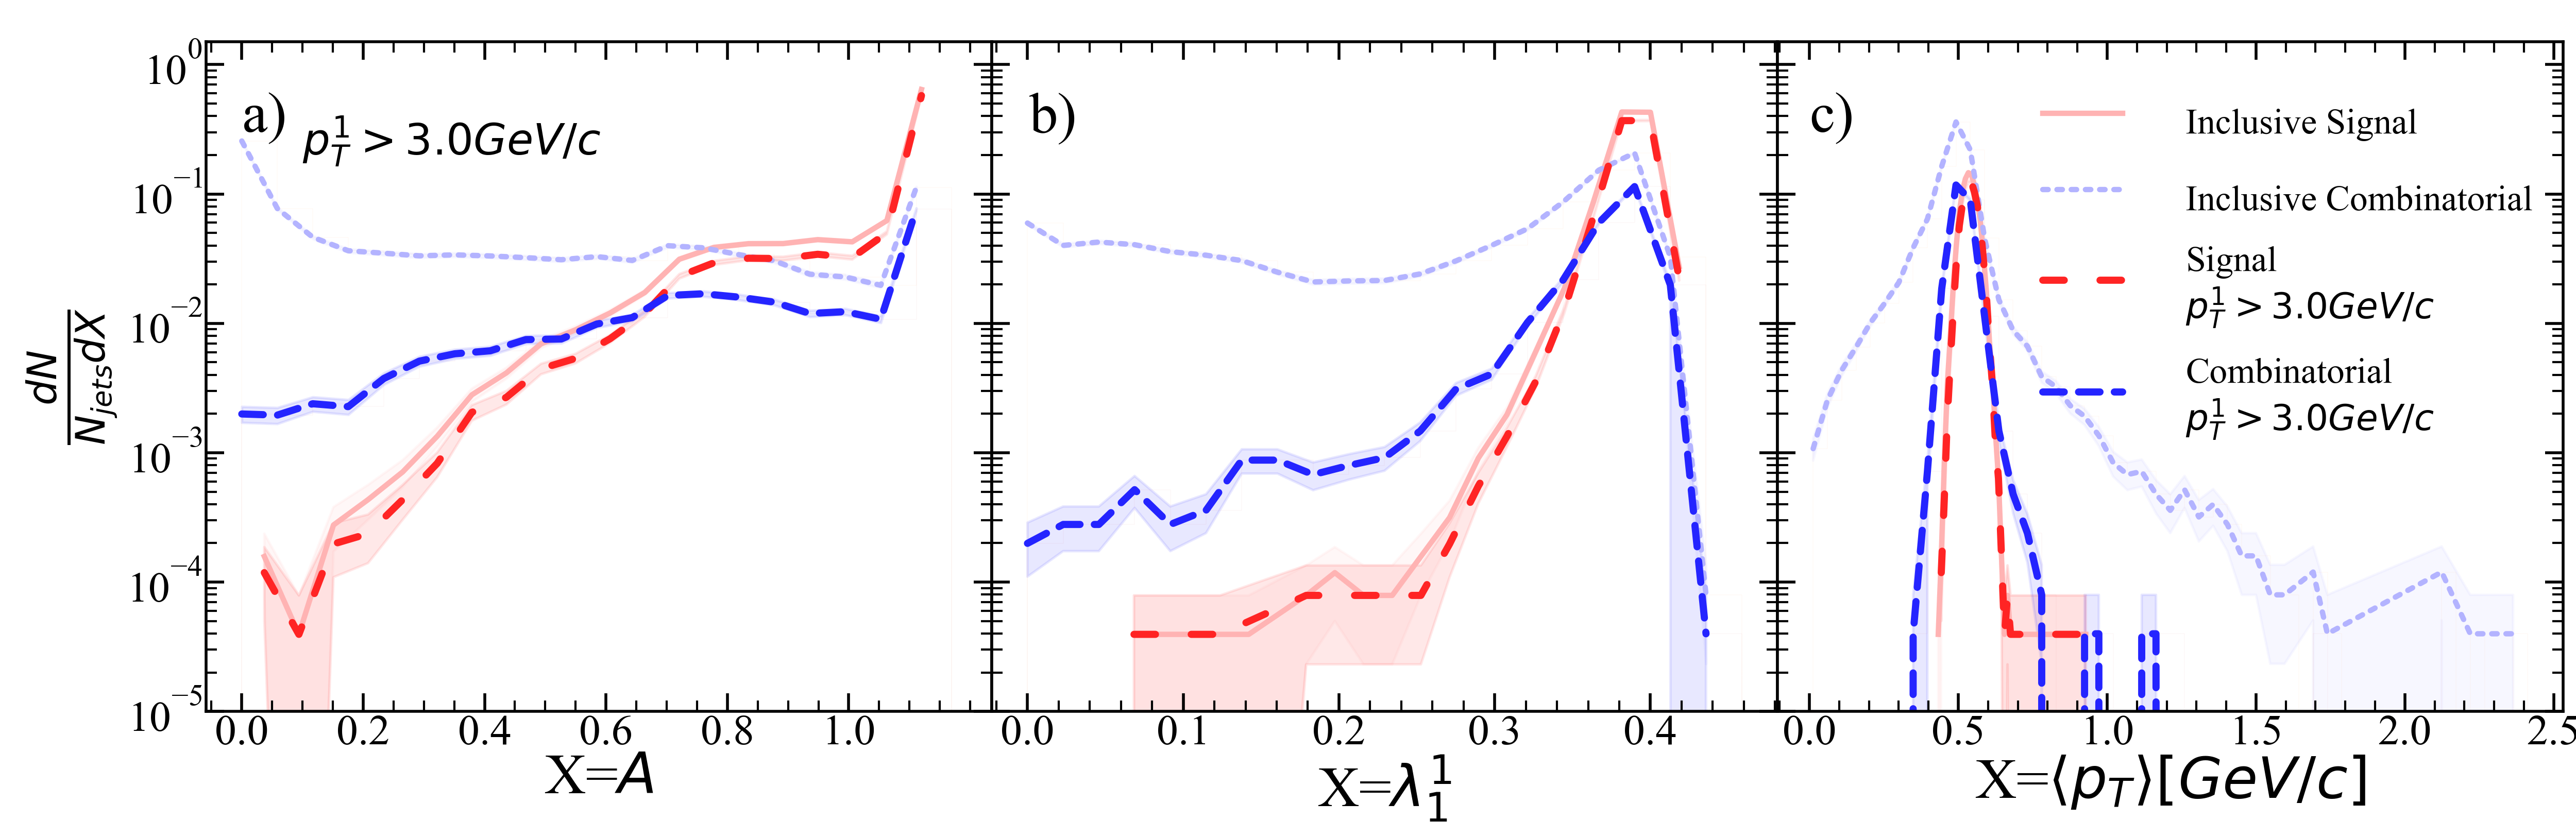}
    \caption{R=0.6 \ptH=10 \GeV}
    \label{fig:pT1_06_10}
\end{figure*}

\begin{figure*}
    \centering
    \includegraphics[width=\linewidth]{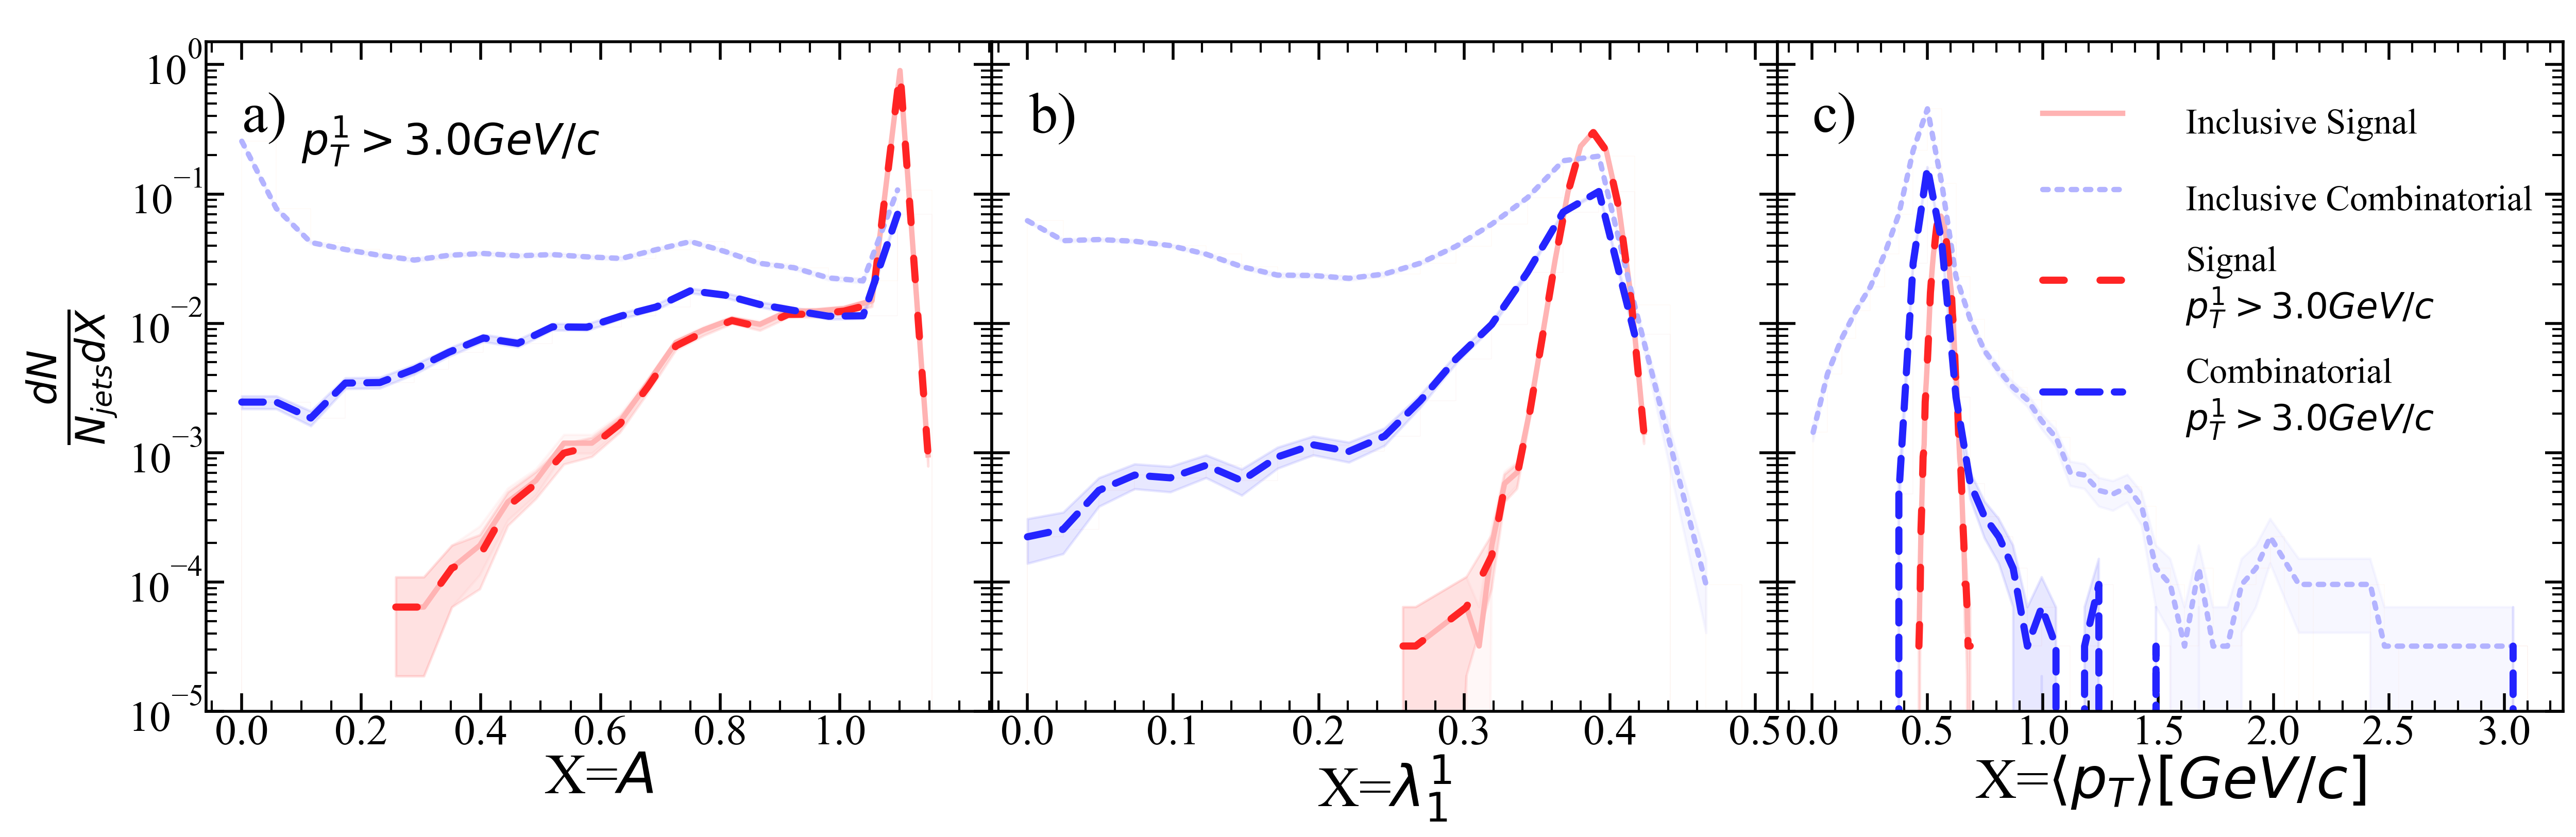}
    \caption{R=0.6 \ptH=20 \GeV}
    \label{fig:pT1_06_20}
\end{figure*}

\begin{figure*}
    \centering
    \includegraphics[width=\linewidth]{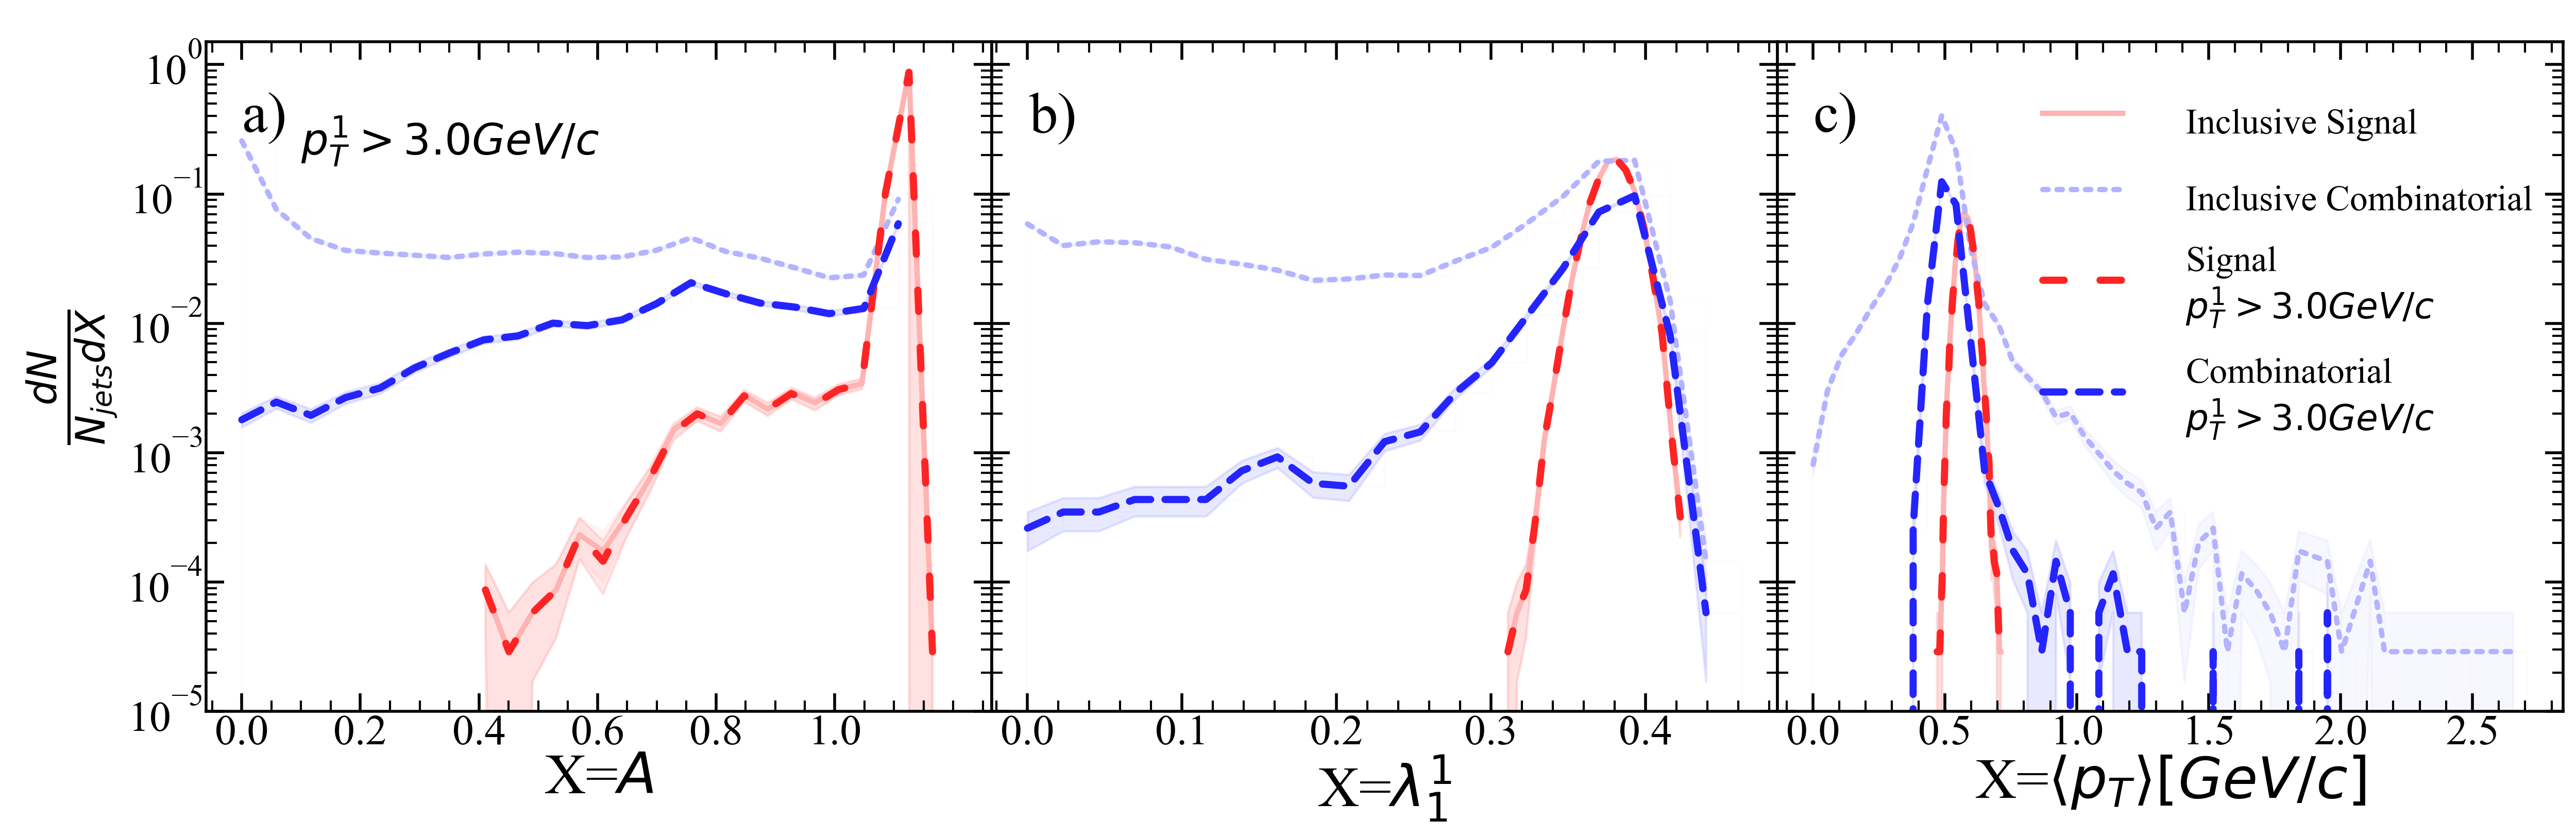}
    \caption{R=0.6 \ptH=30 \GeV}
    \label{fig:pT1_06_30}
\end{figure*}

\begin{figure*}
    \centering
    \includegraphics[width=\linewidth]{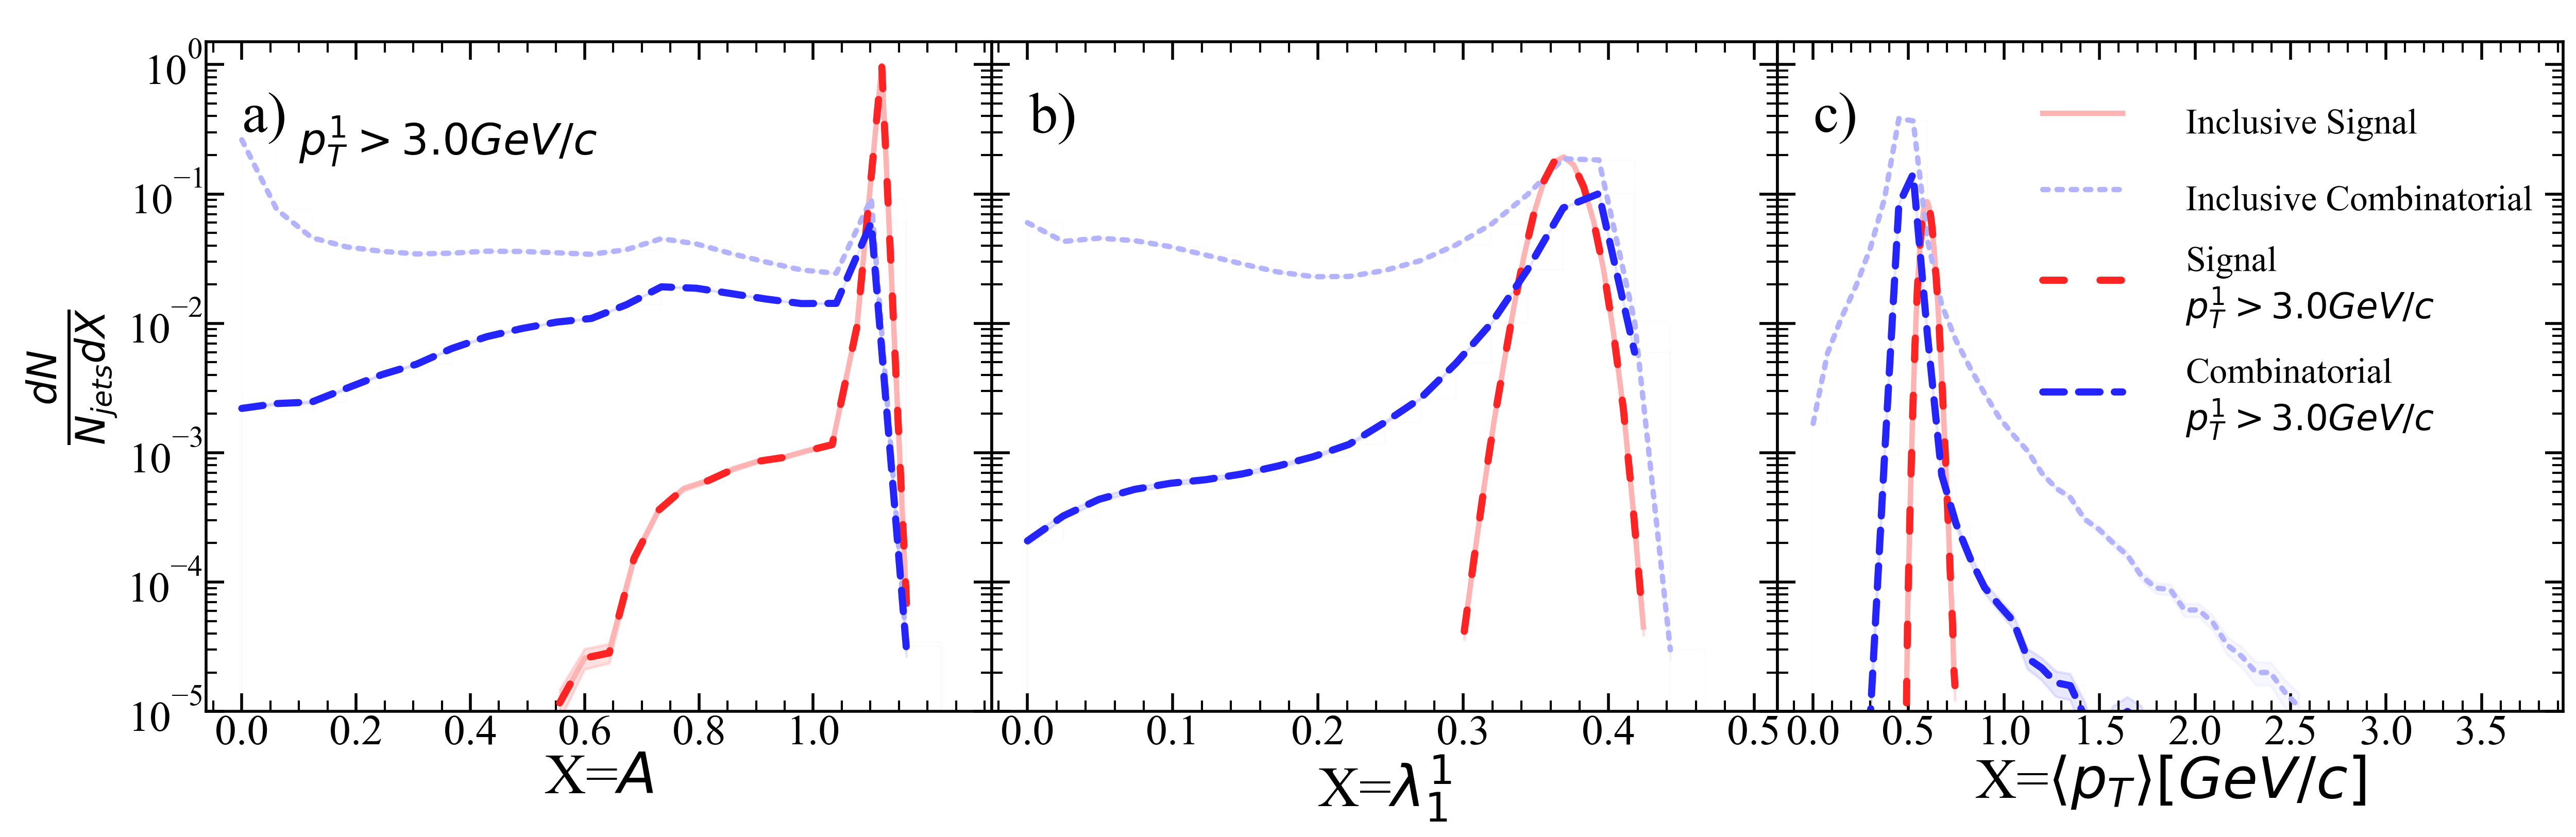}
    \caption{R=0.6 \ptH=40 \GeV}
    \label{fig:pT1_06_40}
\end{figure*}

\begin{figure*}
    \centering
    \includegraphics[width=\linewidth]{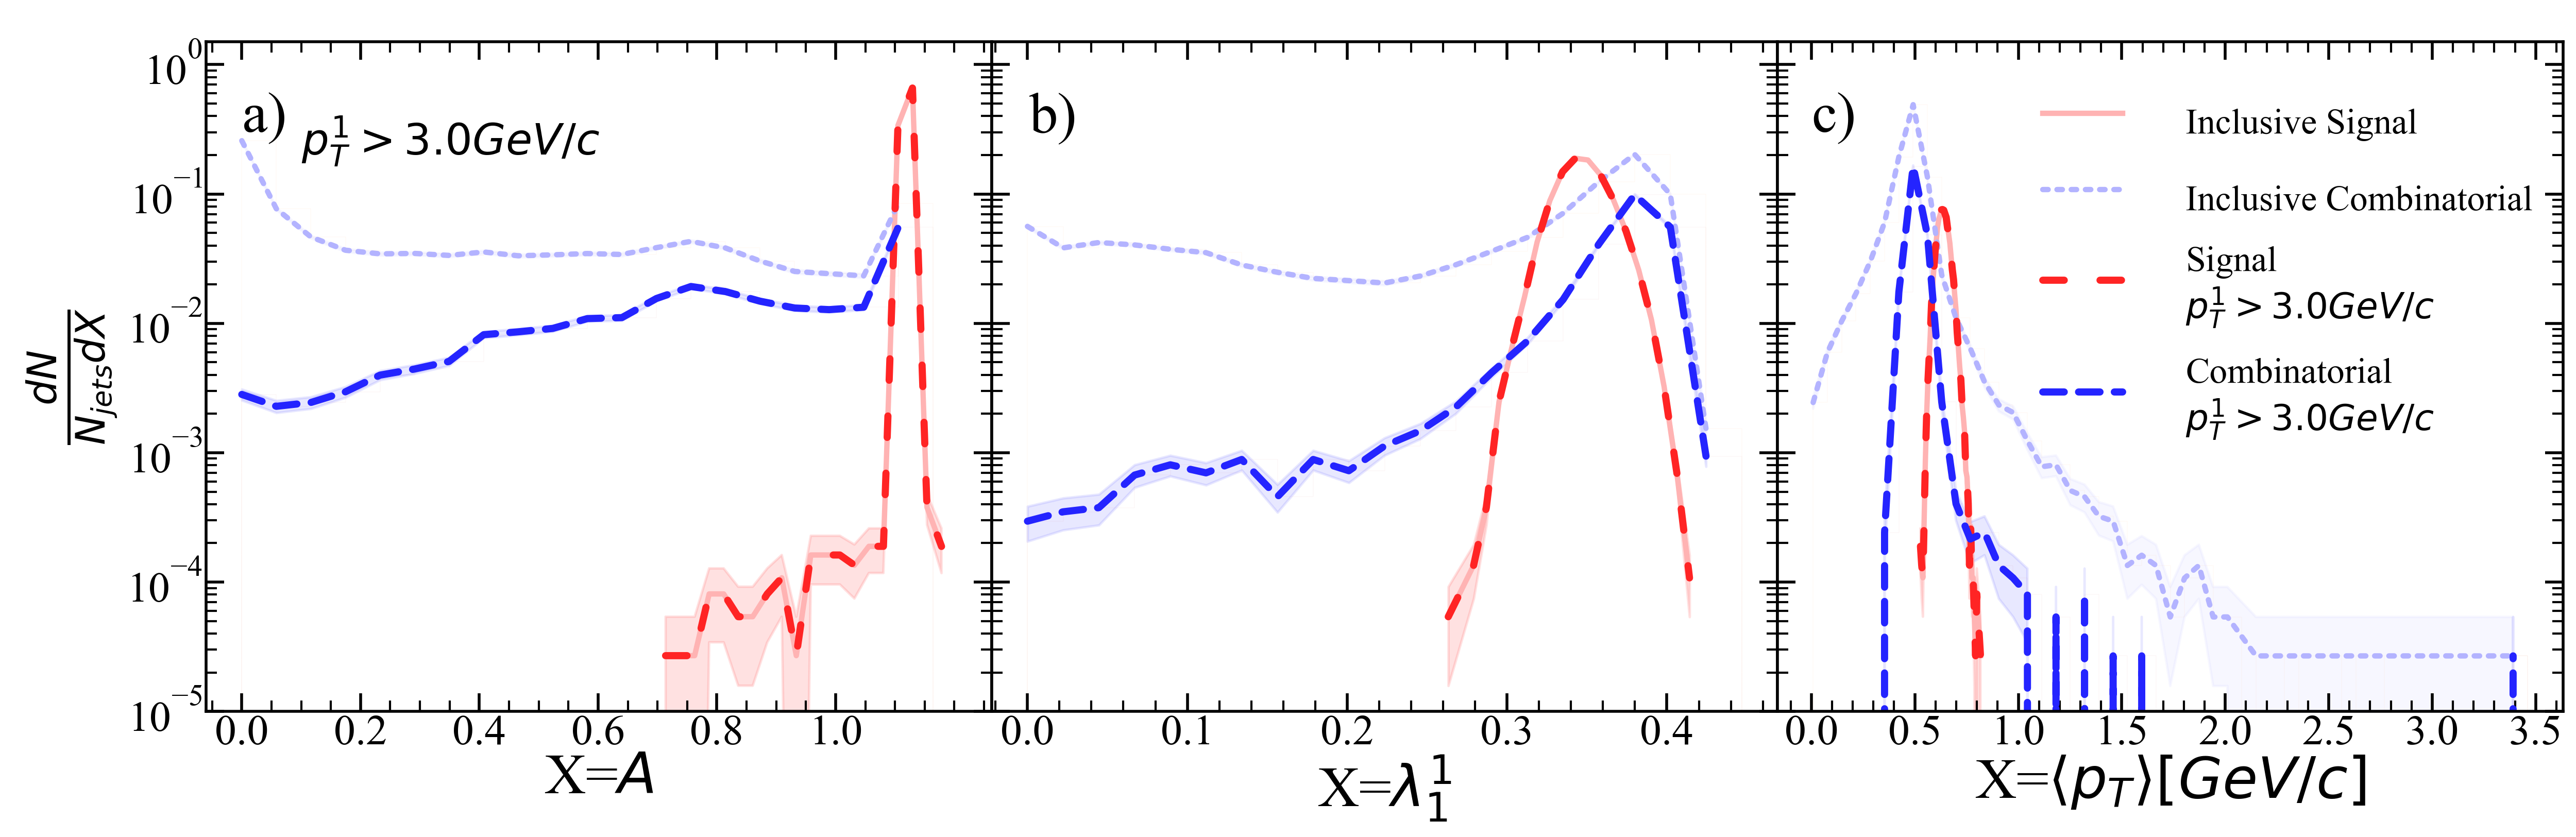}
    \caption{R=0.6 \ptH=60 \GeV}
    \label{fig:pT1_06_60}
\end{figure*}

\begin{figure*}
    \centering
    \includegraphics[width=\linewidth]{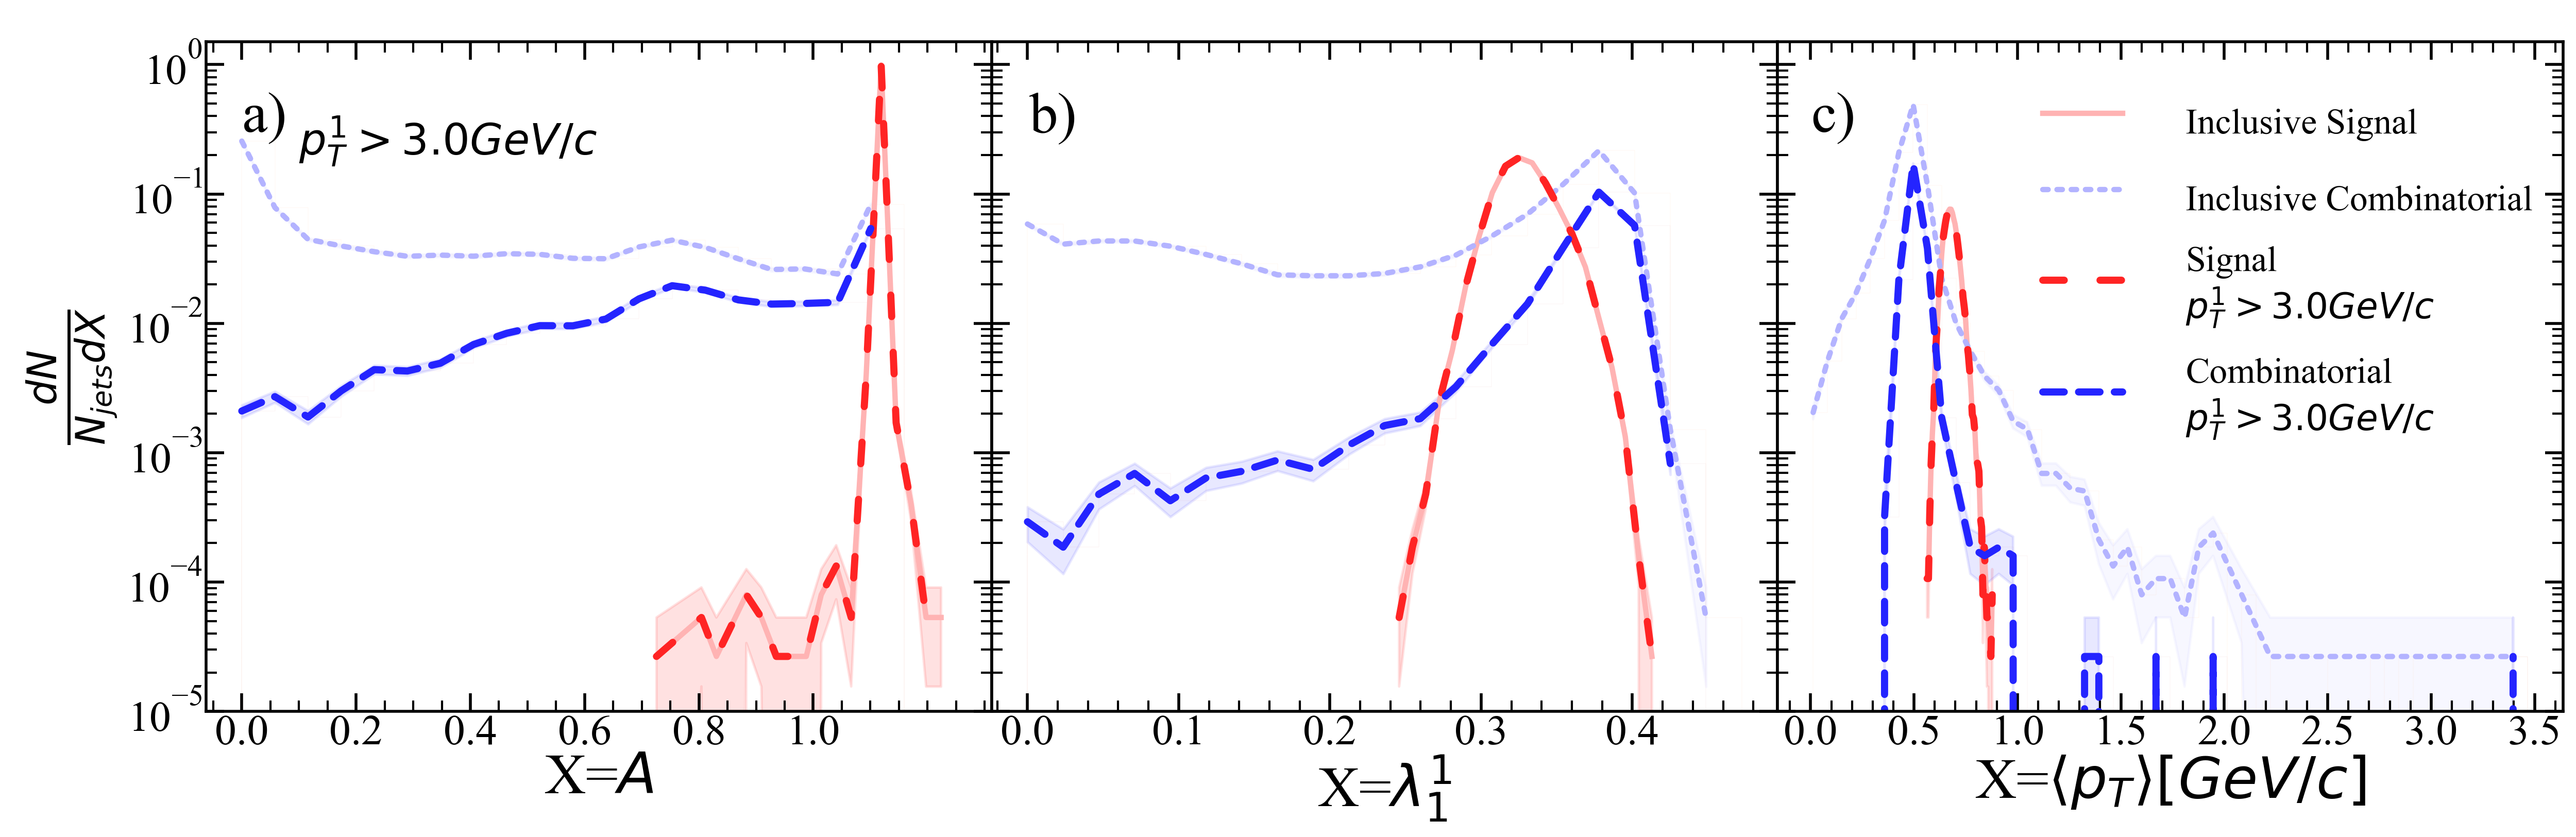}
    \caption{R=0.6 \ptH=80 \GeV}
    \label{fig:pT1_06_80}
\end{figure*}
\clearpage
\subsection{Silhouette values for each kinematic selection: a) no selection, b) area selection, c) leading hadron momentum selection, d) area and tighter leading hadron momentum selections.}

\begin{figure*}
    \centering
    \includegraphics[width=\linewidth]{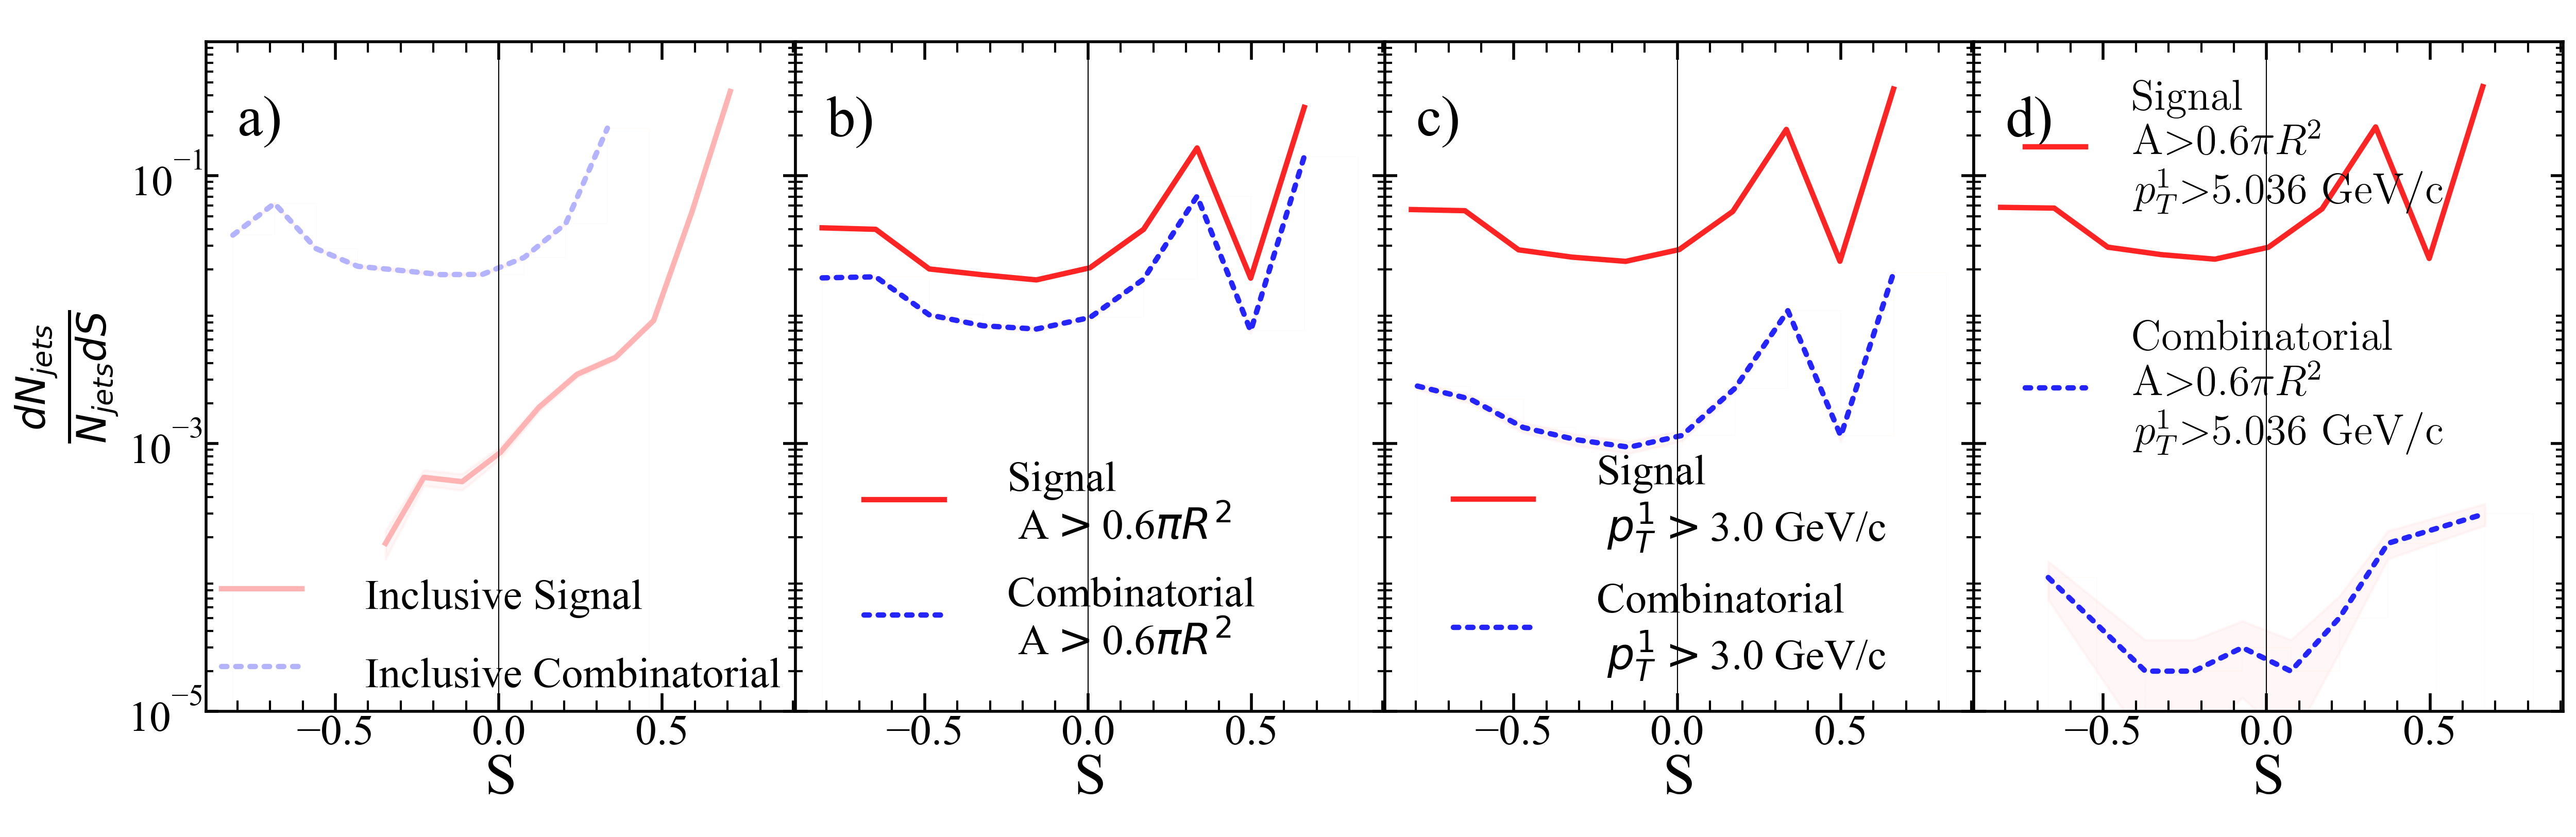}
    \caption{R=0.2 \ptH=10 \GeV}
    \label{fig:sil_02_10}
\end{figure*}

\begin{figure*}
    \centering
    \includegraphics[width=\linewidth]{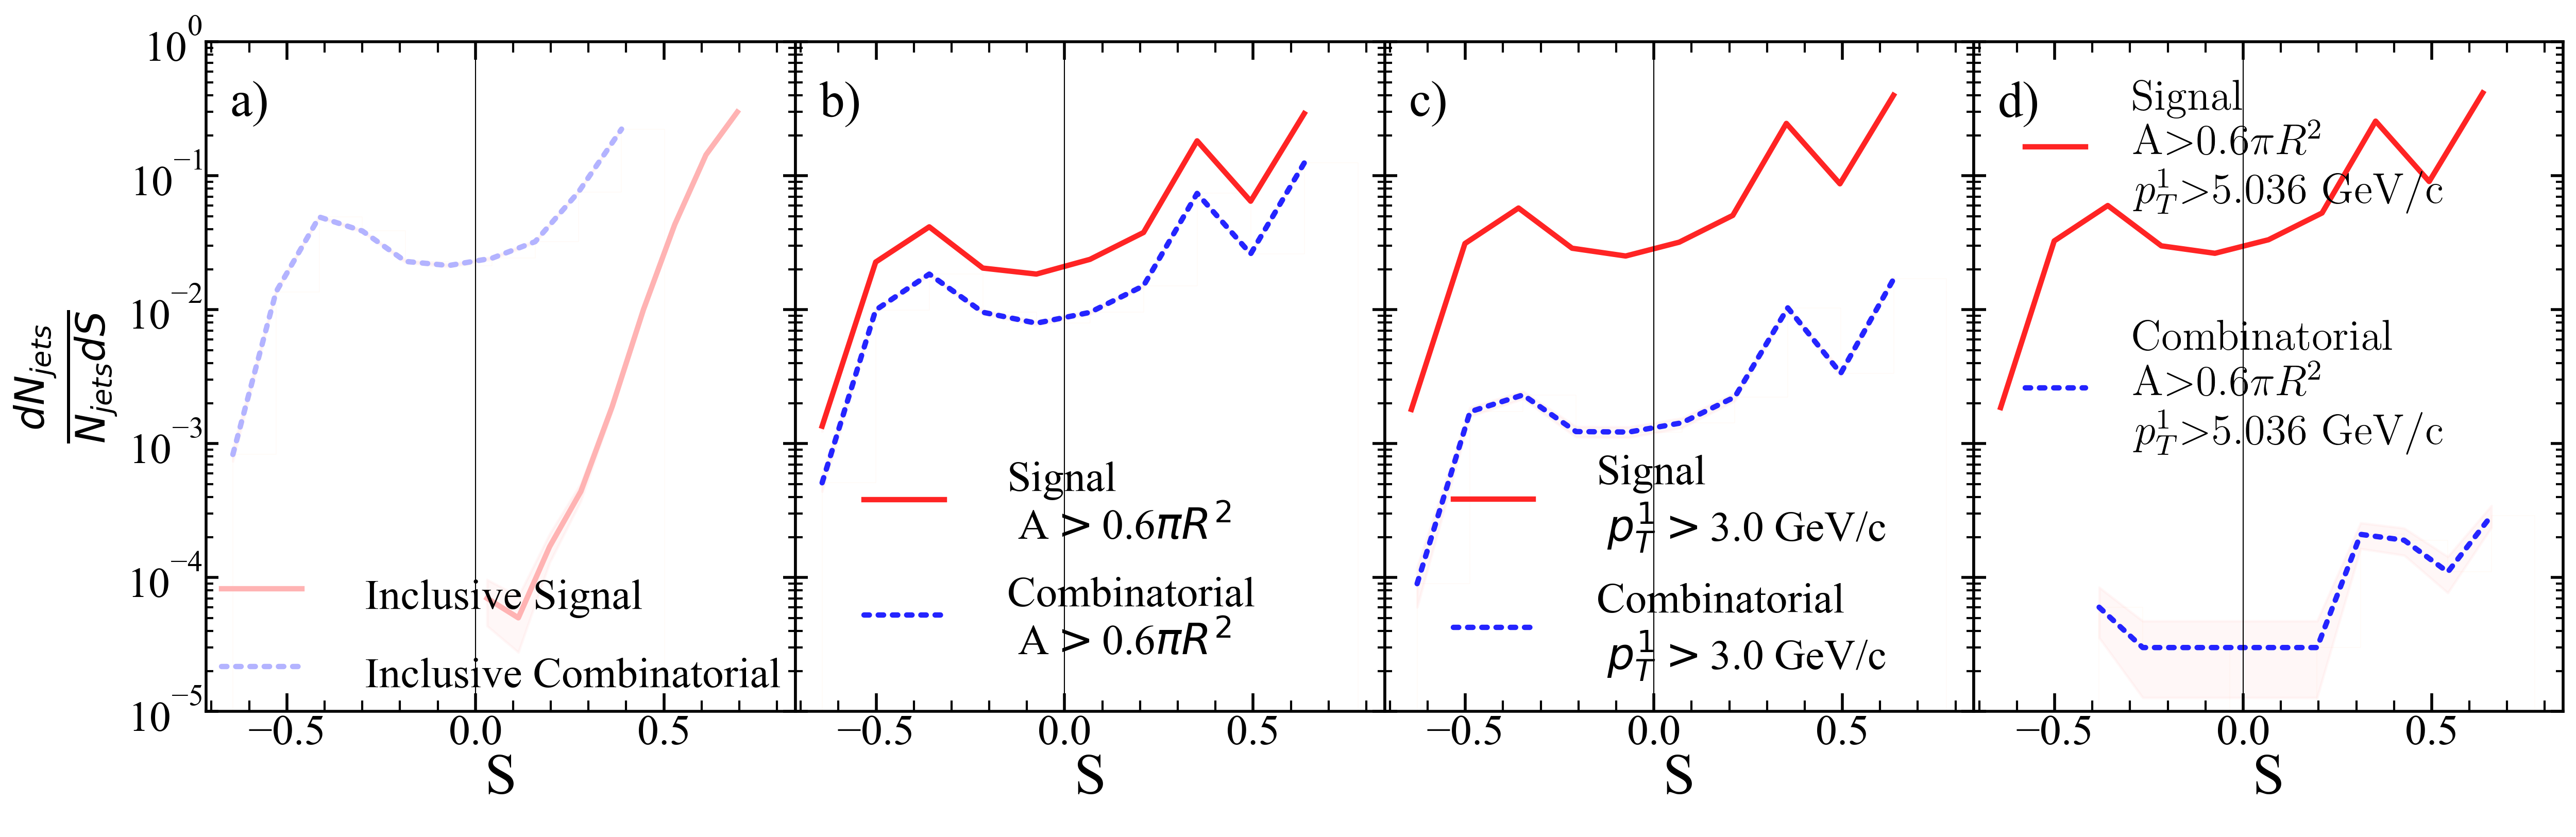}
    \caption{R=0.2 \ptH=20 \GeV}
    \label{fig:sil_02_20}
\end{figure*}

\begin{figure*}
    \centering
    \includegraphics[width=\linewidth]{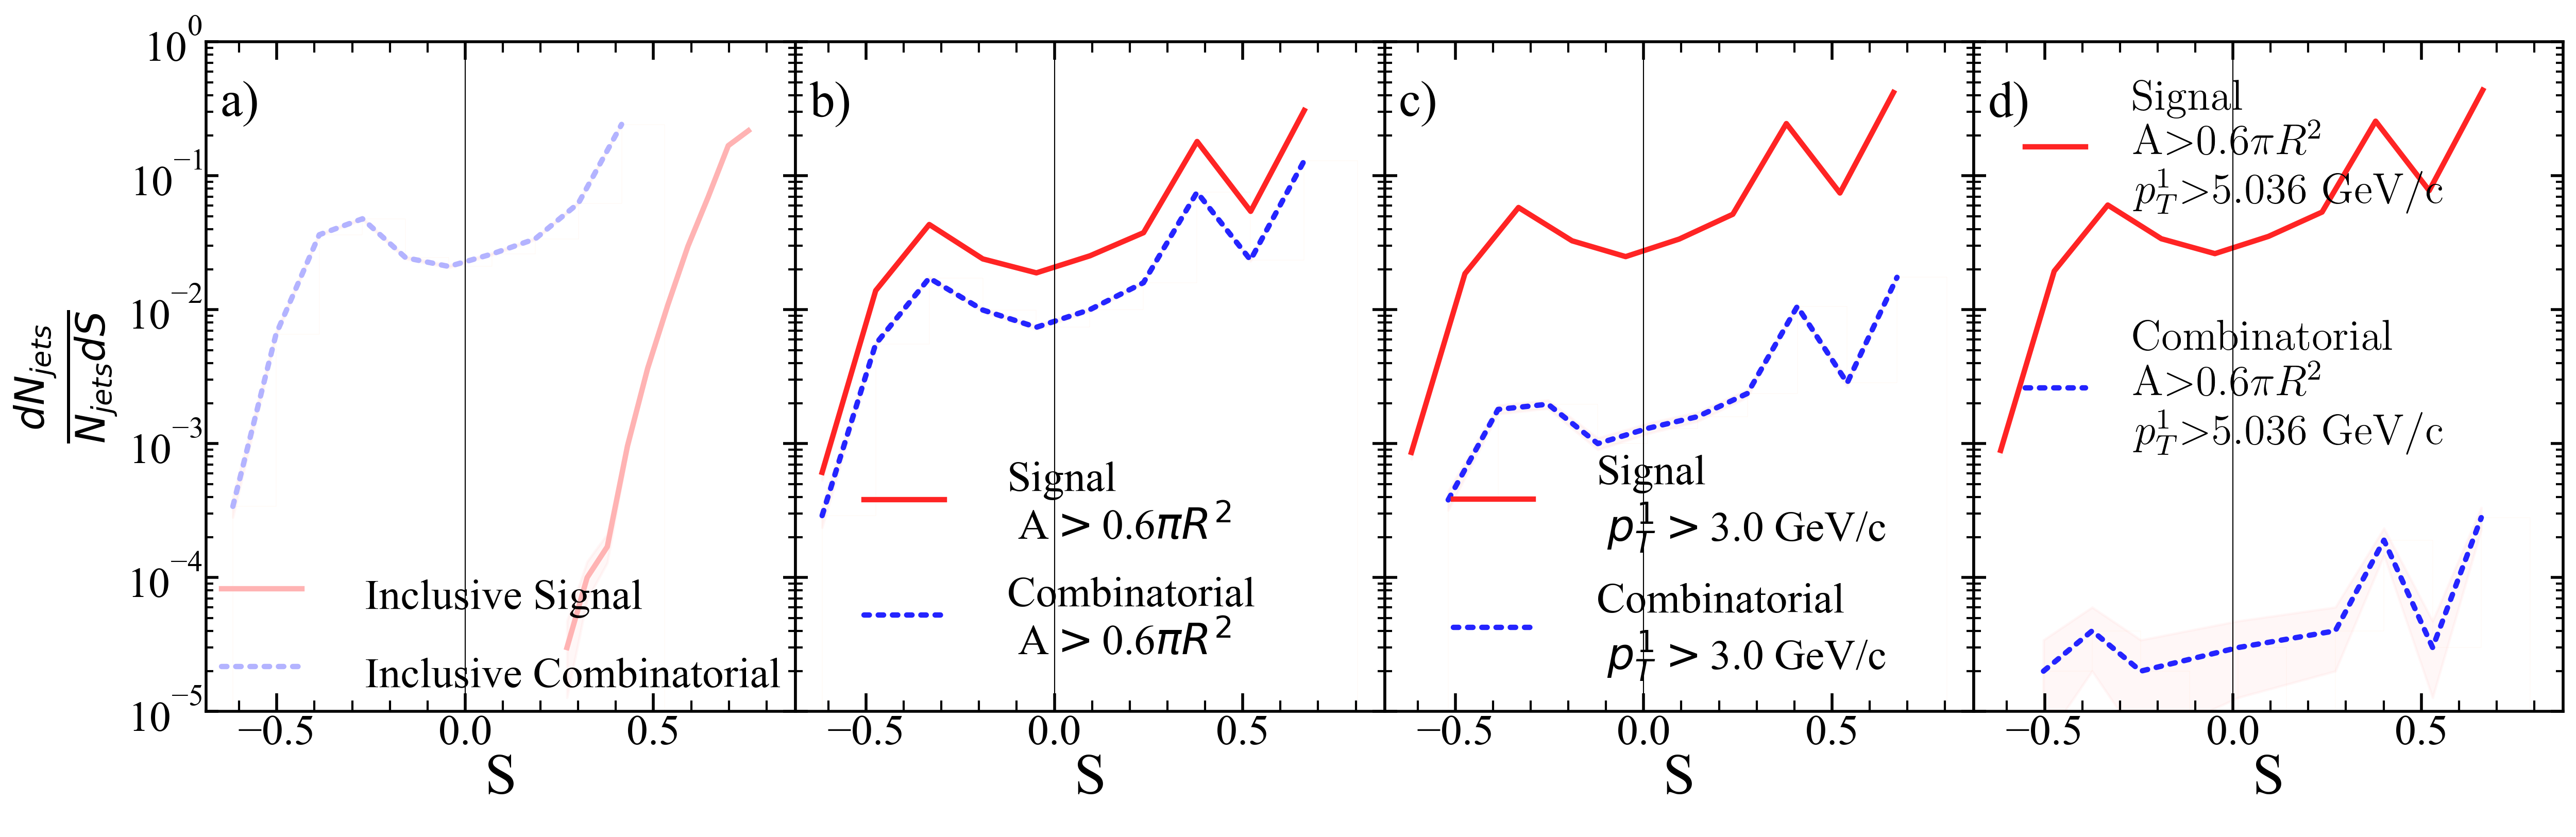}
    \caption{R=0.2 \ptH=30 \GeV}
    \label{fig:sil_02_30}
\end{figure*}

\begin{figure*}
    \centering
    \includegraphics[width=\linewidth]{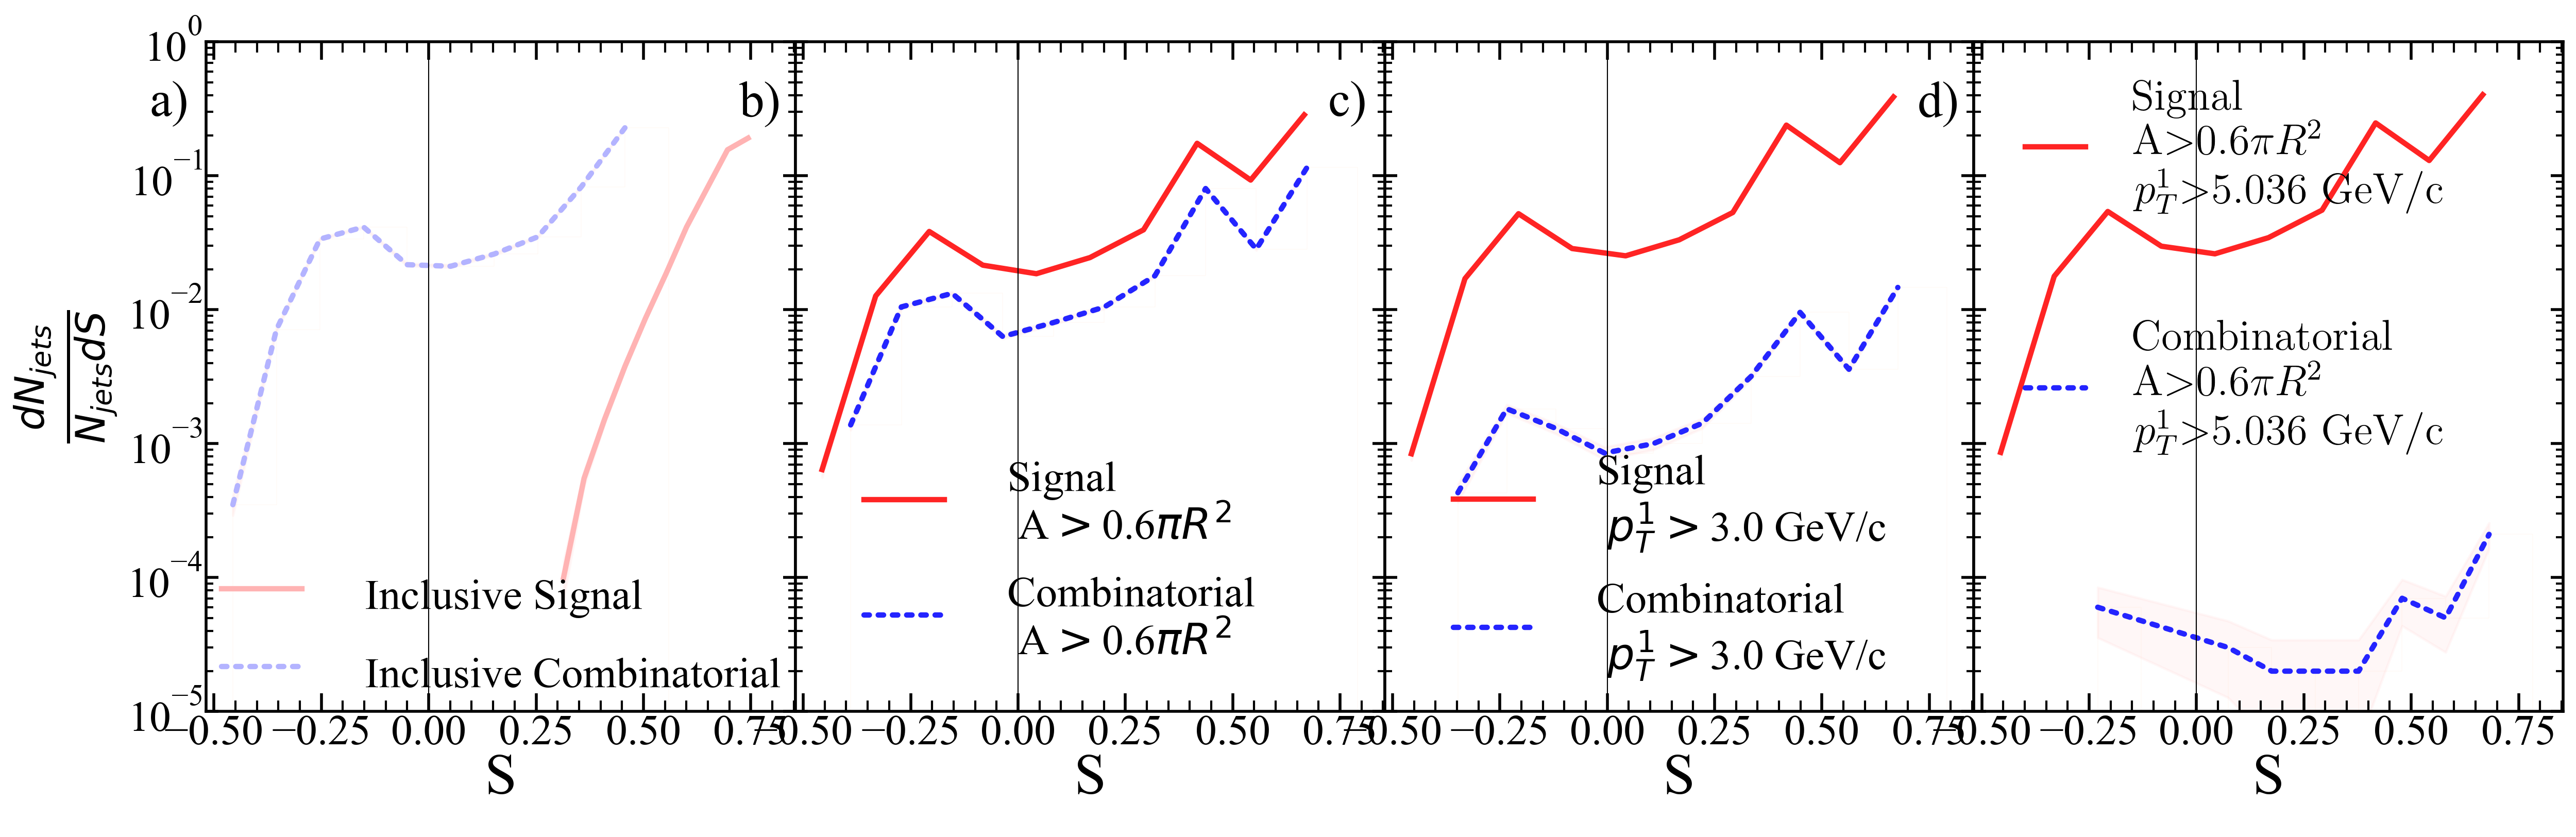}
    \caption{R=0.2 \ptH=40 \GeV}
    \label{fig:sil_02_40}
\end{figure*}

\begin{figure*}
    \centering
    \includegraphics[width=\linewidth]{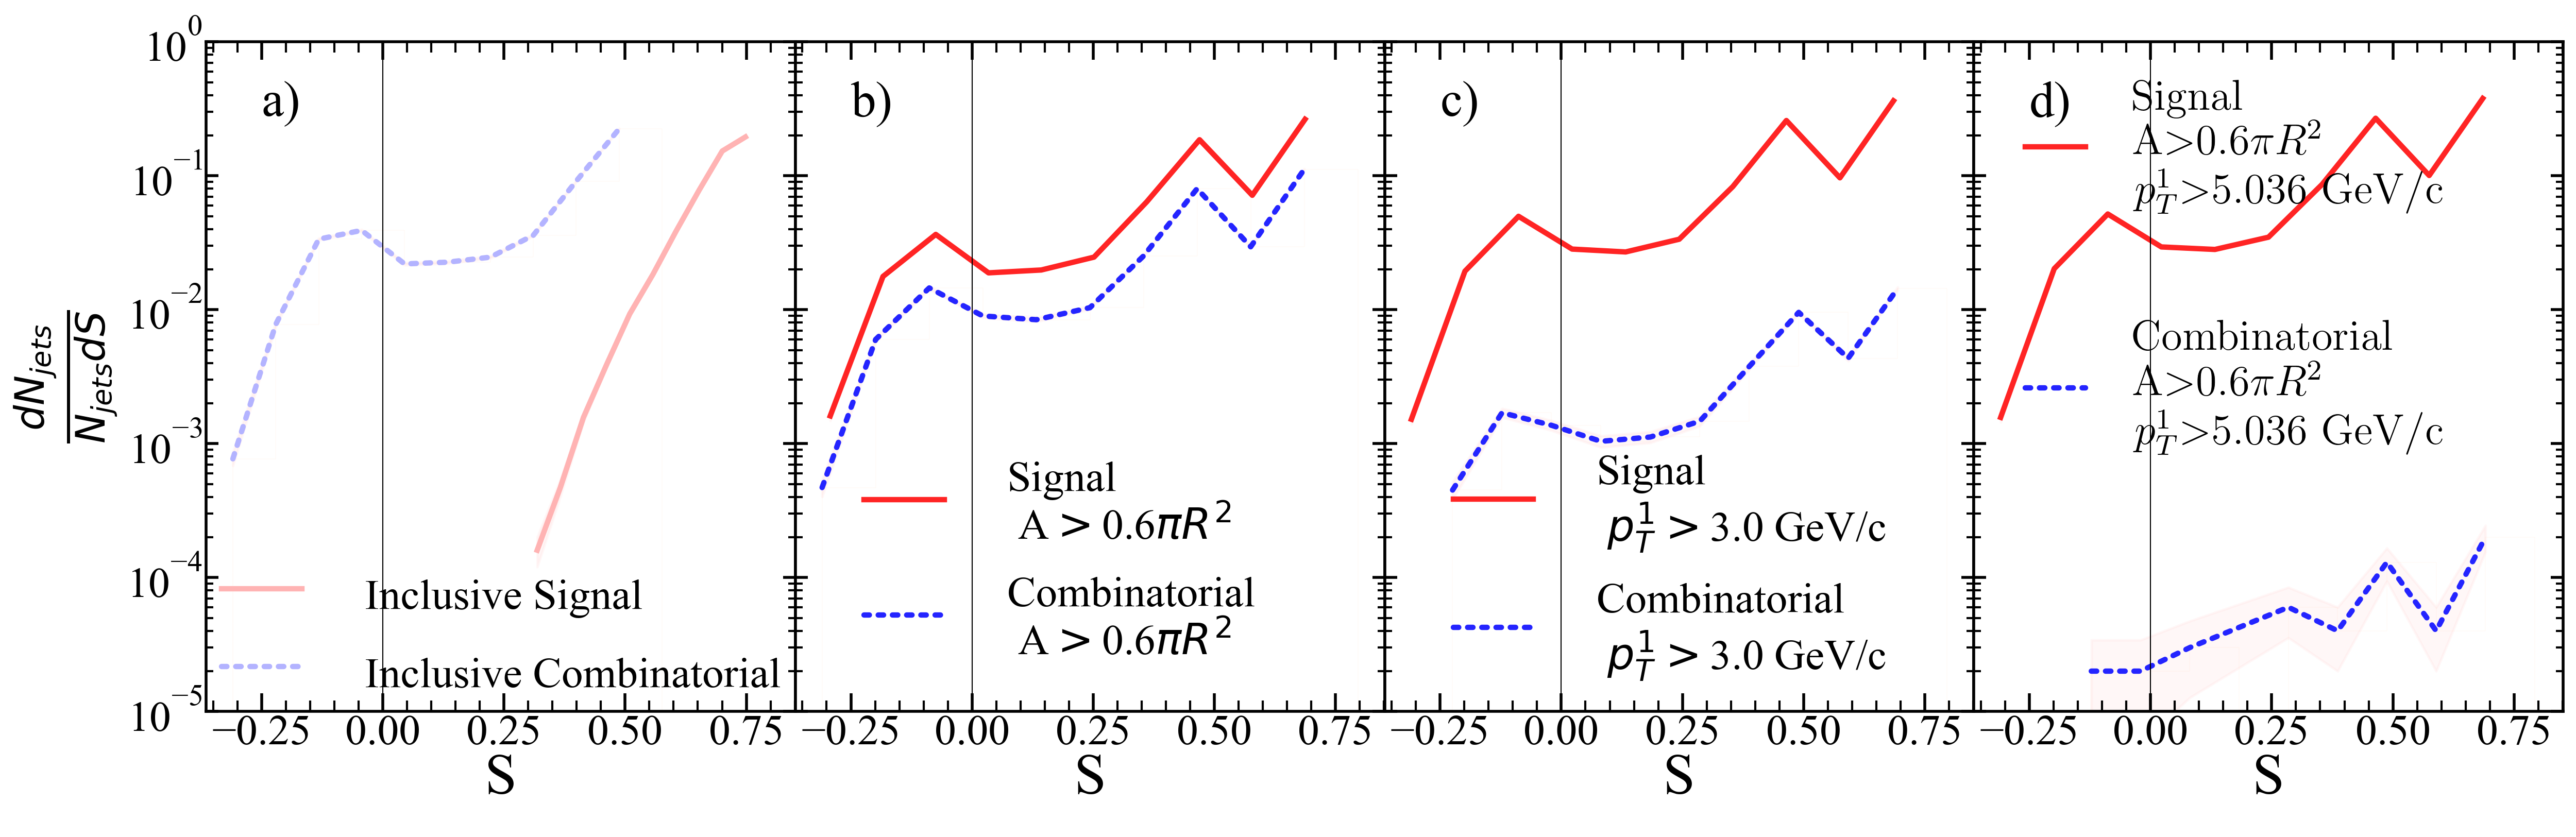}
    \caption{R=0.2 \ptH=60 \GeV}
    \label{fig:sil_02_60}
\end{figure*}

\begin{figure*}
    \centering
    \includegraphics[width=\linewidth]{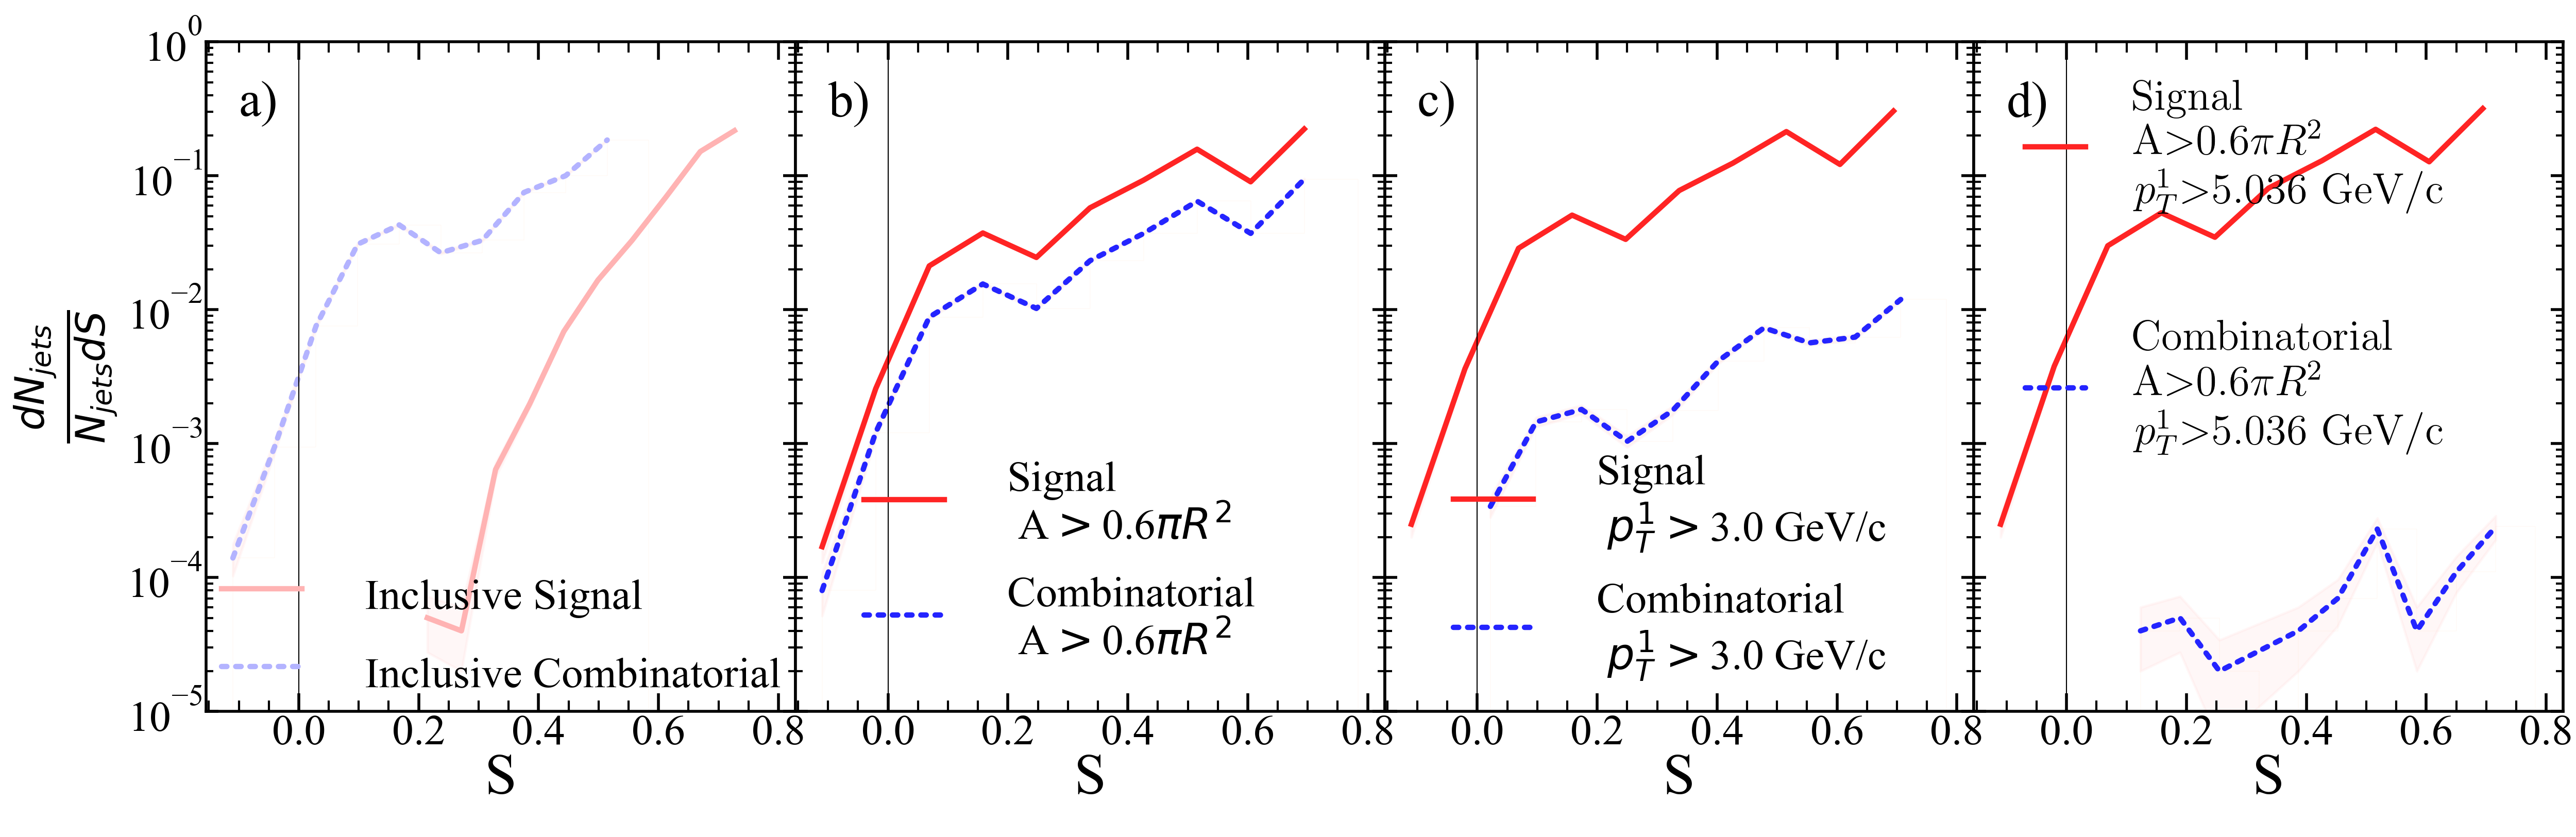}
    \caption{R=0.2 \ptH=80 \GeV}
    \label{fig:sil_02_80}
\end{figure*}

\begin{figure*}
    \centering
    \includegraphics[width=\linewidth]{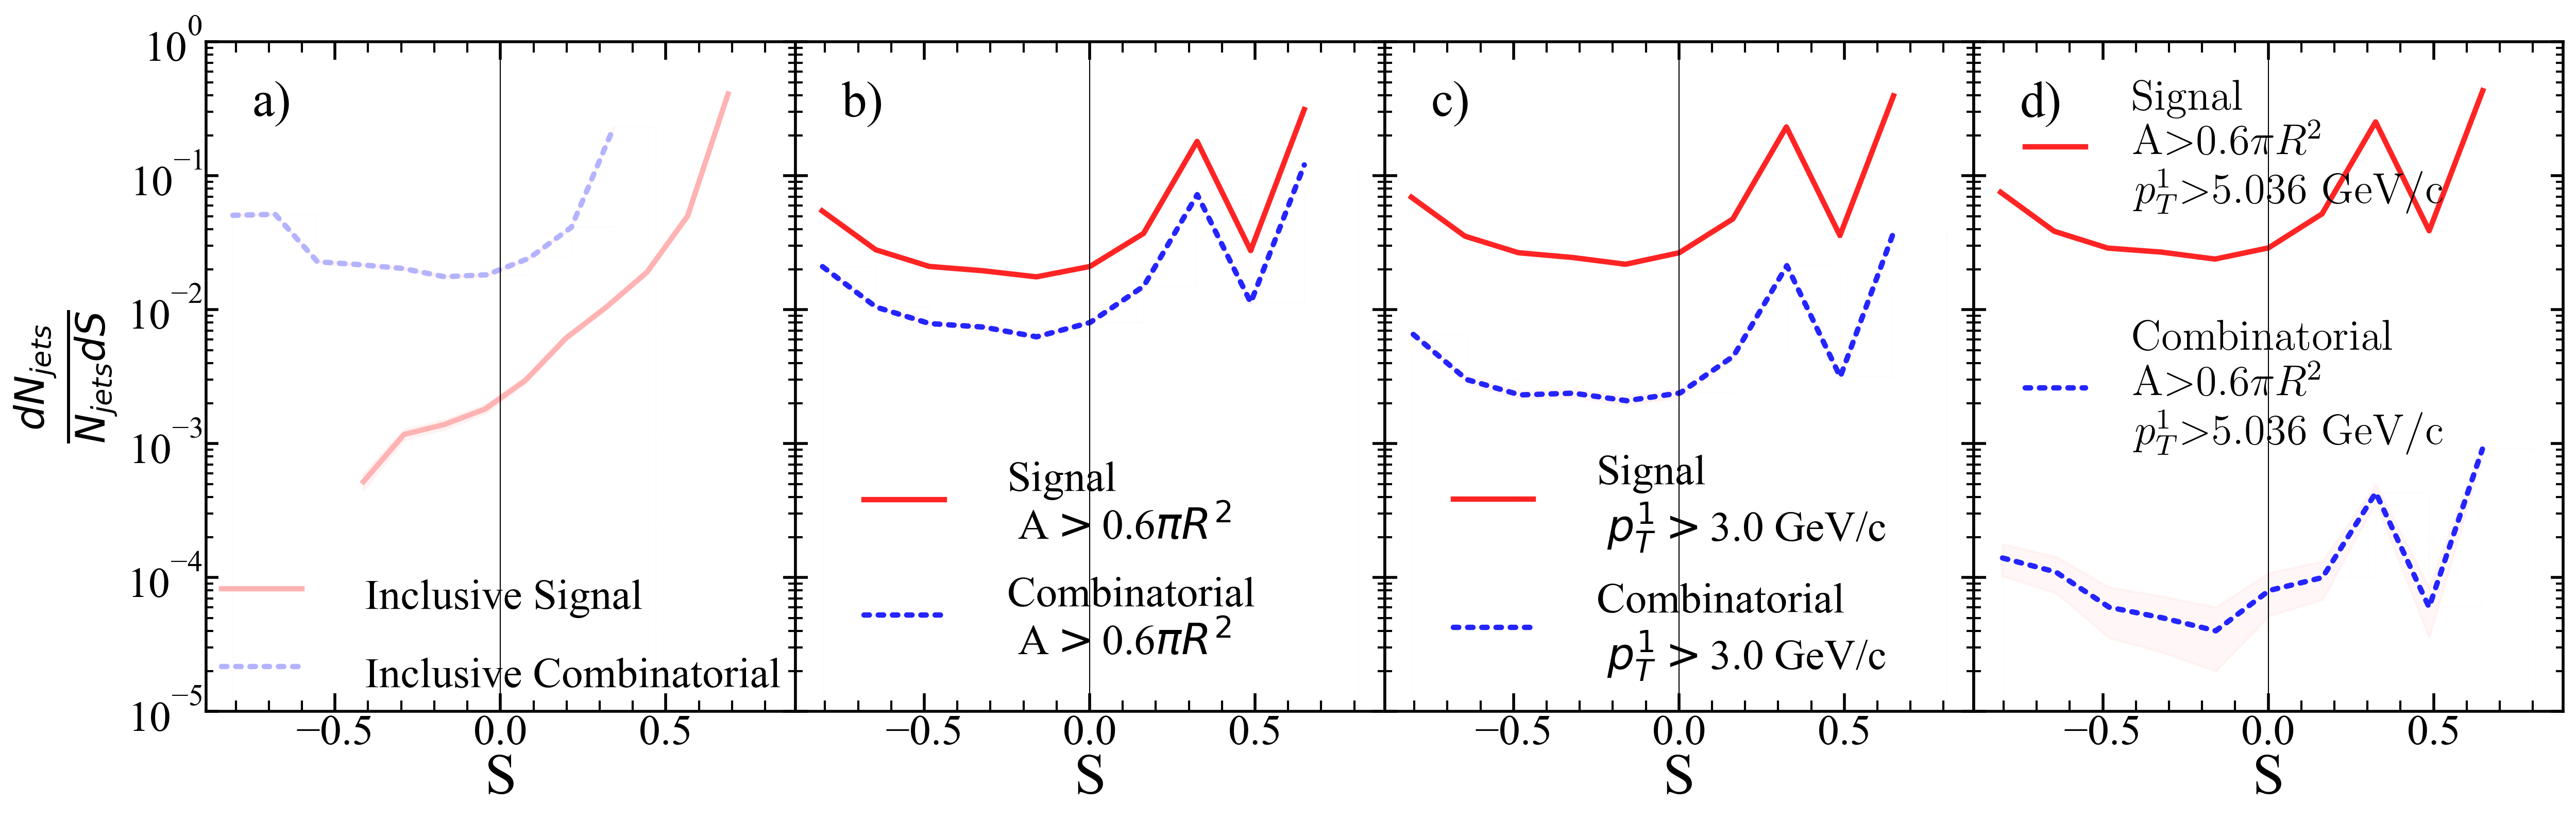}
    \caption{R=0.3 \ptH=10 \GeV}
    \label{fig:sil_03_10}
\end{figure*}

\begin{figure*}
    \centering
    \includegraphics[width=\linewidth]{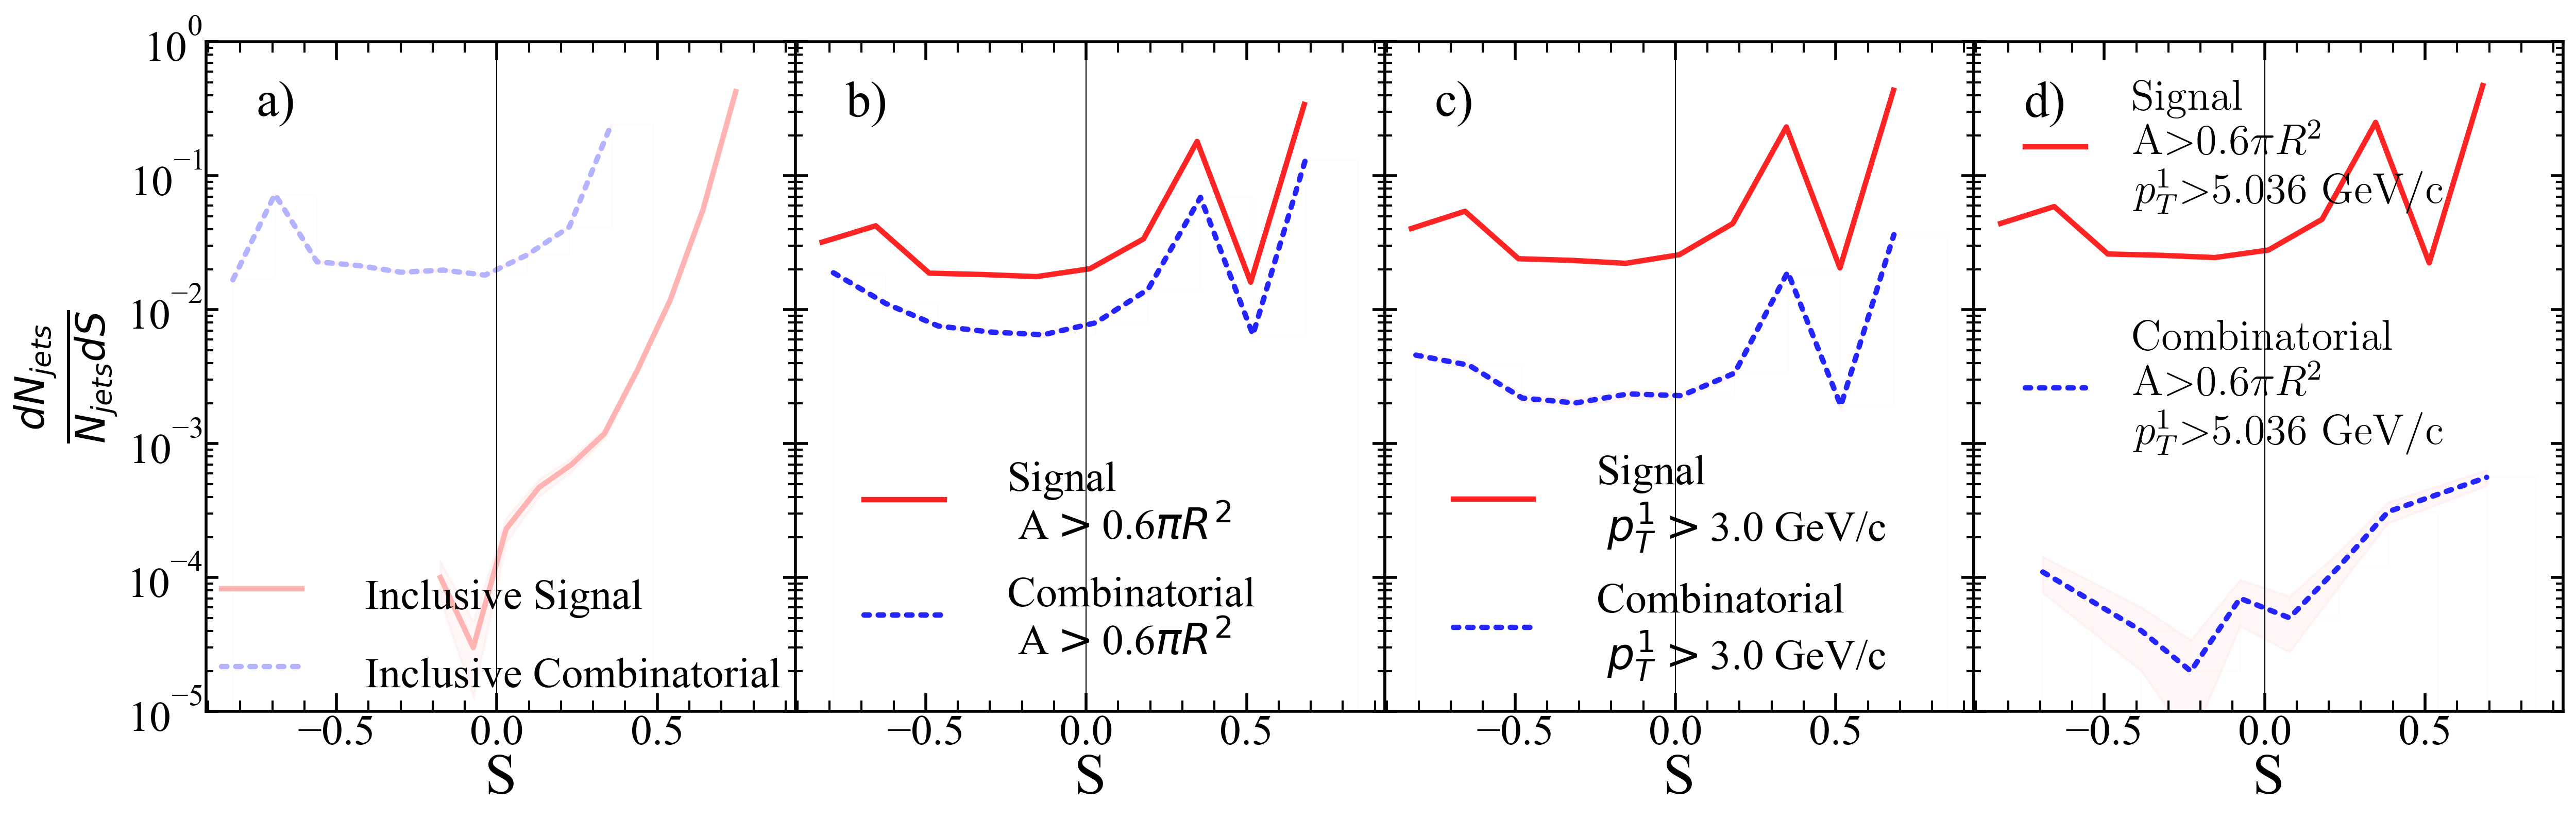}
    \caption{R=0.3 \ptH=20 \GeV}
    \label{fig:sil_03_20}
\end{figure*}

\begin{figure*}
    \centering
    \includegraphics[width=\linewidth]{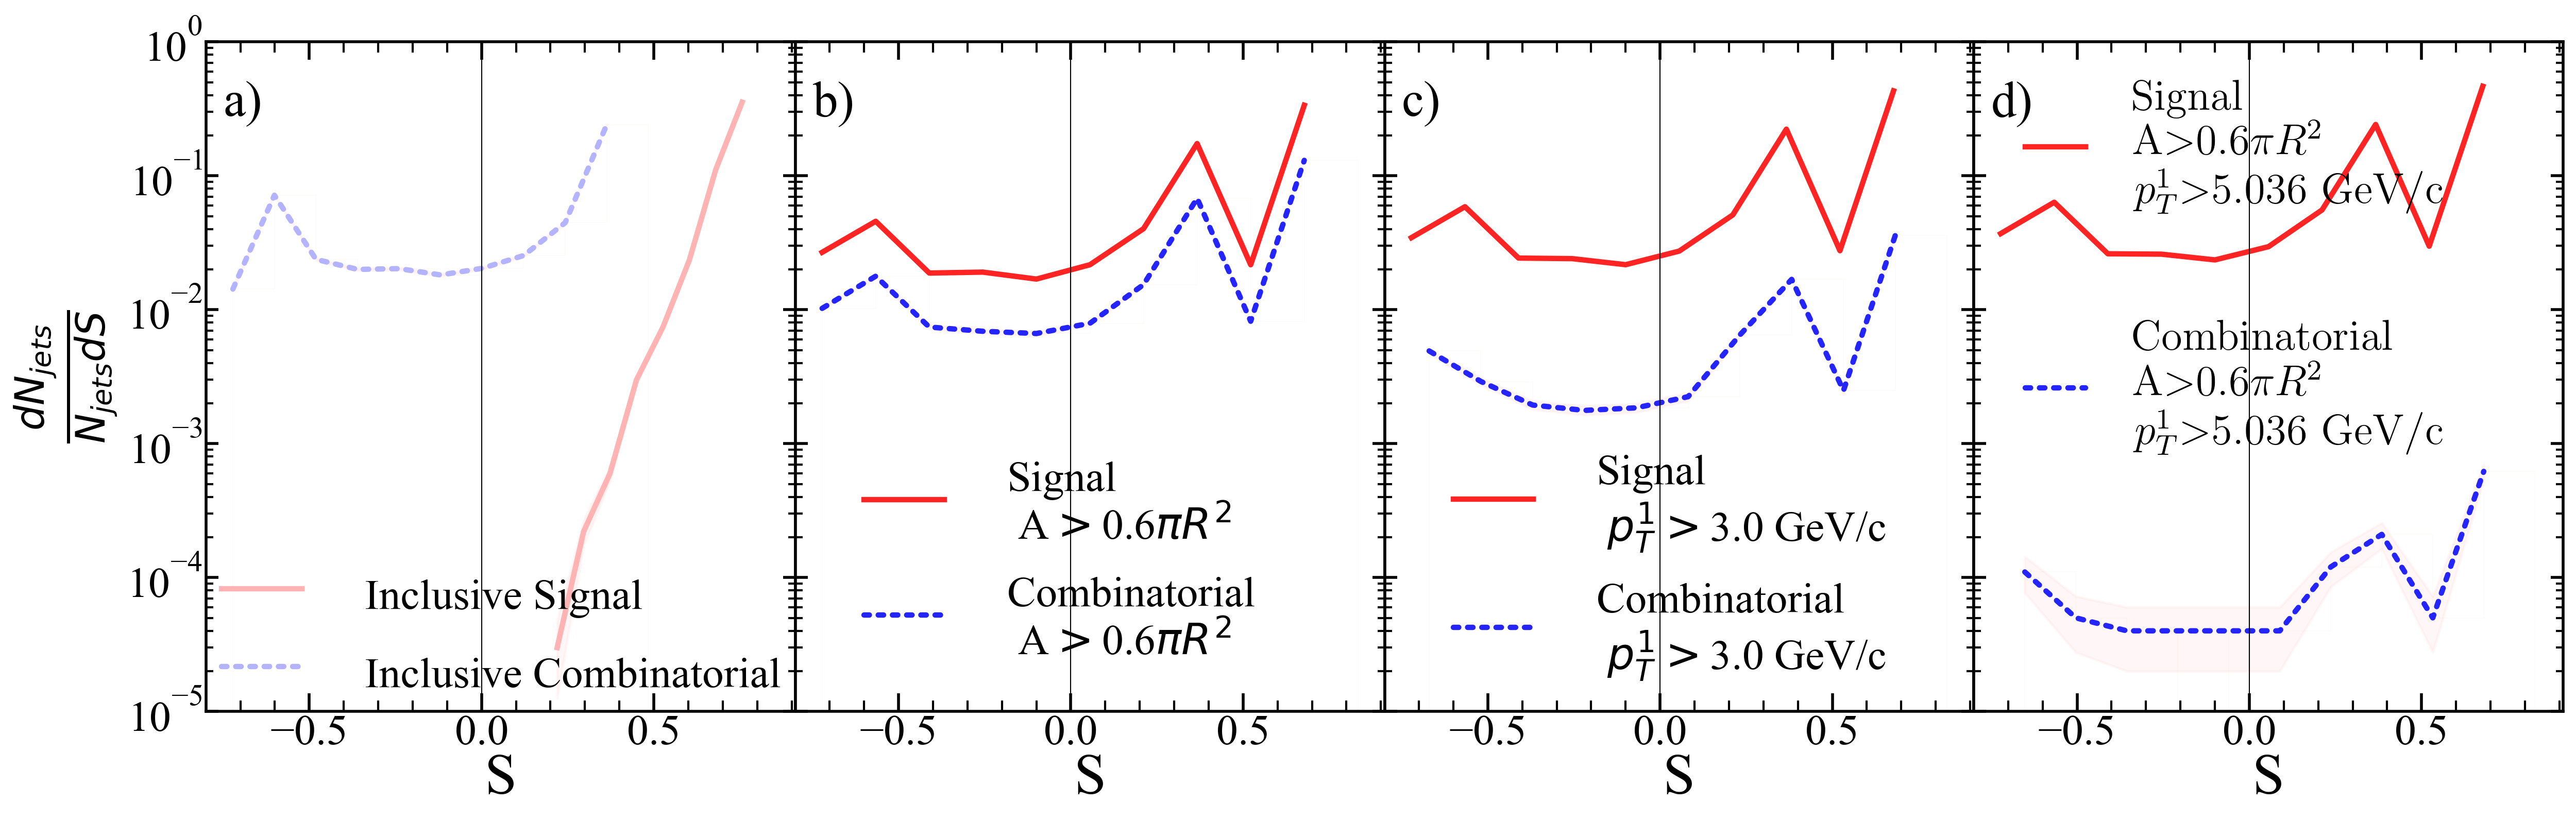}
    \caption{R=0.3 \ptH=30 \GeV}
    \label{fig:sil_03_30}
\end{figure*}

\begin{figure*}
    \centering
    \includegraphics[width=\linewidth]{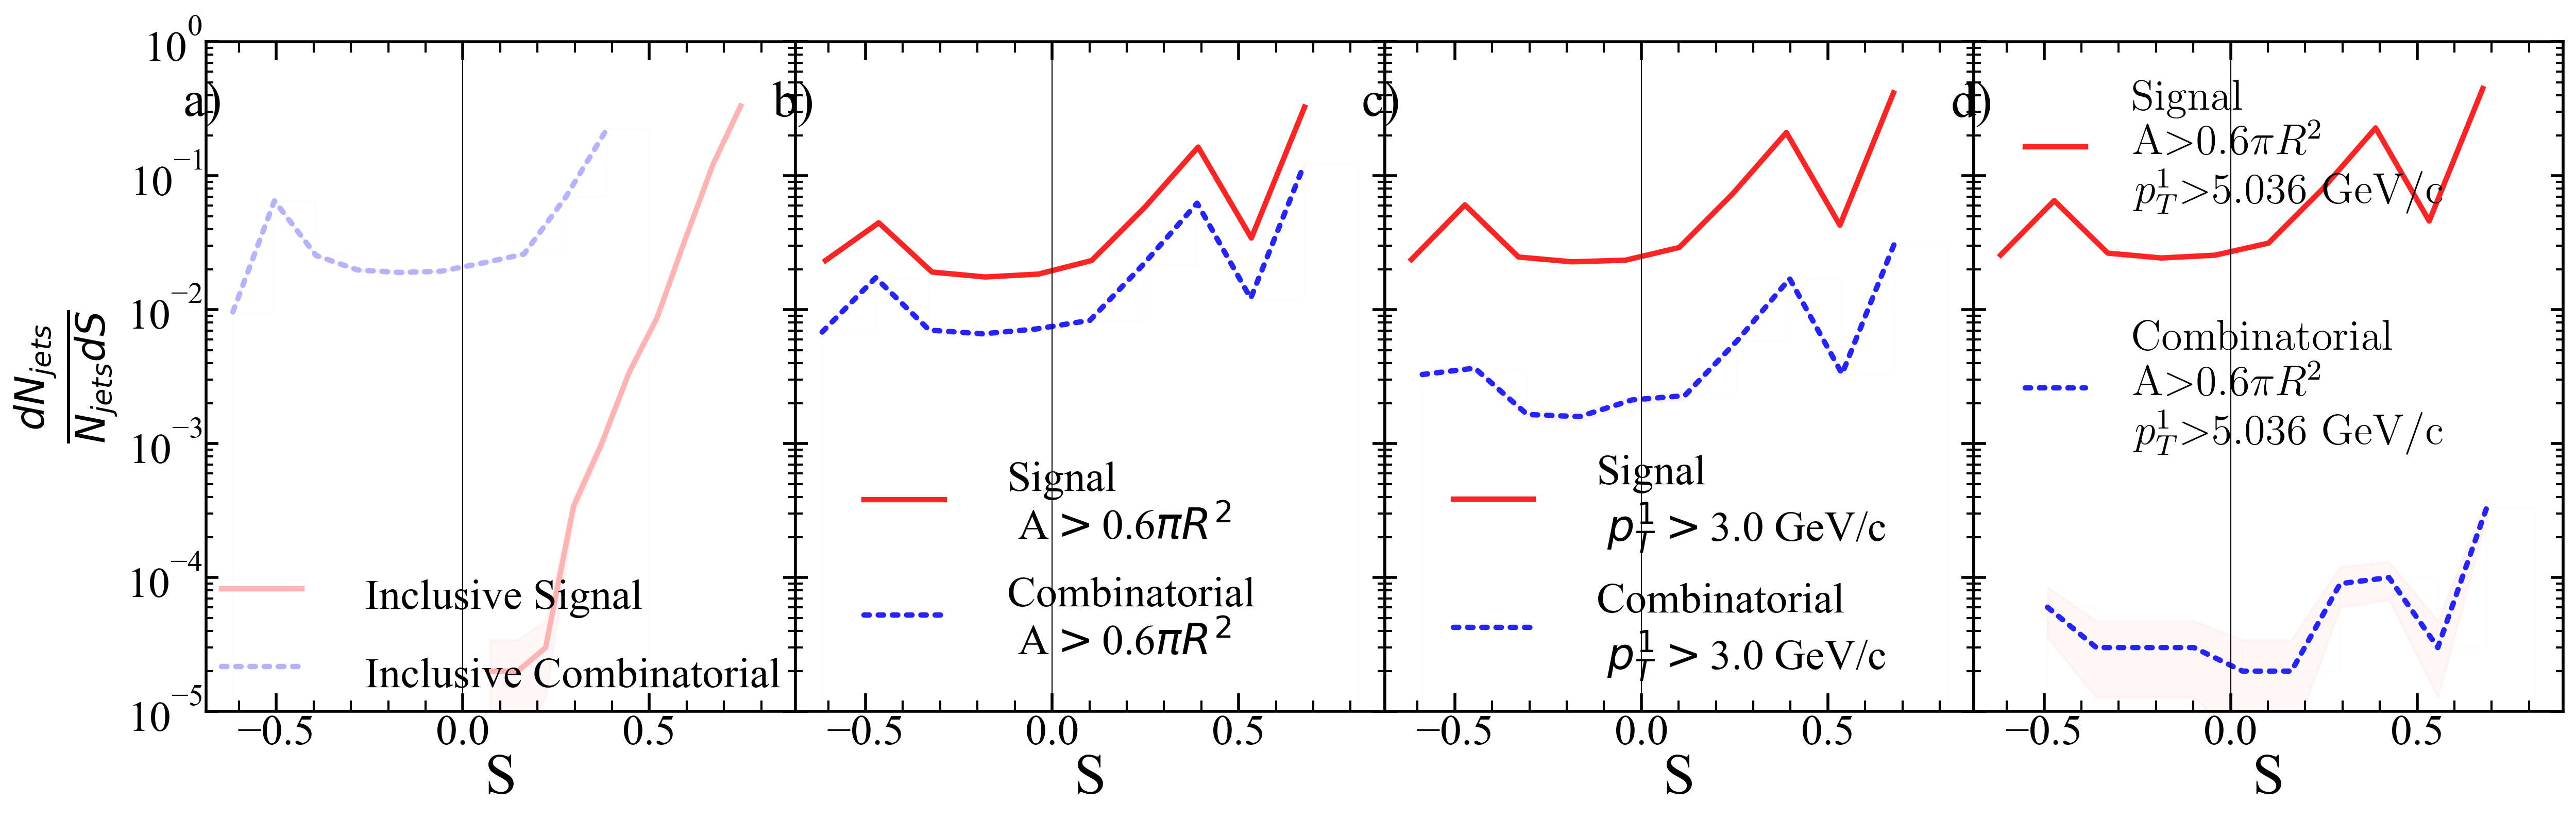}
    \caption{R=0.3 \ptH=40 \GeV}
    \label{fig:sil_03_40}
\end{figure*}

\begin{figure*}
    \centering
    \includegraphics[width=\linewidth]{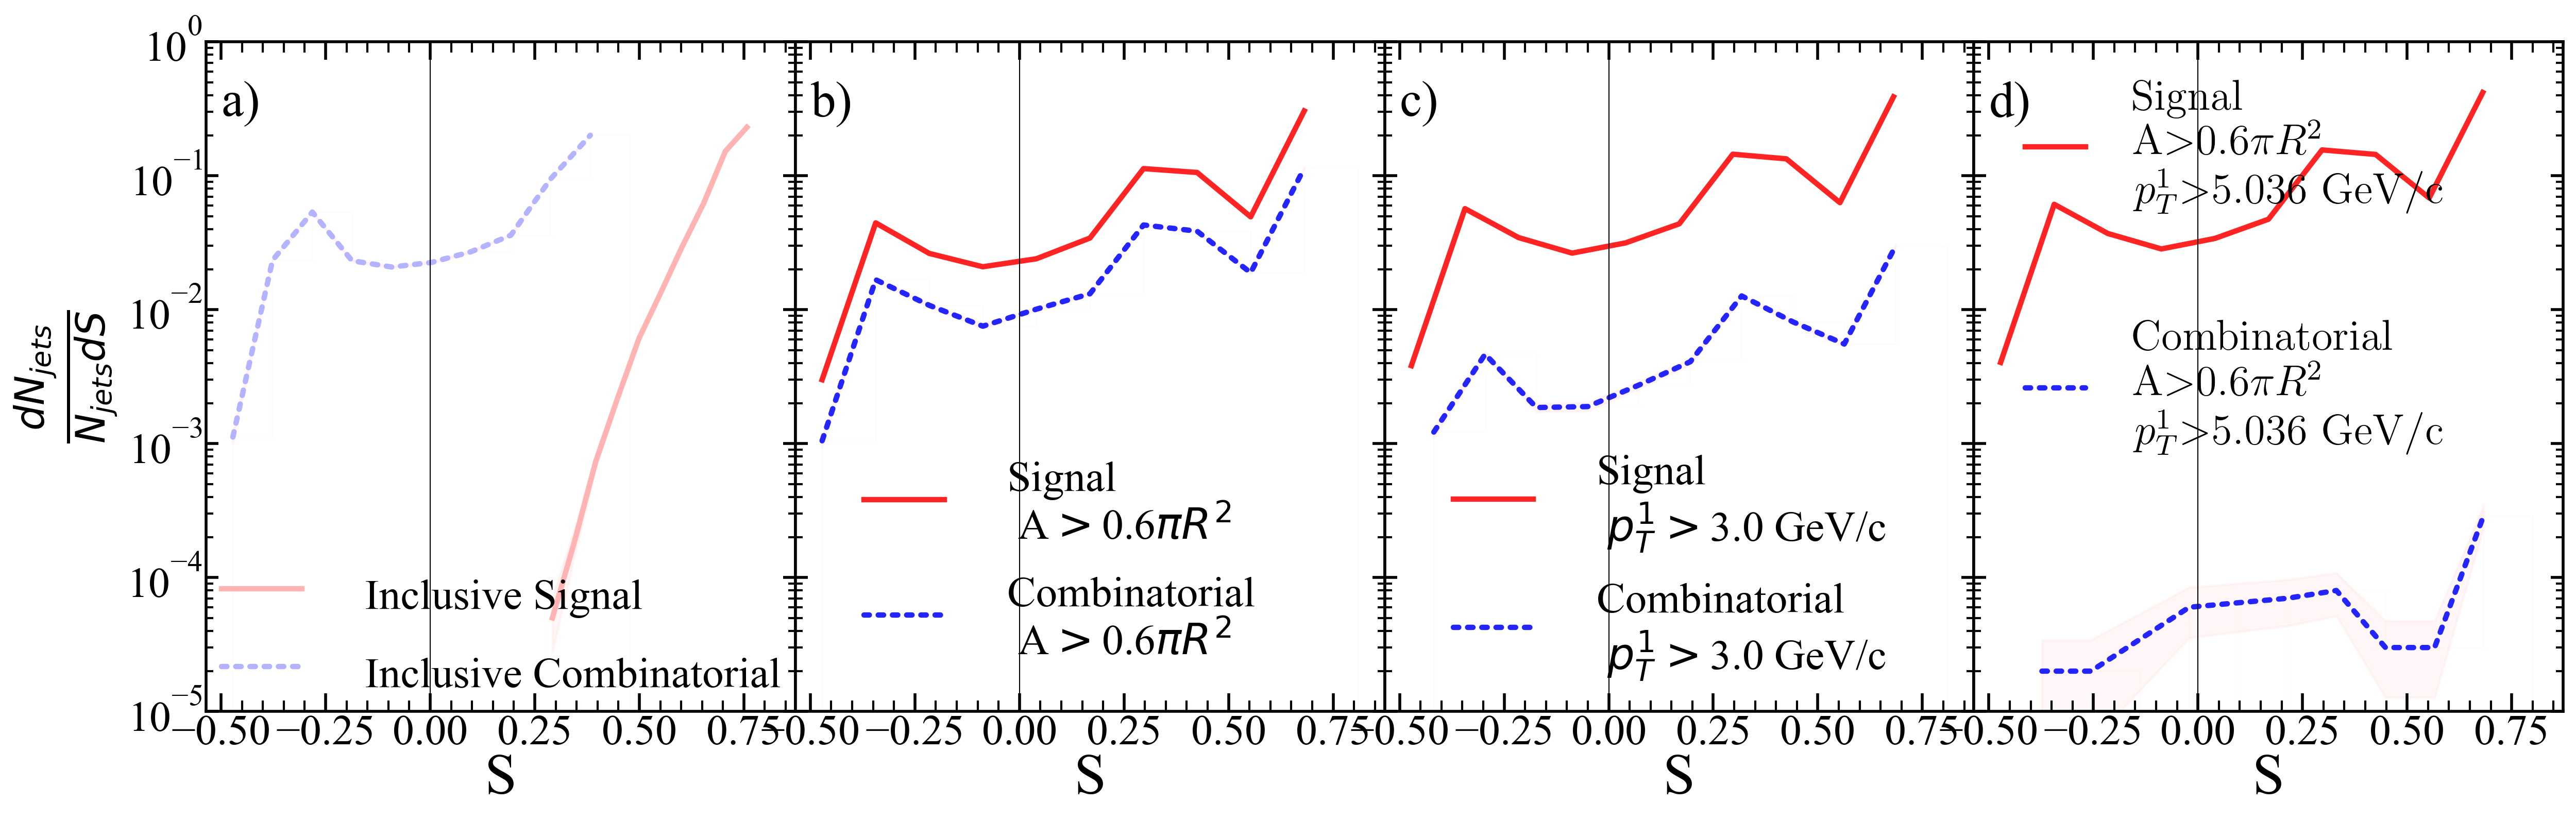}
    \caption{R=0.3 \ptH=60 \GeV}
    \label{fig:sil_03_60}
\end{figure*}

\begin{figure*}
    \centering
    \includegraphics[width=\linewidth]{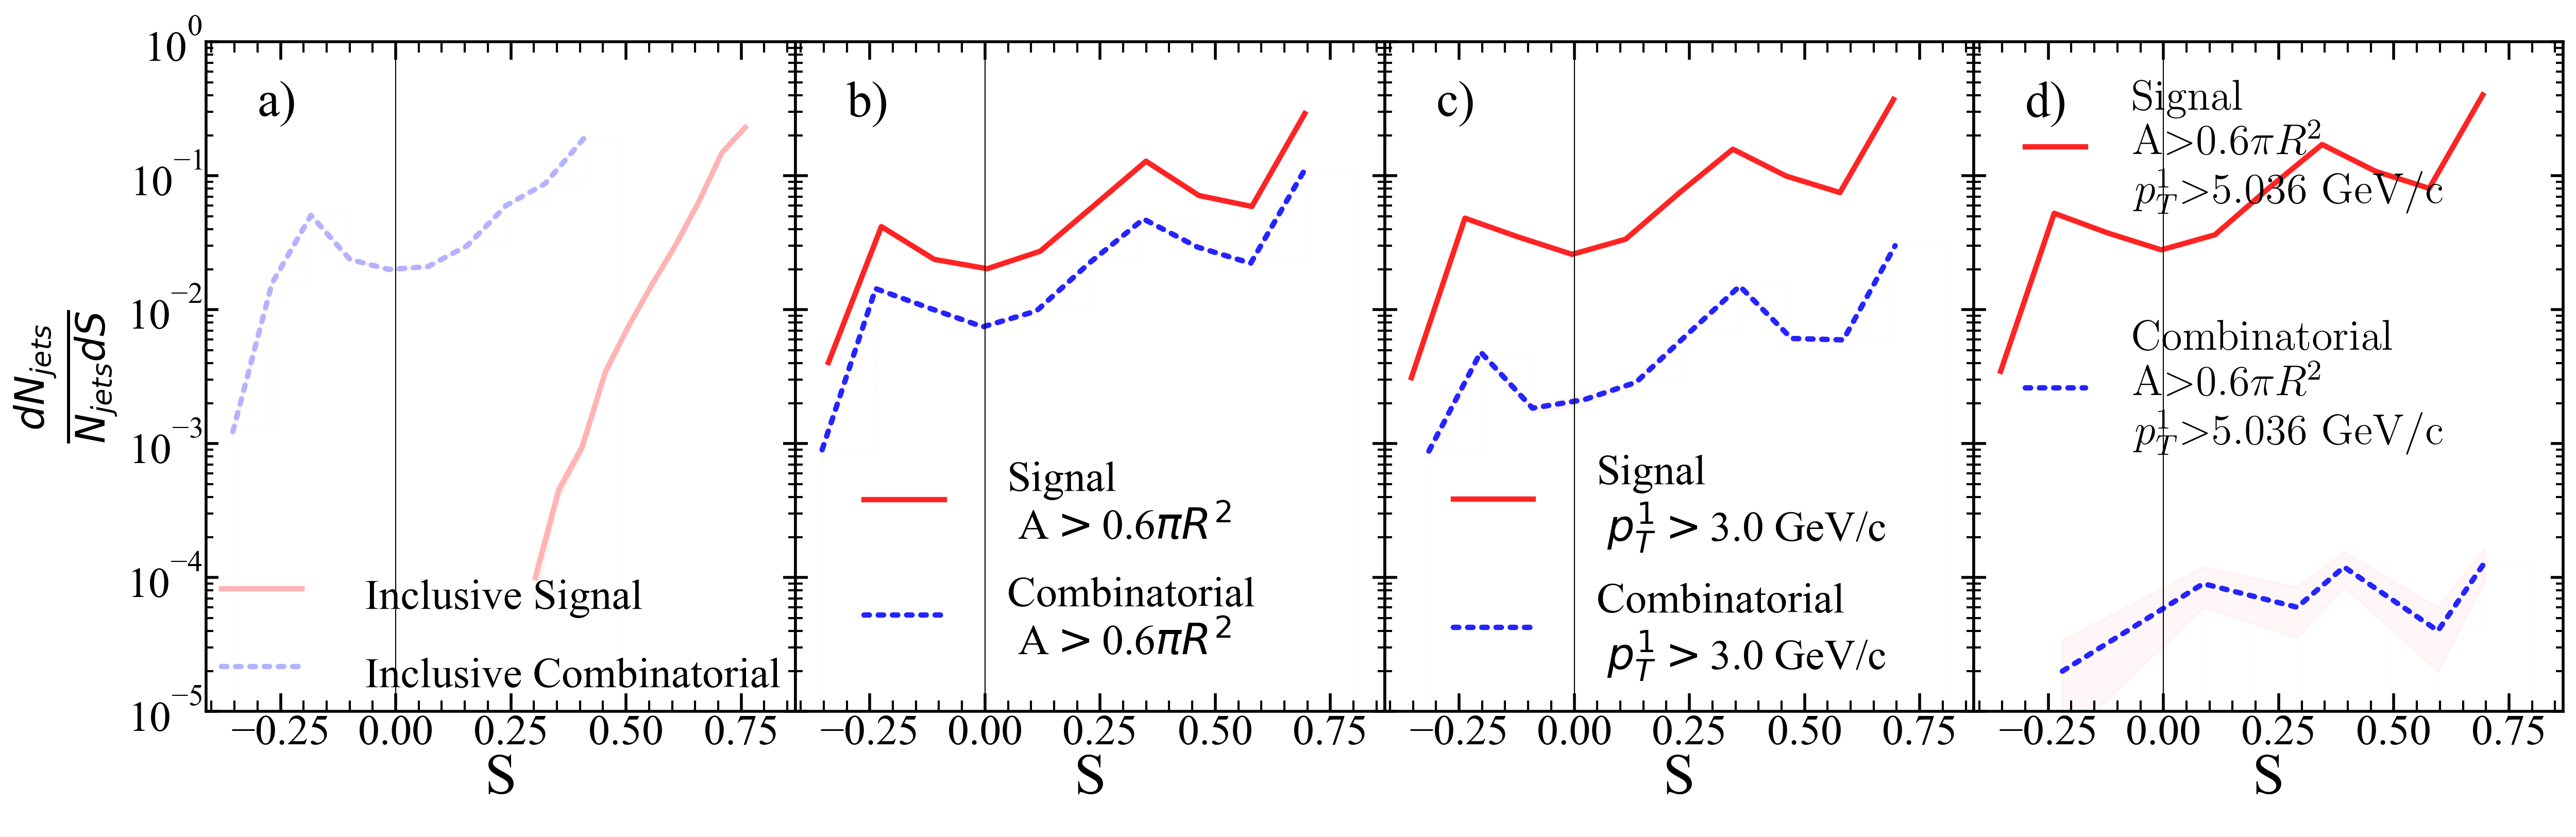}
    \caption{R=0.3 \ptH=80 \GeV}
    \label{fig:sil_03_80}
\end{figure*}

\begin{figure*}
    \centering
    \includegraphics[width=\linewidth]{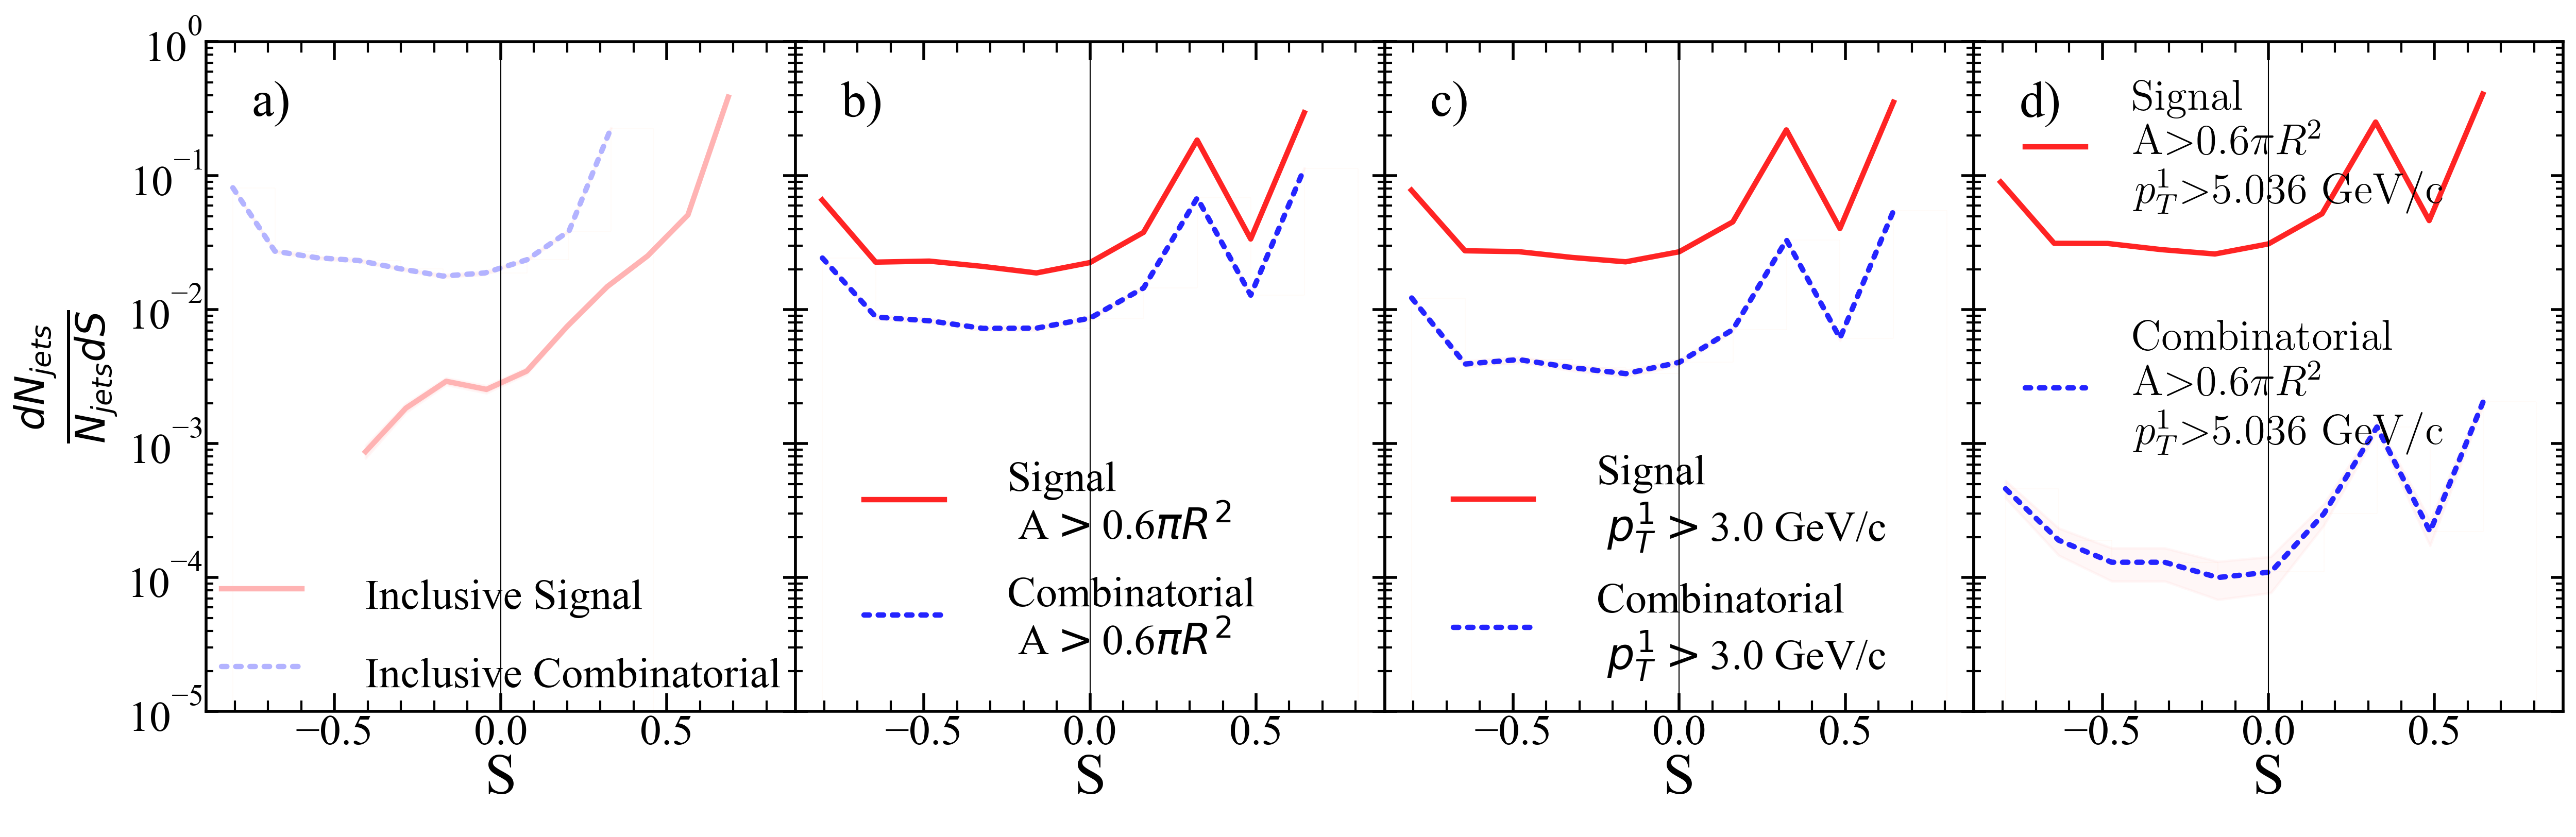}
    \caption{R=0.4 \ptH=10 \GeV}
    \label{fig:sil_04_10}
\end{figure*}

\begin{figure*}
    \centering
    \includegraphics[width=\linewidth]{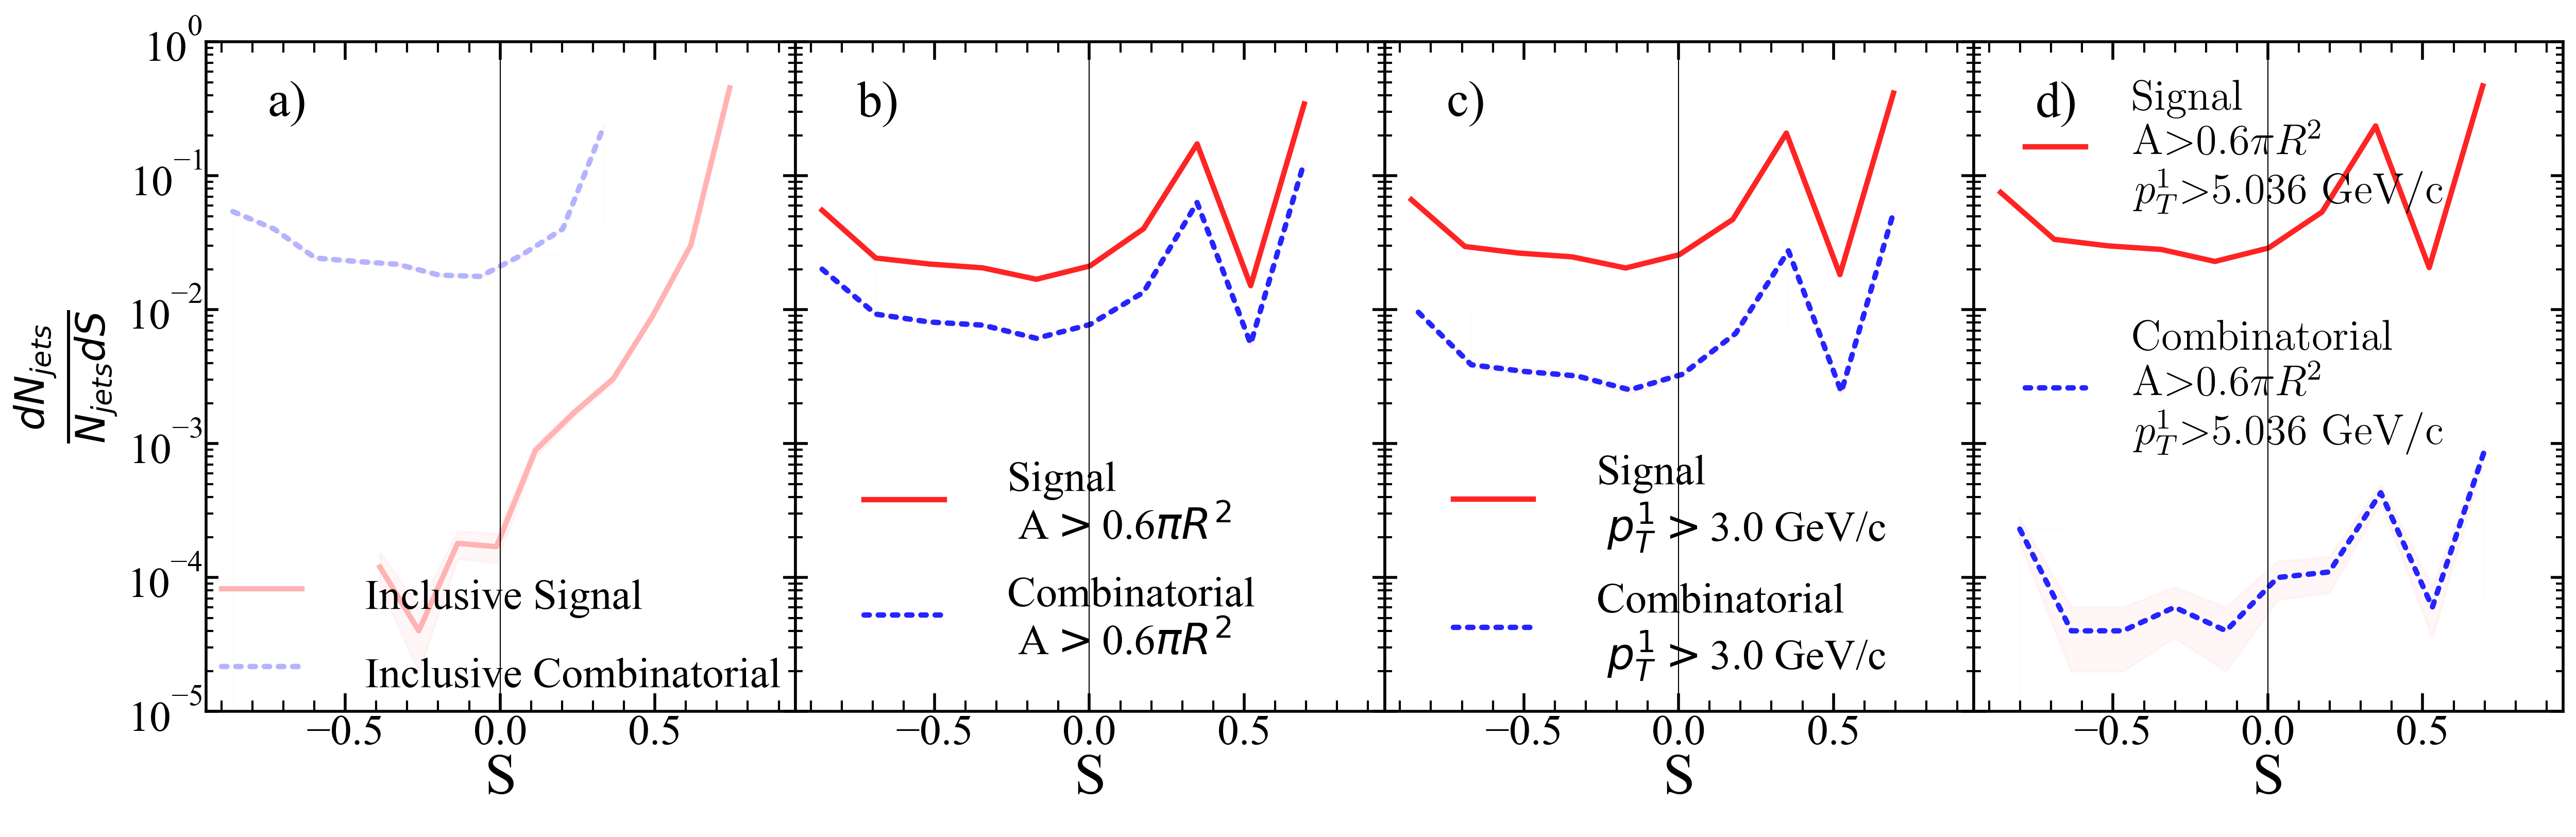}
    \caption{R=0.4 \ptH=20 \GeV}
    \label{fig:sil_04_20}
\end{figure*}

\begin{figure*}
    \centering
    \includegraphics[width=\linewidth]{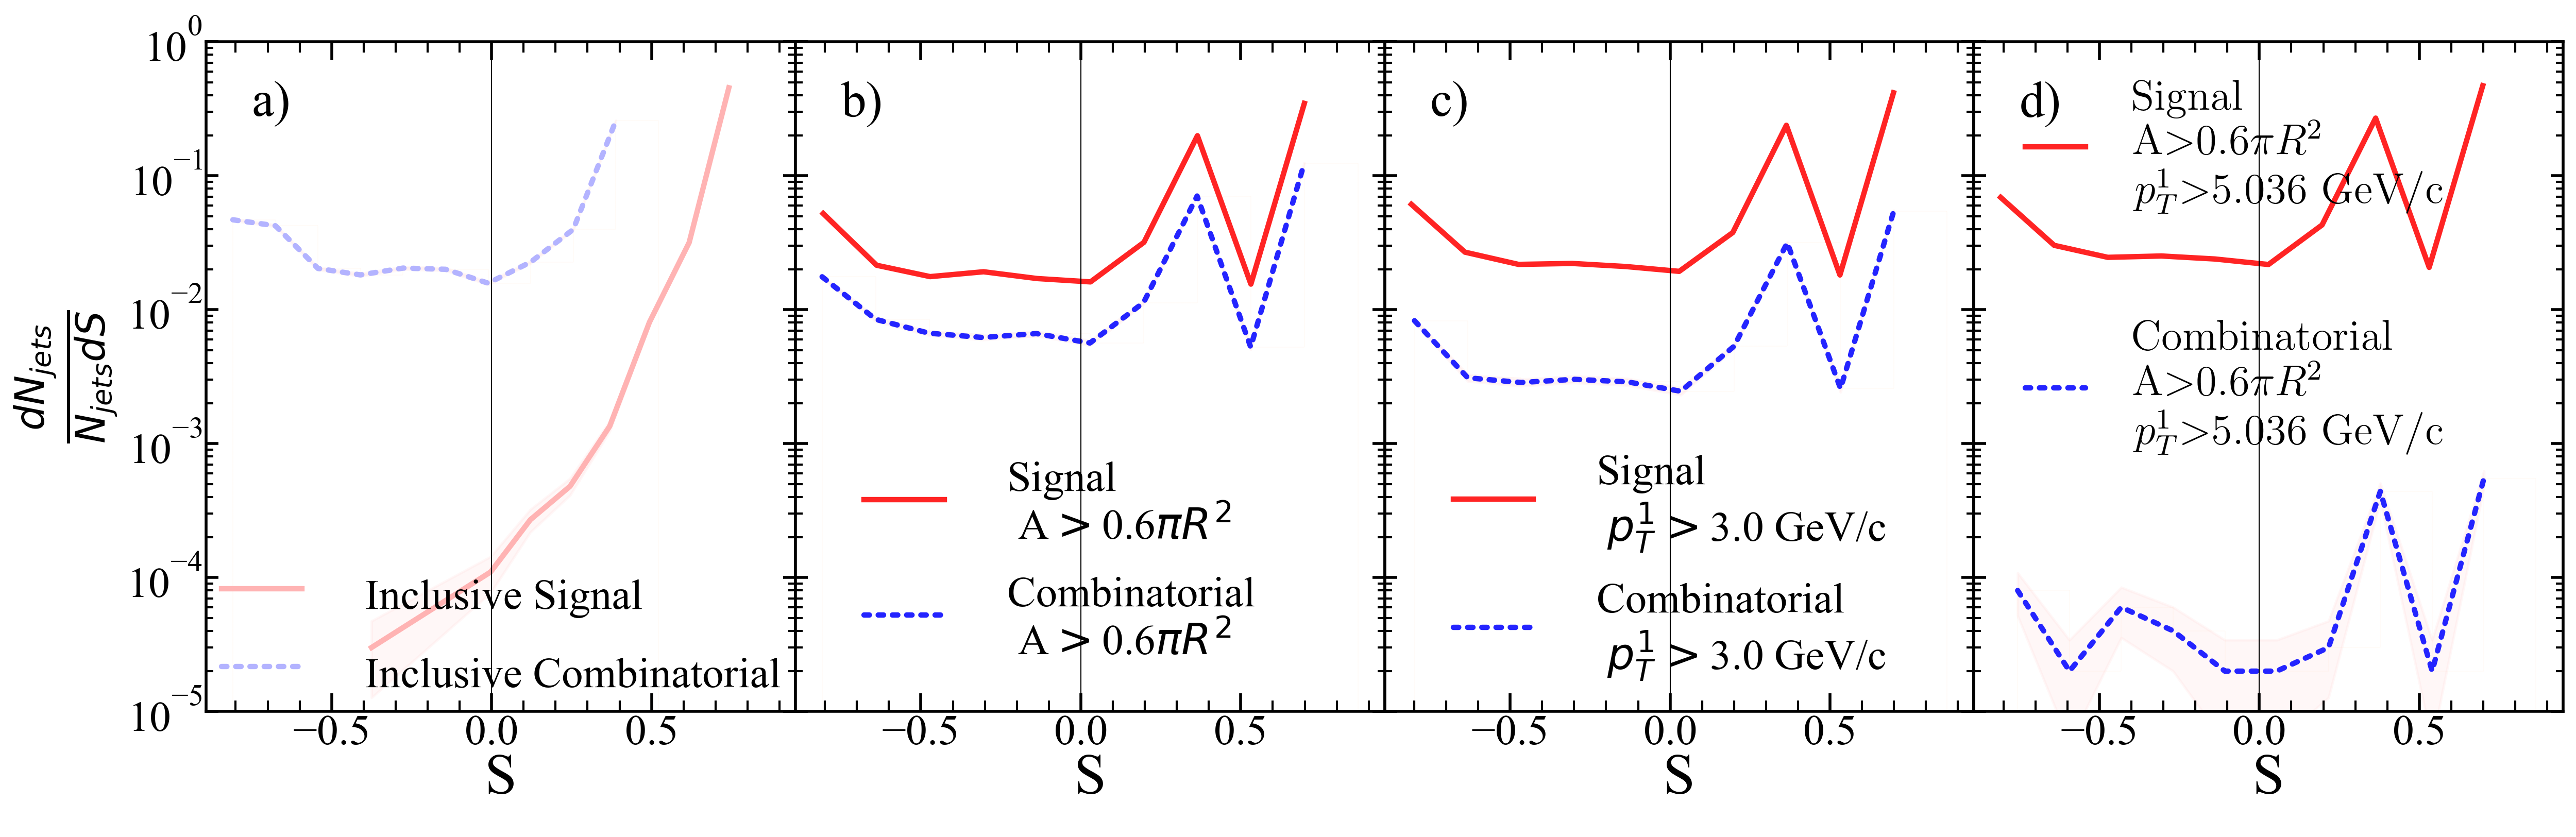}
    \caption{R=0.4 \ptH=30 \GeV}
    \label{fig:sil_04_30}
\end{figure*}

\begin{figure*}
    \centering
    \includegraphics[width=\linewidth]{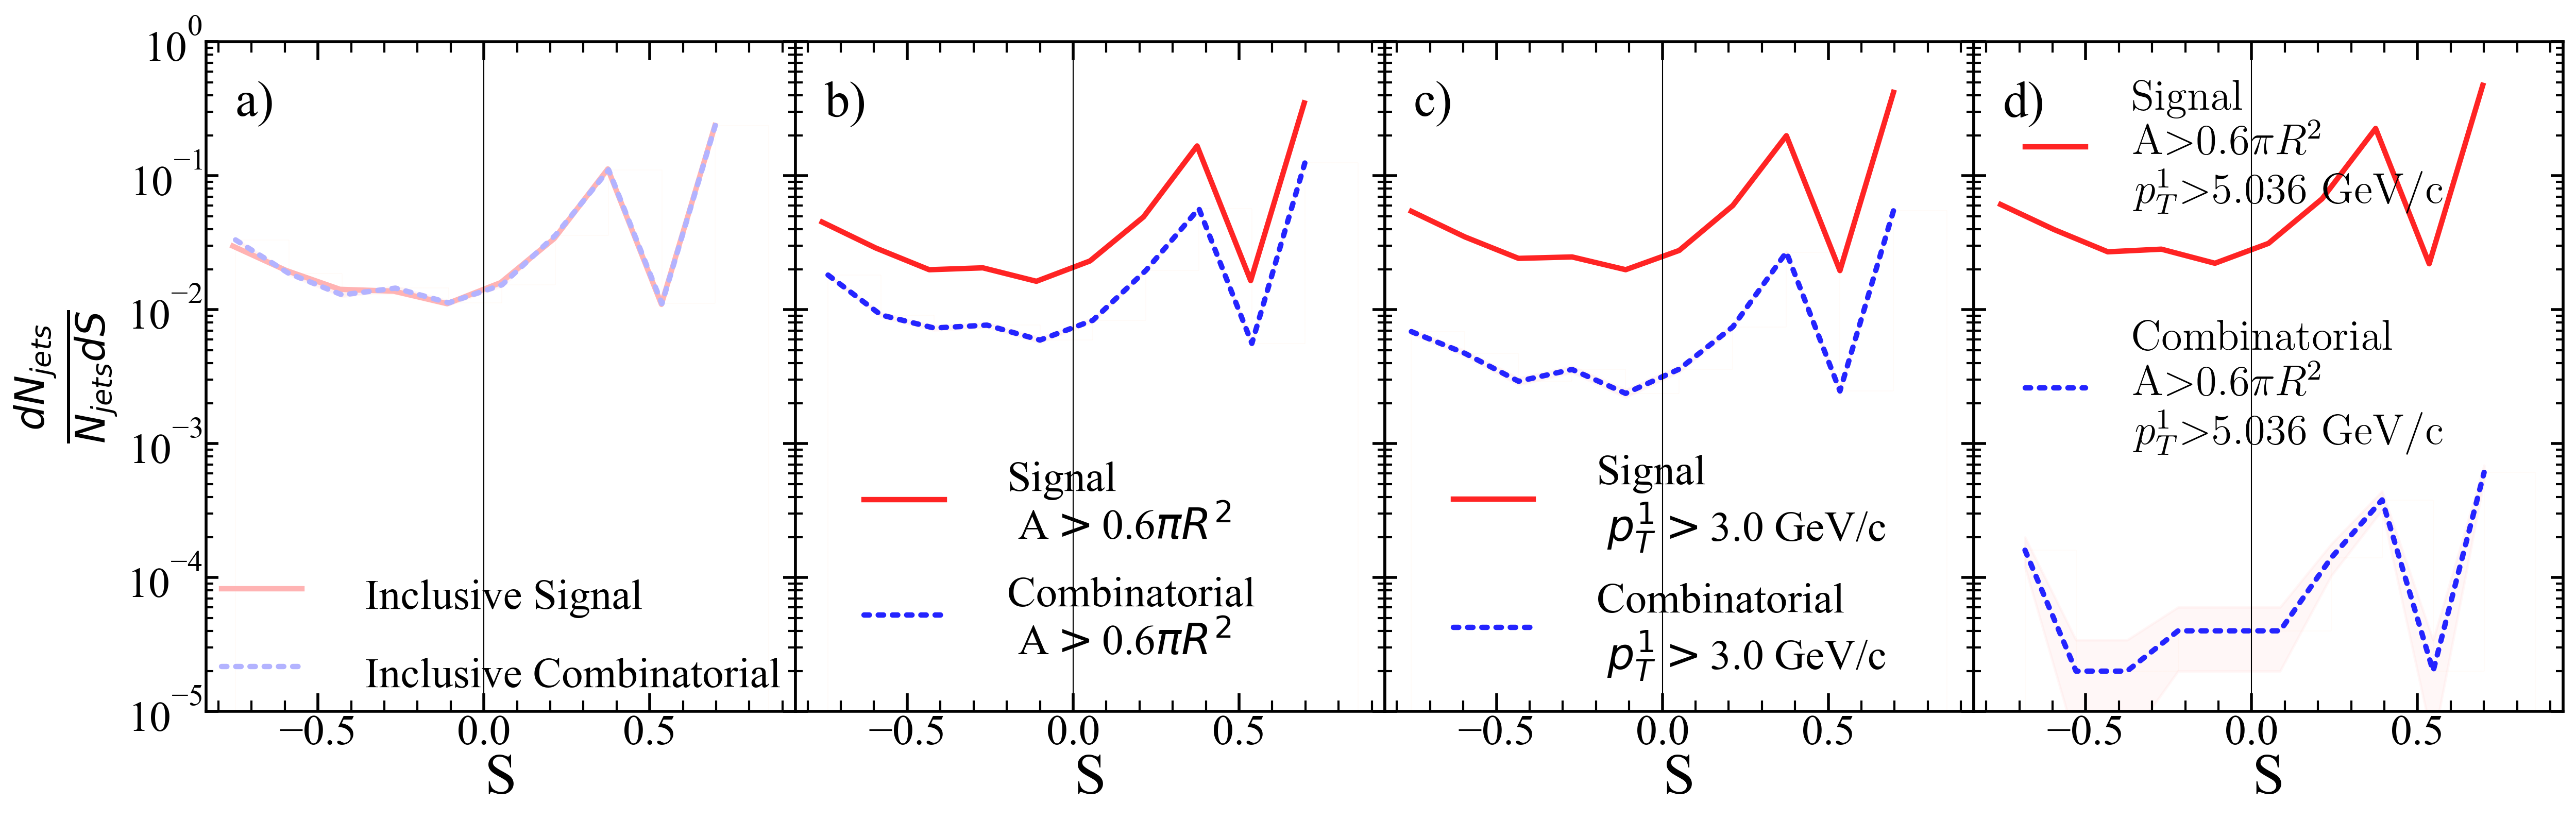}
    \caption{R=0.4 \ptH=40 \GeV}
    \label{fig:sil_04_40}
\end{figure*}

\begin{figure*}
    \centering
    \includegraphics[width=\linewidth]{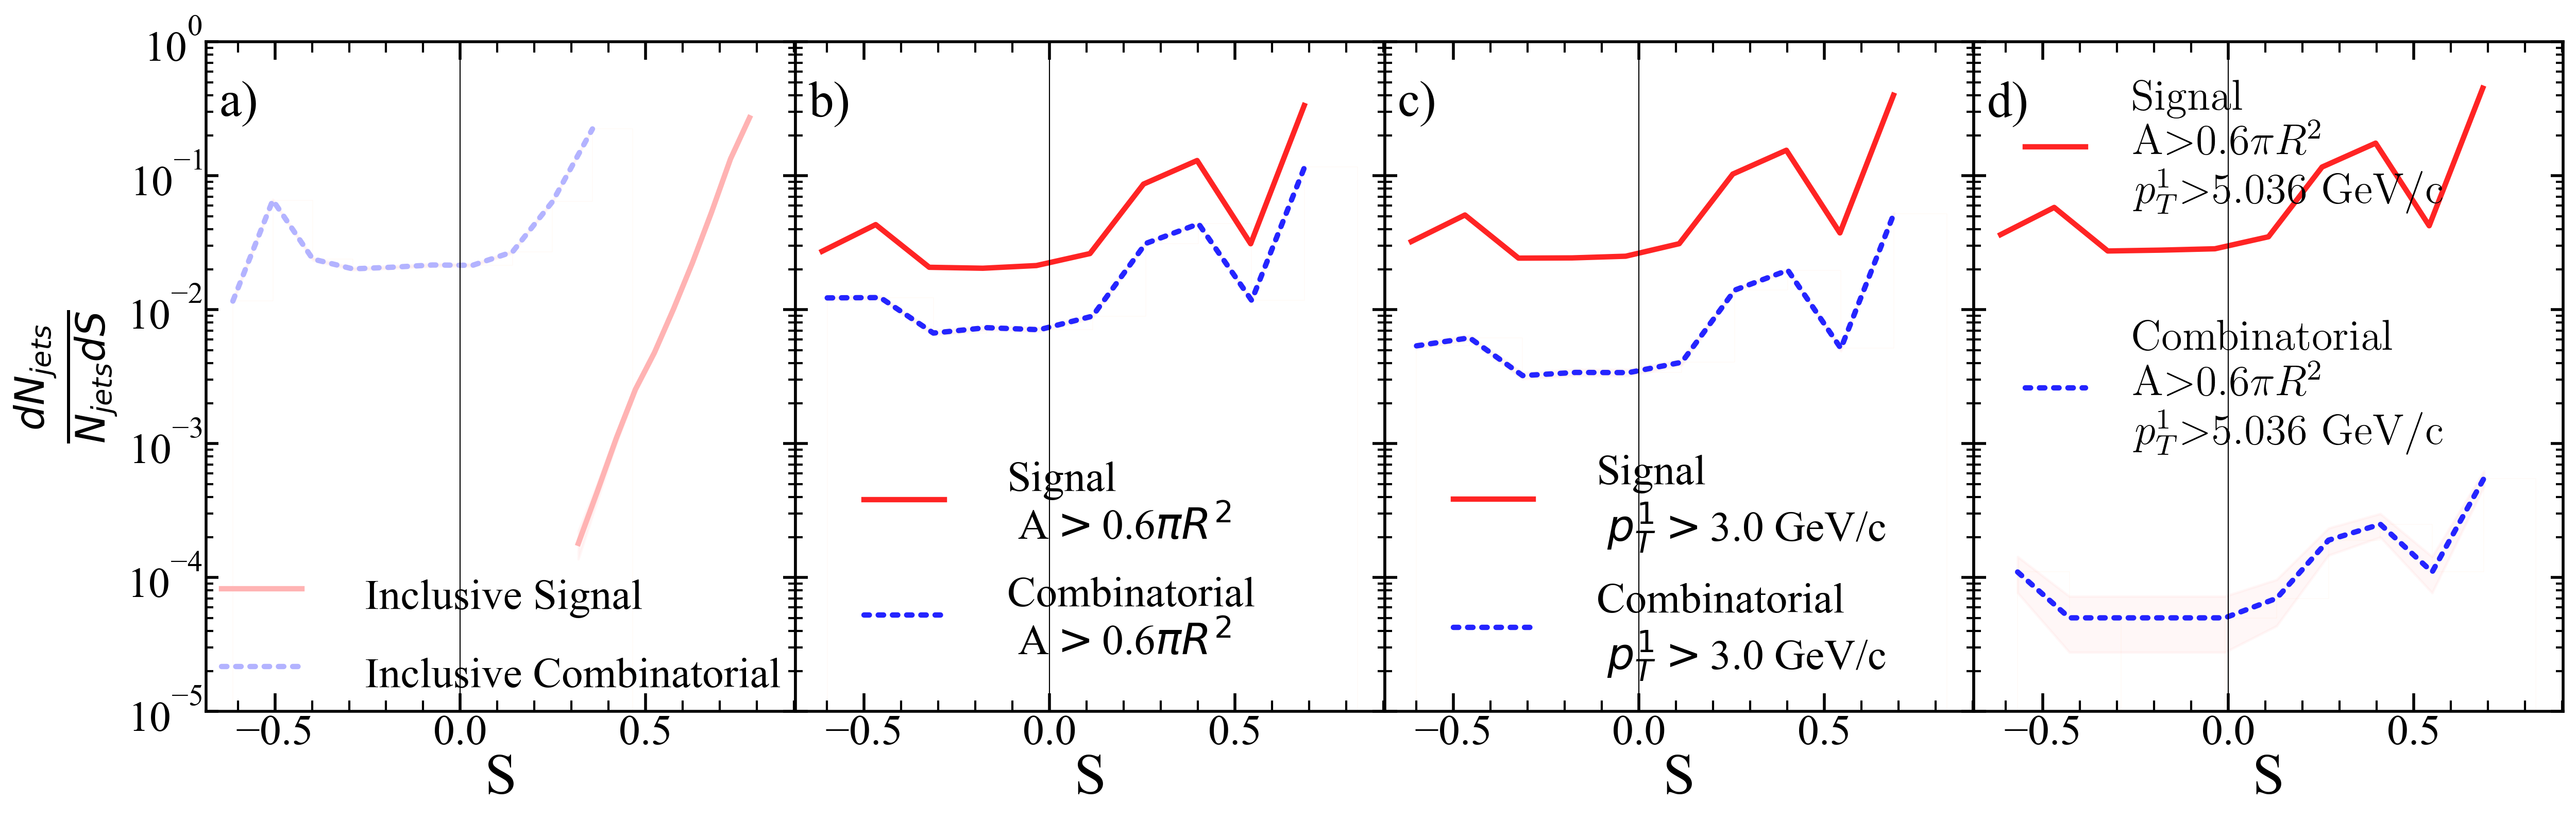}
    \caption{R=0.4 \ptH=60 \GeV}
    \label{fig:sil_04_60}
\end{figure*}

\begin{figure*}
    \centering
    \includegraphics[width=\linewidth]{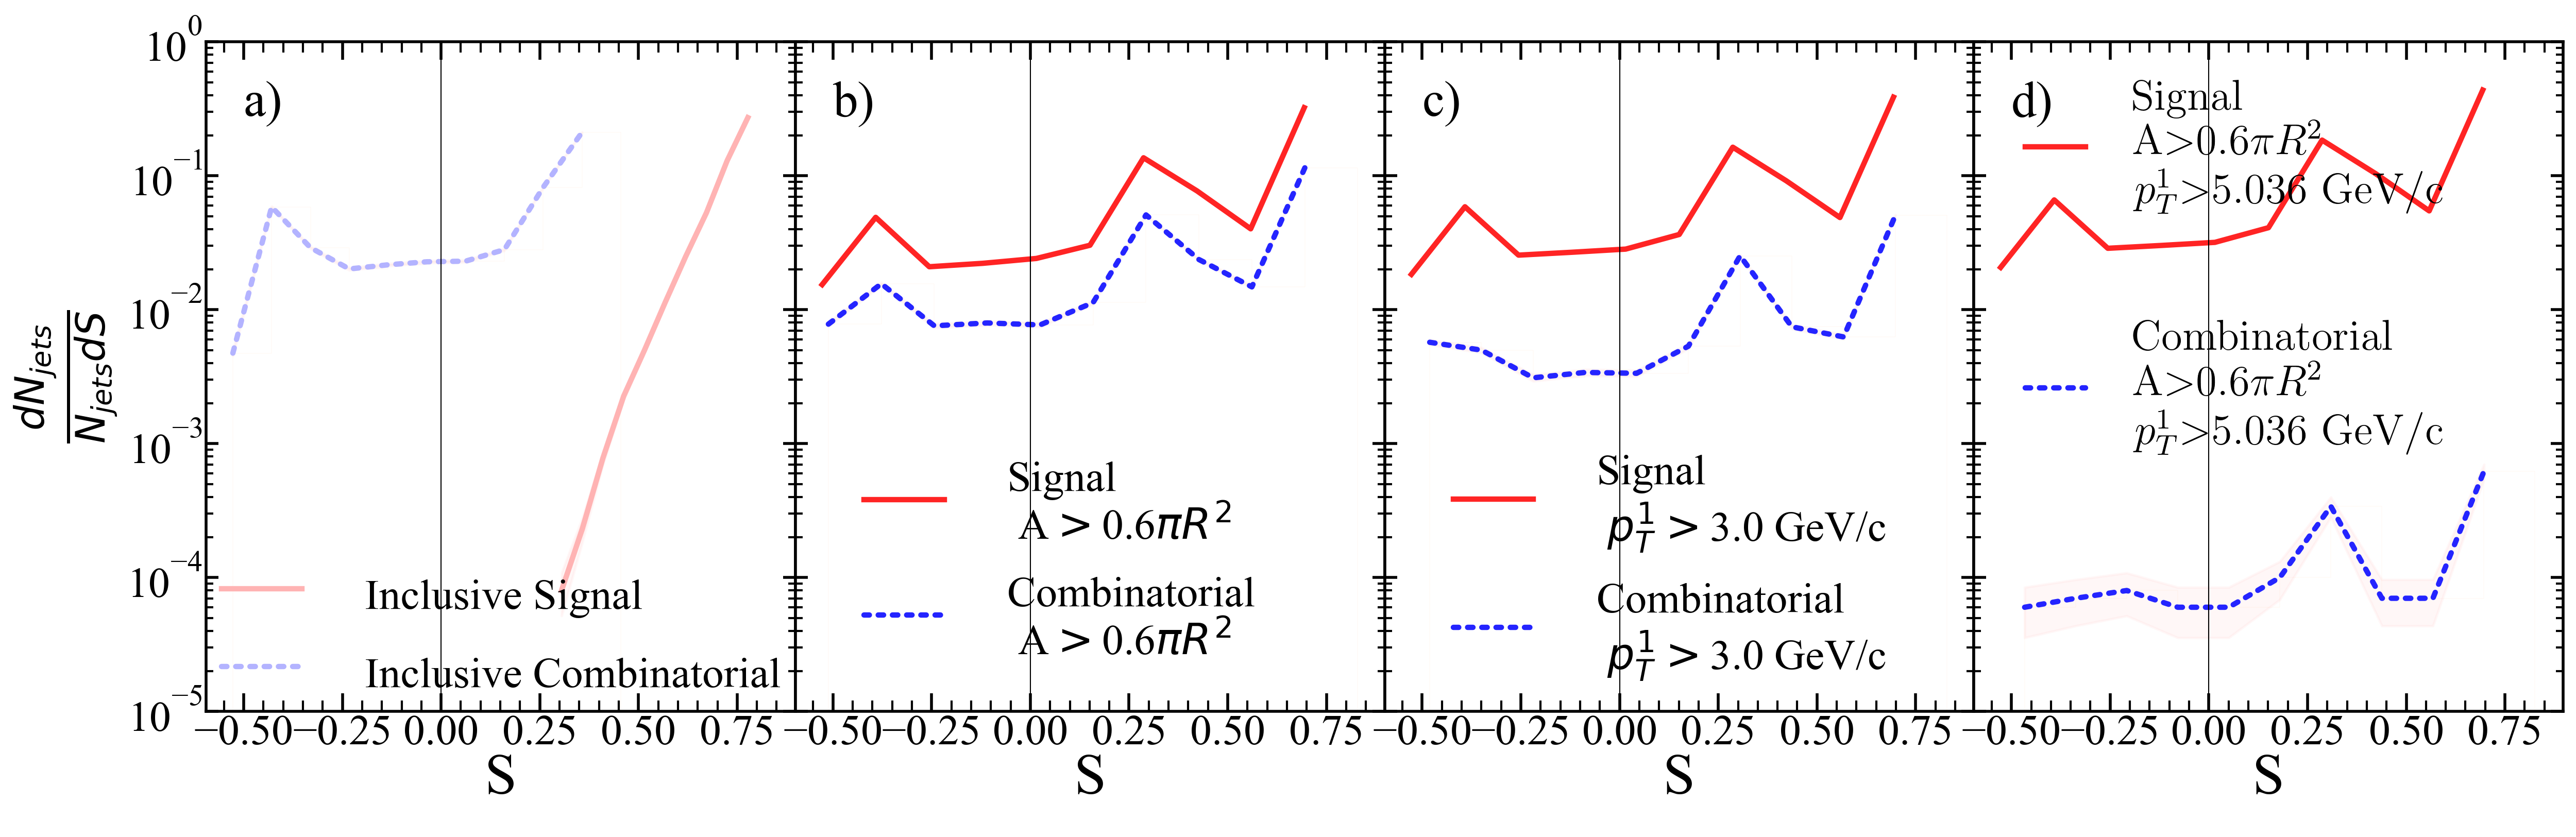}
    \caption{R=0.4 \ptH=80 \GeV}
    \label{fig:sil_04_80}
\end{figure*}

\begin{figure*}
    \centering
    \includegraphics[width=\linewidth]{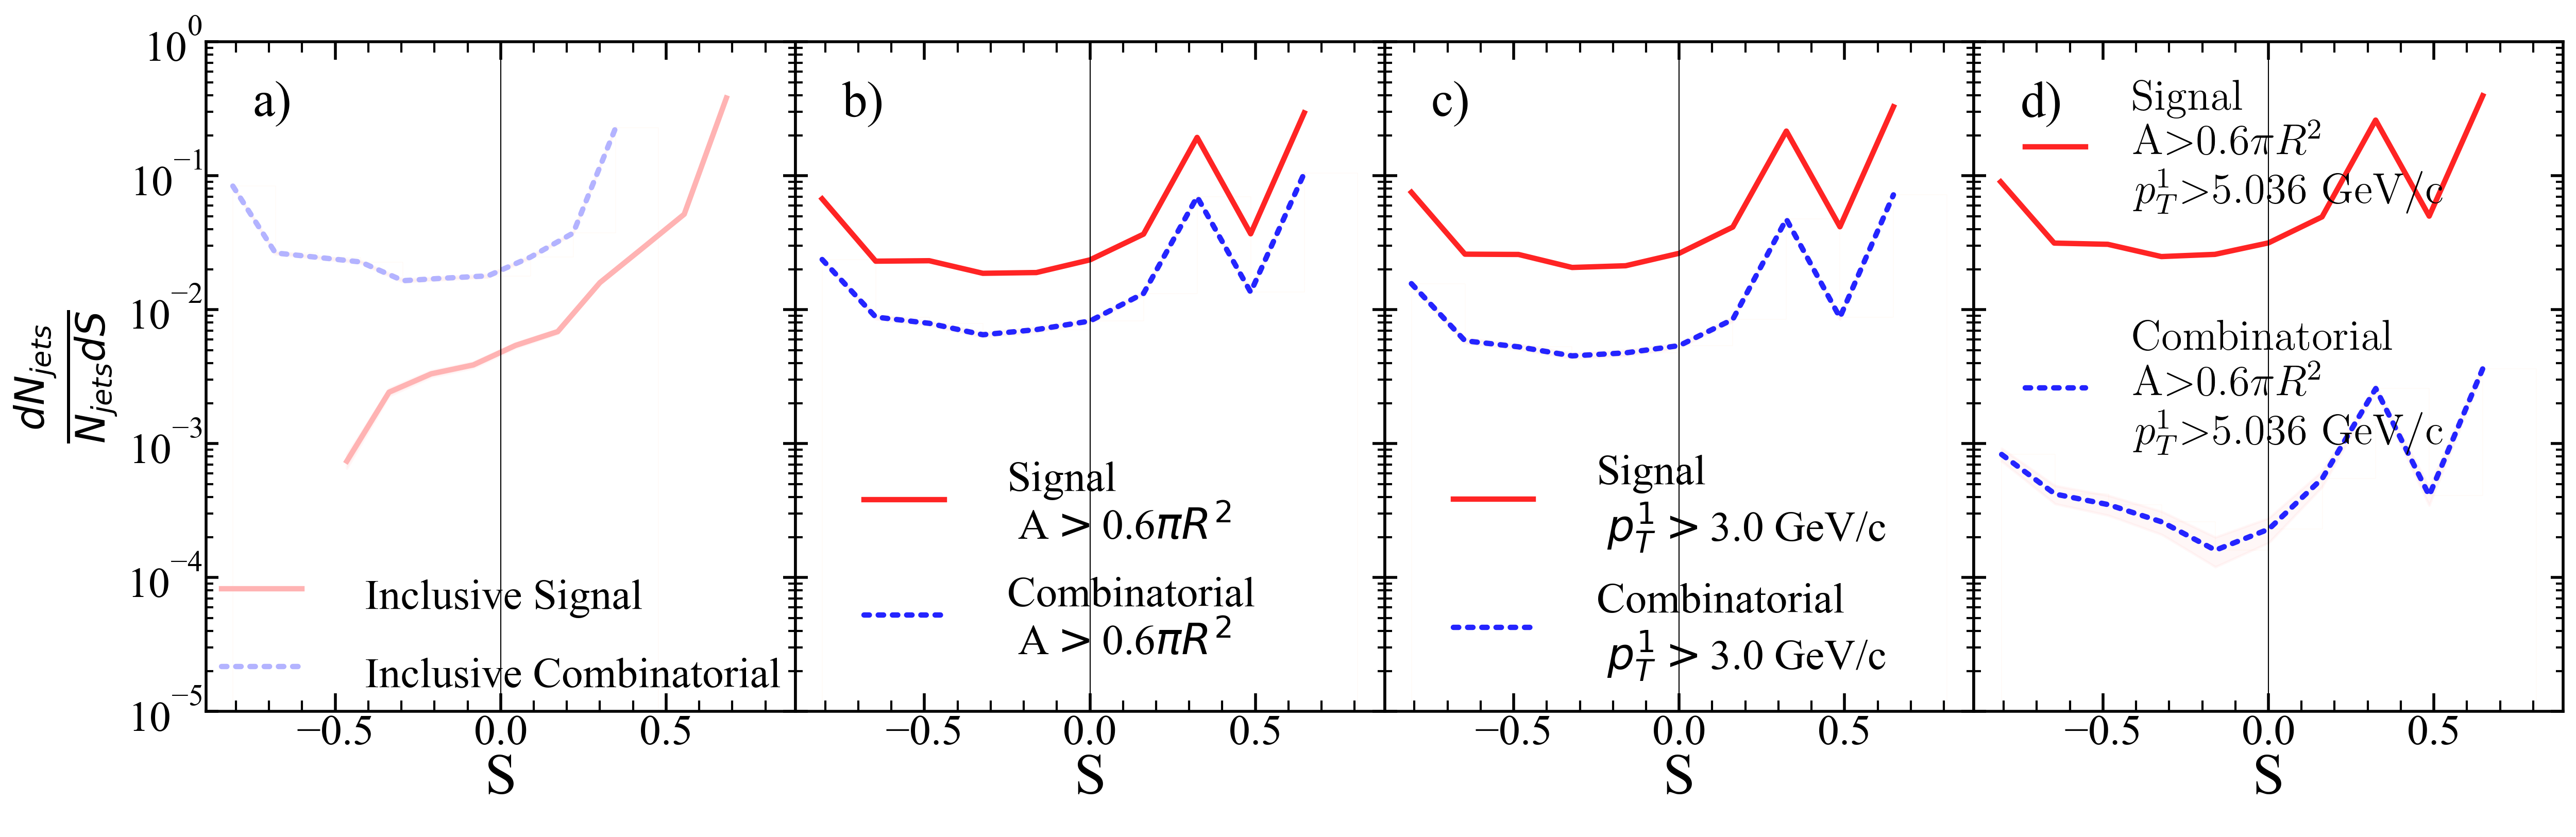}
    \caption{R=0.5 \ptH=10 \GeV}
    \label{fig:sil_05_10}
\end{figure*}

\begin{figure*}
    \centering
    \includegraphics[width=\linewidth]{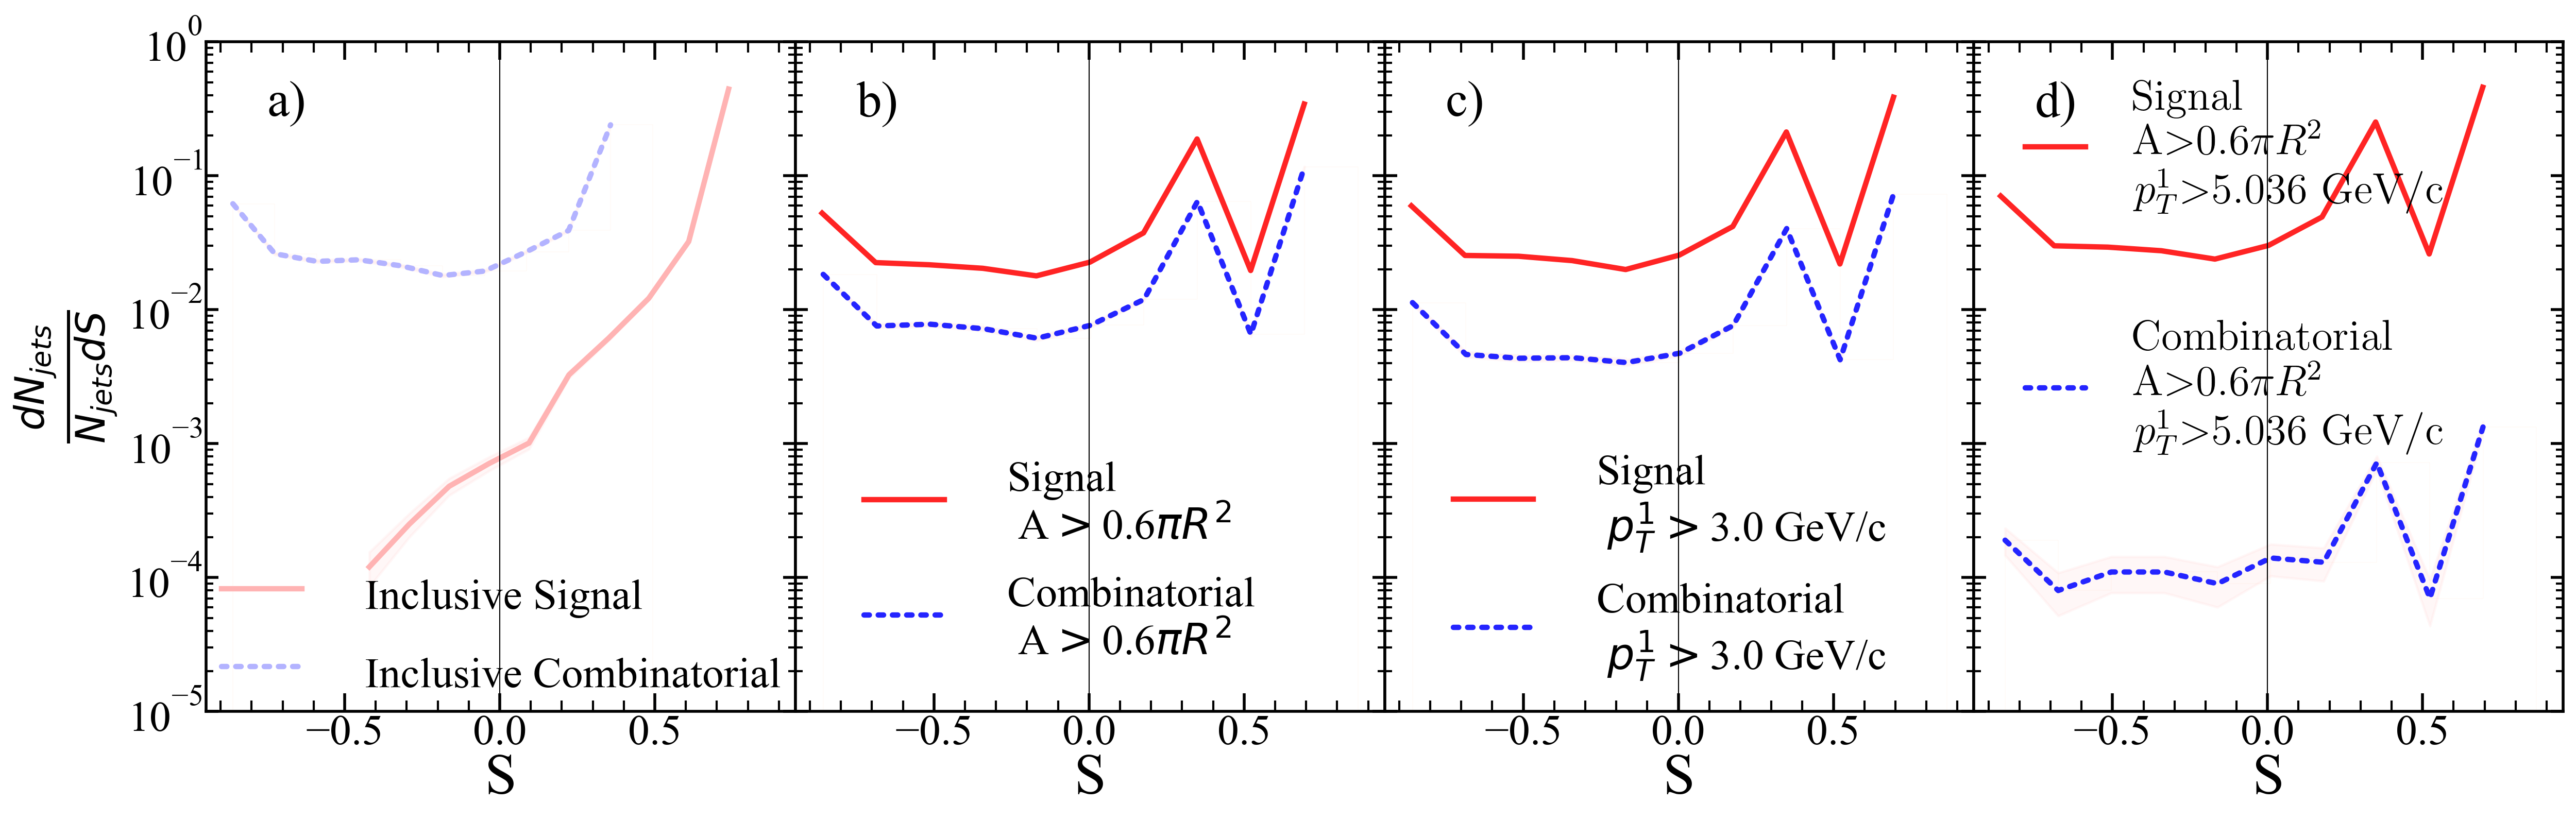}
    \caption{R=0.5 \ptH=20 \GeV}
    \label{fig:sil_05_20}
\end{figure*}

\begin{figure*}
    \centering
    \includegraphics[width=\linewidth]{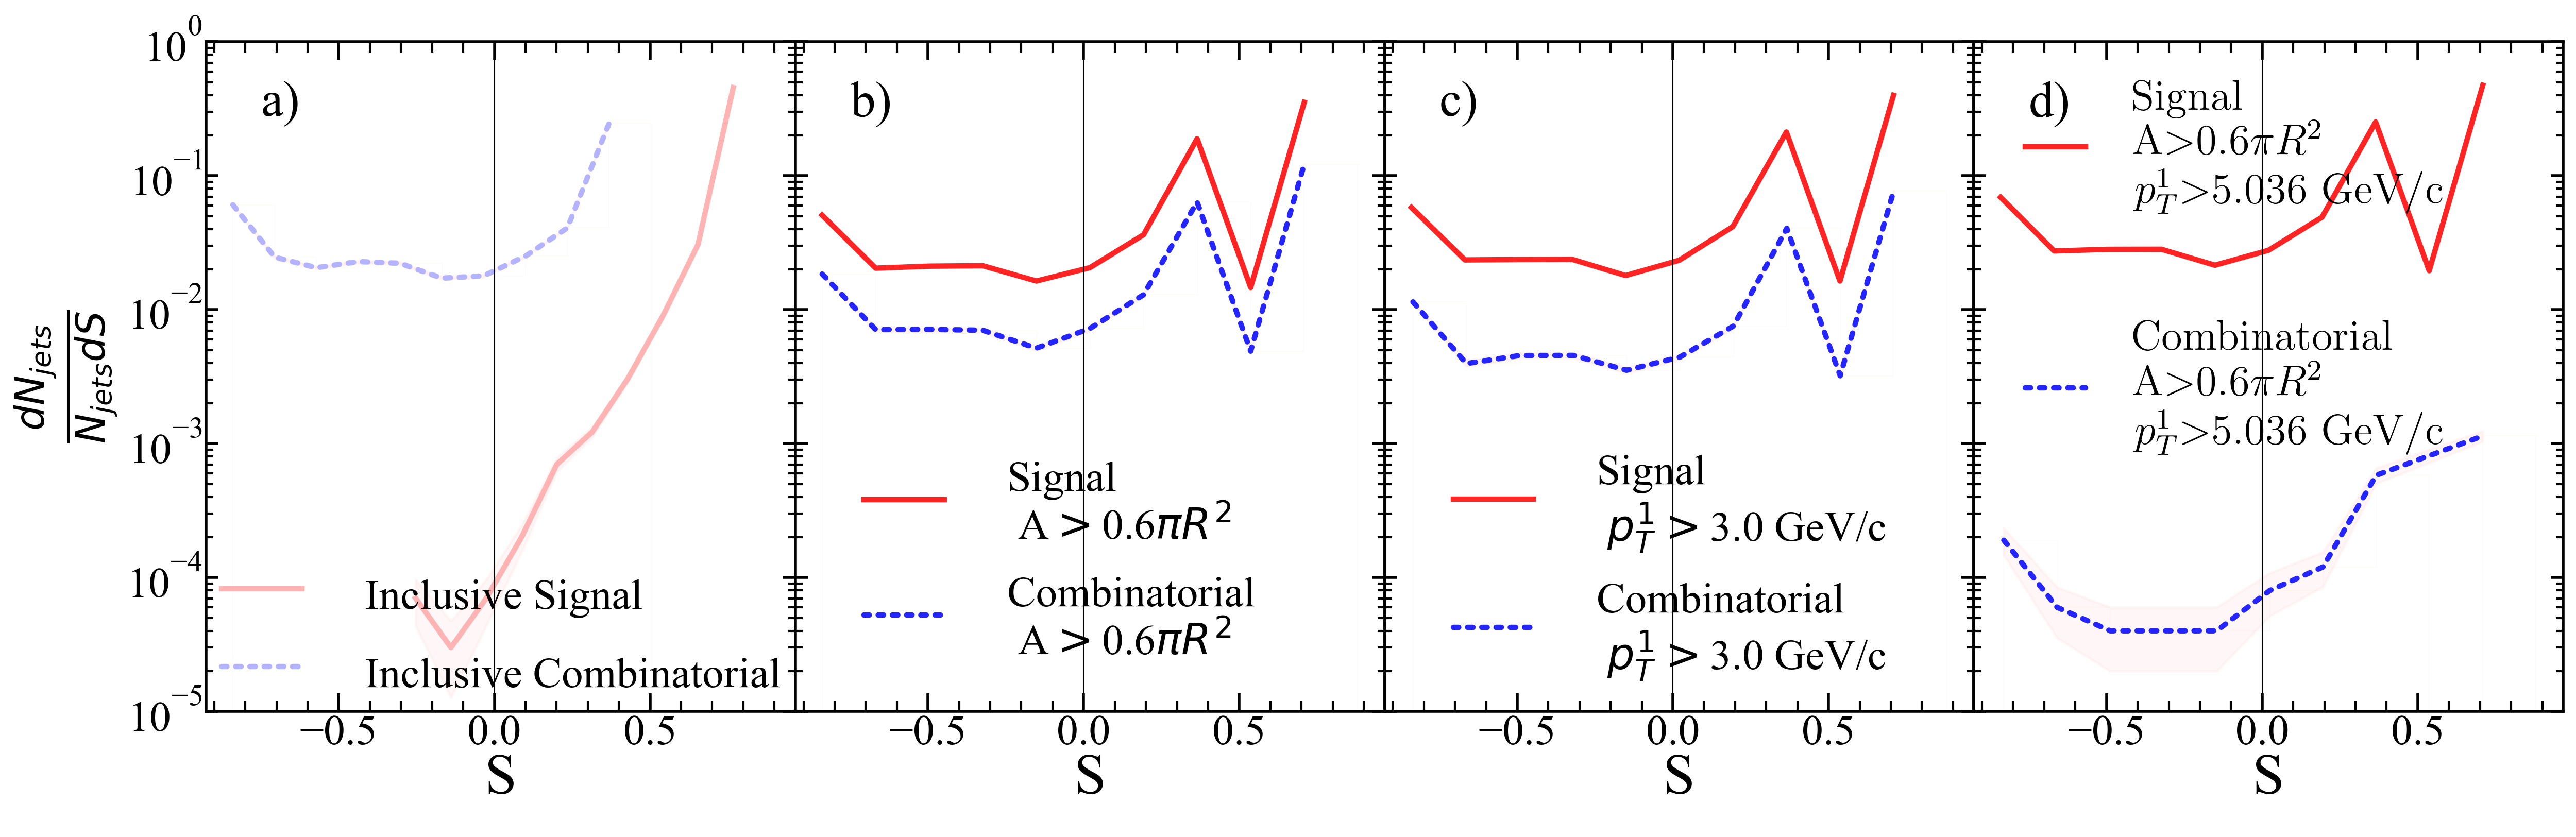}
    \caption{R=0.5 \ptH=30 \GeV}
    \label{fig:sil_05_30}
\end{figure*}

\begin{figure*}
    \centering
    \includegraphics[width=\linewidth]{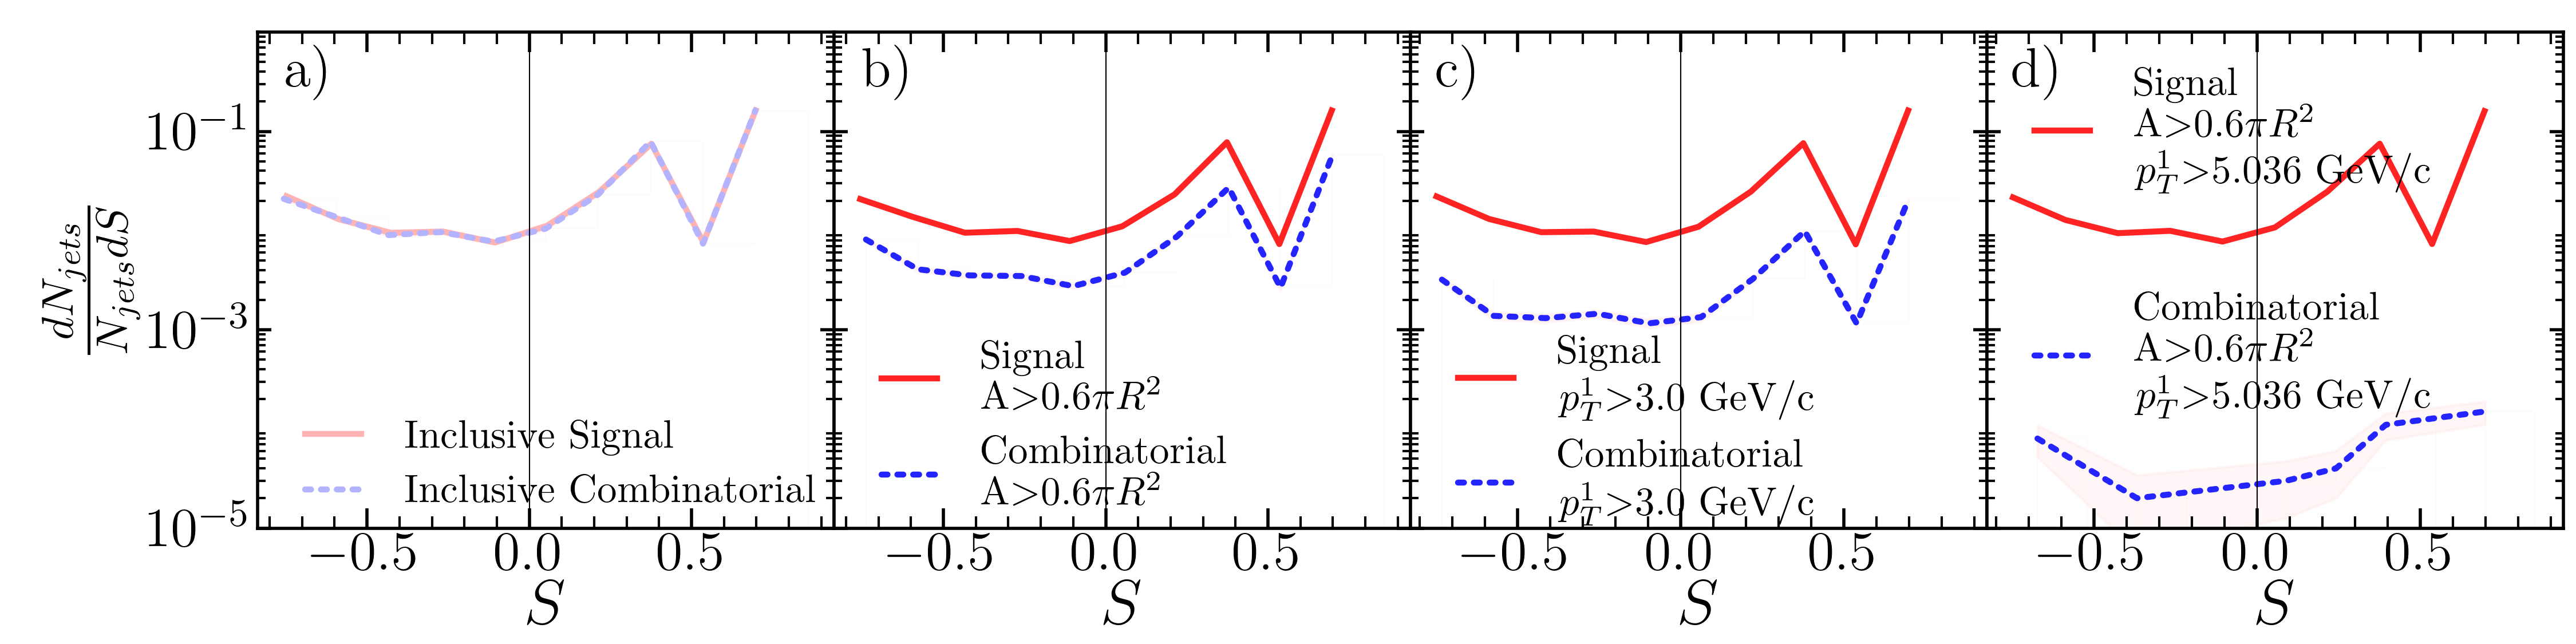}
    \caption{R=0.5 \ptH=40 \GeV}
    \label{fig:sil_05_40}
\end{figure*}

\begin{figure*}
    \centering
    \includegraphics[width=\linewidth]{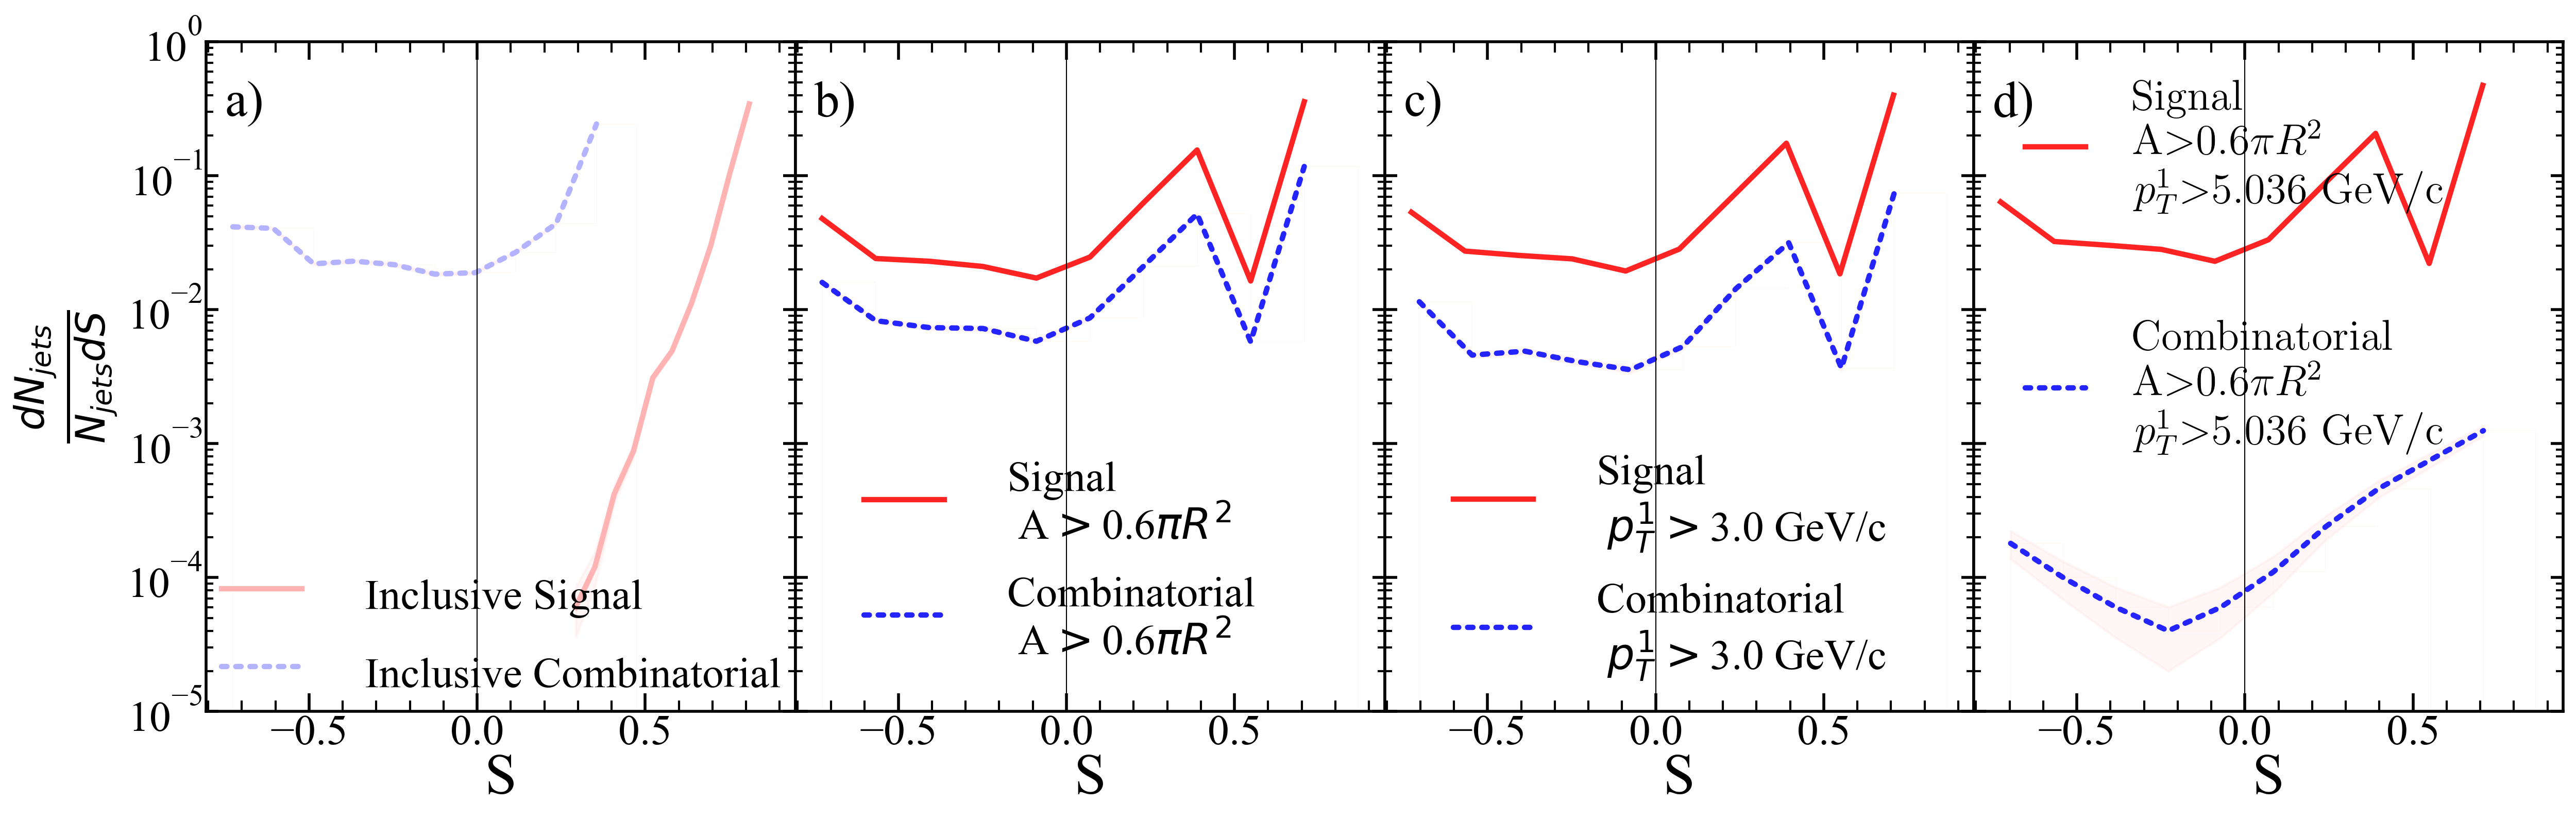}
    \caption{R=0.5 \ptH=60 \GeV}
    \label{fig:sil_05_60}
\end{figure*}

\begin{figure*}
    \centering
    \includegraphics[width=\linewidth]{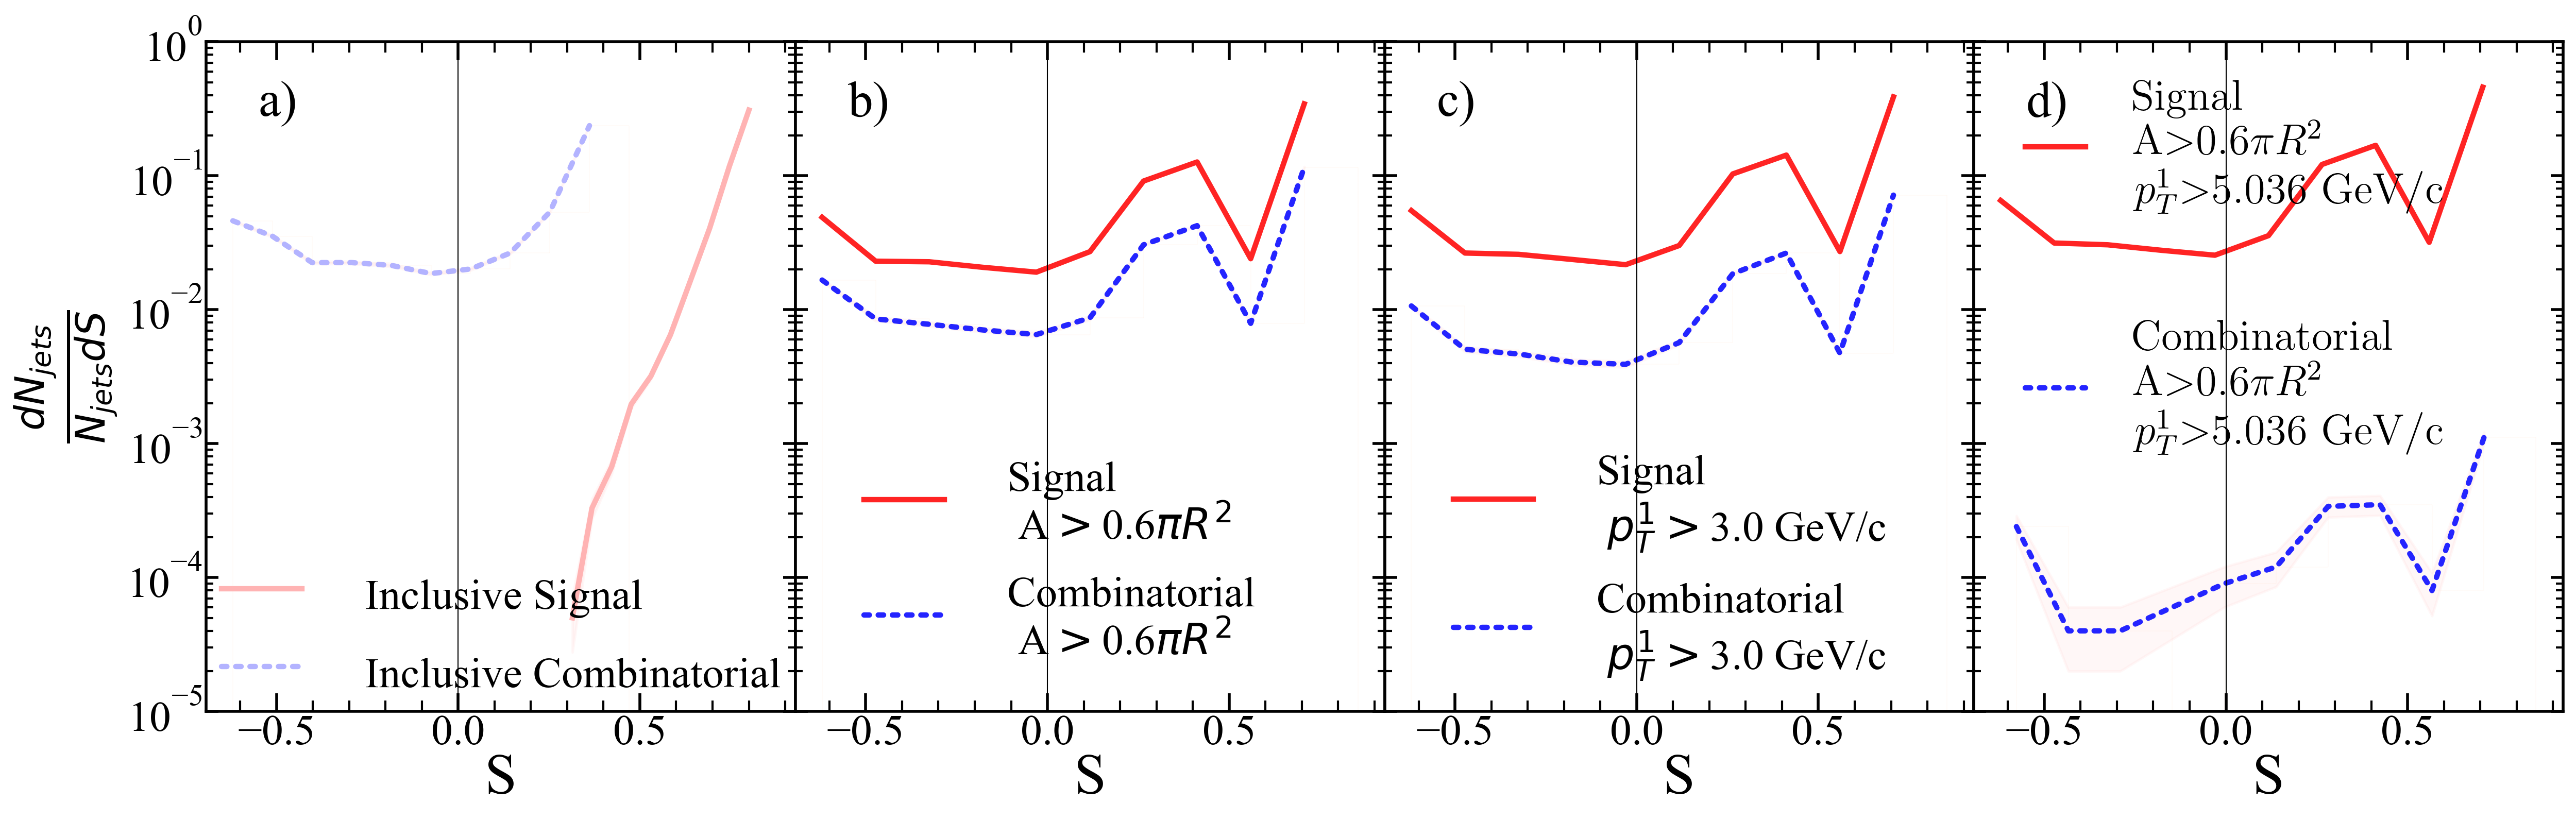}
    \caption{R=0.5 \ptH=80 \GeV}
    \label{fig:sil_05_80}
\end{figure*}

\begin{figure*}
    \centering
    \includegraphics[width=\linewidth]{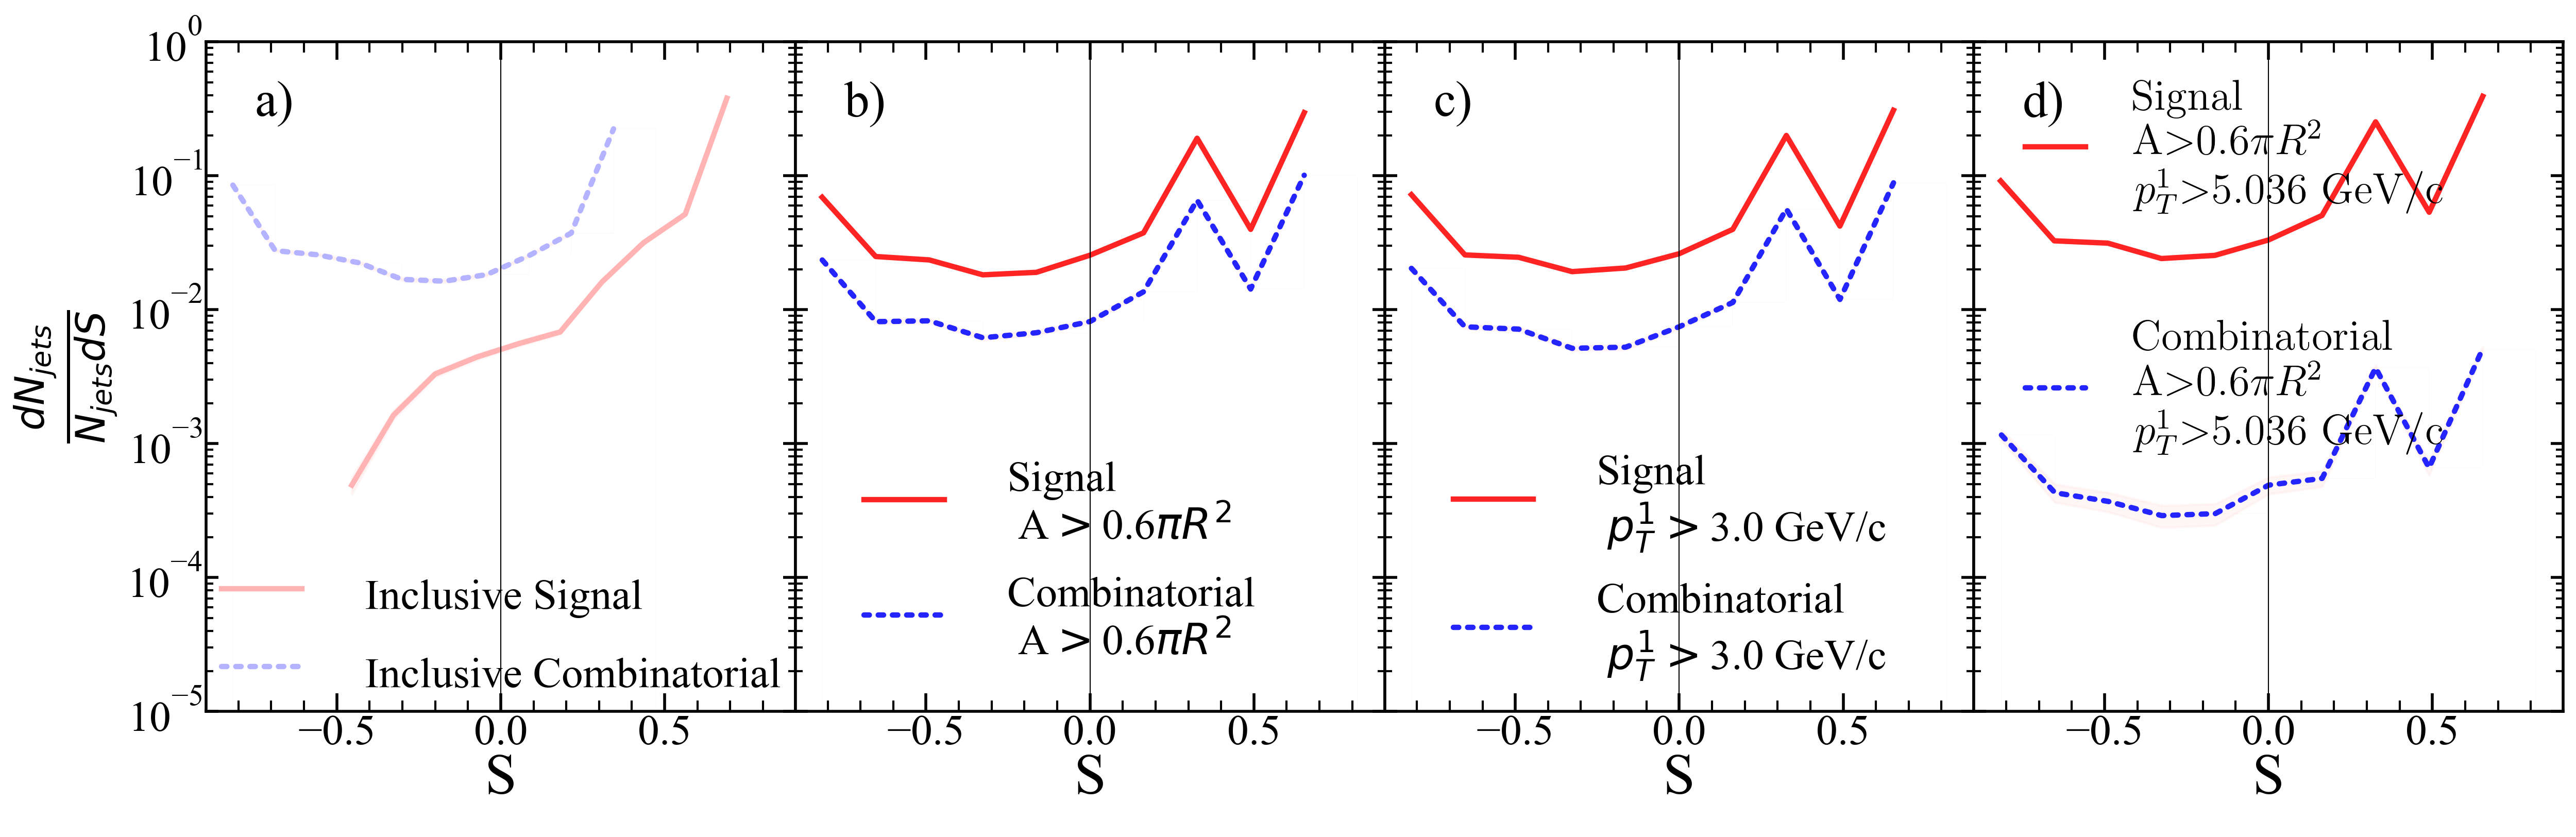}
    \caption{R=0.6 \ptH=10 \GeV}
    \label{fig:sil_06_10}
\end{figure*}

\begin{figure*}
    \centering
    \includegraphics[width=\linewidth]{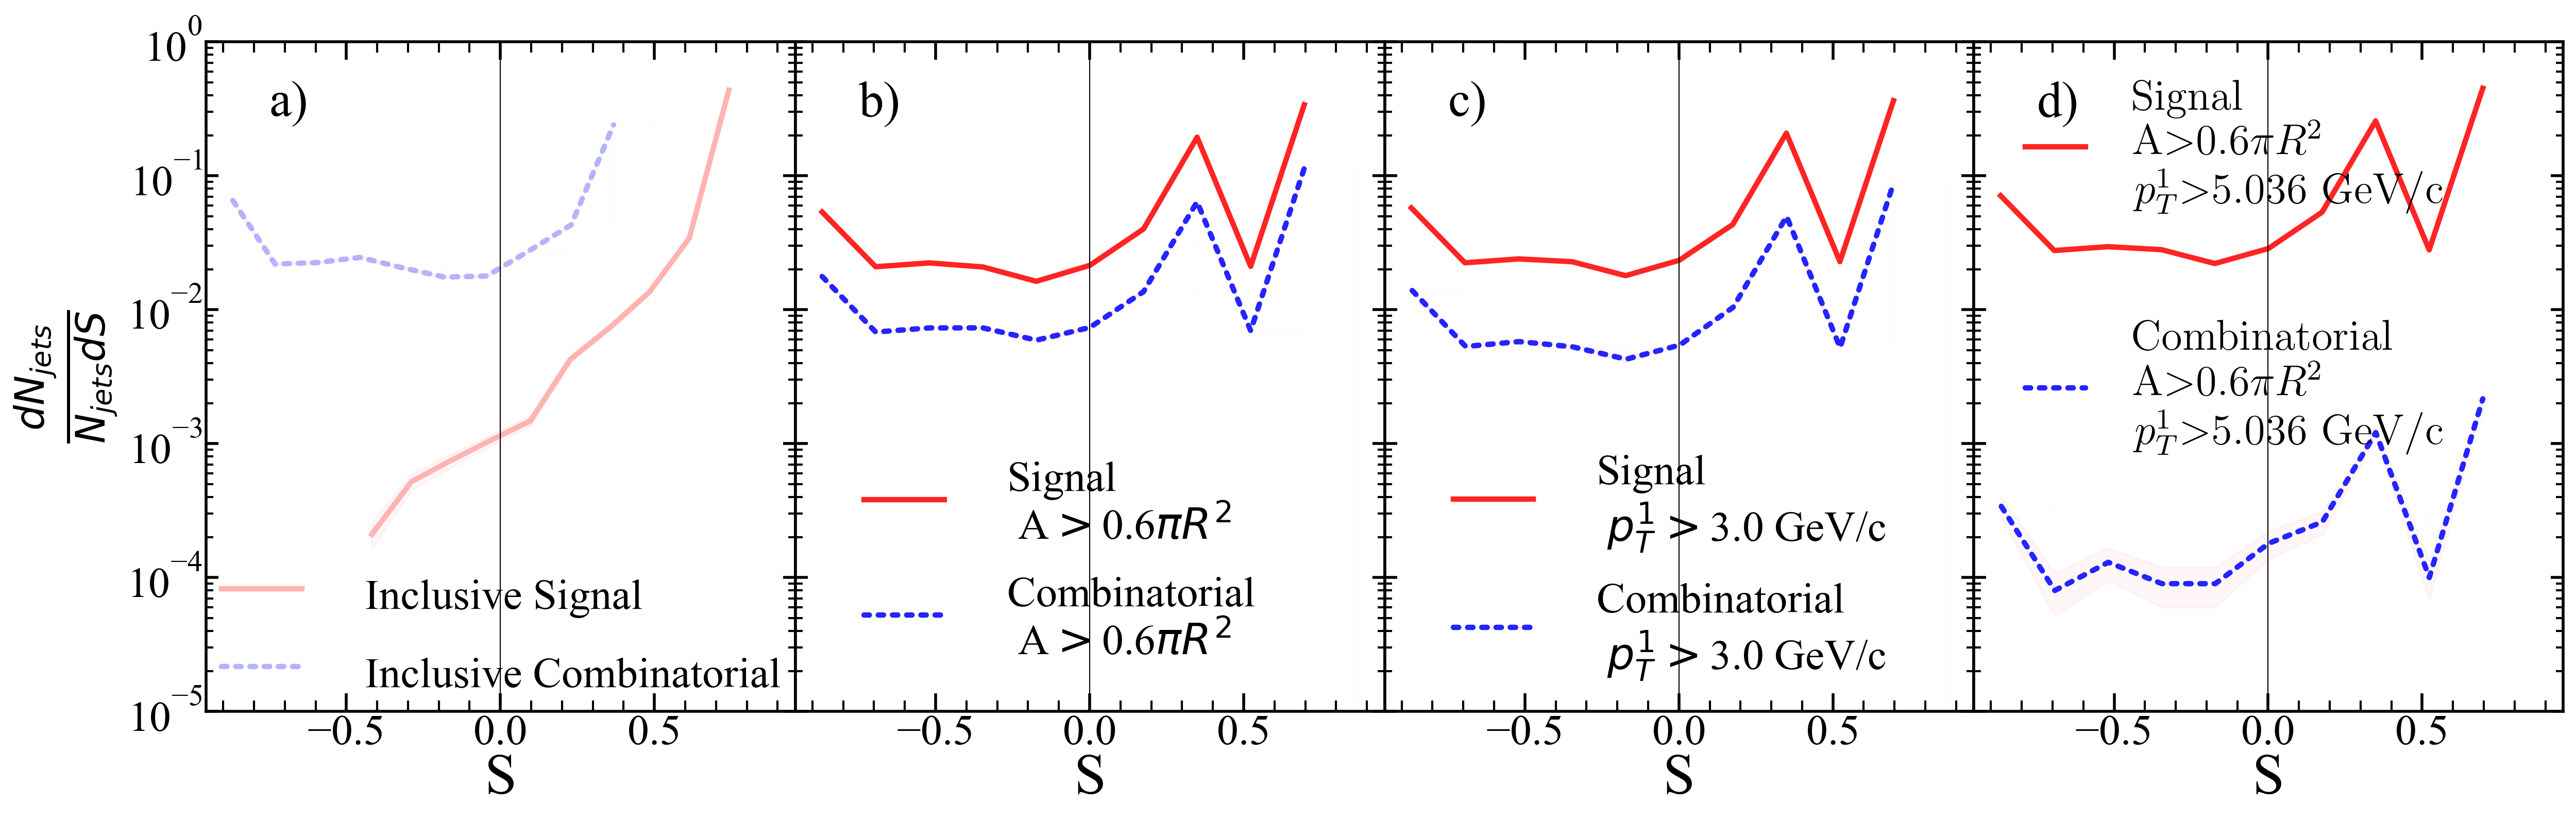}
    \caption{R=0.6 \ptH=20 \GeV}
    \label{fig:sil_06_20}
\end{figure*}

\begin{figure*}
    \centering
    \includegraphics[width=\linewidth]{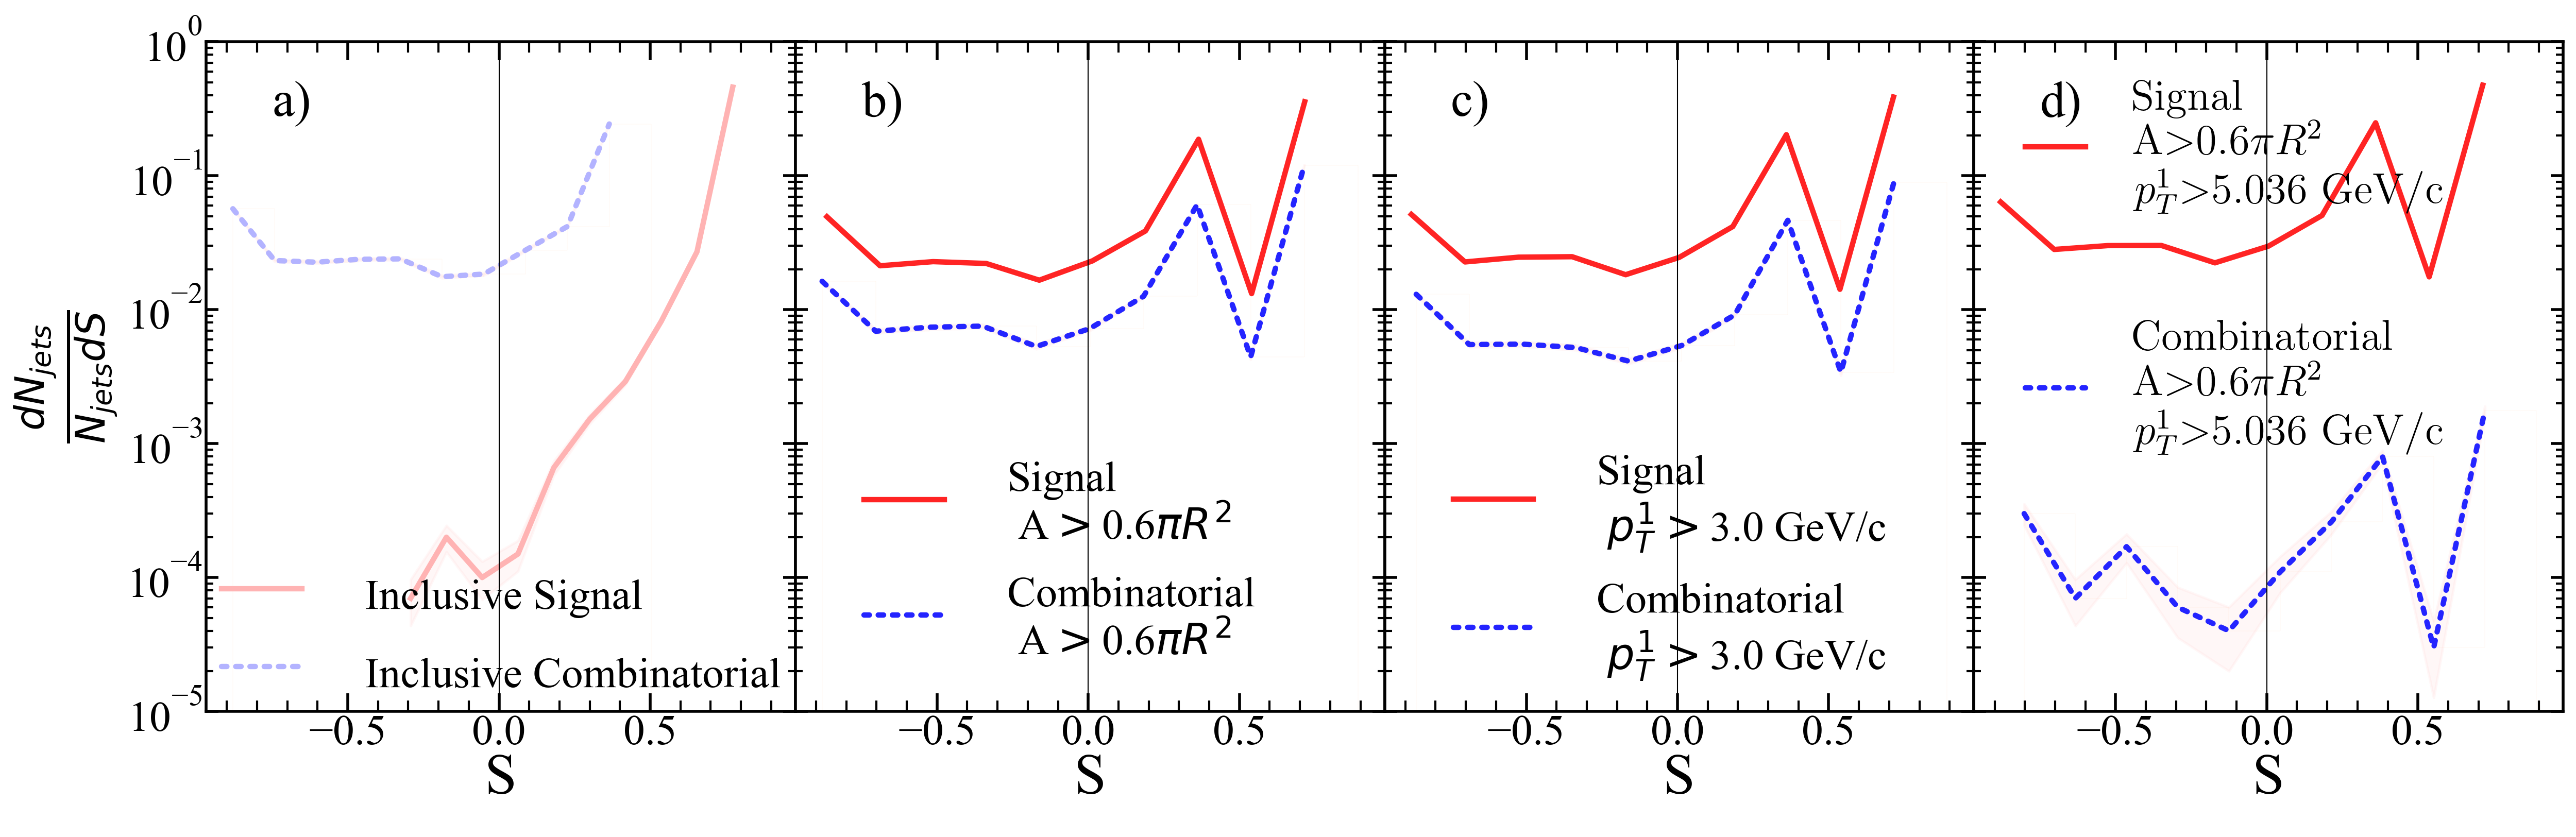}
    \caption{R=0.6 \ptH=30 \GeV}
    \label{fig:sil_06_30}
\end{figure*}

\begin{figure*}
    \centering
    \includegraphics[width=\linewidth]{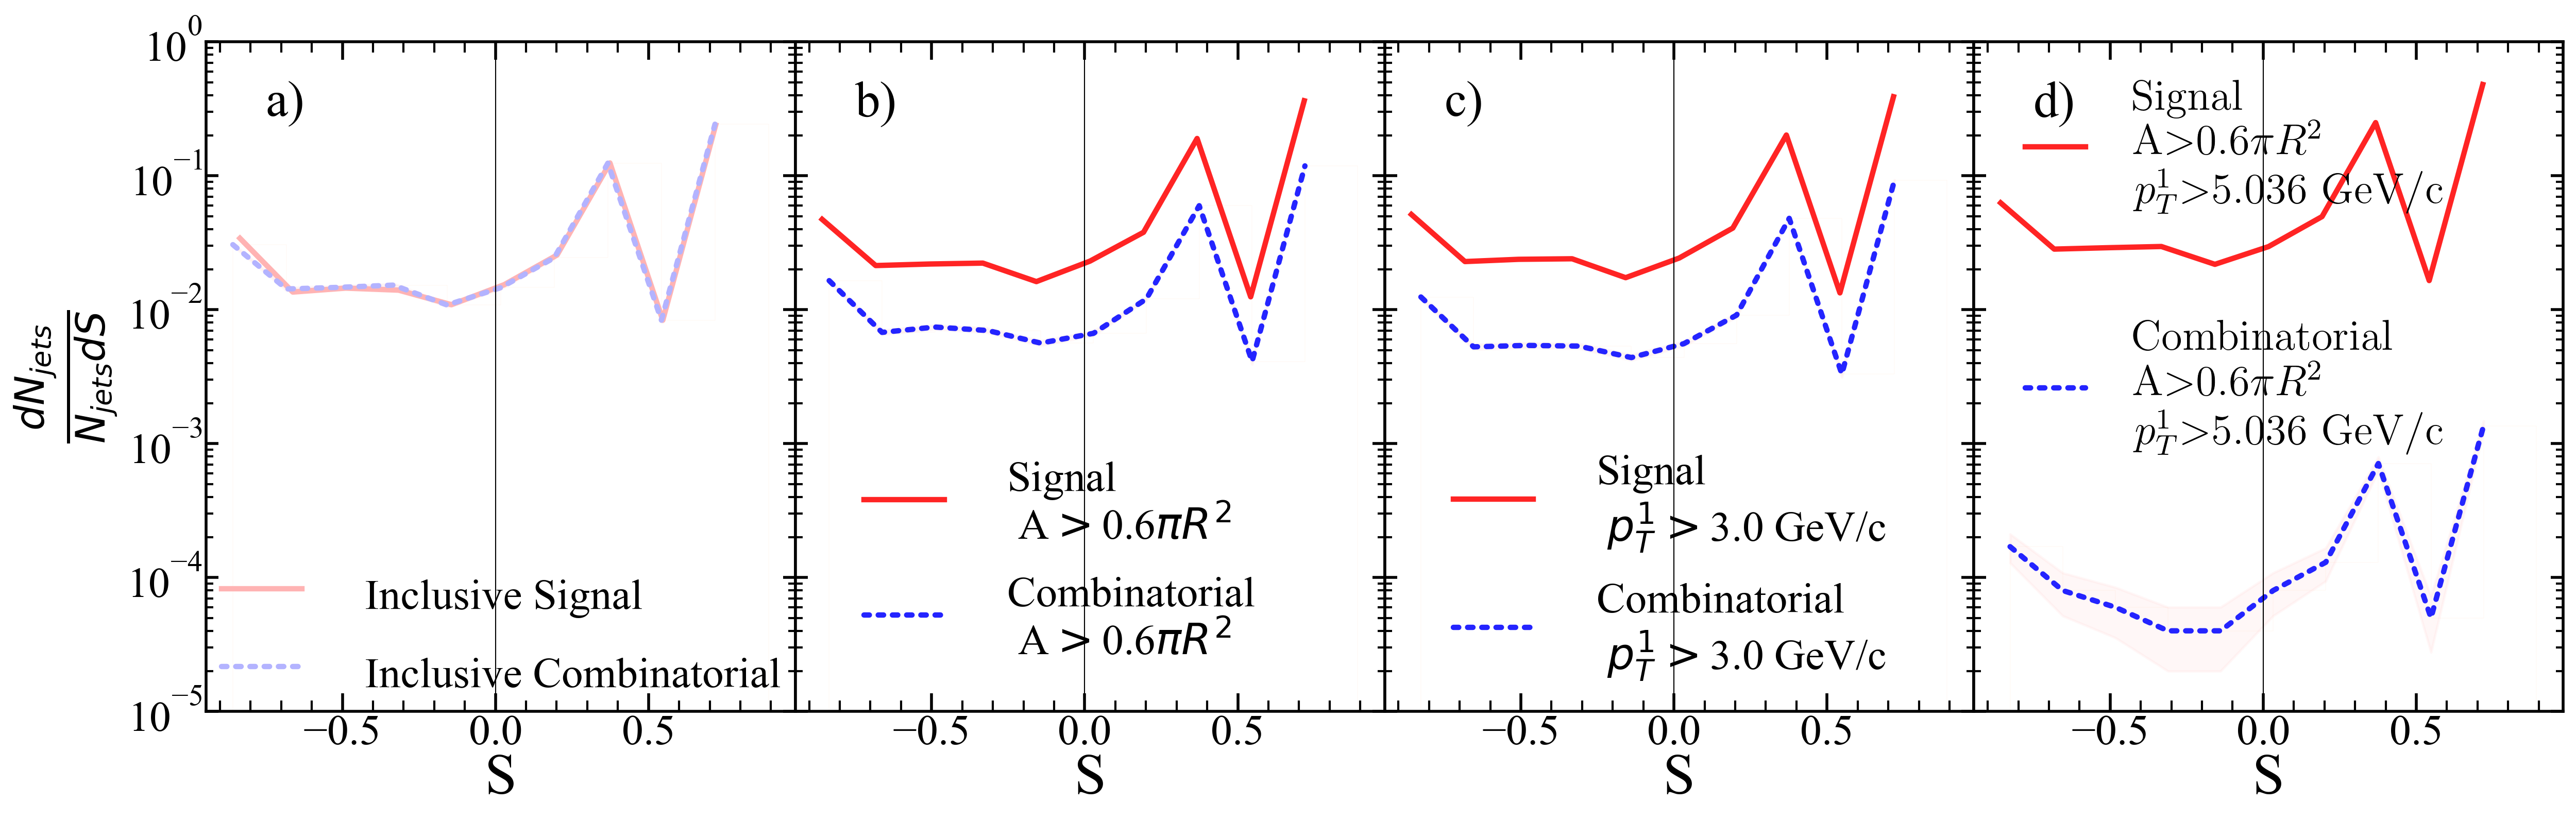}
    \caption{R=0.6 \ptH=40 \GeV}
    \label{fig:sil_06_40}
\end{figure*}

\begin{figure*}
    \centering
    \includegraphics[width=\linewidth]{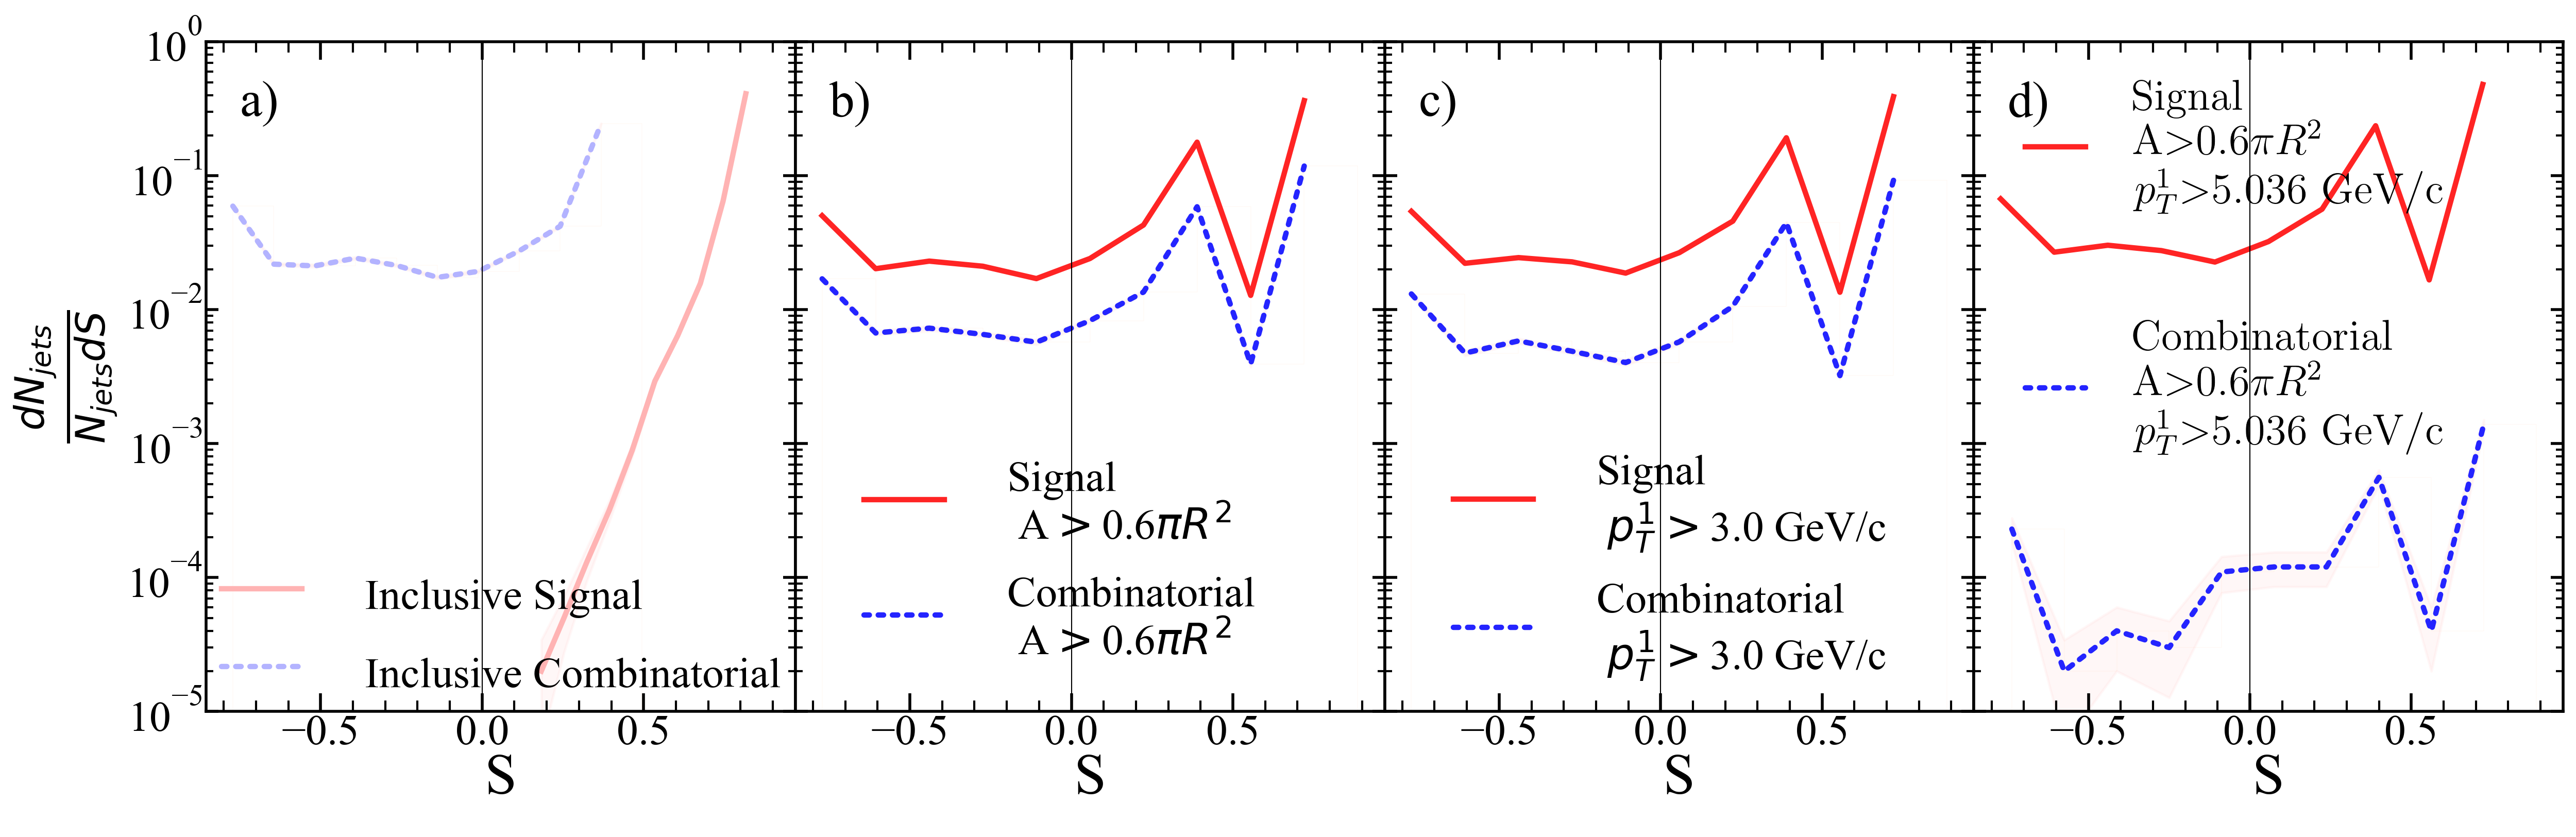}
    \caption{R=0.6 \ptH=60 \GeV}
    \label{fig:sil_06_60}
\end{figure*}

\begin{figure*}
    \centering
    \includegraphics[width=\linewidth]{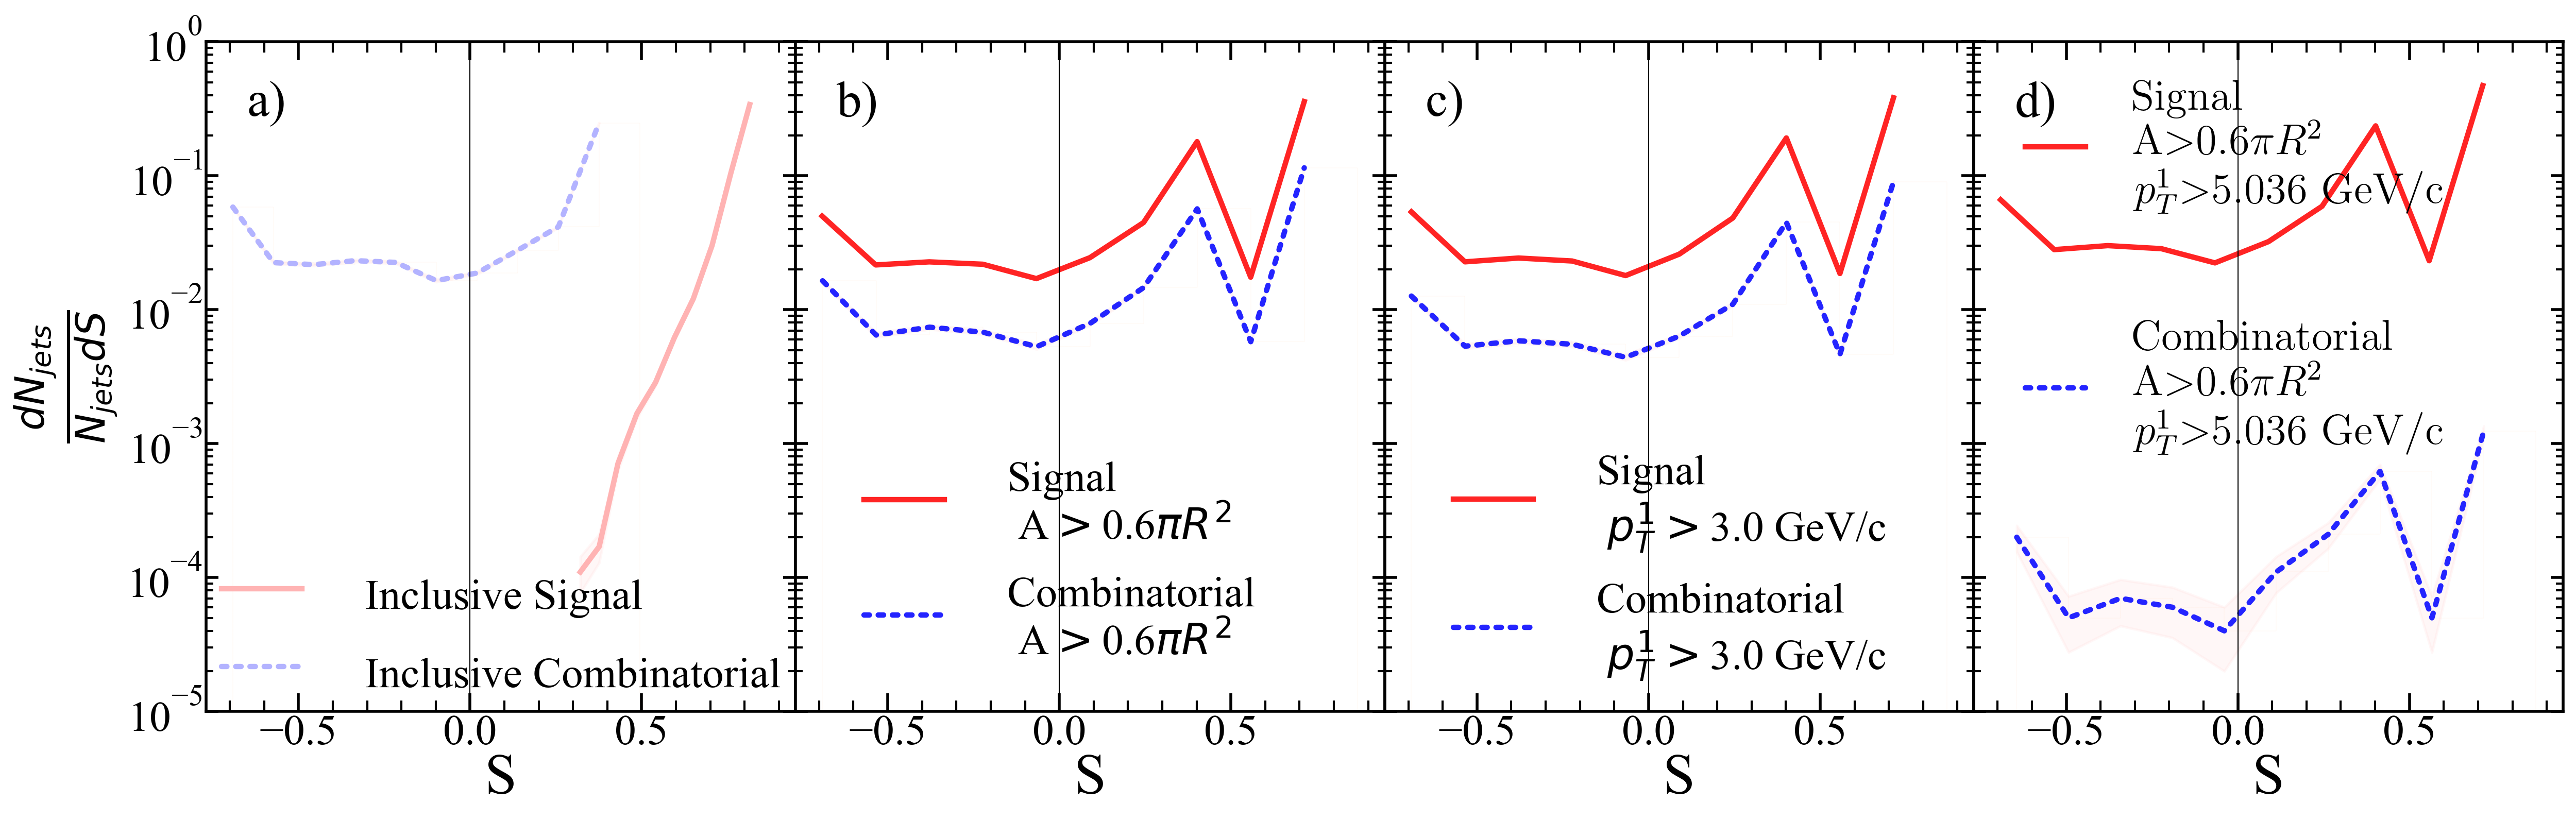}
    \caption{R=0.6 \ptH=80 \GeV}
    \label{fig:sil_06_80}
\end{figure*}
\clearpage
\subsection{\zSub for each kinematic selection.}

\begin{figure*}
    \centering
    \includegraphics[width=\linewidth]{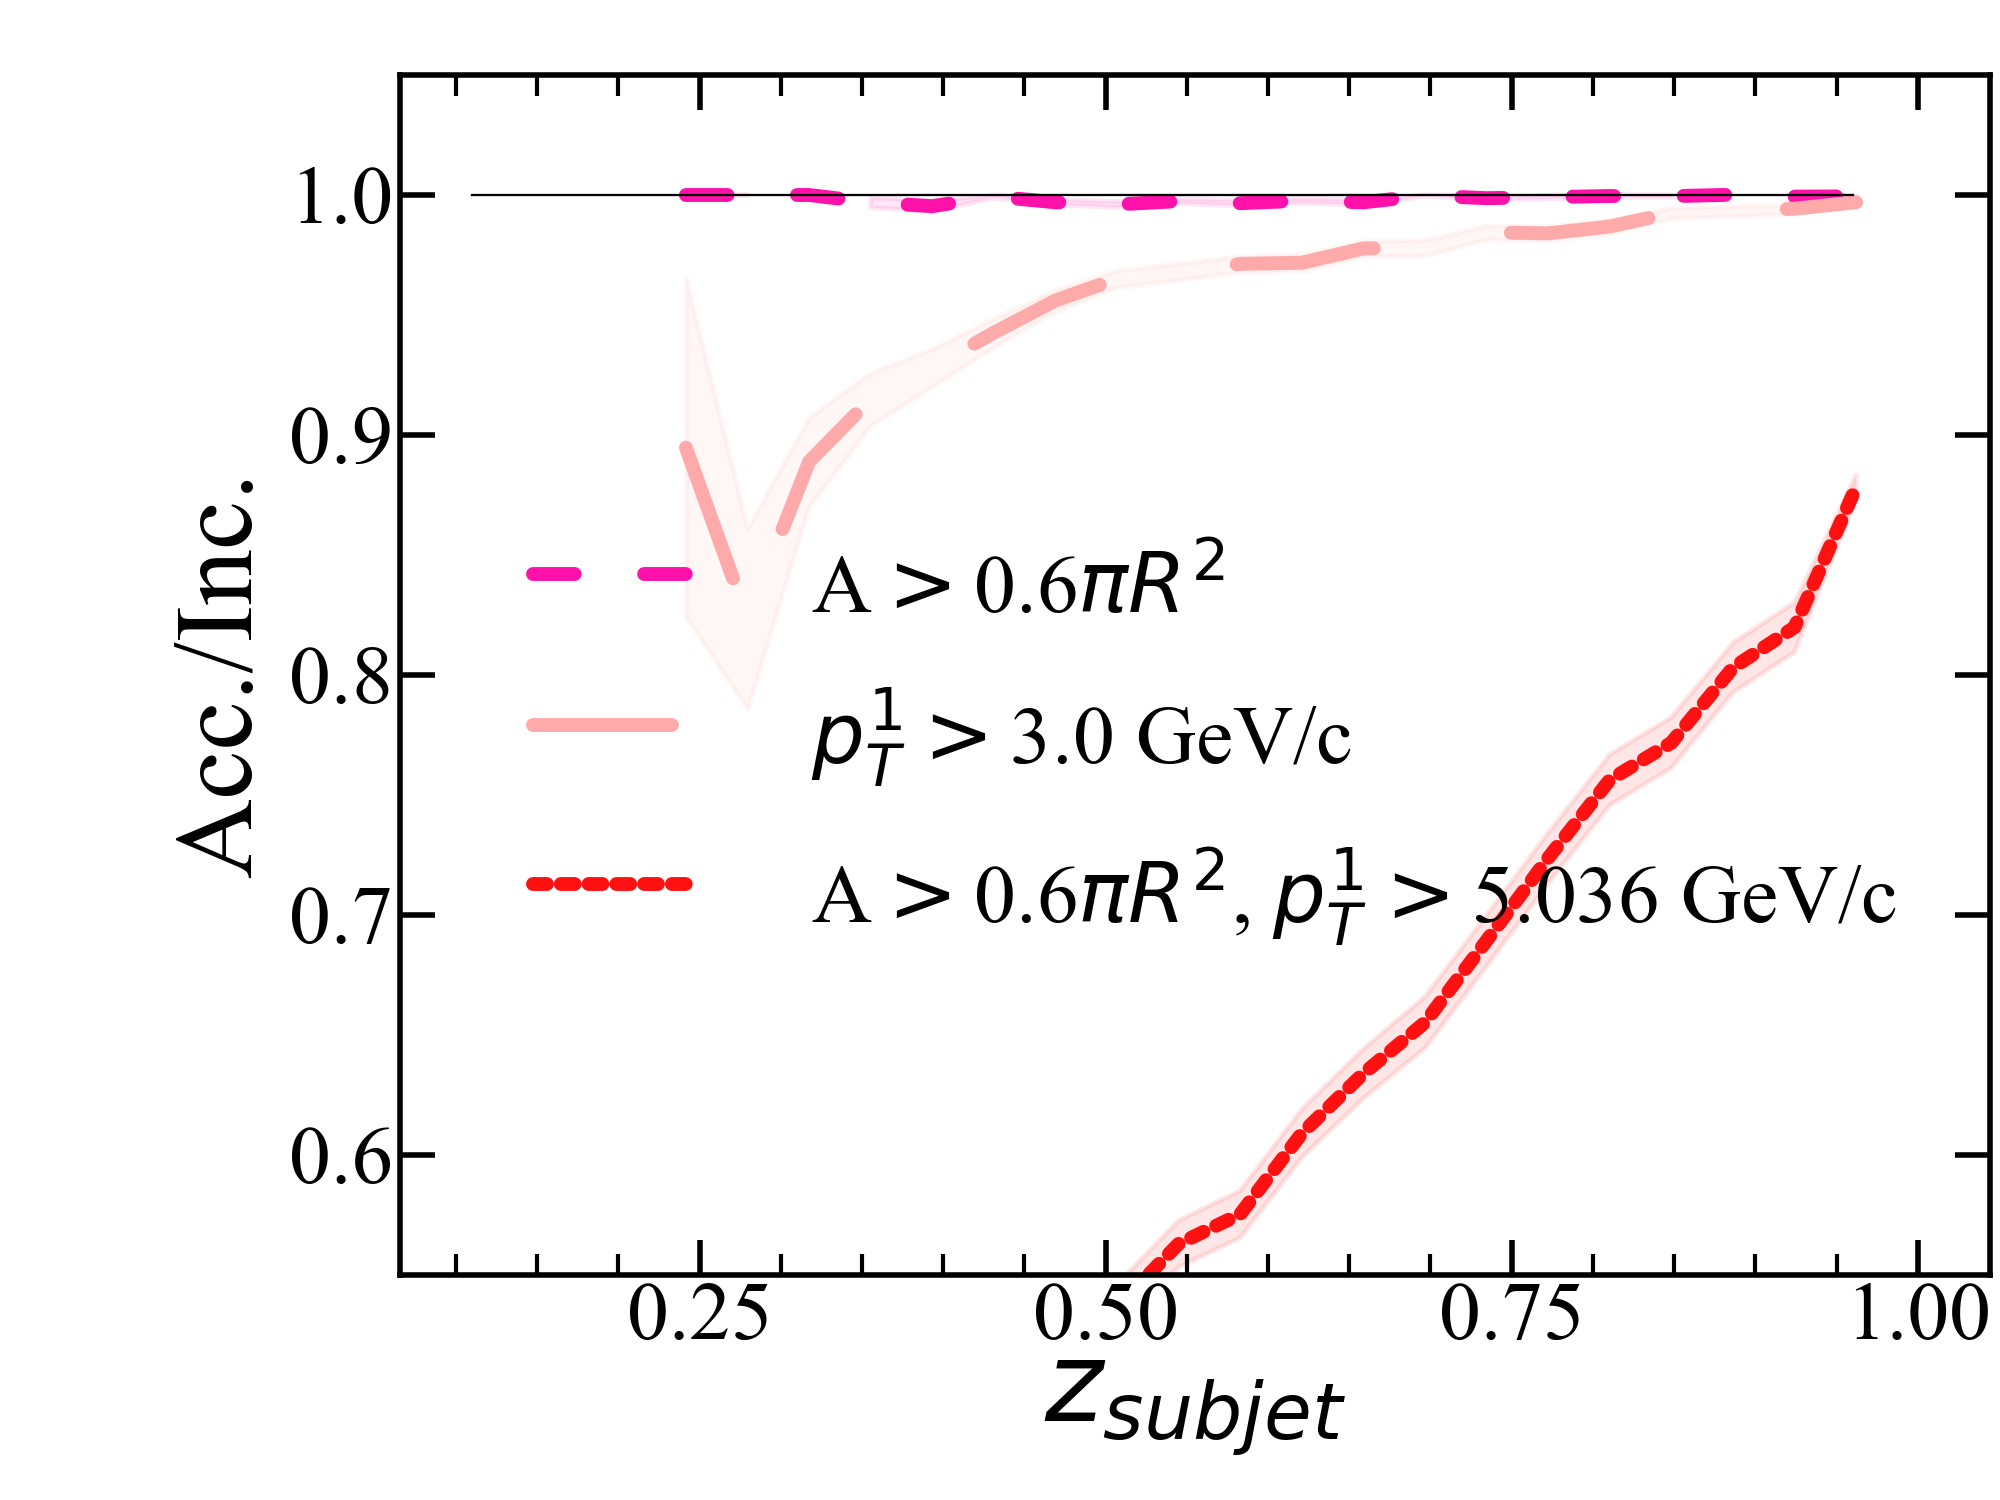}
    \caption{R=0.2 \ptH=10 \GeV}
    \label{fig:z_sub_02_10}
\end{figure*}

\begin{figure*}
    \centering
    \includegraphics[width=\linewidth]{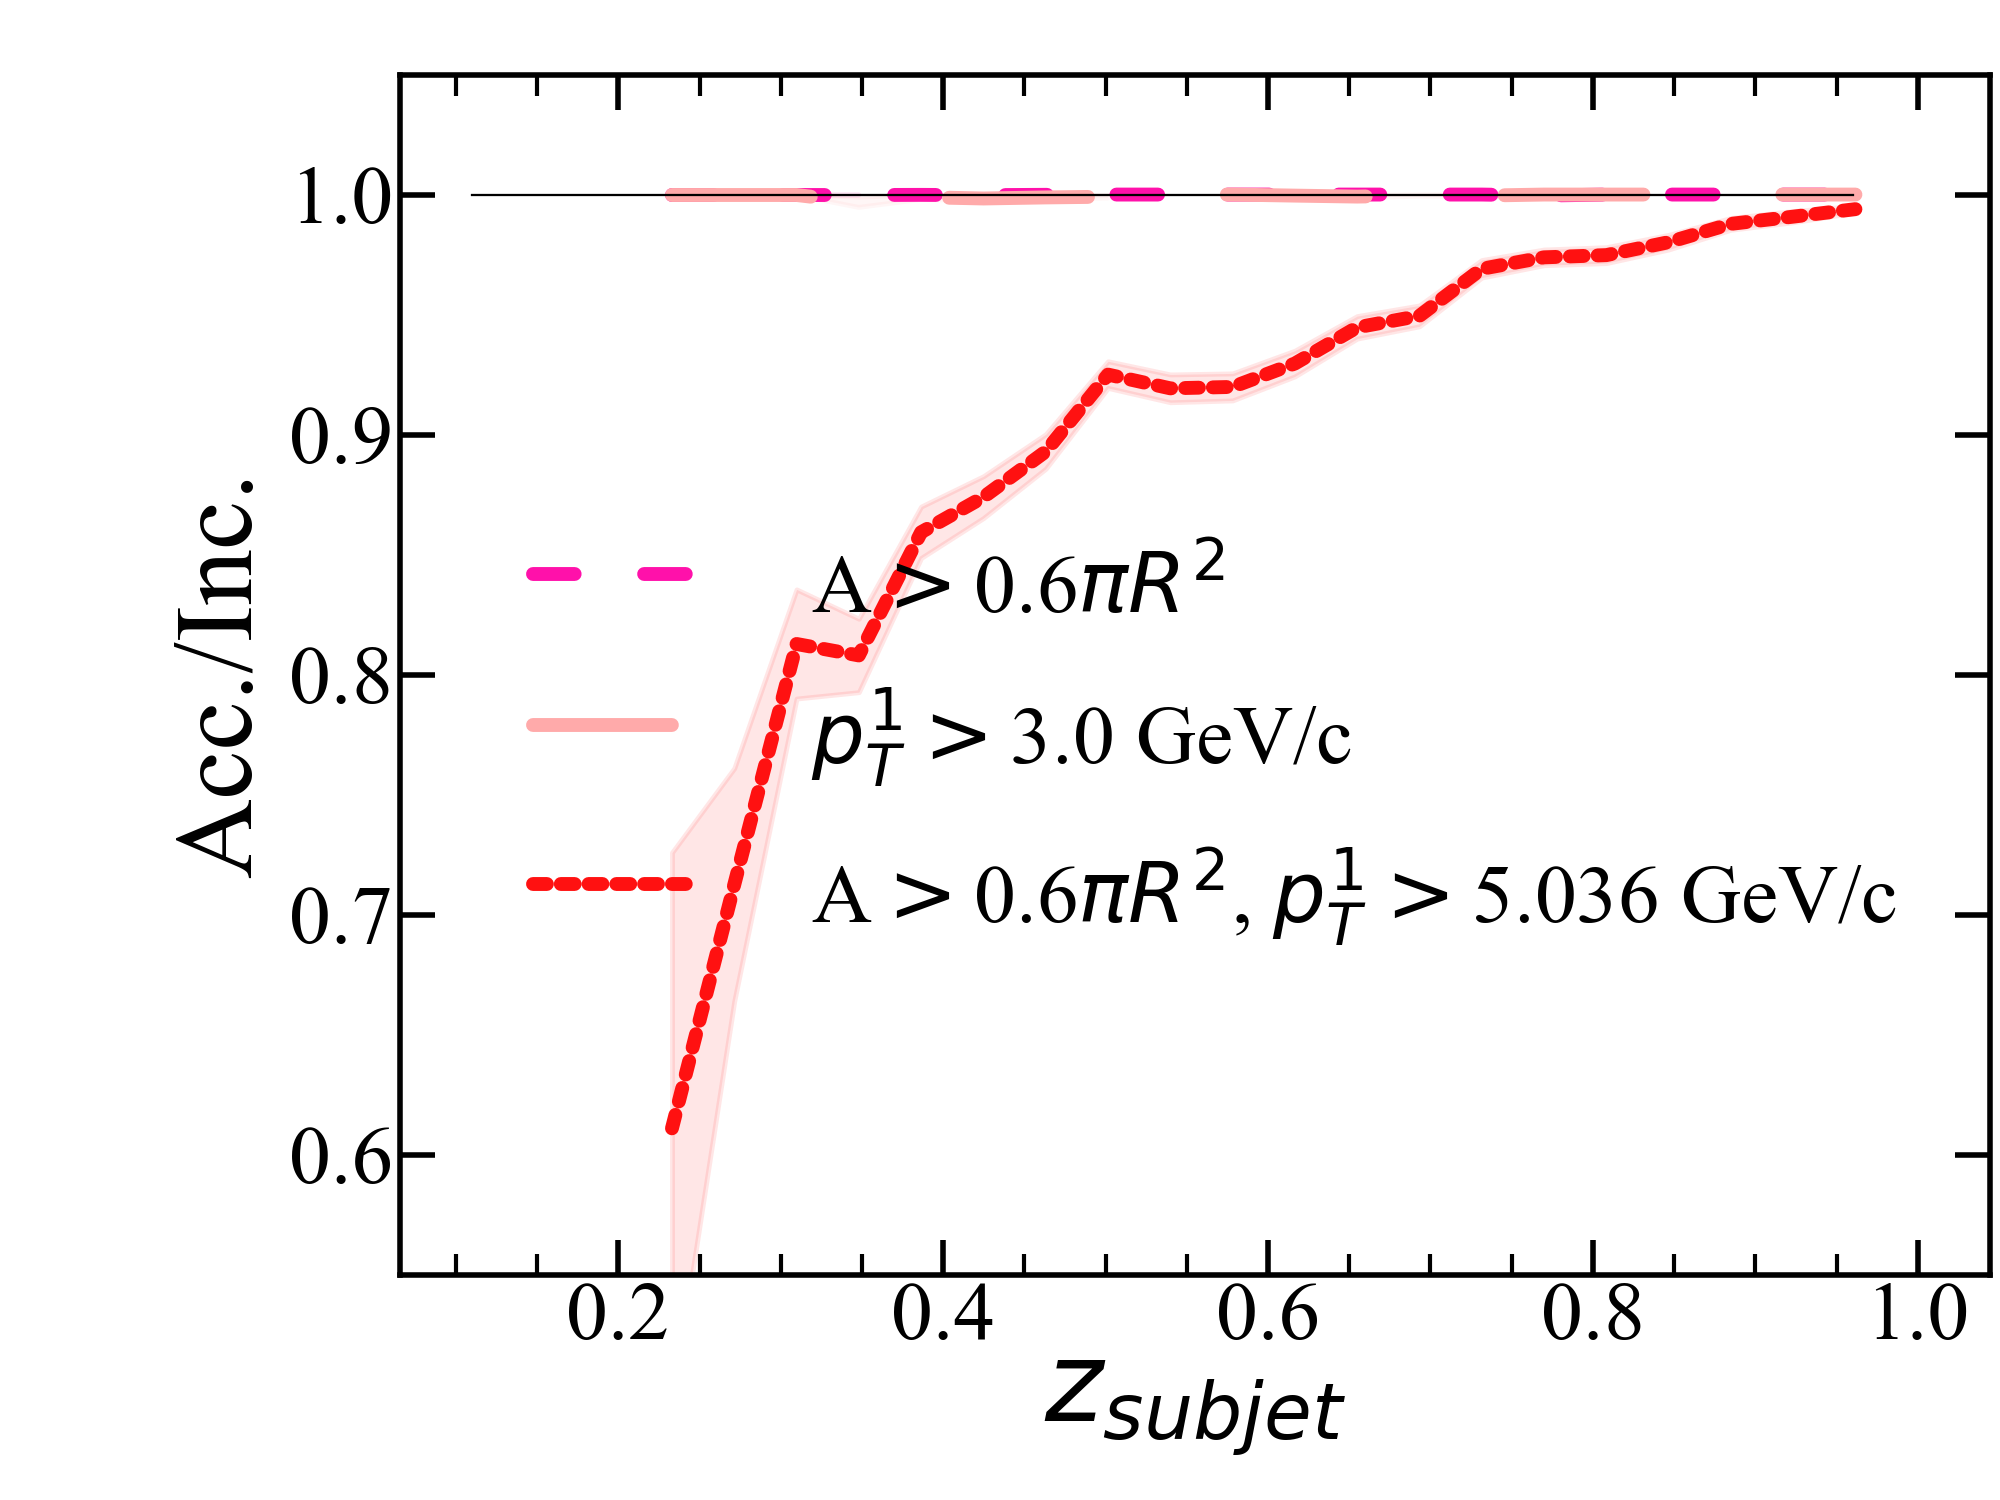}
    \caption{R=0.2 \ptH=20 \GeV}
    \label{fig:z_sub_02_20}
\end{figure*}

\begin{figure*}
    \centering
    \includegraphics[width=\linewidth]{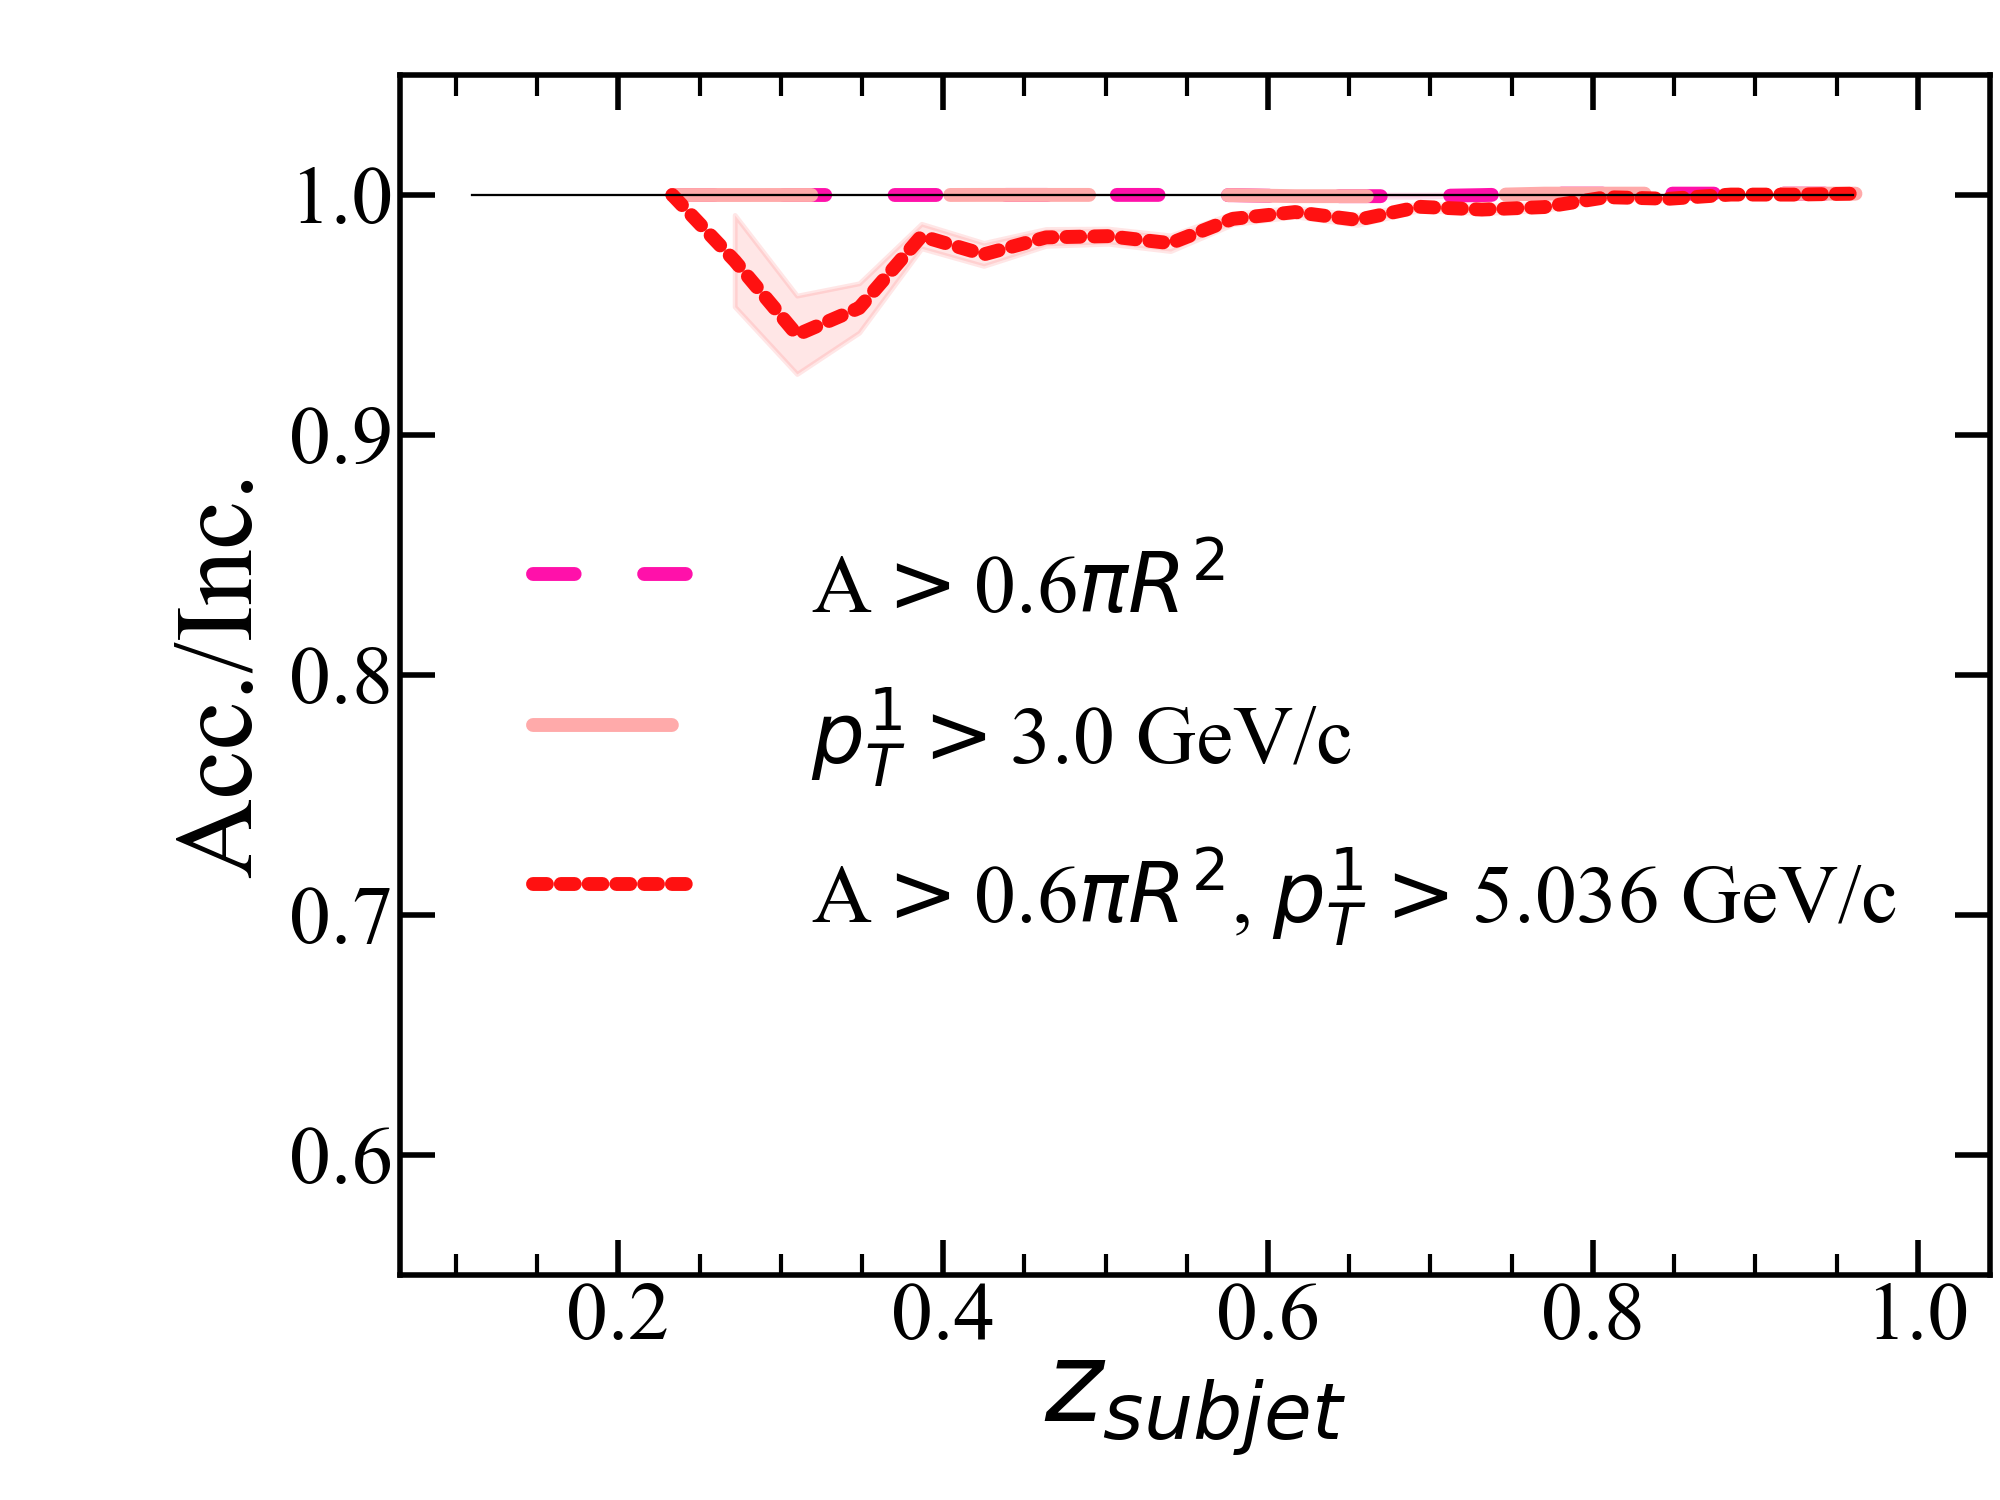}
    \caption{R=0.2 \ptH=30 \GeV}
    \label{fig:z_sub_02_30}
\end{figure*}

\begin{figure*}
    \centering
    \includegraphics[width=\linewidth]{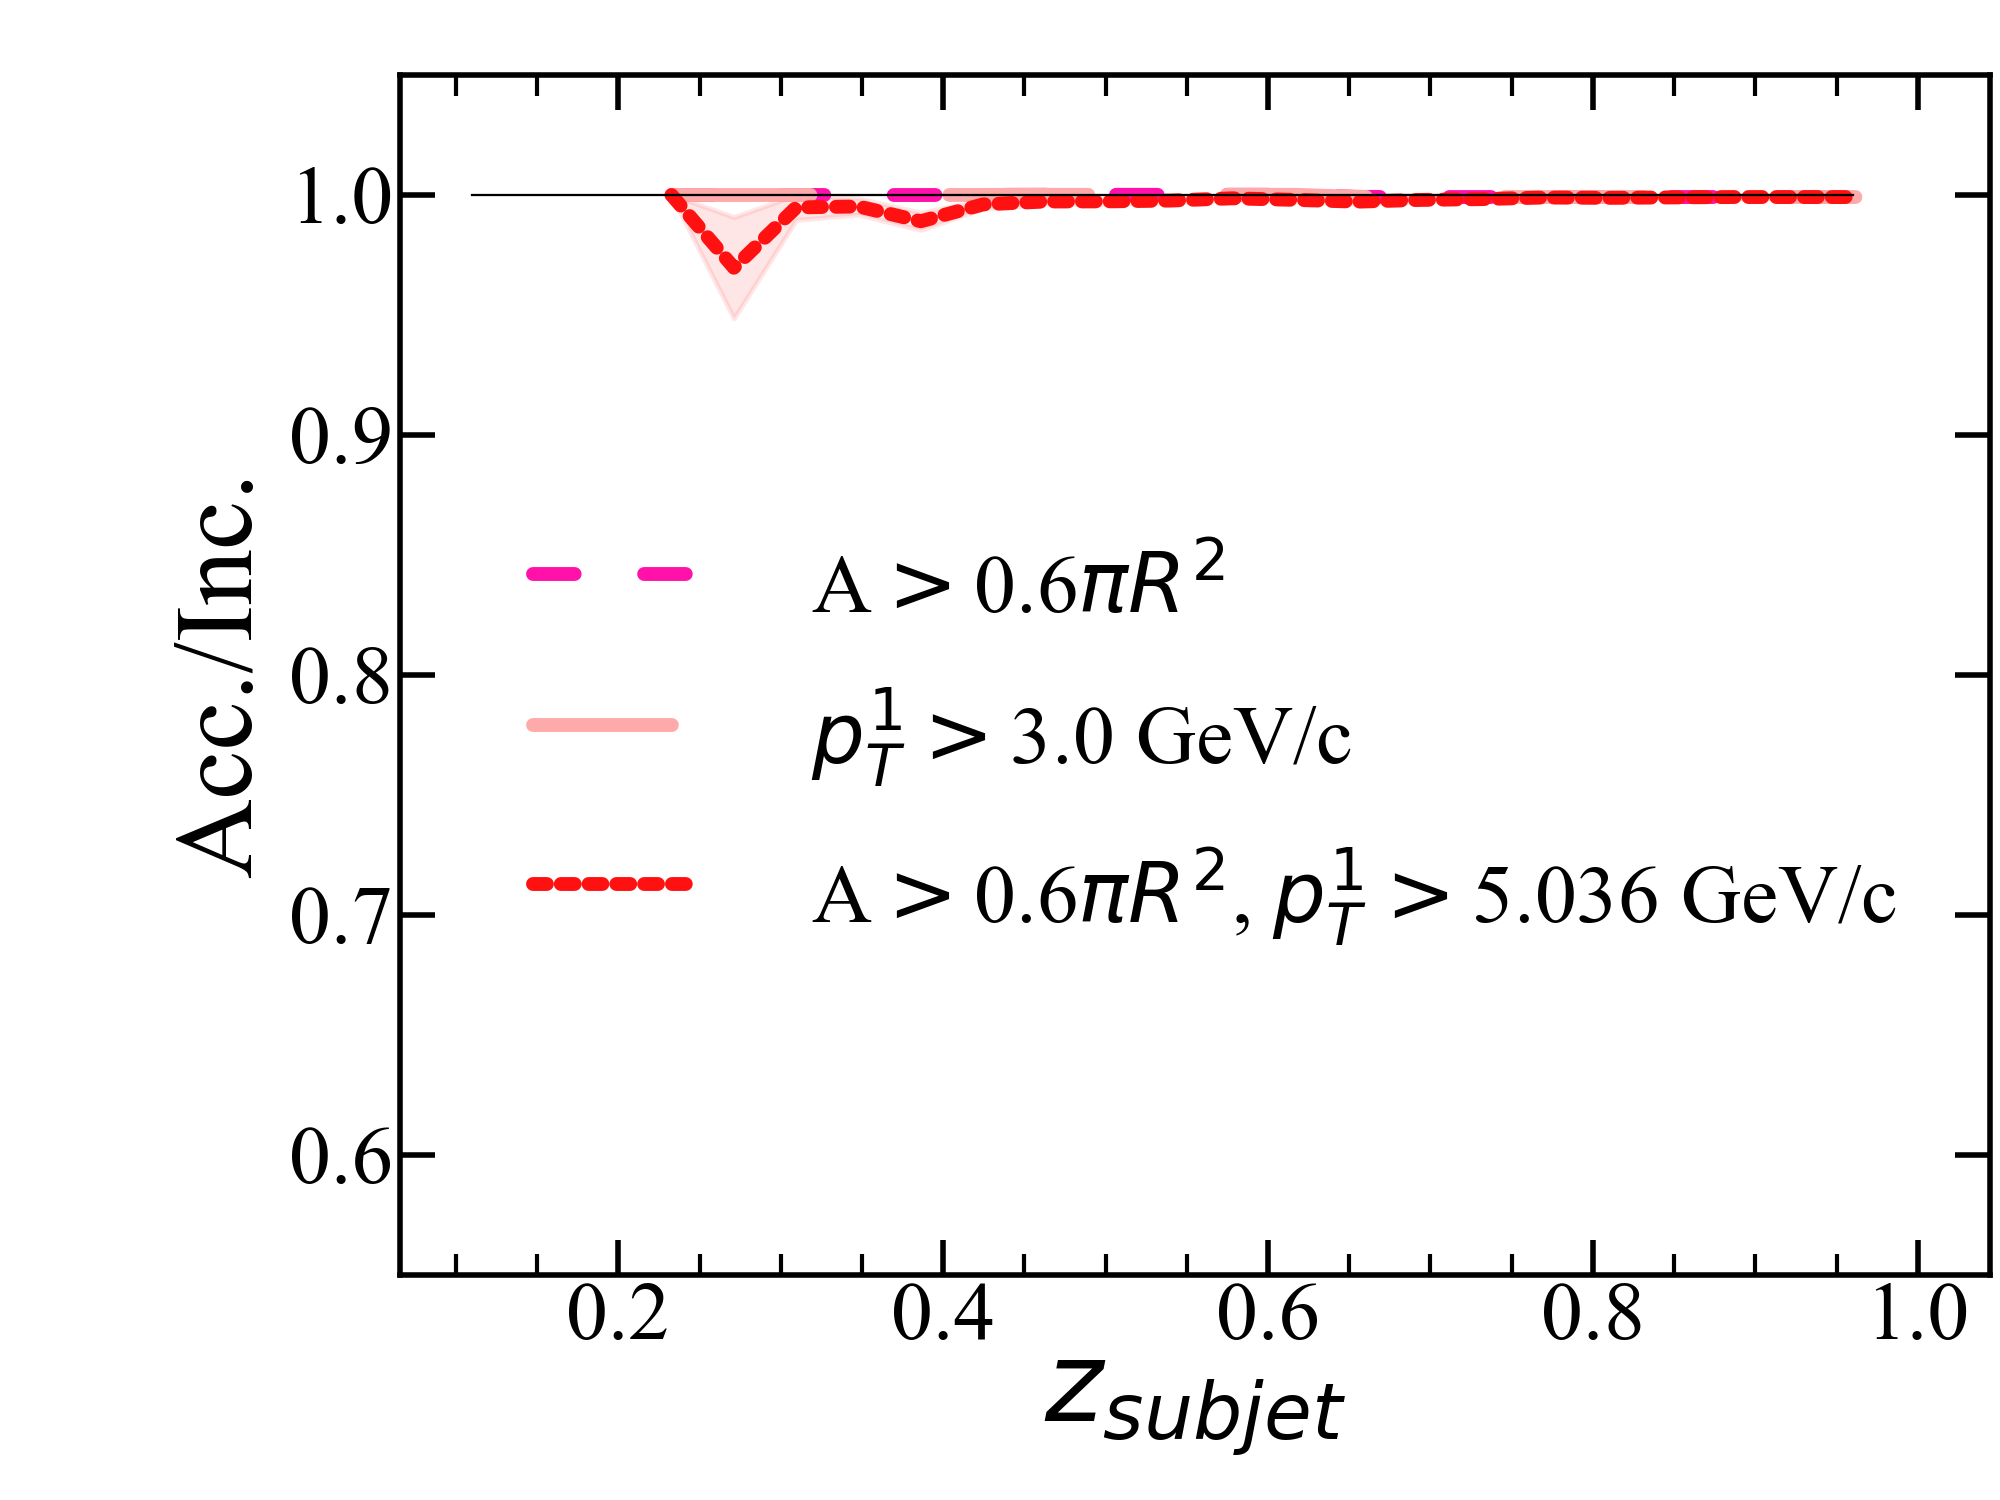}
    \caption{R=0.2 \ptH=40 \GeV}
    \label{fig:z_sub_02_40}
\end{figure*}

\begin{figure*}
    \centering
    \includegraphics[width=\linewidth]{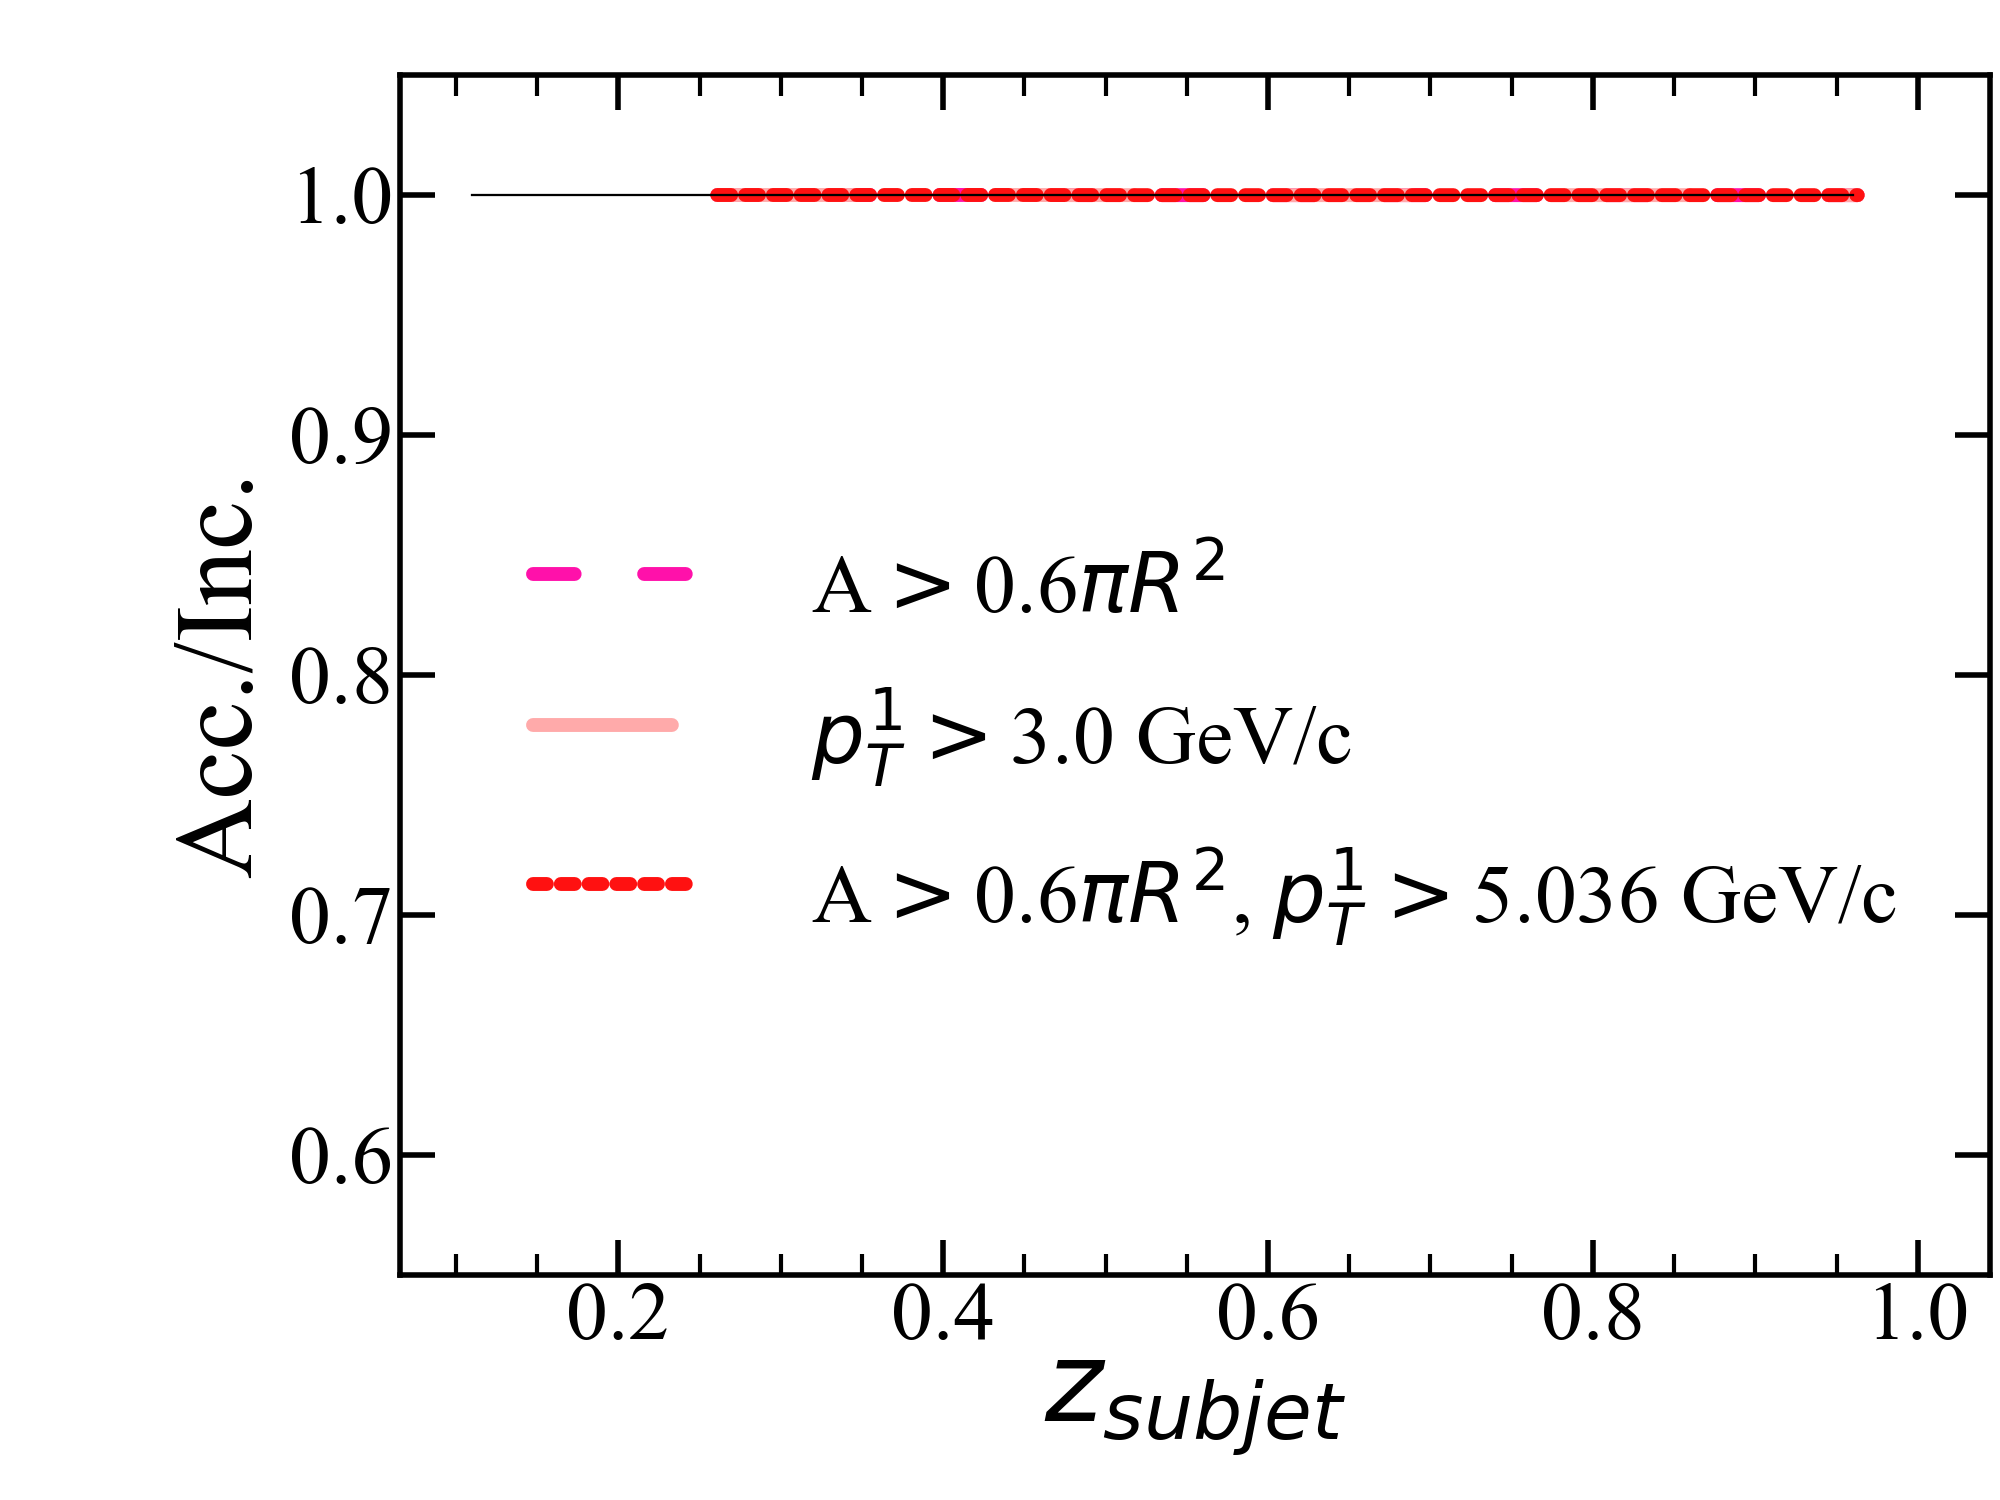}
    \caption{R=0.2 \ptH=60 \GeV}
    \label{fig:z_sub_02_60}
\end{figure*}

\begin{figure*}
    \centering
    \includegraphics[width=\linewidth]{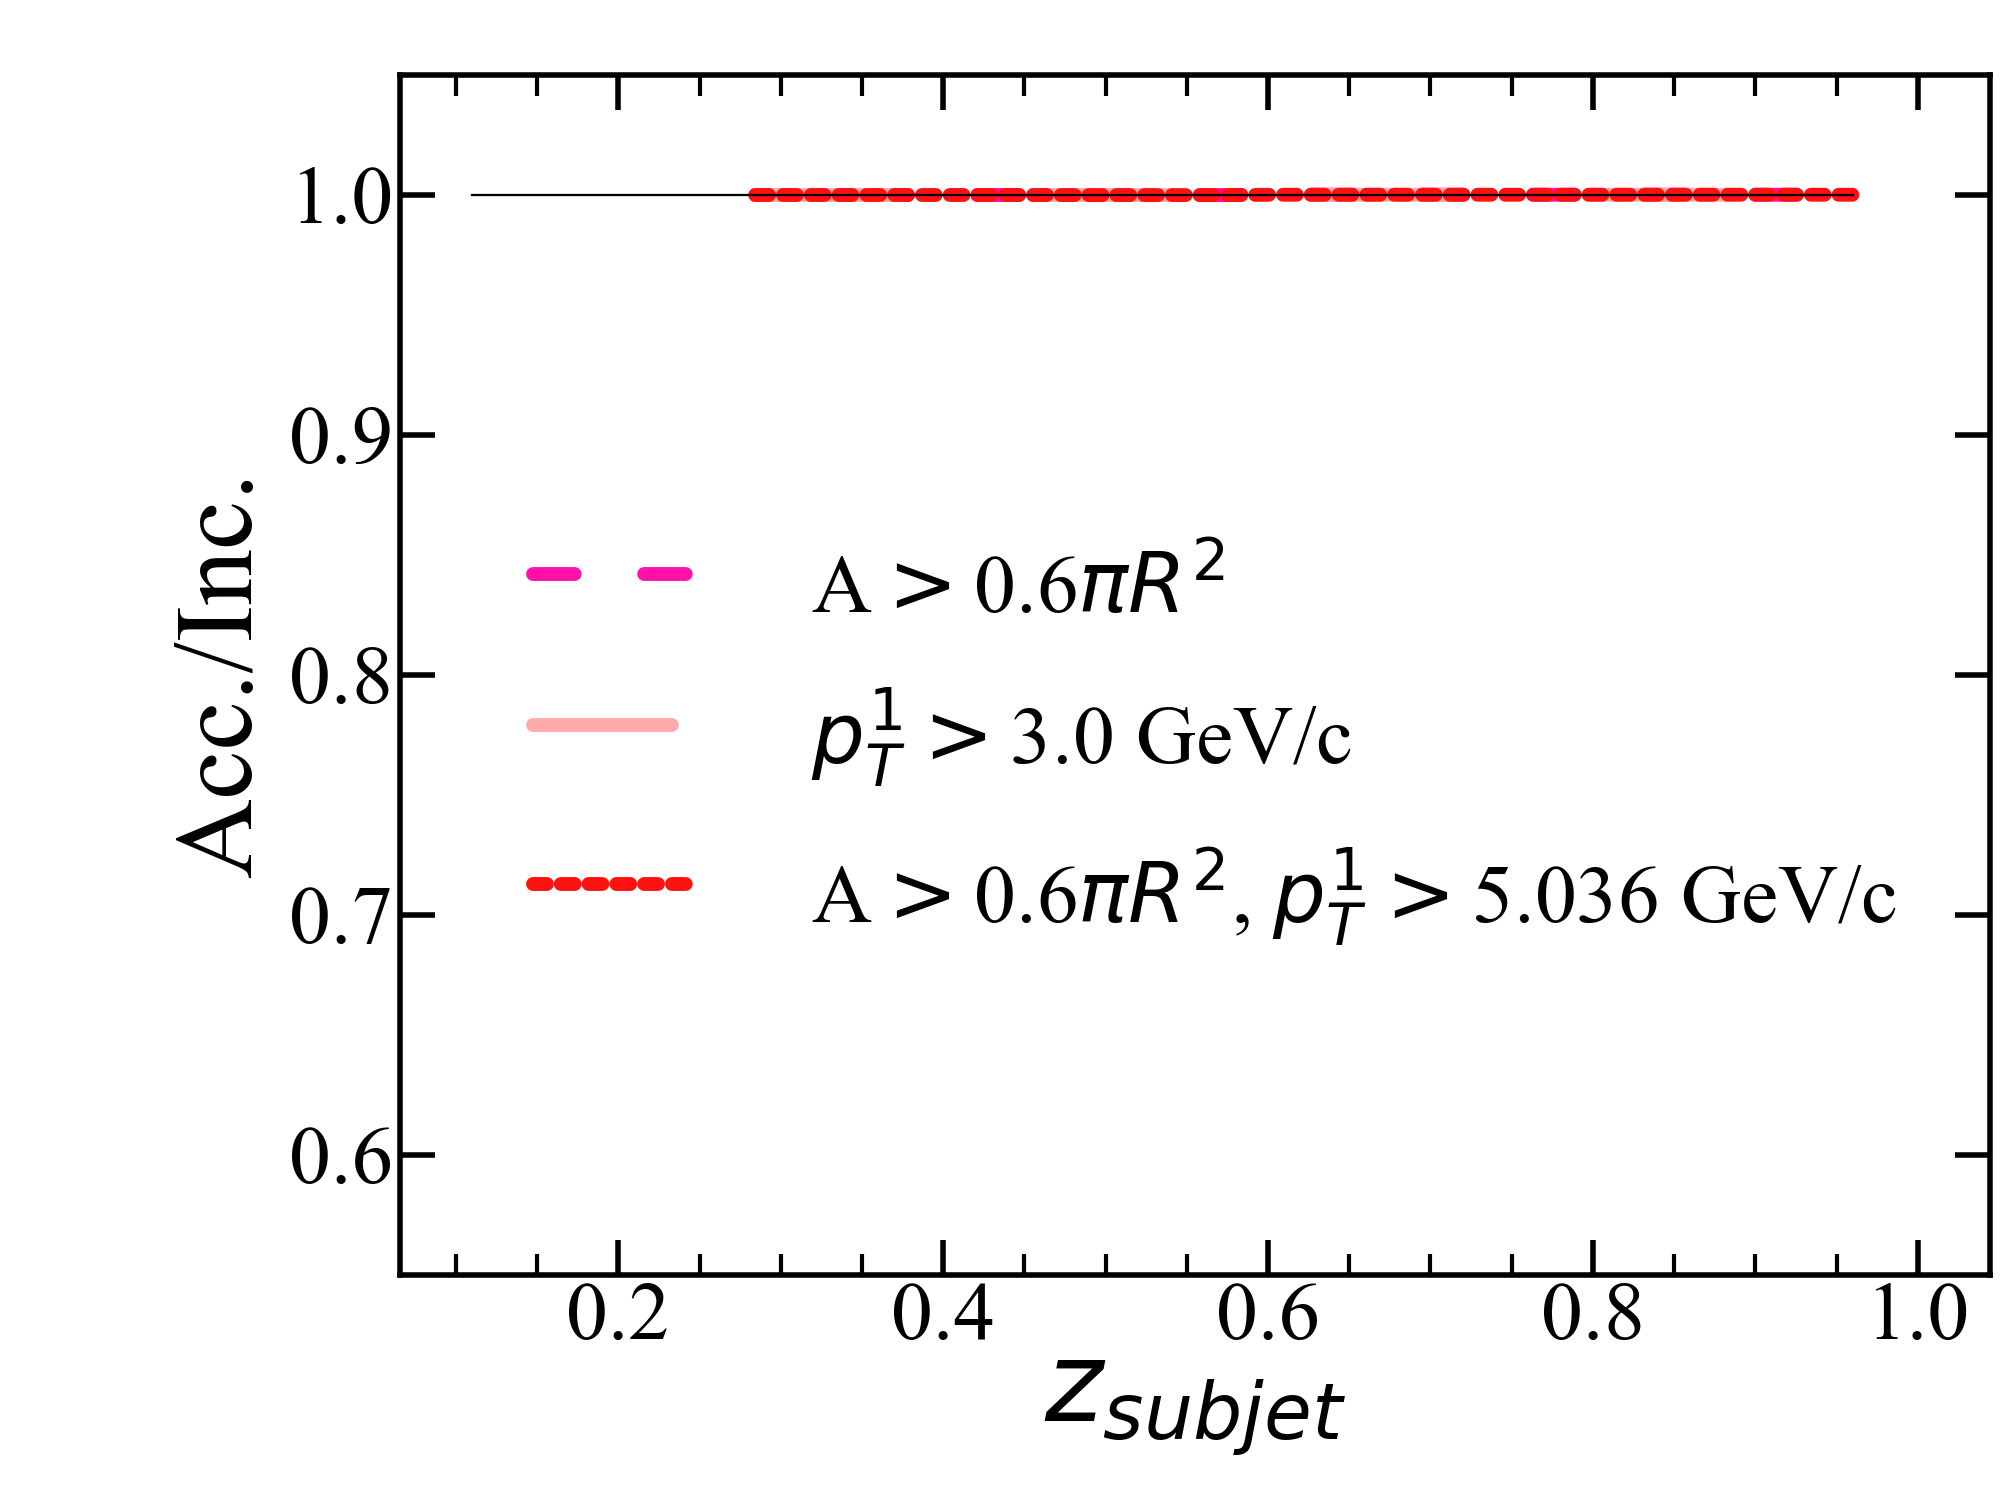}
    \caption{R=0.2 \ptH=80 \GeV}
    \label{fig:z_sub_02_80}
\end{figure*}

\begin{figure*}
    \centering
    \includegraphics[width=\linewidth]{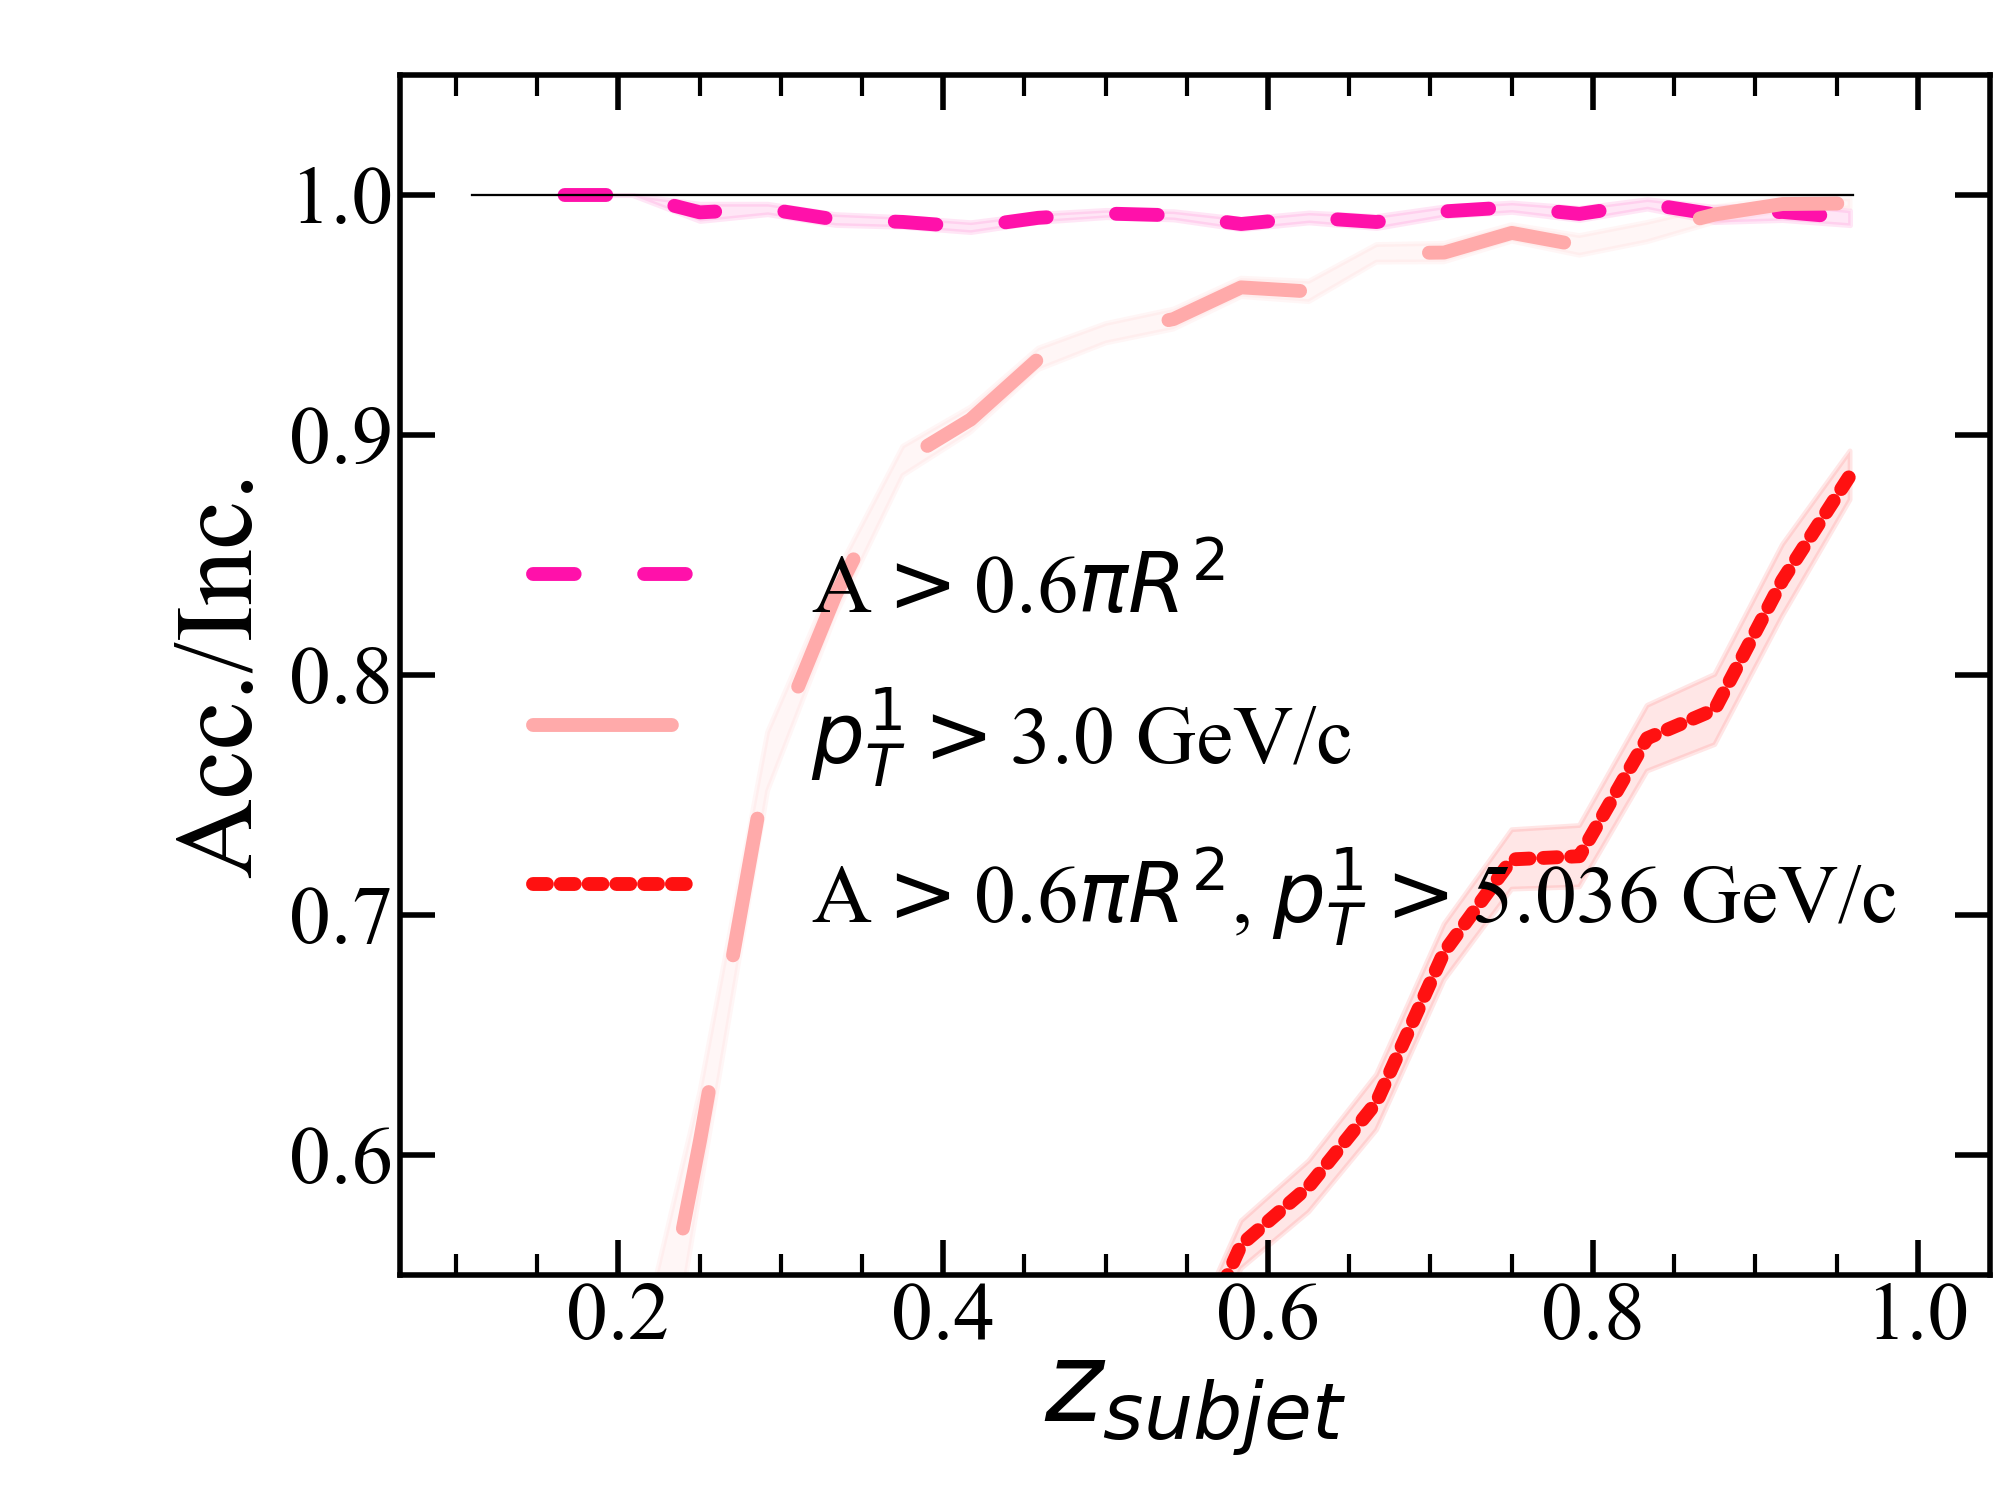}
    \caption{R=0.3 \ptH=10 \GeV}
    \label{fig:z_sub_03_10}
\end{figure*}

\begin{figure*}
    \centering
    \includegraphics[width=\linewidth]{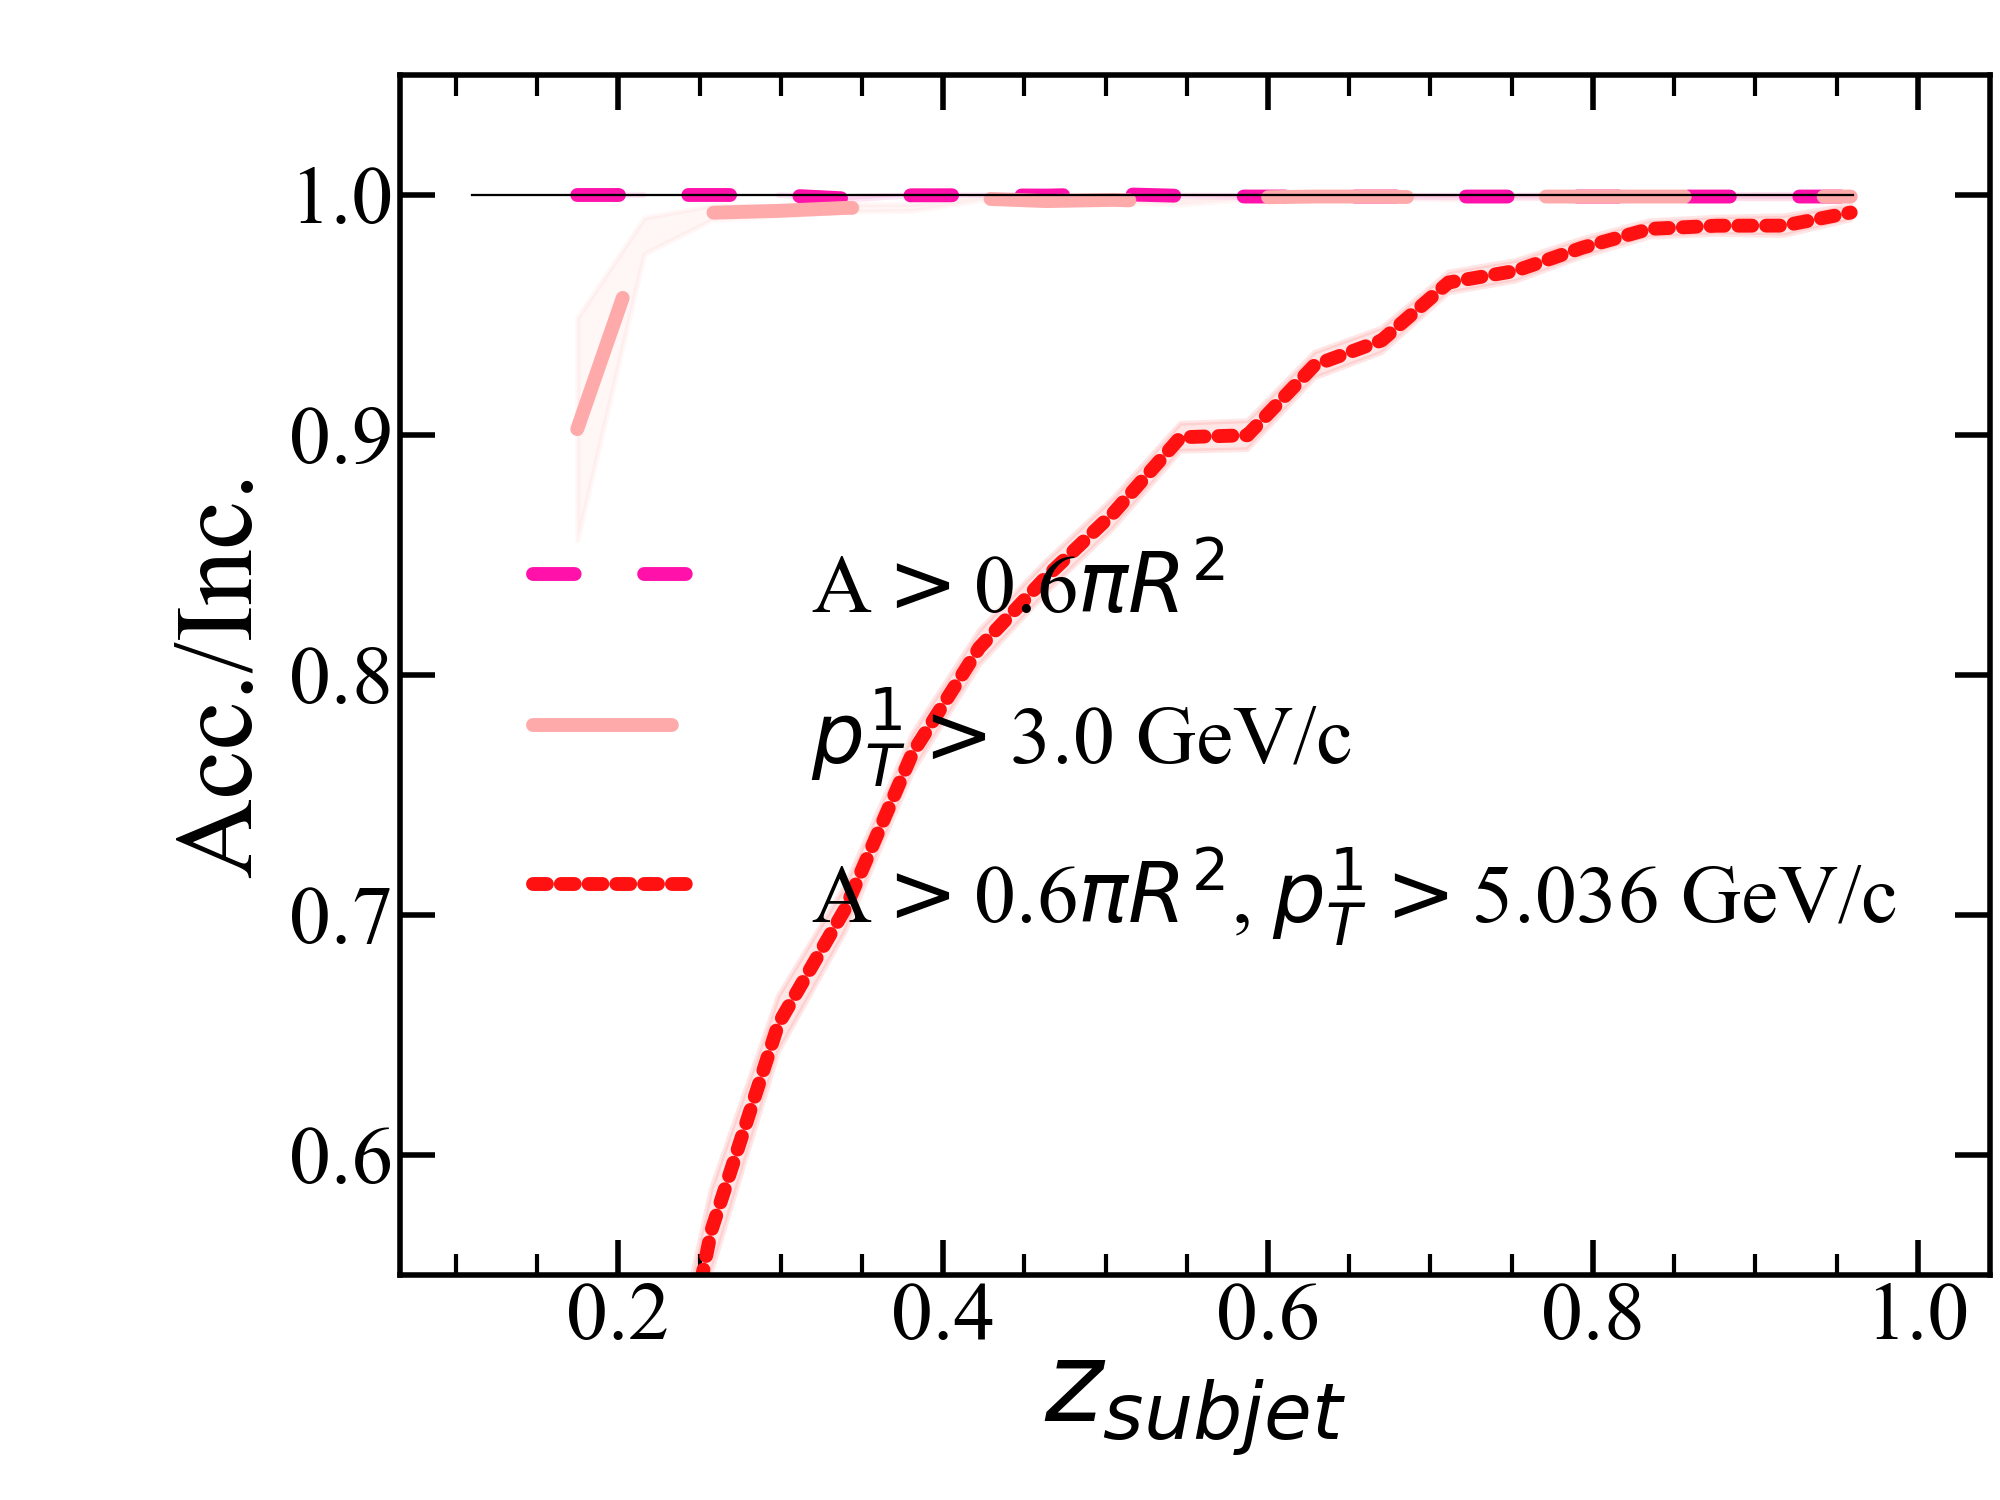}
    \caption{R=0.3 \ptH=20 \GeV}
    \label{fig:z_sub_03_20}
\end{figure*}

\begin{figure*}
    \centering
    \includegraphics[width=\linewidth]{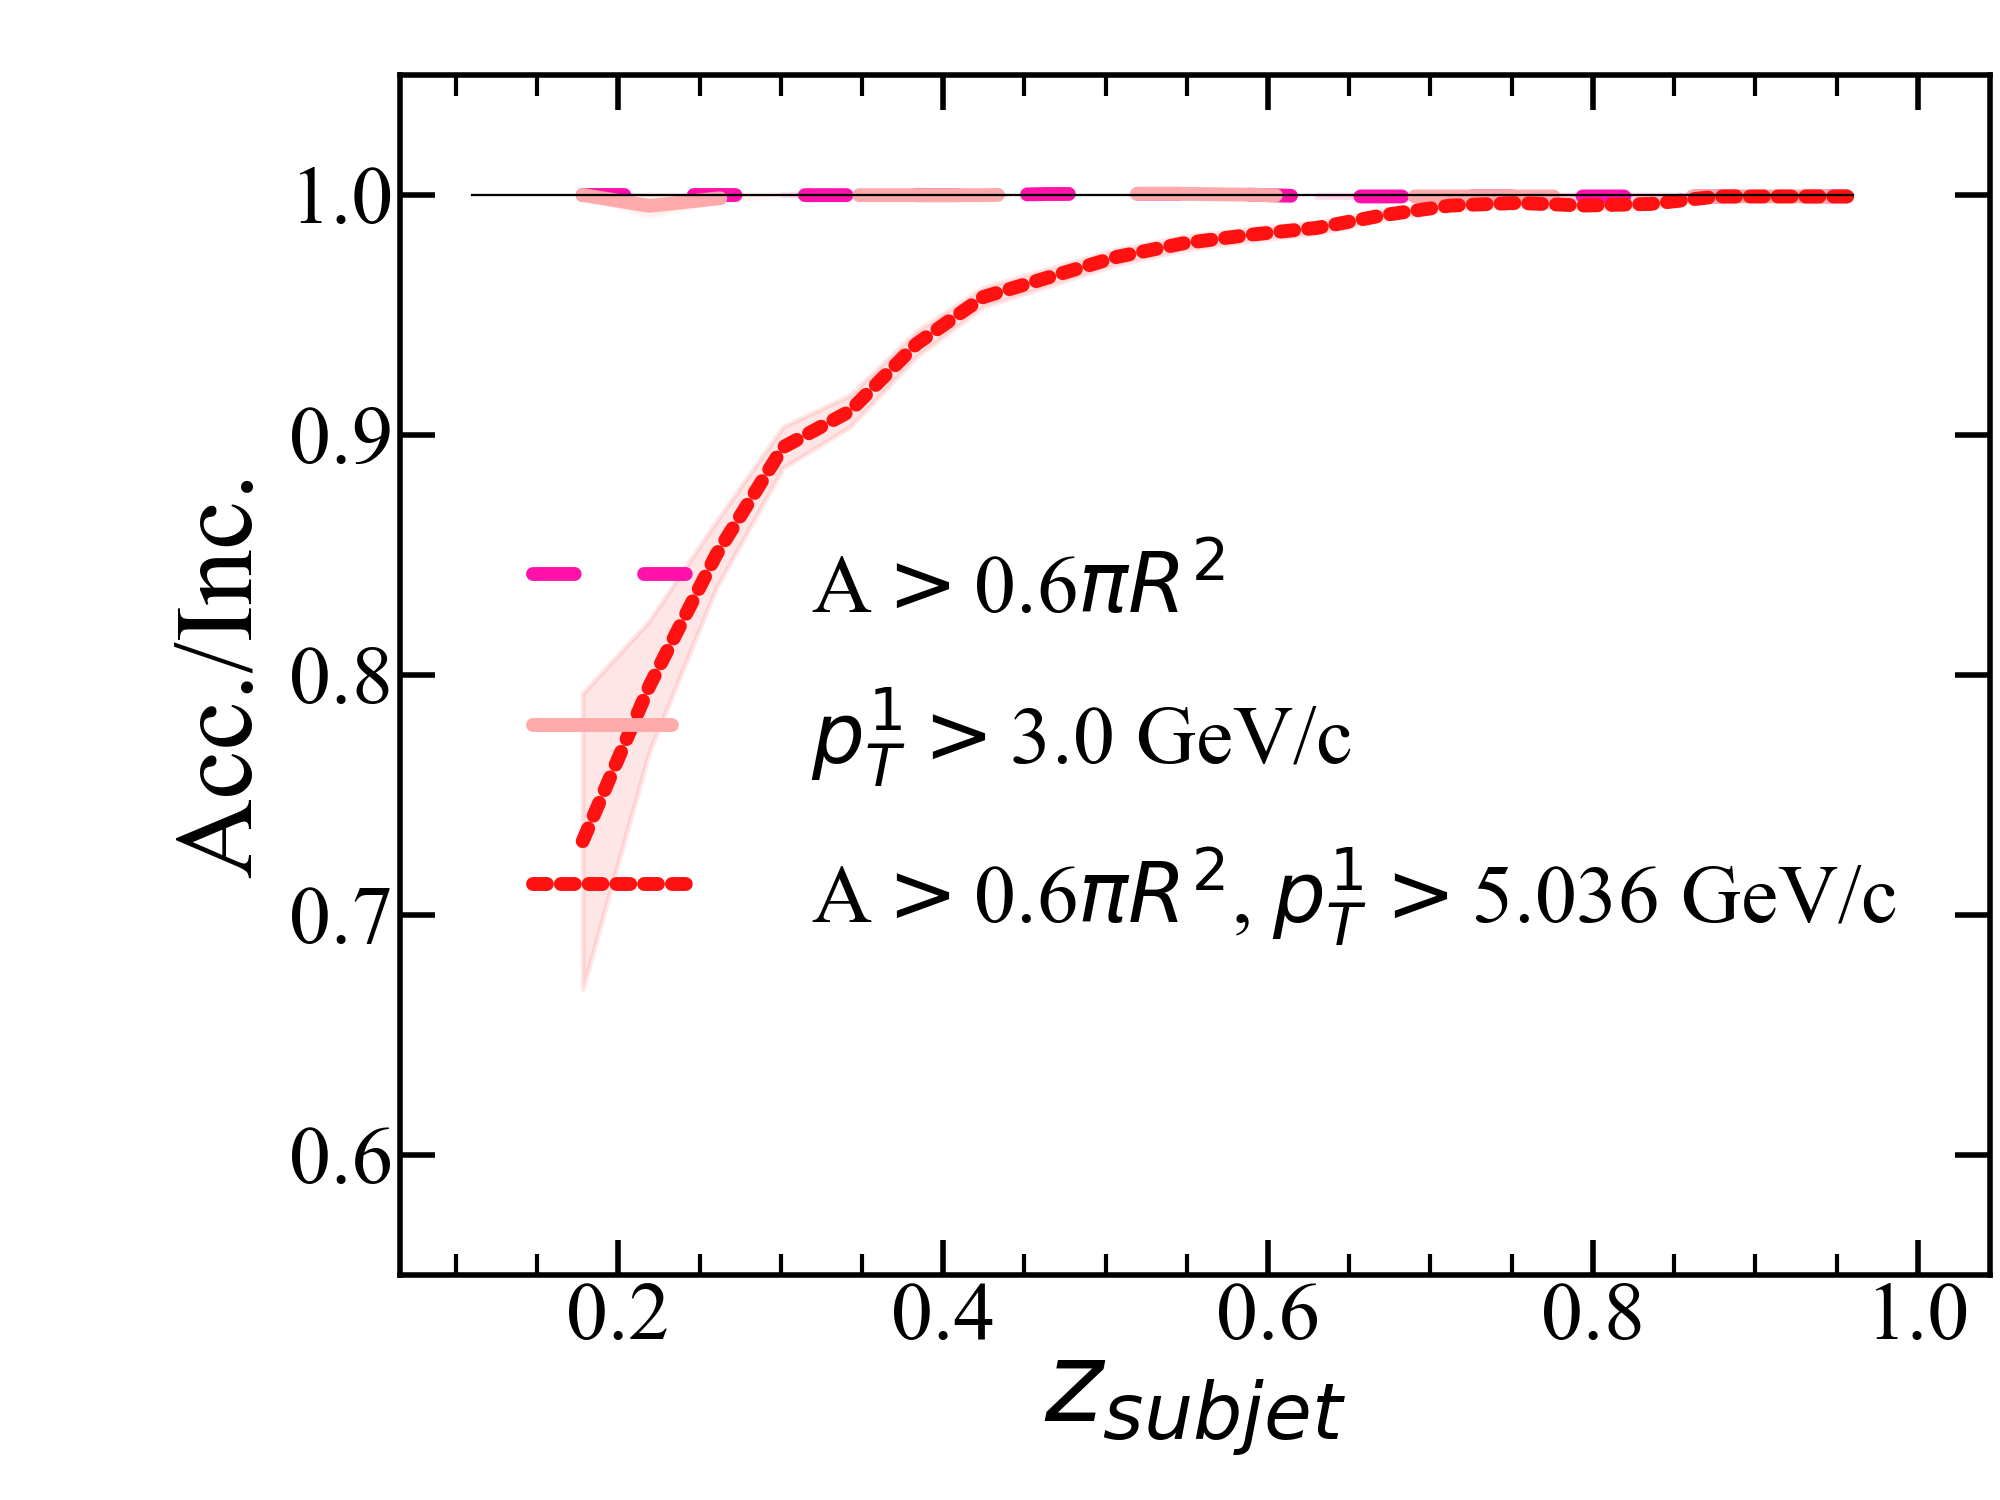}
    \caption{R=0.3 \ptH=30 \GeV}
    \label{fig:z_sub_03_30}
\end{figure*}

\begin{figure*}
    \centering
    \includegraphics[width=\linewidth]{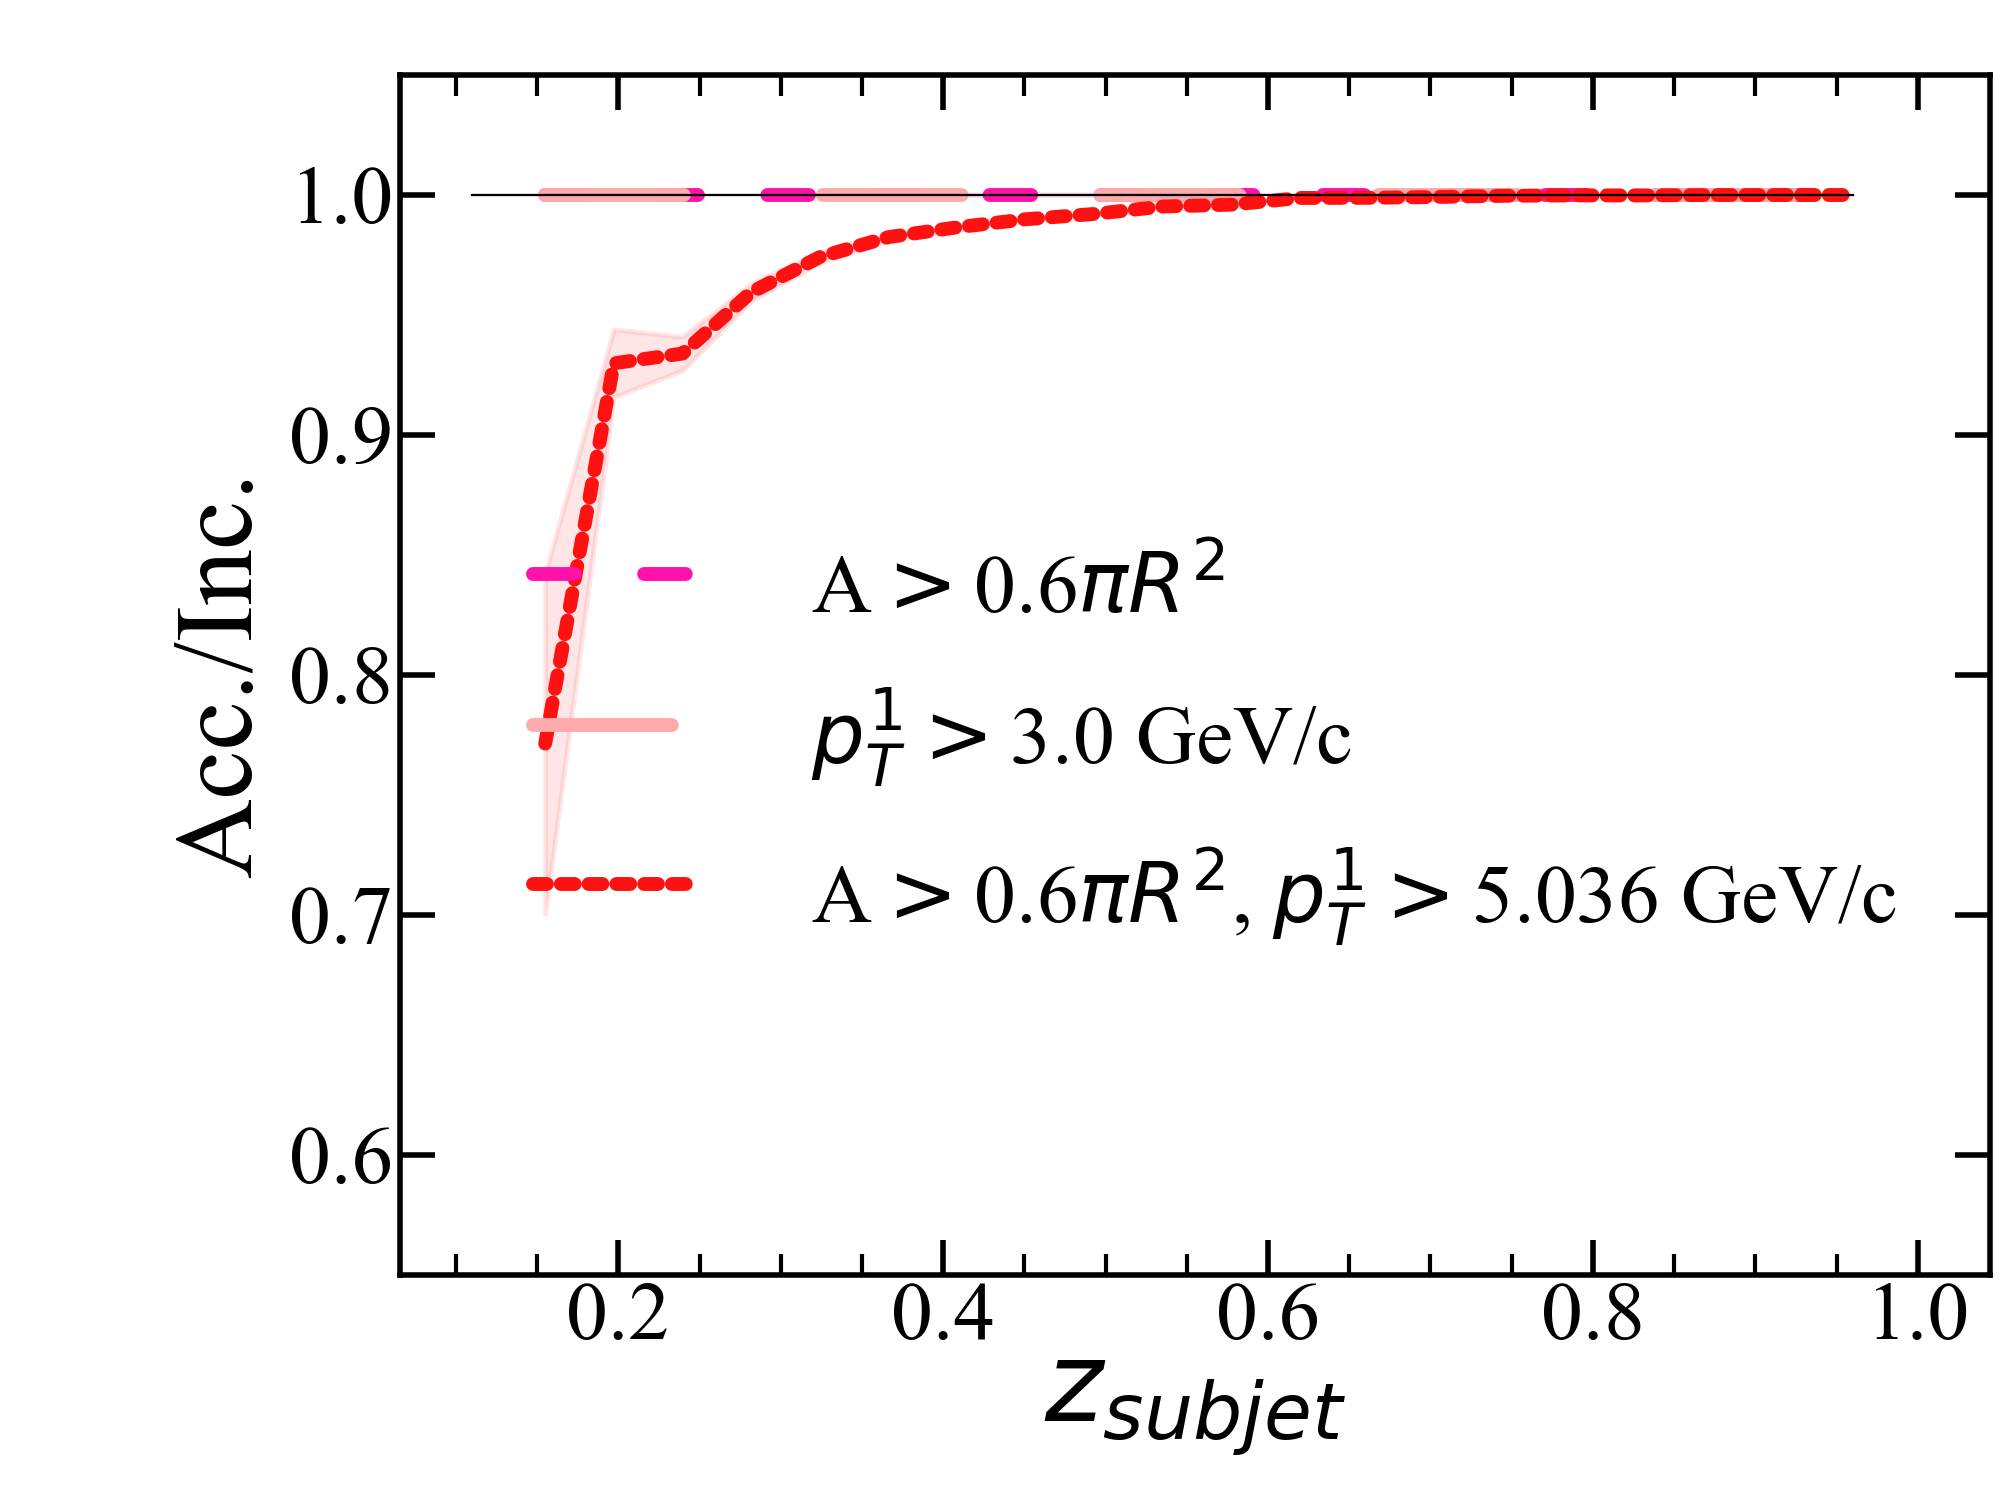}
    \caption{R=0.3 \ptH=40 \GeV}
    \label{fig:z_sub_03_40}
\end{figure*}

\begin{figure*}
    \centering
    \includegraphics[width=\linewidth]{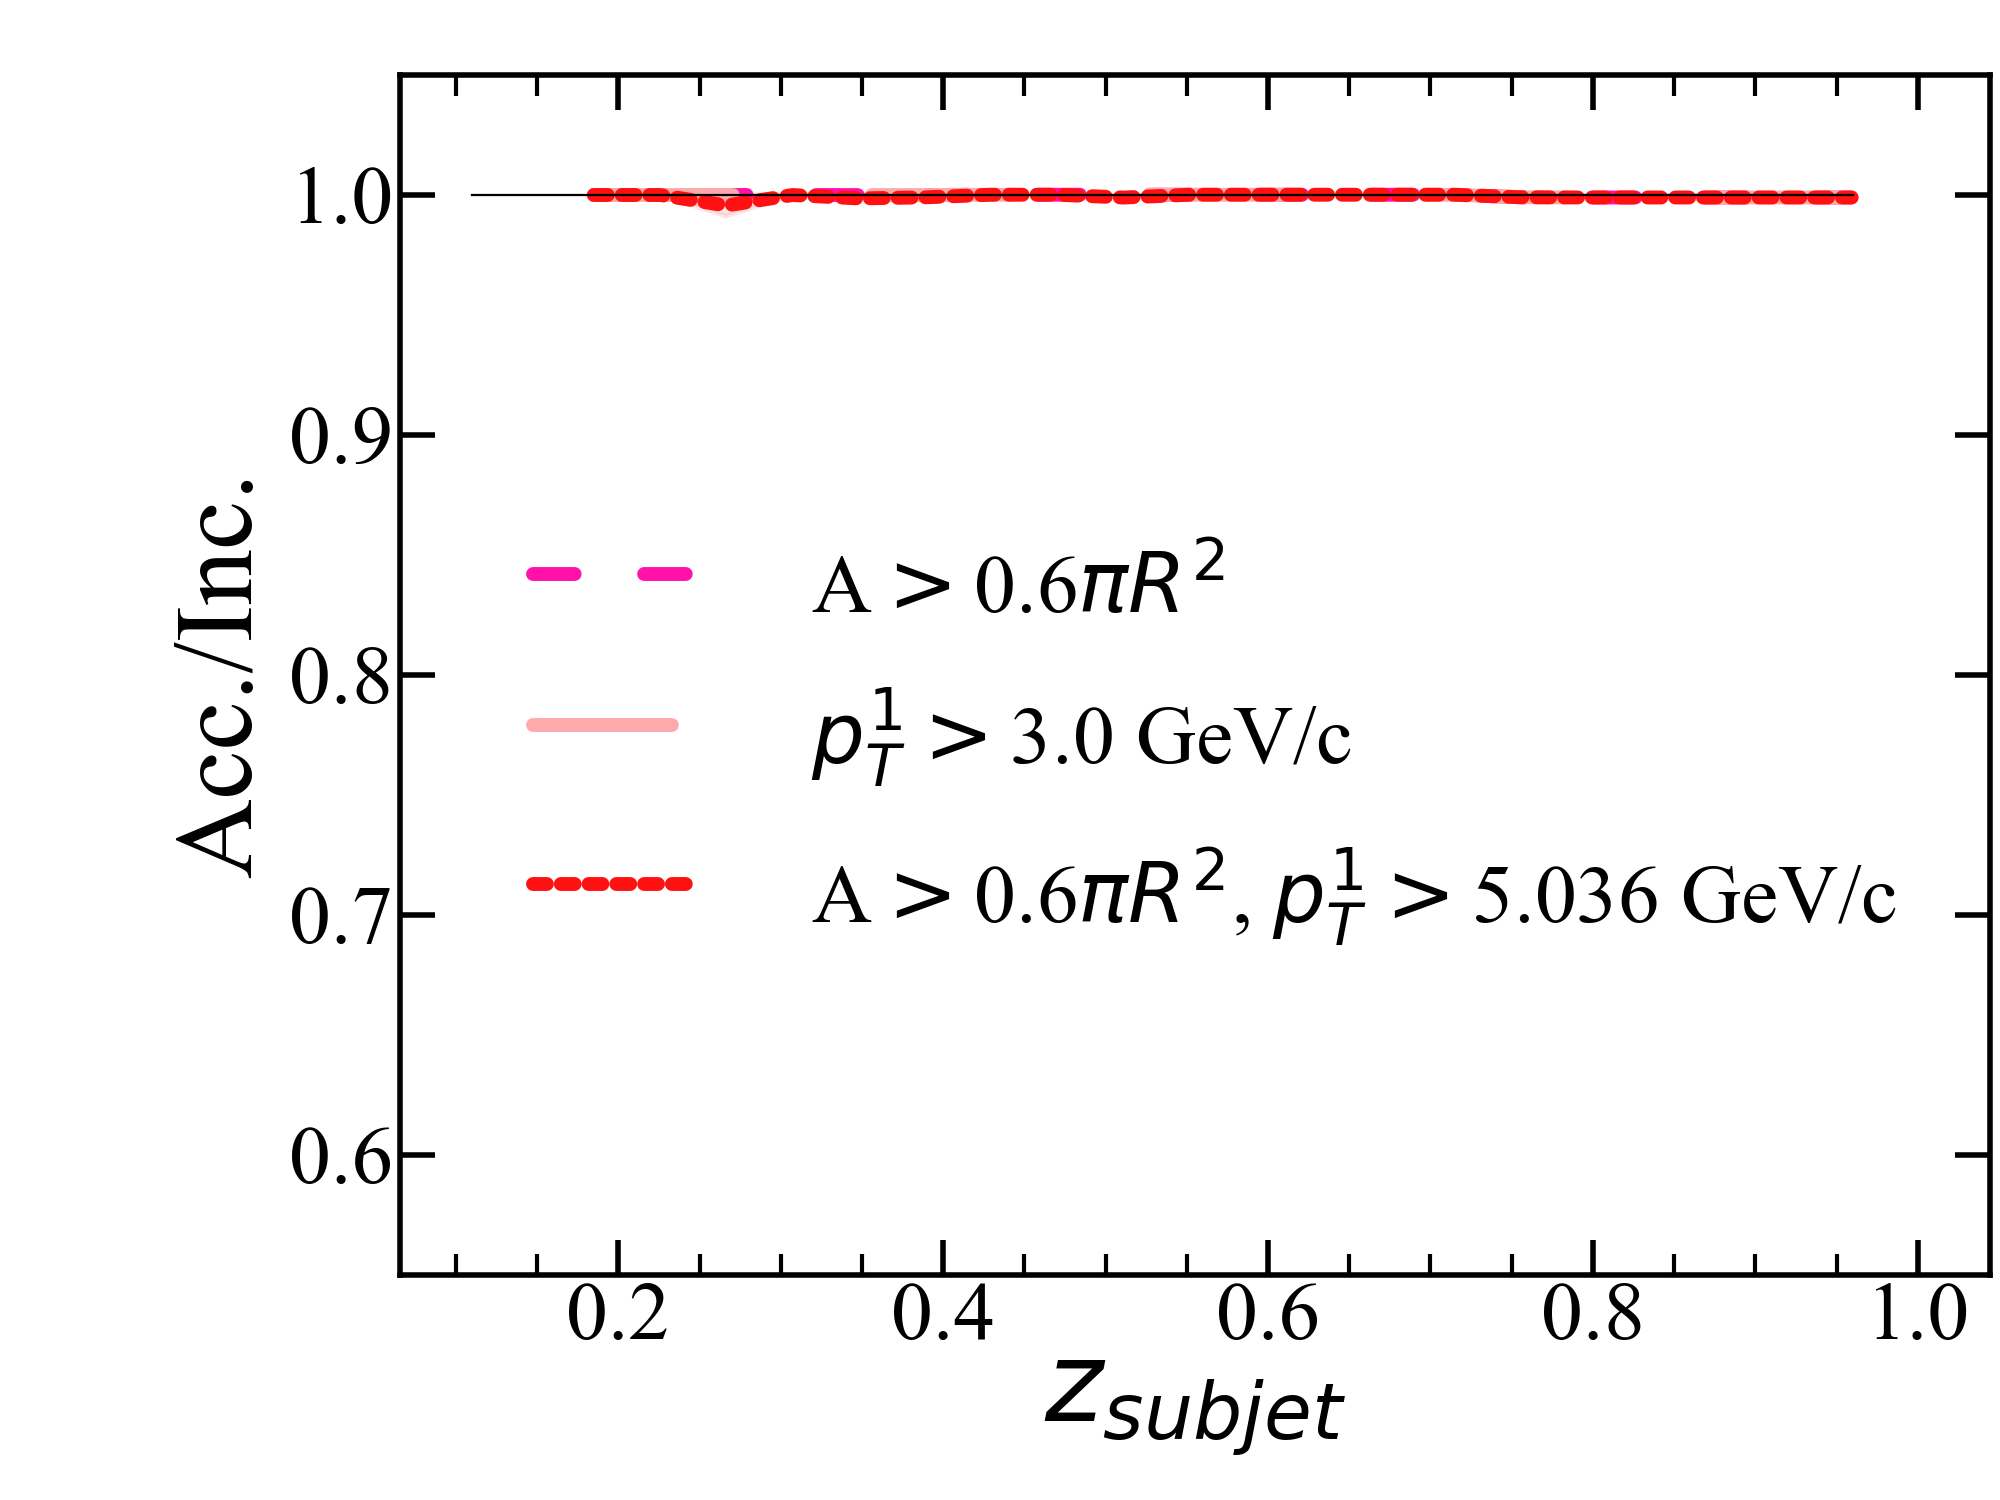}
    \caption{R=0.3 \ptH=60 \GeV}
    \label{fig:z_sub_03_60}
\end{figure*}

\begin{figure*}
    \centering
    \includegraphics[width=\linewidth]{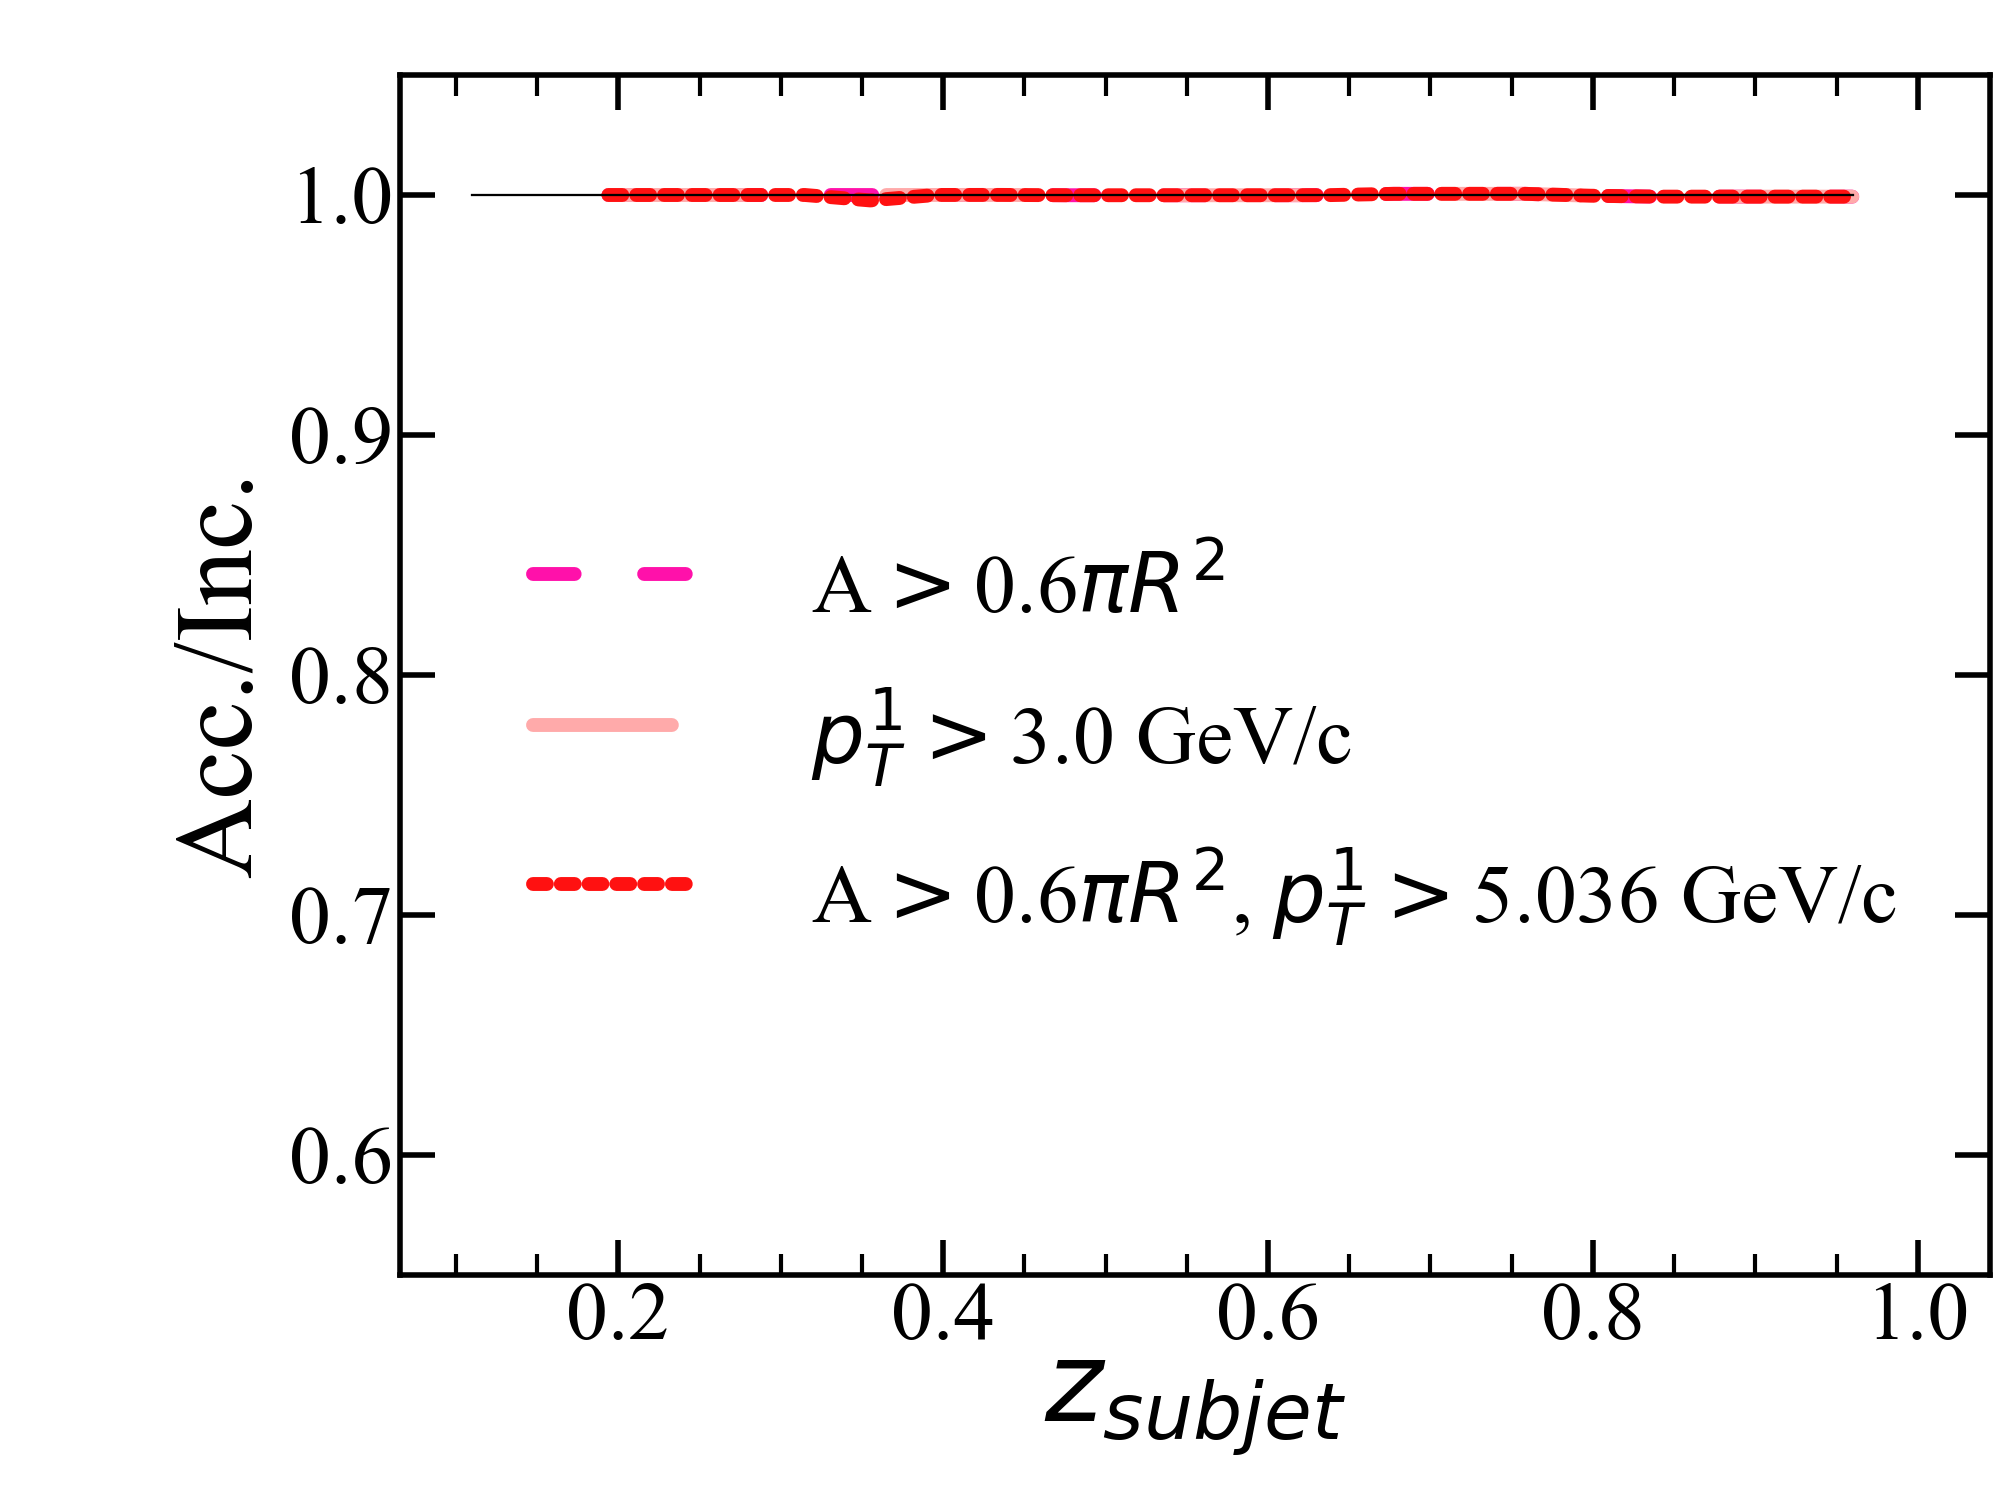}
    \caption{R=0.3 \ptH=80 \GeV}
    \label{fig:z_sub_03_80}
\end{figure*}

\begin{figure*}
    \centering
    \includegraphics[width=\linewidth]{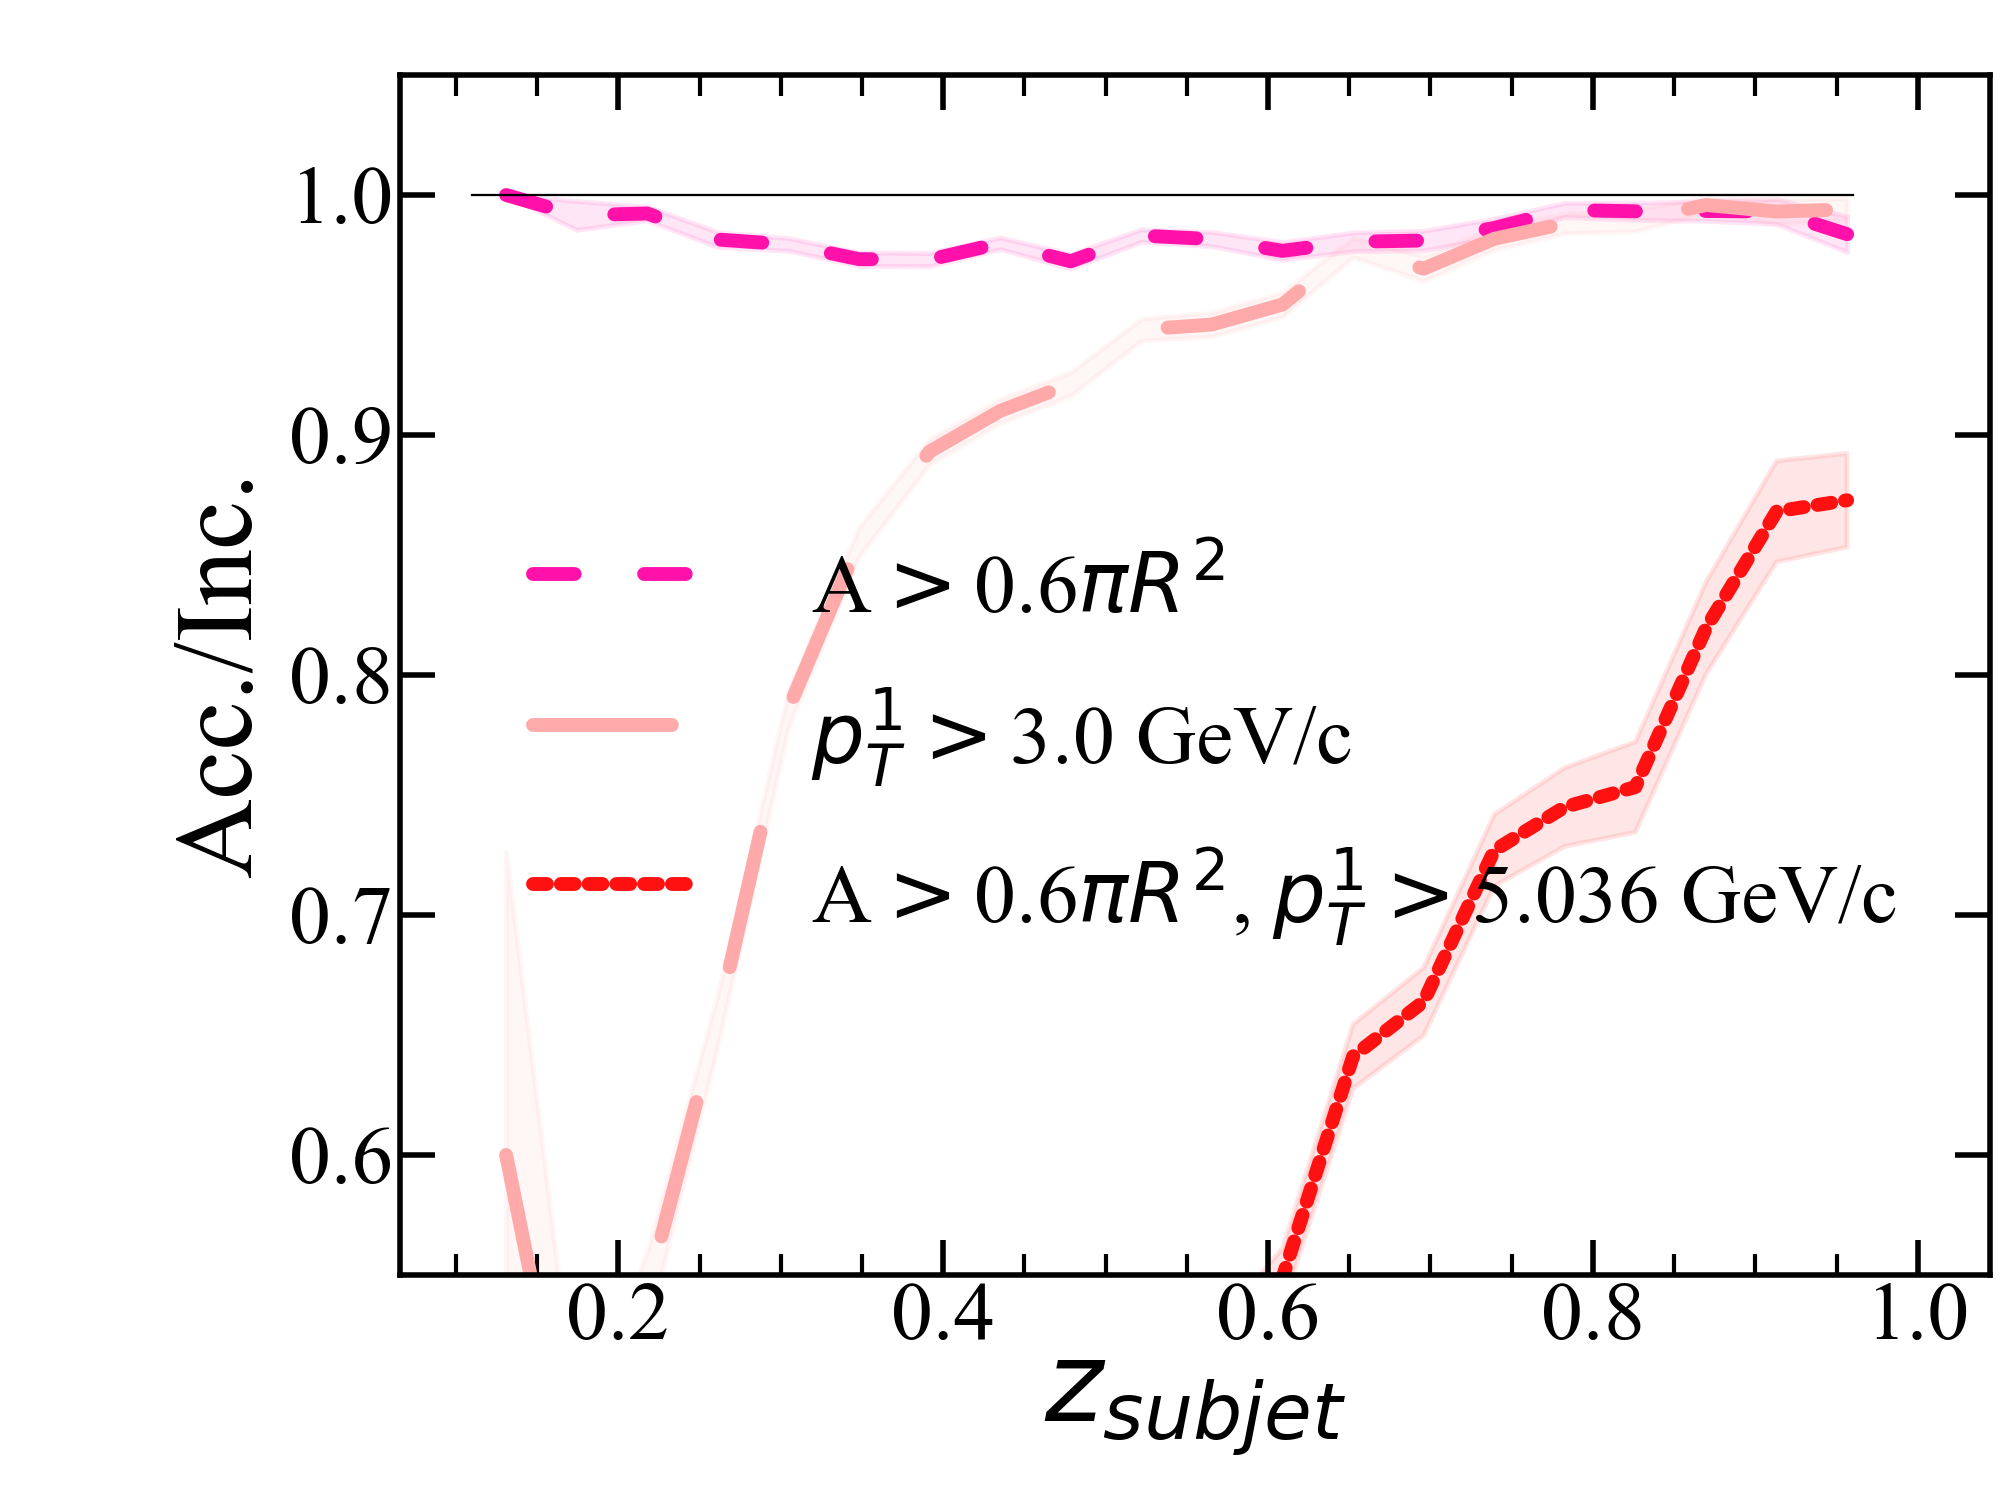}
    \caption{R=0.4 \ptH=10 \GeV}
    \label{fig:z_sub_04_10}
\end{figure*}

\begin{figure*}
    \centering
    \includegraphics[width=\linewidth]{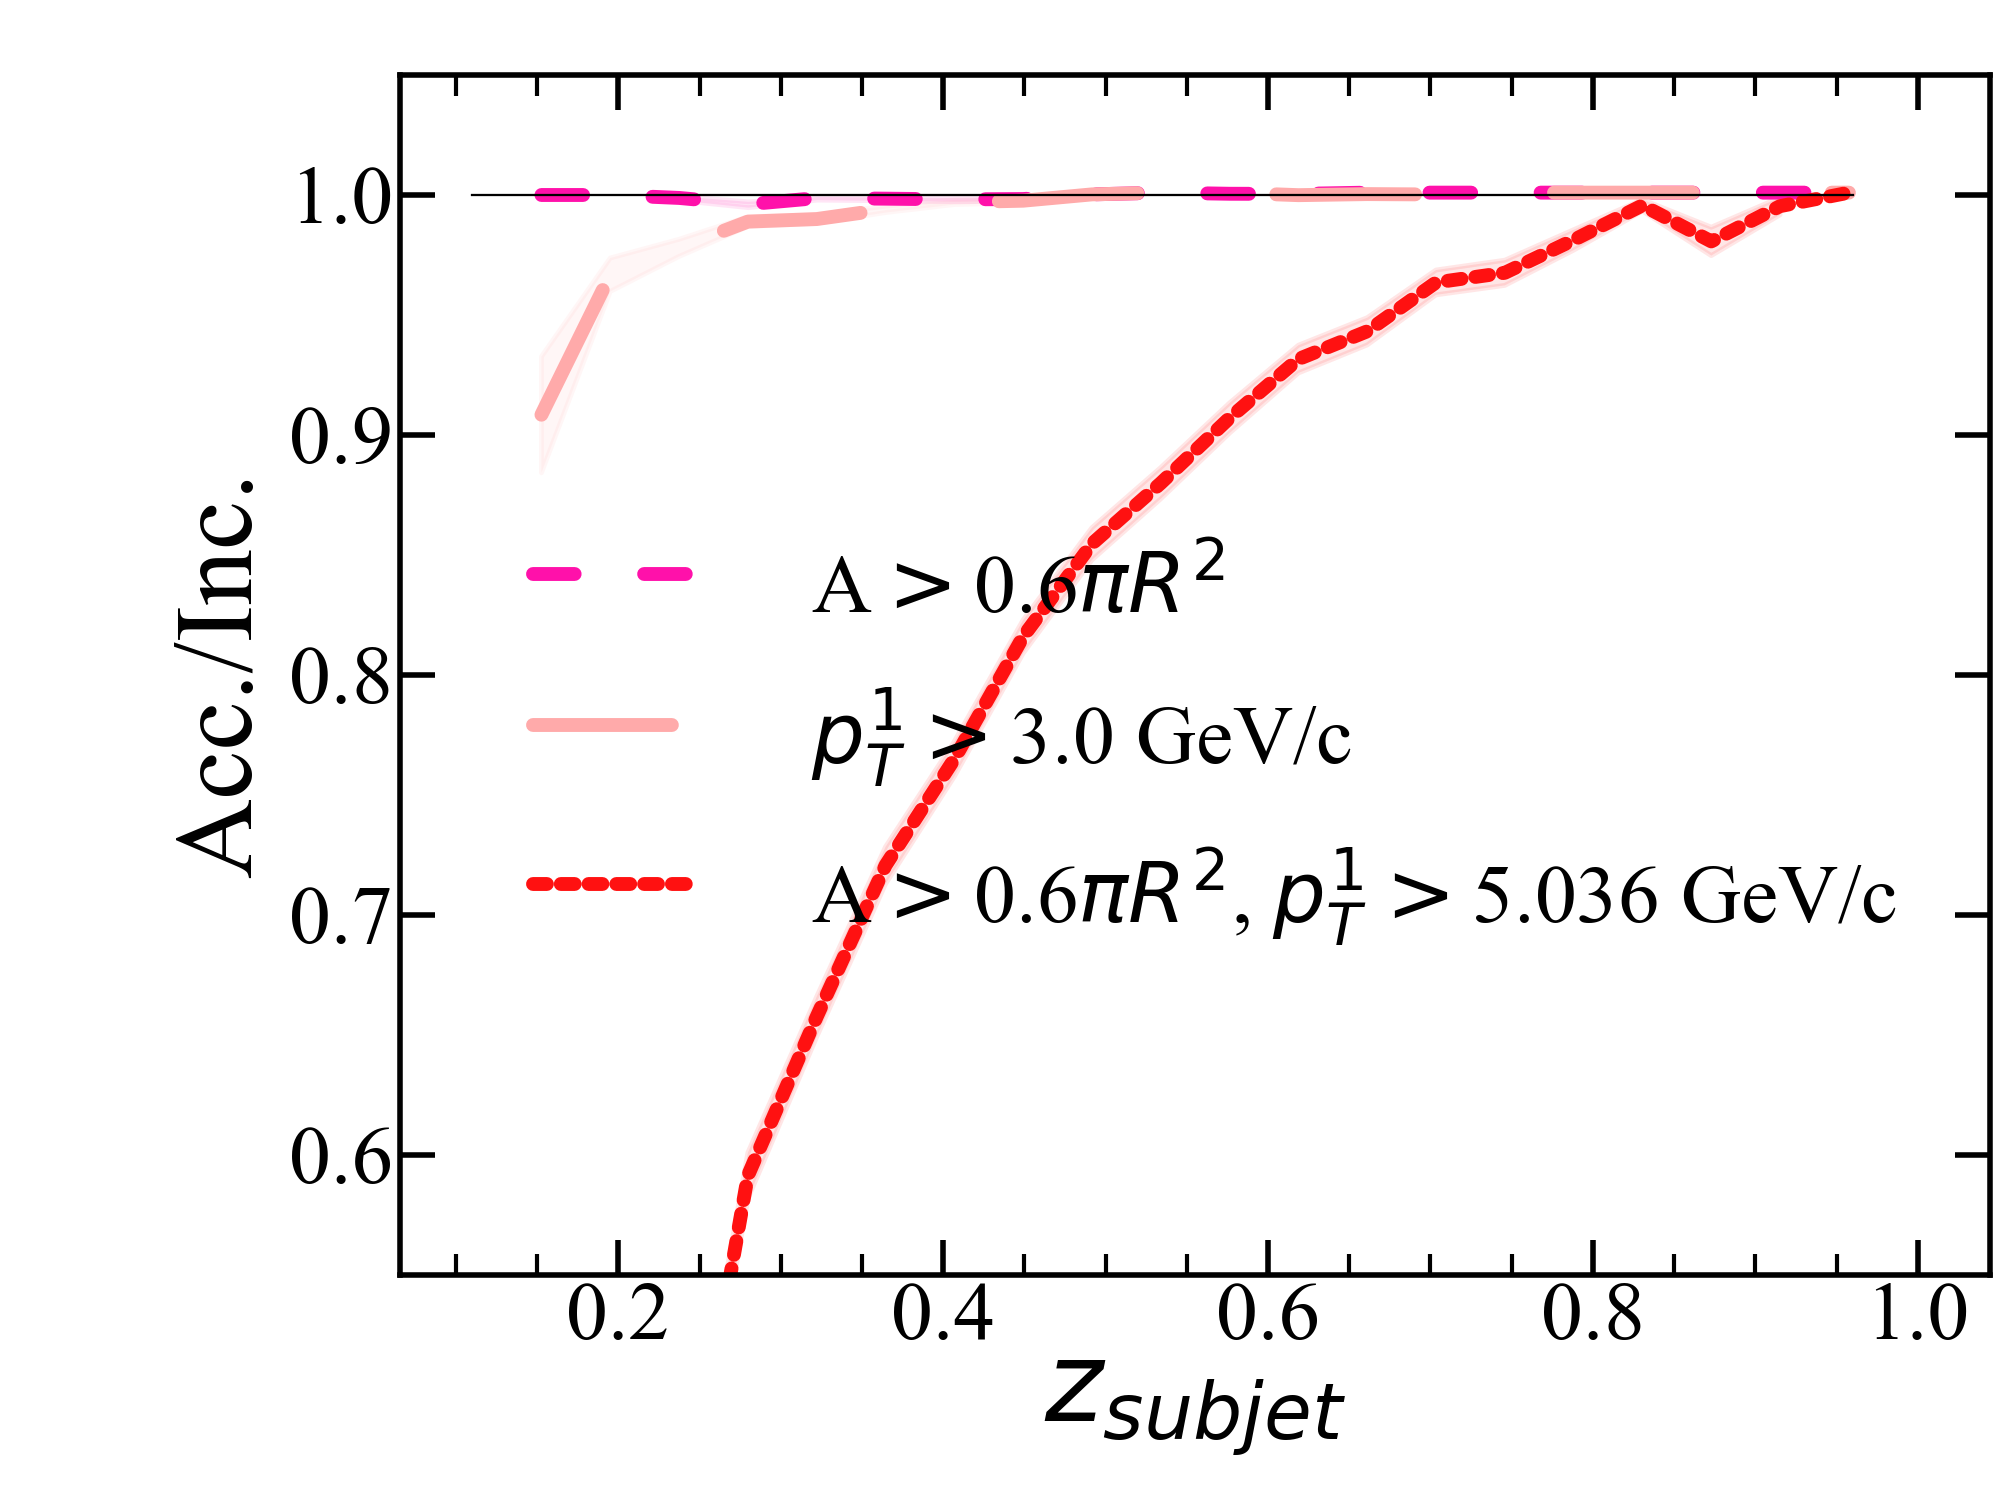}
    \caption{R=0.4 \ptH=20 \GeV}
    \label{fig:z_sub_04_20}
\end{figure*}

\begin{figure*}
    \centering
    \includegraphics[width=\linewidth]{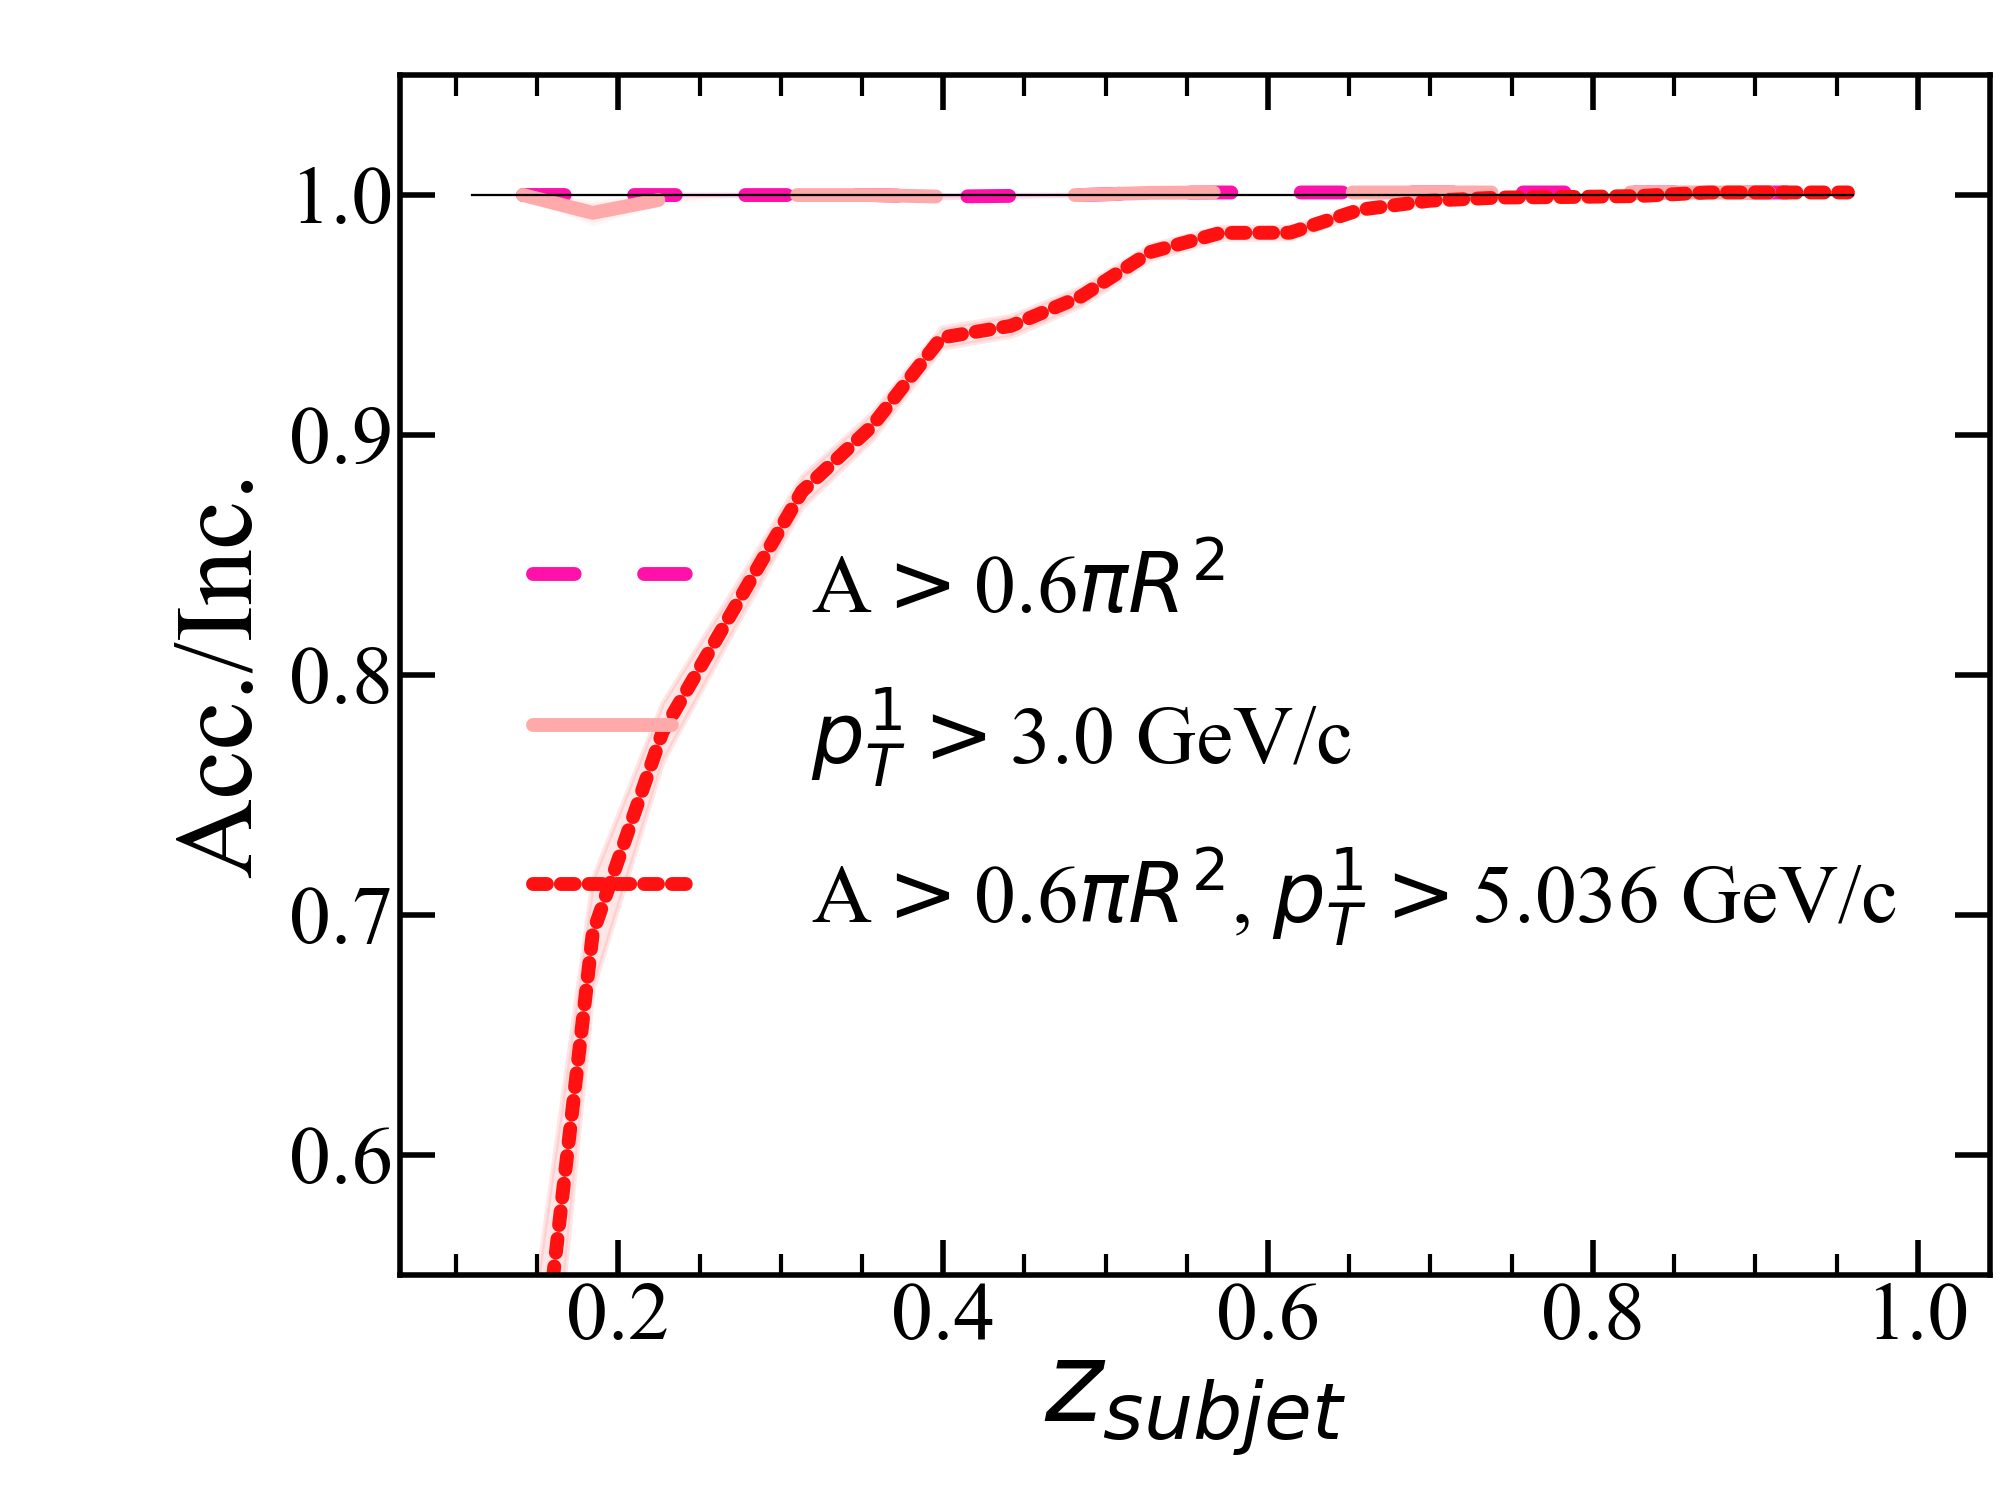}
    \caption{R=0.4 \ptH=30 \GeV}
    \label{fig:z_sub_04_30}
\end{figure*}

\begin{figure*}
    \centering
    \includegraphics[width=\linewidth]{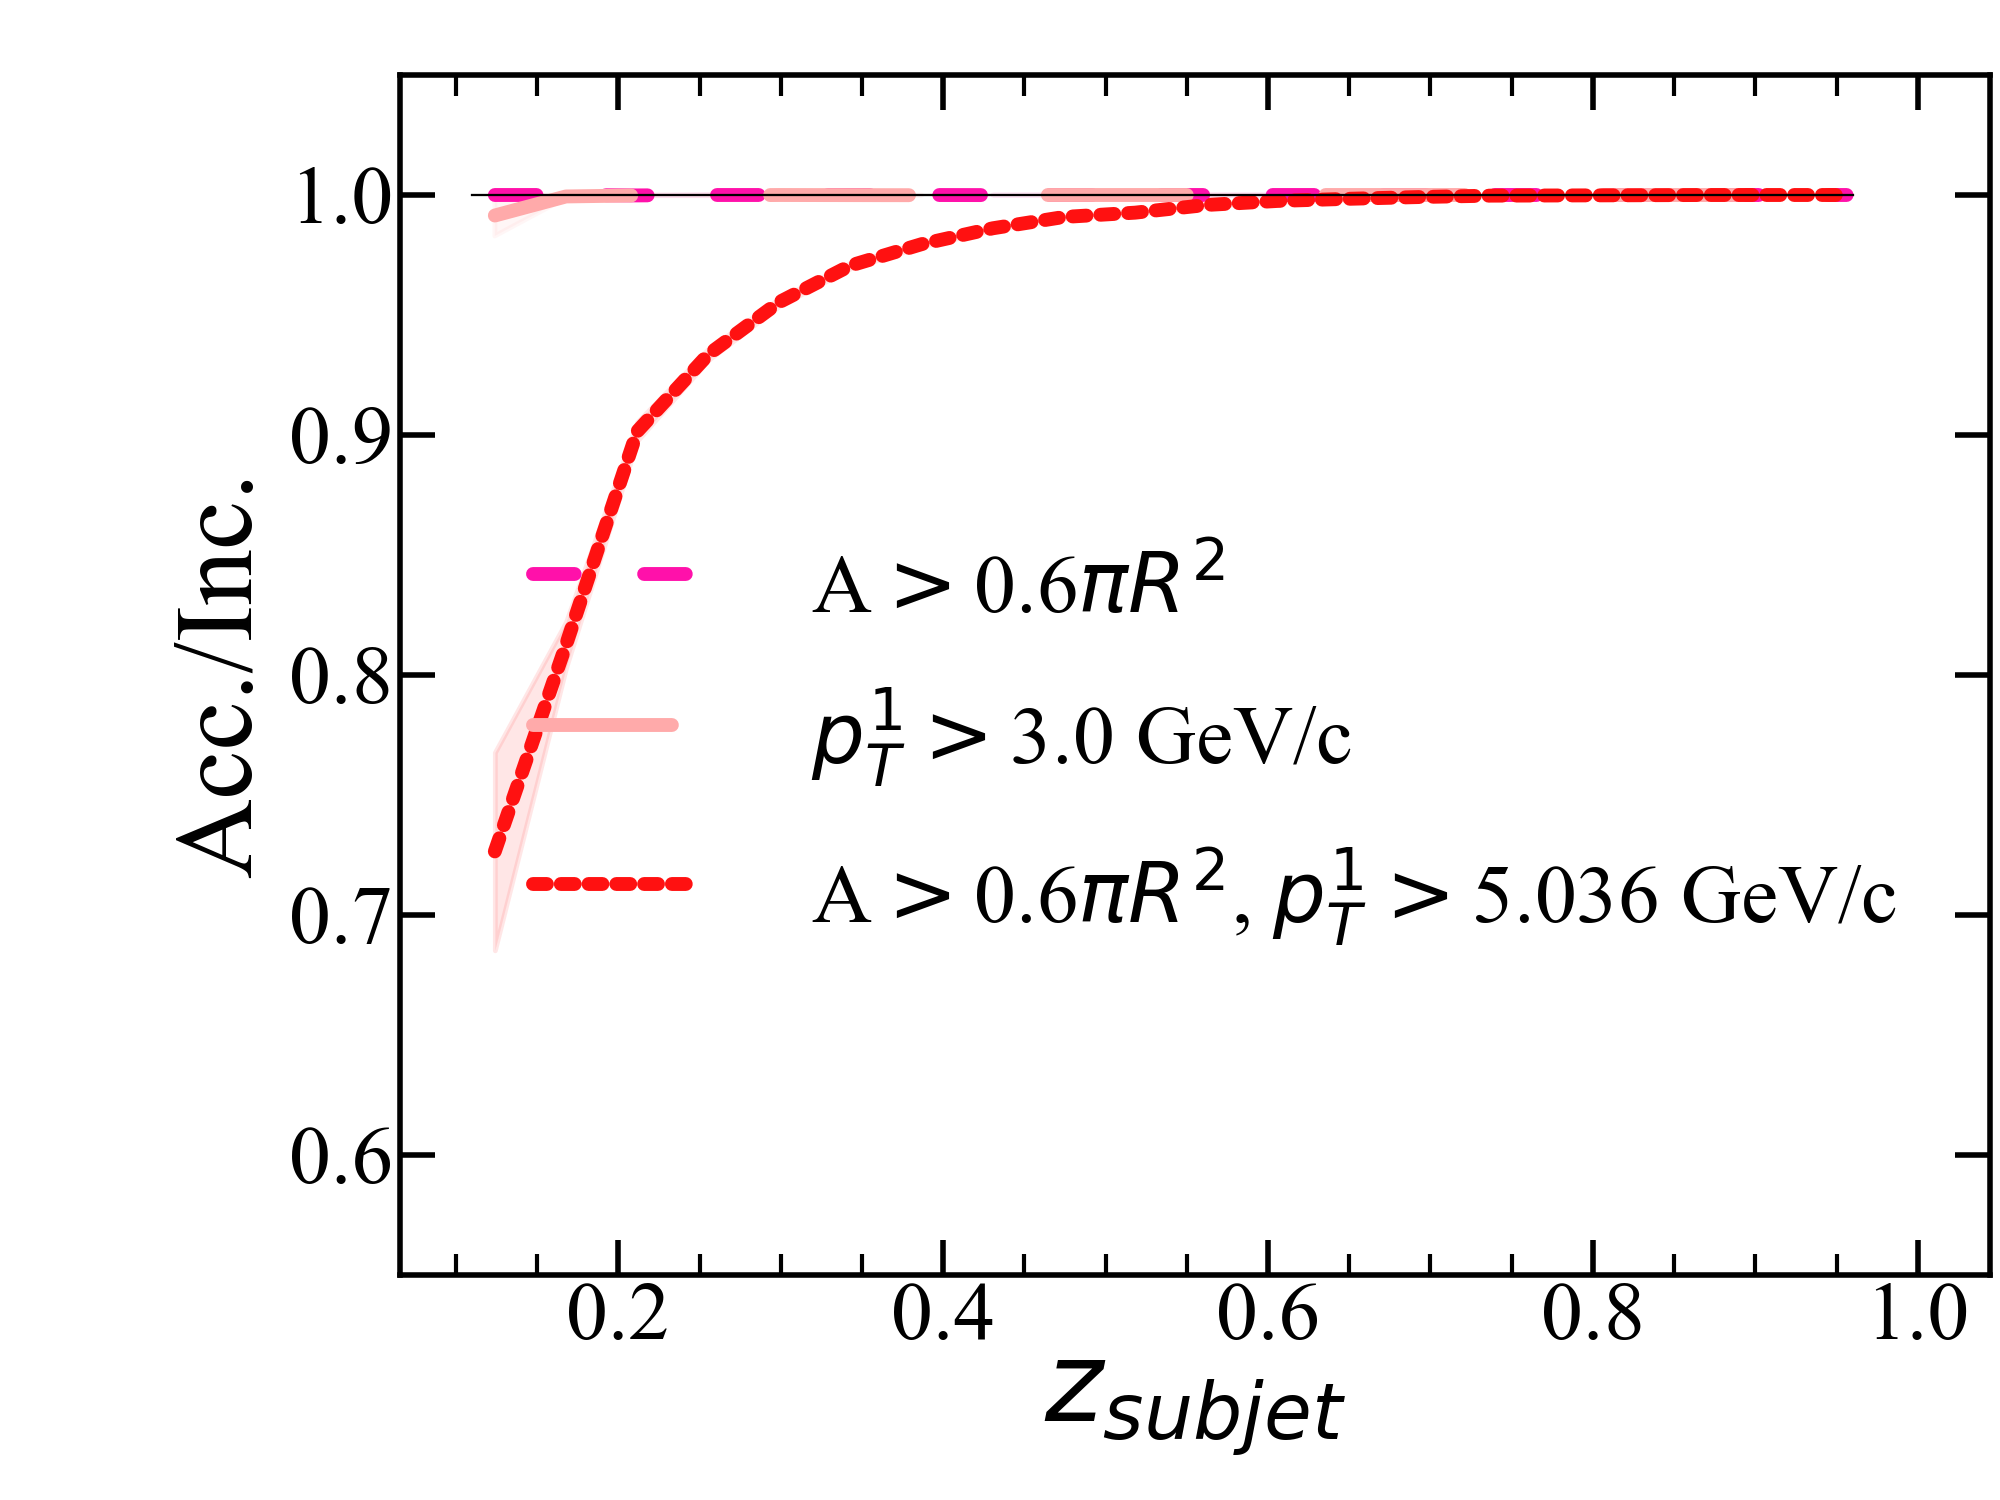}
    \caption{R=0.4 \ptH=40 \GeV}
    \label{fig:z_sub_04_40}
\end{figure*}

\begin{figure*}
    \centering
    \includegraphics[width=\linewidth]{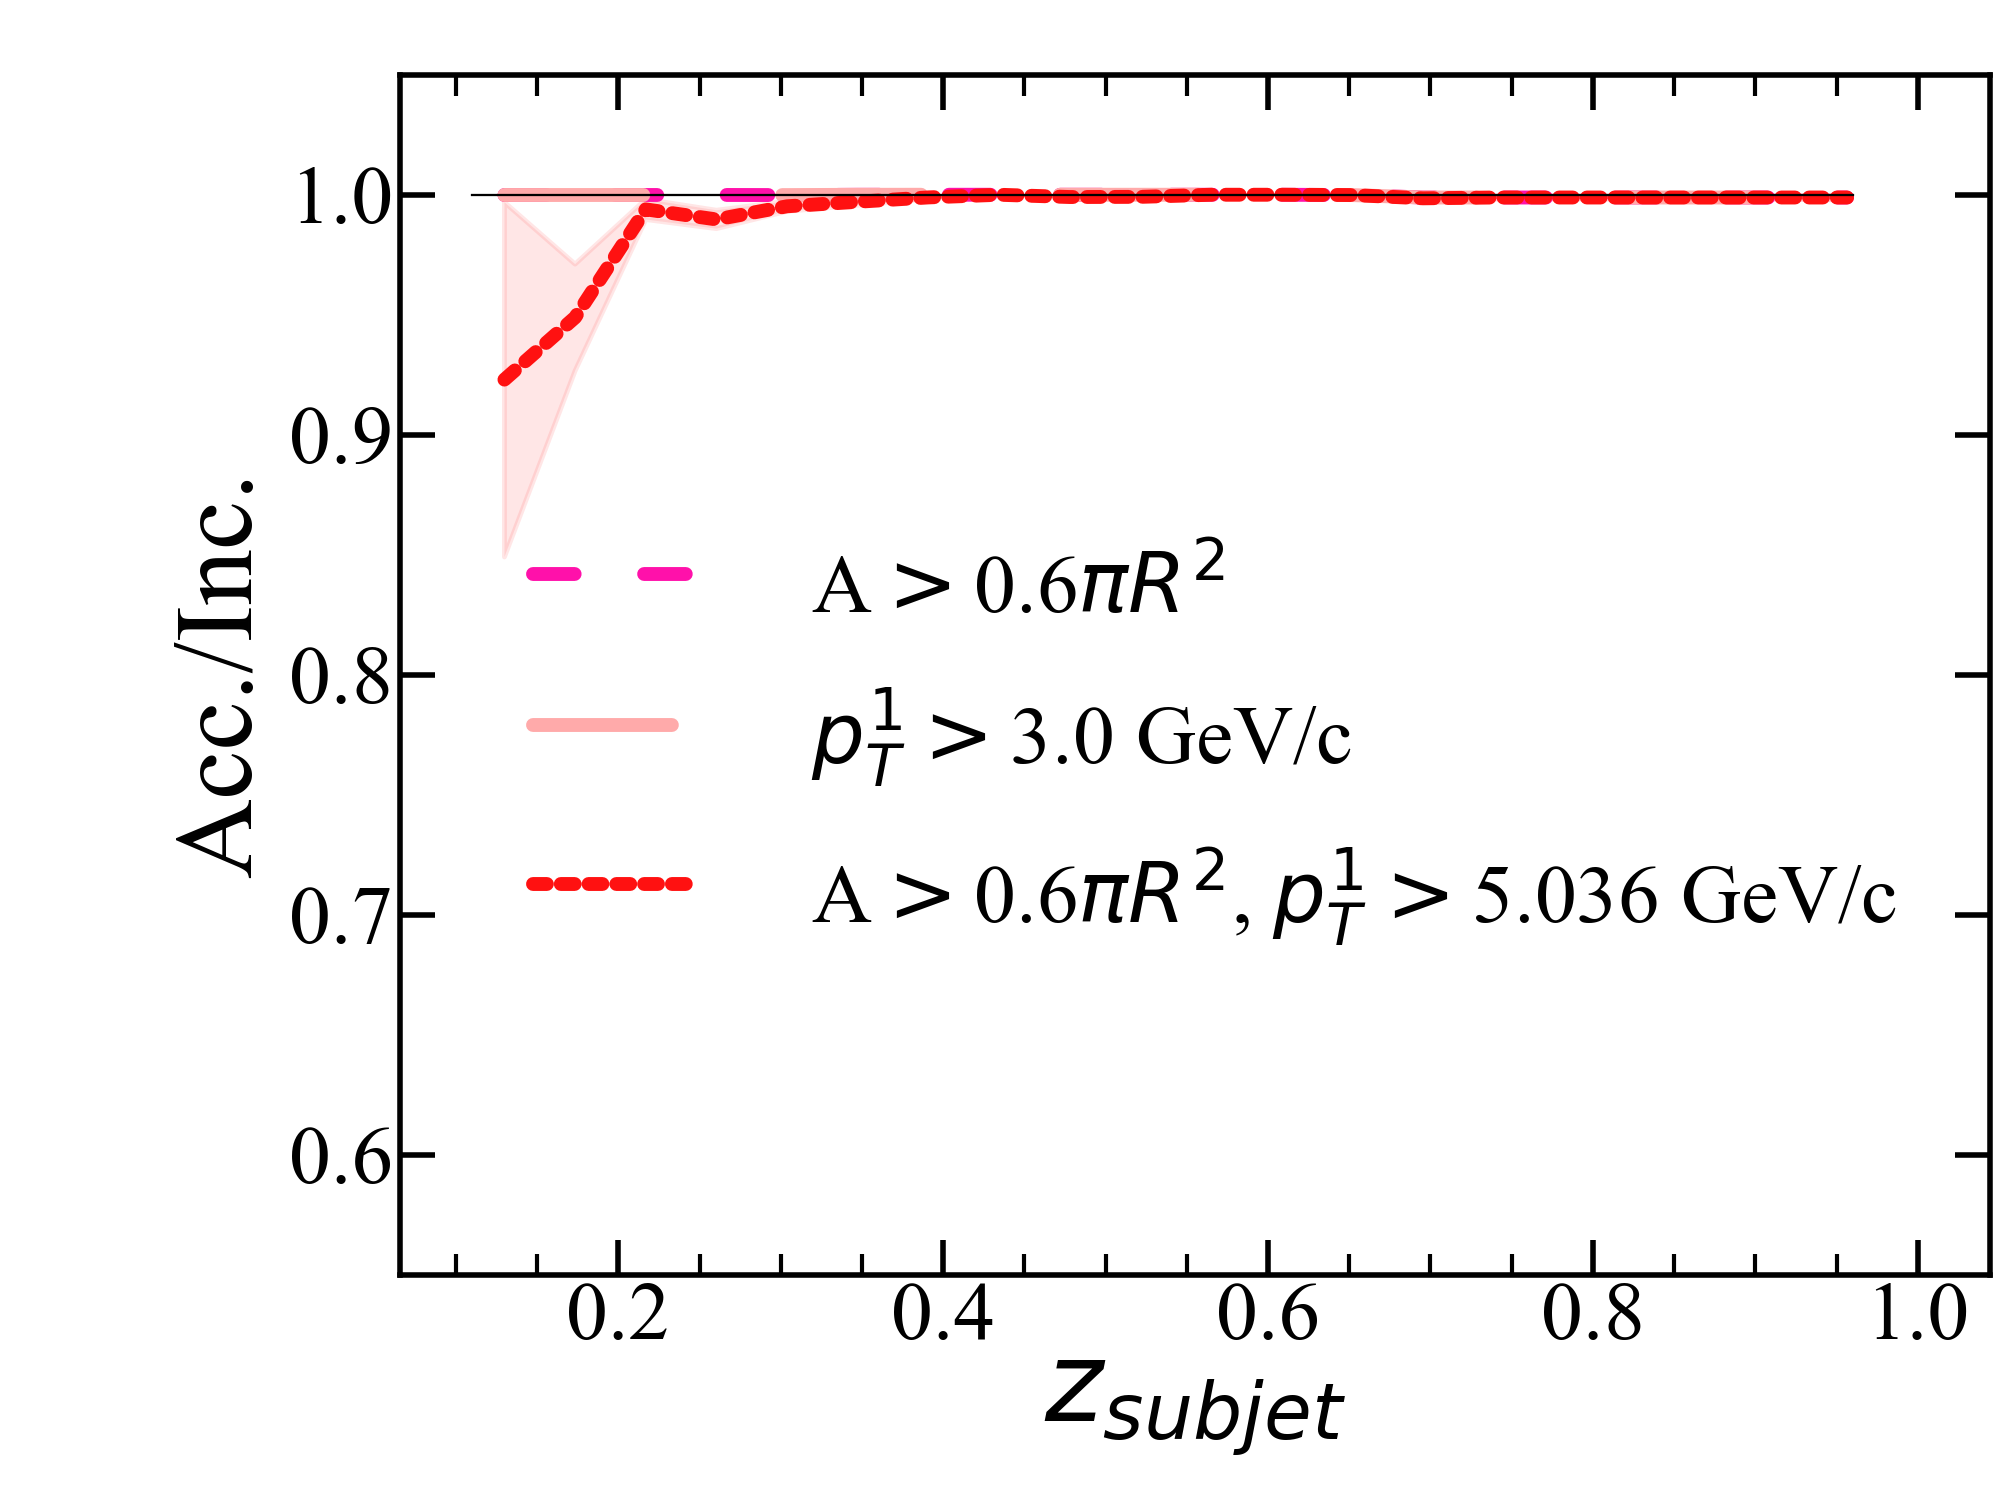}
    \caption{R=0.4 \ptH=60 \GeV}
    \label{fig:z_sub_04_60}
\end{figure*}

\begin{figure*}
    \centering
    \includegraphics[width=\linewidth]{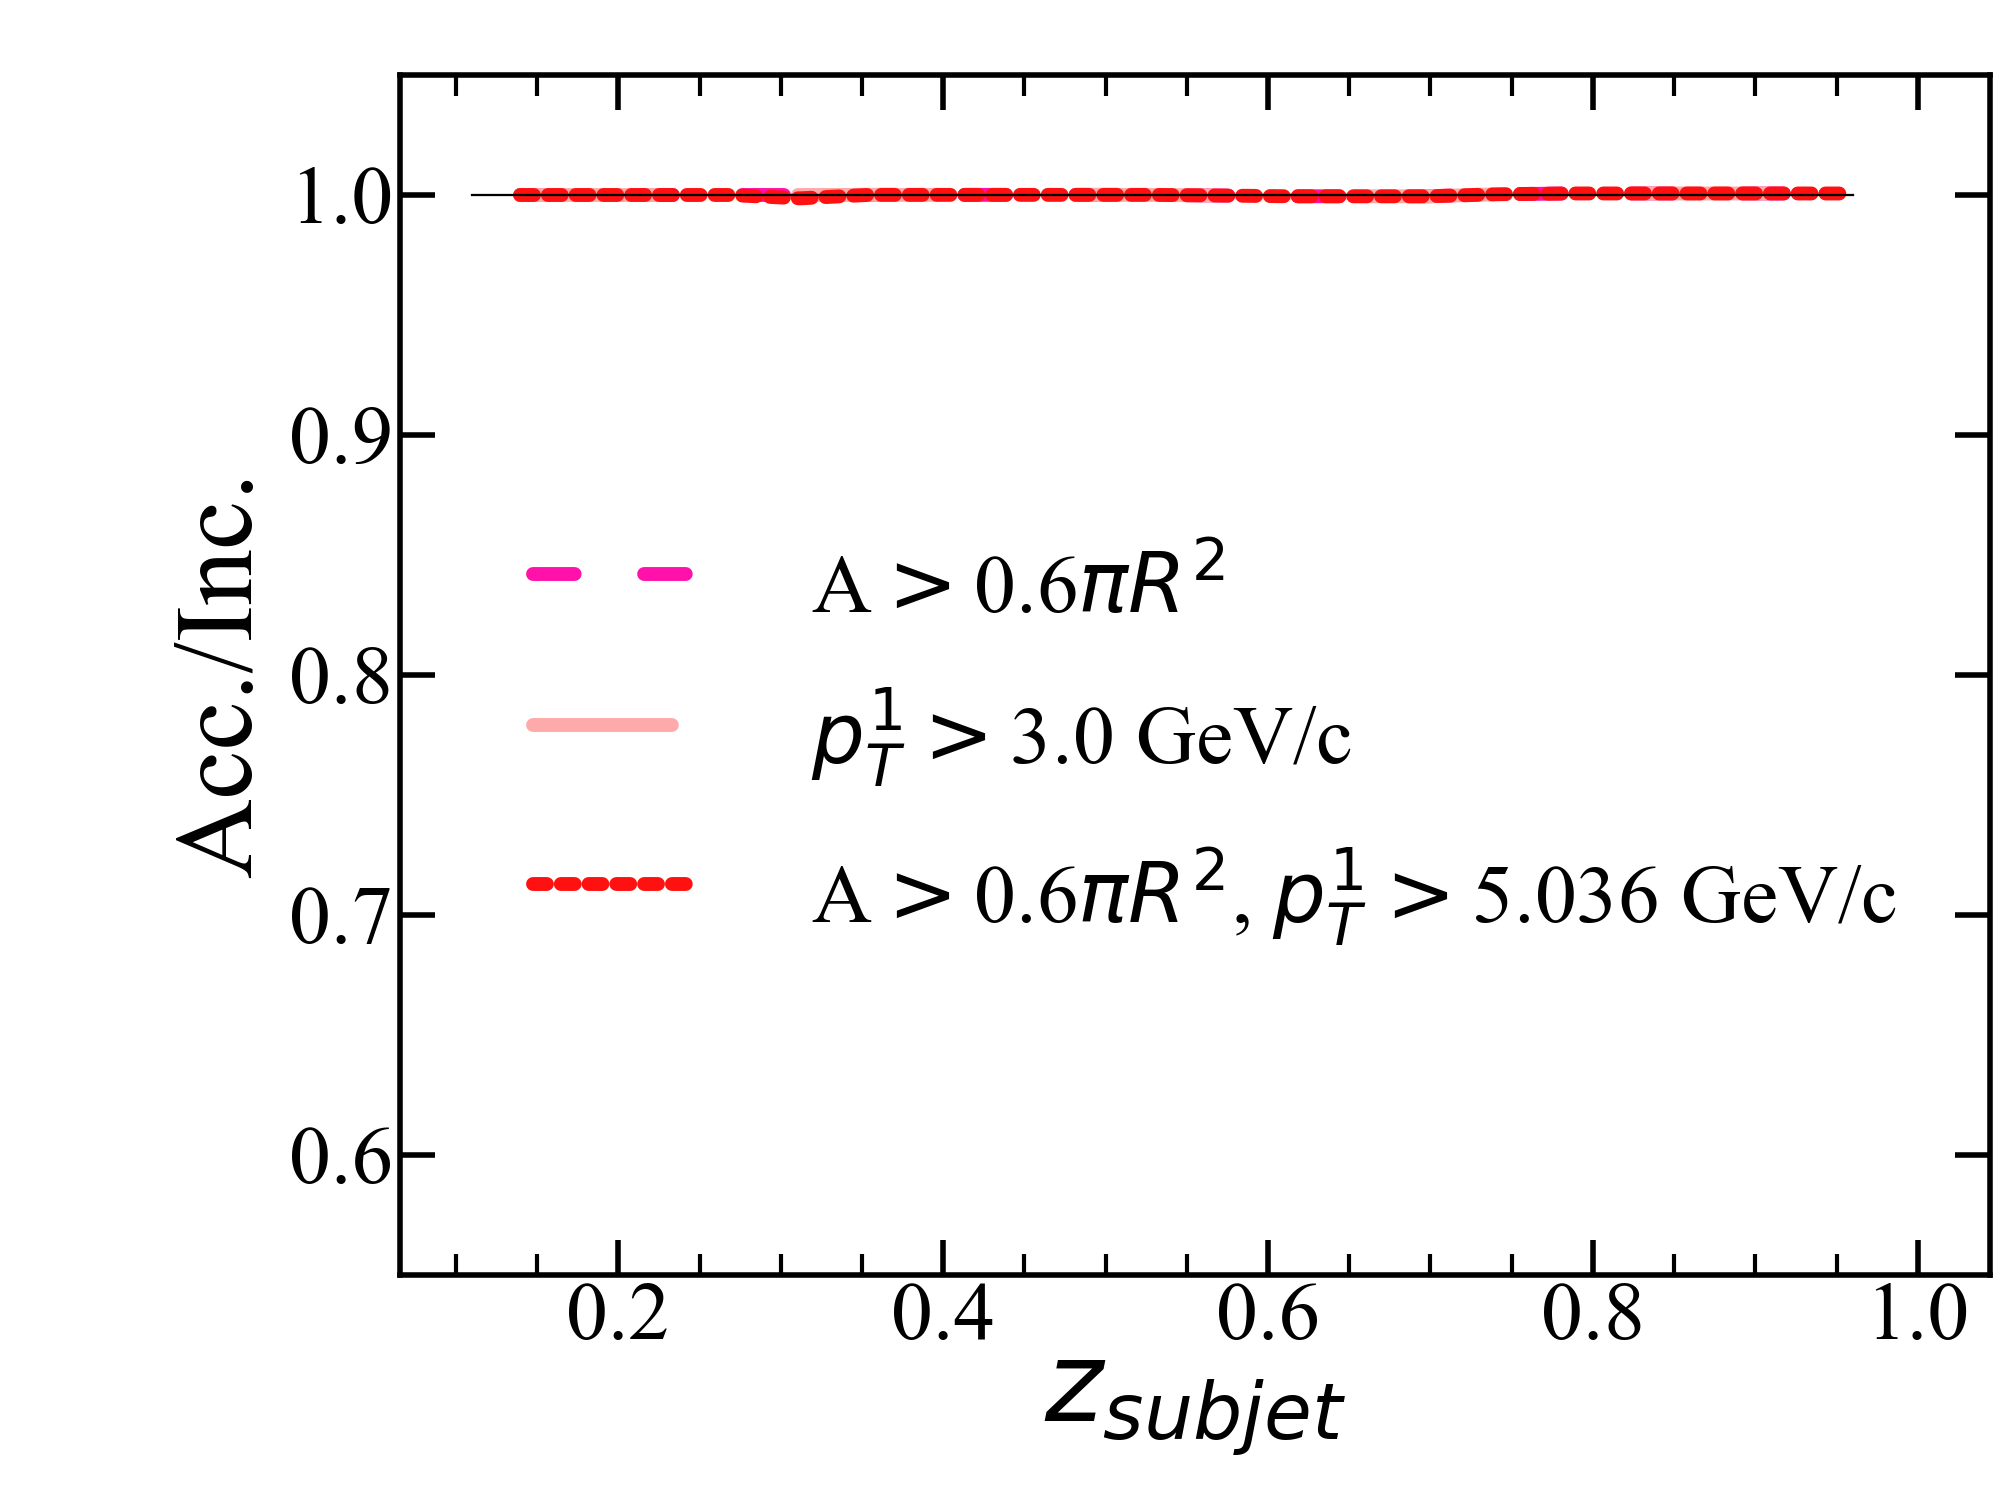}
    \caption{R=0.4 \ptH=80 \GeV}
    \label{fig:z_sub_04_80}
\end{figure*}

\begin{figure*}
    \centering
    \includegraphics[width=\linewidth]{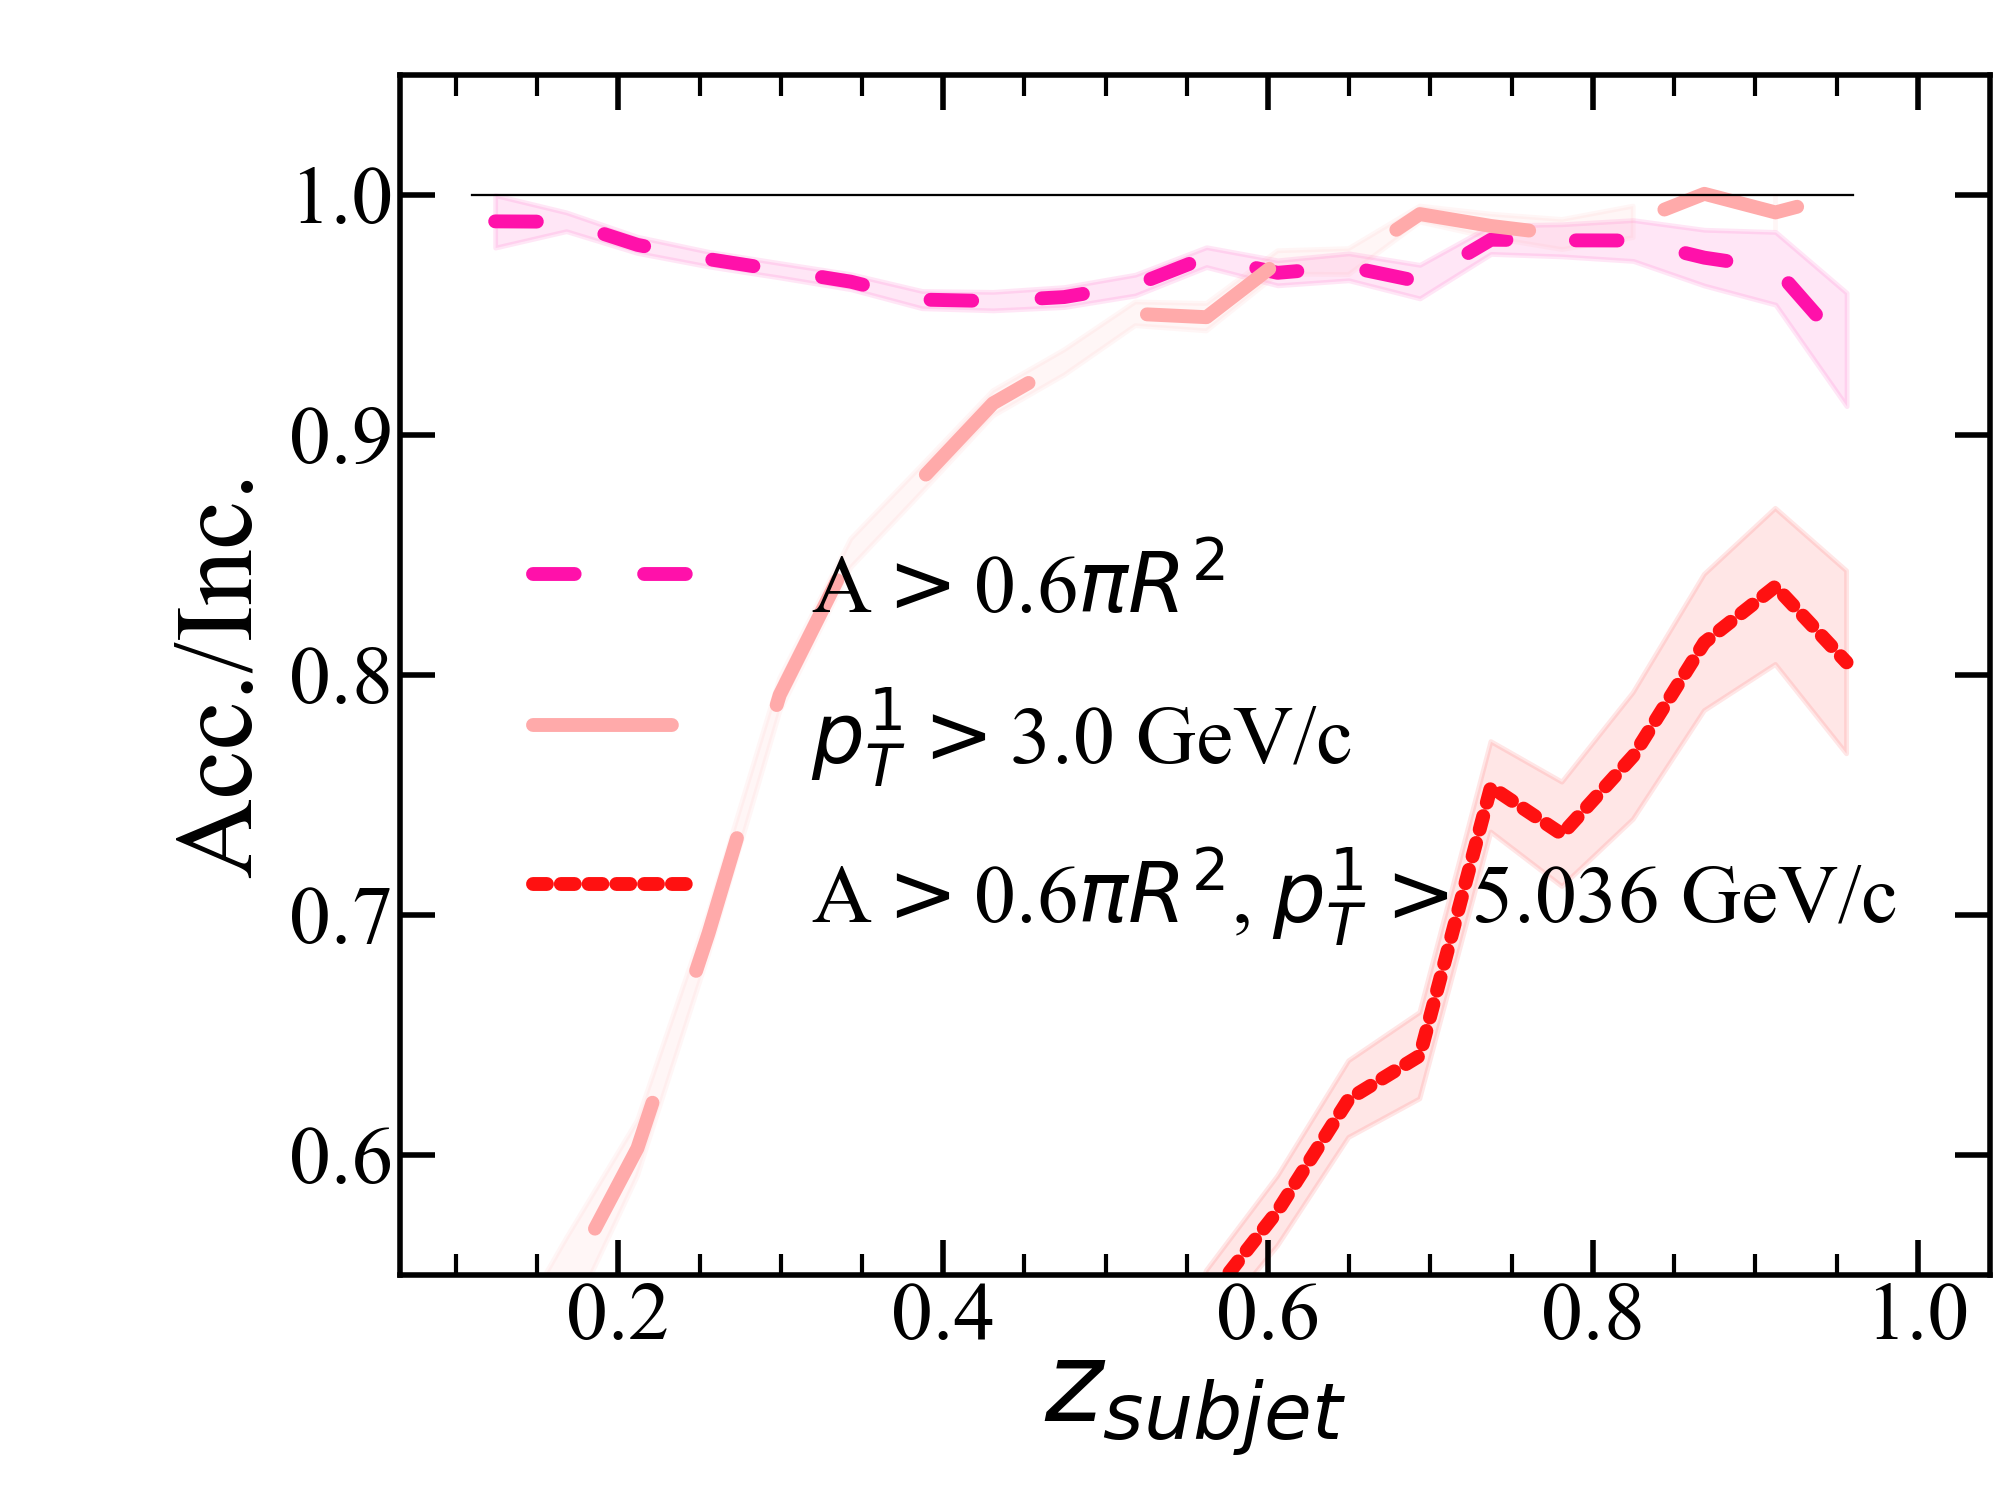}
    \caption{R=0.5 \ptH=10 \GeV}
    \label{fig:z_sub_05_10}
\end{figure*}

\begin{figure*}
    \centering
    \includegraphics[width=\linewidth]{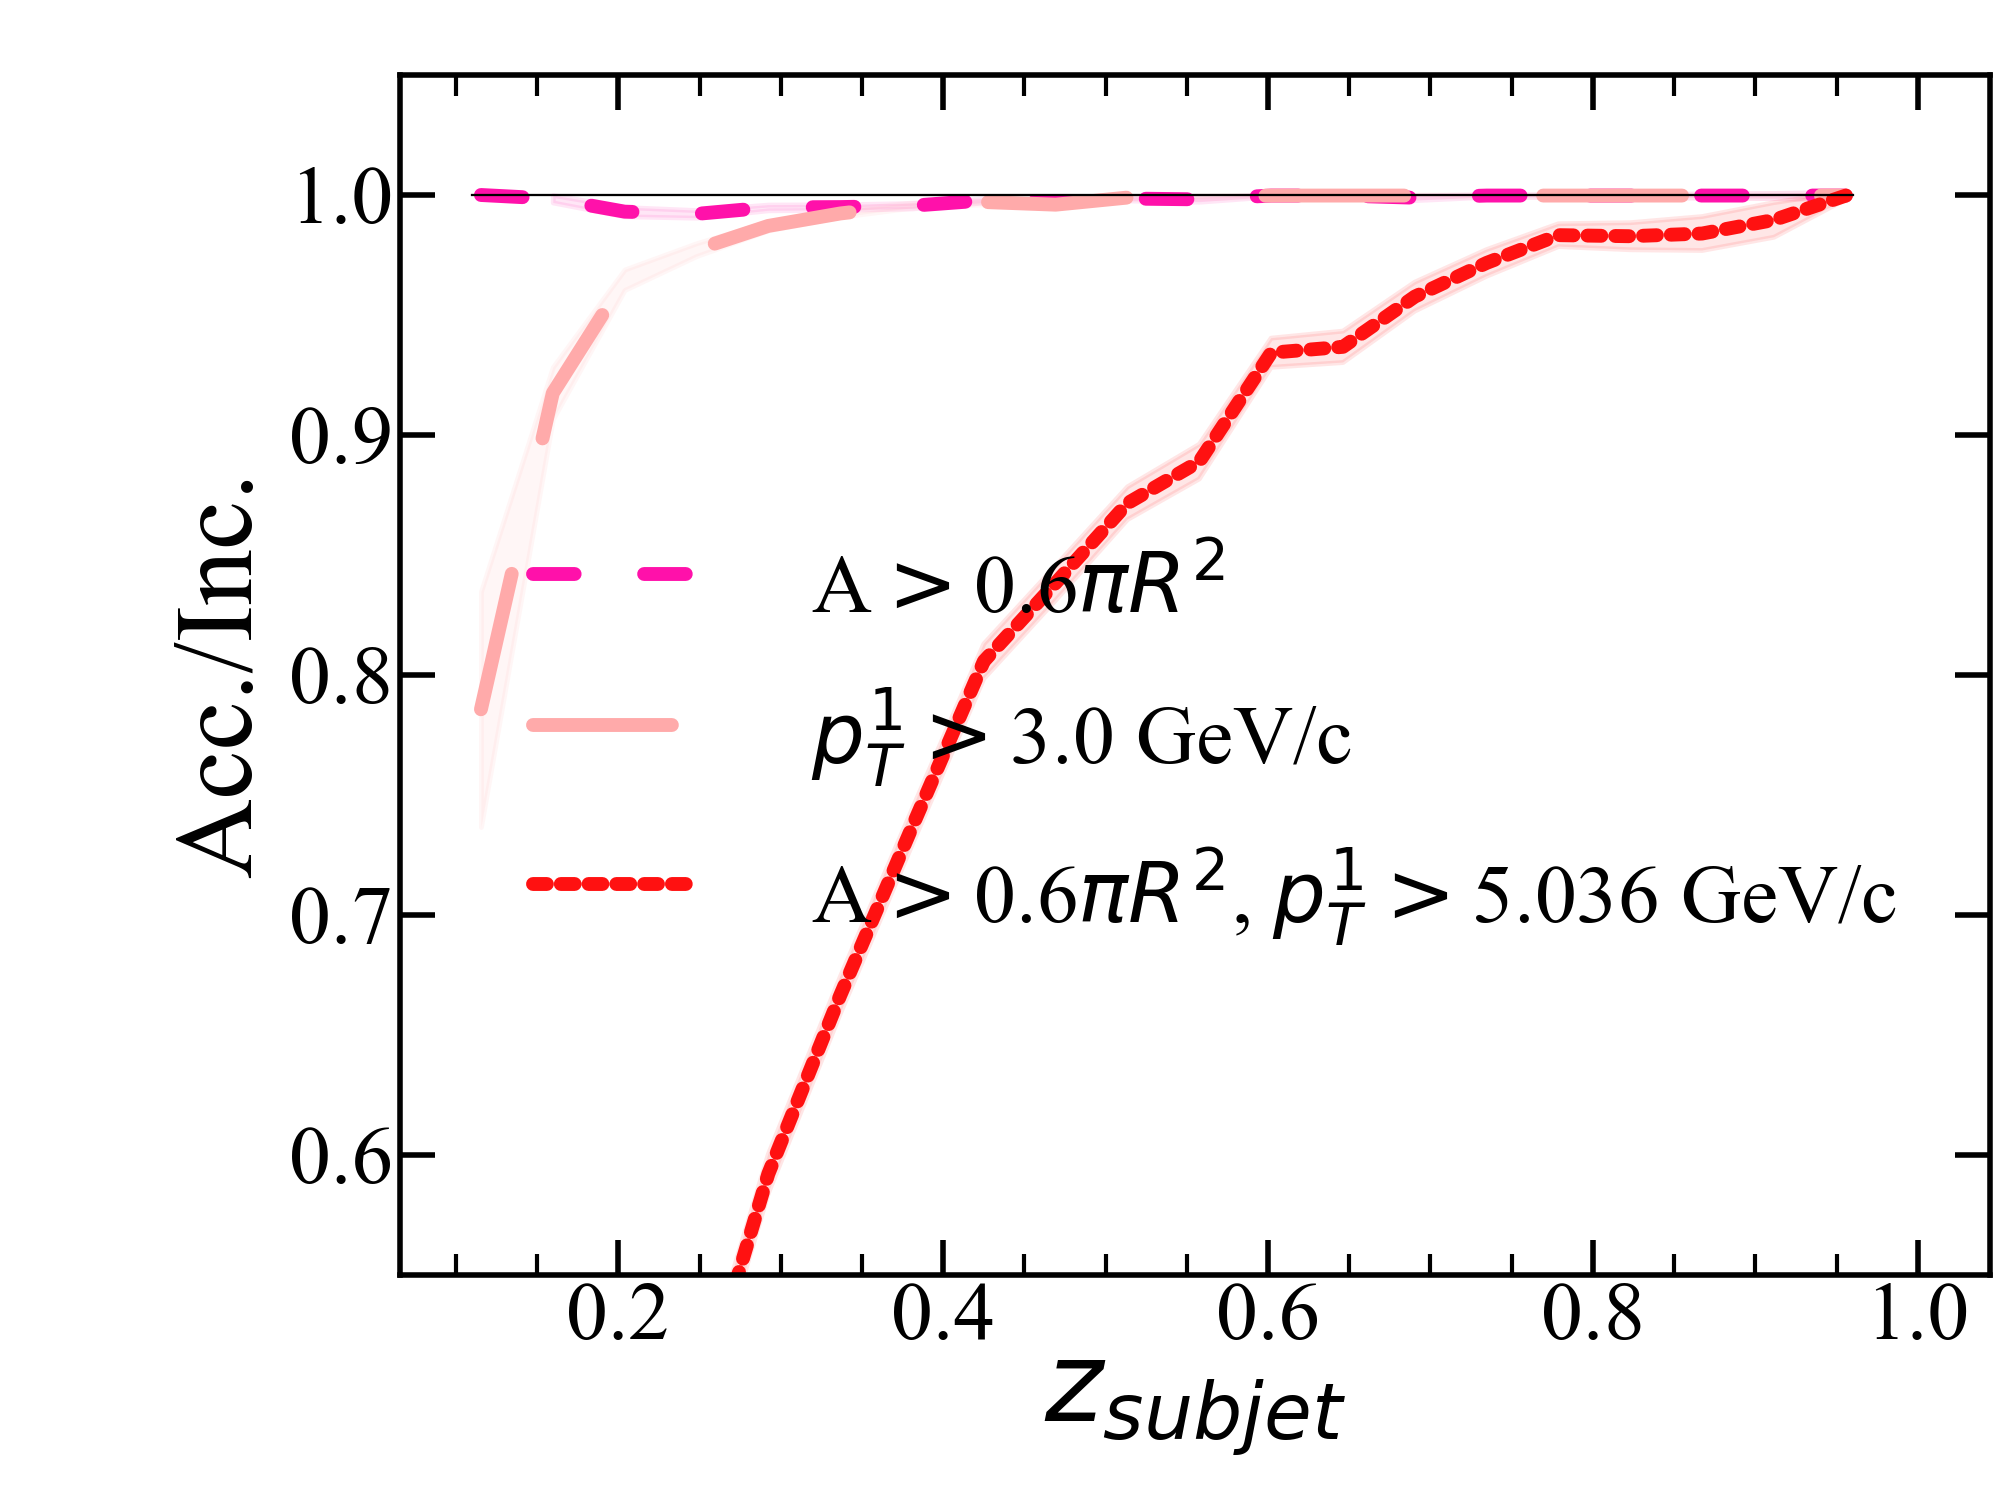}
    \caption{R=0.5 \ptH=20 \GeV}
    \label{fig:z_sub_05_20}
\end{figure*}

\begin{figure*}
    \centering
    \includegraphics[width=\linewidth]{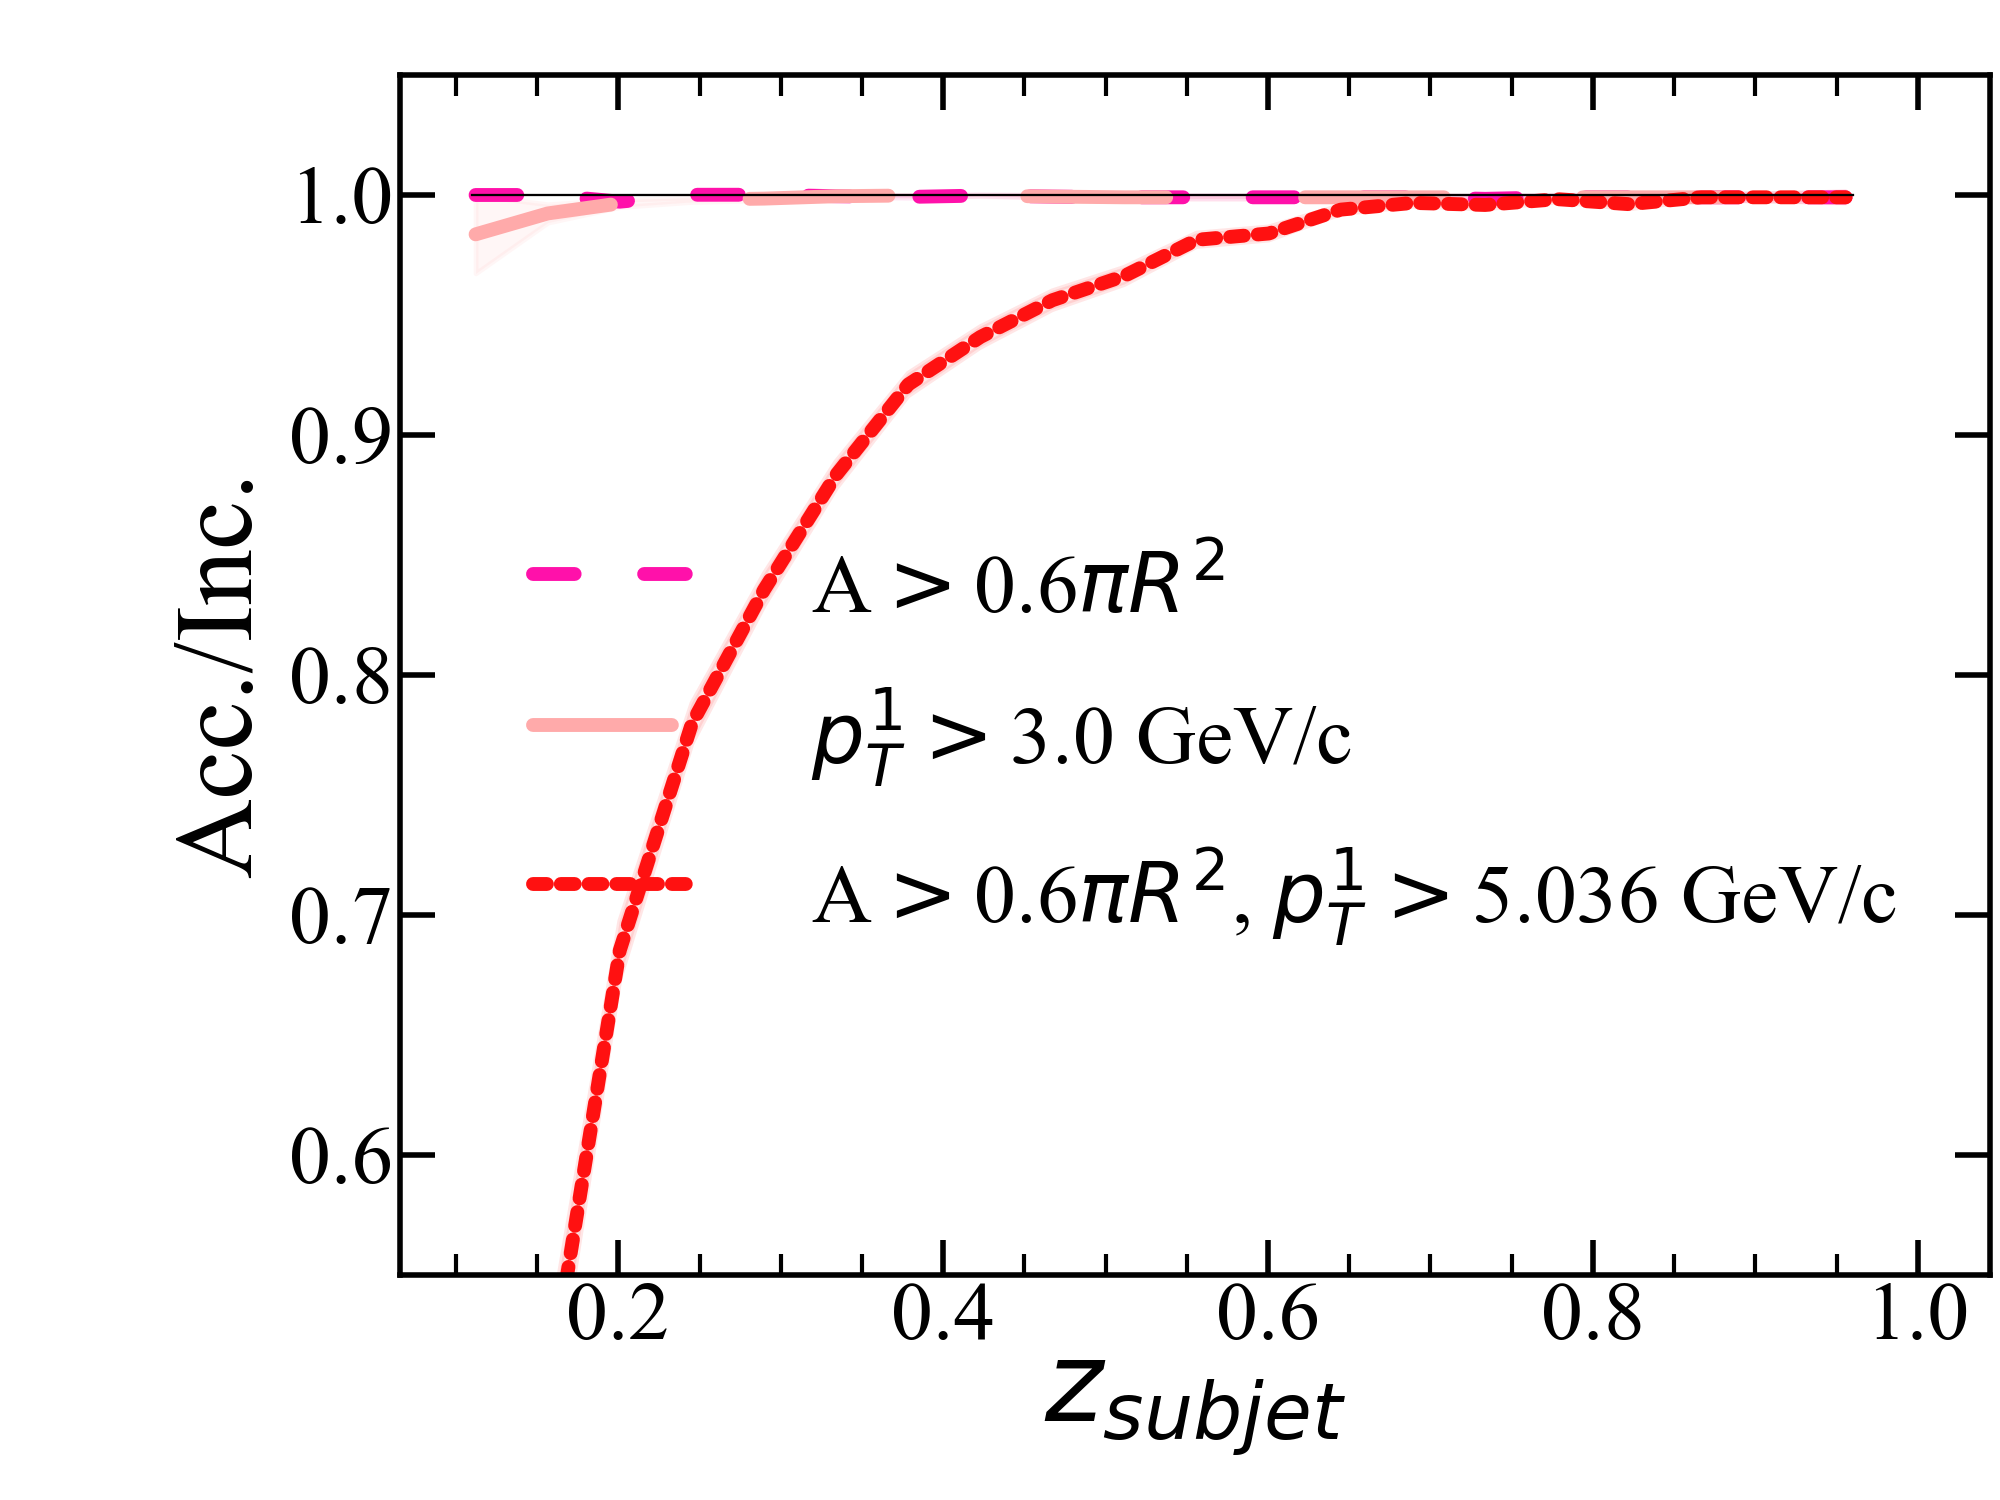}
    \caption{R=0.5 \ptH=30 \GeV}
    \label{fig:z_sub_05_30}
\end{figure*}

\begin{figure*}
    \centering
    \includegraphics[width=\linewidth]{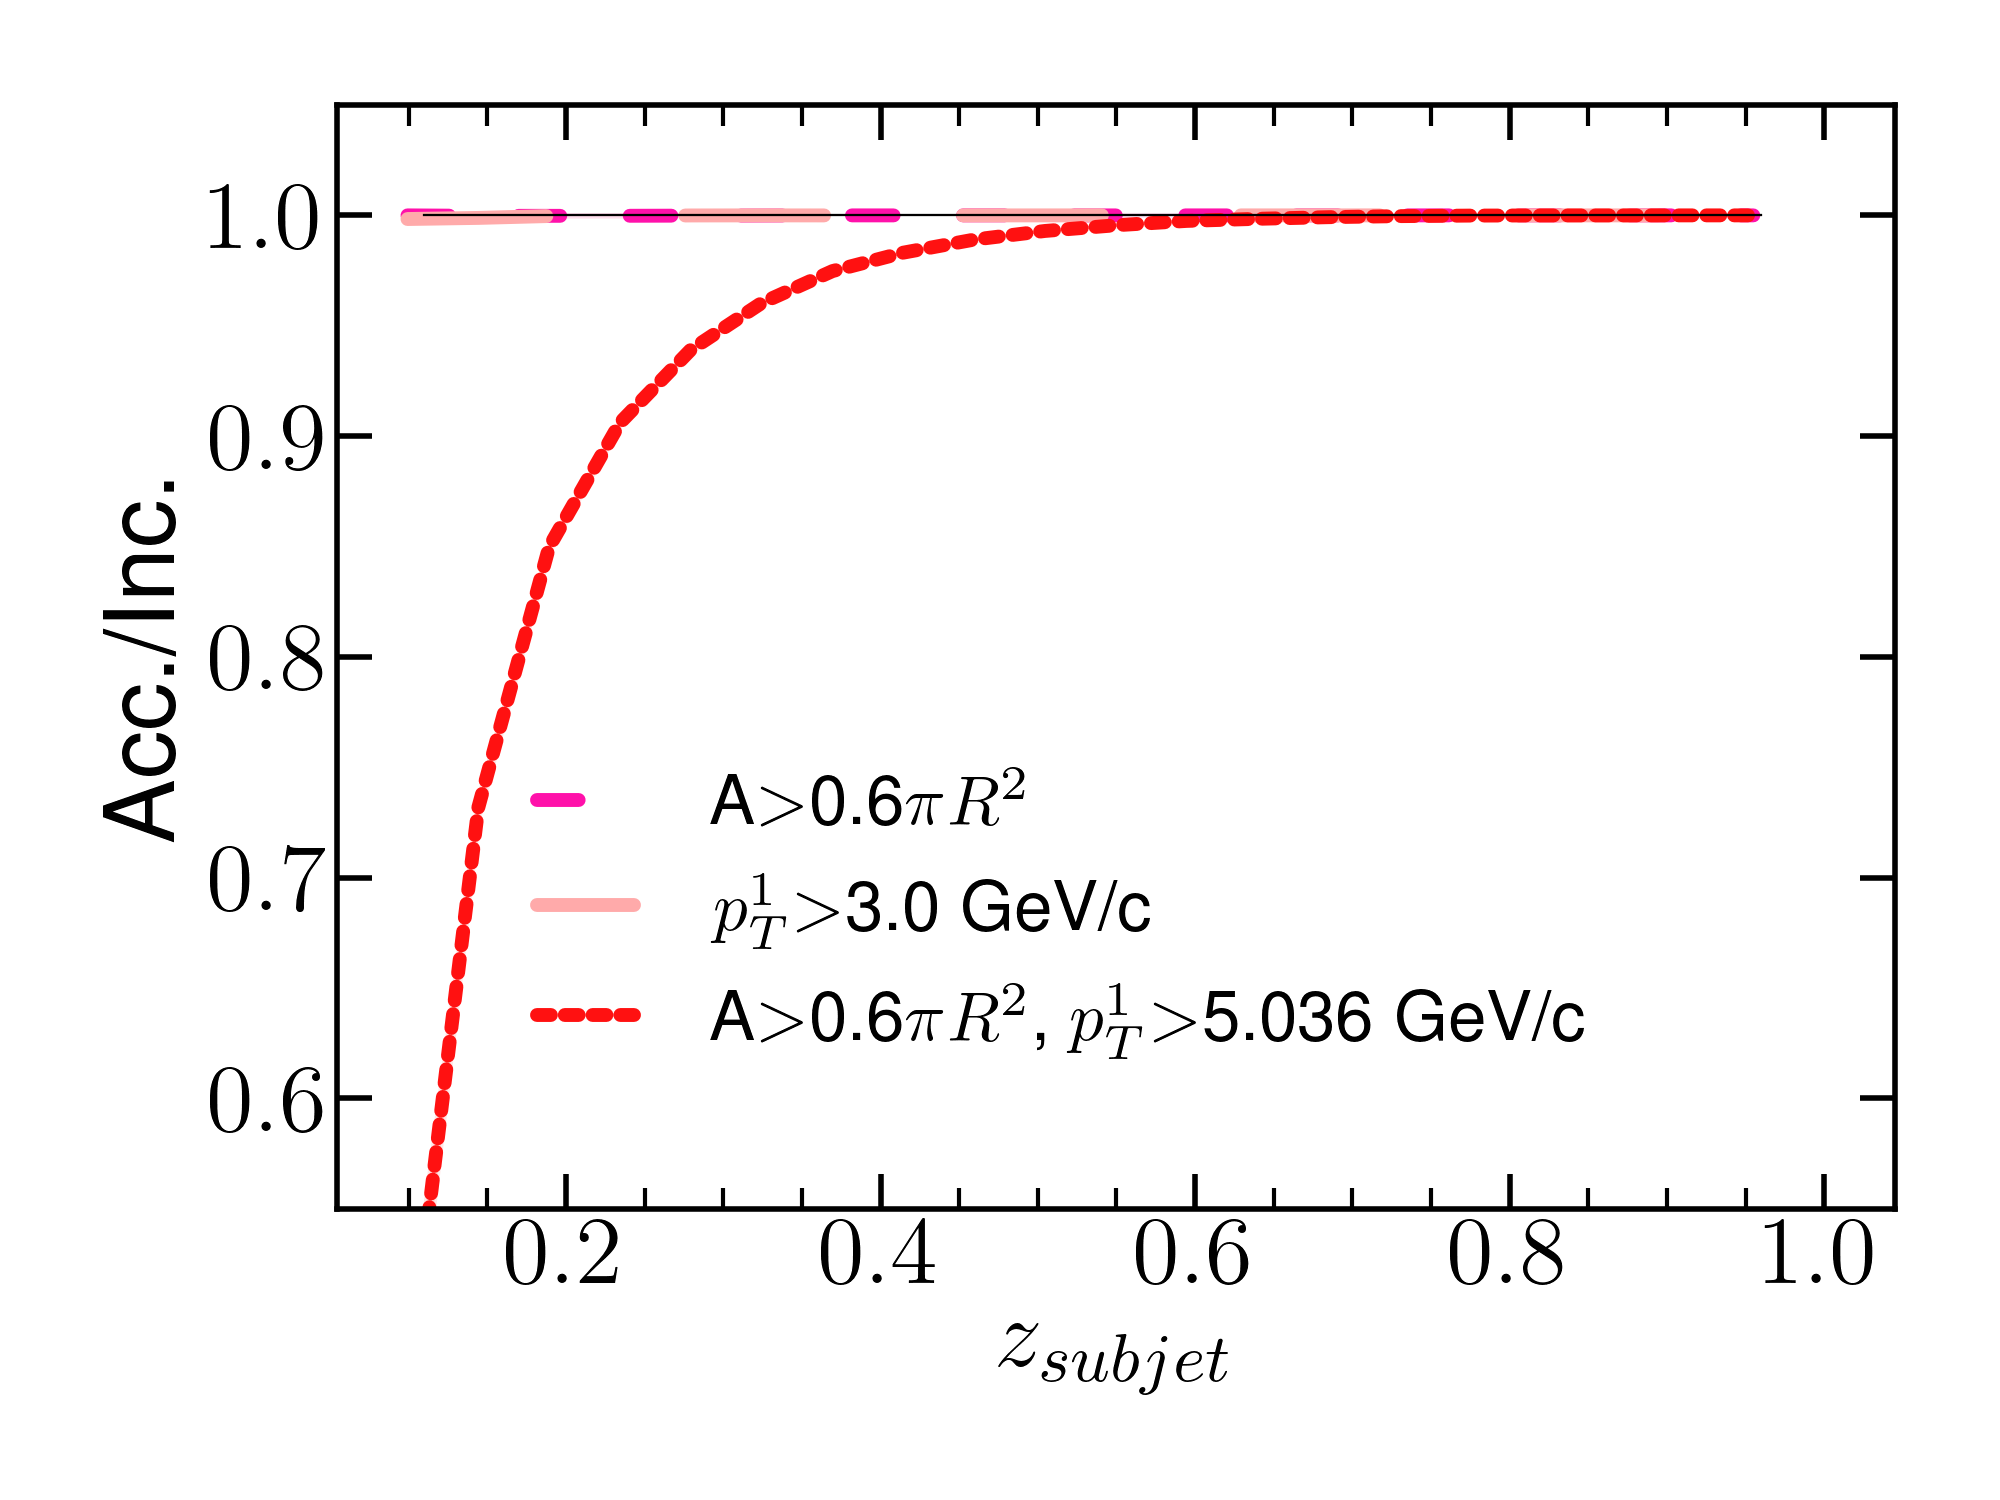}
    \caption{R=0.5 \ptH=40 \GeV}
    \label{fig:z_sub_05_40}
\end{figure*}

\begin{figure*}
    \centering
    \includegraphics[width=\linewidth]{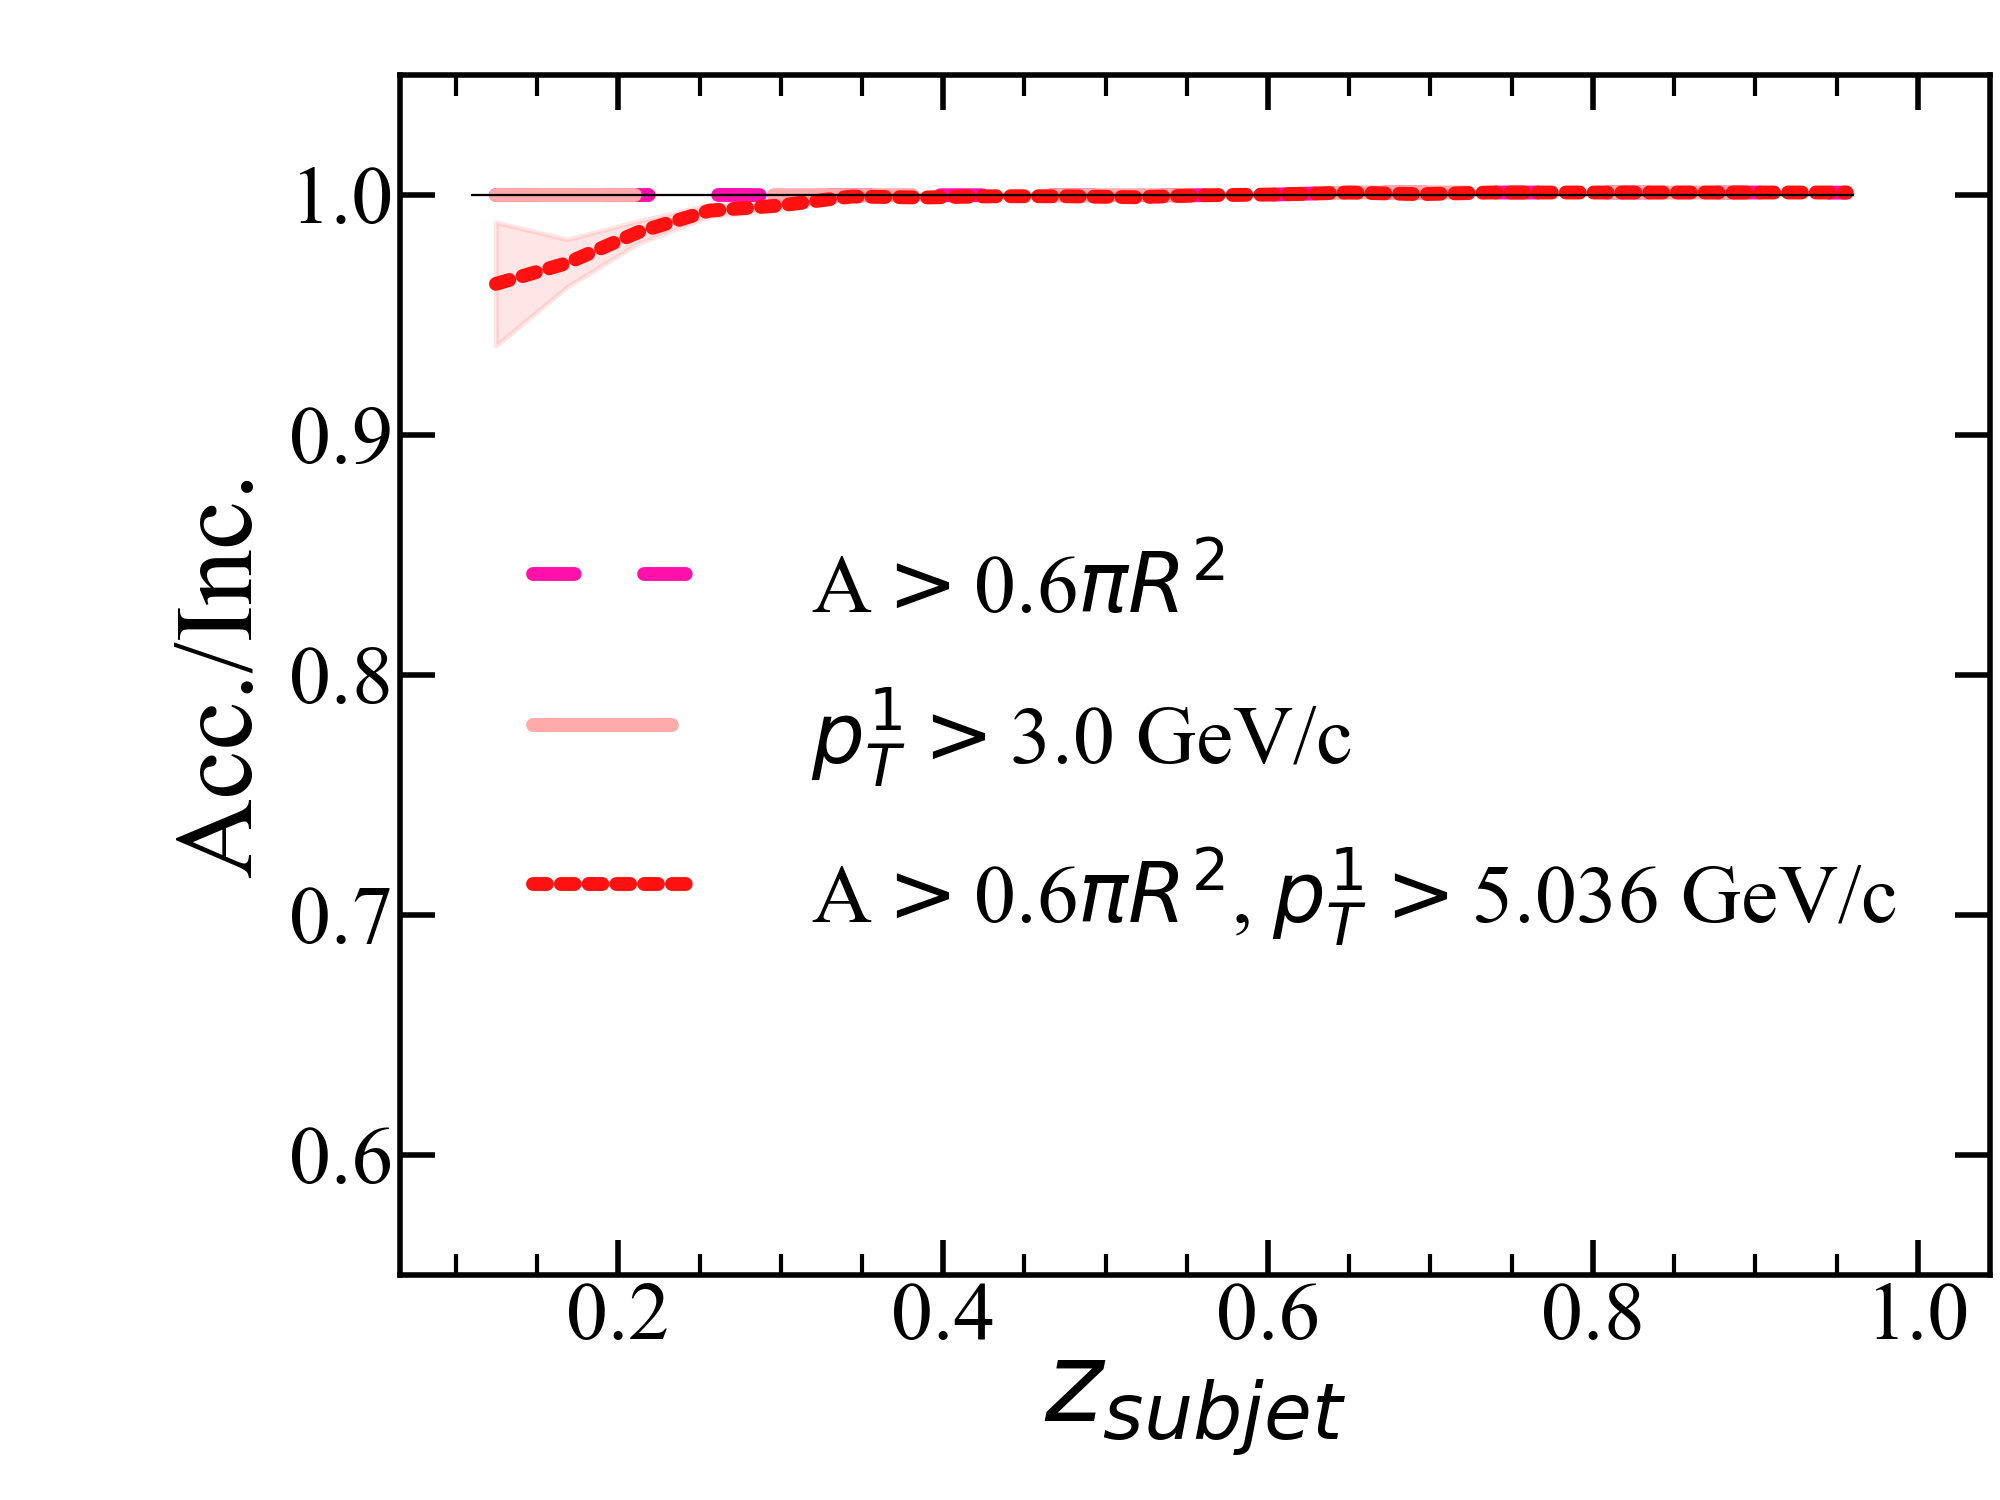}
    \caption{R=0.5 \ptH=60 \GeV}
    \label{fig:z_sub_05_60}
\end{figure*}

\begin{figure*}
    \centering
    \includegraphics[width=\linewidth]{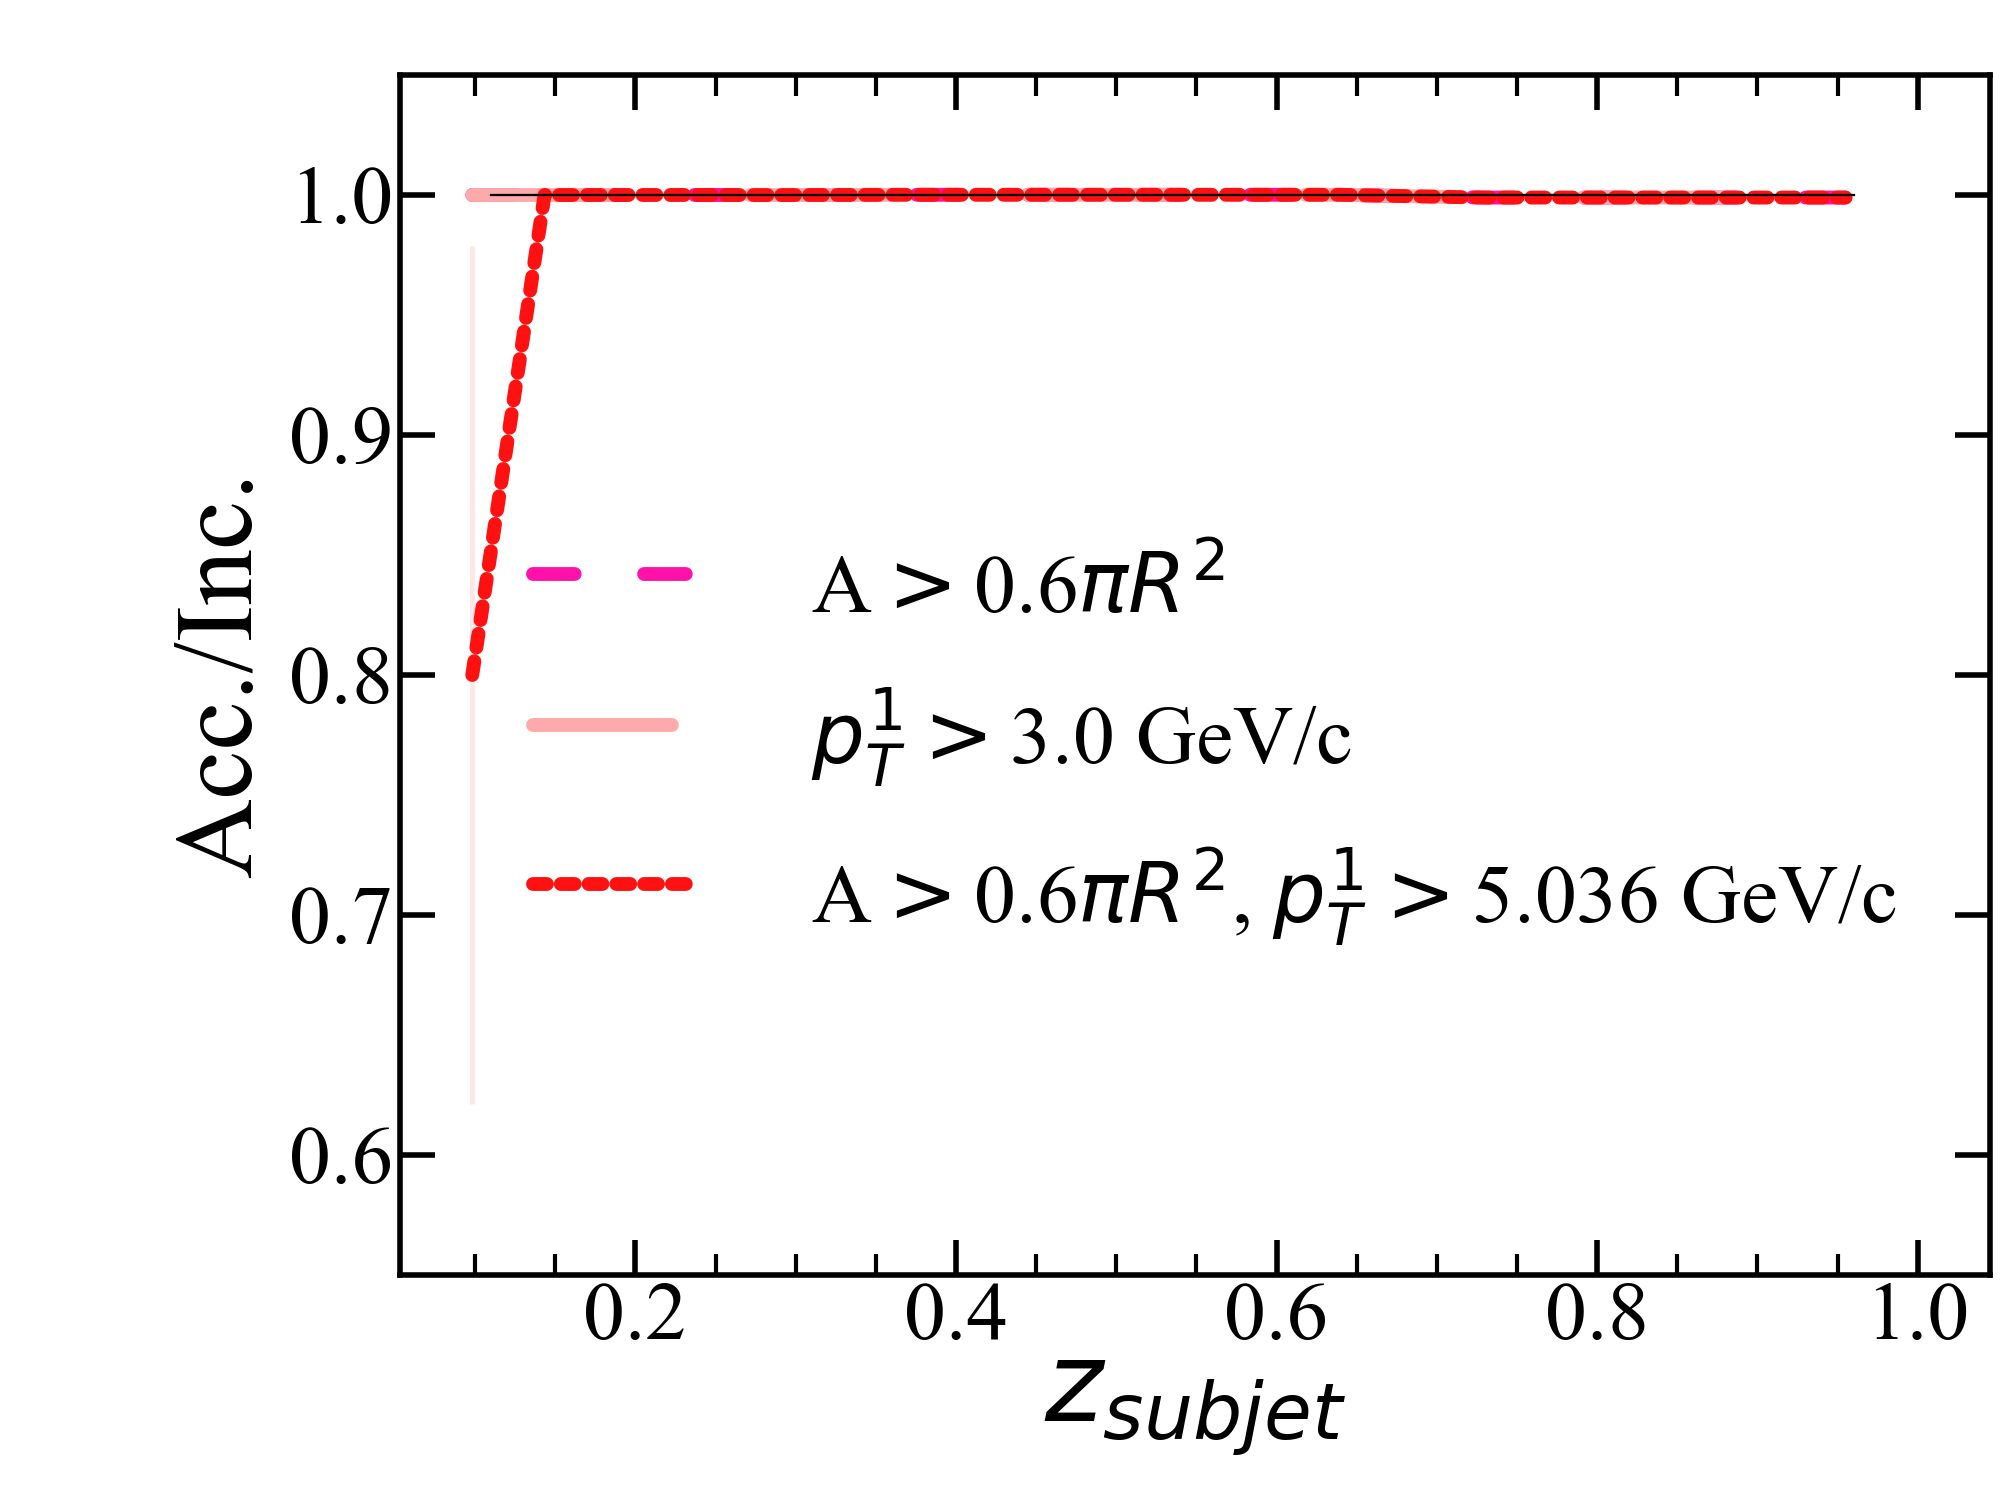}
    \caption{R=0.5 \ptH=80 \GeV}
    \label{fig:z_sub_05_80}
\end{figure*}

\begin{figure*}
    \centering
    \includegraphics[width=\linewidth]{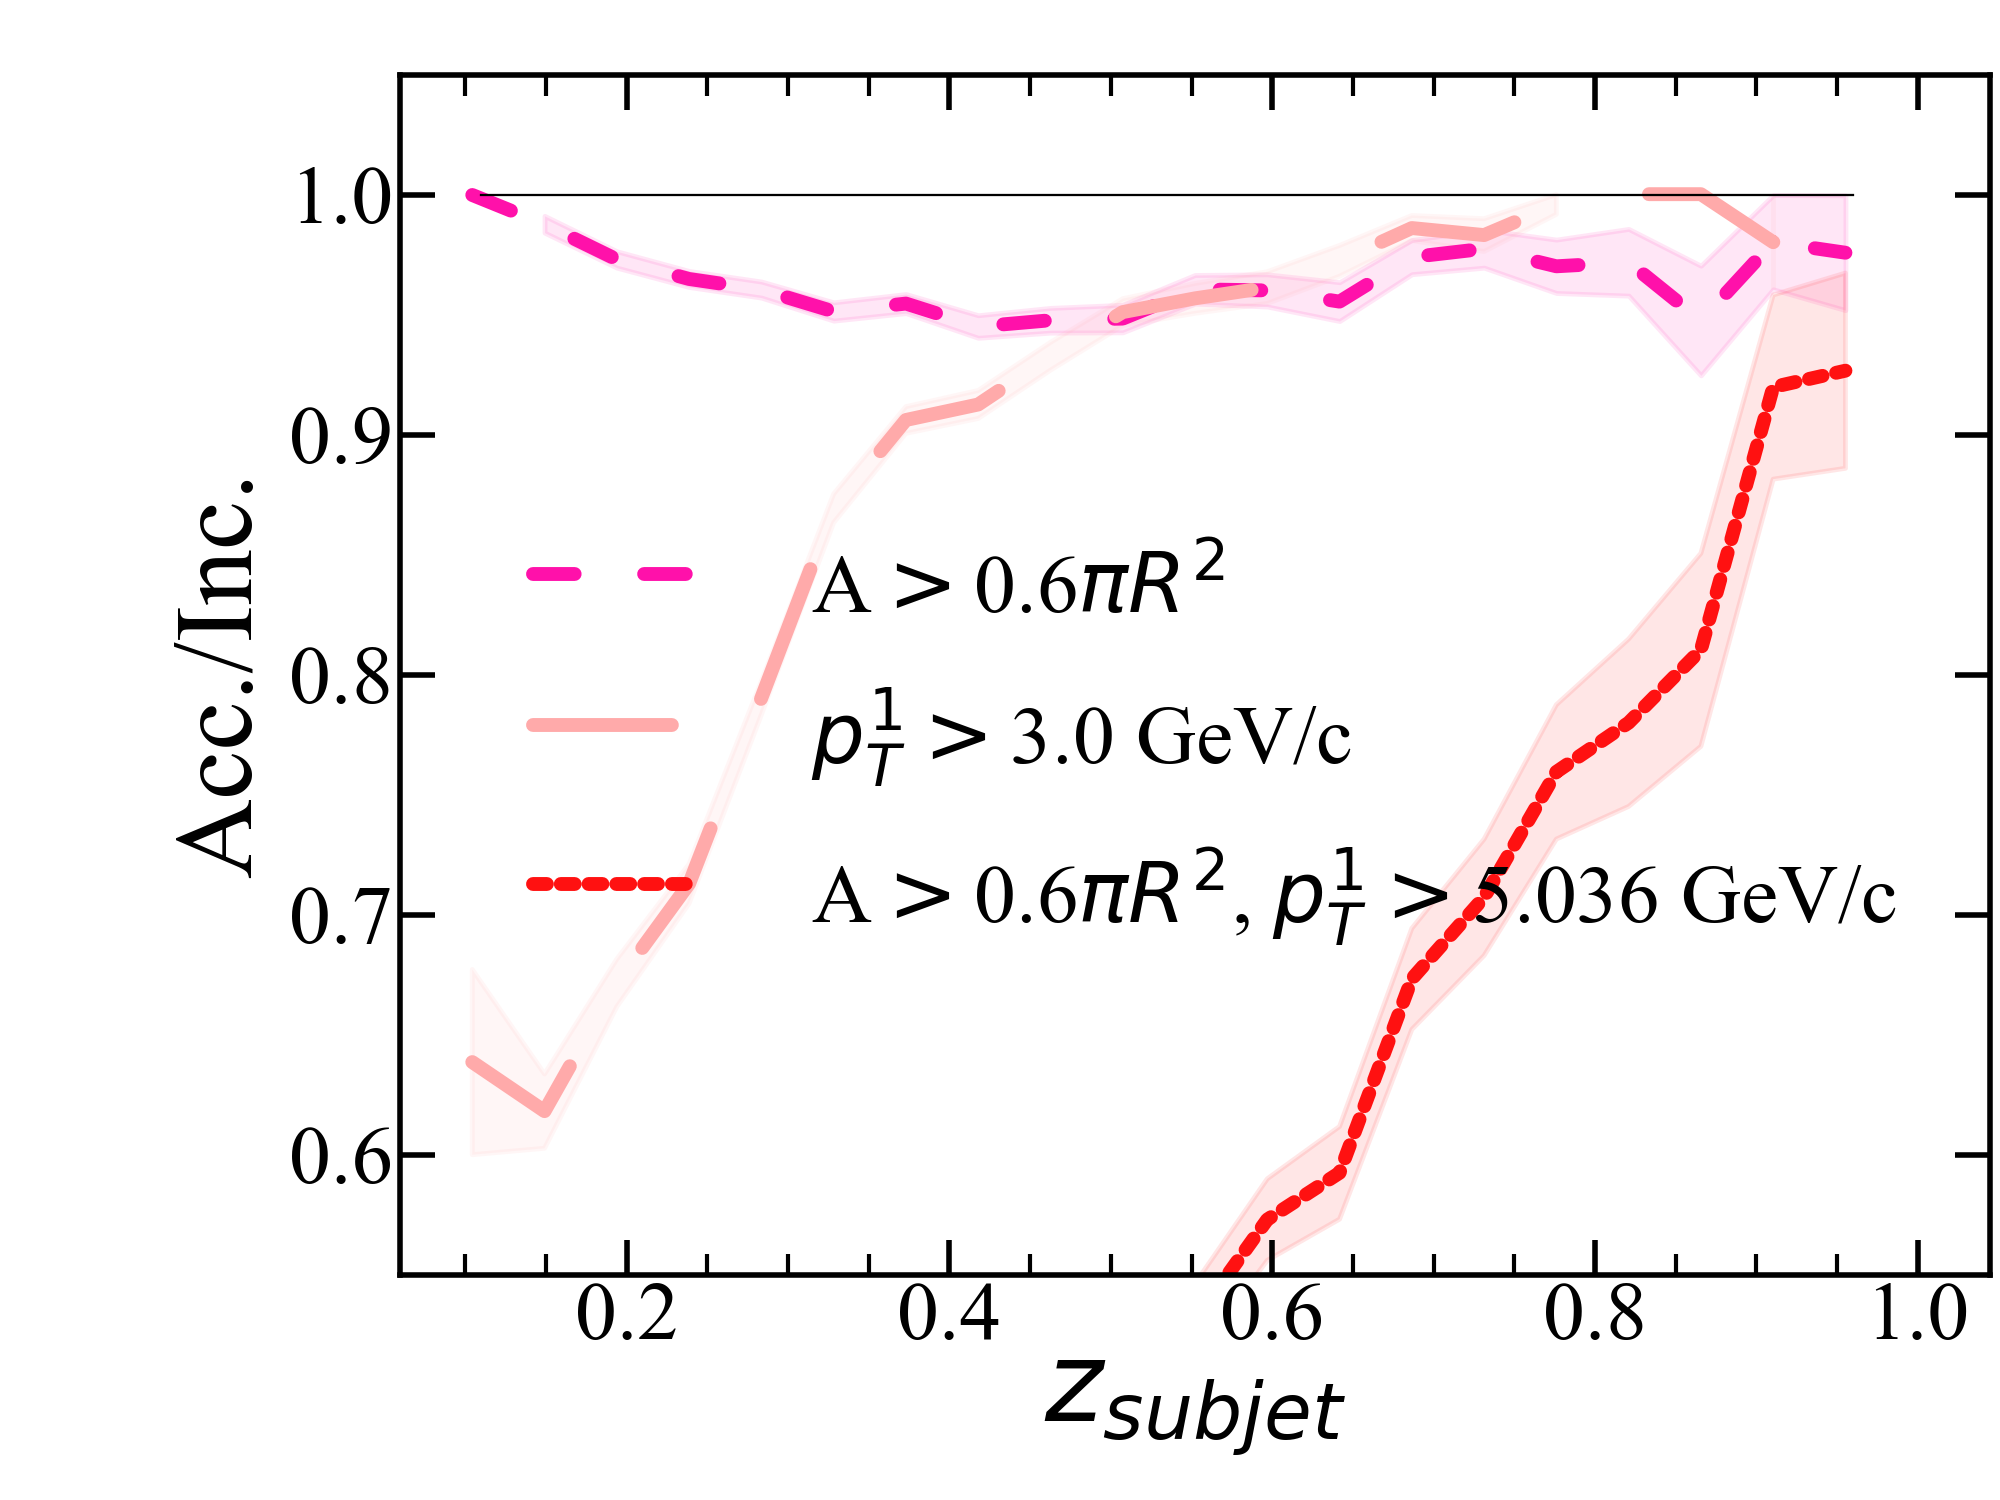}
    \caption{R=0.6 \ptH=10 \GeV}
    \label{fig:z_sub_06_10}
\end{figure*}

\begin{figure*}
    \centering
    \includegraphics[width=\linewidth]{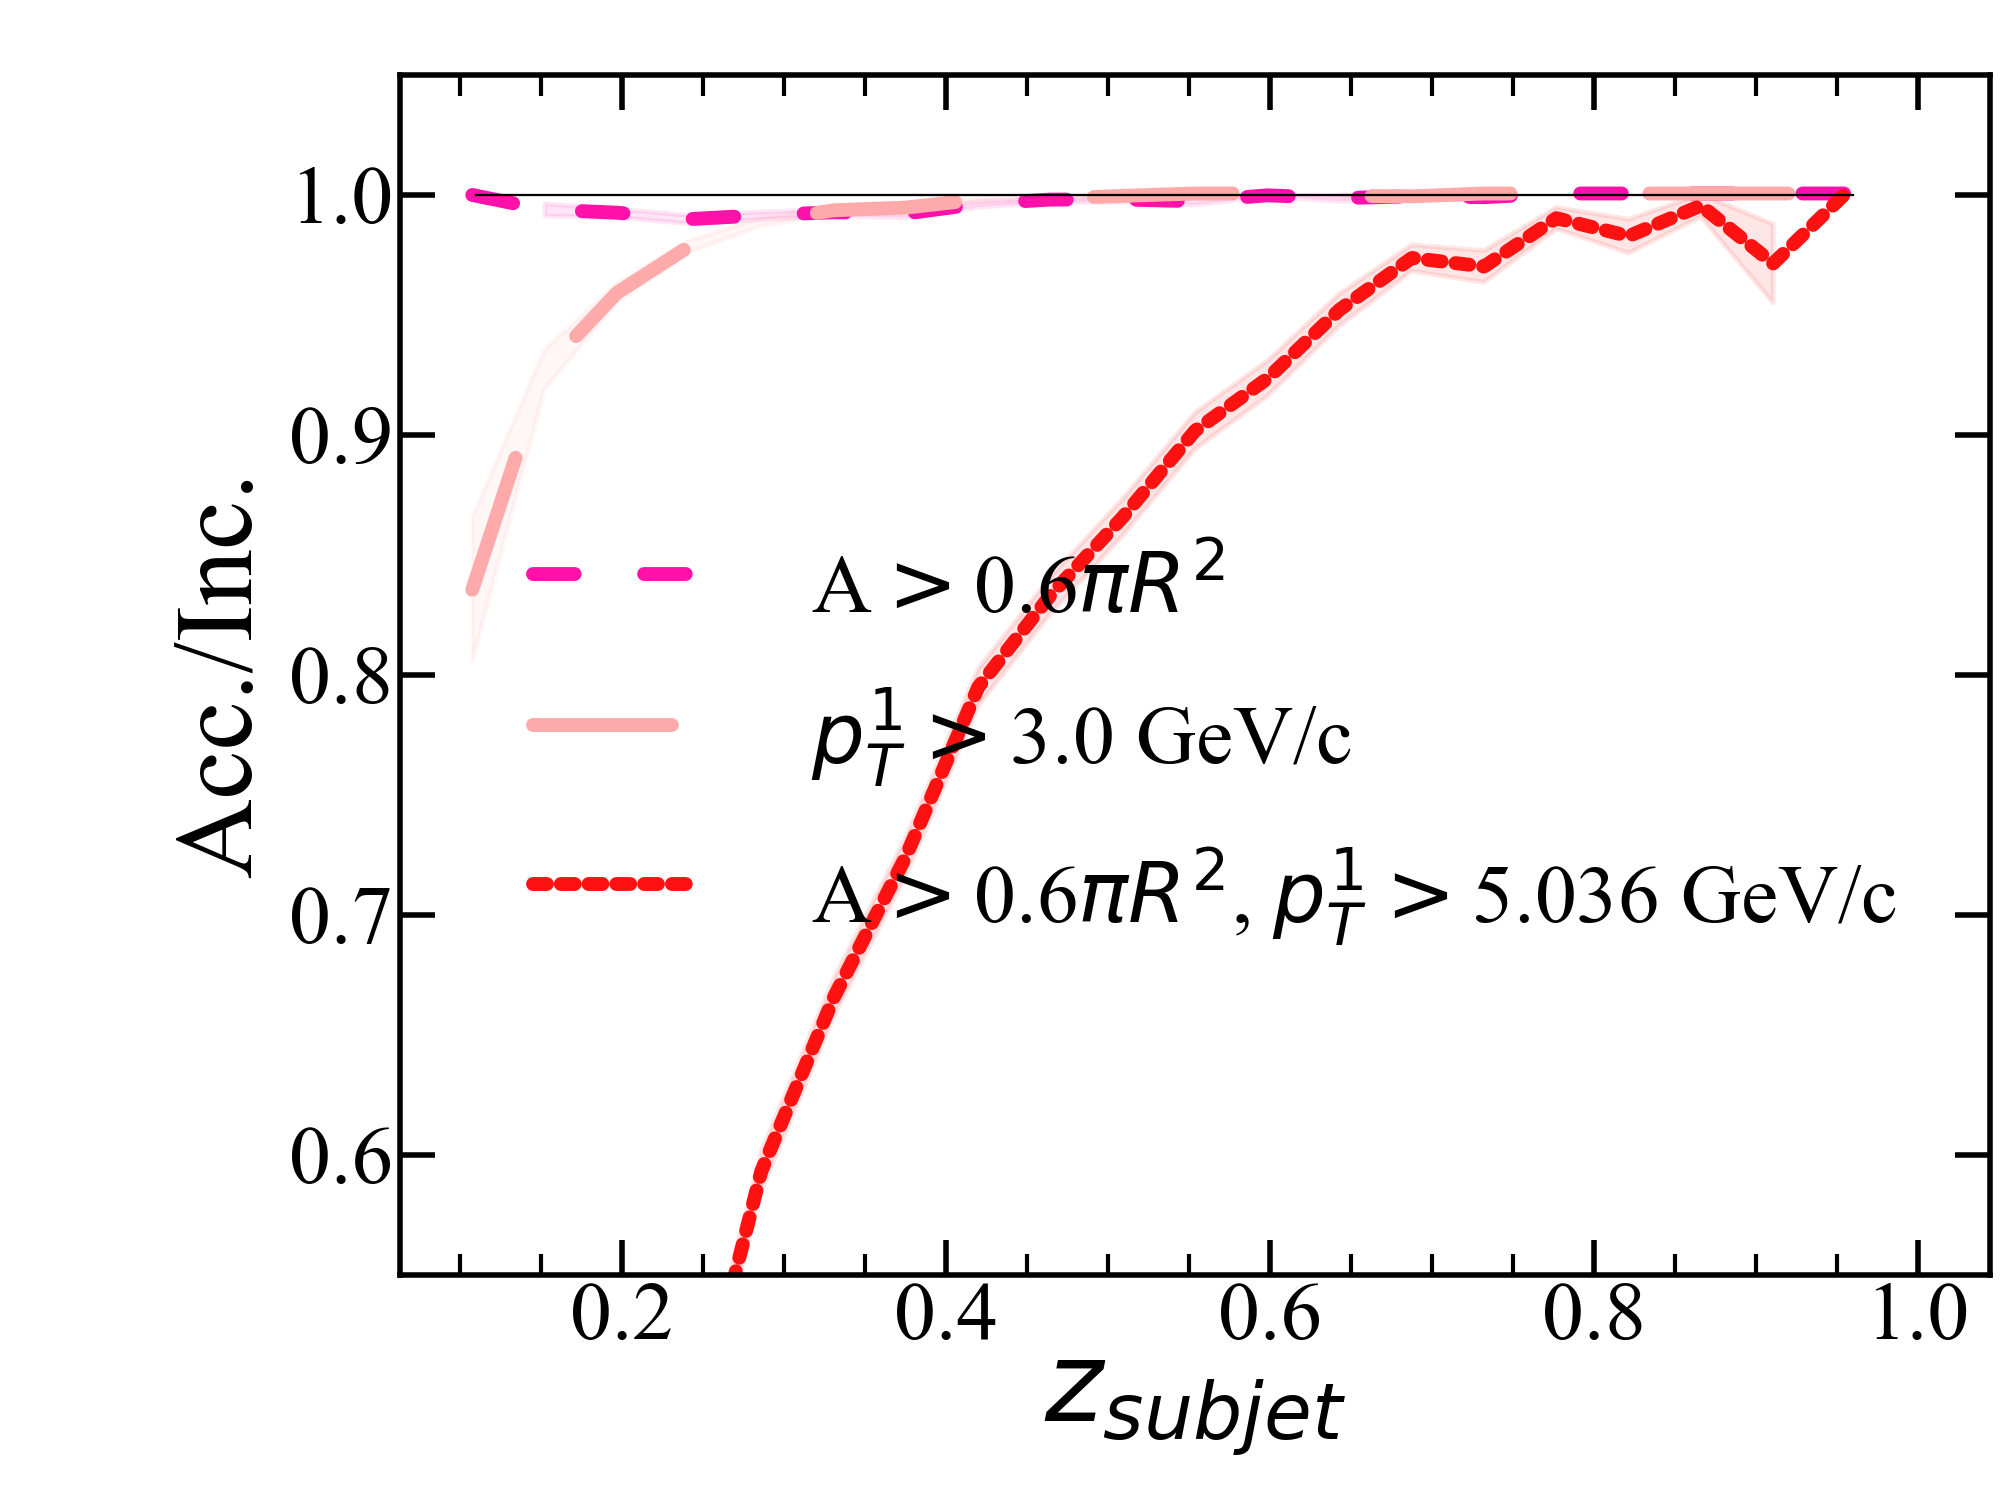}
    \caption{R=0.6 \ptH=20 \GeV}
    \label{fig:z_sub_06_20}
\end{figure*}

\begin{figure*}
    \centering
    \includegraphics[width=\linewidth]{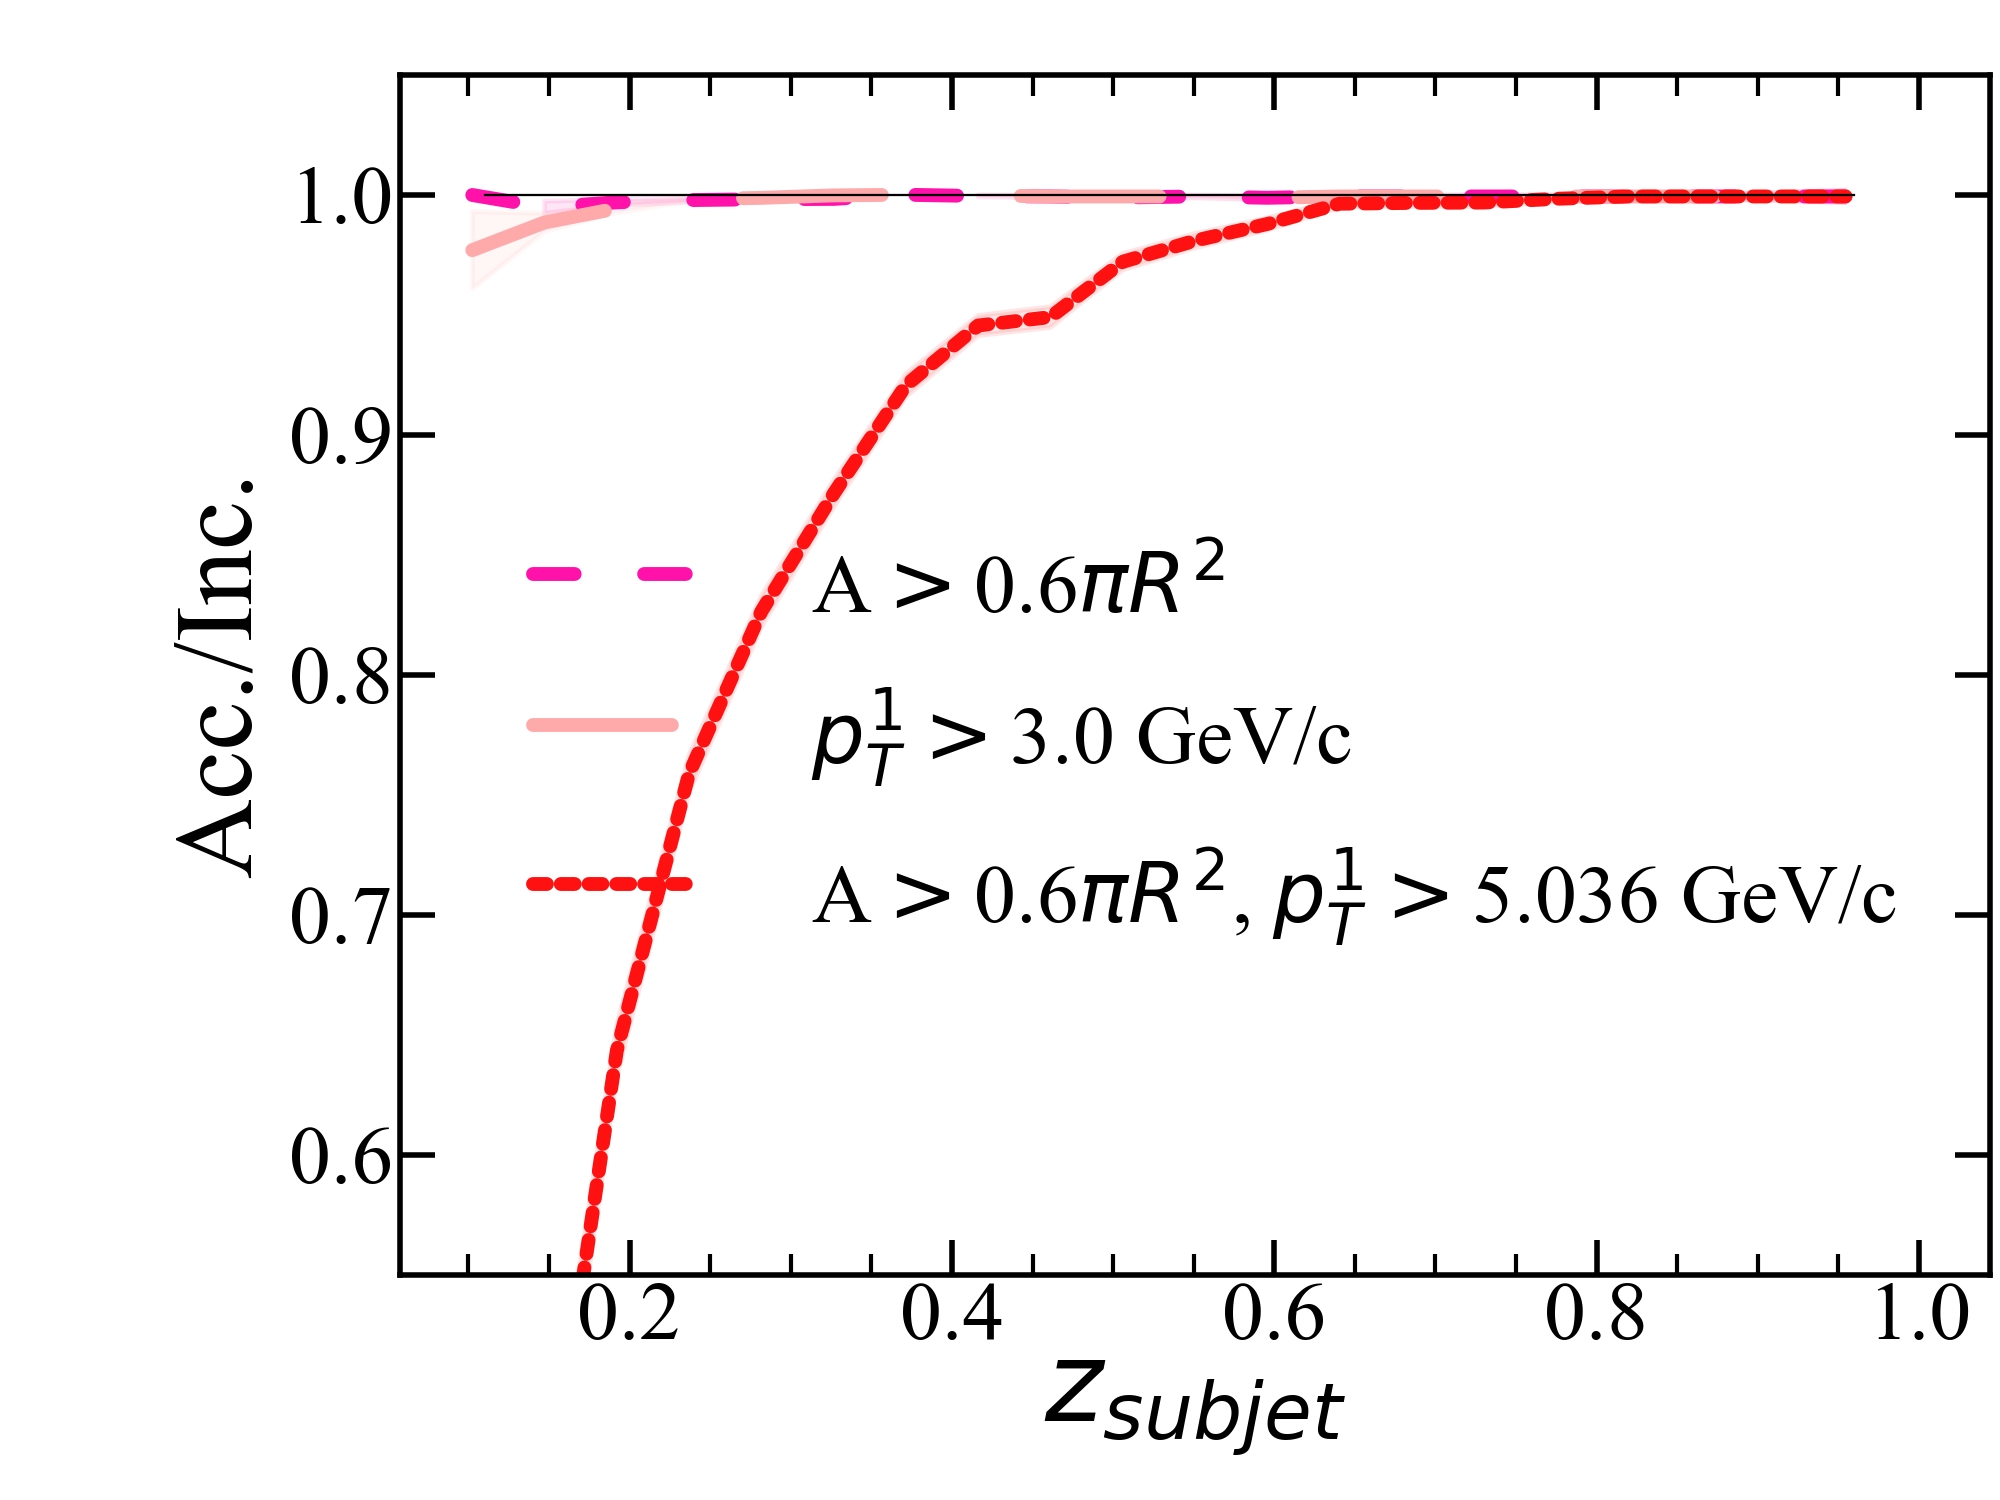}
    \caption{R=0.6 \ptH=30 \GeV}
    \label{fig:z_sub_06_30}
\end{figure*}

\begin{figure*}
    \centering
    \includegraphics[width=\linewidth]{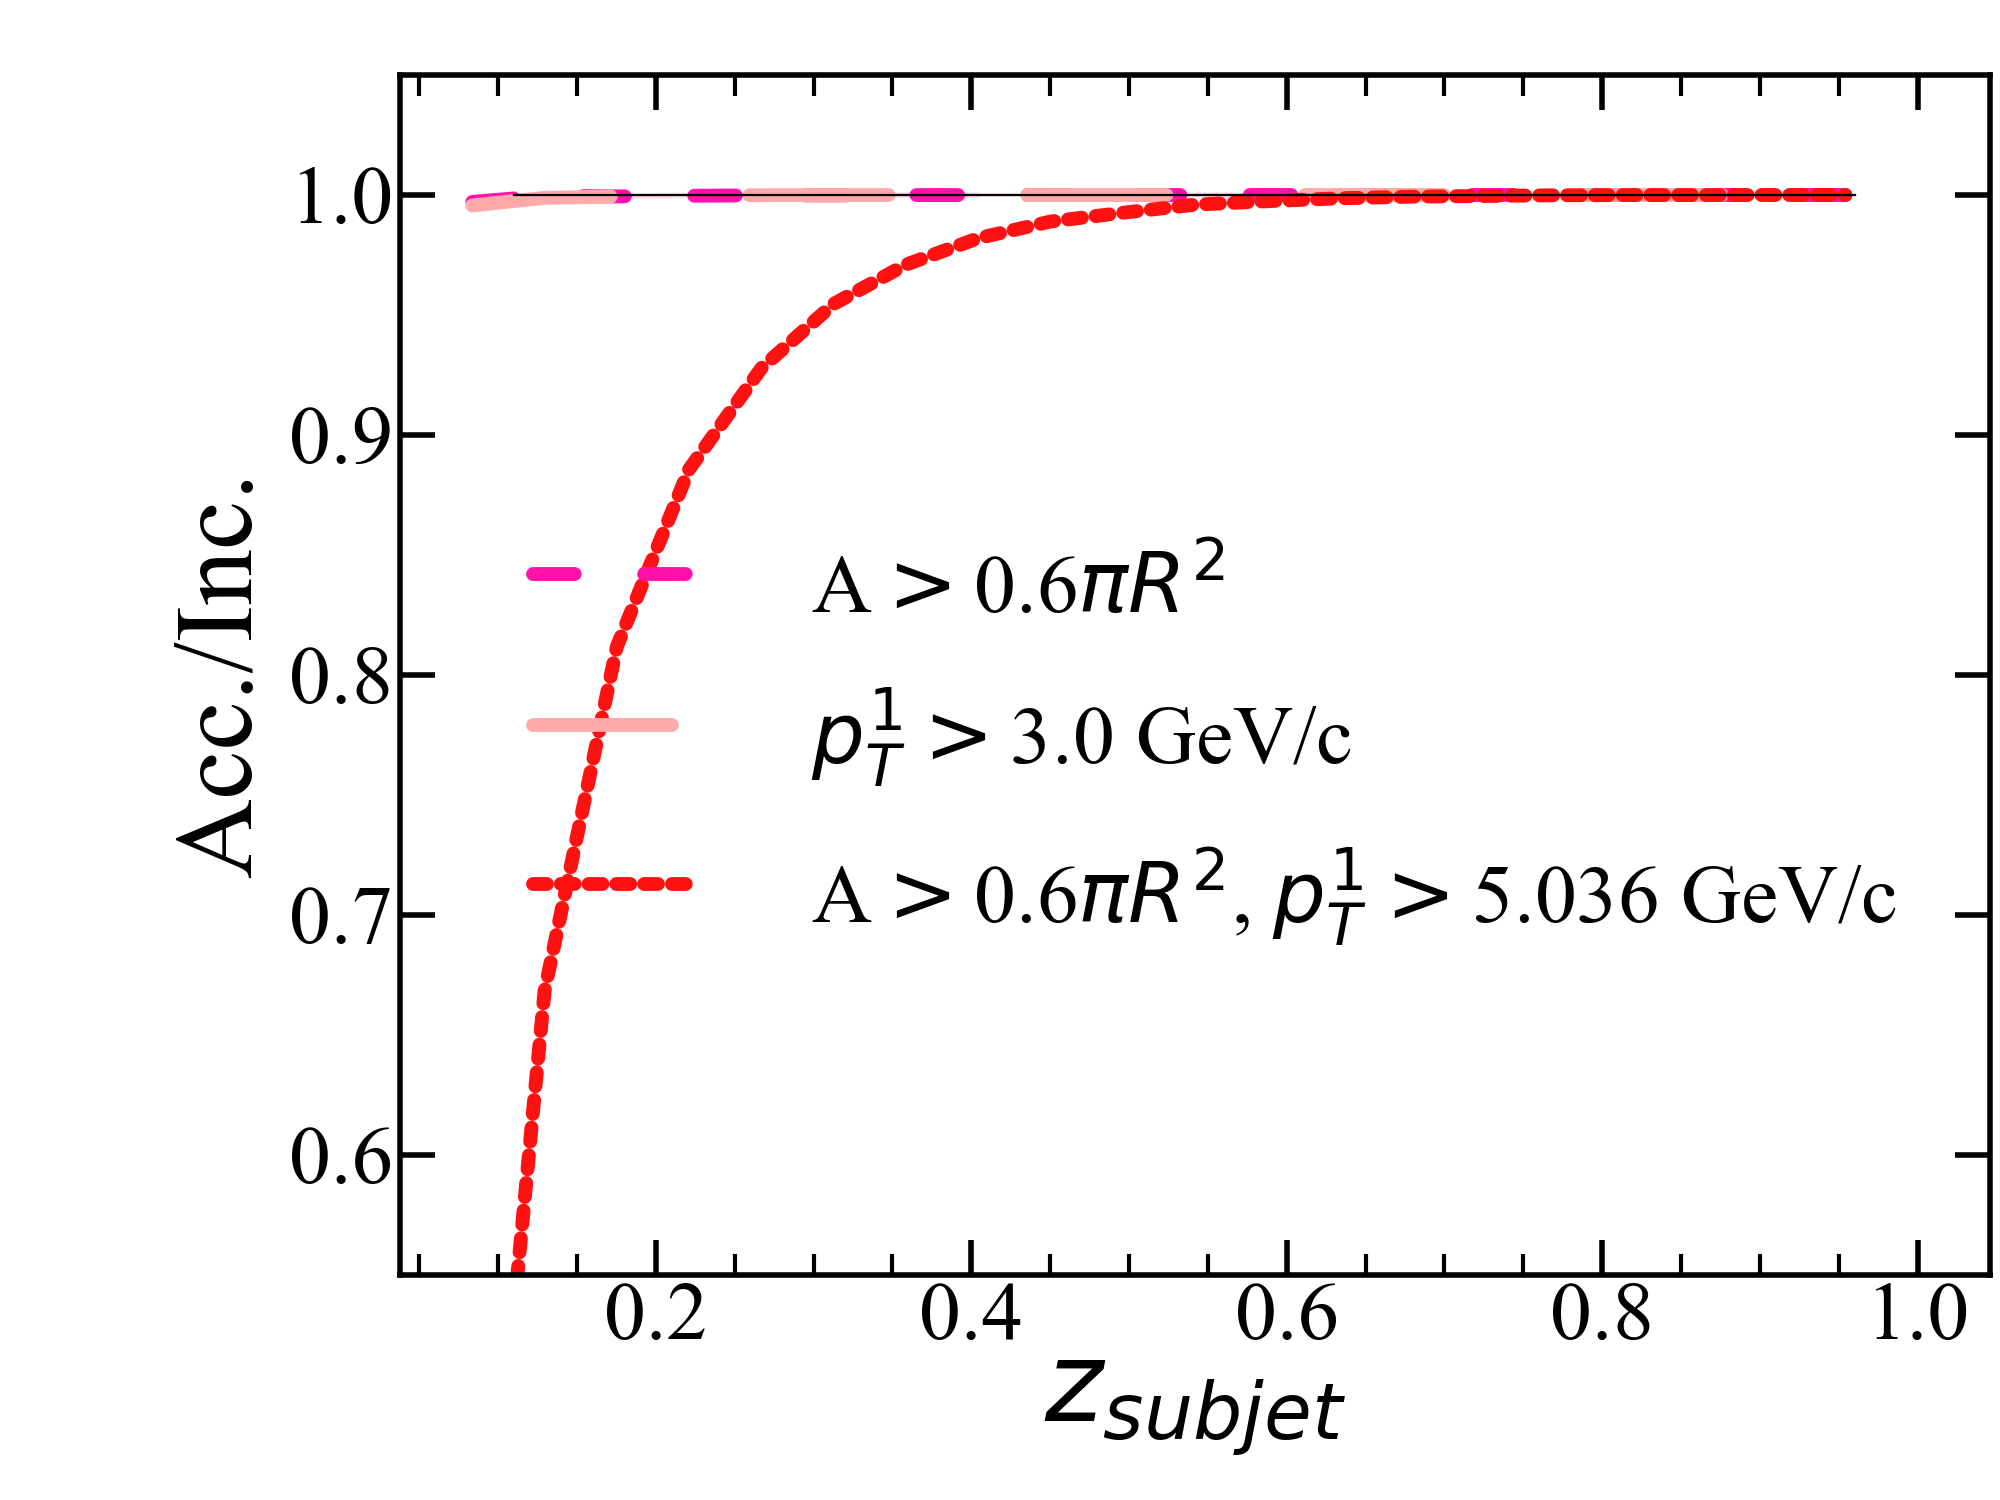}
    \caption{R=0.6 \ptH=40 \GeV}
    \label{fig:z_sub_06_40}
\end{figure*}

\begin{figure*}
    \centering
    \includegraphics[width=\linewidth]{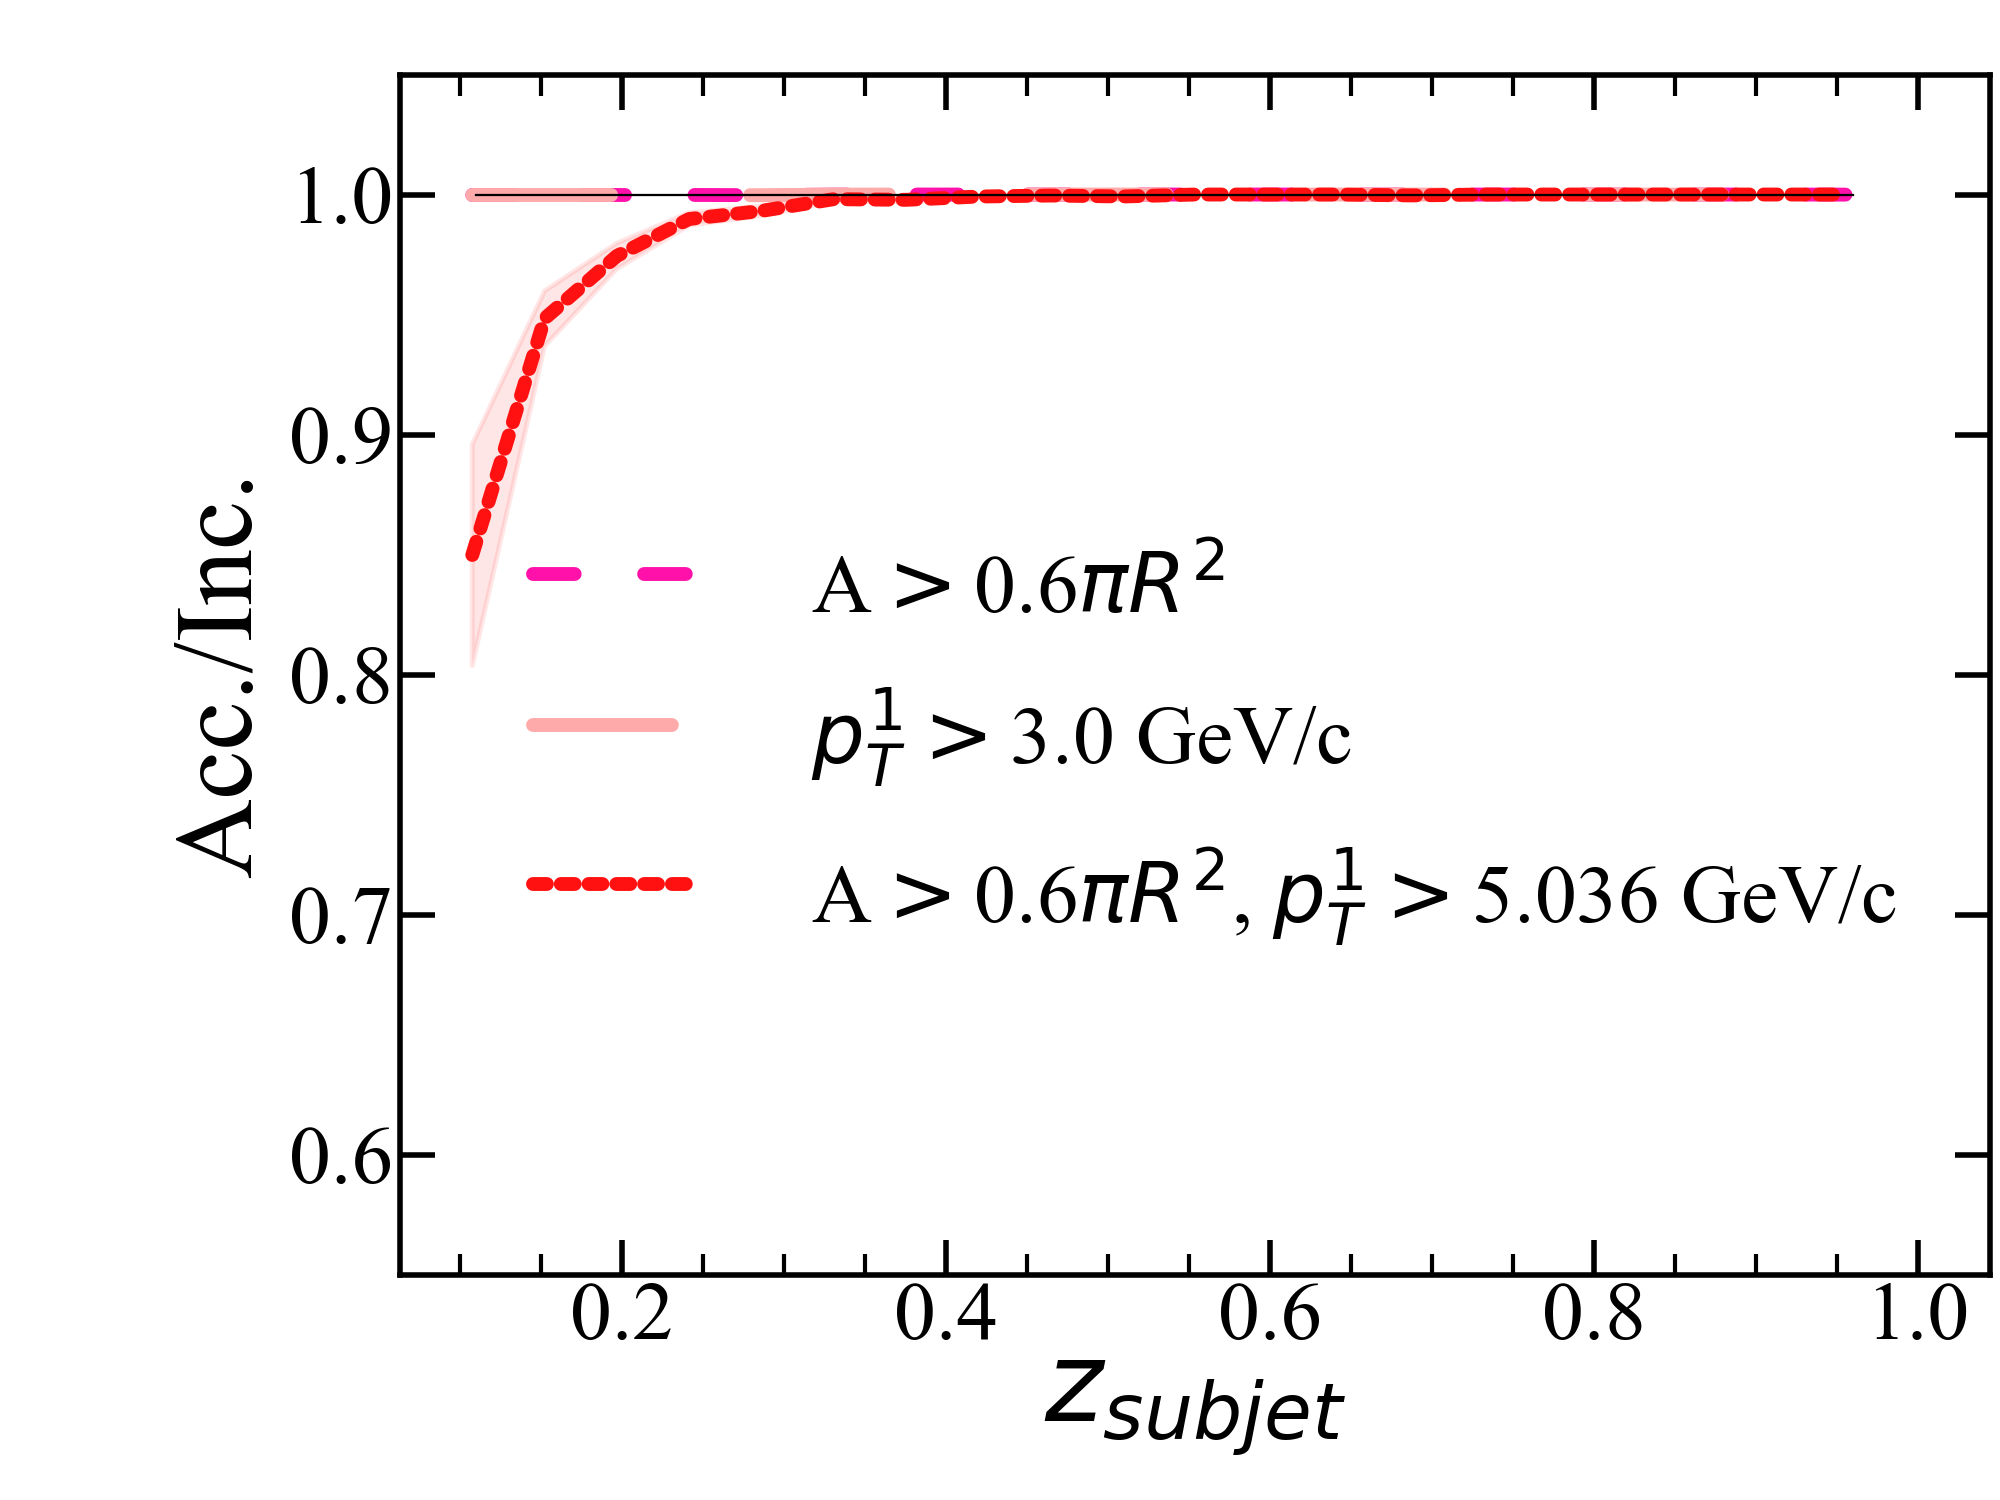}
    \caption{R=0.6 \ptH=60 \GeV}
    \label{fig:z_sub_06_60}
\end{figure*}

\begin{figure*}
    \centering
    \includegraphics[width=\linewidth]{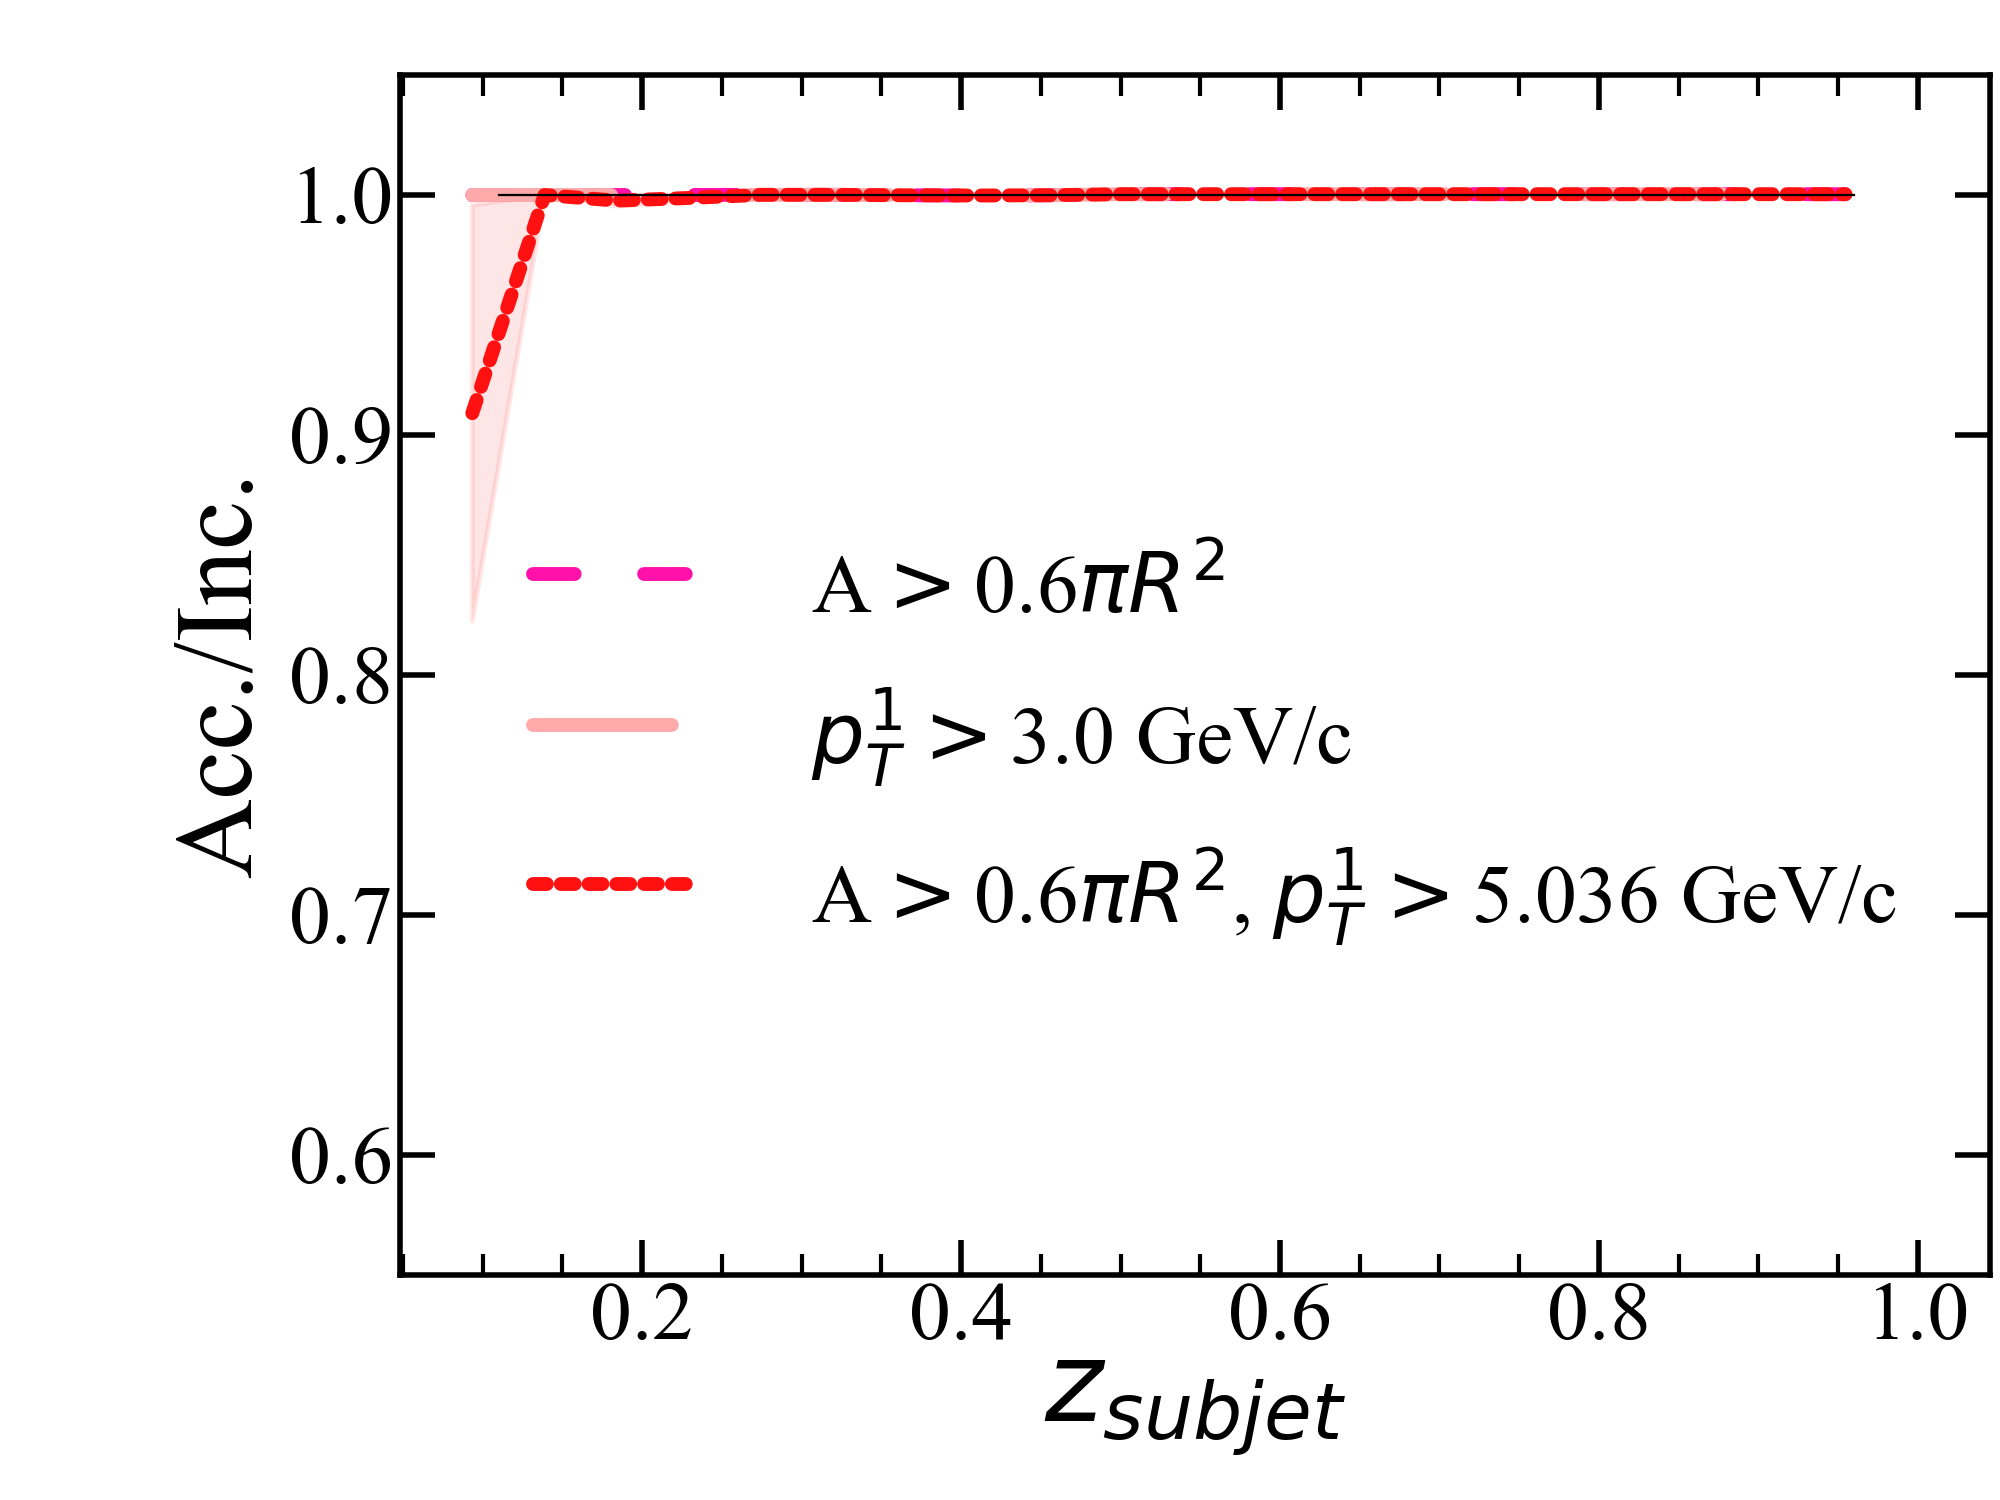}
    \caption{R=0.6 \ptH=80 \GeV}
    \label{fig:z_sub_06_80}
\end{figure*}
